# Supplementary material for: ProofOptimizer: Training Language Models to Simplify Proofs without Human Demonstrations
Source: arXiv:2510.15700 ancillary file (2025-10-17)
Supplement: Supplementary file 1 [file full_paper.pdf]

# ProofOptimizer: Training Language Models to Simplify Proofs without Human Demonstrations

**Alex Gu**

*Meta FAIR & MIT CSAIL*

*gua@mit.edu*

**Bartosz Piotrowski**

*Meta FAIR*

*bpio@meta.com*

**Fabian Gloeckle**

*Meta FAIR & École des Ponts Paris*

*fgloeckle@meta.com*

**Kaiyu Yang**

*Meta FAIR*

*kaiyuy@meta.com*

**Aram H. Markosyan**

*Meta FAIR*

*aram.math@gmail.com*

## Abstract

Neural theorem proving has advanced rapidly in the past year, reaching IMO gold-medalist capabilities and producing formal proofs that span thousands of lines. Although such proofs are mechanically verified by formal systems like Lean, their excessive length renders them difficult for humans to comprehend and limits their usefulness for mathematical insight. Proof simplification is therefore a critical bottleneck. Yet, training data for this task is scarce, and existing methods—mainly agentic scaffolding with off-the-shelf LLMs—struggle with the extremely long proofs generated by RL-trained provers. We introduce *ProofOptimizer*, the first language model trained to simplify Lean proofs without requiring additional human supervision. ProofOptimizer is trained via expert iteration and reinforcement learning, using Lean to verify simplifications and provide training signal. At inference time, it operates within an iterative proof-shortening workflow, progressively reducing proof length. Experiments show that ProofOptimizer substantially compresses proofs generated by state-of-the-art RL-trained provers on standard benchmarks, reducing proof length by 87% on miniF2F, 57% on PutnamBench, and 49% on Seed-Prover’s IMO 2025 proofs. Beyond conciseness, the simplified proofs check faster in Lean and further improve downstream prover performance when reused as training data for supervised finetuning.

# Contents

|          |                                                                         |           |
|----------|-------------------------------------------------------------------------|-----------|
| <b>1</b> | <b>Introduction</b>                                                     | <b>4</b>  |
| <b>2</b> | <b>Proof Simplification: Task and Metrics</b>                           | <b>5</b>  |
| <b>3</b> | <b>ProofOptimizer: LLMs for Proof Simplification</b>                    | <b>6</b>  |
| 3.1      | Training . . . . .                                                      | 6         |
| 3.1.1    | ProofOptimizer-ExpIt: Expert Iteration . . . . .                        | 7         |
| 3.1.2    | ProofOptimizer-RL: Online Reinforcement Learning . . . . .              | 7         |
| 3.2      | Inference-Time Techniques . . . . .                                     | 7         |
| <b>4</b> | <b>Experiments</b>                                                      | <b>8</b>  |
| 4.1      | Expert Iteration vs. RL vs. Test-Time RL . . . . .                      | 8         |
| 4.2      | Analysis of Repair with Execution Feedback . . . . .                    | 9         |
| 4.3      | Iterative Proof Shortening . . . . .                                    | 10        |
| <b>5</b> | <b>Additional Benefits of Proof Simplification</b>                      | <b>11</b> |
| 5.1      | Training on Simplified Proofs Improves Generation . . . . .             | 11        |
| 5.2      | Simplified Proofs Have a Shorter Execution Time . . . . .               | 12        |
| 5.2.1    | Optimizing for Heartbeats instead of Proof Length . . . . .             | 13        |
| <b>6</b> | <b>Related Works</b>                                                    | <b>13</b> |
| <b>7</b> | <b>Conclusion</b>                                                       | <b>14</b> |
| <b>8</b> | <b>Acknowledgments</b>                                                  | <b>14</b> |
| <b>A</b> | <b>Lean Base Model and Proof Simplification Data Details</b>            | <b>20</b> |
| A.1      | General Base Model for Lean . . . . .                                   | 20        |
| A.2      | Generating a Dataset of Theorems and Proofs for Shortening . . . . .    | 20        |
| A.3      | Statistics of Proof Simplification Training Dataset . . . . .           | 23        |
| <b>B</b> | <b>Training Metrics throughout RL</b>                                   | <b>26</b> |
| <b>C</b> | <b>Full Results and Extended Analysis of Iterative Proof Shortening</b> | <b>27</b> |

|          |                                                                                              |           |
|----------|----------------------------------------------------------------------------------------------|-----------|
| C.1      | Table of Iterative Proof Shortening Results . . . . .                                        | 27        |
| C.2      | Effect of $k$ on $\text{min}@k$ and $\text{red}@k$ throughout simplification . . . . .       | 27        |
| C.3      | Details on Seed-Prover IMO Proof Shortening . . . . .                                        | 28        |
| <b>D</b> | <b>Comparison with Qwen2.5, GPT-4o, and Gemini-2.5-Pro</b>                                   | <b>30</b> |
| <b>E</b> | <b>Full Results and Extended Analysis of Repair with Execution Feedback</b>                  | <b>32</b> |
| <b>F</b> | <b>Evaluation Dataset Details</b>                                                            | <b>35</b> |
| <b>G</b> | <b>Examples of Proofs Simplified by ProofOptimizer</b>                                       | <b>37</b> |
| <b>H</b> | <b>Proof Speedup and Slowdown Analysis and Examples</b>                                      | <b>42</b> |
| H.1      | Iterative Proof Shortening Results with Heartbeat Metric . . . . .                           | 42        |
| H.2      | Examples of Proof Speedup and Slowdown after Simplification . . . . .                        | 43        |
| <b>I</b> | <b>Derivation of Closed Form for <math>\text{min}@k</math> and <math>\text{max}@k</math></b> | <b>47</b> |
| <b>J</b> | <b>Hyperparameters</b>                                                                       | <b>48</b> |
| <b>K</b> | <b>Prompts</b>                                                                               | <b>49</b> |
| K.1      | Proof Simplification Prompt . . . . .                                                        | 49        |
| K.2      | Proof Sketching Prompts . . . . .                                                            | 49        |
| K.3      | Goedel-Prover Repair Prompt . . . . .                                                        | 50        |
| <b>L</b> | <b>Python Code for Proof Length</b>                                                          | <b>52</b> |
| <b>M</b> | <b>Proofs</b>                                                                                | <b>53</b> |

# 1 Introduction

Theorem proving in formal environments such as Lean (de Moura et al., 2015) provides an excellent testbed for training large language models (LLMs) in mathematical reasoning via reinforcement learning (RL). Since Lean can mechanically verify proofs, it filters hallucinations and provides reliable reward signals, and enables unlimited high-quality synthetic reasoning data. Leveraging these benefits, LLMs finetuned with RL have achieved near gold-medal performance on the International Mathematical Olympiad (IMO) (Chen et al., 2025) and shown strong results on difficult college-level benchmarks like PutnamBench (Lin et al., 2025b).

However, RL-trained provers often generate proofs that are correct but excessively long and inscrutable. Since their only reward signal is the *correctness of generated proofs*, the resulting models produce proofs that are *correct yet suboptimal*: convoluted, bloated with redundant steps, or reliant on unnecessarily strong automation where a simple step would suffice. For example, Seed-Prover (Chen et al., 2025)’s **Lean proof of IMO 2025 P1** consists of 4,357 lines of code, 16x longer (by character count) than its **informal counterpart**. Such proofs pose several practical drawbacks: they are (1) difficult for humans to comprehend, limiting their value as a source of mathematical insight; (2) less suitable as synthetic training data, since models may struggle to learn from convoluted proofs; and (3) computationally inefficient to compile in Lean, which is especially problematic when integrated into existing formal libraries like mathlib (mathlib Community, 2019).

These challenges highlight the need for *proof simplification: transforming existing formal proofs into simpler forms while preserving correctness*. In this work, we adopt a natural notion of simplicity: *proof length*, measured by the number of Lean tokens. However, our approach is agnostic to the choice of simplicity metric: it is not restricted to proof length, but applies to any automatically computable measure (Kinyon, 2018).

Prior work on proof simplification (Ahuja et al., 2024) focuses on agentic scaffolding around API-only LLMs such as GPT-4o. While these methods can shorten human-written Lean proofs, they are ineffective at simplifying the long proofs generated by SoTA RL-trained LLM provers such as Seed-Prover and Goedel-Prover-V2 (Lin et al., 2025b), precisely the setting where simplification is most valuable. A natural alternative is to finetune LLMs directly for proof simplification, but progress in this direction is limited by the lack of suitable training data, namely aligned pairs of proofs before and after simplification.

We introduce *ProofOptimizer*, an LLM-based system for simplifying long and convoluted proofs in Lean. ProofOptimizer integrates three components: (i) a symbolic Lean linter that identifies and removes redundant steps, (ii) a 7B parameter language model finetuned specifically for proof simplification, and (iii) an iterative inference-time algorithm for progressively shortening proofs. Given an input proof, the Lean linter first eliminates the most obvious redundancies. The language model then generates multiple candidate simplifications, and the iterative algorithm repeatedly applies the model to the currently shortest proof, further reducing its length. Training follows two paradigms. In expert iteration, the model proposes simplifications that are verified by Lean and incorporated into the training data for supervised finetuning. In reinforcement learning, proof length and correctness serve as the reward signal. Both approaches enable continual improvement without requiring any human-annotated simplification data.

First, we evaluate ProofOptimizer on long proofs generated by state-of-the-art neural theorem provers. Specifically, we consider proofs produced by Goedel-Prover-V2 on two standard benchmarks—MiniF2F (Zheng et al., 2021) and PutnamBench—as well as four proofs released

by Seed-Prover for IMO 2025. Our final models achieve significant results (Fig. 1), shortening MiniF2F proofs by an average of 63% in a single shot and PutnamBench proofs by 26% with 32 attempts, substantially outperforming Gemini-2.5-Pro (Sec. 4.1). At inference time, test-time RL improves single-shot miniF2F performance to 72%. With iterative shortening, we achieve further per-proof average reductions of 87% (MiniF2F) and 57% (PutnamBench) and reduce the length of three out of four Seed-Prover IMO 2025 proofs by more than half.

Second, we conduct ablation studies to evaluate the effect of key design choices. During training, RL achieves the best single-sample performance but reduces multi-sample diversity. At inference time, using the same RL recipe further improves single-shot performance (Sec. 4.1). Repairing incorrect simplifications from execution feedback with Goedel-Prover-V2 effectively corrects errors, but leads to repaired proofs even longer than the originals (Sec. 4.2). Overall, iterative proof shortening offers the best balance between performance and diversity, achieving the strongest results (Sec. 4.3).

Third, we conduct preliminary experiments suggesting two downstream benefits of proof shortening. Training our base model on shortened proofs leads to 2% better performance on miniF2F relative to training on unshortened proofs (Sec. 5.1). Also, shortening proofs often decreases their execution time, with 28% of proofs showing at least a 1.5x speedup after shortening (Sec. 5.2).

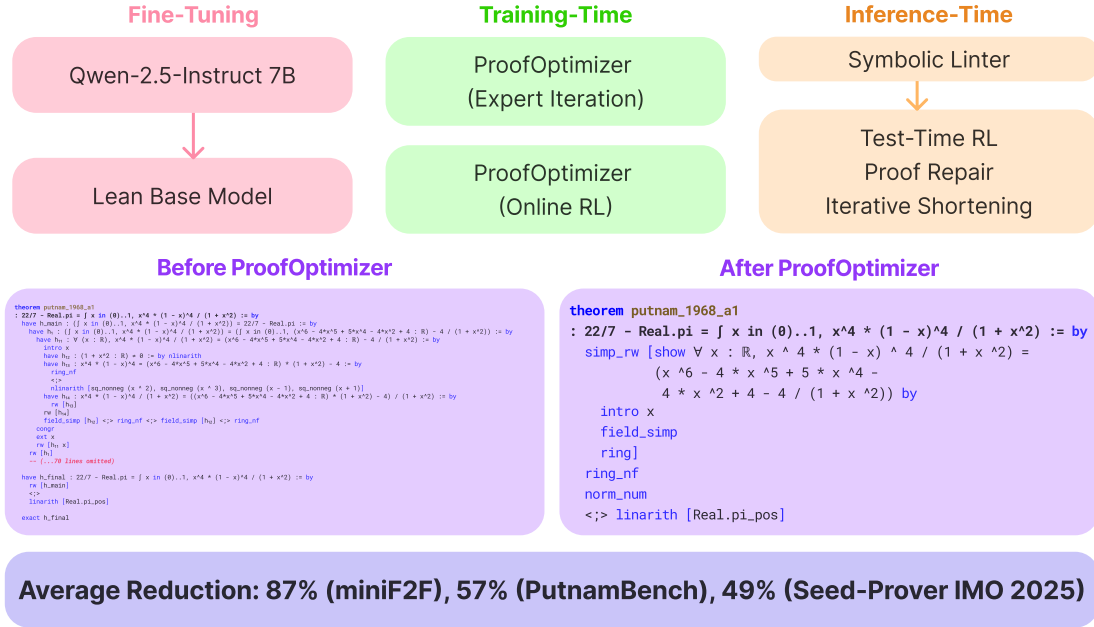

Figure 1: Overview of our pipeline. ProofOptimizer reduces the shortest generated proof of a Putnam problem from 1097 to 76 tokens.

## 2 Proof Simplification: Task and Metrics

**Task Definition** We formalize the proof simplification task as minimizing the complexity of a given proof. Specifically, for a valid formal statement  $s$  with proof  $p$ , the goal is to produce an alternative proof  $p^*$  of  $s$  that minimizes a complexity measure  $\mathcal{L}$ :

$$p^* = \arg \min_{x \text{ proves } s} \mathcal{L}(x)$$

Our method is agnostic to the choice of complexity measure  $\mathcal{L}$ , provided that it is deterministic and can be automatically computed from the proof. This flexibility encompasses the metrics used in prior work (Ahuja et al., 2024). In the rest of this paper, we adopt proof length as the measure of complexity, defined as the number of tokens produced by a Lean-specific tokenizer. Our proof length measure correlates with character count but does not penalize long identifier names, and it ignores comments and line breaks. We denote the length of a proof  $x$  by  $|x|$ , i.e.,  $\mathcal{L}(x) = |x|$ .

**Evaluation Metrics** Given an original proof  $p$  and  $k$  candidate simplifications generated by the model,  $p'_1, p'_2, \dots, p'_k$ , we define  $l_i = \min(|p|, |p'_i|)$  if  $p'_i$  is a valid proof and  $l_i = |p|$  otherwise. (Intuitively, an invalid attempt reverts to the original proof length). We evaluate proof simplification using two metrics:

- $\text{min@k} \triangleq \min_i \{l_i\}$  denotes the minimum shortened proof length (lower is better).
- $\text{red@k} \triangleq \max_i \left\{ \frac{|p| - l_i}{|p|} \right\} = 1 - \frac{\text{min@k}}{|p|}$  denotes the maximum relative proof length reduction from the original proof (higher is better).

Note that these metrics may not always be correlated: a method that only excels at shortening long proofs has a lower  $\text{min@k}$  and  $\text{red@k}$  than one that only excels at shortening short proofs. As with the  $\text{pass@k}$  metric (Chen et al., 2021), we report our metrics via an unbiased estimator using  $n > k$  samples (see Appendix I). We average  $\text{min@k}$  and  $\text{red@k}$  across samples in a dataset to get overall length and reduction metrics.

### 3 ProofOptimizer: LLMs for Proof Simplification

#### 3.1 Training

**Lean Base Model** First, we train a general-purpose Lean model by fine-tuning Qwen-2.5-7B-Instruct on a combination of five tasks: natural language problem solving, Lean 4 code completion, auto-formalization (problems and solutions), formal theorem proving, and tactic/proof state prediction.

**Dataset for Proof Simplification** We employ a four-stage pipeline to generate high-quality proof simplification training data.

1. *Problem Collection*: We first compile a dataset of theorem proving problems from Goedel-Pset, filtering out simple computational problems. Each problem consists of a natural language problem, solution, and Lean problem statement.
2. *Proof Sketching*: We train a model that formalizes a problem’s natural language solution into a Lean proof sketch consisting of a few high-level proof steps (usually 2-10) with lower level details omitted and filled in with Lean’s sorry tactic.
3. *Theorem Extraction and Filtering*: For each proof sketch, we extract each proof step into its own separate theorem. At the core, we are taking longer proofs and breaking them down into separate sub-theorems. We collect a total of 518K theorems this way. As we found some of these theorems to be trivial, we design an automation tactic to filter these out, leaving 307K theorems remaining.

4. *Proof Generation*: We use Goedel-Prover-V2-32B to generate proofs of these theorems. The model successfully produces Lean proofs of 145K theorems, which we use as our dataset for training.

For more details about our base model and dataset collection, see Appendix A. Next, we describe our two training recipes: expert iteration and online reinforcement learning.

### 3.1.1 ProofOptimizer-ExpIt: Expert Iteration

We leverage a STaR-like (Zelikman et al., 2022) iterative training algorithm to improve our model. At a high level, we start with our base model  $\pi_0$  and the collection of 145K proofs  $P_0$ . At each iteration, we attempt to simplify each proof, train our model on successful proof simplifications, and use the collection of simplified proofs as seed proofs for the next iteration. More precisely, at each iteration  $i$ , we do the following:

1. **Sample**: For each proof  $x \in P_i$ , use  $\pi_i$  to sample 4 simplifications  $Y_p \triangleq \{y_x^1, y_x^2, y_x^3, y_x^4\} \sim \pi_i(x)$ .
2. **Filter**: Use the Lean compiler to find the shortest correct simplification  $y_x \in \{x\} \cup Y_x$ . Create a training dataset of proof simplifications  $D_i = \{(x, y_x) \mid \text{len}(y_x) \leq 0.8 \cdot \text{len}(x), x \in P_i\}$ . The length constraint is designed to encourage the model to learn more substantial simplifications rather than trivial ones. For iterations after the first, as  $x$  may have been simplified from a more complex proof  $x' \in P_0$ , we also add  $(x', y_x)$  pairs to  $D_i$ , which are valid and larger proof simplifications. Also, collect simplified proofs  $\pi_{i+1} = \{s_x \mid x \in P_i\}$  for the next iteration.
3. **Train**: Fine-tune  $\pi_i$  on  $D_i$  to get  $\pi_{i+1}$ .

### 3.1.2 ProofOptimizer-RL: Online Reinforcement Learning

In addition to expert iteration as described in the previous section, we train a proof optimizer model with online reinforcement learning. Using the same dataset as in expert iteration, the reinforcement learning task consists in producing a valid but shorter proof  $y$  for a statement given an initial proof  $x$ . The reward is defined as the relative shortening  $R(x, y) = \frac{|y| - |x|}{|x|}$  if  $y$  is valid and  $|y| \leq |x|$ , and  $R(x, y) = 0$  otherwise. We employ an asynchronous variant of the GRPO algorithm (Shao et al., 2024) with advantage  $A_i = R_i - \frac{1}{k} \sum_{j \leq k} R_j$  baselined with the average reward of  $k = 8$  samples, no advantage normalization by standard deviation (Liu et al., 2025b), no KL regularization, and omitting sequences with zero advantage.

## 3.2 Inference-Time Techniques

First, we implement a symbolic linter that removes extraneous tactics via Lean’s `linter.unusedTactic` linter, which detects tactics that do not change the proof state and provides messages like `'norm_num' tactic does nothing`. We then compare the following techniques on the linted proofs:

- **Test-Time RL**: We use the setup described in Section 3.1.2 and perform reinforcement learning on our two evaluation sets (jointly). Our test-time RL keeps the input proof fixed, meaning improvements occur solely in the model’s parameters.

- **Repair with Execution Feedback:** In this scheme, if ProofOptimizer fails to simplify a proof, we collect the execution feedback and ask Goedel-Prover-V2-32B to repair the proof with the error messages. Then, we apply the symbolic linter on the new proofs to further shorten successful repairs.
- **Iterative Proof Shortening:** For a given proof, we sample  $k$  candidate shortenings and take the shortest correct one. Then, we sample  $k$  shortenings of the new proof, take the shortest correct one – and so on.

## 4 Experiments

For all evaluations, we use proofs generated by Goedel-Prover-V2 (Lin et al., 2025a) on two popular datasets in formal math, miniF2F (Zheng et al., 2021) and PutnamBench (Tsoukalas et al., 2024). For miniF2F, we use  $n = 194$  proofs (average length 334), and for PutnamBench, we use  $n = 75$  proofs (average length 1468). More details and examples of proofs in our evaluation set can be found in Appendix F.

### 4.1 Expert Iteration vs. RL vs. Test-Time RL

First, we compare our two training schemes: expert iteration and RL. Starting from our Lean base model, we train *ProofOptimizer-Explt* by performing three rounds of expert iteration (Sec. 3.1.1) and *ProofOptimizer-RL* by performing online RL (Sec. 3.1.2) after two rounds of expert iteration. Table 1 shows min@k and red@k scores with respect to linted proofs. We observe steady improvements during each round of expert iteration for both @1 and @32 metrics. **Our final model outperforms Gemini-2.5-Pro**, a strong reasoning model, even when given proof state annotations similar to Chain-of-States in ImProver (Ahuja et al., 2024).

Next, we see that **ProofOptimizer-RL significantly improves single sample (@1) metrics at the expense of diversity collapse**, an issue commonly identified during RL training (Gehring et al., 2024; Walder and Karkhanis, 2025; Yue et al., 2025). In Fig. 2 (a, b), we show the evolution of red@1 during training, observing that miniF2F reduction steadily rises while PutnamBench reduction experiences oscillations. This tension is likely because the distribution of training data is more similar in length to miniF2F than PutnamBench, which has a mean proof length of 4x that of the training set.

Finally, we find that test-time RL leads to even further improvements on min@1 and red@1. This is expected, as the model is able to directly tune its weights to learn from successful simplifications at test-time. However, like ProofOptimizer-RL, we observe an even smaller gap between @1 and @32 metrics. In Fig. 2 (c, d), we observe a much more stable evaluation red@1 curve because the distribution gap between the training and evaluation sets is eliminated.



Table 1: **Min@k and Red@k throughout expert iteration and online RL.** Our RL model has strong @1 results, while our ExpIt model has strong @32 results. RL metrics are Gaussian-smoothed.

| Dataset      | Category | Model                       | Min@1 ↓     | Min@32 ↓    | Red@1 ↑      | Red@32 ↑     |
|--------------|----------|-----------------------------|-------------|-------------|--------------|--------------|
| miniF2F      | ExpIt    | <i>Linted</i>               | 302         |             | 0.0%         |              |
|              |          | Gemini-2.5-Pro              | 280         | 207         | 24.3%        | 57.2%        |
|              |          | Gemini-2.5-Pro + States     | 283         | 207         | 26.4%        | 58.7%        |
|              |          | Base (7B)                   | 283         | 202         | 17.6%        | 56.2%        |
|              |          | Base + It 1                 | 266         | 178         | 33.4%        | 67.0%        |
|              |          | Base + It 2                 | 251         | 166         | 45.1%        | 70.6%        |
|              |          | <i>ProofOptimizer-ExpIt</i> | 241         | <b>153</b>  | 49.0%        | <b>72.3%</b> |
|              | RL       | <i>ProofOptimizer-RL</i>    | <b>190</b>  | <b>152</b>  | <b>63.6%</b> | <b>70.9%</b> |
|              |          | <i>It 2 + Test-Time RL</i>  | <b>160</b>  | <b>154</b>  | <b>72.5%</b> | <b>73.4%</b> |
| Putnam Bench | ExpIt    | <i>Linted</i>               | 1359        |             | 0.0%         |              |
|              |          | Gemini-2.5-Pro              | 1348        | 1303        | 5.5%         | 18.0%        |
|              |          | Gemini-2.5-Pro + States     | 1371        | 1319        | 6.1%         | 19.2%        |
|              |          | Base (7B)                   | 1341        | 1222        | 3.9%         | 20.5%        |
|              |          | Base + It 1                 | 1341        | 1215        | 5.2%         | 22.5%        |
|              |          | Base + It 2                 | 1335        | 1186        | 6.9%         | 24.7%        |
|              |          | <i>ProofOptimizer-ExpIt</i> | 1328        | <b>1161</b> | 8.2%         | <b>26.3%</b> |
|              | RL       | <i>ProofOptimizer-RL</i>    | <b>1303</b> | 1258        | <b>14.9%</b> | 21.1%        |
|              |          | <i>It 2 + Test-Time RL</i>  | <b>1260</b> | 1255        | <b>23.8%</b> | 24.2%        |

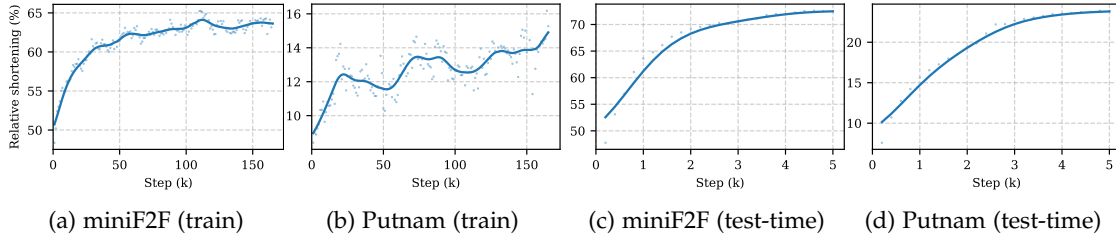

Figure 2: **Evolution of proof reduction (red@1) during RL training (a, b) and test-time RL (c, d).** We use Gaussian smoothing ( $\sigma = 5$  evaluation intervals for RL training and  $\sigma = 3$  for test-time RL). See Fig. 9 for the corresponding red@32 metrics.

## 4.2 Analysis of Repair with Execution Feedback

As described in Sec. 3.2, we (1) sample 64 simplifications for each proof with ProofOptimizer-ExpIt, (2) repair incorrect proofs with Goedel-Prover-V2-32B, and (3) shorten successful repairs with our linter. **Overall, we find while repair with execution feedback leads to improvements, it underperforms resampling because repaired proofs are often even longer than the original proofs.** Fig. 3 (left) shows the average proof length and reduction % after sampling, repair, and linting. We our linter to be effective on repaired proofs, decreasing the average repaired proof length from 644  $\rightarrow$  576 (miniF2F) and 877  $\rightarrow$  788 (PutnamBench). In Fig. 3 (right), we plot the proof length of the original proofs (before Step 1) against simplified proofs (Step 1) and repaired

Table 2: Step-by-step success rates, revealing the main bottleneck of long repaired proofs.

| Dataset     | Simplification               | Repair                      | Shorter than best (before/after linter)                                  |
|-------------|------------------------------|-----------------------------|--------------------------------------------------------------------------|
| miniF2F     | $\frac{7852}{12416}$ (63.2%) | $\frac{2840}{4564}$ (62.2%) | $\frac{76}{2840} \rightarrow \frac{137}{2840}$ (2.7% $\rightarrow$ 4.8%) |
| PutnamBench | $\frac{1288}{4800}$ (26.8%)  | $\frac{613}{3512}$ (17.4%)  | $\frac{5}{613} \rightarrow \frac{11}{613}$ (0.8% $\rightarrow$ 1.8%)     |

proofs (Step 2). A majority of the repaired proofs (green dots) are above the  $y = x$  line, meaning they are longer than the original proofs, let alone the simplified proofs (blue dots).

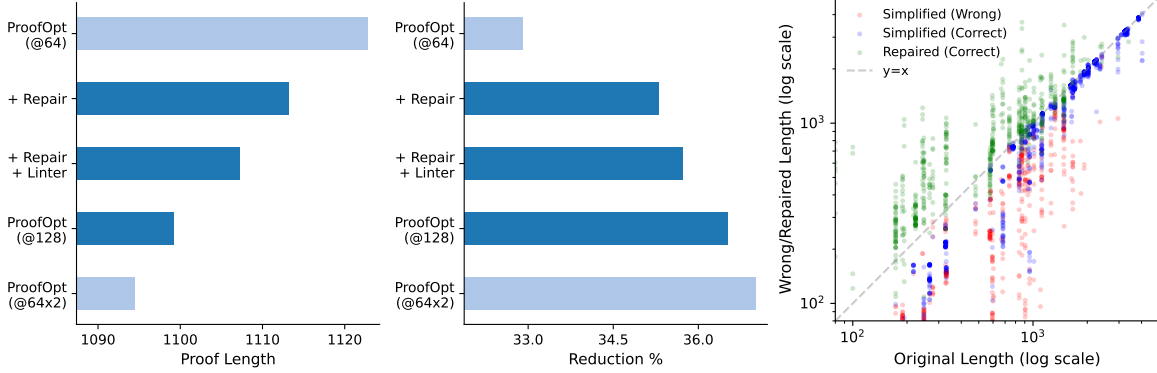

Figure 3: Analysis of execution-based repair with Goedel-Prover-V2 on PutnamBench.

In Table 2, we analyze the success rate of each step of our pipeline. However, the key issue remains to be the high length of the repaired proofs. Even after linting, only 4.8% (miniF2F) / 1.8% (Putnam) of post-linted proofs are shorter than the best proof found by ProofOptimizer during simplification. We refer the reader to Appendix E for further analysis and examples.

### 4.3 Iterative Proof Shortening

In Fig. 4 (left), we show the results of iterative proof shortening on miniF2F and PutnamBench proofs using *ProofOptimizer-Expt*. First, we do 64 samples per iteration for 6 iterations, observing steady improvement at each iteration. To demonstrate the potential of further scaling, we do 1024 samples at iterations 7 and 8 and see significant improvement (see Appendix C.2 for analysis on sample size). **Overall, ProofOptimizer combined with iterative proof shortening is very effective on miniF2F and PutnamBench, as average proof length is reduced from 334  $\rightarrow$  75 and 1468  $\rightarrow$  811, for an average per-proof reduction of 87.9%/57.2%.** In Fig. 4 (right), we plot the overall shortening against the length of the original proof, observing that longer proofs remain challenging to simplify.

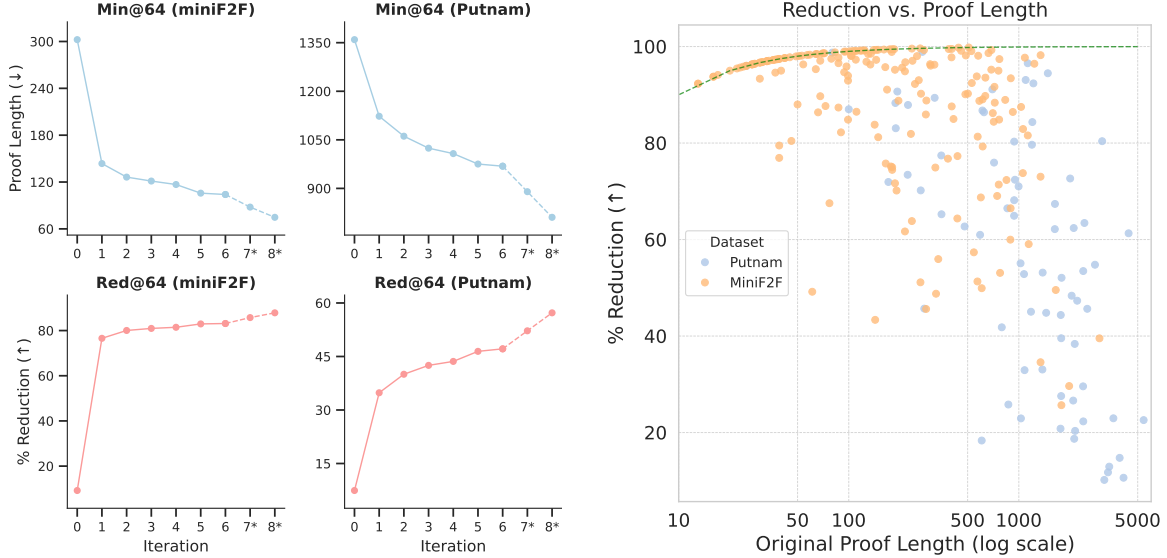

Figure 4: Iterative Shortening: per-iteration improvement (left) and effect of proof length (right)

Finally, in Table 3, we demonstrate the effectiveness of ProofOptimizer on an out-of-distribution dataset, Seed-Prover’s **four IMO 2025 proofs**. With an order of magnitude higher sampling budget, we achieve a significant reduction in the proof length for all four problems, showcasing the potential of our model and technique. Details about our full setup are in Appendix C.3.

Table 3: Iterative shortening achieves significant reduction for Seed-Prover’s IMO 2025 proofs.

|                         | P1    | P3    | P4    | P5    |
|-------------------------|-------|-------|-------|-------|
| Original Proof Length   | 36478 | 16377 | 29147 | 8658  |
| Simplified Proof Length | 20506 | 7907  | 14531 | 4002  |
| Length Reduction        | 43.8% | 51.7% | 50.1% | 53.8% |

## 5 Additional Benefits of Proof Simplification

### 5.1 Training on Simplified Proofs Improves Generation

Next, we investigate whether fine-tuning on simplified proofs can be advantageous compared to fine-tuning on longer, raw proofs. To do so, we prepare two datasets of identical problems, the first containing a set of proofs generated by Goedel-Prover-V2 and the second containing the same proofs simplified by ProofOptimizer-ExpIt. The average proof length of the original and simplified proofs is 147 and 85, respectively. We do continued supervised fine-tuning (SFT) starting from our base model (Sec. A.1) with a standard negative log-likelihood (NLL) loss.

In Fig. 5 (left), we compare the training loss between the two datasets. As expected, the initial loss when using original proofs is higher, as models have not seen such long proofs during initial fine-tuning. However, the losses quickly converge. We observe that training on original proofs causes occasional loss spikes, which we suspect are due to several data batches that are hard to

learn (e.g. extremely long proofs). Decreasing the learning rate mitigated these training loss spikes but did not improve validation accuracy. In Fig. 5 (right), we compare the miniF2F scores of the two models during SFT, showing that training on simplified proofs results in slightly higher evaluation accuracy despite the two settings having identical training losses.

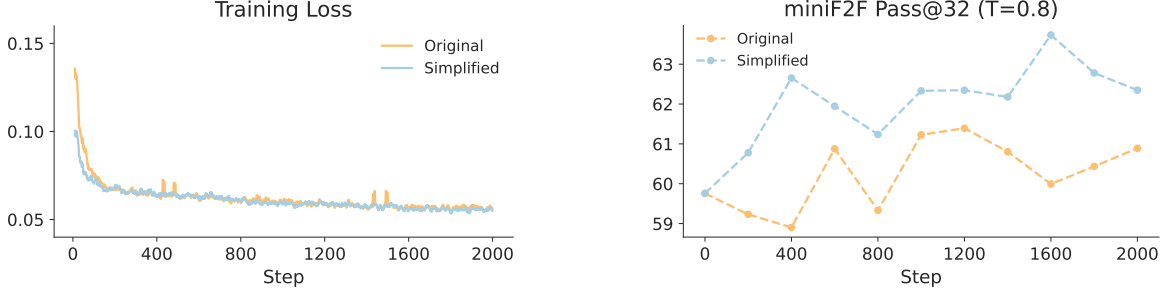

Figure 5: Training loss (left) and miniF2F score (right) after SFT on simplified vs. original proofs.

## 5.2 Simplified Proofs Have a Shorter Execution Time

We also observe that proofs simplified by ProofOptimizer often exhibit a faster execution time. We measure proof execution time with `lake env lean --profile`, excluded library import time (imports are always the same but actual time may vary due to caching effects). We compare the execution times of each proof before and after iterative shortening in Fig. 6 (scatter). For both datasets, we visibly observe that a majority of points lie below the  $y = x$  line, signifying speedup. Fig. 6 (histograms) also show the distribution of speedup ratios  $\frac{\text{time}_{\text{orig}}}{\text{time}_{\text{new}}}$ . Of the 75 PutnamBench proofs, 50/75 have a speedup of over 10%, and 22/75 of those have a speedup of over 50%. We also observe that proofs with a higher original execution time tend to show more speedup. The same trends hold for miniF2F, where 114/194 and 56/194 proofs have a speedup over 10% and 50%, respectively. Finally, we observe 25% and 81% speedups on Seed-Prover’s proofs for P3 and P4 of the IMO 2025 (Sec. C.3).

Upon qualitatively analyzing the proofs, we observe that the original proofs often have extraneous tactics that are eliminated by the simplified proofs. However, we also find several cases where the simplified proofs are much slower than the original proof, which usually occurs when a faster proof algorithm is replaced by a shorter but slower method (e.g. brute force with `interval_cases`). We provide two examples of each in Appendix H.2.

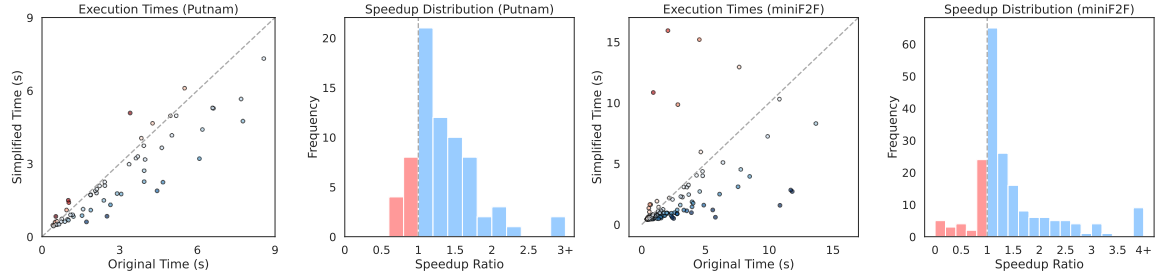

Figure 6: Simplified proofs are frequently faster than original proofs on miniF2F and PutnamBench.

### 5.2.1 Optimizing for Heartbeats instead of Proof Length

As we stated in Sec. 2, our complexity measure  $\mathcal{L}$  generalizes beyond proof length. Next, we set  $\mathcal{L}$  to be the number of Lean heartbeats<sup>1</sup>, a proxy of execution time that can run efficiently in parallel. With this metric, we run eight iterations of the same inference-time algorithm using ProofOptimizer-ExpIt. In Fig. 7 (a, b), we show analogous plots as earlier for miniF2F. Observe that this time, all the points are now on or below the  $y = x$  line, eliminating the short but slow proofs we saw in Fig. 6. Overall, we observe faster proofs, with 138/194 and 81/194 miniF2F proofs showing a speedup over 10% and 50%, respectively (compared to 114/194 and 56/194 before using the length metric). In Fig. 7 (c), we see that while the lengths of the proofs found with this metric are slightly longer than before, there is still considerable shortening. Finally, Fig. 7 (d) explains this by showing that proof length and number of heartbeats are generally correlated. In the future, optimizing for a combination of proof length and heartbeat count could lead to improvements in both readability and execution time. Full results can be found in Sec. H.1.

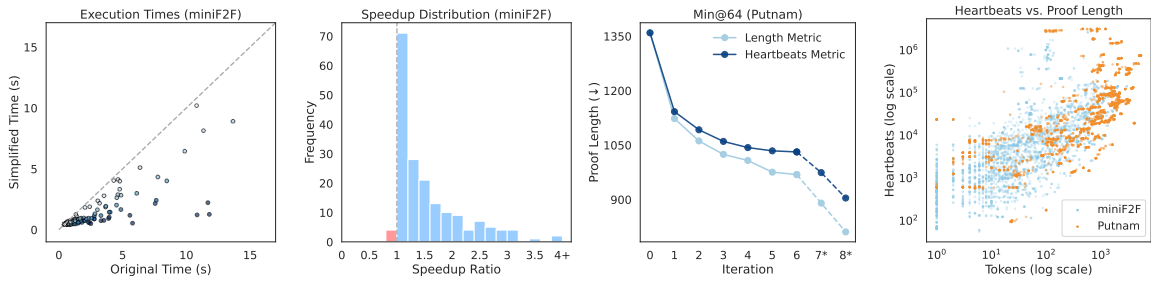

Figure 7: Using heartbeats instead of proof length as complexity measure

## 6 Related Works

**LLMs for Theorem Proving in Lean** Formal theorem proving is a rapidly growing frontier in AI for mathematics and software verification (Yang et al., 2024b; Li et al., 2024). Progress is typically measured with benchmarks of mathematical theorems in Lean such as miniF2F (Zheng et al., 2021), PutnamBench (Tsoukalas et al., 2024), and ProofNet (Azerbayev et al., 2023). Recently, there have been many LLMs developed for Lean such as Seed-Prover (Chen et al., 2025), Goedel-Prover (Lin et al., 2025a), DeepSeek-Prover (Ren et al., 2025), and Kimina-Prover (Wang et al., 2025). There have also been post-training techniques built on top of these models, such as with expert iteration (Lin et al., 2024), proof sketching (Cao et al., 2025), tree search (Lample et al., 2022; Zimmer et al., 2025), self-play (Dong and Ma, 2025), proof repair (Ospanov et al., 2025), and RL (Gloeckle et al., 2024).

**AI for Program Simplification** A related line of work makes programs shorter or more efficient (Schkufza et al., 2013; Mankowitz et al., 2023; Shypula et al., 2023; Gautam et al., 2024). In parallel, library learning aims to discover reusable abstractions, often eliminating repeated code and shortening programs (Ellis et al., 2023; Grand et al., 2023; Kaliszyk and Urban, 2015; Wang et al., 2023; Zhou et al., 2024; Berlot-Attwell et al., 2024). Finally, symbolic reasoning techniques like program slicing (Weiser, 2009), super-optimization (Sasnauskas et al., 2017), or partial evaluation (Jones, 1996) can also shorten and optimize low-level code.

<sup>1</sup>We use `#count_heartbeats` with `set_option Elab.async false`

**Automated Proof Shortening** Frieder et al. (2024) study factors that make Lean proofs easier to understand, motivating shorter proofs for maintainability. Classically, there have also been many symbolic methods targeting shortening proofs in SAT and first-order logic languages (Rahul and Necula, 2001; Vyskočil et al., 2010; Wernhard and Bibel, 2024; Gladshtein et al., 2024; Kinyon, 2018). On the neural side, GPT-f (Polu and Sutskever, 2020) generated 23 verified proofs shorter than those in the Metamath library. Most related to our work, ImProver (Ahuja et al., 2024), is an inference-time method for proof shortening using GPT-4o with proof states and retrieval. In contrast, we use training-time approaches (expert iteration and RL), analyze complementary inference-time techniques, and focus on shortening longer proofs generated by SoTA LLMs.

## 7 Conclusion

We present ProofOptimizer, the first language model trained to simplify Lean proofs. Unlike prior work that wraps existing LLMs around agentic scaffolding, we train a model using expert iteration and RL, coupled with a symbolic linter and iterative proof shortening at inference time. While simple, our approach already yields nontrivial results, reducing proof length by an average of 87% on MiniF2F, 57% on PutnamBench, and 49% on Seed-Prover’s IMO 2025 proofs. As AI becomes more tightly integrated with mathematics, we envision a future where AI-generated proofs are not only correct but also concise and readable, with simplification serving as a critical bridge between rigorous formal proofs and human intuitive understanding.

## 8 Acknowledgments

We thank Heather Macbeth for suggesting the experiments in Sec. 5.2.1 and writing the code to count heartbeats, Albert Jiang and Melanie Matchett Wood for discussions regarding desiderata in proof simplification, Amaury Hayat for providing guidance throughout the project, and many members at FAIR for various technical contributions, suggestions, and insightful discussions.

## References

- Josh Achiam, Steven Adler, Sandhini Agarwal, Lama Ahmad, Ilge Akkaya, Florencia Leoni Aleman, Diogo Almeida, Janko Altenschmidt, Sam Altman, Shyamal Anadkat, et al. GPT-4 technical report. *arXiv preprint arXiv:2303.08774*, 2023. (Cited on pg. 30)
- Riyaz Ahuja, Jeremy Avigad, Prasad Tetali, and Sean Welleck. Improver: Agent-based automated proof optimization. *arXiv preprint arXiv:2410.04753*, 2024. (Cited on pg. 4, 6, 8, 14)
- Leni Aniva, Chuyue Sun, Brando Miranda, Clark Barrett, and Sanmi Koyejo. Pantograph: A machine-to-machine interaction interface for advanced theorem proving, high level reasoning, and data extraction in lean 4. In *International Conference on Tools and Algorithms for the Construction and Analysis of Systems*, pages 104–123. Springer, 2025. (Cited on pg. 20)
- Hugh Leather Aram H. Markosyan, Gabriel Synnaeve. Leanuniverse: A library for consistent and scalable lean4 dataset management. <https://github.com/facebookresearch/LeanUniverse>, 2024. (Cited on pg. 20)
- Zhangir Azerbayev, Bartosz Piotrowski, Hailey Schoelkopf, Edward W Ayers, Dragomir Radev, and Jeremy Avigad. Proofnet: Autoformalizing and formally proving undergraduate-level mathematics. *arXiv preprint arXiv:2302.12433*, 2023. (Cited on pg. 13, 20)
- Ian Berlot-Attwell, Frank Rudzicz, and Xujie Si. Library learning doesn’t: The curious case of the single-use” library”. *arXiv preprint arXiv:2410.20274*, 2024. (Cited on pg. 13)
- Chenrui Cao, Liangcheng Song, Zenan Li, Xinyi Le, Xian Zhang, Hui Xue, and Fan Yang. Reviving dsp for advanced theorem proving in the era of reasoning models. *arXiv preprint arXiv:2506.11487*, 2025. (Cited on pg. 13)
- Luoxin Chen, Jinming Gu, Liankai Huang, Wenhao Huang, Zhicheng Jiang, Allan Jie, Xiaoran Jin, Xing Jin, Chenggang Li, Kaijing Ma, et al. Seed-prover: Deep and broad reasoning for automated theorem proving, 2025. URL <https://arxiv.org/abs/2507.23726>, 2025. (Cited on pg. 4, 13, 28)
- Mark Chen, Jerry Tworek, Heewoo Jun, Qiming Yuan, Henrique Ponde de Oliveira Pinto, Jared Kaplan, Harri Edwards, Yuri Burda, Nicholas Joseph, Greg Brockman, Alex Ray, Raul Puri, Gretchen Krueger, Michael Petrov, Heidy Khlaaf, Girish Sastry, Pamela Mishkin, Brooke Chan, Scott Gray, Nick Ryder, Mikhail Pavlov, Alethea Power, Lukasz Kaiser, Mohammad Bavarian, Clemens Winter, Philippe Tillet, Felipe Petroski Such, Dave Cummings, Matthias Plappert, Fotios Chantzis, Elizabeth Barnes, Ariel Herbert-Voss, William Hebgen Guss, Alex Nichol, Alex Paino, Nikolas Tezak, Jie Tang, Igor Babuschkin, Suchir Balaji, Shantanu Jain, William Saunders, Christopher Hesse, Andrew N. Carr, Jan Leike, Josh Achiam, Vedant Misra, Evan Morikawa, Alec Radford, Matthew Knight, Miles Brundage, Mira Murati, Katie Mayer, Peter Welinder, Bob McGrew, Dario Amodei, Sam McCandlish, Ilya Sutskever, and Wojciech Zaremba. Evaluating large language models trained on code, 2021. URL <https://arxiv.org/abs/2107.03374>. (Cited on pg. 6, 47)
- Gheorghe Comanici, Eric Bieber, Mike Schaeckermann, Ice Pasupat, Noveen Sachdeva, Inderjit Dhillon, Marcel Blistein, Ori Ram, Dan Zhang, Evan Rosen, et al. Gemini 2.5: Pushing the frontier with advanced reasoning, multimodality, long context, and next generation agentic capabilities. *arXiv preprint arXiv:2507.06261*, 2025. (Cited on pg. 30)



- Leonardo Mendonça de Moura, Soonho Kong, Jeremy Avigad, Floris van Doorn, and Jakob von Raumer. The lean theorem prover (system description). In Amy P. Felty and Aart Middeldorp, editors, *Automated Deduction - CADE-25 - 25th International Conference on Automated Deduction, Berlin, Germany, August 1-7, 2015, Proceedings*, volume 9195 of *Lecture Notes in Computer Science*, pages 378–388. Springer, 2015. doi: 10.1007/978-3-319-21401-6\\_26. URL [https://doi.org/10.1007/978-3-319-21401-6\\_26](https://doi.org/10.1007/978-3-319-21401-6_26). (Cited on pg. 4)
- Kefan Dong and Tengyu Ma. Stp: Self-play llm theorem provers with iterative conjecturing and proving. *arXiv preprint arXiv:2502.00212*, 2025. (Cited on pg. 13, 20)
- Kevin Ellis, Lionel Wong, Maxwell Nye, Mathias Sable-Meyer, Luc Cary, Lore Anaya Pozo, Luke Hewitt, Armando Solar-Lezama, and Joshua B Tenenbaum. Dreamcoder: growing generalizable, interpretable knowledge with wake-sleep bayesian program learning. *Philosophical Transactions of the Royal Society A*, 381(2251):20220050, 2023. (Cited on pg. 13)
- Simon Frieder, Jonas Bayer, Katherine M Collins, Julius Berner, Jacob Loader, András Juhász, Fabian Ruehle, Sean Welleck, Gabriel Poesia, Ryan-Rhys Griffiths, et al. Data for mathematical copilots: Better ways of presenting proofs for machine learning. *arXiv preprint arXiv:2412.15184*, 2024. (Cited on pg. 14)
- Dhruv Gautam, Spandan Garg, Jinu Jang, Neel Sundaresan, and Roshanak Zilouchian Moghaddam. Refactorbench: Evaluating stateful reasoning in language agents through code. In *NeurIPS 2024 Workshop on Open-World Agents*, 2024. (Cited on pg. 13)
- Jonas Gehring, Kunhao Zheng, Jade Copet, Vegard Mella, Quentin Carbonneaux, Taco Cohen, and Gabriel Synnaeve. Rlef: Grounding code llms in execution feedback with reinforcement learning. *arXiv preprint arXiv:2410.02089*, 2024. (Cited on pg. 8)
- Vladimir Gladshtein, George Pîrlea, and Ilya Sergey. Small scale reflection for the working lean user. *arXiv preprint arXiv:2403.12733*, 2024. (Cited on pg. 14)
- Fabian Gloeckle, Jannis Limperg, Gabriel Synnaeve, and Amaury Hayat. Abel: Sample efficient online reinforcement learning for neural theorem proving. In *The 4th Workshop on Mathematical Reasoning and AI at NeurIPS’24*, 2024. (Cited on pg. 13)
- Gabriel Grand, Lionel Wong, Maddy Bowers, Theo X Olausson, Muxin Liu, Joshua B Tenenbaum, and Jacob Andreas. Lilo: Learning interpretable libraries by compressing and documenting code. *arXiv preprint arXiv:2310.19791*, 2023. (Cited on pg. 13)
- Albert Q Jiang, Sean Welleck, Jin Peng Zhou, Wenda Li, Jiacheng Liu, Mateja Jamnik, Timothée Lacroix, Yuhuai Wu, and Guillaume Lample. Draft, sketch, and prove: Guiding formal theorem provers with informal proofs. *arXiv preprint arXiv:2210.12283*, 2022. (Cited on pg. 20)
- Neil D Jones. An introduction to partial evaluation. *ACM Computing Surveys (CSUR)*, 28(3):480–503, 1996. (Cited on pg. 13)
- Cezary Kaliszyk and Josef Urban. Learning-assisted theorem proving with millions of lemmas. *Journal of symbolic computation*, 69:109–128, 2015. (Cited on pg. 13)
- Michael Kinyon. Proof simplification and automated theorem proving. *CoRR*, abs/1808.04251, 2018. URL <http://arxiv.org/abs/1808.04251>. (Cited on pg. 4, 14)
- Guillaume Lample, Timothee Lacroix, Marie-Anne Lachaux, Aurelien Rodriguez, Amaury Hayat, Thibaut Lavril, Gabriel Ebner, and Xavier Martinet. Hypertree proof search for neural theorem proving. *Advances in neural information processing systems*, 35:26337–26349, 2022. (Cited on pg. 13)



- Jia LI, Edward Beeching, Lewis Tunstall, Ben Lipkin, Roman Soletskyi, Shengyi Costa Huang, Kashif Rasul, Longhui Yu, Albert Jiang, Ziju Shen, Zihan Qin, Bin Dong, Li Zhou, Yann Fleureau, Guillaume Lample, and Stanislas Polu. Numinamath. [<https://huggingface.co/AI-M0/NuminaMath-1.5>] ([https://github.com/project-numina/aimo-progress-prize/blob/main/report/numina\\_dataset.pdf](https://github.com/project-numina/aimo-progress-prize/blob/main/report/numina_dataset.pdf)), 2024. (Cited on pg. 20, 22)
- Zhaoyu Li, Jialiang Sun, Logan Murphy, Qidong Su, Zenan Li, Xian Zhang, Kaiyu Yang, and Xujie Si. A survey on deep learning for theorem proving. *arXiv preprint arXiv:2404.09939*, 2024. (Cited on pg. 13)
- Haohan Lin, Zhiqing Sun, Sean Welleck, and Yiming Yang. Lean-star: Learning to interleave thinking and proving. *arXiv preprint arXiv:2407.10040*, 2024. (Cited on pg. 13)
- Yong Lin, Shange Tang, Bohan Lyu, Jiayun Wu, Hongzhou Lin, Kaiyu Yang, Jia Li, Mengzhou Xia, Danqi Chen, Sanjeev Arora, et al. Goedel-prover: A frontier model for open-source automated theorem proving. *arXiv preprint arXiv:2502.07640*, 2025a. (Cited on pg. 8, 13, 20, 21)
- Yong Lin, Shange Tang, Bohan Lyu, Ziran Yang, Jui-Hui Chung, Haoyu Zhao, Lai Jiang, Yihan Geng, Jiawei Ge, Jingruo Sun, et al. Goedel-prover-v2: Scaling formal theorem proving with scaffolded data synthesis and self-correction. *arXiv preprint arXiv:2508.03613*, 2025b. (Cited on pg. 4)
- Junqi Liu, Xiaohan Lin, Jonas Bayer, Yael Dillies, Weijie Jiang, Xiaodan Liang, Roman Soletskyi, Haiming Wang, Yunzhou Xie, Beibei Xiong, et al. Combibench: Benchmarking llm capability for combinatorial mathematics. *arXiv preprint arXiv:2505.03171*, 2025a. (Cited on pg. 20)
- Zichen Liu, Changyu Chen, Wenjun Li, Penghui Qi, Tianyu Pang, Chao Du, Wee Sun Lee, and Min Lin. Understanding r1-zero-like training: A critical perspective, 2025b. URL <https://arxiv.org/abs/2503.20783>. (Cited on pg. 7)
- Daniel J Mankowitz, Andrea Michi, Anton Zhernov, Marco Gelmi, Marco Selvi, Cosmin Paduraru, Edouard Leurent, Shariq Iqbal, Jean-Baptiste Lesciau, Alex Ahern, et al. Faster sorting algorithms discovered using deep reinforcement learning. *Nature*, 618(7964):257–263, 2023. (Cited on pg. 13)
- The mathlib Community. The lean mathematical library. *CoRR*, abs/1910.09336, 2019. URL <http://arxiv.org/abs/1910.09336>. (Cited on pg. 4)
- Azim Ospanov, Farzan Farnia, and Roozbeh Yousefzadeh. Apollo: Automated llm and lean collaboration for advanced formal reasoning. *arXiv preprint arXiv:2505.05758*, 2025. (Cited on pg. 13)
- Stanislas Polu and Ilya Sutskever. Generative language modeling for automated theorem proving. *arXiv preprint arXiv:2009.03393*, 2020. (Cited on pg. 14)
- Shree Prakash Rahul and George C Necula. *Proof optimization using lemma extraction*. Computer Science Division, University of California, 2001. (Cited on pg. 14)
- ZZ Ren, Zhihong Shao, Junxiao Song, Huajian Xin, Haocheng Wang, Wanbiao Zhao, Liyue Zhang, Zhe Fu, Qihao Zhu, Dejian Yang, et al. Deepseek-prover-v2: Advancing formal mathematical reasoning via reinforcement learning for subgoal decomposition. *arXiv preprint arXiv:2504.21801*, 2025. (Cited on pg. 13)
- Raimondas Sasnauskas, Yang Chen, Peter Collingbourne, Jeroen Ketema, Gratian Lup, Jubi Taneja, and John Regehr. Souper: A synthesizing superoptimizer. *arXiv preprint arXiv:1711.04422*, 2017. (Cited on pg. 13)

- Eric Schkufza, Rahul Sharma, and Alex Aiken. Stochastic superoptimization. *ACM SIGARCH Computer Architecture News*, 41(1):305–316, 2013. (Cited on pg. 13)
- Zhihong Shao, Peiyi Wang, Qihao Zhu, Runxin Xu, Junxiao Song, Xiao Bi, Haowei Zhang, Mingchuan Zhang, Y. K. Li, Y. Wu, and Daya Guo. Deepseekmath: Pushing the limits of mathematical reasoning in open language models, 2024. URL <https://arxiv.org/abs/2402.03300>. (Cited on pg. 7)
- Alexander Shypula, Aman Madaan, Yimeng Zeng, Uri Alon, Jacob Gardner, Milad Hashemi, Graham Neubig, Parthasarathy Ranganathan, Osbert Bastani, and Amir Yazdanbakhsh. Learning performance-improving code edits. *arXiv preprint arXiv:2302.07867*, 2023. (Cited on pg. 13)
- Qwen Team. Qwen2.5: A party of foundation models, September 2024. URL <https://qwenlm.github.io/blog/qwen2.5/>. (Cited on pg. 30)
- George Tsoukalas, Jasper Lee, John Jennings, Jimmy Xin, Michelle Ding, Michael Jennings, Amityay Thakur, and Swarat Chaudhuri. PutnamBench: Evaluating neural theorem-provers on the putnam mathematical competition. *Advances in Neural Information Processing Systems*, 37: 11545–11569, 2024. (Cited on pg. 8, 13, 20)
- Jiří Vyskočil, David Stanovský, and Josef Urban. Automated proof compression by invention of new definitions. In *International Conference on Logic for Programming Artificial Intelligence and Reasoning*, pages 447–462. Springer, 2010. (Cited on pg. 14)
- Christian Walder and Deep Karkhanis. Pass@ k policy optimization: Solving harder reinforcement learning problems. *arXiv preprint arXiv:2505.15201*, 2025. (Cited on pg. 8)
- Haiming Wang, Huajian Xin, Chuanyang Zheng, Lin Li, Zhengying Liu, Qingxing Cao, Yinya Huang, Jing Xiong, Han Shi, Enze Xie, et al. Lego-prover: Neural theorem proving with growing libraries. *arXiv preprint arXiv:2310.00656*, 2023. (Cited on pg. 13)
- Haiming Wang, Mert Unsal, Xiaohan Lin, Mantas Baksys, Junqi Liu, Marco Dos Santos, Flood Sung, Marina Vinyes, Zhenzhe Ying, Zekai Zhu, et al. Kimina-prover preview: Towards large formal reasoning models with reinforcement learning. *arXiv preprint arXiv:2504.11354*, 2025. (Cited on pg. 13)
- Mark Weiser. Program slicing. *IEEE Transactions on software engineering*, (4):352–357, 2009. (Cited on pg. 13)
- Christoph Wernhard and Wolfgang Bibel. Investigations into proof structures. *Journal of Automated Reasoning*, 68(4):24, 2024. (Cited on pg. 14)
- An Yang, Baosong Yang, Binyuan Hui, Bo Zheng, Bowen Yu, Chang Zhou, Chengpeng Li, Chengyuan Li, Dayiheng Liu, Fei Huang, Guanting Dong, Haoran Wei, Huan Lin, Jialong Tang, Jialin Wang, Jian Yang, Jianhong Tu, Jianwei Zhang, Jianxin Ma, Jin Xu, Jingren Zhou, Jinze Bai, Jinzheng He, Junyang Lin, Kai Dang, Keming Lu, Keqin Chen, Kexin Yang, Mei Li, Mingfeng Xue, Na Ni, Pei Zhang, Peng Wang, Ru Peng, Rui Men, Ruize Gao, Runji Lin, Shijie Wang, Shuai Bai, Sinan Tan, Tianhang Zhu, Tianhao Li, Tianyu Liu, Wenbin Ge, Xiaodong Deng, Xiaohuan Zhou, Xingzhang Ren, Xinyu Zhang, Xipin Wei, Xuancheng Ren, Yang Fan, Yang Yao, Yichang Zhang, Yu Wan, Yunfei Chu, Yuqiong Liu, Zeyu Cui, Zhenru Zhang, and Zhihao Fan. Qwen2 technical report. *arXiv preprint arXiv:2407.10671*, 2024a. (Cited on pg. 20)
- Kaiyu Yang, Gabriel Poesia, Jingxuan He, Wenda Li, Kristin Lauter, Swarat Chaudhuri, and Dawn Song. Formal mathematical reasoning: A new frontier in ai. *arXiv preprint arXiv:2412.16075*, 2024b. (Cited on pg. 13)

- Huaiyuan Ying, Zijian Wu, Yihan Geng, Jiayu Wang, Dahua Lin, and Kai Chen. Lean workbook: A large-scale lean problem set formalized from natural language math problems. *Advances in Neural Information Processing Systems*, 37:105848–105863, 2024. (Cited on pg. 20)
- Zhouliang Yu, Ruotian Peng, Keyi Ding, Yizhe Li, Zhongyuan Peng, Minghao Liu, Yifan Zhang, Zheng Yuan, Huajian Xin, Wenhao Huang, et al. Formalmath: Benchmarking formal mathematical reasoning of large language models. *arXiv preprint arXiv:2505.02735*, 2025. (Cited on pg. 20)
- Yang Yue, Zhiqi Chen, Rui Lu, Andrew Zhao, Zhaokai Wang, Yang Yue, Shiji Song, and Gao Huang. Does reinforcement learning really incentivize reasoning capacity in llms beyond the base model?, 2025. URL <https://arxiv.org/abs/2504.13837>. (Cited on pg. 8)
- Eric Zelikman, Yuhuai Wu, Jesse Mu, and Noah Goodman. Star: Bootstrapping reasoning with reasoning. *Advances in Neural Information Processing Systems*, 35:15476–15488, 2022. (Cited on pg. 7)
- Kunhao Zheng, Jesse Michael Han, and Stanislas Polu. Minif2f: a cross-system benchmark for formal olympiad-level mathematics. *arXiv preprint arXiv:2109.00110*, 2021. (Cited on pg. 4, 8, 13, 20)
- Jin Peng Zhou, Yuhuai Wu, Qiyang Li, and Roger Grosse. Refactor: Learning to extract theorems from proofs. *arXiv preprint arXiv:2402.17032*, 2024. (Cited on pg. 13)
- Matthieu Zimmer, Xiaotong Ji, Rasul Tutunov, Anthony Bordg, Jun Wang, and Haitham Bou Ammar. Bourbaki: Self-generated and goal-conditioned mdps for theorem proving. *arXiv preprint arXiv:2507.02726*, 2025. (Cited on pg. 13)

# A Lean Base Model and Proof Simplification Data Details

## A.1 General Base Model for Lean

In this section, we describe the data recipe for training our general-purpose base model in Lean. We fine-tune Qwen-2.5-7B-Instruct (Yang et al., 2024a) on around 1B Lean tokens on a combination of diverse math and Lean-related tasks, as follows:

- **Natural Language Problem Solving:** The model is trained on natural language mathematics problems with associated solutions so that it has general math capabilities. We use NuminaMath-1.5 (LI et al., 2024), a high-quality set of such pairs.
- **Lean Code Completion:** We use a subset of Lean code from GitHub, using GPT-4o with heuristics to classify whether code is Lean 3 or Lean 4. We include only the Lean 4 subset of the code.
- **Auto-formalization:** In order to teach the model to associate natural language with Lean, we train the model to perform auto-formalization of both problems and solutions from natural language to Lean 4 in our data mix. For problems, we use natural language problems with Lean problem statement formalizations from high-quality datasets: CombiBench (Liu et al., 2025a), Compfiles, FormalMATH (Yu et al., 2025), Goedel-Pset (Lin et al., 2025a), Lean Workbook (Ying et al., 2024), miniF2F (Zheng et al., 2021), ProofNet (Azerbaiyev et al., 2023), and PutnamBench (Tsoukalas et al., 2024). We include solution autoformalization data from the Goedel-Pset-v1-Solved dataset by mapping Lean solutions with natural language solutions.
- **Formal Theorem Proving:** We use a set of conjectures and proofs from STP (Dong and Ma, 2025), which is a diverse collection of theorems and proofs in Lean 4 generated via expert iteration while training their model.
- **Tactic and Proof State Prediction:** Finally, to teach the model about proof states, we use pre-extracted data from LeanUniverse (Aram H. Markosyan, 2024) and extract additional data using the Pantograph (Aniva et al., 2025) tool. For each proof in STP, we extract each tactic, as well as the proof states before and after the tactic. The model is given the proof state before the tactic and asked to predict both the tactic and the proof state following the tactic.

## A.2 Generating a Dataset of Theorems and Proofs for Shortening

Next, we describe how we generate our training dataset of proofs to be shortened.

**Formalizing Proofs with Sketches to Derive Subtheorems** While there are many datasets such as Goedel-Pset and Lean Workbook, we find that they have a high density of simple computational problems posed as proofs rather than high-quality proving problems. In Goedel-Pset, we estimate that only 5% of the problems are proof problems<sup>2</sup>, leading to a lack of high-quality theorem proving data. To combat this, we develop a technique to generate diverse and interesting theorems based on the idea of proof sketching (Jiang et al., 2022).

<sup>2</sup>We estimate whether a problem is a computational problem via a heuristic filter of whether the problem has any of the keywords: *prove, show, establish, demonstrate, verify*

The key idea is that we can leverage existing natural language solutions to identify core steps in a proof. We first train our Lean base model to take a natural language solution and auto-formalizing into a high-level proof, which we call a *proof sketch*, an example shown in Listing 1. In the proof sketch, core steps are represented via *have* statements, and lower-level details are omitted and left as *sorry* statements. We then filter sketches are then filtered by the Lean compiler to remove non-compiling sketches.

Once we have a set of compiling sketches, we extract each *sorry* goal into a new theorem via the `extract_goal` tactic, which turns it into a theorem that is equivalent to what needs to be proved at that particular *sorry*. For example, extracting the second *sorry* in Listing 1 results in the theorem shown in Listing 2. By extracting these *sorry* statements, we are able to generate 518K theorems.

```

theorem lean_workbook_plus_22532 (a b : ℕ → ℝ)
  (h₀ : 0 < a ∧ 0 < b)
  (h₁ : ∀ n, a (n + 1) = a n + 2)
  (h₂ : ∀ n, b (n + 1) = b n * 2)
  (h₃ : a 1 = 1)
  (h₄ : b 1 = 1)
  (h₅ : ∑ k in Finset.range 3, b k = 7) :
  ∑ k in Finset.range n, (a k * b k) = (2 * n - 3) * 2^n + 3 := by
  -- Lemma 1: Prove that the sequence {a_n} is an arithmetic sequence.
  have lemma1 : ∀ n, a (n + 1) = a n + 2 := by
    sorry

  -- Lemma 2: Express a_n in terms of n.
  have lemma2 : ∀ n, a n = 2 * n - 1 := by
    sorry

  -- Lemma 3: Express b_n in terms of n.
  have lemma3 : ∀ n, b n = 2^(n - 1) := by
    sorry

  -- Lemma 4: Calculate the sum of the first n terms of the sequence {a_n b_n}.
  have lemma4 : ∀ n, ∑ k in Finset.range n, (a k * b k) = (2 * n - 3) * 2^n + 3 := by
    sorry

  -- Apply lemma4 to conclude the theorem.
  exact lemma4 n

```

Listing 1: Example of a proof sketch

```

theorem lean_workbook_plus_22532.extracted_1_1 (a b : ℕ → ℝ) (h₀ : 0 < a ∧ 0 < b) (h₁ : ∀
  ↪ (n : ℕ), a (n + 1) = a n + 2)
  (h₂ : ∀ (n : ℕ), b (n + 1) = b n * 2) (h₃ : a 1 = 1) (h₄ : b 1 = 1) (h₅ : ∑ k ∈
  ↪ Finset.range 3, b k = 7)
  (lemma1 : ∀ (n : ℕ), a (n + 1) = a n + 2) (n : ℕ) : a n = 2 * ↑n - 1 := sorry

```

Listing 2: Example of an extracted theorem

**Fine-Tuning our Model for Proof Sketching** In order to fine-tune our model for proof sketching, we first curate a dataset of natural language problems (with corresponding Lean problem formalizations) and solutions by combining Goedel-Pset-v1 (Lin et al., 2025a) with NuminaMath-1.5

(LI et al., 2024). Then, we use Qwen-2.5-32B-Instruct to produce proof-sketches based on these natural language solutions similar to that in Listing 1. We filter out compiling sketches and train our Lean base model on them. In Table 4, we show the results of fine-tuning. Since it can be tricky to measure the objective correctness of a sketch, we use the proxy of compile rate, finding our model performs better than Qwen2.5-32B and is smaller and can do inference faster.

Table 4: Proof sketching ability of models

| Model                   | compile@1 | compile@16 |
|-------------------------|-----------|------------|
| Qwen2.5 7B (zero-shot)  | 3.6       | 7.0        |
| Qwen2.5 7B (one-shot)   | 4.9       | 19.0       |
| Qwen2.5 32B (zero-shot) | 21.1      | 62.0       |
| Qwen2.5 32B (one-shot)  | 35.1      | 75.0       |
| Ours (7B)               | 54.8      | 89.1       |

**Generating Proofs for Simplification** Because proof sketching can generate steps or sub-theorems that are too incremental, we first filter out trivial theorems that can be easily solved by automation tactics in Lean. For example, the first sorry in Listing 1 is just a restatement of hypothesis  $h_1$  and can be solved via `rfl`. While this theorem is correct, it is not challenging for the model. Therefore, we design an AUTO tactic (Listing 3) that tries a series of Lean automation tactics such as `linarith` and `aesop` to filter out these simple theorems, leaving 307K of the original 518K theorems (filtering out 41%).

For the remaining theorems, we attempt to generate proofs of these theorems with Goedel-Prover-V2-32B, a strong open-source proving model. With 4 attempts per theorem, the model is able to prove 145K theorems, which we use as targets for proof simplification. Statistics and examples of these proofs can be found in the next section, Appendix A.3.

```
macro "AUTO" : tactic =>
  '(tactic|
    repeat'
      (try rfl
        try tauto
        try assumption
        try norm_num
        try ring
        try ring_nf at *
        try ring_nf! at *
        try native_decide
        try omega
        try simp [*] at *
        try field_simp at *
        try positivity
        try linarith
        try nlinarith
        try exact?
        try aesop))
```

Listing 3: AUTO tactic for filtering trivial theorems

### A.3 Statistics of Proof Simplification Training Dataset

The minimum, Q1, median, Q3, and maximum proof lengths of our training dataset are 1, 103, 204, 411, and 10958. The mean is 334. In Fig. 8, we show the distribution of lengths, observing its right-skewed nature. Examples of proofs are shown in Listings 4 and 5. Compared to the proofs in our evaluation sets, we observe that training proofs often have more unused hypotheses, as they are derived from extracting the proof state, which may contain hypotheses that are not used for that particular sub-goal.

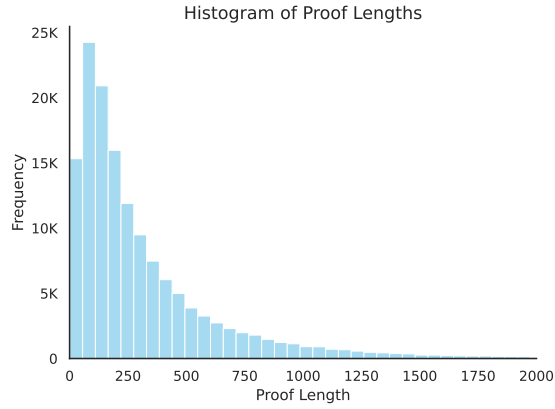

Figure 8: Histogram of proof lengths.

```

theorem extracted_1 (a b : ℝ) (ha : 0 ≤ a) (ha1 : a ≤ 1) (hb : b = a ^ 3 + 1 / (1 + a))
  (lemma1 : 1 - a + a ^ 2 - a ^ 3 ≤ 1 / (1 + a)) (lemma2 : b ≥ 1 - a + a ^ 2) (lemma3 : 1 - a
    ↔ + a ^ 2 ≥ 3 / 4)
  (lemma4 : b ≤ 3 / 2) : 3 / 4 < b := by
  have h_main : 3 / 4 < b := by
    by_contra h
    -- Assume for contradiction that b ≤ 3/4
    have h1 : b ≤ 3 / 4 := by linarith
    -- From lemma2, b ≥ 1 - a + a^2, and from lemma3, 1 - a + a^2 ≥ 3/4
    have h2 : 1 - a + a ^ 2 ≤ 3 / 4 := by
      linarith
    -- But from lemma3, 1 - a + a^2 ≥ 3/4, so 1 - a + a^2 = 3/4
    have h3 : 1 - a + a ^ 2 = 3 / 4 := by
      linarith
    -- Solve 1 - a + a^2 = 3/4 to get a = 1/2
    have h4 : a = 1 / 2 := by
      have h41 : a ^ 2 - a + 1 / 4 = 0 := by
        nlinarith
      have h42 : (a - 1 / 2) ^ 2 = 0 := by
        nlinarith
      have h43 : a - 1 / 2 = 0 := by
        nlinarith
      linarith
    -- Substitute a = 1/2 into b = a^3 + 1/(1 + a)
    have h5 : b = 19 / 24 := by
      rw [hb]
      rw [h4]
      norm_num
    -- But 19/24 > 3/4, so b > 3/4, contradiction
    have h6 : b > 3 / 4 := by
      rw [h5]
      norm_num
    linarith
  exact h_main

```

Listing 4: Example of Proof Simplification Training Task (Length 158)



```

theorem extracted_1 (n : ℕ) (hn : 3 ≤ n) (lemmal : Nat.card ↑{k | k ≤ n ∧ k ≠ 0} = n) :
  Nat.card ↑{k | k ≤ n - 1 ∧ k ≠ 0} = n - 1 := by
  have h_main : Nat.card ↑{k : ℕ | k ≤ n - 1 ∧ k ≠ 0} = n - 1 := by
    have h₁ : {k : ℕ | k ≤ n - 1 ∧ k ≠ 0} = Set.Icc 1 (n - 1) := by
      apply Set.ext
    intro k
    simp only [Set.mem_setOf_eq, Set.mem_Icc]
    constructor
  · intro h
    have h₂ : k ≤ n - 1 := h.1
    have h₃ : k ≠ 0 := h.2
    have h₄ : 1 ≤ k := by
      by_contra h₄
      -- If k < 1, then k = 0 since k is a natural number
      have h₅ : k = 0 := by
        omega
      contradiction
    exact ⟨h₄, h₂⟩
  · intro h
    have h₂ : 1 ≤ k := h.1
    have h₃ : k ≤ n - 1 := h.2
    have h₄ : k ≤ n - 1 := h₃
    have h₅ : k ≠ 0 := by
      by_contra h₅
      -- If k = 0, then 1 ≤ k would be false
      have h₆ : k = 0 := by simp using h₅
      omega
    exact ⟨h₄, h₅⟩
  rw [h₁]
  -- Calculate the cardinality of the set {1, ..., n - 1}
  have h₂ : Nat.card (Set.Icc 1 (n - 1) : Set ℕ) = n - 1 := by
    -- Use the fact that the cardinality of the interval [1, n - 1] is n - 1
    have h₃ : n - 1 ≥ 1 := by
      have h₄ : n ≥ 3 := hn
      omega
    -- Use the formula for the cardinality of the interval [a, b]
    rw [Nat.card_eq_fintype_card]
    -- Use the fact that the cardinality of the interval [1, n - 1] is n - 1
    rw [Fintype.card_ofFinset]
    -- Convert the set to a finset and calculate its cardinality
    <|> simp [Finset.Icc_eq_empty, Finset.card_range, Nat.succ_le_iff]
    <|> cases n with
    | zero => contradiction
    | succ n =>
      cases n with
      | zero => contradiction
      | succ n =>
        cases n with
        | zero => contradiction
        | succ n =>
          simp_all [Finset.Icc_eq_empty, Finset.card_range, Nat.succ_le_iff]
          <|> ring_nf at *
          <|> omega
  rw [h₂]
  exact h_main

```

Listing 5: Example of Proof Simplification Training Task (Length 295)

## B Training Metrics throughout RL

In Section 4.1, we observed that expert iteration leads to higher diversity as witnessed by better @32 metrics, while reinforcement learning with standard reinforcement learning algorithms maximizing expected rewards leads to higher @1 metrics. In Figure 9, we show the evolution of proof shortening  $\text{red}@1$  alongside  $\text{red}@32$ . Initial @32 metrics are slowly distilled into @1, but the improvement on @32 metrics is limited.

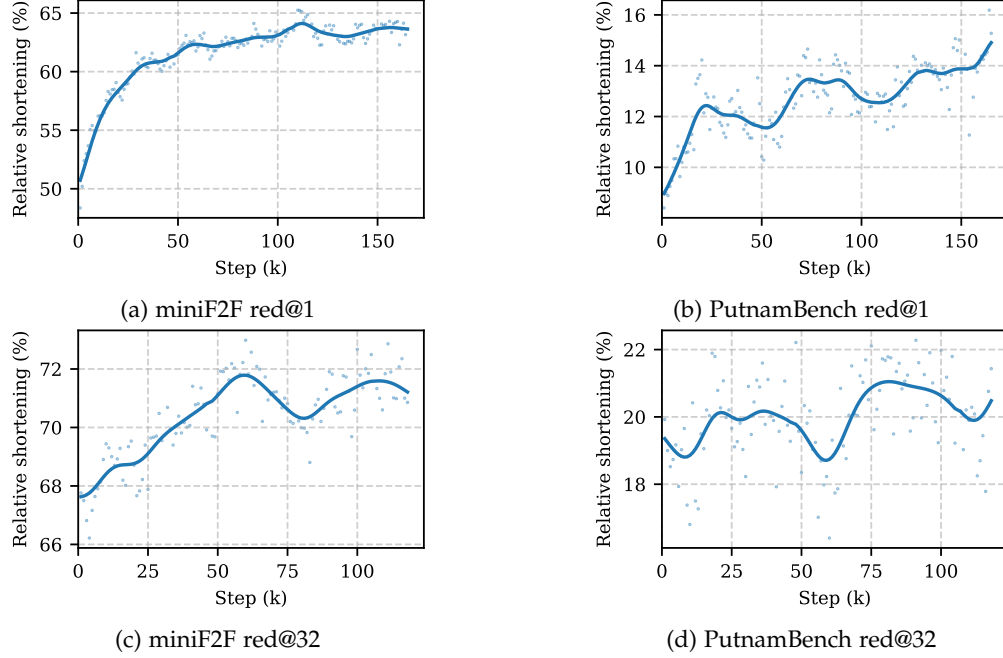

Figure 9: **Reduction metrics @1 and @32 over the course of RL.** GRPO maximizes  $\text{red}@1$  at the cost of diversity, as  $\text{red}@32$  only marginally increases in comparison.

## C Full Results and Extended Analysis of Iterative Proof Shortening

### C.1 Table of Iterative Proof Shortening Results

Table 5 is a tabular form of Fig. 4, showing the proof length after each iteration of proof shortening.

Table 5: Min@64 (rounded to nearest integer) and reduction (%) of miniF2F and PutnamBench proofs across inference-time iterations. Iterations 1 – 6 are done with 64 samples, and 7 – 8 with 1024 samples.

| Dataset | Model      | Orig | Lint | It 1 | It 2 | It 3 | It 4 | It 5 | It 6 | It 7* | It 8* |
|---------|------------|------|------|------|------|------|------|------|------|-------|-------|
| miniF2F | Min@64     | 334  | 302  | 144  | 126  | 121  | 117  | 106  | 104  | 88    | 75    |
|         | Red@64 (%) | 0.0  | 9.2  | 76.6 | 80.0 | 81.0 | 81.5 | 82.9 | 83.1 | 85.7  | 87.9  |
| Putnam  | Min@64     | 1468 | 1359 | 1123 | 1061 | 1024 | 1007 | 975  | 969  | 890   | 811   |
|         | Red@64 (%) | 0.0  | 7.4  | 34.8 | 40.0 | 42.5 | 43.6 | 46.4 | 47.1 | 52.2  | 57.2  |

### C.2 Effect of $k$ on min@ $k$ and red@ $k$ throughout simplification

In this section, we analyze the effect of increasing  $k$  on min@ $k$  and red@ $k$ . First, we analyze this trend when attempting to simplify the initial, linted proof, shown in Table 6 and Fig. 10. We observe a relatively log-linear gain in both metrics.

For comparison, we analyze the same trend but for simplifying proofs that have already gone many iterations of simplification. In Fig. 11, we analyze proofs that have gone 7 iterations of proof simplification. We see a different pattern, where min@ $k$  falls slower for lower  $k$  and then log-linearly afterwards. Intuitively, as proofs become more simplified, they become harder to simplify in a low-shot setting, and exploring more diverse simplifications becomes crucial.

Table 6: Min@ $k$  and Red@ $k$  for increasing values of  $k$

| Dataset     | Metric       | Original | Linter | @1    | @2    | @4    | @8    | @16   |
|-------------|--------------|----------|--------|-------|-------|-------|-------|-------|
| miniF2F     | Min@ $k$     | 334      | 302    | 142   | 141   | 139   | 137   | 134   |
|             | Red@ $k$ (%) | 0.0%     | 9.2%   | 77.1% | 77.3% | 77.7% | 78.1% | 78.6% |
| PutnamBench | Min@ $k$     | 1468     | 1359   | 1120  | 1117  | 1112  | 1105  | 1094  |
|             | Red@ $k$ (%) | 0.0%     | 7.4%   | 35.2% | 35.5% | 35.9% | 36.5% | 37.3% |

| Dataset     | Metric       | @32   | @64   | @128  | @256  | @512  | @1024 |
|-------------|--------------|-------|-------|-------|-------|-------|-------|
| miniF2F     | Min@ $k$     | 130   | 126   | 122   | 118   | 114   | 110   |
|             | Red@ $k$ (%) | 79.2% | 79.9% | 80.6% | 81.2% | 81.8% | 82.4% |
| PutnamBench | Min@ $k$     | 1080  | 1063  | 1043  | 1023  | 1004  | 987   |
|             | Red@ $k$ (%) | 38.4% | 39.7% | 41.3% | 42.9% | 44.3% | 45.7% |

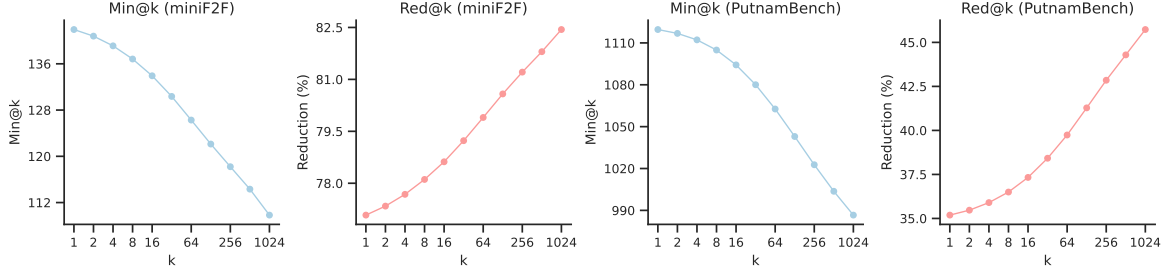

Figure 10: Effect of scaling  $k$  (sample count) on Min@ $k$  and Red@ $k$  (initial iteration)

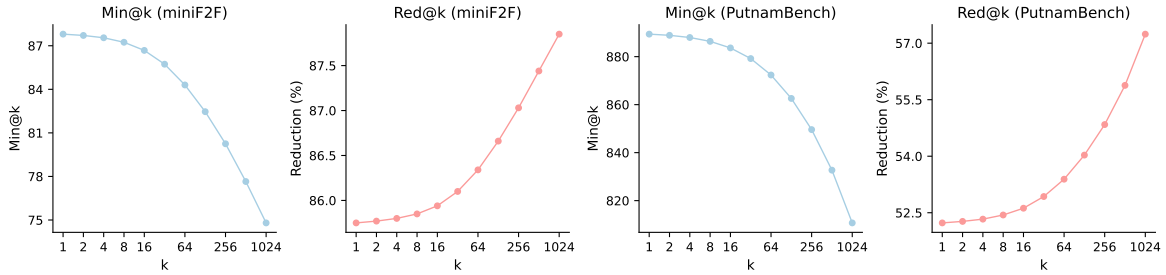

Figure 11: Effect of scaling  $k$  (sample count) on Min@ $k$  and Red@ $k$  (later iteration)

### C.3 Details on Seed-Prover IMO Proof Shortening

Earlier in 2025, Seed-Prover released Lean proofs of four problems that the model successfully solved from the 2025 International Mathematical Olympiad (IMO) (Chen et al., 2025). They solved problems 3, 4, and 5 were solved during the contest window, and problem 1 later after the competition. However, the proofs of these problems are extremely verbose, especially compared to their informal counterparts. Using iterative proof shortening, our ProofOptimizer is able to successfully reduce the proof length of their proofs for P3, P4, and P5 by over half, as well as the longer P1 by 43.8%. In addition, we find that our shortened proofs for P4 and P5 show a 25% and 81% (respectively) speedup over the original proofs (Table 7).

Table 7: Results for ProofOptimizer + Iterative Shortening on IMO 2025 Proof Simplification

| Problem | Length   |            |           | Runtime  |            |         |
|---------|----------|------------|-----------|----------|------------|---------|
|         | Original | Simplified | Reduction | Original | Simplified | Speedup |
| P1      | 36478    | 20506      | 43.79%    | 399.7    | 392.3      | 1.02×   |
| P3      | 16377    | 7907       | 51.72%    | 39.7     | 39.1       | 1.02×   |
| P4      | 29147    | 14531      | 50.15%    | 453.8    | 362.5      | 1.25×   |
| P5      | 8658     | 4002       | 53.78%    | 61.0     | 33.7       | 1.81×   |

We use proofs from the [official GitHub repository](#) using Mathlib 4.14.0 (our model was trained on Mathlib 4.19.0). Before shortening, we replace invocations of `exact?` and `apply?` with the actual proof that is found. Each of the proofs is divided into a collection of smaller lemmas and theorems (problems 1, 3, 4, and 5 have 80, 52, 88, and 14 theorems, respectively). Since

running iterative shortening on the entire proof will suffer from long context issues, we treat each sub-lemma/sub-theorem as an individual target for shortening. At the end, we combine the shortened theorems to produce the complete shortened proof. When feeding a sub-theorem into ProofOptimizer, we include as context the theorem definition (but not proof) of all other theorems that occur in its proof. Finally, to ensure the correctness of our simplified proofs, we use **SafeVerify** to confirm that all four simplified proofs match the specification of the original proof without any environmental manipulation. We remark that our setup does *not* consider the space of structure-level simplifications, as we retain all sub-theorem statements from the original proof and only simplify their proofs. In addition, as our proof length metric only measures the length of proofs, it does not take into account unnecessarily long or redundant sub-theorem statements.

As this experiment aims to provide a simple demonstration of the potential of our approach rather than perform a controlled scientific study, we do not fix the number of iterations or samples per iteration across problems. Approximately, we use 15-20 iterations of shortening with 64-4096 samples per iteration. Taking inspiration from the analysis in Sec. C.2, we generally use less samples for the first few iterations and increase the number of samples for later iterations to maximize reduction per sample. We also allocate more samples to sub-theorems that show more simplification potential in early iterations. In total, we used approximately 3000 H100 GPU hours per problem.

## D Comparison with Qwen2.5, GPT-4o, and Gemini-2.5-Pro

In Table 8, we compare *ProofOptimizer* models with several off the shelf models, namely Qwen 2.5 (Team, 2024), GPT-4o (Achiam et al., 2023), and Gemini-2.5-Pro (Comanici et al., 2025). For all models, we feed the output of the symbolic linter as input, and report overall reduction with respect to the *original (unlintered)* proof.

Table 8: **Proof length of miniF2F and PutnamBench proofs for various models.** Specially trained proof minimization models outperform prompted off-the-shelf models. Reinforcement learning achieves best @1 metrics but at the cost of reducing diversity, as witnessed by improved @32 metrics with expert iteration.

| Dataset         | Model                   | Min@1 | Min@32 | Red@1 | Red@32 |
|-----------------|-------------------------|-------|--------|-------|--------|
| miniF2F         | <i>Original</i>         | 334   |        | 0.0%  |        |
|                 | <i>Linter</i>           | 302   |        | 9.2%  |        |
|                 | Qwen2.5-Instruct 7B     | 294   | 267    | 25.7% | 41.8%  |
|                 | Qwen2.5-Instruct 32B    | 288   | 252    | 30.0% | 47.3%  |
|                 | GPT-4o                  | 283   | 258    | 35.2% | 47.9%  |
|                 | GPT-4o + States         | 266   | 290    | 32.9% | 46.5%  |
|                 | Gemini-2.5-Pro          | 280   | 207    | 31.6% | 62.0%  |
|                 | Gemini-2.5-Pro + States | 283   | 208    | 31.6% | 62.0%  |
|                 | ProofOptimizer-ExpIt    | 241   | 153    | 53.9% | 74.9%  |
|                 | ProofOptimizer-RL       | 190   | 152    | 67.1% | 73.4%  |
| Putnam<br>Bench | <i>Original</i>         | 1468  |        | 0.0%  |        |
|                 | <i>Linter</i>           | 1359  |        | 7.4%  |        |
|                 | Qwen2.5-Instruct 7B     | 1358  | 1339   | 9.0%  | 14.8%  |
|                 | Qwen2.5-Instruct 32B    | 1353  | 1304   | 10.9% | 20.7%  |
|                 | GPT-4o                  | 1355  | 1336   | 10.9% | 18.2%  |
|                 | GPT-4o + States         | 1379  | 1358   | 9.3%  | 15.9%  |
|                 | Gemini-2.5-Pro          | 1348  | 1303   | 12.7% | 24.5%  |
|                 | Gemini-2.5-Pro + States | 1371  | 1319   | 11.5% | 24.1%  |
|                 | ProofOptimizer-ExpIt    | 1328  | 1161   | 15.2% | 31.9%  |
|                 | ProofOptimizer-RL       | 1303  | 1258   | 21.6% | 27.1%  |

In Fig. 12, we compare the specific optimized proofs between Gemini and ProofOptimizer. For both data sets it can be seen that the longer the proof, the more challenging it is to shorten it. This is because although long proofs have more potential for shortening, the models struggle to maintain correctness of them. Still, ProofOptimizer is able to bring some improvements for the long proofs (see the top right part of the PutnamBench plot). In miniF2F, there is a significant number of proofs that can be minimized to just one step, which typically boils down to invoking one proof automation tactic (like `linarith` instead of applying a sequence of more explicit proof steps).

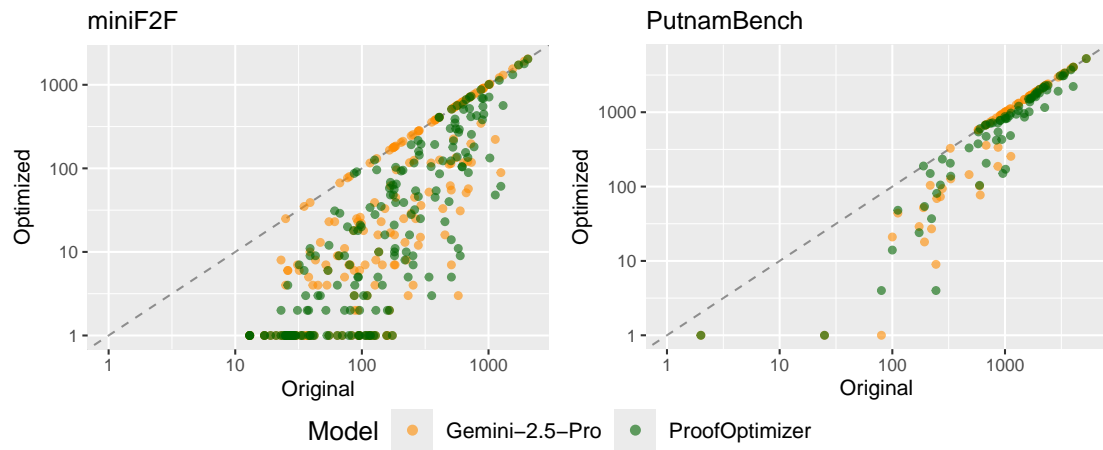

Figure 12: Comparison of optimized proofs between ProofOptimizer (green) and Gemini 2.5 Pro (yellow)

## E Full Results and Extended Analysis of Repair with Execution Feedback

This section contains the full results of the experiments in Sec. 4.2. All simplification attempts are done on the set of linted proofs. Table 9, Figure 13, and Figure 14 are extended versions of Fig. 3 for both PutnamBench and miniF2F. The settings are as follows:

- **ProofOptimizer**: *ProofOptimizer-ExpIt*, with 64 simplification attempts per proof.
- **+ Repair**: The previous setting, with 1 attempted repair by Goedel-Prover-V2-32B.
- **+ Repair + Linter**: The previous setting, with our linter applied to all proofs.
- **ProofOptimizer (@128)**: *ProofOptimizer-ExpIt*, with 128 simplification attempts per proof
- **ProofOptimizer (@64x2)**: *ProofOptimizer-ExpIt* with 64 simplification attempts per proof, and the best simplified proof for each problem is then fed back for an additional 64 attempts.

We remark that these baselines are normalizing for sample count rather than running time. Sampling a repair from Goedel-Prover-V2-32B takes considerably longer than sampling a simplification from our model. This is both because it is a larger model (32B vs. 7B) and because their model relies on CoT, causing their average response length to be significantly longer than ours.

Table 9: Results of execution-based repair strategies

| Dataset      | Model                  | Min@64 | Min@64 × 2 | Red@64 | Red@64 × 2 |
|--------------|------------------------|--------|------------|--------|------------|
| miniF2F      | <i>Linter</i>          | 302    |            | 9.2%   |            |
|              | ProofOptimizer         | 144    | -          | 75.5%  | -          |
|              | + Repair               | -      | 136        | -      | 77.3%      |
|              | + Repair + Linter      | -      | 132        | -      | 77.9%      |
|              | ProofOptimizer (@128)  | -      | 130        | -      | 78.9%      |
|              | ProofOptimizer (It 2)  | -      | 125        | -      | 80.2%      |
| Putnam Bench | <i>Linter</i>          | 1359   |            | 7.4%   |            |
|              | ProofOptimizer         | 1123   | -          | 32.9%  | -          |
|              | + Repair               | -      | 1113       | -      | 35.3%      |
|              | + Repair + Linter      | -      | 1107.2     | -      | 35.7%      |
|              | ProofOptimizer (@128)  | -      | 1099       | -      | 36.5%      |
|              | ProofOptimizer (@64x2) | -      | 1095       | -      | 37.0%      |



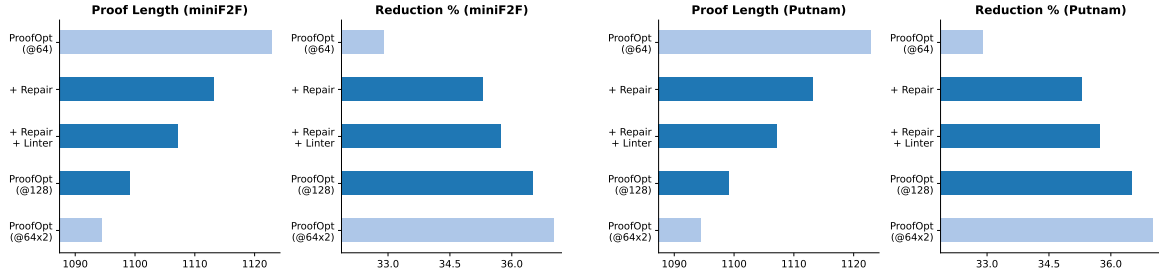

Figure 13: Results of Execution-Based Repair with Goedel-Prover

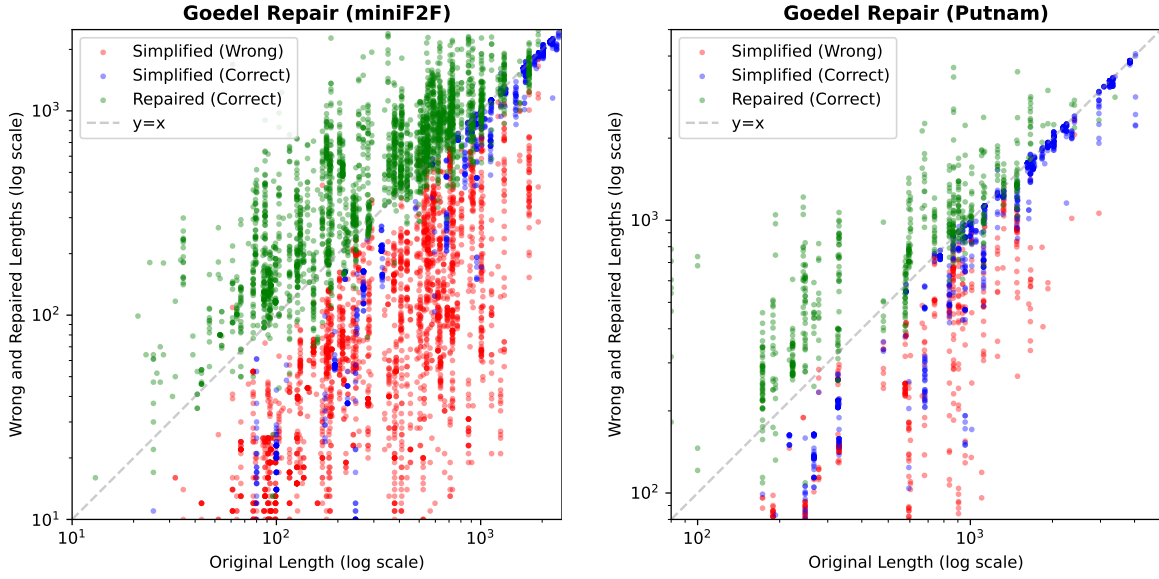

Figure 14: Comparison of Proof Lengths with Execution-Based Repair

Finally, in Listings 6 and 7, we show an example of a proof that was successfully repaired. Note that the repaired proof has many components in common with the original proof.

```

theorem mathd_numbertheory_314
  (r n : ℕ) (h₀ : r = 1342 % 13) (h₁ : 0 < n)
  (h₂ : 1342|n) (h₃ : n % 13 < r)
  : 6710 ≤ n := by
  have h_r : r = 3 := by rw [h₀]
  have h_main : 6710 ≤ n := by
    have h₄ : n % 13 < 3 := by
      rw [h_r] at h₃
    exact h₃
  obtain ⟨k, rfl⟩ := h₂
  have h₅ : 0 < k := by
    by_contra h
    push_neg at h
    have h₆ : k = 0 := by omega
    simp [h₆] at h₁
  by_contra! h₆
  have h₇ : k ≤ 4 := by
    by_contra h₈
    have h₉ : k ≥ 5 := by omega
    have h₁₀ : 1342 * k ≥ 1342 * 5 := by
      ↪ nlinarith
    omega
  interval_cases k <|> norm_num
  ↪ [Nat.mul_mod, Nat.add_mod,
    ↪ Nat.mod_mod] at h₄ ⊢
  exact h_main

```

Listing 6: Original Lean Proof (Length 126)

```

theorem mathd_numbertheory_314 -- Wrong
  (... statement omitted) := by
  rw [h₀] at h₃
  have : n % 13 < 3 := by omega
  obtain ⟨k, rfl⟩ := h₂
  omega

theorem mathd_numbertheory_314 -- Correct
  (... statement omitted) := by
  have h_r : r = 3 := by
    rw [h₀]
  <|> norm_num
  <|> rfl
  have h_main : 6710 ≤ n := by
    have h₄ : n % 13 < 3 := by
      rw [h_r] at h₃
    exact h₃
  obtain ⟨k, rfl⟩ := h₂
  by_contra! h
  have h₅ : k ≤ 4 := by
    omega
  interval_cases k <|> norm_num
  ↪ [Nat.mul_mod, Nat.add_mod,
    ↪ Nat.mod_mod] at h₄ ⊢ <|>
    (try omega) <|> (try contradiction)
  exact h_main

```

Listing 7: Wrong Simplification and Correct Repair (Length 93)

## F Evaluation Dataset Details

For our evaluation datasets, we use miniF2F and PutnamBench proofs sampled from Goedel-LM/Goedel-Prover-V2-32B. For miniF2F, we sample with temperature 1 and top-p 0.95. For PutnamBench, we use proofs provided by the team. In both cases, we take the shortest passing proof for each problem in Mathlib 4.19.0, resulting in 194 proofs for miniF2F and 75 proofs for PutnamBench. Table 10 and Figure 15 show summary statistics of our dataset. One sample from each dataset is shown in Listings 8 and 9.

As a sidenote, we observe a discrepancy in Goedel-Prover-V2-32B’s results with Lean versions. Upon testing their model, we measured 90% (pass@64) and 86 (pass@184) on miniF2F and PutnamBench with Mathlib 4.9, but only 80% (pass@64) and 75 (pass@184) with Mathlib 4.19. In this paper, we use Mathlib 4.19 rather than 4.9, as it is more recent and likely more useful to the Lean community.

Table 10: Summary statistics of proof lengths in evaluation dataset

| Dataset     | $n$ | Min | Q1  | Median | Q3   | Max  | Mean |
|-------------|-----|-----|-----|--------|------|------|------|
| MiniF2F     | 194 | 13  | 64  | 167    | 499  | 2980 | 334  |
| PutnamBench | 75  | 2   | 608 | 1179   | 2110 | 5420 | 1468 |

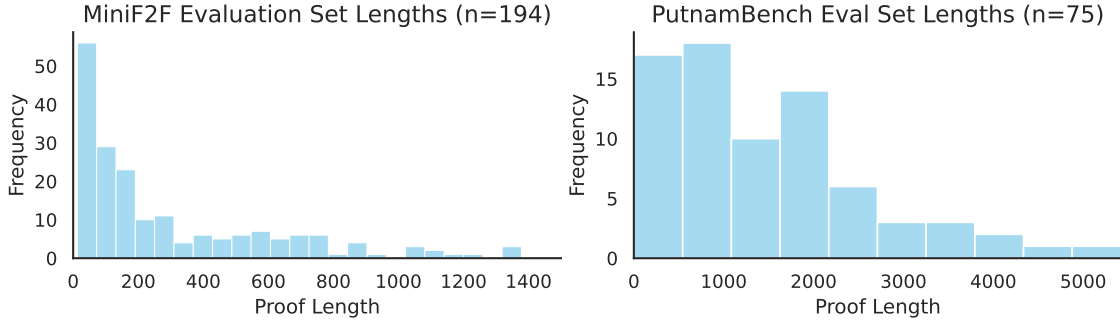

Figure 15: Histograms of proof lengths for our miniF2F and PutnamBench evaluation sets.

```

theorem mathd_numbertheory_185
  (n : ℕ)
  (h₀ : n % 5 = 3) :
  (2 * n) % 5 = 1 := by
  have h₁ : (2 * n) % 5 = 1 := by
    have h₂ : (2 * n) % 5 = (2 * (n % 5)) % 5 := by
      simp [Nat.mul_mod, Nat.mod_mod]
    <=> ring_nf at *
    <=> omega
  rw [h₂]
  rw [h₀]
  <=> norm_num
  <=> rfl

exact h₁

```

Listing 8: Example of miniF2F Eval Task (Length 65)

```

theorem putnam_1993_a2
(x : ℕ → ℝ)
(xnonzero : ∀ n : ℕ, x n ≠ 0)
(hx : ∀ n ≥ 1, (x n) ^ 2 - x (n - 1) * x (n + 1) = 1)
: ∃ a : ℝ, ∀ n ≥ 1, x (n + 1) = a * x n - x (n - 1) := by
  have h_main : ∀ (n : ℕ), n ≥ 1 → (x (n + 1) + x (n - 1)) / x n = (x 2 + x 0) / x 1 := by
    intro n hn
    have h1 : ∀ (n : ℕ), n ≥ 1 → (x (n + 1) + x (n - 1)) / x n = (x (n + 2) + x n) / x (n +
      ↪ 1) := by
      intro n hn
      have h2 : (x (n + 1)) ^ 2 - x n * x (n + 2) = 1 := by
        have h3 := hx (n + 1) (by linarith)
        simp [Nat.add_assoc] using h3
      have h3 : (x n) ^ 2 - x (n - 1) * x (n + 1) = 1 := hx n hn
      have h4 : x (n + 2) * x n + (x n) ^ 2 - (x (n + 1)) ^ 2 - x (n - 1) * x (n + 1) = 0 := by
        linarith
      have h5 : (x (n + 2) + x n) * x n - (x (n + 1) + x (n - 1)) * x (n + 1) = 0 := by
        ring_nf at h4 ⊢
        linarith
      have h6 : x n ≠ 0 := xnonzero n
      have h7 : x (n + 1) ≠ 0 := xnonzero (n + 1)
      have h8 : (x (n + 2) + x n) / x (n + 1) - (x (n + 1) + x (n - 1)) / x n = 0 := by
        field_simp [h6, h7] at h5 ⊢
        nlinarith
      linarith

  have h2 : ∀ (n : ℕ), n ≥ 1 → (x (n + 1) + x (n - 1)) / x n = (x 2 + x 0) / x 1 := by
    intro n hn
    induction' hn with n hn IH
    · norm_num
    · have h3 := h1 n hn
      have h4 := h1 (n + 1) (by linarith)
      simp [Nat.add_assoc] at h3 h4 ⊢
      <|>
      (try norm_num at * <|>
      try linarith) <|>
      (try simp_all [Nat.add_assoc]) <|>
      (try ring_nf at * <|>
      try linarith) <|>
      (try field_simp [xnonzero] at * <|>
      try nlinarith)
      <|>
      linarith
    exact h2 n hn

  have h_exists_a : ∃ (a : ℝ), ∀ (n : ℕ), n ≥ 1 → x (n + 1) = a * x n - x (n - 1) := by
    use (x 2 + x 0) / x 1
    intro n hn
    have h1 : (x (n + 1) + x (n - 1)) / x n = (x 2 + x 0) / x 1 := h_main n hn
    have h2 : x n ≠ 0 := xnonzero n
    have h3 : (x (n + 1) + x (n - 1)) / x n = (x 2 + x 0) / x 1 := by rw [h1]
    have h4 : x (n + 1) + x (n - 1) = ((x 2 + x 0) / x 1) * x n := by
      field_simp [h2] at h3 ⊢
      <|> nlinarith
    have h5 : x (n + 1) = ((x 2 + x 0) / x 1) * x n - x (n - 1) := by linarith
    exact h5

  exact h_exists_a

```

Listing 9: Example of PutnamBench Eval Task (Length 715)

## G Examples of Proofs Simplified by ProofOptimizer

In Listings 10 to 17, we show proofs successfully optimized with ProofOptimizer and iterative shortening. Some proofs were syntactically modified to fit on the page (new lines removed, multiple lines compressed into one).

```
theorem mathd_algebra_338 -- Original Proof
(a b c : ℝ)
(h₀ : 3 * a + b + c = -3)
(h₁ : a + 3 * b + c = 9)
(h₂ : a + b + 3 * c = 19) :
a * b * c = -56 := by
have h₃ : b = a + 6 := by
  have h₃₁ : -a + b = 6 := by
    have h₃₂ : (a + 3 * b + c) - (3 * a + b
    ↪ + c) = 9 - (-3) := by
      linarith
    linarith
  linarith

have h₄ : c = a + 11 := by
  have h₄₁ : -a + c = 11 := by
    have h₄₂ : (a + b + 3 * c) - (3 * a + b
    ↪ + c) = 19 - (-3) := by
      linarith
    linarith
  linarith

have h₅ : a = -4 := by
  have h₅₁ : 3 * a + b + c = -3 := h₀
  rw [h₃, h₄] at h₅₁
  ring_nf at h₅₁
  linarith

have h₆ : b = 2 := by
  rw [h₃]
  rw [h₅]
  <|> norm_num

have h₇ : c = 7 := by
  rw [h₄]
  rw [h₅]
  <|> norm_num

have h₈ : a * b * c = -56 := by
  rw [h₅, h₆, h₇]
  <|> norm_num

exact h₈
```

Listing 10: Original Proof (Length 214)

```
theorem mathd_algebra_338
(a b c : ℝ)
(h₀ : 3 * a + b + c = -3)
(h₁ : a + 3 * b + c = 9)
(h₂ : a + b + 3 * c = 19) :
a * b * c = -56 := by
  have : a = -4 := by linarith
  subst_vars
  nlinarith
```

Listing 11: Simplified Proof (Length 11)

```

theorem putnam_2015_a2
(a : ℕ → ℤ)
(abase : a 0 = 1 ∧ a 1 = 2)
(arec : ∀ n ≥ 2, a n = 4 * a (n - 1) - a (n - 2))
: Odd ((181) : ℕ) ∧ ((181) : ℕ).Prime ∧ (((181) : ℕ) : ℤ) | a 2015 := by
  constructor
  · decide
  constructor
  · norm_num [Nat.Prime]
  have h₁ : ∀ n : ℕ, (a (n + 10) : ℤ) ≡ - (a n : ℤ) [ZMOD 181] := by
    intro n
    induction' n using Nat.strong_induction_on with n ih
    rcases n with (| _ | _ | _ | _ | _ | _ | _ | _ | _ | n) <|>
    simp_all [Int.ModEq, abase, arec] <|> omega
  have h₂ : (a 5 : ℤ) ≡ 0 [ZMOD 181] := by norm_num [Int.ModEq, abase, arec]
  have h₃ : (a 2015 : ℤ) ≡ 0 [ZMOD 181] := by
    have h₄ : ∀ k : ℕ, (a (10 * k + 5) : ℤ) ≡ 0 [ZMOD 181] := by
      intro k
      induction' k with k ih
      · norm_num [Int.ModEq] at h₂ ⊢
        <|> simp [abase, arec] using h₂
      · have h₅ := h₁ (10 * k + 5)
        have h₆ := h₁ (10 * k + 6)
        have h₇ := h₁ (10 * k + 7)
        have h₈ := h₁ (10 * k + 8)
        have h₉ := h₁ (10 * k + 9)
        have h₁₀ := h₁ (10 * k + 10)
        norm_num [Int.ModEq] at h₅ h₆ h₇ h₈ h₉ h₁₀ ih ⊢
        <|> ring_nf at * <|> omega
    have h₅ : (a 2015 : ℤ) ≡ 0 [ZMOD 181] := by
      have h₆ : (a (10 * 201 + 5) : ℤ) ≡ 0 [ZMOD 181] := h₄ 201
      norm_num at h₆ ⊢
      <|> simp [add_assoc] using h₆
    exact h₅
  exact Int.dvd_of_emod_eq_zero h₃

```

Listing 12: Original Proof (Length 324)

```

theorem putnam_2015_a2
(a : ℕ → ℤ)
(abase : a 0 = 1 ∧ a 1 = 2)
(arec : ∀ n ≥ 2, a n = 4 * a (n - 1) - a (n - 2))
: Odd ((181) : ℕ) ∧ ((181) : ℕ).Prime ∧ (((181) : ℕ) : ℤ) | a 2015 := by
  constructor
  · decide
  constructor
  · norm_num [Nat.Prime]
  rw [show 2015 = 10 * 201 + 5 by norm_num]
  have h₁ : ∀ n : ℕ, a (10 * n + 5) ≡ 0 [ZMOD 181] := by
    intro n
    induction' n with k ih
    · norm_num [abase, arec, Int.ModEq]
    · rw [Nat.mul_succ]
      simp_all [Int.ModEq, arec]
      omega
  have h₂ := h₁ 201
  exact Int.dvd_of_emod_eq_zero h₂

```

Listing 13: Simplified Proof (Length 82)

```

theorem imo_1960_p2
(x : ℝ)
(h₀ : 0 ≤ 1 + 2 * x)
(h₁ : (1 - Real.sqrt (1 + 2 * x))^2 ≠ 0)
(h₂ : (4 * x^2) / (1 - Real.sqrt (1 + 2*x))^2 < 2*x + 9)
(h₃ : x ≠ 0) :
-(1 / 2) ≤ x ∧ x < 45 / 8 := by
constructor
· nlinarith [sq_nonneg (x + 1 / 2)]
· set s := Real.sqrt (1 + 2 * x) with hs
  have h₅₁ : 0 ≤ 1 + 2 * x := h₀
  have h₅₂ : s ≥ 0 := Real.sqrt_nonneg _
  have h₅₃ : s ^ 2 = 1 + 2 * x := by
    rw [hs]
    rw [Real.sq_sqrt] <|> linarith
  have h₅₄ : (1 - s) ^ 2 ≠ 0 := by simpa [hs] using h₁
  have h₅₅ : s ≠ 1 := by
    intro h
    have h₅₅₁ : (1 - s) ^ 2 = 0 := by
      rw [h]
      norm_num
    contradiction
  have h₅₆ : (s + 1) ^ 2 * (s - 1) ^ 2 = (s ^ 2 - 1) ^ 2 := by
    ring
  have h₅₇ : (s ^ 2 - 1 : ℝ) ^ 2 = 4 * x ^ 2 := by
    rw [h₅₃]
    ring
  have h₅₈ : (4 : ℝ) * x ^ 2 / (s - 1) ^ 2 = (s + 1) ^ 2 := by
    have h₅₈₁ : (s - 1 : ℝ) ^ 2 ≠ 0 := by
      intro h
      have h₅₈₂ : (1 - s : ℝ) ^ 2 = 0 := by
        calc
          (1 - s : ℝ) ^ 2 = (s - 1 : ℝ) ^ 2 := by ring
          _ = 0 := by rw [h]
      contradiction
    field_simp [h₅₈₁] at h₅₇
    nlinarith
  have h₅₉ : (4 : ℝ) * x ^ 2 / (1 - s) ^ 2 = (s + 1) ^ 2 := by
    rw [← h₅₈]
    ring
  nlinarith [sq_nonneg (s - 1)]

```

Listing 14: Original Proof (Length 330)

```

theorem imo_1960_p2
(x : ℝ)
(h₀ : 0 ≤ 1 + 2 * x)
(h₁ : (1 - Real.sqrt (1 + 2 * x))^2 ≠ 0)
(h₂ : (4 * x^2) / (1 - Real.sqrt (1 + 2*x))^2 < 2*x + 9)
(h₃ : x ≠ 0) :
-(1 / 2) ≤ x ∧ x < 45 / 8 := by
constructor
· nlinarith [sq_nonneg (x + 1 / 2)]
· have h₅₇ : (4 : ℝ) * x ^ 2 / (1 - Real.sqrt (1 + 2 * x)) ^ 2 = (1 + Real.sqrt (1 + 2 *
  ↪ x)) ^ 2 := by
    have h₅₈ : (1 - Real.sqrt (1 + 2 * x)) ^ 2 ≠ 0 := by assumption
    field_simp [h₅₈]
    nlinarith [sq_sqrt (show 0 ≤ 1 + 2 * x by assumption)]
  nlinarith [sq_sqrt (show 0 ≤ 1 + 2 * x by assumption),
    Real.sqrt_nonneg (1 + 2 * x)]

```

Listing 15: Simplified Proof (Length 125)

```

theorem putnam_1990_a1
  (T : ℕ → ℤ)
  (hT012 : T 0 = 2 ∧ T 1 = 3 ∧ T 2 = 6)
  (hTn : ∀ n, T (n + 3) = (n + 7) * T (n + 2) - 4 * (n + 3) * T (n + 1) + (4 * n + 4) * T n) :
  T = ((fun n : ℕ => (n)! , fun n : ℕ => 2 ^ n) : (ℕ → ℤ) × (ℕ → ℤ)).1 + ((fun n : ℕ => (n)!, fun n : ℕ => 2 ^ n) : (ℕ → ℤ) × (ℕ → ℤ)
  ↪> ).2 := by
  by
  have h_main : ∀ (n : ℕ), T n = (n ! : ℤ) + 2 ^ n := by
    intro n
    have h1 : T n = (n ! : ℤ) + 2 ^ n := by
      have h2 : ∀ n : ℕ, T n = (n ! : ℤ) + 2 ^ n := by
        intro n
        induction n using Nat.strong_induction_on with
        | h n ih =>
          match n with
          | 0 =>
            norm_num [hT012]
            <|>
            simp_all [Nat.factorial]
            <|>
            norm_num
          | 1 =>
            norm_num [hT012]
            <|>
            simp_all [Nat.factorial]
            <|>
            norm_num
          | 2 =>
            norm_num [hT012]
            <|>
            simp_all [Nat.factorial]
            <|>
            norm_num
          | n + 3 =>
            have h3 := hTn n
            have h4 := ih n (by omega)
            have h5 := ih (n + 1) (by omega)
            have h6 := ih (n + 2) (by omega)
            simp [h4, h5, h6, pow_add, pow_one, Nat.factorial_succ, Nat.mul_add, Nat.add_mul] at h3 ⊢
            <|>
            ring_nf at h3 ⊢ <|>
            norm_cast at h3 ⊢ <|>
            simp_all [Nat.factorial_succ, pow_add, pow_one, mul_assoc]
            <|>
            ring_nf at * <|>
            norm_num at * <|>
            nlinarith
        exact h2 n
      exact h1
    have h_final : T = ((fun n : ℕ => (n)! , fun n : ℕ => 2 ^ n) : (ℕ → ℤ) × (ℕ → ℤ)).1 + ((fun n : ℕ => (n)!, fun n : ℕ => 2 ^ n) : (ℕ → ℤ) ×
    ↪> (ℕ → ℤ)).2 := by
      funext n
      have h1 : T n = (n ! : ℤ) + 2 ^ n := h_main n
      simp [h1, Pi.add_apply]
      <|> norm_cast <|> simp [Nat.cast_add] <|> ring_nf
      apply h_final

```

```

theorem putnam_1990_a1
  (T : ℕ → ℤ)
  (hT012 : T 0 = 2 ∧ T 1 = 3 ∧ T 2 = 6)
  (hTn : ∀ n, T (n + 3) = (n + 7) * T (n + 2) - 4 * (n + 3) * T (n + 1) + (4 * n + 4) * T n)
  ↪> :
  T = ((fun n : ℕ => (n)! , fun n : ℕ => 2 ^ n) : (ℕ → ℤ) × (ℕ → ℤ)).1 + ((fun n : ℕ =>
  ↪> (n)!, fun n : ℕ => 2 ^ n) : (ℕ → ℤ) × (ℕ → ℤ)).2 := by
  ext n
  induction' n using Nat.strong_induction_on with n ih
  match n with
  | 0 => simp_all
  | 1 => simp_all
  | 2 => simp_all
  | n + 3 =>
    simp_all [Nat.factorial_succ]
    ring_nf

```

Listing 16: Original Proof (Length 320) and Simplified Proof (Length 34)



```

theorem putnam_1968_a1
: 22/7 - Real.pi = ∫ x in (0)..1, x^4 * (1 - x)^4 / (1 + x^2) := by
have h_main : (∫ x in (0)..1, x^4 * (1 - x)^4 / (1 + x^2)) = 22/7 - Real.pi := by
have h1 : (∫ x in (0)..1, x^4 * (1 - x)^4 / (1 + x^2)) = (∫ x in (0)..1, (x^6 - 4*x^5 + 5*x^4 - 4*x^2 + 4 : ℝ) - 4 / (1 + x^2)) := by
have h11 : ∀ (x : ℝ), x^4 * (1 - x)^4 / (1 + x^2) = (x^6 - 4*x^5 + 5*x^4 - 4*x^2 + 4 : ℝ) - 4 / (1 + x^2) := by
  intro x
  have h12 : (1 + x^2 : ℝ) ≠ 0 := by nlinarith
  have h13 : x^4 * (1 - x)^4 = (x^6 - 4*x^5 + 5*x^4 - 4*x^2 + 4 : ℝ) * (1 + x^2) - 4 := by
    ring_nf <|> nlinarith [sq_nonneg (x ^ 2), sq_nonneg (x ^ 3), sq_nonneg (x - 1), sq_nonneg (x + 1)]
  have h14 : x^4 * (1 - x)^4 / (1 + x^2) = ((x^6 - 4*x^5 + 5*x^4 - 4*x^2 + 4 : ℝ) * (1 + x^2) - 4) / (1 + x^2) := by
    rw [h13]
    rw [h14]
  field_simp [h12] <|> ring_nf <|> field_simp [h12] <|> ring_nf
  congr
  ext x
  rw [h11 x]
  rw [h1]
have h2 : (∫ x in (0)..1, (x^6 - 4*x^5 + 5*x^4 - 4*x^2 + 4 : ℝ) - 4 / (1 + x^2)) = (∫ x in (0)..1, (x^6 - 4*x^5 + 5*x^4 - 4*x^2 + 4 : ℝ)) - (∫ x
  ↪ in (0)..1, (4 : ℝ) / (1 + x^2)) := by
  apply intervalIntegral.integral_sub
  · apply Continuous.intervalIntegrable
    continuity
  · apply Continuous.intervalIntegrable
    have h3 : Continuous (fun x : ℝ => (4 : ℝ) / (1 + x ^ 2)) := by
      apply Continuous.div
      · exact continuous_const
      · exact Continuous.add continuous_const (continuous_pow 2)
    intro x
    have h4 : (1 + x ^ 2 : ℝ) ≠ 0 := by nlinarith
    exact h4
  exact h3
  rw [h2]
have h3 : (∫ x in (0)..1, (x^6 - 4*x^5 + 5*x^4 - 4*x^2 + 4 : ℝ)) = (22 / 7 : ℝ) := by
  norm_num [integral_id, mul_comm] <|> ring_nf <|> norm_num <|> linarith [Real.pi_pos]
have h4 : (∫ x in (0)..1, (4 : ℝ) / (1 + x^2)) = Real.pi := by
have h41 : (∫ x in (0)..1, (4 : ℝ) / (1 + x ^ 2)) = 4 * (∫ x in (0)..1, (1 : ℝ) / (1 + x ^ 2)) := by
have h42 : (∫ x in (0)..1, (4 : ℝ) / (1 + x ^ 2)) = (∫ x in (0)..1, 4 * (1 : ℝ) / (1 + x ^ 2)) := by
  congr
  ext x <|> ring_nf
  rw [h42]
have h43 : (∫ x in (0)..1, 4 * (1 : ℝ) / (1 + x ^ 2)) = 4 * (∫ x in (0)..1, (1 : ℝ) / (1 + x ^ 2)) := by
  simp [intervalIntegral.integral_comp_mul_left (fun x => (1 : ℝ) / (1 + x ^ 2))] <|>
  norm_num <|> field_simp <|> ring_nf <|> norm_num <|> linarith [Real.pi_pos]
  rw [h43]
  rw [h41]
have h44 : (∫ x in (0)..1, (1 : ℝ) / (1 + x ^ 2)) = Real.pi / 4 := by
have h45 : (∫ x in (0)..1, (1 : ℝ) / (1 + x ^ 2)) = Real.arctan 1 - Real.arctan 0 := by
  rw [integral_one_div_one_add_sq] <|> norm_num
  rw [h45]
have h46 : Real.arctan 1 = Real.pi / 4 := by
  norm_num [Real.arctan_one]
have h47 : Real.arctan 0 = 0 := by
  norm_num [Real.arctan_zero]
  rw [h46, h47] <|> ring_nf <|> norm_num
  rw [h44] <|> ring_nf <|> norm_num
  rw [h3, h4] <|> ring_nf <|> norm_num
have h_final : 22/7 - Real.pi = ∫ x in (0)..1, x^4 * (1 - x)^4 / (1 + x^2) := by
  rw [h_main] <|> linarith [Real.pi_pos]
exact h_final

```

```

theorem putnam_1968_a1
: 22/7 - Real.pi = ∫ x in (0)..1, x^4 * (1 - x)^4 / (1 + x^2) := by
  simp_rw [show ∀ x : ℝ, x ^ 4 * (1 - x) ^ 4 / (1 + x ^ 2) = (x ^ 6 - 4 * x ^ 5 + 5 * x ^ 4 - 4 *
    ↪ x ^ 2 + 4 - 4 / (1 + x ^ 2)) by
    intro x
    field_simp
    ring]
  ring_nf
  norm_num
  <|> linarith [Real.pi_pos]

```

Listing 17: Original Proof (Length 1097) and Simplified Proof (Length 76)

## H Proof Speedup and Slowdown Analysis and Examples

### H.1 Iterative Proof Shortening Results with Heartbeat Metric

Table 11 and Fig. 16 show the results of iterative proof shortening using proof length vs. heartbeats as optimization metrics. Observe that while optimizing for heartbeats isn’t nearly as effective for proof length, it still leads to considerable simplification.

Table 11: Comparison of Min@64 (rounded to nearest integer), reduction (%), Heartbeats@64 (in thousands), and reduction (%) across inference-time iterations for miniF2F and PutnamBench proofs. Iterations 1–6 use 64 samples, and 7–8 use 1024 samples. The first group shows the standard (length-optimized) setting; the second group shows the new (heartbeat-optimized) experiment.

| Dataset | Metric                           | Orig | Lint | It 1 | It 2 | It 3 | It 4 | It 5 | It 6 | It 7* | It 8* |
|---------|----------------------------------|------|------|------|------|------|------|------|------|-------|-------|
| miniF2F | <i>Optimizing for Length</i>     |      |      |      |      |      |      |      |      |       |       |
|         | Min@64                           | 334  | 302  | 144  | 126  | 121  | 117  | 106  | 104  | 88    | 75    |
|         | Red@64 (%)                       | 0.0  | 9.2  | 76.6 | 80.0 | 81.0 | 81.5 | 82.9 | 83.1 | 85.7  | 87.9  |
|         | <i>Optimizing for Heartbeats</i> |      |      |      |      |      |      |      |      |       |       |
|         | Min@64                           | 334  | 302  | 163  | 145  | 139  | 135  | 129  | 125  | 112   | 96    |
|         | Red@64 (%)                       | 0.0  | 9.2  | 71.3 | 74.8 | 75.8 | 76.3 | 76.9 | 77.4 | 79.0  | 81.3  |
|         | HB@64 (K)                        | 36.3 | 36.2 | 14.5 | 13.6 | 13.3 | 13.2 | 13.0 | 12.8 | 11.9  | 10.4  |
|         | HB Red@64                        | 0.0  | 0.2  | 43.3 | 46.7 | 48.2 | 48.5 | 48.8 | 49.6 | 51.5  | 57.0  |
| Putnam  | <i>Optimizing for Length</i>     |      |      |      |      |      |      |      |      |       |       |
|         | Min@64                           | 1468 | 1359 | 1123 | 1061 | 1024 | 1007 | 975  | 969  | 890   | 811   |
|         | Red@64 (%)                       | 0.0  | 7.4  | 34.8 | 40.0 | 42.5 | 43.6 | 46.4 | 47.1 | 52.2  | 57.2  |
|         | <i>Optimizing for Heartbeats</i> |      |      |      |      |      |      |      |      |       |       |
|         | Min@64                           | 1468 | 1359 | 1142 | 1092 | 1060 | 1043 | 1034 | 1031 | 974   | 904   |
|         | Red@64 (%)                       | 0.0  | 7.4  | 32.2 | 36.2 | 38.7 | 39.7 | 40.5 | 40.8 | 44.0  | 49.2  |
|         | HB@64 (K)                        | 221  | 219  | 199  | 157  | 155  | 140  | 136  | 136  | 122   | 111   |
|         | HB Red@64                        | 0.0  | 0.7  | 18.5 | 23.9 | 26.9 | 28.4 | 29.5 | 29.6 | 34.0  | 39.5  |

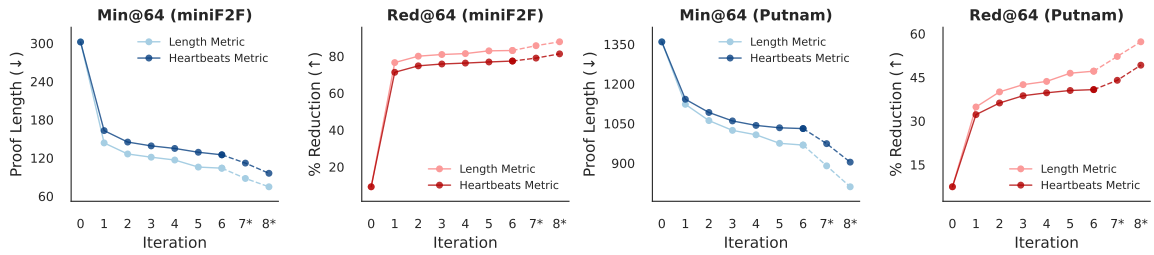

Figure 16: Optimizing for length vs. heartbeats

## H.2 Examples of Proof Speedup and Slowdown after Simplification

We analyze two examples of proof speedup and slowdown. In Listing 18, we observe that the original proof uses an extraneous amount of tactics within `nlinarith` in order to prove the main conjecture. By removing a majority of these, the simplified proof achieves a 4.7x speedup. In Listing 19, we observe a more extreme case, where the original proof is significantly overcomplicated and can be reduced to one `omega` invocation. `Goedel-Prover-V2-32B` never found this single-tactic proof (with 64 samples) and instead produces proofs with many unnecessary subgoals, leading to a proof with slow execution time.

In several occurrences, we observe that simplified proofs can be significantly slower than the original proof. This is usually because the simplified proof is notationally shorter, but uses a slower approach to complete the proof. For example, in Listing 20, `ProofOptimizer` finds a shorter proof, but the proof is reliant on `simp_all`, `Finset.sum.range.succ`, and `linarith`, which expand the goal into large proof terms that are time-consuming, causing the new proof to be over 10x slower. Another example is shown in Listing 21. Here, the original proof first iterates over all  $m \leq 71$  with `interval_cases m`, tries to simplify using `omega`, and then iterates over all  $n \leq 71$  with `interval_cases n`. `ProofOptimizer`, however, removes the `try omega`, directly doing an exhaustive search over  $(m, n)$ . The `try omega` statement in the original proof made it much faster, removing 69 of the 71 goals, whereas the simplified proof had to iterate through  $n$  for these goals.

```

theorem imo_1983_p6 -- Original Proof, Time: 5.57s
  (a b c : ℝ)
  (h0 : 0 < a ∧ 0 < b ∧ 0 < c)
  (h1 : c < a + b)
  (h2 : b < a + c)
  (h3 : a < b + c) :
  0 ≤ a^2 * b * (a - b) + b^2 * c * (b - c) + c^2 * a * (c - a) := by
  have h_main : 0 ≤ a^2 * b * (a - b) + b^2 * c * (b - c) + c^2 * a * (c - a) := by
    nlinarith [sq_nonneg (a - b), sq_nonneg (b - c), sq_nonneg (c - a),
      mul_nonneg h0.1.le h0.2.1.le, mul_nonneg h0.2.1.le h0.2.2.le, mul_nonneg h0.2.2.le
        ↪ h0.1.le,
      mul_nonneg (sq_nonneg (a - b)) h0.2.2.le, mul_nonneg (sq_nonneg (b - c)) h0.1.le,
      mul_nonneg (sq_nonneg (c - a)) h0.2.1.le, mul_pos h0.1 h0.2.1, mul_pos h0.2.1 h0.2.2,
      mul_pos h0.2.2 h0.1, mul_pos (sub_pos.mpr h1) (sub_pos.mpr h2),
      mul_pos (sub_pos.mpr h2) (sub_pos.mpr h3), mul_pos (sub_pos.mpr h3) (sub_pos.mpr h1),
      sq_nonneg (a + b - 2 * c), sq_nonneg (b + c - 2 * a), sq_nonneg (c + a - 2 * b)]
  exact h_main

theorem imo_1983_p6 -- Simplified Proof, Time: 1.20s
  (a b c : ℝ)
  (h0 : 0 < a ∧ 0 < b ∧ 0 < c)
  (h1 : c < a + b)
  (h2 : b < a + c)
  (h3 : a < b + c) :
  0 ≤ a^2 * b * (a - b) + b^2 * c * (b - c) + c^2 * a * (c - a) := by
  nlinarith [mul_pos (sub_pos.mpr h1) (sub_pos.mpr h2), mul_pos (sub_pos.mpr h2) (sub_pos.mpr
    ↪ h3), mul_pos (sub_pos.mpr h3) (sub_pos.mpr h1), sq_nonneg (a - b), sq_nonneg (b - c),
    ↪ sq_nonneg (c - a)]

```

Listing 18: Example of Speedup after Simplification (orig: 5.6s, new: 1.2s)

```

theorem mathd_numbertheory_765 -- Original Proof, Time: 2.50s
(x : ℤ)
(h₀ : x < 0)
(h₁ : (24 * x) % 1199 = 15) :
x ≤ -449 := by
have h_main : x ≤ -449 := by
  by_contra! h
  have h₂ : -448 ≤ x := by linarith
  have h₃ : x < 0 := h₀
  have h₄ : (24 * x) % 1199 = 15 := h₁
  have h₅ : x ≥ -448 := by linarith
  have h₆ : x ≤ -1 := by
    omega
  -- We will check all possible values of x from -448 to -1 and show that none satisfy (24 *
  -- ↪ x) % 1199 = 15
  have h₇ : False := by
    -- Use the fact that x is between -448 and -1 to check each possible value
    have h₈ : x ≥ -448 := by linarith
    have h₉ : x ≤ -1 := by omega
    -- Use interval_cases to check each possible value of x
    interval_cases x <|> norm_num [Int.mul_emod, Int.add_emod] at h₄ ⊢ <|> omega
  exact h₇
exact h_main

theorem mathd_numbertheory_765 -- Simplified Proof, Time: 0.50s
(x : ℤ)
(h₀ : x < 0)
(h₁ : (24 * x) % 1199 = 15) :
x ≤ -449 := by
  omega

```

Listing 19: Example of Speedup after Simplification (orig: 2.5s, new: 0.5s)

```

theorem aime_1984_p1 -- Original Proof, Time: 0.91s
(u : ℕ → ℚ)
(h₀ : ∀ n, u (n + 1) = u n + 1)
(h₁ : ∑ k ∈ Finset.range 98, u k.succ = 137) :
∑ k ∈ Finset.range 49, u (2 * k.succ) = 93 := by
have h₂ : ∀ (n : ℕ), u n = u 0 + n := by
  (... 14 lines omitted)

have h₃ : 98 * u 0 + 4851 = 137 := by
have h₄ : ∑ k in Finset.range 98, u (k.succ) = 137 := h₁
have h₅ : ∑ k in Finset.range 98, u (k.succ) = ∑ k in Finset.range 98, (u 0 + (k.succ : ℚ)
  ↪ )) := by
  apply Finset.sum_congr rfl
  intro k _
  rw [h₂ (k.succ)]
  <=> simp [Nat.cast_add, Nat.cast_one]
  <=> ring_nf
  <=> norm_num
rw [h₅] at h₄
have h₆ : ∑ k in Finset.range 98, (u 0 + (k.succ : ℚ)) = 98 * u 0 + 4851 := by
have h₇ : ∑ k in Finset.range 98, (u 0 + (k.succ : ℚ)) = ∑ k in Finset.range 98, (u 0 :
  ↪ ℚ) + ∑ k in Finset.range 98, (k.succ : ℚ) := by
  rw [Finset.sum_add_distrib]
  rw [h₇]
have h₈ : ∑ k in Finset.range 98, (u 0 : ℚ) = 98 * u 0 := by
  simp [Finset.sum_const, Finset.card_range]
  <=> ring_nf
rw [h₈]
have h₉ : ∑ k in Finset.range 98, (k.succ : ℚ) = 4851 := by
  norm_num [Finset.sum_range_succ, Finset.sum_range_succ, Finset.sum_range_succ]
  <=>
  rfl
  rw [h₉]
  <=> ring_nf
rw [h₆] at h₄
norm_num at h₄ ⊢
<=> linarith

have h₄ : ∑ k ∈ Finset.range 49, u (2 * k.succ) = 49 * u 0 + 2450 := by
  -- (... 25 lines omitted)
have h₅ : 49 * u 0 = -2357 := by
  -- (... 6 lines omitted)
have h₆ : ∑ k ∈ Finset.range 49, u (2 * k.succ) = 93 := by
  -- (... 4 lines omitted)
  linarith
exact h₆

theorem aime_1984_p1 -- Simplified Proof, Time: 10.84s
(u : ℕ → ℚ)
(h₀ : ∀ n, u (n + 1) = u n + 1)
(h₁ : ∑ k ∈ Finset.range 98, u k.succ = 137) :
∑ k ∈ Finset.range 49, u (2 * k.succ) = 93 := by
simp_all [Finset.sum_range_succ]
linarith

```

Listing 20: Example of Slowdown after Simplification (orig: 0.9s, new: 10.8s)

```

theorem mathd_numbertheory_711 -- Original Proof, 4.87s
(m n : N)
(h0 : 0 < m ∧ 0 < n)
(h1 : Nat.gcd m n = 8)
(h2 : Nat.lcm m n = 112) :
72 ≤ m + n := by
have h_product : m * n = 896 := by
-- (... 5 lines omitted)
have h_main : 72 ≤ m + n := by
  have h3 : 0 < m := h0.1
  have h4 : 0 < n := h0.2
  have h5 : m * n = 896 := h_product
  have h6 : Nat.gcd m n = 8 := h1
  have h7 : Nat.lcm m n = 112 := h2
  have h8 : m + n ≥ 72 := by
    by_contra! h
    -- (... 4 lines omitted)
    have h11 : m ≤ 71 := by nlinarith
    have h12 : n ≤ 71 := by nlinarith
    interval_cases m <;> norm_num at h5 ⊢ <;>
    (try omega) <;>
    (try {
      interval_cases n <;> norm_num at h5 h6 h7 ⊢ <;>
      -- (... 5 lines omitted)
    }) <;>
    -- (... 5 lines omitted)
  exact h8
exact h_main

theorem mathd_numbertheory_711 -- Simplified Proof, 74.63s
(m n : N)
(h0 : 0 < m ∧ 0 < n)
(h1 : Nat.gcd m n = 8)
(h2 : Nat.lcm m n = 112) :
72 ≤ m + n := by
have : m * n = 896 := by
  rw [← Nat.gcd_mul_lcm m n]
  simp_all
by_contra!
have : m ≤ 71 := by nlinarith
have : n ≤ 71 := by nlinarith
interval_cases m <;> interval_cases n <;> simp_all

```

Listing 21: Example of Slowdown after Simplification (orig: 4.9s, new: 74.6s)

## I Derivation of Closed Form for min@k and max@k

In this section, we derive the closed form expression we use for estimating max@k from  $n$  samples based off the classic pass@k metric:

$$\text{max@}k = \frac{1}{\binom{n}{k}} \sum_{i \leq n} \binom{i-1}{k-1} x_i.$$

Let  $X$  be a real random variable,  $X_1, \dots, X_k$  independent realizations of  $X$  and  $X_{(k)} = \max_{i \leq k} X_i$  their maximum. We would like to give an estimator for  $\mathbb{E}[X_{(k)}]$  given  $n \geq k$  independent samples  $x_1 \leq \dots \leq x_n$  of  $X$  sorted by size.

Consider the estimator  $M = \frac{1}{\binom{n}{k}} \sum_{i \leq n} \binom{i-1}{k-1} x_i$ , with the idea being that there exist  $\binom{n}{k}$  ways to choose  $k$  out of the  $n$  samples overall, out of which  $\binom{i-1}{k-1}$  select the  $i$ -th and then  $k-1$  with a smaller index.

We compute

$$\begin{aligned} \mathbb{E}_{x_i} \left[ \frac{1}{\binom{n}{k}} \sum_{i \leq n} \binom{i-1}{k-1} x_i \right] &= \mathbb{E}_{x_i} \left[ \frac{1}{\binom{n}{k}} \sum_{I \subseteq \{1, \dots, n\}, |I|=k} x_{\max I} \right] \\ &= \frac{1}{\binom{n}{k}} \sum_{I \subseteq \{1, \dots, n\}, |I|=k} \mathbb{E}_{x_i} [x_{\max I}] \\ &= \frac{1}{\binom{n}{k}} \sum_{I \subseteq \{1, \dots, n\}, |I|=k} \mathbb{E}_{x_i} \left[ \max_{j \in I} x_j \right] \\ &= \frac{1}{\binom{n}{k}} \sum_{I \subseteq \{1, \dots, n\}, |I|=k} \mathbb{E} [X_{(k)}] \\ &= \mathbb{E} [X_{(k)}] \end{aligned}$$

by the counting argument explained above, linearity of expectation, ordering of the  $x_i$  and independence.

Note that this is a generalization of the pass@k metric, which covers the case of Bernoulli distributed  $X$  ([Chen et al., 2021](#)).

We recommend using a numerically stable implementation that computes the ratio  $\frac{\binom{i-1}{k-1}}{\binom{n}{k}}$  by canceling a  $(k-1)!$  factor and pairing up numerator and denominator factors.

Moreover, the min@k estimator can be obtained as  $\text{min@}k(x_1, \dots, x_n) = -\text{max@}k(-x_1, \dots, -x_n)$ .

## J Hyperparameters

In this section, we detail the hyperparameters we use throughout our various training and inference experiments. Prompts can be found in the next section, Appendix K.

**Iterative Training (Sec. 3.1.1):** For each round of SFT, we use an effective batch size of 64 (2 nodes, 8 H100/node, 4 gradient accumulation steps) and learning rate  $1e-5$ . We use a cosine scheduler with minimum learning rate  $1e-8$  and 100 steps of warm-up starting from  $1e-30$ . For inference, we use  $\tau = 1.0$  and top-p 0.95.

**Reinforcement learning (Sec 3.1.2):** Our setup is asynchronous online reinforcement learning with 16 trainer and 16 worker GPUs, and 16 environment copies per worker GPU. We use a global training batch size of 32 (local batch size 2 per trainer), a constant learning rate of  $6e-8$  following a linear warmup over 200 steps, a GRPO group size of 8, mean normalization but no variance normalization, no KL penalty and model updates sent to workers every 100 steps. Workers use For inference, we use  $\tau = 1.0$  and top-p 1.0, and evaluations use  $\tau = 1.0$  and top-p 0.95.

For test-time reinforcement learning we use the same settings but halve the number of trainers and workers.

**Execution Feedback and Goedel-Prover for Repair (Sec. 4.2):** We use temperature  $\tau = 0.2$  and top-p 0.95 with a maximum prompt length of 8192 and a maximum generation length of 32768.

**Iterative Shortening (Sec. 4.3):** For iterations 1 through 6, we use temperature  $\tau = 1.0$  and top-p 0.95. We increase the temperature to  $\tau = 1.2$  for iteration 7, and to  $\tau = 1.5$  for iteration 8. We find that the higher temperatures in later iterations are helpful for increasing diversity with 1024 samples.

**Lean Base Model (Sec. A.1):** We use an effective batch size of 512 (2 nodes, 8 H100/node, 32 gradient accumulation steps) and learning rate  $1e-5$  with 100 steps of warm-up starting from  $1e-30$ . We train with a maximum sequence length of 8192 for 2000 steps.

**Proof Sketching (Sec. A.2):** We use an effective batch size of 64 (2 nodes, 8 H100/node, 4 gradient accumulation steps) and learning rate  $1e-5$  with 100 steps of warm-up starting from  $1e-30$ . We train with a maximum sequence length of 8192 for 50 steps. Evaluation is done with temperature  $\tau = 0.8$  and top-p 0.95.

**Comparison with Leading Models (Sec. D):** For our model and Qwen2.5-32B, we use  $\tau = 1.0$  and top-p 0.95. For GPT-4o and Gemini-2.5-Pro, we use the default settings with  $\tau = 1.0$ .



## K Prompts

### K.1 Proof Simplification Prompt

```
You are given a correct Lean 4 proof of a mathematical theorem.
Your goal is to simplify and clean up the proof, making it shorter and more readable while ensuring it
  ↪ is still correct.

Here is the original proof:
```lean4
{statement}
```

Now, provide your simplified proof. Do NOT modify the theorem or header, and surround your proof in
  ↪ ```lean4 and ``` tags.
```

Listing 22: Zero-shot Proof Sketching Prompt

### K.2 Proof Sketching Prompts

```
Your task is to translate a natural language math solution into a Lean 4 proof sketch that follows the
  ↪ structure of the natural language solution. Follow these guidelines:
1. Analyze the natural language solution and identify the key steps.
2. Translate each key step into Lean 4 syntax, structuring your proof using 'have' statements for
  ↪ clarity. Include all core steps from the natural language solution.
3. Use 'sorry' to replace individual proofs of lower-level steps, ensuring that your proof skeleton
  ↪ would compile successfully in Lean 4.
4. Surround your Lean 4 proof sketch in ```lean4 and ``` tags.

Problem:
{problem}

Solution:
{solution}

Lean 4 Statement:
```lean4
{statement}
```

Now, provide your Lean 4 proof sketch. Do NOT modify the theorem or header, and surround your proof
  ↪ sketch in ```lean4 and ``` tags.
```

Listing 23: Zero-shot Proof Sketching Prompt

```
Your task is to translate a natural language math solution into a Lean 4 proof sketch that follows the
  ↪ structure of the natural language solution. Follow these guidelines:
1. Analyze the natural language solution and identify the key steps.
2. Translate each key step into Lean 4 syntax, structuring your proof using 'have' statements for
  ↪ clarity. Include all core steps from the natural language solution.
3. Use 'sorry' to replace individual proofs of lower-level steps, ensuring that your proof skeleton
  ↪ would compile successfully in Lean 4.
4. Surround your Lean 4 proof sketch in ```lean4 and ``` tags.

Here is an example:
```

```

Problem:
Prove that if  $p, q$  are primes such that  $q$  is divisible by  $p$ , then  $p$  must be equal to  $q$ .

Solution:
Since  $q$  is prime, it only has 2 divisors: 1 and itself. Therefore, since  $p$  divides  $q$ , either  $p=1$  or  $p=q$ . Because  $p$  is a prime,  $p \neq 1$ , so  $p=q$ .

Lean 4 Statement:
'''lean4
import Mathlib

theorem prime_divides_prime_equal (p q : N) (hp : Prime p) (hq : Prime q) (h : p | q) : p = q := by
  sorry
'''

Lean 4 Proof Sketch:
'''lean4
import Mathlib

theorem prime_divides_prime_equal (p q : N) (hp : Prime p) (hq : Prime q) (h : p | q) : p = q := by
  -- Lemma 1: Since  $q$  is prime, it only has 2 divisors: 1 and itself.
  have lemma1 : p = 1  $\vee$  p = q := by
    sorry

  -- Lemma 2: Since  $p$  is prime,  $p \neq 1$ .
  have lemma2 : p  $\neq$  1 := by
    sorry

  -- Now, do case analysis on lemma1 to conclude  $p = q$ .
  cases lemma1 with
  | inl h_left =>
    contradiction
  | inr h_right =>
    exact h_right
'''

Now, it is your turn to provide your Lean 4 proof sketch for a new problem. Do NOT modify the theorem
header, and surround your proof sketch in '''lean4 and ''' tags.

Problem:
{problem}

Solution:
{solution}

Lean 4 Statement:
'''lean4
{statement}
'''

Lean 4 Proof Sketch

```

Listing 24: One-shot Proof Sketching Prompt

### K.3 Goedel-Prover Repair Prompt

In Listing 25, use a modified version of Goedel-Prover’s repair prompt found in their [codebase](#). The main difference is that because we do not have proofs annotated with CoT’s, our `lean_proof` only contains a proof.

Complete the following Lean 4 code:

```
```lean4
{formal_statement}```
```

Before producing the Lean 4 code to formally prove the given theorem, provide a detailed proof plan  
↪ outlining the main proof steps and strategies.

The plan should highlight key ideas, intermediate lemmas, and proof structures that will guide the  
↪ construction of the final formal proof.

Here is the proof:

```
```lean4
{lean_proof}```
```

The proof (Round 1) is not correct. Following is the compilation error message, where we use <error></>  
↪ error> to signal the position of the error.

```
{error_message_for_prev_round}
```

Before producing the Lean 4 code to formally prove the given theorem, provide a detailed analysis of  
↪ the error message.

Listing 25: Goedel-Prover Repair Prompt

## L Python Code for Proof Length

```
import re
from collections import Counter

def proof_length(statement_and_proof):
    lean_operators = [':=', '!=', '&&', '-.', '->', '←', '...', '...', '::', ':>',
                      '<:', '<:', '==', '||', '=>', '<=', '>=', '-1', '?_']
    lean_operators_spaced = [' '.join(conn) for conn in lean_operators]
    lean_operators_dict = dict(zip(lean_operators_spaced, lean_operators))
    def lexer(lean_snippet):
        tokenized_lines = []
        for line in lean_snippet.splitlines():
            tokens = []
            token = ''
            for ch in line:
                if ch == ' ':
                    if token:
                        tokens.append(token)
                        token = ''
                elif str.isalnum(ch) or (ch in "_."):
                    token += ch
                else:
                    if token:
                        tokens.append(token)
                        token = ''
                    tokens.append(ch)
            if token:
                tokens.append(token)
            tokenized_line = ' '.join(tokens)
            for conn in lean_operators_spaced:
                if conn in tokenized_line:
                    tokenized_line = tokenized_line.replace(conn, lean_operators_dict[conn])
            tokenized_lines.append(tokenized_line)
        return '\n'.join(tokenized_lines)

    def remove_statement(statement_and_proof):
        if " := by" in statement_and_proof:
            return statement_and_proof.split(" := by", maxsplit=1)[1].strip()
        return statement_and_proof.split(" :=", maxsplit=1)[1].strip()

    def remove_comments(lean_snippet):
        # multi-line comments
        lean_snippet = re.sub(r" */-.*-/ ", "", lean_snippet, flags=re.DOTALL)
        # single-line comments
        lean_snippet = re.sub(r" ---.*", "", lean_snippet)
        return lean_snippet

    try:
        proof = remove_statement(statement_and_proof)
        proof = remove_comments(proof)
        proof_tokenized = lexer(proof)
        return sum([len(l.split(' ')) for l in proof_tokenized.splitlines()])
    except:
        return 10**9
```

## **M Proofs**

In this section, we include the original and simplified proofs for miniF2F, PutnamBench, and IMO 2025.

# MiniF2F Proofs

```
-- Orig Proof
import Mathlib
import Aesop

set_option maxHeartbeats 0

open BigOperators Real Nat Topology Rat

theorem mathd_algebra_478
  (b h v : ℝ)
  (h₁ : 0 < b ∧ 0 < h ∧ 0 < v)
  (h₂ : v = 1 / 3 * (b * h))
  (h₃ : b = 30)
  (h₄ : h = 13 / 2) :
  v = 65 := by
  have h₅ : v = 65 := by
    rw [h₁]
    rw [h₂, h₃]
    ring_nf at *
    <> norm_num at *
    <> linarith
  exact h₅

-- Simplified Proof
import Mathlib
import Aesop

set_option maxHeartbeats 0

open BigOperators Real Nat Topology Rat

theorem mathd_algebra_478
  (b h v : ℝ)
  (h₁ : 0 < b ∧ 0 < h ∧ 0 < v)
  (h₂ : v = 1 / 3 * (b * h))
  (h₃ : b = 30)
  (h₄ : h = 13 / 2) :
  v = 65 := by
  subst_vars
  linarith

-- Orig Proof
import Mathlib
import Aesop

set_option maxHeartbeats 0

open BigOperators Real Nat Topology Rat

theorem mathd_numbertheory_3 :
  (x ∈ Finset.range 10, ((x + 1)^2)) % 10 = 5 :=
  by
  have h_sum : x ∈ Finset.range 10, ((x + 1)^2) =
  → 385 := by
    decide
  have h_mod : (x ∈ Finset.range 10, ((x + 1)^2))
  → % 10 = 5 := by
    rw [h_sum]
    <> norm_num
  apply h_mod

-- Simplified Proof
import Mathlib
import Aesop

set_option maxHeartbeats 0

open BigOperators Real Nat Topology Rat

theorem mathd_numbertheory_3 :
  (x ∈ Finset.range 10, ((x + 1)^2)) % 10 = 5 :=
  by
  decide

-- Orig Proof
import Mathlib
import Aesop

set_option maxHeartbeats 0

open BigOperators Real Nat Topology Rat

theorem mathd_algebra_141
  (a b : ℝ)
  (h₁ : (a * b) = 180)
  (h₂ : 2 * (a + b) = 54) :
  (a^2 + b^2) = 369 := by
  linarith

-- Orig Proof
import Mathlib
import Aesop

set_option maxHeartbeats 0

open BigOperators Real Nat Topology Rat

theorem mathd_algebra_44
  (s t : ℝ)
  (h₁ : s = 9 - 2 * t)
  (h₂ : t = 3 * s + 1) :
  s = 1 ∧ t = 4 := by
  have h₃ : t = 4 := by
    have h₄ : t = 3 * (9 - 2 * t) + 1 := by
      rw [h₁] at h₂
      linarith
    -- Solve for t using the equation t = 3*(9 -
    -- 2*t) + 1
    linarith
  have h₅ : s = 1 := by
    have h₆ : s = 9 - 2 * t := h₁
    rw [h₃]
    rw [h₂]
    norm_num
  have h₇ : s = 1 ∧ t = 4 := by
    exact ⟨h₅, h₆⟩

-- Simplified Proof
import Mathlib
import Aesop

set_option maxHeartbeats 0

open BigOperators Real Nat Topology Rat

theorem mathd_algebra_44
  (s t : ℝ)
  (h₁ : s = 9 - 2 * t)
  (h₂ : t = 3 * s + 1) :
  s = 1 ∧ t = 4 := by
  constructor
  all_goals
    linarith

-- Orig Proof
import Mathlib
import Aesop

set_option maxHeartbeats 0

open BigOperators Real Nat Topology Rat

theorem numbertheory_4x3m7y3neq2003
  (x y : ℤ) :
  4 * x^3 - 7 * y^3 ≠ 2003 := by
  have h_main : (4 * x^3 - 7 * y^3) % 7 ≠ 2003
  → % 7 := by
    have h₁ : (4 * x^3 - 7 * y^3) % 7 = (4 * x
    → ^ 3) % 7 := by
      have h₂ : (7 * y^3 : ℤ) % 7 = 0 := by
        norm_num [Int.mul_emod, pow_three]
      have h₃ : (4 * x^3 - 7 * y^3 : ℤ) % 7 =
      → ((4 * x^3 : ℤ) % 7 - (7 * y^3 : ℤ) %
      → 7) % 7 := by
        simp [Int.sub_emod]
      rw [h₁]
      simp [h₂]
      <> omega
    have h₄ : (2003 : ℤ) % 7 = 1 := by norm_num
    rw [h₁]
    have h₅ : (4 * x^3 : ℤ) % 7 ≠ 1 := by
      have h₆ : x % 7 = 0 ∨ x % 7 = 1 ∨ x % 7 = 2 ∨
      → x % 7 = 3 ∨ x % 7 = 4 ∨ x % 7 = 5 ∨ x % 7
      → = 6 := by
        omega
      rcases h₆ with ⟨h₇, | h₈, | h₉, | h₁₀, | h₁₁, |
      → h₁₂⟩ <>
      (try { norm_num [h₇, pow_three,
      → Int.mul_emod, Int.emod_emod] }) <>
      (try { omega }) <>
      (try {
        simp [h₇, pow_three, Int.mul_emod,
        → Int.emod_emod]
        <> norm_num <> omega
      })
    have h₈ : (4 * x^3 : ℤ) % 7 ≠ 1 := h₅
    omega
  have h_final : 4 * x^3 - 7 * y^3 ≠ 2003 := by
    intro h
    have h₉ : (4 * x^3 - 7 * y^3) % 7 = 2003 %
    → 7 := by
      rw [h]
    have h₁₀ : (4 * x^3 - 7 * y^3) % 7 ≠ 2003 %
    → 7 := h_main
    contradiction
  exact h_final

-- Simplified Proof
import Mathlib
import Aesop

set_option maxHeartbeats 0
```

```
open BigOperators Real Nat Topology Rat

theorem numbertheory_4x3m7y3neq2003
  (x y : ℤ) :
  4 * x^3 - 7 * y^3 ≠ 2003 := by
  have : 4 * x^3 % 7 ≠ 2003 % 7 := by
    have : x % 7 = 0 ∨ x % 7 = 1 ∨ x % 7 = 2 ∨ x %
    → 7 = 3 ∨ x % 7 = 4 ∨ x % 7 = 5 ∨ x % 7 = 6
    → := by omega
    rcases this with ⟨h | h | h | h | h | h | h⟩
    <> simp [h, Int.mul_emod, pow_three]
  omega

-- Orig Proof
import Mathlib
import Aesop

set_option maxHeartbeats 0

open BigOperators Real Nat Topology Rat

theorem mathd_numbertheory_1124
  (n : ℕ)
  (h₁ : n ≤ 9)
  (h₂ : 18374 * 10 + n) :
  n = 4 := by
  have h_main : n = 4 := by
    have h₃ : n ≤ 9 := h₁
    interval_cases n <> norm_num at h₃ <>
    (try omega) <>
    (try {
      rcases h₃ with ⟨k, hk⟩
      norm_num at hk
      <> omega
    })
  exact h_main

-- Simplified Proof
import Mathlib
import Aesop

set_option maxHeartbeats 0

open BigOperators Real Nat Topology Rat

theorem mathd_numbertheory_1124
  (n : ℕ)
  (h₁ : n ≤ 9)
  (h₂ : 18374 * 10 + n) :
  n = 4 := by
  omega

-- Orig Proof
import Mathlib
import Aesop

set_option maxHeartbeats 0

open BigOperators Real Nat Topology Rat

theorem mathd_algebra_209
  (ω : Equiv ℝ ℝ)
  (h₁ : ω.2 2 = 10)
  (h₂ : ω.2 10 = 1)
  (h₃ : ω.2 1 = 2) :
  ω.1 (ω.1 10) = 1 := by
  have h₄ : ω.1 10 = 2 := by
    have h₅ : ω.1 (ω.2 2) = 2 := by
      apply Equiv.apply_symm_apply
      rw [h₁] at h₅
      exact h₅
  have h₆ : ω.1 2 = 1 := by
    have h₇ : ω.1 (ω.2 1) = 1 := by
      apply Equiv.apply_symm_apply
      rw [h₂] at h₇
      exact h₇
  have h₈ : ω.1 (ω.1 10) = 1 := by
    rw [h₆]
    rw [h₃]
    exact h₈

-- Simplified Proof
import Mathlib
import Aesop

set_option maxHeartbeats 0

open BigOperators Real Nat Topology Rat

theorem mathd_algebra_209
  (ω : Equiv ℝ ℝ)
  (h₁ : ω.2 2 = 10)
  (h₂ : ω.2 10 = 1)
  (h₃ : ω.2 1 = 2) :
  ω.1 (ω.1 10) = 1 := by
  have h₄ : ω.right_inv 2
  have h₅ : ω.right_inv 1
  simp_all

-- Orig Proof
import Mathlib
import Aesop

set_option maxHeartbeats 0

open BigOperators Real Nat Topology Rat

theorem mathd_numbertheory_237 :
  (x k ∈ (Finset.range 101), k) % 6 = 4 := by
  have h_main : (x k ∈ (Finset.range 101), k) % 6 =
  → 4 := by
    rfl
  exact h_main

-- Simplified Proof
import Mathlib
```

```

import Aesop

set_option maxHeartbeats 0

open BigOperators Real Nat Topology Rat

theorem mathd_numbertheory_237 :
  (∃ k ∈ (Finset.range 101), k) % 6 = 4 := by
  rfl

-----
-- Orig Proof
import Mathlib
import Aesop

set_option maxHeartbeats 0

open BigOperators Real Nat Topology Rat

theorem mathd_algebra_33
  (x y z : ℝ)
  (h₁ : x ≠ 0)
  (h₂ : 2 * x = 5 * y)
  (h₃ : 7 * y = 10 * z) :
  z / x = 7 / 25 := by
  have h₄ : y = (2 * x) / 5 := by
    have h₄₁ : 5 * y = 2 * x := by linarith
    have h₄₂ : y = (2 * x) / 5 := by
      apply Eq.symm
      -- Solve for y by dividing both sides by 5
      ring_nf at h₄₁
      linarith
    exact h₄₂
  have h₅ : z = (7 * x) / 25 := by
    have h₅₁ : 7 * y = 10 * z := h₃
    have h₅₂ : y = (2 * x) / 5 := h₄
    rw [h₅₁] at h₅₁
    -- Simplify the equation 7 * ((2 * x) / 5) = 10
    -- z
    ring_nf at h₅₁
    -- Solve for z by dividing both sides by 10
    linarith
  have h₆ : z / x = 7 / 25 := by
    have h₆₁ : z = (7 * x) / 25 := h₅
    rw [h₆₁]
    -- Simplify ((7 * x) / 25) / x to 7 / 25
    <|> ring_nf
    <|> field_simp [h₆₁]
    <|> ring_nf
    rw [h₆₁]
  exact h₆

-- Simplified Proof
import Mathlib
import Aesop

set_option maxHeartbeats 0

open BigOperators Real Nat Topology Rat

theorem mathd_algebra_33
  (x y z : ℝ)
  (h₁ : x ≠ 0)
  (h₂ : 2 * x = 5 * y)
  (h₃ : 7 * y = 10 * z) :
  z / x = 7 / 25 := by
  field_simp
  linarith

-----
-- Orig Proof
import Mathlib
import Aesop

set_option maxHeartbeats 0

open BigOperators Real Nat Topology Rat

theorem aime_1983_p1 (x y z w : ℝ) (ht : 1 < x ∧ 1
  < y ∧ 1 < z) (hw : 0 ≤ w)
  (h0 : Real.log w / Real.log x = 24) (h1 :
  <|> Real.log w / Real.log y = 40)
  (h2 : Real.log w / Real.log (x * y * z) = 12)
  <|> Real.log w / Real.log z = 60 := by
  have hx : (x : ℝ) > 1 := by
    norm_cast
    <|> linarith [ht.1]
  have hy : (y : ℝ) > 1 := by
    norm_cast
    <|> linarith [ht.2.1]
  have hz : (z : ℝ) > 1 := by
    norm_cast
    <|> linarith [ht.2.2]
  have hxy : Real.log (w : ℝ) = 24 * Real.log (x : ℝ) := by
    field_simp [Real.log_ne_zero_of_pos_of_ne_one
      <|> (by positivity : (0 : ℝ) < x) (by
        <|> linarith : (x : ℝ) ≠ 1)] at h0
    linarith
  have hxy : Real.log w = 40 * Real.log y := by
    field_simp [Real.log_ne_zero_of_pos_of_ne_one
      <|> (by positivity : (0 : ℝ) < y) (by
        <|> linarith : (y : ℝ) ≠ 1)] at h1
    linarith
  have hxyz : Real.log w = 12 * (Real.log x +
    <|> Real.log y + Real.log z) := by
    have h3 : Real.log (x * y * z) = Real.log x +
      <|> Real.log y + Real.log z := by
      rw [Real.log_mul, Real.log_mul] <|>
      <|> positivity
    field_simp [Real.log_ne_zero_of_pos_of_ne_one
      <|> (by positivity : (0 : ℝ) < x * y * z) (by
        <|> have : (x * y * z : ℝ) > 1 := by
          have : (x : ℝ) > 1 := by
            assumption_mod_cast
            have : (y : ℝ) > 1 := by
              assumption_mod_cast
            have : (z : ℝ) > 1 := by
              assumption_mod_cast
            calc
              (x * y * z : ℝ) = (x : ℝ) * (y : ℝ) *
                <|> (z : ℝ) := by norm_cast
              > 1 * 1 * 1 := by gcongr <|>
                <|> 1 := by norm_num
            linarith
          have h11 : Real.log (x * y * z : ℝ) >
            <|> Real.log 1 := by
              apply Real.log_lt_log (by positivity)
              <|> norm_num at h7
              <|> nlinarith
          have h12 : Real.log 1 = (0 : ℝ) := by
            norm_num
            linarith
          have h6 : Real.log (w : ℝ) = 12 * Real.log (x *
            <|> y * z : ℝ) := by
              field_simp [h5] at h4
              <|> nlinarith
          rw [h6, h3]
              <|> ring_nf
              <|> linarith
            linarith
          have hxyz' : Real.log (x : ℝ) = Real.log (y : ℝ) +
            <|> Real.log (z : ℝ) := by
              have h3 : 24 * Real.log (x : ℝ) = 12 *
                <|> (Real.log (x : ℝ) + Real.log (y : ℝ) +
                  <|> Real.log (z : ℝ)) := by
                  linarith [hxy, hxyz]
              have h4 : 2 * Real.log (x : ℝ) = Real.log (x : ℝ)
                <|> + Real.log (y : ℝ) + Real.log (z : ℝ) :=
                <|> by linarith
              linarith
            have hz' : Real.log (z : ℝ) = (2 / 5 : ℝ) *
              <|> Real.log (x : ℝ) := by
              have h3 : Real.log (x : ℝ) = Real.log (y : ℝ) +
                <|> Real.log (z : ℝ) := hxyz'
              have h4 : 3 * Real.log (x : ℝ) = 5 * Real.log
                <|> (y : ℝ) := hxy
              have h5 : Real.log (y : ℝ) = (3 / 5 : ℝ) *
                <|> Real.log (x : ℝ) := by
              have h6 : Real.log (y : ℝ) = (3 / 5 : ℝ) *
                <|> Real.log (x : ℝ) := by
              apply Eq.symm
              -- Solve for Real.log y in terms of
              <|> Real.log x
              ring_nf at h4
              linarith
              have h6 : Real.log (x : ℝ) = (3 / 5 : ℝ) *
                <|> Real.log (x : ℝ) + Real.log (z : ℝ) := by
              linarith
              have h7 : Real.log (z : ℝ) = (2 / 5 : ℝ) *
                <|> Real.log (x : ℝ) := by
              ring_nf at h6
              nlinarith
              exact h7
            have h_main : Real.log (w : ℝ) / Real.log (z : ℝ)
              <|> = 60 := by
              have h3 : Real.log (w : ℝ) = 24 * Real.log (x
                <|> : ℝ) := hux
              have h4 : Real.log (z : ℝ) = (2 / 5 : ℝ) *
                <|> Real.log (x : ℝ) := hz'
            have h5 : Real.log (x : ℝ) > 0 := Real.log_pos
              <|> hx
            have h6 : Real.log (z : ℝ) > 0 := by
              <|> Real.log (z : ℝ) = (2 / 5 : ℝ) *
                <|> Real.log (x : ℝ)
              <|> Real.log (x : ℝ) > 0 := hx
            have h7 : Real.log (z : ℝ) = (2 / 5 : ℝ) *
              <|> Real.log (x : ℝ) := hz'
            have h8 : (2 / 5 : ℝ) > 0 := by
              <|> Real.log (x : ℝ) > 0 := hx
            have h9 : Real.log (x : ℝ) > 0 :=
              <|> Real.log_pos hx
            have h10 : Real.log (z : ℝ) = (2 / 5 : ℝ) *
              <|> Real.log (x : ℝ) := hz'
            have h11 : Real.log (z : ℝ) > 0 := by
              rw [h10]
              positivity
              linarith
            have h7 : Real.log (w : ℝ) / Real.log (z : ℝ) =
              <|> 60 := by
              rw [h3, h4]
              field_simp [h5.ne']
              <|> ring_nf
              <|> field_simp [h5.ne']
              <|> nlinarith
              exact h7
            simp using h_main
          -- Simplified Proof
          import Mathlib
          import Aesop
          set_option maxHeartbeats 0
          open BigOperators Real Nat Topology Rat
          theorem aime_1983_p1 (x y z w : ℝ) (ht : 1 < x ∧ 1
            < y ∧ 1 < z) (hw : 0 ≤ w)
            (h0 : Real.log w / Real.log x = 24) (h1 :
            <|> Real.log w / Real.log y = 40)
            (h2 : Real.log w / Real.log (x * y * z) = 12)
            <|> Real.log w / Real.log z = 60 := by
            have hx : (x : ℝ) > 1 := by
              norm_cast
              <|> linarith [ht.1]
            have hy : (y : ℝ) > 1 := by
              norm_cast
              <|> linarith [ht.2.1]
            have hz : (z : ℝ) > 1 := by
              norm_cast
              <|> linarith [ht.2.2]
            have hxy : Real.log (w : ℝ) = 24 * Real.log (x : ℝ) := by
              <|> Real.log (x : ℝ) ≠ 0 := by
              have h4 : Real.log (x : ℝ) > 0 :=
                <|> Real.log_pos hx
              linarith
            have h4 : Real.log (w : ℝ) / Real.log (x : ℝ) =
              <|> 24 := by simp using h0
            field_simp [h3] at h4
            <|> ring_nf at h4
            <|> nlinarith
            have hxy : Real.log (w : ℝ) = 40 * Real.log (y : ℝ)
              <|> := by
              have h3 : Real.log (y : ℝ) ≠ 0 := by
              have h4 : Real.log (y : ℝ) > 0 :=
                <|> Real.log_pos hy
              linarith
            have h4 : Real.log (w : ℝ) / Real.log (y : ℝ) =
              <|> 40 := by simp using h1
            field_simp [h3] at h4

```

```

set_option maxHeartbeats 0

open BigOperators Real Nat Topology Rat

theorem amc12b_2020_p2 :
  ((100 ^ 2 - 7 ^ 2) :  $\mathbb{N}$ ) / (70 ^ 2 - 11 ^ 2) *
     $\rightarrow$  ((70 - 11) * (70 + 11) / ((100 - 7) *
      (100 + 7))) = 1 := by
  have h : ((100 ^ 2 - 7 ^ 2) :  $\mathbb{N}$ ) / (70 ^ 2 - 11 ^ 2)
     $\rightarrow$  2 * ((70 - 11) * (70 + 11) / ((100 - 7) *
      (100 + 7))) = 1 := by
    norm_num [pow_two]
  <|>
  ring_nf
  <|>
  norm_num
  <|>
  rfl

apply h

-- Simplified Proof
import Mathlib
import Aesop

set_option maxHeartbeats 0

open BigOperators Real Nat Topology Rat

theorem amc12b_2020_p2 :
  ((100 ^ 2 - 7 ^ 2) :  $\mathbb{N}$ ) / (70 ^ 2 - 11 ^ 2) *
     $\rightarrow$  ((70 - 11) * (70 + 11) / ((100 - 7) *
      (100 + 7))) = 1 := by
    norm_num
  <|>
  -- Orig Proof
  import Mathlib
  import Aesop

set_option maxHeartbeats 0

open BigOperators Real Nat Topology Rat

theorem amc12b_2021_p3
  (h :  $\mathbb{N}$ )
  (h1 : 2 + 1 / (1 + 1 / (2 + 2 / (3 + x))) = 144 /
     $\rightarrow$  53) :
  x = 3 / 4 := by
  have h1 : 1 / (1 + 1 / (2 + 2 / (3 + x))) = 38 /
     $\rightarrow$  53 := by
    have h11 : 1 / (1 + 1 / (2 + 2 / (3 + x))) =
       $\rightarrow$  144 / 53 - 2 := by
      linarith
    rw [h11]
    norm_num

  have h1 : 1 + 1 / (2 + 2 / (3 + x)) = 53 / 38 :=
    by
  have h11 : 1 + 1 / (2 + 2 / (3 + x)) = 1 / (38
     $\rightarrow$  / 53) := by
  have h12 : 1 / (1 + 1 / (2 + 2 / (3 + x))) =
     $\rightarrow$  38 / 53 := h1
  have h13 : 1 + 1 / (2 + 2 / (3 + x))  $\neq$  0 := by
    by_contra h
    rw [h] at h13
    norm_num at h13
    <|> linarith
  have h14 : 1 / (1 + 1 / (2 + 2 / (3 + x))) =
     $\rightarrow$  38 / 53 := h1
  have h15 : (1 + 1 / (2 + 2 / (3 + x))) = 1 /
     $\rightarrow$  (38 / 53) := by
    have h16 : (1 + 1 / (2 + 2 / (3 + x)))  $\neq$  0
      := h13
    field_simp at h14
    <|> nlinarith
    linarith
  rw [h15]
  <|> norm_num

  have h1 : 1 / (2 + 2 / (3 + x)) = 15 / 38 := by
  have h11 : 1 / (2 + 2 / (3 + x)) = 53 / 38 - 1
    := by
    linarith
  rw [h11]
  <|> norm_num

  have h1 : 2 + 2 / (3 + x) = 38 / 15 := by
  have h11 : 2 + 2 / (3 + x) = 1 / (15 / 38) := by
  have h12 : 1 / (2 + 2 / (3 + x)) = 15 / 38 :=
     $\rightarrow$  h1
  have h13 : 2 + 2 / (3 + x)  $\neq$  0 := by
    by_contra h
    rw [h] at h13
    norm_num at h13
    <|> linarith
  have h14 : 1 / (2 + 2 / (3 + x)) = 15 / 38 :=
     $\rightarrow$  h1
  have h15 : (2 + 2 / (3 + x)) = 1 / (15 / 38)
    := by
  have h16 : (2 + 2 / (3 + x))  $\neq$  0 := h13
  field_simp at h14
  <|> nlinarith
  linarith
  rw [h15]
  <|> norm_num

  have h1 : 2 / (3 + x) = 8 / 15 := by
  have h11 : 2 / (3 + x) = 38 / 15 - 2 := by
    linarith
  rw [h11]
  <|> norm_num
  <|>
  (try ring_nf at * <|> linarith)
  <|>
  (try field_simp at * <|> ring_nf at * <|>
     $\rightarrow$  linarith)

  have h1 : (3 + x) / 2 = 15 / 8 := by
  have h11 : (3 + x) / 2 = 15 / 8 := by

```

```

  have h12 : 2 / (3 + x) = 8 / 15 := h1
  have h13 : 3 + x  $\neq$  0 := by
    by_contra h
    rw [h] at h13
    norm_num at h13
    <|> linarith
  have h14 : (3 + x) / 2 = 15 / 8 := by
  have h15 : 2 / (3 + x) = 8 / 15 := h1
  field_simp at h13
  <|> nlinarith
  exact h14
  exact h15

  have h1 : 3 + x = 15 / 4 := by
  have h11 : (3 + x) / 2 = 15 / 8 := h1
  have h12 : 3 + x = 15 / 4 := by
    linarith
  exact h12
  exact h1

-- Simplified Proof
import Mathlib
import Aesop

set_option maxHeartbeats 0

open BigOperators Real Nat Topology Rat

theorem amc12b_2021_p3
  (x :  $\mathbb{N}$ )
  (h1 : 2 + 1 / (1 + 1 / (2 + 2 / (3 + x))) = 144 /
     $\rightarrow$  53) :
  x = 3 / 4 := by
  have h1 : 1 / (1 + 1 / (2 + 2 / (3 + x))) = 38 /
     $\rightarrow$  53 := by
    linarith
  have h11 : 1 + 1 / (2 + 2 / (3 + x))  $\neq$  0 := by
    by_contra h
    rw [h] at h11
    norm_num at h11
    field_simp at h11
  have h12 : 2 / (3 + x) = 8 / 15 := by
  have h13 : 2 + 2 / (3 + x) = 38 / 15 := by
  have h14 : 1 / (2 + 2 / (3 + x)) = 15 / 38 :=
     $\rightarrow$  by
    linarith
  have h15 : 2 + 2 / (3 + x)  $\neq$  0 := by
    by_contra h
    rw [h] at h15
    norm_num at h15
    field_simp at h15
    linarith
  have h16 : (3 + x) / 2 = 15 / 8 := by
  have h17 : 2 / (3 + x) = 8 / 15 := by
    linarith
  have h18 : 3 + x  $\neq$  0 := by
    by_contra h
    rw [h] at h18
    norm_num at h18
    field_simp at h18
    linarith
  linarith
  <|>
  -- Orig Proof
  import Mathlib
  import Aesop

set_option maxHeartbeats 0

open BigOperators Real Nat Topology Rat

theorem mathd_algebra_419
  (a b :  $\mathbb{N}$ )
  (h1 : a = -1)
  (h2 : b = 5) :
  -a - b^2 + 3 * (a * b) = -39 := by
  have h1 : -a - b^2 + 3 * (a * b) = -39 := by
    rw [h1, h2]
    norm_num
    <|>
    ring_nf
    <|>
    norm_num
    <|>
    linarith
  exact h1

-- Simplified Proof
import Mathlib
import Aesop

set_option maxHeartbeats 0

open BigOperators Real Nat Topology Rat

theorem mathd_algebra_419
  (a b :  $\mathbb{N}$ )
  (h1 : a = -1)
  (h2 : b = 5) :
  -a - b^2 + 3 * (a * b) = -39 := by
    subst_vars
    norm_num
  <|>
  -- Orig Proof
  import Mathlib
  import Aesop

set_option maxHeartbeats 0

open BigOperators Real Nat Topology Rat

theorem algebra_sqineq_unitcircatpabsamblt1
  (a b :  $\mathbb{N}$ )
  (h1 : a^2 + b^2 = 1) :
  a * b + |a - b|  $\leq$  1 := by
  have h_main : a * b + |a - b|  $\leq$  1 := by
    cases' le_or_lt 0 (a - b) with h h
    -- Case 1: a - b  $\geq$  0
    have h1 : |a - b| = a - b := by
      rw [abs_of_nonneg h]
    rw [h1]
    have h2 : (a - b) ^ 2 = 1 - 2 * (a * b) := by
      linarith
    have h3 : a * b + (a - b)  $\leq$  1 := by
      linarith [sq_nonneg (a - b - 1)]
    linarith
    -- Case 2: a - b < 0
    have h1 : |a - b| = -(a - b) := by
      rw [abs_of_neg h]
    <|> linarith
    rw [h1]
    have h2 : (a - b) ^ 2 = 1 - 2 * (a * b) := by
      linarith
    have h3 : a * b + -(a - b)  $\leq$  1 := by
      linarith [sq_nonneg (a - b + 1)]
    linarith
  exact h_main

-- Simplified Proof
import Mathlib
import Aesop

set_option maxHeartbeats 0

open BigOperators Real Nat Topology Rat

theorem algebra_sqineq_unitcircatpabsamblt1
  (a b :  $\mathbb{N}$ )
  (h1 : a^2 + b^2 = 1) :
  a * b + |a - b|  $\leq$  1 := by
    nlinarith [abs_mul_abs_self (a - b)]
  <|>
  -- Orig Proof
  import Mathlib
  import Aesop

set_option maxHeartbeats 0

open BigOperators Real Nat Topology Rat

theorem imo_1983_p6
  (a b c :  $\mathbb{N}$ )
  (h1 : 0 < a  $\wedge$  0 < b  $\wedge$  0 < c)
  (h2 : c < a + b)
  (h3 : b < a + c)
  (h4 : a < b + c) :
  0  $\leq$  a^2 * b * (a - b) + b^2 * c * (b - c) + c^2 *
     $\rightarrow$  a * (c - a) := by
  have h_main : 0  $\leq$  a^2 * b * (a - b) + b^2 * c *
     $\rightarrow$  (b - c) + c^2 * a * (c - a) := by
    nlinarith [sq_nonneg (a - b), sq_nonneg (b -
       $\rightarrow$  c), sq_nonneg (c - a),
      mul_nonneg h1.1.le h2.1.le, mul_nonneg
         $\rightarrow$  h2.2.1.le h2.2.2.le, mul_nonneg h1.2.2.le
           $\rightarrow$  h1.1.le,
      mul_nonneg (sq_nonneg (a - b)) h2.2.2.le,
         $\rightarrow$  mul_nonneg (sq_nonneg (b - c)) h1.1.le,
        mul_nonneg (sq_nonneg (c - a)) h2.2.1.le,
         $\rightarrow$  mul_pos h1.1 h2.2.1, mul_pos h1.2.1 h2.2.2,
        mul_pos h2.2.2 h1.1, mul_pos (sub_pos.mpr h1)
           $\rightarrow$  (sub_pos.mpr h1),
        mul_pos (sub_pos.mpr h1) (sub_pos.mpr h1),
         $\rightarrow$  mul_pos (sub_pos.mpr h1) (sub_pos.mpr h1),
        sq_nonneg (a + b - 2 * c), sq_nonneg (b + c
           $\rightarrow$  - 2 * a), sq_nonneg (c + a - 2 * b)]
  exact h_main

-- Simplified Proof
import Mathlib
import Aesop

set_option maxHeartbeats 0

open BigOperators Real Nat Topology Rat

theorem imo_1983_p6
  (a b c :  $\mathbb{N}$ )
  (h1 : 0 < a  $\wedge$  0 < b  $\wedge$  0 < c)
  (h2 : c < a + b)
  (h3 : b < a + c)
  (h4 : a < b + c) :
  0  $\leq$  a^2 * b * (a - b) + b^2 * c * (b - c) + c^2 *
     $\rightarrow$  a * (c - a) := by
  nlinarith [mul_pos (sub_pos.mpr h1) (sub_pos.mpr
     $\rightarrow$  h1), mul_pos (sub_pos.mpr h1)
     $\rightarrow$  (sub_pos.mpr h1), mul_pos (sub_pos.mpr
     $\rightarrow$  h1) (sub_pos.mpr h1), sq_nonneg (a - b),
     $\rightarrow$  sq_nonneg (b - c), sq_nonneg (c - a)]
  <|>
  -- Orig Proof
  import Mathlib
  import Aesop

set_option maxHeartbeats 0

open BigOperators Real Nat Topology Rat

theorem mathd_numbertheory_427
  (a :  $\mathbb{N}$ )
  (h1 : a = {x k  $\in$  (Nat.divisors 500), k}) :
   $\exists$  k  $\in$  Finset.filter (  $\lambda$  x => Nat.Prime x)
     $\rightarrow$  (Nat.divisors a), k = 25 := by
  have h1 : {x k  $\in$  (Nat.divisors 500), k} = 1092 := by
    rw [show {x k  $\in$  (Nat.divisors 500), k} = 1092 by
       $\rightarrow$  {Nat.divisors}
    ]
    -- We need to compute the sum of all divisors
     $\rightarrow$  of 500.

```

```

  (a b :  $\mathbb{N}$ )
  (h1 : a^2 + b^2 = 1) :
  a * b + |a - b|  $\leq$  1 := by
  have h_main : a * b + |a - b|  $\leq$  1 := by
    cases' le_or_lt 0 (a - b) with h h
    -- Case 1: a - b  $\geq$  0
    have h1 : |a - b| = a - b := by
      rw [abs_of_nonneg h]
    rw [h1]
    have h2 : (a - b) ^ 2 = 1 - 2 * (a * b) := by
      linarith
    have h3 : a * b + (a - b)  $\leq$  1 := by
      linarith [sq_nonneg (a - b - 1)]
    linarith
    -- Case 2: a - b < 0
    have h1 : |a - b| = -(a - b) := by
      rw [abs_of_neg h]
    <|> linarith
    rw [h1]
    have h2 : (a - b) ^ 2 = 1 - 2 * (a * b) := by
      linarith
    have h3 : a * b + -(a - b)  $\leq$  1 := by
      linarith [sq_nonneg (a - b + 1)]
    linarith
  exact h_main

-- Simplified Proof
import Mathlib
import Aesop

set_option maxHeartbeats 0

open BigOperators Real Nat Topology Rat

theorem algebra_sqineq_unitcircatpabsamblt1
  (a b :  $\mathbb{N}$ )
  (h1 : a^2 + b^2 = 1) :
  a * b + |a - b|  $\leq$  1 := by
    nlinarith [abs_mul_abs_self (a - b)]
  <|>
  -- Orig Proof
  import Mathlib
  import Aesop

set_option maxHeartbeats 0

open BigOperators Real Nat Topology Rat

theorem imo_1983_p6
  (a b c :  $\mathbb{N}$ )
  (h1 : 0 < a  $\wedge$  0 < b  $\wedge$  0 < c)
  (h2 : c < a + b)
  (h3 : b < a + c)
  (h4 : a < b + c) :
  0  $\leq$  a^2 * b * (a - b) + b^2 * c * (b - c) + c^2 *
     $\rightarrow$  a * (c - a) := by
  have h_main : 0  $\leq$  a^2 * b * (a - b) + b^2 * c *
     $\rightarrow$  (b - c) + c^2 * a * (c - a) := by
    nlinarith [sq_nonneg (a - b), sq_nonneg (b -
       $\rightarrow$  c), sq_nonneg (c - a),
      mul_nonneg h1.1.le h2.1.le, mul_nonneg
         $\rightarrow$  h2.2.1.le h2.2.2.le, mul_nonneg h1.2.2.le
           $\rightarrow$  h1.1.le,
      mul_nonneg (sq_nonneg (a - b)) h2.2.2.le,
         $\rightarrow$  mul_nonneg (sq_nonneg (b - c)) h1.1.le,
        mul_nonneg (sq_nonneg (c - a)) h2.2.1.le,
         $\rightarrow$  mul_pos h1.1 h2.2.1, mul_pos h1.2.1 h2.2.2,
        mul_pos h2.2.2 h1.1, mul_pos (sub_pos.mpr h1)
           $\rightarrow$  (sub_pos.mpr h1),
        mul_pos (sub_pos.mpr h1) (sub_pos.mpr h1),
         $\rightarrow$  mul_pos (sub_pos.mpr h1) (sub_pos.mpr h1),
        sq_nonneg (a + b - 2 * c), sq_nonneg (b + c
           $\rightarrow$  - 2 * a), sq_nonneg (c + a - 2 * b)]
  exact h_main

-- Simplified Proof
import Mathlib
import Aesop

set_option maxHeartbeats 0

open BigOperators Real Nat Topology Rat

theorem imo_1983_p6
  (a b c :  $\mathbb{N}$ )
  (h1 : 0 < a  $\wedge$  0 < b  $\wedge$  0 < c)
  (h2 : c < a + b)
  (h3 : b < a + c)
  (h4 : a < b + c) :
  0  $\leq$  a^2 * b * (a - b) + b^2 * c * (b - c) + c^2 *
     $\rightarrow$  a * (c - a) := by
  nlinarith [mul_pos (sub_pos.mpr h1) (sub_pos.mpr
     $\rightarrow$  h1), mul_pos (sub_pos.mpr h1)
     $\rightarrow$  (sub_pos.mpr h1), mul_pos (sub_pos.mpr
     $\rightarrow$  h1) (sub_pos.mpr h1), sq_nonneg (a - b),
     $\rightarrow$  sq_nonneg (b - c), sq_nonneg (c - a)]
  <|>
  -- Orig Proof
  import Mathlib
  import Aesop

set_option maxHeartbeats 0

open BigOperators Real Nat Topology Rat

theorem mathd_numbertheory_427
  (a :  $\mathbb{N}$ )
  (h1 : a = {x k  $\in$  (Nat.divisors 500), k}) :
   $\exists$  k  $\in$  Finset.filter (  $\lambda$  x => Nat.Prime x)
     $\rightarrow$  (Nat.divisors a), k = 25 := by
  have h1 : {x k  $\in$  (Nat.divisors 500), k} = 1092 := by
    rw [show {x k  $\in$  (Nat.divisors 500), k} = 1092 by
       $\rightarrow$  {Nat.divisors}
    ]
    -- We need to compute the sum of all divisors
     $\rightarrow$  of 500.

```



```

-- First, we find all divisors of 500 by
-- factoring it into primes: 500 = 2^2 * 5^3.
-- The divisors are all numbers of the form
-- 2^a * 5^b where 0 ≤ a ≤ 2 and 0 ≤ b ≤ 3.
-- We can enumerate them as follows:
-- 1, 2, 4, 5, 10, 20, 25, 50, 100, 125, 250,
-- 500.
-- Their sum is 1 + 2 + 4 + 5 + 10 + 20 + 25 +
-- 50 + 100 + 125 + 250 + 500 = 1092.
-- We will use the fact that the sum of
-- divisors function is multiplicative.
-- For h = p1^e1 * p2^e2 * ... * pk^ek, u(n) =
-- (p1^0 + p1^1 + ... + p1^e1) * ... * (pk^0 +
-- pk^1 + ... + pk^ek).
-- For 500 = 2^2 * 5^3, u(500) = (1 + 2 + 4) *
-- (1 + 5 + 25 + 125) = 7 * 156 = 1092.
-- We can also compute the sum directly by
-- listing all divisors.
-- Here, we will use the multiplicative
-- property to compute the sum.
-- First, we find the sum of divisors of 4
-- (2^2): 1 + 2 + 4 = 7.
-- Next, we find the sum of divisors of 125
-- (5^3): 1 + 5 + 25 + 125 = 156.
-- Then, we multiply these sums: 7 * 156 =
-- 1092.
-- This matches the direct computation.
-- In Lean, we can use the fact that the sum
-- of divisors of 500 is 1092.
-- We can compute the sum of divisors of 500
-- directly by evaluating the sum.
rfl
</> decide

have h : a = 1092 := by
  rw [h]
  rw [h]
  </> rfl

have h : x k ∈ Finset.filter (fun x => Nat.Prime
  => x) (Nat.divisors a), k = 25 := by
  rw [h]
  -- Now we need to find the sum of the prime
  -- divisors of 1092
  -- The prime factorization of 1092 is 2^2 * 3 *
  -- 7 * 13
  -- The prime divisors are 2, 3, 7, 13
  -- Their sum is 2 + 3 + 7 + 13 = 25
  rw [show (x k ∈ Finset.filter (fun x =>
    Nat.Prime x) (Nat.divisors 1092), k) = 25
    by
  rw [show (Finset.filter (fun x => Nat.Prime
    x) (Nat.divisors 1092)) = {2, 3, 7, 13} by
  -- We need to show that the prime divisors
  -- of 1092 are exactly {2, 3, 7, 13}
  apply Finset.ext
  intro x
  simp only [Finset.mem_filter,
    Finset.mem_insert, Finset.mem_singleton,
    Nat.mem_divisors]
  constructor
  -- Prove the forward direction: if x is a
  -- prime divisor of 1092, then x is in {2,
  -- 3, 7, 13}
  have h : x | 1092 := by tauto
  have h : Nat.Prime x := by tauto
  have h : x ≠ 0 := by
    intro h
    rw [h] at h
    norm_num at h
    have h : x ≤ 1092 := Nat.le_of_dvd (by
  → norm_num) h
  interval_cases x <> norm_num
  [Nat.Prime] at h. <>
  (try omega) <> (try norm_num at h.) </>
  <> (try contradiction) <> (try aesop)
  -- Prove the reverse direction: if x is in
  -- {2, 3, 7, 13}, then x is a prime divisor
  -- of 1092
  intro h
  have h : x = 2 ∨ x = 3 ∨ x = 7 ∨ x = 13
  := by aesop
  rcases h with (rfl | rfl | rfl | rfl)
  -- Case x = 2
  norm_num [Nat.Prime]
  <> decide
  -- Case x = 3
  norm_num [Nat.Prime]
  <> decide
  -- Case x = 7
  norm_num [Nat.Prime]
  <> decide
  -- Case x = 13
  norm_num [Nat.Prime]
  <> decide
  ]
  -- Now we need to compute the sum of the
  -- elements in {2, 3, 7, 13}
  norm_num
  </> rfl
]

-- Simplified Proof
import Mathlib
import Aesop

set_option maxHeartbeats 0

open BigOperators Real Nat Topology Rat

theorem mathd_numbertheory_427
(a : ℕ)
(h : a = (x k ∈ (Nat.divisors 500), k)) :

```

```

      field_simp [hh11] at hh11 ⊢
    <|> nlinarith
  exact hh11
  linarith
  exact hh11
  have hh11 : (4 : ℝ) * x ^ 2 / (1 - s) ^ 2 = (s +
    → 1) ^ 2 := by
  have hh11 : (1 - s : ℝ) ^ 2 = (s - 1 : ℝ) ^ 2
    := by
  ring
  rw [hh11]
  rw [hh11]
  have hh11 : (s + 1) ^ 2 < s ^ 2 + 8 := by
  have hh11 : (4 : ℝ) * x ^ 2 / (1 - s) ^ 2 < 2
    → x + 9 = hh11
  have hh11 : (4 : ℝ) * x ^ 2 / (1 - s) ^ 2 =
    → (s + 1) ^ 2 := hh11
  rw [hh11] at hh11
  have hh11 : (s + 1) ^ 2 < 2 * x + 9 := by
  → linarith
  have hh11 : (2 : ℝ) * x = s ^ 2 - 1 := by
  nlinarith [hh11]
  nlinarith [hh11]
  have hh11 : s < 7 / 2 := by
  nlinarith [sq_nonneg (s - 1)]
  have hh11 : s ^ 2 < (7 / 2 : ℝ) ^ 2 := by
  have hh11 : 0 ≤ s := hh11
  have hh11 : s < 7 / 2 := hh11
  nlinarith [sq_nonneg (s - 7 / 2)]
  have hh11 : 1 + 2 * x < (7 / 2 : ℝ) ^ 2 := by
  nlinarith [hh11]
  have hh11 : x < 45 / 8 := by
  norm_num at hh11 ⊢
  <|> nlinarith
  exact hh11

exact (hh, hh)

-- Simplified Proof
import Mathlib
import Aesop

set_option maxHeartbeats 0

open BigOperators Real Nat Topology Rat

theorem imo_1960_p2
  (x : ℝ)
  (hh : 0 ≤ 1 + 2 * x)
  (hh : (1 - Real.sqrt (1 + 2 * x)) ^ 2 ≠ 0)
  (hh : (4 * x ^ 2) / (1 - Real.sqrt (1 + 2 * x)) ^ 2 <
    → 2 * x + 9)
  (hh : x ≠ 0) :
  ¬(1 / 2) ≤ x ∧ x < 45 / 8 := by
  constructor
  nlinarith [sq_nonneg (x + 1 / 2)]
  · have hh : (4 : ℝ) * x ^ 2 / (1 - Real.sqrt (1 +
    → 2 * x)) ^ 2 = (1 + Real.sqrt (1 + 2 * x))
    → ^ 2 := by
  have hh : (1 - Real.sqrt (1 + 2 * x)) ^ 2 ≠
    → 0 := by assumption
  field_simp [hh]
  nlinarith [sq_sqrt (show 0 ≤ 1 + 2 * x by
    → assumption)]
  nlinarith [sq_sqrt (show 0 ≤ 1 + 2 * x by
    → assumption),
    Real.sqrt_nonneg (1 + 2 * x)]

-----
-- Orig Proof
import Mathlib
import Aesop

set_option maxHeartbeats 0

open BigOperators Real Nat Topology Rat

theorem imo_1963_p5 :
  Real.cos (π / 7) - Real.cos (2 * π / 7) +
    → Real.cos (3 * π / 7) = 1 / 2 := by
  have hh : 2 * Real.sin (π / 7) * (Real.cos (π /
    → 7) - Real.cos (2 * π / 7) * Real.cos (3 *
    → π / 7)) = Real.sin (π / 7) := by
  have hh : 2 * Real.sin (π / 7) * Real.cos (π /
    → 7) = Real.sin (2 * π / 7) := by
  have hh : Real.sin (2 * π / 7) = 2 * Real.sin
    → (π / 7) * Real.cos (π / 7) := by
  have hh : Real.sin (2 * π / 7) = Real.sin
    → (2 * (π / 7)) := by ring
  rw [hh]
  have hh : Real.sin (2 * (π / 7)) = 2 *
    → Real.sin (π / 7) * Real.cos (π / 7) := by
  rw [Real.sin_two_mul]
  <|> ring
  rw [hh]
  <|> ring
  linarith
  have hh : 2 * Real.sin (π / 7) * Real.cos (π /
    → 7) - 2 * Real.sin (π / 7) * Real.cos (2 *
    → π / 7) + 2 * Real.sin (π / 7) * Real.cos
    → (3 * π / 7) = Real.sin (2 * π / 7) -
    → (Real.sin (3 * π / 7) + Real.sin (-(π /
    → 7))) + (Real.sin (4 * π / 7) + Real.sin
    → -(2 * π / 7))) := by
  rw [hh, hh, hh]
  <|> ring
  rw [hh]
  have hh : Real.sin (4 * π / 7) = Real.sin (3 * π
    → / 7) := by
  have hh : Real.sin (4 * π / 7) = Real.sin (π
    → - 3 * π / 7) := by
  have hh : 4 * π / 7 = π - 3 * π / 7 := by
  → ring
  rw [hh]
  rw [hh]
  have hh : Real.sin (π - 3 * π / 7) = Real.sin
    → (3 * π / 7) := by
  rw [Real.sin_pi_sub]
  rw [hh]
  have hh : Real.sin (-(2 * π / 7)) = -Real.sin
    → (2 * π / 7) := by
  rw [- Real.sin_neg]
  <|> ring_nf
  rw [hh, hh, hh]
  have hh : Real.sin (2 * π / 7) - (Real.sin (3 *
    → π / 7) + -Real.sin (π / 7)) + (Real.sin
    → (3 * π / 7) + Real.sin (2 * π / 7)) =
    → Real.sin (π / 7) := by
  <|> ring_nf
  (try norm_num) <|>
  (try linarith [Real.pi_pos]) <|>
  (try field_simp) <|>
  (try ring_nf) <|>
  (try norm_num) <|>
  (try linarith [Real.pi_pos])

linarith
have hh : Real.sin (π / 7) ≠ 0 := by
  have hh : 0 < π / 7 := by linarith [Real.pi_pos]
  have hh : π / 7 < π := by linarith [Real.pi_pos]
  have hh : 0 < Real.sin (π / 7) :=
    → Real.sin_pos_of_pos_of_lt_pi hh hh
  linarith
have hh : Real.cos (π / 7) - Real.cos (2 * π / 7)
  → + Real.cos (3 * π / 7) = 1 / 2 := by
  have hh : 2 * Real.sin (π / 7) * (Real.cos (π /
    → 7) - Real.cos (2 * π / 7) + Real.cos (3 *
    → π / 7)) = Real.sin (π / 7) := hh
  have hh : Real.sin (π / 7) ≠ 0 := hh
  have hh : Real.cos (π / 7) - Real.cos (2 * π /
    → 7) + Real.cos (3 * π / 7) = 1 / 2 := by
  apply mul_left_cancel, hh
  nlinarith [Real.sin_le_one (π / 7),
    → Real.cos_le_one (π / 7), Real.sin_le_one
    → (2 * π / 7),
    → Real.cos_le_one (2 * π / 7),
    → Real.sin_le_one (3 * π / 7),
    → Real.cos_le_one (3 * π / 7)]
  exact hh

-- Simplified Proof
import Mathlib
import Aesop

set_option maxHeartbeats 0

open BigOperators Real Nat Topology Rat

theorem imo_1963_p5 :
  Real.cos (π / 7) - Real.cos (2 * π / 7) +
    → Real.cos (3 * π / 7) = 1 / 2 := by
  have hh : 2 * Real.sin (π / 7) * (Real.cos (π /
    → 7) - Real.cos (2 * π / 7) * Real.cos (3 *
    → π / 7)) = Real.sin (π / 7) := by
  have hh : 2 * Real.sin (π / 7) * Real.cos (π /
    → 7) = Real.sin (2 * π / 7) := by
  have hh : Real.sin (2 * π / 7) = 2 * Real.sin
    → (π / 7) * Real.cos (π / 7) := by
  have hh : Real.sin (2 * π / 7) = Real.sin
    → (2 * (π / 7)) := by ring
  rw [hh]
  have hh : Real.sin (2 * (π / 7)) = 2 *
    → Real.sin (π / 7) * Real.cos (π / 7) := by
  rw [Real.sin_two_mul]
  <|> ring
  rw [hh]
  <|> ring
  linarith
  have hh : 2 * Real.sin (π / 7) * Real.cos (π /
    → 7) - 2 * Real.sin (π / 7) * Real.cos (2 *
    → π / 7) + 2 * Real.sin (π / 7) * Real.cos
    → (3 * π / 7) = Real.sin (2 * π / 7) -
    → (Real.sin (3 * π / 7) + Real.sin (-(π /
    → 7))) + (Real.sin (4 * π / 7) + Real.sin
    → -(2 * π / 7))) := by
  rw [hh, hh, hh]
  <|> ring
  rw [hh]
  have hh : Real.sin (4 * π / 7) = Real.sin (3 * π
    → / 7) := by
  have hh : Real.sin (4 * π / 7) = Real.sin (π
    → - 3 * π / 7) := by
  have hh : 4 * π / 7 = π - 3 * π / 7 := by
  → ring
  rw [hh]
  rw [hh]
  have hh : Real.sin (π - 3 * π / 7) = Real.sin
    → (3 * π / 7) := by
  rw [Real.sin_pi_sub]
  rw [hh]
  have hh : Real.sin (-(2 * π / 7)) = -Real.sin
    → (2 * π / 7) := by
  rw [- Real.sin_neg]
  <|> ring_nf
  rw [hh, hh, hh]
  have hh : Real.sin (2 * π / 7) - (Real.sin (3 *
    → π / 7) + -Real.sin (π / 7)) + (Real.sin
    → (3 * π / 7) + Real.sin (2 * π / 7)) =
    → Real.sin (π / 7) := by
  <|> ring_nf
  (try norm_num) <|>
  (try linarith [Real.pi_pos]) <|>
  (try field_simp) <|>
  (try ring_nf) <|>
  (try norm_num) <|>
  (try linarith [Real.pi_pos])

linarith

```

```

have h10 : Real.sin (π / 7 + 3 * π / 7) =
  → Real.sin (4 * π / 7) := by
have h11 : π / 7 + 3 * π / 7 = 4 * π / 7 :=
  → by ring
rw [h11]
have h12 : Real.sin (π / 7 - 3 * π / 7) =
  → Real.sin (- (2 * π / 7)) := by
have h13 : π / 7 - 3 * π / 7 = - (2 * π / 7)
  → := by ring
rw [h13]
have [h10, h12, h13]
have h14 : 2 * Real.sin (π / 7) * (Real.cos (π /
  → 7) - Real.cos (2 * π / 7) + Real.cos (3 *
  → π / 7)) = Real.sin (2 * π / 7) -
  → (Real.sin (3 * π / 7) + Real.sin (- (π /
  → 7))) + (Real.sin (4 * π / 7) + Real.sin
  → (- (2 * π / 7))) := by
linarith
rw [h14]
have h15 : Real.sin (4 * π / 7) = Real.sin (3 * π
  → / 7) := by
have h16 : Real.sin (4 * π / 7) = Real.sin (π
  → - 3 * π / 7) := by
have h17 : 4 * π / 7 = π - 3 * π / 7 := by
  → ring
rw [h17]
have h18 : Real.sin (π - 3 * π / 7) = Real.sin
  → (3 * π / 7) := by
  → rw [Real.sin_pi_sub]
  → rw [h18]
have h19 : Real.sin (- (2 * π / 7)) = -Real.sin
  → (2 * π / 7) := by
  → rw [- Real.sin_neg]
have h20 : Real.sin (- (π / 7)) = -Real.sin (π /
  → 7) := by
  → rw [- Real.sin_neg]
  → rw [h20, h19]
linarith
have h21 : Real.sin (π / 7) ≠ 0 := by
have h22 : 0 < π / 7 := by linarith [Real.pi_pos]
have h23 : π / 7 < π := by linarith [Real.pi_pos]
have h24 : 0 < Real.sin (π / 7) :=
  → Real.sin_pos_of_pos_of_lt_pi h22 h23
linarith
apply mul_left_cancel, h24
mlinarith [Real.sin_le_one (π / 7),
  → Real.cos_le_one (π / 7), Real.sin_le_one
  → (2 * π / 7),
  → Real.cos_le_one (2 * π / 7), Real.sin_le_one (3
  → * π / 7), Real.cos_le_one (3 * π / 7)]
-----
-- Orig Proof
import Mathlib
import Aesop

set_option maxHeartbeats 0

open BigOperators Real Nat Topology Rat

theorem mathd_numbertheory_430
(a b c : ℕ)
(h1 : 1 ≤ a ∧ a ≤ 9)
(h2 : 1 ≤ b ∧ b ≤ 9)
(h3 : 1 ≤ c ∧ c ≤ 9)
(h4 : a ≠ b)
(h5 : a ≠ c)
(h6 : b ≠ c)
(h7 : a + b = c)
(h8 : 10 * a + a - b = 2 * c)
(h9 : c * b = 10 * a + a + a) :
a + b + c = 8 := by
revert h1 h2 h3 h4 h5 h6 h7 h8
norm_num
intros
interval_cases a <> interval_cases b <>
  → interval_cases c <> simp_all
-----
-- Orig Proof
import Mathlib
import Aesop

set_option maxHeartbeats 0

open BigOperators Real Nat Topology Rat

theorem induction_12dvd4expnpip20
(n : ℕ) :
12 ∣ 4(n+1) + 20 := by
have hmain : 12 ∣ 4(n+1) + 20 := by
  apply Nat.dvd_of_mod_eq_zero
  have h1 : (4(n+1) + 20) % 12 = 0 := by
    have h2 : ∀ n : ℕ, (4(n+1) + 20) % 12 = 0 :=
      → by
        intro n
        induction n with
        | zero =>
          norm_num
        | succ n ih =>
          simp [pow_succ, Nat.mul_mod,
            → Nat.add_mod] at ih +
            <> omega
          exact h2 n
          exact h
          exact hmain
-----
-- Simplified Proof
import Mathlib
import Aesop

set_option maxHeartbeats 0

open BigOperators Real Nat Topology Rat

theorem induction_12dvd4expnpip20
(n : ℕ) :
12 ∣ 4(n+1) + 20 := by
  induction n <> omega
-----
-- Orig Proof
import Mathlib
import Aesop

set_option maxHeartbeats 0

open BigOperators Real Nat Topology Rat

theorem mathd_algebra_459
(a b c d : ℕ)
(h1 : 3 * a = b + c + d)
(h2 : 4 * b = a + c + d)
(h3 : 2 * c = a + b + d)
(h4 : 8 * a + 10 * b + 6 * c = 24) :
d.den + d.num = 28 := by
have h5 : 5 * b = 4 * a := by
  have h6 : 4 * b - 3 * a = a - b := by
    linarith
  linarith
have h7 : 3 * c = 4 * a := by
  have h8 : 2 * c - 3 * a = a - c := by
    linarith
  linarith
have h9 : a = 1 := by
  have h10 : 24 * a = 24 := by
    have h11 : 8 * a + 10 * b + 6 * c = 24 := h4
    have h12 : 5 * b = 4 * a := h5
    have h13 : 3 * c = 4 * a := h7
    have h14 : 10 * b = 8 * a := by linarith
    have h15 : 6 * c = 8 * a := by linarith
    linarith
  have h16 : b = 4 / 5 := by
    have h17 : 5 * b = 4 * a := h5
    rw [h17] at h16
    norm_num at h16 +
    <> linarith
  have h18 : c = 4 / 3 := by
    have h19 : 3 * c = 4 * a := h7
    rw [h19] at h18
    norm_num at h18 +
    <> linarith
  have h20 : d = 13 / 15 := by
    have h21 : 3 * a = b + c + d := h1
    rw [h21, h16, h18] at h20
    norm_num at h20 +
    <> linarith
-----
have hfinal : a + b + c = 8 := by
  rcases hmain with (rfl, rfl, rfl)
  <> norm_num
  <> aesop
exact hfinal

```

```

theorem mathd_algebra_160
  (n x : ℕ)
  (h₁ : n + x = 97)
  (h₂ : n + 5 * x = 265) :
  n + 2 * x = 139 := by
  have h₃ : x = 42 := by
    have h₄ : 4 * x = 168 := by
      have h₅ : (n + 5 * x) - (n + x) = 265 - 97 :=
        by
          linarith
    linarith
  -- Solve for x using the equation 4x = 168
  linarith

have h₆ : n = 55 := by
have h₇ : n + x = 97 := h₆
rw [h₇] at h₁
linarith

have h₈ : n + 2 * x = 139 := by
rw [h₈, h₇]
<> norm_num

exact h₈

-- Simplified Proof
import Mathlib
import Aesop

set_option maxHeartbeats 0

open BigOperators Real Nat Topology Rat

theorem mathd_algebra_160
  (n x : ℕ)
  (h₁ : n + x = 97)
  (h₂ : n + 5 * x = 265) :
  n + 2 * x = 139 := by
  linarith
  -----
  -- Orig Proof
  import Mathlib
  import Aesop

  set_option maxHeartbeats 0

  open BigOperators Real Nat Topology Rat

  theorem mathd_numbertheory_277
    (m n : ℕ)
    (h₁ : Nat.gcd m n = 6)
    (h₂ : Nat.lcm m n = 126) :
    60 ≤ m + n := by
    have h₃ : m * n = 756 := by
      rw [Nat.gcd_mul_lcm m n]
      simp_all
    have h₄ : 6 ∣ m := Nat.dvd_of_mod_eq_zero (by rw
      → [- h₁]; exact Nat.mod_eq_zero_of_dvd
      → (Nat.gcd_dvd_left m n))
    have h₅ : 6 ∣ n := Nat.dvd_of_mod_eq_zero (by rw
      → [- h₁]; exact Nat.mod_eq_zero_of_dvd
      → (Nat.gcd_dvd_right m n))
    obtain (a, rfl) := h₄
    obtain (b, rfl) := h₅
    have h₆ : a * b = 21 := by
      linarith
    have h₇ : 60 ≤ 6 * (a + b) := by
      have h₈ : a ≤ 21 := Nat.le_of_dvd (by
        → norm_num) (by use b; linarith)
      have h₉ : b ≤ 21 := Nat.le_of_dvd (by
        → norm_num) (by use a; linarith)
      interval_cases a <> norm_num at h₈ h₉ <> omega
      linarith
  -----
  -- Orig Proof
  import Mathlib
  import Aesop

  set_option maxHeartbeats 0

  open BigOperators Real Nat Topology Rat

  theorem mathd_numbertheory_559
    (x y : ℕ)
    (h₁ : x % 3 = 2)
    (h₂ : y % 5 = 4)
    (h₃ : x % 10 = y % 10) :
    14 ≤ x := by
    have h₄_main : 14 ≤ x := by
      by_contra! h
      have h₅ : x ≤ 13 := by linarith
      have h₆ : x % 3 = 2 := h₅
      have h₇ : y % 5 = 4 := h₅
      have h₈ : x % 10 = y % 10 := h₅
      have h₉ : x ≤ 13 := by linarith
      interval_cases x <> norm_num
      → [Nat.mod_eq_of_lt] at h₅ h₆ h₉ <>
      (try omega) <>
      (try {
        have h₁₀ : y % 5 = 4 := h₇
        have h₁₁ : y % 10 = 4 := by omega
        have h₁₂ : y % 5 = 4 := h₁₁
        omega
      }) <>
      (try {
        have h₁₃ : y % 5 = 4 := h₇
        have h₁₄ : y % 10 = 4 := by omega
        omega
      })
    exact h₄_main

  -- Simplified Proof
  import Mathlib
  import Aesop

  set_option maxHeartbeats 0

  open BigOperators Real Nat Topology Rat

  theorem mathd_numbertheory_559
    (x y : ℕ)
    (h₁ : x % 3 = 2)
    (h₂ : y % 5 = 4)
    (h₃ : x % 10 = y % 10) :
    14 ≤ x := by
    omega
  -----
  -- Orig Proof
  import Mathlib
  import Aesop

  set_option maxHeartbeats 0

  open BigOperators Real Nat Topology Rat

  theorem mathd_algebra_24
    (x : ℝ)
    (h₁ : x / 50 = 40) :
    x = 2000 := by
    linarith
  -----
  -- Orig Proof
  import Mathlib
  import Aesop

  set_option maxHeartbeats 0

  open BigOperators Real Nat Topology Rat

  theorem mathd_algebra_176
    (x : ℝ) :
    (x + 1)² * x = x³ + 2 * x² + x := by
    have h_main : (x + 1)² * x = x³ + 2 * x² + x
      → := by
        ring_nf
        <>
        (try norm_num)
        <>
        (try linarith)
        <>
        (try nlinarith)

    apply h_main

  -- Simplified Proof
  import Mathlib
  import Aesop

  set_option maxHeartbeats 0

  open BigOperators Real Nat Topology Rat

  theorem mathd_algebra_176
    (x : ℝ) :
    (x + 1)² * x = x³ + 2 * x² + x := by
    ring
  -----
  -- Orig Proof
  import Mathlib
  import Aesop

  set_option maxHeartbeats 0

  open BigOperators Real Nat Topology Rat

  theorem mathd_numbertheory_353
    (s : ℕ)
    (h₁ : s = ∑ k ∈ Finset.Icc 2010 4018, k) :
    s % 2009 = 0 := by
    have h₂ : ∑ k ∈ Finset.Icc 2010 4018, k = 2009 *
      → 3014 := by
      have h₃ : ∑ k ∈ Finset.Icc 2010 4018, k = ∑ k
        → in Finset.range 4019, k - ∑ k in
        → Finset.range 2010, k := by
        have h₄ : ∑ k ∈ Finset.range 4019, k = ∑ k
          → in Finset.range 2010, k + ∑ k in
          → Finset.Ico 2010 4019, k := by
          rw [Finset.sum_range_add_sum_Ico _ (by
            → norm_num : 2010 ≤ 4019)]
          <> simp [add_comm]
        have h₅ : ∑ k ∈ Finset.Ico 2010 4019, k = ∑
          → k in Finset.range 4019, k - ∑ k in
          → Finset.range 2010, k := by
          omega
        rw [h₃]
      rw [h₂]
    have h₃ : ∑ k ∈ Finset.range 4019, k = 4019 *
      → 4018 / 2 := by
      rw [Finset.sum_range_id]
      <> rfl
    have h₄ : ∑ k ∈ Finset.range 2010, k = 2010 *
      → 2009 / 2 := by
      rw [Finset.sum_range_id]
      <> rfl
    rw [h₃, h₄]
    <> norm_num
    <> rfl

    exact h₃

  -- Simplified Proof
  import Mathlib
  import Aesop

  set_option maxHeartbeats 0

  open BigOperators Real Nat Topology Rat

  theorem mathd_numbertheory_353
    (s : ℕ)
    (h₁ : s = ∑ k ∈ Finset.Icc 2010 4018, k) :
    s % 2009 = 0 := by
    rw [h₁]
    have : ∑ k ∈ Finset.Icc 2010 4018, k = 2009 *
      → 3014 := by

```



```

open BigOperators Real Nat Topology Rat

theorem mathd_numbertheory_447 :
  ∃ k ∈ Finset.filter (· x => 3x) (Finset.Icc 1
    → 49), (k % 10) = 78 := by
  have h : ∃ k ∈ Finset.filter (· x => 3x)
    → (Finset.Icc 1 49), (k % 10) = 78 := by
    rfl
  apply h

-- Simplified Proof
import Mathlib
import Aesop

set_option maxHeartbeats 0

open BigOperators Real Nat Topology Rat

theorem mathd_numbertheory_447 :
  ∃ k ∈ Finset.filter (· x => 3x) (Finset.Icc 1
    → 49), (k % 10) = 78 := by
  rfl
  -----
-- Orig Proof
import Mathlib
import Aesop

set_option maxHeartbeats 0

open BigOperators Real Nat Topology Rat

theorem mathd_numbertheory_328 :
  (5^999999) % 7 = 6 := by
  have h_main : (5^999999) % 7 = 6 := by
    norm_num [pow_succ, Nat.mul_mod, Nat.pow_mod]
  <|> rfl

  apply h_main

-- Simplified Proof
import Mathlib
import Aesop

set_option maxHeartbeats 0

open BigOperators Real Nat Topology Rat

theorem mathd_numbertheory_328 :
  (5^999999) % 7 = 6 := by
  norm_num
  -----
-- Orig Proof
import Mathlib
import Aesop

set_option maxHeartbeats 0

open BigOperators Real Nat Topology Rat

theorem algebra_sqineq_at2malt1
  (a : ℝ) :
  a * (2 - a) ≤ 1 := by
  have h_main : a * (2 - a) ≤ 1 := by
    have h₁ : a * (2 - a) = 2 * a - a ^ 2 := by
      ring
    rw [h₁]
    have h₂ : 2 * a - a ^ 2 ≤ 1 := by
      nlinarith [sq_nonneg (a - 1)]
    exact h
  exact h_main

-- Simplified Proof
import Mathlib
import Aesop

set_option maxHeartbeats 0

open BigOperators Real Nat Topology Rat

theorem algebra_sqineq_at2malt1
  (a : ℝ) :
  a * (2 - a) ≤ 1 := by
  nlinarith [sq_nonneg (a - 1)]
  -----
-- Orig Proof
import Mathlib
import Aesop

set_option maxHeartbeats 0

open BigOperators Real Nat Topology Rat

theorem mathd_algebra_171
  (f : ℝ → ℝ)
  (h : ∀ x, f x = 5 * x + 4) :
  f 1 = 9 := by
  have h₁ : f 1 = 9 := by
    have h₂ : f 1 = 5 * (1 : ℝ) + 4 := by
      rw [h]
    <|> norm_num
  <|> norm_num
  exact h₁

-- Simplified Proof
import Mathlib
import Aesop

set_option maxHeartbeats 0

open BigOperators Real Nat Topology Rat

theorem mathd_algebra_171
  (f : ℝ → ℝ)
  (h : ∀ x, f x = 5 * x + 4) :
  f 1 = 9 := by
  simp_all
  norm_num
  -----
-- Orig Proof

```

```

import Mathlib
import Aesop

set_option maxHeartbeats 0

open BigOperators Real Nat Topology Rat

theorem mathd_algebra_188
  (ω : Equiv ℝ ℝ)
  (h : ω.1 2 = ω.2 2) :
  ω.1 (ω.1 2) = 2 := by
  have h₁ : ω.1 (ω.2 2) = 2 := by
    apply Equiv.apply_symm_apply

  have h₂ : ω.1 (ω.1 2) = 2 := by
    calc
      ω.1 (ω.1 2) = ω.1 (ω.2 2) := by
        rw [h]
      = 2 := h₁

  exact h₁

-- Simplified Proof
import Mathlib
import Aesop

set_option maxHeartbeats 0

open BigOperators Real Nat Topology Rat

theorem mathd_algebra_188
  (ω : Equiv ℝ ℝ)
  (h : ω.1 2 = ω.2 2) :
  ω.1 (ω.1 2) = 2 := by
  simp_all
  -----
-- Orig Proof
import Mathlib
import Aesop

set_option maxHeartbeats 0

open BigOperators Real Nat Topology Rat

theorem imo_1959_p1
  (n : ℕ)
  (h₀ : 0 < n) :
  Nat.gcd (21*n + 4) (14*n + 3) = 1 := by
  have h₁ : Nat.gcd (21*n + 4) (14*n + 3) = Nat.gcd
    (14*n + 3) (7*n + 1) := by
    have h₂ : 21 * n + 4 = 1 * (14 * n + 3) + (7 *
      n + 1) := by
      ring_nf
    <|> omega
  <|> simp [Nat.gcd_comm,
    → Nat.gcd_add_mul_right_right,
    → Nat.gcd.assoc]
  <|> ring_nf at *
  <|> norm_num
  <|> omega

  have h₂ : Nat.gcd (14*n + 3) (7*n + 1) = 1 := by
    have h₃ : 14 * n + 3 = 2 * (7 * n + 1) + 1 :=
      by
      ring_nf
    <|> omega
  rw [h₃]
  <|> simp [Nat.gcd_comm,
    → Nat.gcd_add_mul_right_right,
    → Nat.gcd.assoc]
  <|> ring_nf at *
  <|> norm_num
  <|> omega

  have h₃ : Nat.gcd (21*n + 4) (14*n + 3) = 1 := by
    rw [h₁]
    rw [h₃]

  exact h₁

-- Simplified Proof
import Mathlib
import Aesop

set_option maxHeartbeats 0

open BigOperators Real Nat Topology Rat

theorem imo_1959_p1
  (n : ℕ)
  (h₀ : 0 < n) :
  Nat.gcd (21*n + 4) (14*n + 3) = 1 := by
  rw [Nat.gcd_comm]
  rw [show 21 * n + 4 = 1 * (14 * n + 3) + (7 * n +
    1) by ring]
  rw [show 14 * n + 3 = 2 * (7 * n + 1) + 1 by
    → ring]
  simp
  -----
-- Orig Proof
import Mathlib
import Aesop

set_option maxHeartbeats 0

open BigOperators Real Nat Topology Rat

theorem mathd_numbertheory_175 :
  (2^2010) % 10 = 4 := by
  have h_main : (2^2010) % 10 = 4 := by
    norm_num
  <|> rfl

  exact h_main

-- Simplified Proof
import Mathlib
import Aesop

```

```

set_option maxHeartbeats 0

open BigOperators Real Nat Topology Rat

theorem mathd_numbertheory_175 :
  (2^2010) % 10 = 4 := by
  norm_num
  -----
-- Orig Proof
import Mathlib
import Aesop

set_option maxHeartbeats 0

open BigOperators Real Nat Topology Rat

theorem mathd_numbertheory_227
  (x y n : ℕ+)
  (h₀ : (x / (4 : ℝ) + y / 6 = (x + y) / n) :
  n = 5 := by
  have h₁ : (n : ℝ) * (3 * (x : ℝ) + 2 * (y : ℝ)) =
    → 12 * ((x : ℝ) + (y : ℝ)) := by
    have h₂ : ((x : ℝ) / 4 + (y : ℝ) / 6 = (x + y
      : ℝ) / (n : ℝ)) := by
      norm_cast at h₀
    <|> simp_all [PNat.ne_zero]
    <|> field_simp at h₀ <|> ring_nf at h₀ <|>
      → nlinarith
  have h₃ : (n : ℝ) ≠ 0 := by
    norm_cast
    <|> exact PNat.ne_zero n
  field_simp at h₂ <|>
    ring_nf at h₂
  nlinarith [sq_pos_of_pos (show (0 : ℝ) < (n : ℝ
    → ) by exact_mod_cast n.prop)]

  have h₄ : (4 : ℝ) < (n : ℝ) := by
    have h₅ : 0 < (x : ℝ) := by exact_mod_cast
    → x.prop
  have h₆ : 0 < (y : ℝ) := by exact_mod_cast
    → y.prop
  have h₇ : 0 < (n : ℝ) := by exact_mod_cast
    → n.prop
  have h₈ : (n : ℝ) * (3 * (x : ℝ) + 2 * (y : ℝ
    → )) = 12 * ((x : ℝ) + (y : ℝ)) := h₁
  have h₉ : (4 : ℝ) < (n : ℝ) := by
    by_contra h
    have h₁₀ : (n : ℝ) ≤ 4 := by linarith
    have h₁₁ : (n : ℝ) * (3 * (x : ℝ) + 2 * (y : ℝ
      → )) ≤ 4 * (3 * (x : ℝ) + 2 * (y : ℝ)) := by
      nlinarith
    have h₁₂ : 12 * ((x : ℝ) + (y : ℝ)) ≤ 4 * (3 *
      → (x : ℝ) + 2 * (y : ℝ)) := by
      linarith
    have h₁₃ : (y : ℝ) > 0 := by positivity
    nlinarith
  exact h₃

  have h₄ : (n : ℝ) < (6 : ℝ) := by
    have h₅ : 0 < (x : ℝ) := by exact_mod_cast
    → x.prop
  have h₆ : 0 < (y : ℝ) := by exact_mod_cast
    → y.prop
  have h₇ : 0 < (n : ℝ) := by exact_mod_cast
    → n.prop
  have h₈ : (n : ℝ) * (3 * (x : ℝ) + 2 * (y : ℝ
    → )) = 12 * ((x : ℝ) + (y : ℝ)) := h₁
  have h₉ : (n : ℝ) < (6 : ℝ) := by
    by_contra h
    have h₁₀ : (n : ℝ) ≥ 6 := by linarith
    have h₁₁ : (n : ℝ) * (3 * (x : ℝ) + 2 * (y : ℝ
      → )) ≥ 6 * (3 * (x : ℝ) + 2 * (y : ℝ)) := by
      nlinarith
    have h₁₂ : 12 * ((x : ℝ) + (y : ℝ)) ≥ 6 * (3 *
      → (x : ℝ) + 2 * (y : ℝ)) := by
      linarith
    have h₁₃ : (x : ℝ) > 0 := by positivity
    nlinarith
  exact h₃

  have h₄ : n = 5 := by
    have h₅ : (n : ℕ) = 5 := by
      have h₆ : (n : ℝ) > 4 := h₄
      have h₇ : (n : ℝ) < 6 := h₄
      have h₈ : (n : ℕ) > 4 := by
        norm_cast at h₆ <|>
          <|>
            (try norm_num at h₆ <|>
              (try linarith) <|>
                (try omega))
      have h₉ : (n : ℕ) < 6 := by
        norm_cast at h₇ <|>
          <|>
            (try norm_num at h₇ <|>
              (try linarith) <|>
                (try omega))
      have h₁₀ : (n : ℕ) = 5 := by
        omega
      exact h₅
    exact by
      norm_cast at h₅ <|>
        <|>
          (try simp_all) <|>
            (try omega)

  exact h₄

-- Simplified Proof
import Mathlib
import Aesop

set_option maxHeartbeats 0

open BigOperators Real Nat Topology Rat

theorem mathd_numbertheory_227
  (x y n : ℕ+)

```



```

(h₁ : x / (4 : ℝ) + y / 6 = (x + y) / n) :
n = 5 := by
have h₁ : (n : ℝ) * (3 * (x : ℝ) + 2 * (y : ℝ)) =
→ 12 * ((x : ℝ) + (y : ℝ)) := by
field_simp at h₁
ring_nf at h₁
nlinarith [sq_pos_of_pos (show (0 : ℝ) < (n : ℝ)
→) by exact_mod_cast n.prop]]
have h₂ : (4 : ℝ) < (n : ℝ) := by
have h₂ : 0 < (x : ℝ) := by exact_mod_cast
→ x.prop
have h₂ : 0 < (y : ℝ) := by exact_mod_cast
→ y.prop
have h₂ : 0 < (n : ℝ) := by exact_mod_cast
→ n.prop
have h₂ : (n : ℝ) * (3 * (x : ℝ) + 2 * (y : ℝ)
→)) = 12 * ((x : ℝ) + (y : ℝ)) := h₁
nlinarith
have h₃ : (n : ℝ) < (6 : ℝ) := by
have h₃ : 0 < (x : ℝ) := by exact_mod_cast
→ x.prop
have h₃ : 0 < (y : ℝ) := by exact_mod_cast
→ y.prop
have h₃ : 0 < (n : ℝ) := by exact_mod_cast
→ n.prop
have h₃ : (n : ℝ) * (3 * (x : ℝ) + 2 * (y : ℝ)
→)) = 12 * ((x : ℝ) + (y : ℝ)) := h₁
nlinarith
have h₄ : n = 5 := by
have h₄ : (n : ℕ) = 5 := by
have h₄ : (n : ℝ) > 4 := h₁
have h₄ : (n : ℝ) < 6 := h₃
have h₄ : (n : ℕ) > 4 := by
norm_cast at h₄
have h₄ : (n : ℕ) < 6 := by
norm_cast at h₄
omega
exact by
norm_cast at h₄
exact h₄
-----
-- Orig Proof
import Mathlib
import Aesop

set_option maxHeartbeats 0

open BigOperators Real Nat Topology Rat

theorem aime_1997_p9
(a : ℝ)
(h₁ : 0 < a)
(h₂ : 1 / a - Int.floor (1 / a) = a² - Int.floor
→ (a²))
(h₃ : 2 < a²)
(h₄ : a² < 3) :
a¹² - 144 * (1 / a) = 233 := by
have h_floor_a2 : Int.floor (a² : ℝ) = 2 := by
have h₁ : (2 : ℝ) ≤ a² := by linarith
have h₂ : a² < (3 : ℝ) := by linarith
have h₃ : Int.floor (a² : ℝ) = 2 := by
rw [Int.floor_eq_iff]
rw [norm_num at h₁, h₂]
constructor <> nlinarith
exact h₃
have h_a_gt_1 : a > 1 := by
by.contra h
have h₁ : a ≤ 1 := by linarith
have h₂ : a² ≤ 1 := by
have h₂ : 0 < a := h₁
have h₂ : a ≤ 1 := h₁
nlinarith
linarith
have h_floor_1a : Int.floor ((1 : ℝ) / a) = 0 :=
→ by
have h₁ : 0 < (1 : ℝ) / a := by positivity
have h₂ : (1 : ℝ) / a < 1 := by
have h₃ : a > 1 := h_a_gt_1
have h₄ : (1 : ℝ) / a < 1 := by
rw [div_lt_one (by positivity)]
<> nlinarith
exact h₄
have h₃ : Int.floor ((1 : ℝ) / a) = 0 := by
rw [Int.floor_eq_iff]
norm_num at h₁, h₂
constructor <> norm_num <>
(try norm_num at h₁, h₂) <>
(try linarith) <>
{
have h₁ : 0 < a := by positivity
have h₂ : 0 < (1 : ℝ) / a := by positivity
have h₃ : (1 : ℝ) / a < 1 := h₁
linarith
}
exact h₃
have h_main_eq : (1 : ℝ) / a = a² - 2 := by
have h₁ : (1 : ℝ) / a - Int.floor ((1 : ℝ) / a)
→ = a² - Int.floor (a² : ℝ) := by
exact_mod_cast h₁
have h₂ : (Int.floor ((1 : ℝ) / a) : ℝ) = 0 :=
→ by
norm_cast
<> simp [h_floor_1a]
have h₃ : (Int.floor (a² : ℝ) : ℝ) = 2 := by
norm_cast
<> simp [h_floor_a2]
rw [h₁, h₂] at h₃
ring_nf at h₃
linarith
have h_cubic : a³ - 2*a - 1 = 0 := by
have h₁ : (1 : ℝ) / a = a² - 2 := h_main_eq
have h₂ : a ≠ 0 := by linarith

```

```

exact h
-- Simplified Proof
import Mathlib
import Aesop

set_option maxHeartbeats 0

open BigOperators Real Nat Topology Rat

theorem mathd_numbertheory_728 :
  (29^13 - 5^13) % 7 = 3 := by
  norm_num
  -----
-- Orig Proof
import Mathlib
import Aesop

set_option maxHeartbeats 0

open BigOperators Real Nat Topology Rat

theorem mathd_algebra_487
  (a b c d : ℝ)
  (h₁ : b = a^2)
  (h₂ : a + b = 1)
  (h₃ : d = c^2)
  (h₄ : c + d = 1)
  (h₅ : a + c) :
  Real.sqrt ((a - c)^2 + (b - d)^2) = Real.sqrt 10
  := by
  have h₆ : a^2 + a - 1 = 0 := by
    have h₆₁ : a + b = 1 := h₁
    have h₆₂ : b = a^2 := h₂
    rw [h₆₁] at h₆
    ring_nf at h₆
    linarith
  have h₇ : c^2 + c - 1 = 0 := by
    have h₇₁ : c + d = 1 := h₄
    have h₇₂ : d = c^2 := h₃
    rw [h₇₁] at h₇
    ring_nf at h₇
    linarith
  have h₈ : a + c = -1 := by
    have h₈₁ : a^2 + a - 1 = 0 := h₆
    have h₈₂ : a^2 + a - 1 = 0 := h₇
    have h₈₃ : c^2 + c - 1 = 0 := h₇
    have h₈₄ : a + c = -1 := h₈
    apply mul_left_cancel. (sub_ne_zero.mpr h₈)
    nlinarith [sq_pos_of_ne_zero (sub_ne_zero.mpr h₈), sq_nonneg (a - c)]
  exact h₈

have h₉ : (a - c)^2 = 5 := by
  have h₉₁ : a^2 + a - 1 = 0 := h₆
  have h₉₂ : a^2 + a - 1 = 0 := h₇
  have h₉₃ : c^2 + c - 1 = 0 := h₇
  have h₉₄ : a + c = -1 := h₈
  have h₉₅ : a^2 + a - 1 = 0 := by
    nlinarith [sq_pos_of_ne_zero (sub_ne_zero.mpr h₈), sq_nonneg (a + c)]
  exact h₉

have h₁₀ : (b - d)^2 = 5 := by
  have h₁₀₁ : b = a^2 := h₂
  have h₁₀₂ : d = c^2 := h₃
  have h₁₀₃ : a + c = -1 := h₈
  have h₁₀₄ : (a - c)^2 = 5 := h₉
  calc
    (b - d)^2 = (a^2 - c^2)^2 := by
      rw [h₁₀₁, h₁₀₂]
    <> ring_nf
    = ((a - c) * (a + c))^2 := by
      ring_nf
    <>
    nlinarith
    = (a - c)^2 * (a + c)^2 := by
      ring_nf
    = 5 * (a + c)^2 := by
      rw [h₁₀]
    <> ring_nf
    = 5 * (-1)^2 := by
      rw [h₁₀]
    <> ring_nf
    = 5 := by
      norm_num
    = 5 := by rfl

have h₁₁ : (a - c)^2 + (b - d)^2 = 10 := by
  have h₁₁₁ : (a - c)^2 = 5 := h₉
  have h₁₁₂ : (b - d)^2 = 5 := h₁₀
  linarith

have h₁₂ : Real.sqrt ((a - c)^2 + (b - d)^2) =
  Real.sqrt 10 := by
  rw [h₁₂]
  <>
  simp [Real.sqrt_eq_iff_sq_eq]
  <>
  ring_nf
  <>
  norm_num
  apply h₁

-- Simplified Proof
import Mathlib
import Aesop

set_option maxHeartbeats 0

open BigOperators Real Nat Topology Rat

theorem mathd_algebra_487
  (a b c d : ℝ)
  (h₁ : b = a^2)
  (h₂ : a + b = 1)
  (h₃ : d = c^2)
  (h₄ : c + d = 1)

```

```

(h₅ : a ≠ c) :
  Real.sqrt ((a - c)^2 + (b - d)^2) = Real.sqrt 10
  := by
  have h₆ : a + c = -1 := by
    apply mul_left_cancel. (sub_ne_zero.mpr h₅)
    nlinarith
  rw [show (a - c)^2 + (b - d)^2 = 10 by nlinarith]
  -----
-- Orig Proof
import Mathlib
import Aesop

set_option maxHeartbeats 0

open BigOperators Real Nat Topology Rat

theorem
  (m n : ℕ)
  (f : ℕ → ℕ)
  (h₁ : ∀ x, f x = 4^x + 6^x + 9^x)
  (h₂ : 0 < m ∧ 0 < n)
  (h₃ : m ≤ n) :
  f (2^m) f (2^n) := by
  have h_main : ∀ (x : ℕ), 0 < x → f x ∣ f (2 * x)
  := by
    intro x hx
    have h₁ : f x = 4^x + 6^x + 9^x := h₁
    have h₂ : f (2 * x) = 4^(2 * x) + 6^(2 * x) + 9^(2 * x) := by
      rw [h₁]
    <> ring_nf
    rw [h₁, h₂]
    have h₃ : (4 : ℕ)^x > 0 := by positivity
    have h₄ : (6 : ℕ)^x > 0 := by positivity
    have h₅ : (9 : ℕ)^x > 0 := by positivity
    have h₆ : (4 : ℕ)^(2 * x) = (4^x)^2 := by
      rw [show (2 : ℕ) * x = x + x by ring]
      simp [pow_add, pow_mul]
    <> ring_nf
    have h₇ : (6 : ℕ)^(2 * x) = (6^x)^2 := by
      rw [show (2 : ℕ) * x = x + x by ring]
      simp [pow_add, pow_mul]
    <> ring_nf
    have h₈ : (9 : ℕ)^(2 * x) = (9^x)^2 := by
      rw [show (2 : ℕ) * x = x + x by ring]
      simp [pow_add, pow_mul]
    <> ring_nf
    rw [h₁, h₂, h₆]
    -- We need to show that 4^x + 6^x + 9^x divides
    -- (4^x)^2 + (6^x)^2 + (9^x)^2
    -- We use the identity (a + b + c)^2 = a^2 +
    -- b^2 + c^2 + 2(ab + bc + ca)
    -- Therefore, a^2 + b^2 + c^2 = (a + b + c)^2 -
    -- 2(ab + bc + ca)
    -- We show that a + b + c divides ab + bc + ca
    have h₉ : (4 : ℕ)^x * (9 : ℕ)^x = (6 : ℕ)^x
    <> ring_nf
    calc
      (4 : ℕ)^x * (9 : ℕ)^x = (4 * 9)^x :=
        by
          rw [mul_pow]
        = 36^x := by norm_num
        = (6 : ℕ)^(2 * x) := by
          calc
            36^x = (6^2)^x := by norm_num
            = 6^(2 * x) := by
              rw [- pow_mul]
              <> ring_nf
    have h₁₀ : (6 : ℕ)^(2 * x) := by rfl
    <> ring_nf
    calc
      (6 : ℕ)^x * (6 : ℕ)^x = 6^(x + x) :=
        by
          rw [- pow_add]
          = 6^(2 * x) := by
            ring_nf
            <> simp [mul_comm]
            <> ring_nf
    have h₁₁ : (4 : ℕ)^x * (9 : ℕ)^x = (6 : ℕ)^x
    <> ring_nf
    calc
      (4 : ℕ)^x * (6 : ℕ)^x := by
        linarith
    -- Using the above, we can show that (4^x + 6^x
    -- + 9^x) divides 2 * (4^x * 6^x + 6^x * 9^x
    -- + 9^x * 4^x)
    -- And thus divides (4^x)^2 + (6^x)^2 + (9^x)^2
    have h₁₂ : (4^x + 6^x + 9^x) ∣ ((4^x)^2
    -- + (6^x)^2 + (9^x)^2) := by
      have h₁₂₁ : (4^x)^2 + (6^x)^2 + (9^x)^2 =
        (4^x + 6^x + 9^x)^2 - 2 *
        (4^x * 6^x + 6^x * 9^x + 9^x * 4^x) := by
        have h₁₂₁₁ : (4^x + 6^x + 9^x)^2 = (4
        -- + 6^x + 9^x)^2 + 2 * (4^x * 6^x +
        -- 6^x * 9^x + 9^x * 4^x) := by
          have h₁₂₁₁₁ : (4^x + 6^x + 9^x)^2 = (4
          -- + 6^x + 9^x)^2 + 2 * (4^x * 6^x +
          -- 6^x * 9^x + 9^x * 4^x) := by
            ring_nf
            <>
            simp [pow_two, mul_add, add_mul,
            -- mul_comm, mul_left_comm, mul_assoc]
            <>
            ring_nf
            <>
            omega
          have h₁₂₁₁₂ : (4^x + 6^x + 9^x)^2 ≥ 2 *
          -- (4^x * 6^x + 6^x * 9^x + 9^x * 4^x)
          -- := by
            have h₁₂₁₁₂₁ : 0 < 4^x := by positivity
            have h₁₂₁₁₂₂ : 0 < 6^x := by positivity
            have h₁₂₁₁₂₃ : 0 < 9^x := by positivity
            nlinarith [sq_nonneg (4^x - 6^x),
            -- sq_nonneg (6^x - 9^x), sq_nonneg (9^x
            -- - 4^x)]

```

```

omega
have h₁ : (4^x + 6^x + 9^x) ∣ 2 * (4^x
-- + 6^x + 9^x + 4^x) := by
  have h₁₁ : 2 * (4^x + 6^x + 9^x + 4^x) =
  -- (4^x + 6^x + 9^x) * (4^x + 6^x + 9^x
  -- + 4^x) := by
    have h₁₁₁ : 4^x + 9^x = 6^x + 6^x
    <> ring_nf
    calc
      4^x + 9^x = (4 * 9)^x := by rw
    <> [mul_pow]
    = 36^x := by norm_num
    = (6^2)^x := by norm_num
    = 6^(2 * x) := by rw [- pow_mul]
  <> ring_nf
  = (6^x)^2 := by
    calc
      6^(2 * x) = 6^(x + x) := by
        ring_nf
      = 6^x * 6^x := by rw
  <> [pow_add]
  = (6^x)^2 := by ring
  calc
    2 * (4^x * 6^x + 6^x * 9^x + 9^x * 4^x) =
    -- 2 * (4^x * 6^x + 6^x * 9^x + 9^x * 4^x) := by ring
    = 2 * (4^x * 6^x + 6^x * 9^x + 9^x * 4^x) := by
      rw [h₁₁]
    = 2 * (6^x * (4^x + 9^x + 6^x
    -- + 4^x)) := by ring
    = (4^x + 6^x + 9^x) * (2 * 6^x
    -- + 4^x) := by ring
    = (4^x + 6^x + 9^x) * (2 * 6^x
    -- + 4^x) := by rfl
    rw [h₁]
  <>
  exact (2 * 6^x, by ring)
have h₂ : (4^x + 6^x + 9^x) ∣ (4^x +
-- 6^x + 9^x)^2 := by
  use (4^x + 6^x + 9^x)
  <> ring
  have h₂₁ : (4^x + 6^x + 9^x) ∣ (4^x +
  -- 6^x + 9^x)^2 - 2 * (4^x * 6^x + 6^x *
  -- 9^x + 9^x * 4^x) := by
    exact Nat.dvd_sub' h₁ h₁
  rw [h₂] at *
  exact h₂
exact h₂

have h_inductive_step : ∀ (k : ℕ), f (2^k) ∣ f
  (2^(m + k)) := by
  intro k
  have h₃ : ∀ (k : ℕ), f (2^k) ∣ f (2^(m + k))
  := by
    intro k
    induction' k with k ih
    . -- Base case: k = 0
    <> simp [pow_add, pow_zero]
    <>
    exact dvd_refl
    . -- Inductive step: assume the statement
    -- holds for k, prove for k + 1
    have h₄ : f (2^(m + k)) ∣ f (2^(2^(m +
    -- k))) := by
      have h₄₁ : 0 < 2^(m + k) := by
        apply pow_pos
        norm_num
      have h₄₂ : f (2^(m + k)) ∣ f (2^(2^(m +
      -- k))) := by
        apply h_main
        <> positivity
      exact h₄
    have h₄ : f (2^k) ∣ f (2^(m + k)) := ih
    have h₄ : f (2^(2^(m + k))) = f (2^(m
    -- + k + 1)) := by
      have h₄₁ : 2 * (2^(m + k)) = 2^(m + k +
      -- 1) := by
        calc
          2 * (2^(m + k)) = 2^1 * 2^(m +
          -- k) := by norm_num
          = 2^(1 + (m + k)) := by rw [-
          -- pow_add]
          = 2^(m + k + 1) := by ring_nf
      rw [h₄]
    <> simp [pow_add, pow_one]
    <> ring_nf
    have h₄ : f (2^k) ∣ f (2^(m + k + 1)) :=
    -- by
      have h₄₁ : f (2^(m + k + 1)) = f (2 * (2
      -- ^ (m + k))) := by
        rw [h₄]
        <> ring_nf
        rw [h₄]
        exact dvd_trans h₁ h₄
      simp [add_assoc] using h₄
    exact h₄ k

have h_final : f (2^m) ∣ f (2^n) := by
  have h₅ : ∃ (k : ℕ), n = m + k := by
    use n - m
    have h₅₁ : m ≤ n := h₅
    have h₅ : m + (n - m) = n := by
      omega
    linarith
  obtain k, hk₁ := h₅
  have h₅ : f (2^m) ∣ f (2^(m + k)) :=
  -- h_inductive_step k
  have h₅ : f (2^(m + k)) = f (2^n) := by
    rw [hk₁]
    <> simp [pow_add]
    <> ring_nf
    rw [h₅] at h₅

```





```

    rw [Real.log_mul (by positivity) (by
      → positivity)]
  rw [h1, h2, h3, h4]
  have h5 : Real.log (2 ^ 4) = 4 * Real.log 2 :=
    by
      rw [Real.log_pow] <|> norm_num
  have h6 : Real.log (2 ^ 3) = 3 * Real.log 2 :=
    by
      rw [Real.log_pow] <|> norm_num
  have h7 : Real.log (2 ^ 5) = 5 * Real.log 2 :=
    by
      rw [Real.log_pow] <|> norm_num
  have h8 : Real.log (2 ^ 2) = 2 * Real.log 2 :=
    by
      rw [Real.log_pow] <|> norm_num
  rw [h5, h6, h7, h8]
  have h9 : Real.log 2 ≠ 0 := by
    exact Real.log_ne_zero_of_pos_of_ne_one (by
      → norm_num) (by norm_num)
  have h10 : Real.log 5 ≠ 0 := by
    exact Real.log_ne_zero_of_pos_of_ne_one (by
      → norm_num) (by norm_num)
  field_simp [h9, h10]
  ring_nf
  <|>
  (try norm_num) <|>
  {
    have h11 : Real.log 5 > 0 := Real.log_pos
      → (by norm_num)
    nlinarith [Real.log_pos (by norm_num : (1
      → : s) < 2),
      Real.log_pos (by norm_num : (1 : s) < 5)]
  } <|>
  {
    have h12 : Real.log 5 > 0 := Real.log_pos
      → (by norm_num)
    nlinarith [Real.log_pos (by norm_num : (1
      → : s) < 2),
      Real.log_pos (by norm_num : (1 : s) < 5)]
  } <|>
  {
    have h13 : Real.log 5 > 0 := Real.log_pos
      → (by norm_num)
    nlinarith [Real.log_pos (by norm_num : (1
      → : s) < 2),
      Real.log_pos (by norm_num : (1 : s) < 5)]
  } <|>
  {
    have h14 : Real.log 5 > 0 := Real.log_pos
      → (by norm_num)
    nlinarith [Real.log_pos (by norm_num : (1
      → : s) < 2),
      Real.log_pos (by norm_num : (1 : s) < 5)]
  }
}
exact h_main
-- Simplified Proof
import Mathlib
import Aesop

set_option maxHeartbeats 0

open BigOperators Real Nat Topology Rat

theorem amc12b_2021_p9 :
  (Real.log 80 / Real.log 2) / (Real.log 2 /
    → Real.log 40) - (Real.log 160 / Real.log
    → 2) / (Real.log 2 / Real.log 20) = 2 := by
  field_simp [Real.log_mul, Real.log_pow, show
    → Real.log 80 = Real.log (2^4 * 5) by
    → norm_num,
    show Real.log 40 = Real.log (2^3 * 5) by
    → norm_num,
    show Real.log 160 = Real.log (2^5 * 5) by
    → norm_num,
    show Real.log 20 = Real.log (2^2 * 5) by
    → norm_num]
  ring
  -----
  -- Orig Proof
  import Mathlib
  import Aesop

  set_option maxHeartbeats 0

  open BigOperators Real Nat Topology Rat

  theorem mathd_algebra_215
  (S : Finset s)
  (h : ∀ (x : s), x ∈ S ↔ (x + 3)^2 = 121) :
  ∑ k ∈ S, k = -6 := by
  have h1 : S = {8, -14} := by
    apply Finset.ext
    intro x
    simp only [Finset.mem_insert,
      → Finset.mem_singleton, h]
    constructor
    · intro h
      have h2 : (x + 3) ^ 2 = 121 := by exact h
      have h3 : x + 3 = 11 ∨ x + 3 = -11 := by
        apply or_iff_not_imp_left.mpr
        intro h4
        apply eq_of_sub_eq_zero
        apply mul_left_cancel, (sub_ne_zero.mpr h4)
        nlinarith
      cases h2 with
      | inl h5 =>
        have h6 : x = 8 := by linarith
        simp [h5]
      | inr h5 =>
        have h6 : x = -14 := by linarith
        simp [h5]
    · intro h
      cases h with
      | inl h =>
        rw [h]
        norm_num
      | inr h =>
        have h7 : ∑ k ∈ S, k = -6 := by
          rw [h]
          norm_num [Finset.sum_pair (show (8 : s) ≠ -14
            → by norm_num)]
        exact h7
  -- Simplified Proof
  import Mathlib
  import Aesop

  set_option maxHeartbeats 0

  open BigOperators Real Nat Topology Rat

  theorem mathd_algebra_215
  (S : Finset s)
  (h : ∀ (x : s), x ∈ S ↔ (x + 3)^2 = 121) :
  ∑ k ∈ S, k = -6 := by
  have h1 : S = {8, -14} := by
    ext x
    simp_all
    constructor
    · intro h
      apply or_iff_not_imp_left.mpr
      intro h2
      apply mul_left_cancel, (sub_ne_zero.mpr h2)
      nlinarith
    · intro h
      apply mul_left_cancel, (sub_ne_zero.mpr h2)
      nlinarith
      rintro (rfl | rfl) <|> norm_num
  rw [this]
  norm_num
  -----
  -- Orig Proof
  import Mathlib
  import Aesop

  set_option maxHeartbeats 0

  open BigOperators Real Nat Topology Rat

  theorem mathd_numbertheory_552
  (f g h : ℕ → ℕ)
  (h1 : ∀ x, f x = 12 * x + 7)
  (h2 : ∀ x, g x = 5 * x + 2)
  (h3 : ∀ x, h x = Nat.gcd (f x) (g x))
  (h4 : Fintype (Set.range h)) :
  ∑ k ∈ (Set.range h).toFinset, k = 12 := by
  have h5 : ∑ (x : ℕ), h x | 11 := by
    intro x
    have h6 : h x = Nat.gcd (f x) (g x) := h3 x
    rw [h6]
    have h7 : f x = 12 * (x : ℕ) + 7 := by
      simp [h1]
    <|> norm_cast
    have h8 : g x = 5 * (x : ℕ) + 2 := by
      simp [h2]
    <|> norm_cast
    have h9 : 5 * f x - 12 * g x = 11 := by
      rw [h7, h8]
      norm_num [mul_add, add_mul, mul_assoc]
    <|> ring_nf at *
    <|> norm_cast
    <|> simp [PNat.ne_zero]
    <|> omega
  have h10 : Nat.gcd (f x) (g x) | f x :=
    → Nat.gcd.dvd_left (f x) (g x)
  have h11 : Nat.gcd (f x) (g x) | g x :=
    → Nat.gcd.dvd_right (f x) (g x)
  have h12 : Nat.gcd (f x) (g x) | 5 * f x :=
    → dvd_mul_of_dvd_right h10 5
  have h13 : Nat.gcd (f x) (g x) | 12 * g x :=
    → dvd_mul_of_dvd_right h11 12
  have h14 : Nat.gcd (f x) (g x) | 5 * f x - 12 *
    → g x := Nat.dvd_sub' h12 h13
  rw [h14] at h5
  exact h5
  have h15 : ∑ (x : ℕ), h x = 11 ∨ h x =
    → 11 := by
    intro x
    have h16 : h x | 11 := h10 x
    have h17 : h x = 1 ∨ h x = 11 := by
      have h18 : h x | 11 := h16
      have h19 : h x ≤ 11 := Nat.le_of_dvd (by
        → norm_num) h18
      interval_cases h x <|> norm_num at h19 <|>
        (try omega) <|> (try { contradiction })
    <|> (try { aesop })
  exact h15
  have h16 : 1 ∈ Set.range h := by
    have h17 : h 1, by norm_num = 1 := by
      have h18 : h 1, by norm_num = Nat.gcd (f 1,
        → by norm_num) (g 1, by norm_num) := h3 1
      rw [h18]
      have h19 : f 1, by norm_num = 12 * (1 : ℕ) +
        → 7 := by
        simp [h1]
      <|> norm_cast
      have h20 : g 1, by norm_num = 5 * (1 : ℕ) + 2
        → := by
        simp [h2]
      <|> norm_cast
      rw [h19, h20]
      norm_num
    <|> decide
  have h17 : (1 : ℕ) ∈ Set.range h := by
    refine' ⟨1, by norm_num, _⟩
  rw [h17]
  exact h16
  have h18 : 11 ∈ Set.range h := by
    have h19 : h 4, by norm_num = 11 := by
      have h20 : h 4, by norm_num = Nat.gcd (f 4,
        → by norm_num) (g 4, by norm_num) := h3 4
      rw [h20]
      have h21 : f 4, by norm_num = 12 * (4 : ℕ) +
        → 7 := by
        simp [h1]
      <|> norm_cast
      have h22 : g 4, by norm_num = 5 * (4 : ℕ) + 2
        → := by
        simp [h2]
      <|> norm_cast
      rw [h21, h22]
      norm_num
    <|> decide
  have h19 : (11 : ℕ) ∈ Set.range h := by
    refine' ⟨4, by norm_num, _⟩
  rw [h19]
  exact h18
  have h20 : ∑ k ∈ (Set.range h).toFinset, k = 12
    → := by
    have h21 : (Set.range h).toFinset = {1, 11} := by
      apply Finset.ext
      intro x
      simp only [Finset.mem_insert,
        → Finset.mem_singleton, h]
      constructor
      · intro hx
        have h22 : x ∈ Set.range h := hx
        have h23 : x = 1 ∨ x = 11 := by
          obtain (y, rfl) := h22
          have h24 : h y = 1 ∨ h y = 11 :=
            → h16 or_eleven y
          cases h24 with
          | inl h25 =>
            simp [h25]
          | inr h25 =>
            simp [h25]
      · intro hx
        cases hx with
        | inl hx =>
          rw [hx]
          exact (by
            use 1, by norm_num
            simp [h1, h2, h3])
        | inr hx =>
          rw [hx]

```

```

    exact (by
      use (4, by norm_num)
      simp [h, h₁, h₂]) ]
  norm_num
  -----
  -- Orig Proof
import Mathlib
import Aesop

set_option maxHeartbeats 0

open BigOperators Real Nat Topology Rat

theorem mathd_numbertheory_293
  (n : ℕ)
  (h₁ : n ≤ 9)
  (h₂ : 11·20 + 100 + 10 * n + 7) :
  n = 5 := by
  have h₃ : n = 5 := by
    have h₄ : n ≤ 9 := h₁
    have h₅ : 11 | 20 * 100 + 10 * n + 7 := h₂
    interval_cases n <|> norm_num at h₄ <|>
    (try omega) <|>
    (try {
      rcases h₄ with ⟨k, hk⟩
      norm_num at hk
      omega
    })
  exact h₃
  -- Simplified Proof
import Mathlib
import Aesop

set_option maxHeartbeats 0

open BigOperators Real Nat Topology Rat

theorem mathd_numbertheory_293
  (n : ℕ)
  (h₁ : n ≤ 9)
  (h₂ : 11·20 + 100 + 10 * n + 7) :
  n = 5 := by
  omega
  -----
  -- Orig Proof
import Mathlib
import Aesop

set_option maxHeartbeats 0

open BigOperators Real Nat Topology Rat

theorem mathd_numbertheory_769 :
  (129·34 + 96·38) % 11 = 9 := by
  have h₁ : (129·34 + 96·38) % 11 = 9 := by
    norm_num [Nat.pow_mod, Nat.add_mod,
      ↪ Nat.mod_mod]
    <|> rfl
  exact h₁
  -- Simplified Proof
import Mathlib
import Aesop

set_option maxHeartbeats 0

open BigOperators Real Nat Topology Rat

theorem mathd_numbertheory_769 :
  (129·34 + 96·38) % 11 = 9 := by
  norm_num
  -----
  -- Orig Proof
import Mathlib
import Aesop

set_option maxHeartbeats 0

open BigOperators Real Nat Topology Rat

theorem aime_1994_p3
  (f : ℤ → ℤ)
  (h₀ : ∀ (x : ℤ), f x + f (x-1) = x²)
  (h₁ : f 19 = 94) :
  f (94) % 1000 = 561 := by
  have h₂ : f 18 = 267 := by
    have h₃ : f 19 + f 18 = (19 : ℤ)² := by
      have h₄ := h₀ 19
      norm_num at h₄ <|>
      linarith
    norm_num [h₁] at h₃ <|>
    linarith
  have h₃ : ∀ (x : ℤ), f x = f (x - 2) + 2 * x - 1
    := by
    intro x
    have h₄ := h₀ x
    have h₅ := h₀ (x - 1)
    have h₆ : f (x - 1) = (x - 1 : ℤ)² - 2 * f (x - 2) := by
      have h₇ := h₀ (x - 1)
      have h₈ := h₀ (x - 2)
      ring_nf at h₇, h₈ <|>
      linarith
    have h₉ : f x + f (x - 1) = (x : ℤ)² := by
      exact h₄
    have h₁₀ : f x = (x : ℤ)² - 2 * f (x - 1) := by
      linarith
    rw [h₃, h₃]
    ring_nf
    <|> nlinarith
  have h₄ : f 94 = 4561 := by
    have h₅ : f 94 = 4561 := by
      have h₆ := h₃ 94
      have h₇ := h₃ 92
      have h₈ := h₃ 90
      have h₉ := h₃ 88
      have h₁₀ := h₃ 86
      have h₁₁ := h₃ 84
      have h₁₂ := h₃ 82
      have h₁₃ := h₃ 80
      have h₁₄ := h₃ 78
      have h₁₅ := h₃ 76
      have h₁₆ := h₃ 74
      have h₁₇ := h₃ 72
      have h₁₈ := h₃ 70
      have h₁₉ := h₃ 68
      have h₂₀ := h₃ 66
      have h₂₁ := h₃ 64
      have h₂₂ := h₃ 62
      have h₂₃ := h₃ 60
      have h₂₄ := h₃ 58
      have h₂₅ := h₃ 56
      have h₂₆ := h₃ 54
      have h₂₇ := h₃ 52
      have h₂₈ := h₃ 50
      have h₂₉ := h₃ 48
      have h₃₀ := h₃ 46
      have h₃₁ := h₃ 44
      have h₃₂ := h₃ 42
      have h₃₃ := h₃ 40
      have h₃₄ := h₃ 38
      have h₃₅ := h₃ 36
      have h₃₆ := h₃ 34
      have h₃₇ := h₃ 32
      have h₃₈ := h₃ 30
      have h₃₉ := h₃ 28
      have h₄₀ := h₃ 26
      have h₄₁ := h₃ 24
      have h₄₂ := h₃ 22
      have h₄₃ := h₃ 20
      have h₄₄ := h₃ 18
      have h₄₅ := h₃ 16
      have h₄₆ := h₃ 14
      have h₄₇ := h₃ 12
      have h₄₈ := h₃ 10
      have h₄₉ := h₃ 8
      have h₅₀ := h₃ 6
      have h₅₁ := h₃ 4
      have h₅₂ := h₃ 2
      norm_num at *
      omega
    }
  -- Orig Proof
import Mathlib
import Aesop

set_option maxHeartbeats 0

open BigOperators Real Nat Topology Rat

theorem mathd_numbertheory_207 :
  8 * 9² + 5 * 9 + 2 = 695 := by
  have h : 8 * 9² + 5 * 9 + 2 = 695 := by
    norm_num
    <|> rfl
  apply h
  -- Simplified Proof
import Mathlib
import Aesop

set_option maxHeartbeats 0

open BigOperators Real Nat Topology Rat

theorem mathd_numbertheory_207 :
  8 * 9² + 5 * 9 + 2 = 695 := by
  norm_num
  -----
  -- Orig Proof
import Mathlib
import Aesop

set_option maxHeartbeats 0

open BigOperators Real Nat Topology Rat

theorem mathd_numbertheory_342 :
  54 % 6 = 0 := by
  have h : 54 % 6 = 0 := by
    norm_num
    exact h
  -- Simplified Proof
import Mathlib
import Aesop

set_option maxHeartbeats 0

open BigOperators Real Nat Topology Rat

theorem mathd_numbertheory_342 :
  54 % 6 = 0 := by
  norm_num
  -----
  -- Orig Proof
import Mathlib
import Aesop

set_option maxHeartbeats 0

open BigOperators Real Nat Topology Rat

theorem mathd_numbertheory_5
  (n : ℕ)
  (h₁ : 10 ≤ n)
  (h₂ : ∃ x, x² = n)
  (h₃ : ∃ t, t³ = n) :
  64 ≤ n := by
  have h₄ : 64 ≤ n := by
    obtain ⟨t, ht⟩ := h₃
    by_contra! h
    -- We will show that if n < 64, then t < 4 and
    -- derive a contradiction.
    have h₅ : t ≤ 3 := by
      by_contra! h
      -- If t ≥ 4, then t³ ≥ 64, which contradicts
      -- n < 64.
      have h₆ : t ≥ 4 := by linarith
      have h₇ : t³ ≥ 4³ := by
        exact Nat.pow_le_pow_of_le_left (by
          linarith) 3
      have h₈ : t³ ≥ 64 := by
        norm_num at h₇ <|>
        linarith
      have h₉ : n ≥ 64 := by
        linarith
      linarith
    -- Now we know t ≤ 3. We will check each case.
    interval_cases t <|> norm_num at ht <|>

```



```

have h13 : 100 * A ≥ 700 := by
  nlinarith
have h14 : C + 10 * M + 100 * A ≥ 700 := by
  have h11 : C + 10 * M ≥ 0 := by
    nlinarith
  omega
have h15 : A ≥ 6 := by
  by_contra h
have h16 : A ≤ 5 := by
  omega
have h17 : 100 * A ≤ 500 := by
  nlinarith
have h18 : C + 10 * M + 100 * A ≤ 599 := by
  have h19 : C ≤ 9 := by
    nlinarith
  have h20 : M ≤ 9 := by
    nlinarith
  have h21 : C + 10 * M ≤ 99 := by
    nlinarith
  omega
omega
have h22 : C + 10 * M = 17 := by
  have h23 : C + 10 * M + 100 * A = 617 := h2
  rw [h2] at h23
  ring_nf at h23
  <> omega
have h24 : M = 1 := by
  have h25 : M ≤ 1 := by
    by_contra h
    have h26 : M ≥ 2 := by omega
    have h27 : C + 10 * M ≥ 20 := by
      have h28 : C ≥ 0 := by omega
    nlinarith
  omega
  by_contra h
  have h29 : M = 0 := by omega
  rw [h29] at h23
  have h30 : C = 17 := by omega
  have h31 : C ≤ 9 := by linarith
  omega
omega
have h32 : C = 7 := by
  have h33 : C + 10 * M = 17 := h22
  rw [h22] at h33
  omega
have h34 : A + M + C = 14 := by
  rw [h34, h35, h36]
  <> norm_num
exact h34
-- Simplified Proof
import Mathlib
import Aesop
set_option maxHeartbeats 0
open BigOperators Real Nat Topology Rat
theorem amc12a_2003_p5
  (A M C : ℕ)
  (h1 : A ≤ 9 ∧ M ≤ 9 ∧ C ≤ 9)
  (h2 : Nat.ofDigits 10 [0,1,C,M,A] + Nat.ofDigits
    → 10 [2,1,C,M,A] = 123422) :
  A + M + C = 14 := by
  simp_all [Nat.ofDigits]
  omega
-----
-- Orig Proof
import Mathlib
import Aesop
set_option maxHeartbeats 0
open BigOperators Real Nat Topology Rat
theorem
  → algebra_2varlineareq_fp3zeq11_3tfmlm5zeqn68_feqn10_zeq7
  (f z : ℂ)
  (h1 : f + 3*z = 11)
  (h2 : 3*(f - 1) - 5*z = -68) :
  f = -10 ∧ z = 7 := by
  constructor
  all_goals
    simp_all [Complex.ext_iff]
    constructor <> nlinarith
-----
-- Orig Proof
import Mathlib
import Aesop
set_option maxHeartbeats 0
open BigOperators Real Nat Topology Rat
theorem mathd_numbertheory_247
  (n : ℕ)
  (h1 : (3 * n) % 11 = 2) :
  n % 11 = 8 := by
  have h2 : n % 11 = 8 := by
    have h3 : (3 * n) % 11 = 2 := h1
    have h4 : n % 11 = 3 ∨ n % 11 = 4 ∨ n % 11 = 5 ∨ n
      % 11 = 6 ∨ n % 11 = 7 ∨ n % 11 = 8 ∨ n %
      11 = 9 ∨ n % 11 = 10 := by
      omega
    rcases h4 with (h4 | h4 | h4 | h4 | h4 | h4 | h4 | h4)
    → | h4 | h4 | h4 | h4 | h4 | h4 | h4 | h4 <>
      (try omega) <>
      (try {
        simp [h4, Nat.mul_mod, Nat.add_mod,
          → Nat.mod_mod] at h4
      })
  exact h2
-- Simplified Proof
import Mathlib
import Aesop
set_option maxHeartbeats 0
open BigOperators Real Nat Topology Rat
theorem mathd_numbertheory_247
  (n : ℕ)
  (h1 : (3 * n) % 11 = 2) :
  n % 11 = 8 := by
  omega
-----
-- Orig Proof
import Mathlib
import Aesop
set_option maxHeartbeats 0
open BigOperators Real Nat Topology Rat
theorem
  → algebra_2varlineareq_fp3zeq11_3tfmlm5zeqn68_feqn10_zeq7
  (h1 : √(n : ℕ), n ∈ S ↔ 0 < n ∧ (n + (1000 : ℕ))
    → / 70 = Int.floor (Real.sqrt n)) :
  S.card = 6 := by
  have h1 : S = {400, 470, 2290, 2360, 2430, 2500}
    → := by
  apply Finset.ext
  intro n
  simp only [Finset.mem_insert,
    → Finset.mem_singleton, h1]
  constructor
  - -- Prove the forward direction: if n ∈ S, then
    → n is one of the six numbers.
  intro h
  have h2 : 0 < n := h.1
  have h3 : (n : ℕ) + 1000 / 70 = Int.floor
    (Real.sqrt n) := by
    exact_mod_cast h.2
  -- We need to show that n is one of the six
  → numbers.
  have h4 : n = 400 ∨ n = 470 ∨ n = 2290 ∨ n =
    2360 ∨ n = 2430 ∨ n = 2500 := by
    -- Use the fact that (n + 1000)/70 =
    → floor(sqrt(n)) to find possible values of
    → n.
  have h5 : (n : ℕ) + 1000 = 70 * (Int.floor
    (Real.sqrt n) : ℕ) := by
    have h6 : ((n : ℕ) + 1000) / 70 =
    (Int.floor (Real.sqrt n) : ℕ) := by
      exact_mod_cast h
  linarith
  have h7 : (n : ℕ) + 1000 = 70 * (Int.floor
    (Real.sqrt n) : ℕ) := by
    norm_cast at h7
    <> field_simp at h7
    <> ring_nf at h7
    <> norm_cast at h7
    (try norm_num at h7) <>
    (try linarith) <>
    (try
      {
        simp_all [Int.cast_inj]
        <> norm_num at *
        <> linarith
      })
    <>
    (try
      {
        norm_num at h7
        <>
        (try linarith)
        <>
        (try
          {
            simp_all [Int.cast_inj]
            <> norm_num at *
            <> linarith
          })
      })
    <>
    (try
      {
        field_simp at h7
        <>
        norm_cast at h7
        <>
        simp_all [Int.cast_inj]
        <>
        norm_num at *
        <>
        linarith
      })
    <>
    (try
      {
        norm_cast at h7
        <>
        simp_all [Int.cast_inj]
        <>
        norm_num at *
        <>
        linarith
      })
  )
  -- Now we have n + 1000 = 70 *
  → floor(sqrt(n)).
  -- Let k = floor(sqrt(n)). Then n = 70k -
  → 1000.
  -- We need to find all integers k such that
  → k^2 ≤ 70k - 1000 < (k + 1)^2 and 70k -
  → 1000 > 0.
  have h8 : ∃ (k : ℕ), (n : ℕ) = 70 * k -
    1000 := by
    use (Int.floor (Real.sqrt n))
    linarith
  obtain (k, h8) := h8

```

```

have h8 : (n : R) = 70 * (k : R) - 1000 :=
by
  norm_cast at h8
  <|>
  (try ring_nf at h8 <|>
  (try norm_num at h8 <|>
  (try linarith) <|>
  (try simp_all [Int.cast_inj]) <|>
  (try norm_cast at h8 <|>
  (try linarith) <|>
  (try ring_nf at h8 <|>
  (try norm_num at h8 <|>
  (try linarith)
have h9 : (k : R) ≤ Real.sqrt n := by
have h10 : (k : R) = Int.floor (Real.sqrt
n) := by
  have h11 : (k : z) = Int.floor
  (Real.sqrt n) := by
    linarith
    norm_cast at h11
    <|> simp_all
    rw [h11]
  exact Int.floor_le (Real.sqrt n)
have h12 : Real.sqrt n < (k : R) + 1 := by
have h13 : (k : R) = Int.floor (Real.sqrt
n) := by
  have h14 : (k : z) = Int.floor
  (Real.sqrt n) := by
    linarith
    norm_cast at h14
    <|> simp_all
    rw [h14]
  exact Int.lt_floor_add_one (Real.sqrt n)
have h15 : (k : R) ^ 2 ≤ (n : R) := by
have h16 : (k : R) < Real.sqrt n := h12
have h17 : 0 ≤ Real.sqrt n :=
  Real.sqrt_nonneg n
have h18 : (k : R) ^ 2 ≤ (Real.sqrt n) ^
2 := by
  nlinarith [Real.sqrt_nonneg n,
  Real.sq_sqrt (by positivity : 0 ≤ (n : R)
  > 0)]
have h19 : (Real.sqrt n) ^ 2 = (n : R) :=
by
  rw [Real.sq_sqrt (by positivity)]
  nlinarith
have h20 : (n : R) < ((k : R) + 1) ^ 2 := by
have h21 : Real.sqrt n < (k : R) + 1 :=
h12
have h22 : 0 ≤ Real.sqrt n :=
  Real.sqrt_nonneg n
have h23 : (Real.sqrt n) ^ 2 < ((k : R) +
1) ^ 2 := by
  nlinarith [Real.sqrt_nonneg n,
  Real.sq_sqrt (by positivity : 0 ≤ (n : R)
  > 0)]
have h24 : (Real.sqrt n) ^ 2 = (n : R) :=
by
  rw [Real.sq_sqrt (by positivity)]
  nlinarith
have h25 : (k : z) ≥ 15 := by
  by_contra h25
  have h26 : (k : z) ≤ 14 := by linarith
  have h27 : (n : z) ≤ 70 * 14 - 1000 := by
    have h28 : (n : z) = 70 * k - 1000 :=
    by linarith
    have h29 : (k : z) ≤ 14 := by linarith
    have h30 : (n : z) ≤ 70 * 14 - 1000 :=
    by
      linarith
      exact h29
  have h31 : (n : N) ≤ 70 * 14 - 1000 := by
    norm_cast at h31
    <|>
    (try omega)
  have h32 : (n : N) > 0 := by
  exact_mod_cast h32
  norm_num at h32
  <|>
  (try omega)
  -- Now we have k ≥ 15, and we can find all
  -- possible values of k.
  have h33 : k = 20 ∨ k = 21 ∨ k = 47 ∨ k = 48
  ∨ k = 49 ∨ k = 50 := by
  -- Solve the inequalities to find
  -- possible values of k.
  have h34 : (k : z) ≥ 15 := h25
  have h35 : (k : R) ^ 2 ≤ (n : R) := h15
  have h36 : (n : R) < ((k : R) + 1) ^ 2 :=
  h20
  have h37 : (n : R) = 70 * (k : R) - 1000
  := h8
  have h38 : (k : R) ^ 2 ≤ 70 * (k : R) -
  1000 := by
    linarith
  have h39 : (k : R) ^ 2 ≤ 50 := by
  + 1) ^ 2 := by
    linarith
  have h40 : (k : z) ≤ 50 := by
  by_contra h40
  have h41 : (k : z) ≥ 51 := by linarith
  have h42 : (k : R) ≥ 51 := by
    norm_cast
    have h43 : (k : R) ^ 2 ≥ 51 ^ 2 := by
    nlinarith
    have h44 : 70 * (k : R) - 1000 < ((k :
    R) + 1) ^ 2 := h39
  nlinarith
  -- Now we know 15 ≤ k ≤ 50.
  -- We can check each possible value of k.
  have h45 : k ≤ 50 := by
  exact_mod_cast h45
  have h46 : k ≥ 15 := by
    exact_mod_cast h46
    -- Check each possible value of k from 15
    to 50.
    interval_cases k <|> norm_num at h45 h46
    <|>
    (try norm_num at h45 <|>
    (try
    {
      nlinarith [Real.sqrt_nonneg 400,
      Real.sqrt_nonneg 470, Real.sqrt_nonneg
      2290,
      Real.sqrt_nonneg 2360,
      Real.sqrt_nonneg 2430, Real.sqrt_nonneg
      2500,
      Real.sq_sqrt (show 0 ≤ (400 : R)
      by norm_num),
      Real.sq_sqrt (show 0 ≤ (470 : R)
      by norm_num),
      Real.sq_sqrt (show 0 ≤ (2290 : R)
      by norm_num),
      Real.sq_sqrt (show 0 ≤ (2360 : R)
      by norm_num),
      Real.sq_sqrt (show 0 ≤ (2430 : R)
      by norm_num),
      Real.sq_sqrt (show 0 ≤ (2500 : R)
      by norm_num)]
    } <|>
    (try
    {
      norm_num [h45 at h45 <|>
      (try omega) <|>
      (try
      {
        nlinarith [Real.sqrt_nonneg
        400, Real.sqrt_nonneg 470,
        Real.sqrt_nonneg 2290,
        Real.sqrt_nonneg 2360,
        Real.sqrt_nonneg 2430, Real.sqrt_nonneg
        2500,
        Real.sq_sqrt (show 0 ≤
        (400 : R) by norm_num),
        Real.sq_sqrt (show 0 ≤
        (470 : R) by norm_num),
        Real.sq_sqrt (show 0 ≤
        (2290 : R) by norm_num),
        Real.sq_sqrt (show 0 ≤
        (2360 : R) by norm_num),
        Real.sq_sqrt (show 0 ≤
        (2430 : R) by norm_num),
        Real.sq_sqrt (show 0 ≤
        (2500 : R) by norm_num)]
      }
    )
    )
    -- Now we know k is one of the six values.
    -- We can find the corresponding n.
    have h47 : n = 400 ∨ n = 470 ∨ n = 2290 ∨ n =
    2360 ∨ n = 2430 ∨ n = 2500 := by
    rcases h46 with (rfl | rfl | rfl | rfl | rfl |
    rfl)
    -- Case k = 20
    have h48 : (n : z) = 70 * (20 : z) -
    1000 := by
      norm_cast at h48
      <|>
      (try omega) <|>
      (try linarith)
    have h49 : n = 400 := by
      norm_cast at h49
      <|>
      (try omega) <|>
      (try linarith)
    exact Or.inl h49
    -- Case k = 21
    have h50 : (n : z) = 70 * (21 : z) -
    1000 := by
      norm_cast at h50
      <|>
      (try omega) <|>
      (try linarith)
    have h51 : n = 470 := by
      norm_cast at h51
      <|>
      (try omega) <|>
      (try linarith)
    exact Or.inr (Or.inl h51)
    -- Case k = 47
    have h52 : (n : z) = 70 * (47 : z) -
    1000 := by
      norm_cast at h52
      <|>
      (try omega) <|>
      (try linarith)
    have h53 : n = 2290 := by
      norm_cast at h53
      <|>
      (try omega) <|>
      (try linarith)
    have h54 : n = 2360 := by
      norm_cast at h54
      <|>
      (try omega) <|>
      (try linarith)
    exact Or.inr (Or.inr (Or.inl h54))
    -- Case k = 48
    have h55 : (n : z) = 70 * (48 : z) -
    1000 := by
      norm_cast at h55
      <|>
      (try omega) <|>
      (try linarith)
    have h56 : n = 2360 := by
      norm_cast at h56
      <|>
      (try omega) <|>
      (try linarith)
    exact Or.inr (Or.inr (Or.inr (Or.inl h56)))
    -- Case k = 49
    have h57 : (n : z) = 70 * (49 : z) -
    1000 := by
      norm_cast at h57
      <|>
      (try omega) <|>
      (try linarith)
    have h58 : n = 2430 := by
      norm_cast at h58
      <|>
      (try omega) <|>
      (try linarith)
    exact Or.inr (Or.inr (Or.inr (Or.inr (Or.inl h58))))
    -- Case k = 50
    have h59 : (n : z) = 70 * (50 : z) -
    1000 := by
      norm_cast at h59
      <|>
      (try omega) <|>
      (try linarith)
    have h60 : n = 2500 := by
      norm_cast at h60
      <|>
      (try omega) <|>
      (try linarith)
    exact Or.inr (Or.inr (Or.inr (Or.inr (Or.inr h60))))
    exact h59
    -- Now we know n is one of the six numbers.
    aesop
    -- Prove the reverse direction: if n is one of
    -- the six numbers, then n ∈ S.
    intro h
    have h61 : n = 400 ∨ n = 470 ∨ n = 2290 ∨ n =
    2360 ∨ n = 2430 ∨ n = 2500 := by aesop
    rcases h61 with (rfl | rfl | rfl | rfl | rfl |
    rfl)
    -- Case n = 400
    constructor
    -- Prove 0 < 400
    norm_num
    -- Prove (400 + 1000)/70 = floor(sqrt(400))
    have h62 : Int.floor (Real.sqrt (400 : N))
    = 20 := by
      norm_num [Int.floor_eq_iff,
      Real.le_sqrt, Real.sqrt_lt]
      <|>
      (try norm_num) <|>
      (try
      {
        constructor <|>
        norm_num <|>
        nlinarith [Real.sqrt_nonneg 400,
        Real.sq_sqrt (show 0 ≤ (400 : R) by
        norm_num)]
      }
    )
    have h63 : ((400 : N) : R) + 1000 = 1400 :=
    by norm_num
    have h64 : (1400 : R) / 70 = (20 : R) :=
    by norm_num
    have h65 : (Int.floor (Real.sqrt (400 : N)
    )) : R = (20 : R) := by
      rw [h65]
      <|> norm_num
      norm_num [h65 at *
      <|>
      (try simp_all) <|>
      (try norm_num) <|>
      (try linarith)
      <|>
      (try
      {
        simp_all [Int.cast_inj]
        <|> norm_num at *
        <|> linarith
      }
    )
    -- Case n = 470
    constructor
    -- Prove 0 < 470
    norm_num
    -- Prove (470 + 1000)/70 = floor(sqrt(470))
    have h66 : Int.floor (Real.sqrt (470 : N))
    = 21 := by
      norm_num [Int.floor_eq_iff,
      Real.le_sqrt, Real.sqrt_lt]
      <|>
      (try norm_num) <|>
      (try
      {
        constructor <|>
        norm_num <|>
        nlinarith [Real.sqrt_nonneg 470,
        Real.sq_sqrt (show 0 ≤ (470 : R) by
        norm_num)]
      }
    )
    have h67 : ((470 : N) : R) + 1000 = 1470 :=
    by norm_num
    have h68 : (1470 : R) / 70 = (21 : R) :=
    by norm_num
    have h69 : (Int.floor (Real.sqrt (470 : N)
    )) : R = (21 : R) := by
      rw [h69]
      <|> norm_num
      norm_num [h69 at *
      <|>
      (try simp_all) <|>
      (try norm_num) <|>
      (try linarith)
      <|>
      (try
      {
        simp_all [Int.cast_inj]
        <|> norm_num at *
        <|> linarith
      }
    )
  })

```



```

-- Case n = 2290
constructor
-- Prove 0 < 2290
norm_num
-- Prove (2290 + 1000)/70 =
floor(sqrt(2290))
have h1 : Int.floor (Real.sqrt (2290 : N
)) = 47 := by
norm_num [Int.floor_eq_iff,
Real.le_sqrt, Real.sqrt_lt]
<>
(tr try norm_num) <>
(tr try
{
constructor <>
norm_num <>
nlinarith [Real.sqrt_nonneg 2290,
Real.sq_sqrt (show 0 ≤ (2290 : R) by
norm_num)]
})
have h1 : ((2290 : N) : R) + 1000 = 3290
:= by norm_num
have h2 : (3290 : R) / 70 = (47 : R) :=
by norm_num
have h3 : (Int.floor (Real.sqrt (2290 : N
)) : R) = (47 : R) := by
rw [h1]
<> norm_num
norm_num [h1] at *
<>
(tr try simp_all) <>
(tr try norm_num) <>
(tr try linarith)
<>
(tr try
{
simp_all [Int.cast_inj]
<> norm_num at *
<> linarith
})
})
-- Case n = 2360
constructor
-- Prove 0 < 2360
norm_num
-- Prove (2360 + 1000)/70 =
floor(sqrt(2360))
have h1 : Int.floor (Real.sqrt (2360 : N
)) = 48 := by
norm_num [Int.floor_eq_iff,
Real.le_sqrt, Real.sqrt_lt]
<>
(tr try norm_num) <>
(tr try
{
constructor <>
norm_num <>
nlinarith [Real.sqrt_nonneg 2360,
Real.sq_sqrt (show 0 ≤ (2360 : R) by
norm_num)]
})
have h1 : ((2360 : N) : R) + 1000 = 3360
:= by norm_num
have h2 : (3360 : R) / 70 = (48 : R) :=
by norm_num
have h3 : (Int.floor (Real.sqrt (2360 : N
)) : R) = (48 : R) := by
rw [h1]
<> norm_num
norm_num [h1] at *
<>
(tr try simp_all) <>
(tr try norm_num) <>
(tr try linarith)
<>
(tr try
{
simp_all [Int.cast_inj]
<> norm_num at *
<> linarith
})
})
-- Case n = 2430
constructor
-- Prove 0 < 2430
norm_num
-- Prove (2430 + 1000)/70 =
floor(sqrt(2430))
have h1 : Int.floor (Real.sqrt (2430 : N
)) = 49 := by
norm_num [Int.floor_eq_iff,
Real.le_sqrt, Real.sqrt_lt]
<>
(tr try norm_num) <>
(tr try
{
constructor <>
norm_num <>
nlinarith [Real.sqrt_nonneg 2430,
Real.sq_sqrt (show 0 ≤ (2430 : R) by
norm_num)]
})
have h1 : ((2430 : N) : R) + 1000 = 3430
:= by norm_num
have h2 : (3430 : R) / 70 = (49 : R) :=
by norm_num
have h3 : (Int.floor (Real.sqrt (2430 : N
)) : R) = (49 : R) := by
rw [h1]
<> norm_num
norm_num [h1] at *
<>
(tr try simp_all) <>
(tr try norm_num) <>
(tr try linarith)
<>
(tr try
{
simp_all [Int.cast_inj]
<> norm_num at *
<> linarith
})
})
-- Case n = 2500
constructor
-- Prove 0 < 2500
norm_num
-- Prove (2500 + 1000)/70 =
floor(sqrt(2500))
have h1 : Int.floor (Real.sqrt (2500 : N
)) = 50 := by
norm_num [Int.floor_eq_iff,
Real.le_sqrt, Real.sqrt_lt]
<>
(tr try norm_num) <>
(tr try
{
constructor <>
norm_num <>
nlinarith [Real.sqrt_nonneg 2500,
Real.sq_sqrt (show 0 ≤ (2500 : R) by
norm_num)]
})
have h1 : ((2500 : N) : R) + 1000 = 3500
:= by norm_num
have h2 : (3500 : R) / 70 = (50 : R) :=
by norm_num
have h3 : (Int.floor (Real.sqrt (2500 : N
)) : R) = (50 : R) := by
rw [h1]
<> norm_num
norm_num [h1] at *
<>
(tr try simp_all) <>
(tr try norm_num) <>
(tr try linarith)
<>
(tr try
{
simp_all [Int.cast_inj]
<> norm_num at *
<> linarith
})
})
have h1 : S.card = 6 := by
rw [h1]
<> norm_num
<> rfl
exact h1
-- Simplified Proof
import Mathlib
import Aesop
set_option maxHeartbeats 0
open BigOperators Real Nat Topology Rat
theorem amc12b_2020_p21
(S : Finset N)
(h1 : ∀ (n : N), n ∈ S ↔ 0 < n ∧ (n + (1000 : R))
→ / 70 = Int.floor (Real.sqrt n)) :
S.card = 6 := by
have h1 : S = {400, 470, 2290, 2360, 2430, 2500}
:= by
ext n
simp only [Finset.mem_insert,
Finset.mem_singleton, h1]
constructor
intro h
have h1 : 0 < n := h.1
have h2 : ((n : R) + 1000) / 70 = Int.floor
(Real.sqrt n) := by
exact_mod_cast h.2
have h3 : n = 400 ∨ n = 470 ∨ n = 2290 ∨ n =
2360 ∨ n = 2430 ∨ n = 2500 := by
have h4 : (n : R) + 1000 = 70 * (Int.floor
(Real.sqrt n) : R) := by
have h5 : ((n : R) + 1000) / 70 =
(Int.floor (Real.sqrt n) : R) := by
exact_mod_cast h4
linarith
have h6 : (n : z) + 1000 = 70 * (Int.floor
(Real.sqrt n)) := by
norm_cast at h5 ⊢
have h7 : ∃ (k : z), (n : z) = 70 * k -
1000 := by
use (Int.floor (Real.sqrt n))
linarith
obtain ⟨k, h8⟩ := h7
have h9 : (n : R) = 70 * (k : R) - 1000 :=
by
norm_cast at h8 ⊢
have h10 : (k : R) ≤ Real.sqrt n := by
have h11 : (k : R) = Int.floor (Real.sqrt
n) := by
have h12 : (k : z) = Int.floor
(Real.sqrt n) := by
linarith
norm_cast at h10 ⊢
rw [h10]
exact Int.lt_floor_add_one (Real.sqrt n)
have h13 : (k : R) ^ 2 ≤ (n : R) := by
have h14 : (k : R) ≤ Real.sqrt n := h10

```

```

      norm_cast
      have h152 : n = 2500 := by
        norm_cast at h151
        <|> (try omega)
      exact (Or.inr (Or.inr (Or.inr
    (Or.inr h152))))
    aesop

intro h
have h : n = 400 ∨ n = 470 ∨ n = 2290 ∨ n =
  2360 ∨ n = 2430 ∨ n = 2500 := by aesop
rcases h with (rfl | rfl | rfl | rfl | rfl |
  rfl)

constructor
norm_num
have h : Int.floor (Real.sqrt (400 : ℕ))
  = 20 := by
  norm_num [Int.floor_eq_iff,
    Real.le_sqrt, Real.sqrt_lt]
have h : ((400 : ℕ) : ℝ) + 1000 = 1400 :=
  by norm_num
have h : (1400 : ℝ) / 70 = (20 : ℝ) :=
  by norm_num
norm_num [h] at *
<|> (try simp_all)

constructor
norm_num
have h : Int.floor (Real.sqrt (470 : ℕ))
  = 21 := by
  norm_num [Int.floor_eq_iff,
    Real.le_sqrt, Real.sqrt_lt]
have h : ((470 : ℕ) : ℝ) + 1000 = 1470 :=
  by norm_num
have h : (1470 : ℝ) / 70 = (21 : ℝ) :=
  by norm_num
norm_num [h] at *
<|> (try simp_all)

constructor
norm_num
have h : Int.floor (Real.sqrt (2290 : ℕ))
  = 47 := by
  norm_num [Int.floor_eq_iff,
    Real.le_sqrt, Real.sqrt_lt]
have h : ((2290 : ℕ) : ℝ) + 1000 = 3290
  := by norm_num
have h : (3290 : ℝ) / 70 = (47 : ℝ) :=
  by norm_num
norm_num [h] at *
<|> (try simp_all)

constructor
norm_num
have h : Int.floor (Real.sqrt (2360 : ℕ))
  = 48 := by
  norm_num [Int.floor_eq_iff,
    Real.le_sqrt, Real.sqrt_lt]
have h : ((2360 : ℕ) : ℝ) + 1000 = 3360
  := by norm_num
have h : (3360 : ℝ) / 70 = (48 : ℝ) :=
  by norm_num
norm_num [h] at *
<|> (try simp_all)

constructor
norm_num
have h : Int.floor (Real.sqrt (2430 : ℕ))
  = 49 := by
  norm_num [Int.floor_eq_iff,
    Real.le_sqrt, Real.sqrt_lt]
have h : ((2430 : ℕ) : ℝ) + 1000 = 3430
  := by norm_num
have h : (3430 : ℝ) / 70 = (49 : ℝ) :=
  by norm_num
norm_num [h] at *
<|> (try simp_all)

constructor
norm_num
have h : Int.floor (Real.sqrt (2500 : ℕ))
  = 50 := by
  norm_num [Int.floor_eq_iff,
    Real.le_sqrt, Real.sqrt_lt]
have h : ((2500 : ℕ) : ℝ) + 1000 = 3500
  := by norm_num
have h : (3500 : ℝ) / 70 = (50 : ℝ) :=
  by norm_num
norm_num [h] at *

rw [h]
norm_num
-----
-- Orig Proof
import Mathlib
import Aesop

set_option maxHeartbeats 0

open BigOperators Real Nat Topology Rat

theorem mathd_algebra_107
  (x y : ℝ)
  (h : x^2 + 8 * x + y^2 - 6 * y = 0) :
  (x + 4)^2 + (y - 3)^2 = 5^2 := by
  nlinarith
-----
-- Orig Proof
import Mathlib
import Aesop

set_option maxHeartbeats 0

open BigOperators Real Nat Topology Rat

theorem mathd_numbertheory_495
  (a b : ℕ)
  (h : 0 < a ∧ 0 < b)
  (h : a % 10 = 2)
  (h : b % 10 = 4)
  (h : Nat.gcd a b = 6) :
  108 ≤ Nat.lcm a b := by
  have h1 : a % 30 = 12 := by
    have h1 : a % 6 = 0 := by
      have h2 : 6 | a := by
        have h3 : 6 | Nat.gcd a b := by
          simp [h]
        have h4 : 6 | a := Nat.dvd_trans h3
        → (Nat.gcd_dvd_left a b)
      exact h4
    omega
  have h2 : a % 10 = 2 := h1
  have h3 : a % 30 = 12 := by
    have h4 : a % 30 = 12 := by
      omega
    exact h4
  exact h2
  omega
  have h5 : b % 30 = 24 := by
    have h6 : b % 6 = 0 := by
      have h7 : 6 | b := by
        have h8 : 6 | Nat.gcd a b := by
          simp [h]
        have h9 : 6 | b := Nat.dvd_trans h8
        → (Nat.gcd_dvd_right a b)
      exact h9
    omega
  have h9 : b % 10 = 4 := h5
  have h10 : b % 30 = 24 := by
    omega
  exact h10
  omega
  have h11 : a ≥ 42 ∨ b ≥ 54 := by
    by_contra! h
    have h12 : a < 42 := by linarith
    have h13 : b < 54 := by linarith
    have h14 : a = 12 := by
      have h15 : a % 30 = 12 := h12
      have h16 : a < 42 := h12
      have h17 : a > 0 := h12.1
      interval_cases a <|> norm_num at h14 <|>
        omega
    have h18 : b = 24 := by
      have h19 : b % 30 = 24 := h13
      have h20 : b < 54 := h13
      have h21 : b > 0 := h13.2
      interval_cases b <|> norm_num at h18 <|>
        omega
    have h22 : Nat.gcd a b = 6 := h11
    rw [h22, h14] at h11
    norm_num at h11
    <|> contradiction
  have h1 : a * b ≥ 648 := by
    have h2 : a ≥ 42 ∨ b ≥ 54 := h1
    cases h2 with
    | inl h2 =>
      -- Case: a ≥ 42
      have h3 : a ≥ 42 := h2
      have h4 : b ≥ 24 := by
        -- Prove that b ≥ 24 since b = 24 mod 30
        have h5 : b % 30 = 24 := h5
        have h6 : b > 0 := h5.2
        omega
      have h6 : a * b ≥ 42 * 24 := by
        nlinarith
      have h7 : 42 * 24 ≥ 648 := by norm_num
    | inr h2 =>
      -- Case: b ≥ 54
      have h3 : b ≥ 54 := h2
      have h4 : a ≥ 12 := by
        -- Prove that a ≥ 12 since a = 12 mod 30
        have h5 : a % 30 = 12 := h5
        have h6 : a > 0 := h5.1
        omega
      have h6 : a * b ≥ 12 * 54 := by
        nlinarith
      have h7 : 12 * 54 ≥ 648 := by norm_num
    nlinarith
  have h1 : 108 ≤ Nat.lcm a b := by
    have h2 : a * b = 6 * Nat.lcm a b := by
      have h3 : Nat.gcd a b = 6 := h1
      have h4 : a * b = Nat.gcd a b * Nat.lcm a b
        → by

```



```

norm_num [pow_succ]
<>
positivity

have h_num : (2^2014 + 2^2012 : ℕ) = (2^2012 : ℕ)
  => 5 := by
  norm_num [pow_succ, pow_add, pow_mul,
    => mul_assoc]
  <>
  ring_nf at *
  <>
  norm_num
  <>
  linarith

have h_den : (2^2014 - 2^2012 : ℕ) = (2^2012 : ℕ)
  => 3 := by
  norm_num [pow_succ, pow_add, pow_mul,
    => mul_assoc]
  <>
  ring_nf at *
  <>
  norm_num
  <>
  linarith

have h_main : (2^2014 + 2^2012 : ℕ) / (2^2014 -
  2^2012 : ℕ) = (5 : ℕ) / 3 := by
  rw [h_num, h_den]
  have h : (2 : ℕ) ^ 2012 ≠ 0 := by positivity
  field_simp [h]
  <> ring_nf
  <> norm_num
  <> linarith

exact_mod_cast h_main

-- Simplified Proof
import Mathlib
import Aesop

set_option maxHeartbeats 0

open BigOperators Real Nat Topology Rat

theorem amc12a_2013_p4 :
  (2^2014 + 2^2012) / (2^2014 - 2^2012) = (5 : ℕ) /
  3 := by
  norm_num
  -----
  -- Orig Proof
  import Mathlib
  import Aesop

set_option maxHeartbeats 0

open BigOperators Real Nat Topology Rat

theorem mathd_algebra_392
  (n : ℕ)
  (h₁ : Even n)
  (h₂ : ((n : z) - 2)^2 + (n : z)^2 + ((n : z) + 2)^2 =
    12296) :
  ((n - 2) * n * (n + 2)) / 8 = 32736 := by
  have h₃ : n = 64 := by
    have h₄ : (3 : z) * (n : z) ^ 2 + 8 = 12296 :=
      by
        have h₅ : ((n : z) - 2) ^ 2 + (n : z) ^ 2 +
          ((n : z) + 2) ^ 2 = 12296 := h₂
        ring_nf at h₅
        <> linarith
    have h₆ : (n : z) ^ 2 = 4096 := by
      have h₇ : (3 : z) * (n : z) ^ 2 + 8 = 12296
        => h₄
    linarith
  have h₈ : n ^ 2 = 4096 := by
    norm_cast at h₆
    <> linarith
  have h₉ : n = 64 := by
    have h₁₀ : n ≤ 100 := by
      interval_cases n <> norm_num at h₉
    (try omega) <>
    {
      simp_all [Nat.even_iff]
      <> omega
    }
  exact h₉

have h₁ : ((n - 2) * n * (n + 2)) / 8 = 32736 :=
  by
  rw [h₉]
  <> norm_num
  <> rfl

apply h

-- Simplified Proof
import Mathlib
import Aesop

set_option maxHeartbeats 0

open BigOperators Real Nat Topology Rat

theorem mathd_algebra_392
  (n : ℕ)
  (h₁ : Even n)
  (h₂ : ((n : z) - 2)^2 + (n : z)^2 + ((n : z) + 2)^2 =
    12296) :
  ((n - 2) * n * (n + 2)) / 8 = 32736 := by
  have : n = 64 := by
    linarith
  simp_all
  -----
  -- Orig Proof
  import Mathlib
  import Aesop

```

```

set_option maxHeartbeats 0

open BigOperators Real Nat Topology Rat

theorem mathd_numbertheory_343 :
  (n k ∈ Finset.range 6, (2 * k + 1)) % 10 = 5 := by
  have h_main : (n k ∈ Finset.range 6, (2 * k + 1))
    % 10 = 5 := by
    decide
  exact h_main

-- Simplified Proof
import Mathlib
import Aesop

set_option maxHeartbeats 0

open BigOperators Real Nat Topology Rat

theorem mathd_numbertheory_343 :
  (n k ∈ Finset.range 6, (2 * k + 1)) % 10 = 5 := by
  decide
  -----
  -- Orig Proof
  import Mathlib
  import Aesop

set_option maxHeartbeats 0

open BigOperators Real Nat Topology Rat

theorem mathd_numbertheory_314
  (r n : ℕ)
  (h₁ : r = 1342 % 13)
  (h₂ : 0 < n)
  (h₃ : 1342n)
  (h₄ : n % 13 < r) :
  6710 ≤ n := by
  have h₅ : r = 3 := by
    rw [h₁]
    <> norm_num
    <> rfl

  have h_main : 6710 ≤ n := by
    have h₆ : n % 13 < 3 := by
      rw [h₄] at h₆
      exact h₆
    -- Express n as a multiple of 1342
    obtain (k, rfl) := h₆
    have h₇ : 0 < k := by
      by_contra h₇
      -- If k = 0, then n = 0, which contradicts h₄
      => 0 < n
    push_neg at h₇
    have h₈ : k = 0 := by omega
    simp [h₈] at h₇
    <> omega
    -- We still show that if k < 4, then (1342 * k)
    -- % 13 > 3, which contradicts h₄
    by_contra! h₈
    have h₉ : k ≤ 4 := by
      by_contra h₉
      -- If k ≥ 5, then 1342 * k ≥ 1342 * 5 = 6710,
      -- which contradicts h₄ : 1342 * k < 6710
      have h₁₀ : k ≥ 5 := by omega
      have h₁₁ : 1342 * k ≥ 1342 * 5 := by
        linarith
      omega
    -- Check each case k = 1, 2, 3, 4
    interval_cases k <> norm_num [Nat.mul_mod,
      => Nat.add_mod, Nat.mod_mod] at h₈
    <>
    (try omega) <> (try contradiction)

  exact h_main

-- Simplified Proof
import Mathlib
import Aesop

set_option maxHeartbeats 0

open BigOperators Real Nat Topology Rat

theorem mathd_numbertheory_314
  (r n : ℕ)
  (h₁ : r = 1342 % 13)
  (h₂ : 0 < n)
  (h₃ : 1342n)
  (h₄ : n % 13 < r) :
  6710 ≤ n := by
  rw [h₁] at h₄
  cases' h₄ with k hk
  have : k ≥ 5 := by
    by_contra h
    push_neg at h
    interval_cases k <> omega
  linarith

-- Orig Proof
import Mathlib
import Aesop

set_option maxHeartbeats 0

open BigOperators Real Nat Topology Rat

theorem induction_prodiplonk3le3mionn
  (n : ℕ)
  (h₁ : 0 < n) :
  n k ∈ Finset.Icc 1 n, (1 + (1 : ℝ) / k^3) ≤ (3 : ℝ)
  => 1 / n := by
  induction' h₁ with n hn IH
  . -- Base case: n = 1
    simp using h_base
  . -- Inductive step: assume the statement
    -- holds for n, prove for n + 1
    simp using h_inductive_step n hn IH
  -- Apply the general result to the specific n
  exact h₁ n h₁

exact h_main

-- Simplified Proof
import Mathlib
import Aesop

set_option maxHeartbeats 0

open BigOperators Real Nat Topology Rat

theorem induction_prodiplonk3le3mionn
  (n : ℕ)
  (h₁ : 0 < n) :
  n k ∈ Finset.Icc 1 n, (1 + (1 : ℝ) / k^3) ≤ (3 : ℝ)
  => 1 / n := by
  induction' h₁ with n hn IH
  norm_num
  rw [Finset.prod_Icc_succ_top (by omega : 1 ≤ n +
    1)]
  refine' (mul_le_mul_of_nonneg_right IH (by
    => positivity)).trans _
  have : 0 < (n : ℝ) := by exact_mod_cast hn
  field_simp
  rw [div_le_div_iff (by positivity) (by
    => positivity)]
  ring_nf
  linarith

-----
-- Orig Proof
import Mathlib
import Aesop

set_option maxHeartbeats 0

open BigOperators Real Nat Topology Rat

theorem mathd_algebra_756
  (a b : ℝ)
  (h₁ : (2 : ℝ)^a = 32)
  (h₂ : a^b = 125) :
  b^a = 243 := by
  have h₃ : a = 5 := by
    have h₄ : (2 : ℝ) ^ a = 32 := h₁
    have h₅ : (2 : ℝ) ^ a = (2 : ℝ) ^ (5 : ℝ) := by
      norm_num at h₄
    <> linarith
  -- Use the injectivity of the exponential
  -- function to conclude that a = 5
  have h₆ : a = 5 := by
    apply_fun (fun x => Real.logb 2 x) at h₃
    <>
    field_simp [Real.logb_pow, Real.logb_rpow,
      => Real.logb_pow] at h₃
    <>
    norm_num at h₃
    <> linarith
  exact h₆

```

```

have h_inductive_step : ∀ (m : ℕ), 0 < m => (n k ∈
  => Finset.Icc 1 m, (1 + (1 : ℝ) / k^3) ≤
  => (3 : ℝ) - 1 / (m : ℝ)) => (n k ∈ Finset.Icc
  => 1 (m + 1), (1 + (1 : ℝ) / k^3) ≤ (3 : ℝ) - 1
  => / ((m + 1 : ℕ) : ℝ)) := by
  intro m hm h_ind
  have h₁ : n k ∈ Finset.Icc 1 (m + 1), (1 +
  => (1 : ℝ) / k^3) = (n k ∈ Finset.Icc 1 m, (1 +
  => (1 : ℝ) / k^3)) * (1 + (1 : ℝ) / ((m + 1 : ℕ)
  => ) : ℝ)^3 := by
  rw [Finset.prod_Icc_succ_top (by omega : 1 ≤
  => m + 1)]
  <> simp [Nat.cast_add, Nat.cast_one]
  <> ring_nf
  <> field_simp
  <> ring_nf
  rw [h₁]
  have h₂ : (n k ∈ Finset.Icc 1 m, (1 + (1 : ℝ) /
  => k^3)) * (1 + (1 : ℝ) / ((m + 1 : ℕ) : ℝ)^3)
  => ≤ ((3 : ℝ) - 1 / (m : ℝ)) * (1 + (1 : ℝ) /
  => ((m + 1 : ℕ) : ℝ)^3) := by
  have h₃ : 0 ≤ (1 + (1 : ℝ) / ((m + 1 : ℕ) : ℝ
  => )^3 : ℝ) := by positivity
  have h₄ : (n k ∈ Finset.Icc 1 m, (1 + (1 : ℝ) /
  => k^3)) ≤ (3 : ℝ) - 1 / (m : ℝ) := h_ind
  linarith
  have h₅ : ((3 : ℝ) - 1 / (m : ℝ)) * (1 + (1 : ℝ) /
  => ((m + 1 : ℕ) : ℝ)^3) ≤ (3 : ℝ) - 1 / ((m +
  => 1 : ℕ) : ℝ) := by
  have h₆ : 0 < (m : ℝ) := by exact_mod_cast hm
  have h₇ : 0 < ((m + 1 : ℕ) : ℝ) := by
    => positivity
  have h₈ : 0 < (m : ℝ) * ((m + 1 : ℕ) : ℝ) ^ 3
  => := by positivity
  field_simp [h₆.ne', h₇.ne']
  rw [div_le_div_iff (by positivity) (by
  => positivity)]
  ring_nf
  linarith [sq_nonneg ((m : ℝ) - 1),
    => sq_nonneg ((m : ℝ) + 1)]
  linarith

have h_main : n k ∈ Finset.Icc 1 n, (1 + (1 : ℝ) /
  => k^3) ≤ (3 : ℝ) - 1 / (n : ℝ) := by
  have h₁ : ∀ (n : ℕ), 0 < n => n k ∈ Finset.Icc 1
  => n, (1 + (1 : ℝ) / k^3) ≤ (3 : ℝ) - 1 / (n : ℝ)
  => := by
  intro n hn
  induction' hn with n hn IH
  . -- Base case: n = 1
    simp using h_base
  . -- Inductive step: assume the statement
    -- holds for n, prove for n + 1
    simp using h_inductive_step n hn IH
  -- Apply the general result to the specific n
  exact h₁ n h₁

exact h_main

-- Simplified Proof
import Mathlib
import Aesop

set_option maxHeartbeats 0

open BigOperators Real Nat Topology Rat

theorem induction_prodiplonk3le3mionn
  (n : ℕ)
  (h₁ : 0 < n) :
  n k ∈ Finset.Icc 1 n, (1 + (1 : ℝ) / k^3) ≤ (3 : ℝ)
  => 1 / n := by
  induction' h₁ with n hn IH
  norm_num
  rw [Finset.prod_Icc_succ_top (by omega : 1 ≤ n +
    1)]
  refine' (mul_le_mul_of_nonneg_right IH (by
    => positivity)).trans _
  have : 0 < (n : ℝ) := by exact_mod_cast hn
  field_simp
  rw [div_le_div_iff (by positivity) (by
    => positivity)]
  ring_nf
  linarith

-----
-- Orig Proof
import Mathlib
import Aesop

set_option maxHeartbeats 0

open BigOperators Real Nat Topology Rat

theorem mathd_algebra_756
  (a b : ℝ)
  (h₁ : (2 : ℝ)^a = 32)
  (h₂ : a^b = 125) :
  b^a = 243 := by
  have h₃ : a = 5 := by
    have h₄ : (2 : ℝ) ^ a = 32 := h₁
    have h₅ : (2 : ℝ) ^ a = (2 : ℝ) ^ (5 : ℝ) := by
      norm_num at h₄
    <> linarith
  -- Use the injectivity of the exponential
  -- function to conclude that a = 5
  have h₆ : a = 5 := by
    apply_fun (fun x => Real.logb 2 x) at h₃
    <>
    field_simp [Real.logb_pow, Real.logb_rpow,
      => Real.logb_pow] at h₃
    <>
    norm_num at h₃
    <> linarith
  exact h₆

```

```

have h_b : b = 3 := by
  have h_1 : a ^ b = 125 := h_1
  rw [h_a] at h_1
  have h_2 : (5 : ℕ) ^ b = 125 := by
    exact_mod_cast h_1
  have h_3 : (5 : ℕ) ^ b = (5 : ℕ) ^ (3 : ℕ) := by
    norm_num at h_1
  <|>
  linarith
-- Use the injectivity of the exponential
-- function to conclude that b = 3
have h_4 : b = 3 := by
  apply_fun (fun x => Real.logb 5 x) at h_1
  <|>
  field_simp [Real.logb_pow, Real.logb_rpow,
    Real.logb_pow] at h_1
  <|>
  norm_num at h_1
  <|>
  linarith
exact_mod_cast h_4

have h_main : b * a = 243 := by
  rw [h_b, h_a]
  norm_num
  <|>
  simp [pow_succ]
  <|>
  norm_num
  <|>
  rfl

exact h_main

-- Simplified Proof
import Mathlib
import Aesop

set_option maxHeartbeats 0

open BigOperators Real Nat Topology Rat

theorem mathd_algebra_756
  (a b : ℕ)
  (h_1 : (2 : ℕ) ^ a = 32)
  (h_2 : a ^ b = 125) :
  b * a = 243 := by
  have : a = 5 := by
    rw [show (32 : ℕ) = 2 ^ 5 by norm_num] at h_1
    apply_fun fun x => logb 2 x at h_1
    field_simp [Real.logb_pow] at h_1
    linarith
  subst this
  have : b = 3 := by
    rw [show (125 : ℕ) = 5 ^ 3 by norm_num] at h_2
    apply_fun fun x => logb 5 x at h_2
    field_simp [Real.logb_pow] at h_2
    linarith
  subst this
  norm_num

-- Orig Proof
import Mathlib
import Aesop

set_option maxHeartbeats 0

open BigOperators Real Nat Topology Rat

theorem mathd_algebra_80
  (x : ℕ)
  (h_1 : x ≠ -1)
  (h_2 : (x - 9) / (x + 1) = 2) :
  x = -11 := by
  have h_main : x = -11 := by
    intro h
    apply h
    linarith
  -- Eliminate the fraction by multiplying both
  -- sides by (x + 1)
  field_simp [h_1] at h
  -- Simplify the equation to x - 9 = 2 * (x + 1)
  ring_nf at h
  -- Solve the linear equation x - 9 = 2x + 2
  linarith
  exact h_main

-- Simplified Proof
import Mathlib
import Aesop

set_option maxHeartbeats 0

open BigOperators Real Nat Topology Rat

theorem mathd_algebra_80
  (x : ℕ)
  (h_1 : x ≠ -1)
  (h_2 : (x - 9) / (x + 1) = 2) :
  x = -11 := by
  rw [div_eq_iff] at h_1
  linarith
  aesop

-- Orig Proof
import Mathlib
import Aesop

set_option maxHeartbeats 0

open BigOperators Real Nat Topology Rat

theorem amc12b_2002_p7
  (a b c : ℕ)
  (h_1 : 0 < a ∧ 0 < b ∧ 0 < c)
  (h_2 : b = a + 1)
  (h_3 : c = b + 1)
  (h_4 : a * b * c = 8 * (a + b + c)) :
  a^2 + (b^2 + c^2) = 77 := by
  subst_vars
  nlinarith

-- Orig Proof
import Mathlib
import Aesop

set_option maxHeartbeats 0

open BigOperators Real Nat Topology Rat

theorem mathd_numbertheory_457
  (n : ℕ)
  (h_1 : 0 < n)
  (h_2 : 80325 (n !)) :
  17 ≤ n := by
  have h_1 : 17 ≤ 80325 := by norm_num
  exact dvd_trans h_1 h_2

have h_1 : 17 ≤ n := by
  by_contra h
  -- Assume n < 17 and derive a contradiction
  have h_1 : n ≤ 16 := by linarith
  interval_cases n <|> norm_num
  -- [Nat.factorial_succ,
  -- Nat.dvd_iff_mod_eq_zero] at h_1
  <|>
  (try omega) <|> (try contradiction)

exact h_1

-- Simplified Proof
import Mathlib
import Aesop

set_option maxHeartbeats 0

open BigOperators Real Nat Topology Rat

theorem mathd_numbertheory_457
  (n : ℕ)
  (h_1 : 0 < n)
  (h_2 : 80325 (n !)) :
  17 ≤ n := by
  contrapose! h_1
  interval_cases n <|> norm_num

-- Orig Proof
import Mathlib
import Aesop

set_option maxHeartbeats 0

have h_1 : c = b + 1 := h_1
have h_2 : b = a + 1 := h_1
rw [h_1] at h_1
omega

have h_1 : a = 4 := by
  have h_1 : a * b * c = 8 * (a + b + c) := h_1
  have h_2 : b = a + 1 := h_1
  have h_3 : c = a + 2 := h_1
  rw [h_1, h_2] at h_1
  ring_nf at h_1
  have h_4 : a ≤ 6 := by
    by_contra! h
    have h_5 : a ≥ 7 := by omega
    have h_6 : a * (a + 1) * (a + 2) > 8 * (a +
      (a + 1) + (a + 2)) := by
      have h_7 : a ≥ 7 := h_5
      have h_8 : a * (a + 1) * (a + 2) ≥ 7 * (a +
        1) * (a + 2) := by
        gcongr <|> nlinarith
      have h_9 : 7 * (a + 1) * (a + 2) > 8 * (a +
        (a + 1) + (a + 2)) := by
        nlinarith
      nlinarith
      interval_cases a <|> norm_num at h_1
      <|>
      (try omega) <|> (try nlinarith)

have h_1 : b = 5 := by
  have h_1 : b = a + 1 := h_1
  rw [h_1]
  have h_2 : a = 4 := h_1
  rw [h_1]
  <|> norm_num

have h_1 : c = 6 := by
  have h_1 : c = a + 2 := h_1
  rw [h_1]
  have h_2 : a = 4 := h_1
  rw [h_1]
  <|> norm_num

have h_1 : a^2 + (b^2 + c^2) = 77 := by
  have h_1 : a = 4 := h_1
  have h_2 : b = 5 := h_1
  have h_3 : c = 6 := h_1
  subst_vars
  <|> norm_num
  <|> ring_nf at *
  <|> norm_num at *
  <|> linarith

apply h_1

-- Simplified Proof
import Mathlib
import Aesop

set_option maxHeartbeats 0

open BigOperators Real Nat Topology Rat

theorem amc12b_2002_p7
  (a b c : ℕ)
  (h_1 : 0 < a ∧ 0 < b ∧ 0 < c)
  (h_2 : b = a + 1)
  (h_3 : c = b + 1)
  (h_4 : a * b * c = 8 * (a + b + c)) :
  a^2 + (b^2 + c^2) = 77 := by
  subst_vars
  nlinarith

-- Orig Proof
import Mathlib
import Aesop

set_option maxHeartbeats 0

open BigOperators Real Nat Topology Rat

theorem mathd_numbertheory_457
  (n : ℕ)
  (h_1 : 0 < n)
  (h_2 : 80325 (n !)) :
  17 ≤ n := by
  have h_1 : 17 ≤ 80325 := by norm_num
  exact dvd_trans h_1 h_2

have h_1 : 17 ≤ n := by
  by_contra h
  -- Assume n < 17 and derive a contradiction
  have h_1 : n ≤ 16 := by linarith
  interval_cases n <|> norm_num
  -- [Nat.factorial_succ,
  -- Nat.dvd_iff_mod_eq_zero] at h_1
  <|>
  (try omega) <|> (try contradiction)

exact h_1

-- Simplified Proof
import Mathlib
import Aesop

set_option maxHeartbeats 0

open BigOperators Real Nat Topology Rat

theorem amc12_2000_p12
  (a m c : ℕ)
  (h_1 : a + m + c = 12) :
  a * m * c + a * m + m * c + a * c ≤ 112 := by
  have h_main : a * m * c + a * m + m * c + a * c ≤ 112 := by
    have h_1 : a ≤ 12 := by
      omega
    have h_2 : m ≤ 12 := by
      omega
    have h_3 : c ≤ 12 := by
      omega
    -- We will consider all possible values of a,
    -- m, c that satisfy the constraints
    interval_cases a <|> interval_cases m <|> omega
  exact h_main

-- Simplified Proof
import Mathlib

```

```

import Aesop

set_option maxHeartbeats 0

open BigOperators Real Nat Topology Rat

theorem amc12_2000_p12
(a m c : ℕ)
(h₁ : a + m + c = 12) :
a + m + c + a + m + c + a + m + c ≤ 112 := by
have : a ≤ 12 := by omega
have : m ≤ 12 := by omega
have : c ≤ 12 := by omega
interval_cases a <|> interval_cases m <|> omega
-----
-- Orig Proof
import Mathlib
import Aesop

set_option maxHeartbeats 0

open BigOperators Real Nat Topology Rat

theorem mathd_numbertheory_135
(n A B C : ℕ)
(h₁ : n = 3^17 + 3^10)
(h₂ : 11 ∣ (n + 1))
(h₃ : {A,B,C}.Pairwise (· ∣ ·))
(h₄ : {A,B,C} ⊆ Finset.Icc 0 9)
(h₅ : Odd A ∧ Odd C)
(h₆ : ~ 3 ∣ B)
(h₇ : Nat.digits 10 n = [B,A,B,C,C,A,C,B,A]) :
100 * A + 10 * B + C = 129 := by
have h₈ : n = 129199212 := by
rw [h₇]
<|> norm_num
<|> rfl

have h₉ : Nat.digits 10 n = [2,1,2,9,9,1,9,2,1] :=
  by
  rw [h₇]
  <|> norm_num [Nat.digits_len]
  <|> rfl

have h₁₀ : [B,A,B,C,C,A,C,B,A] =
  [2,1,2,9,9,1,9,2,1] := by
have h₁₁ : [B,A,B,C,C,A,C,B,A] =
  [2,1,2,9,9,1,9,2,1] := by
  rw [← h₉, h₈]
  <|>
  (try decide) <|>
  (try simp_all [List.cons, List.nil]) <|>
  (try ring_nf at *) <|>
  (try norm_num at *) <|>
  (try omega)
exact h₁₁

have h₁₂ : B = 2 := by
have h₁₃ : B = 2 := by
have h₁₄ := congr_arg (fun l => 1.get? 0) h₈
simp [List.get?] at h₁₄
<|>
(try cases B <|> simp_all (config := {decide
  => := true})) <|>
(try omega)
exact h₁₄

have h₁₅ : A = 1 := by
have h₁₆ : A = 1 := by
have h₁₇ := congr_arg (fun l => 1.get? 1) h₈
simp [List.get?] at h₁₇
<|>
(try cases A <|> simp_all (config := {decide
  => := true})) <|>
(try omega)
exact h₁₇

have h₁₈ : C = 9 := by
have h₁₉ : C = 9 := by
have h₂₀ := congr_arg (fun l => 1.get? 3) h₈
simp [List.get?] at h₂₀
<|>
(try cases C <|> simp_all (config := {decide
  => := true})) <|>
(try omega)
exact h₂₀

have h₂₁ : 100 * A + 10 * B + C = 129 := by
rw [h₁₅, h₁₈, h₁₉]
<|> norm_num
<|> rfl

exact h₂₁

-- Simplified Proof
import Mathlib
import Aesop

set_option maxHeartbeats 0

open BigOperators Real Nat Topology Rat

theorem mathd_numbertheory_135
(n A B C : ℕ)
(h₁ : n = 3^17 + 3^10)
(h₂ : 11 ∣ (n + 1))
(h₃ : {A,B,C}.Pairwise (· ∣ ·))
(h₄ : {A,B,C} ⊆ Finset.Icc 0 9)
(h₅ : Odd A ∧ Odd C)
(h₆ : ~ 3 ∣ B)
(h₇ : Nat.digits 10 n = [B,A,B,C,C,A,C,B,A]) :
100 * A + 10 * B + C = 129 := by
simp_all
omega
-----
-- Orig Proof
import Mathlib
import Aesop

set_option maxHeartbeats 0

open BigOperators Real Nat Topology Rat

theorem mathd_algebra_263
(y : ℝ)
(h₁ : 0 ≤ 19 + 3 * y)
(h₂ : Real.sqrt (19 + 3 * y) = 7) :
y = 10 := by
have h₃ : (Real.sqrt (19 + 3 * y)) ^ 2 = 19 + 3 *
  y := by
  rw [Real.sq_sqrt]
  <|> linarith

have h₄ : (Real.sqrt (19 + 3 * y)) ^ 2 = 49 := by
  rw [h₃]
  <|> norm_num

have h₅ : 19 + 3 * y = 49 := by
  linarith

have h₆ : 3 * y = 30 := by
  linarith

have h₇ : y = 10 := by
  linarith

exact h₇

-- Simplified Proof
import Mathlib
import Aesop

set_option maxHeartbeats 0

open BigOperators Real Nat Topology Rat

theorem mathd_algebra_263
(y : ℝ)
(h₁ : 0 ≤ 19 + 3 * y)
(h₂ : Real.sqrt (19 + 3 * y) = 7) :
y = 10 := by
  linarith [Real.sq_sqrt h₁]
-----
-- Orig Proof
import Mathlib
import Aesop

set_option maxHeartbeats 0

open BigOperators Real Nat Topology Rat

theorem amc12a_2020_p7
(a : ℕ → ℕ)
(h₁ : (a 0)^3 = 1)
(h₂ : (a 1)^3 = 8)
(h₃ : (a 2)^3 = 27)
(h₄ : (a 3)^3 = 64)
(h₅ : (a 4)^3 = 125)
(h₆ : (a 5)^3 = 216)
(h₇ : (a 6)^3 = 343) :
∑ k ∈ Finset.range 7, (6 * (a k)^2) - ∑ (2 * ∑ k ∈
  Finset.range 6, (a k)^2) = 658 := by
have h₈ a0 : a 0 = 1 := by
have h₉ : a 0 = 1 := by
have h₁₀ : (a 0)^3 = 1 := h₈
have h₁₁ : a 0 ≤ 1 := by
  linarith [pow_two_nonneg (a 0),
    pow_two_nonneg (a 0 - 1)]
interval_cases a 0 <|> norm_num at h₁₁ <|>
(try omega) <|>
(try linarith)
<|>
(try
  {
    simp_all [pow_succ]
    <|> nlinarith
  })
exact h₁₁

have h₁₂ a1 : a 1 = 2 := by
have h₁₃ : a 1 = 2 := by
have h₁₄ : (a 1)^3 = 8 := h₁₂
have h₁₅ : a 1 ≤ 2 := by
  linarith [pow_two_nonneg (a 1),
    pow_two_nonneg (a 1 - 2)]
interval_cases a 1 <|> norm_num at h₁₅ <|>
(try omega) <|>
(try linarith)
<|>
(try
  {
    simp_all [pow_succ]
    <|> nlinarith
  })
exact h₁₄

have h₁₆ a2 : a 2 = 3 := by
have h₁₇ : a 2 = 3 := by
have h₁₈ : (a 2)^3 = 27 := h₁₆
have h₁₉ : a 2 ≤ 3 := by
  linarith [pow_two_nonneg (a 2),
    pow_two_nonneg (a 2 - 3)]
interval_cases a 2 <|> norm_num at h₁₉ <|>
(try omega) <|>
(try linarith)
<|>
(try
  {
    simp_all [pow_succ]
    <|> nlinarith
  })
exact h₁₈

have h₂₀ a3 : a 3 = 4 := by
have h₂₁ : a 3 = 4 := by
have h₂₂ : (a 3)^3 = 64 := h₂₀
have h₂₃ : a 3 ≤ 4 := by
  linarith [pow_two_nonneg (a 3),
    pow_two_nonneg (a 3 - 4)]
interval_cases a 3 <|> norm_num at h₂₃ <|>
(try omega) <|>
(try linarith)
<|>
(try
  {
    simp_all [pow_succ]
    <|> nlinarith
  })
exact h₂₂

have h₂₄ a4 : a 4 = 5 := by
have h₂₅ : a 4 = 5 := by
have h₂₆ : (a 4)^3 = 125 := h₂₄
have h₂₇ : a 4 ≤ 5 := by
  linarith [pow_two_nonneg (a 4),
    pow_two_nonneg (a 4 - 5)]
interval_cases a 4 <|> norm_num at h₂₇ <|>
(try omega) <|>
(try linarith)
<|>
(try
  {
    simp_all [pow_succ]
    <|> nlinarith
  })
exact h₂₆

have h₂₈ a5 : a 5 = 6 := by
have h₂₉ : a 5 = 6 := by
have h₃₀ : (a 5)^3 = 216 := h₂₈
have h₃₁ : a 5 ≤ 6 := by
  linarith [pow_two_nonneg (a 5),
    pow_two_nonneg (a 5 - 6)]
interval_cases a 5 <|> norm_num at h₃₁ <|>
(try omega) <|>
(try linarith)
<|>
(try
  {
    simp_all [pow_succ]
    <|> nlinarith
  })
exact h₃₀

have h₃₂ a6 : a 6 = 7 := by
have h₃₃ : a 6 = 7 := by
have h₃₄ : (a 6)^3 = 343 := h₃₂
have h₃₅ : a 6 ≤ 7 := by
  linarith [pow_two_nonneg (a 6),
    pow_two_nonneg (a 6 - 7)]
interval_cases a 6 <|> norm_num at h₃₅ <|>
(try omega) <|>
(try linarith)
<|>
(try
  {
    simp_all [pow_succ]
    <|> nlinarith
  })
exact h₃₄

have h₃₆_sum_main : ∑ k ∈ Finset.range 7, (6 * (a
  k)^2) - ∑ (2 * ∑ k ∈ Finset.range 6, (a
  k)^2) = 658 := by
  simp [Finset.sum_range_succ, h₈ a0, h₉ a1, h₁₂ a2,
    h₁₆ a3, h₂₀ a4, h₂₄ a5, h₂₈ a6]
  <|> norm_num
  <|> rfl

exact h₃₆_sum_main

-- Simplified Proof
import Mathlib
import Aesop

set_option maxHeartbeats 0

open BigOperators Real Nat Topology Rat

theorem amc12a_2020_p7
(a : ℕ → ℕ)
(h₁ : (a 0)^3 = 1)
(h₂ : (a 1)^3 = 8)
(h₃ : (a 2)^3 = 27)
(h₄ : (a 3)^3 = 64)
(h₅ : (a 4)^3 = 125)
(h₆ : (a 5)^3 = 216)
(h₇ : (a 6)^3 = 343) :
∑ k ∈ Finset.range 7, (6 * (a k)^2) - ∑ (2 * ∑ k ∈
  Finset.range 6, (a k)^2) = 658 := by
norm_num
have h₈ : ∀ k ≤ 6, a k = k + 1 := by
  intro k hk
  interval_cases k <|> simp_all [Nat.pow_succ]
  <|> nlinarith
  simp_all [Finset.sum_range_succ]
-----
-- Orig Proof
import Mathlib
import Aesop

set_option maxHeartbeats 0

open BigOperators Real Nat Topology Rat

theorem induction_sumkexp3eqsumsq
(n : ℕ) :
∑ k ∈ Finset.range n, k^3 = (∑ k ∈ Finset.range
  n, k)^2 := by
have h_lemma : ∀ (n : ℕ), 2 * ∑ k in Finset.range
  n, k = ∑ m * (m - 1) := by
  intro m
  have h : ∀ m : ℕ, 2 * ∑ k in Finset.range m, k =
    ∑ m * (m - 1) := by

```

```

intro m
induction m with
| zero => simp
| succ m ih =>
  cases m with
  | zero => simp [Finset.sum_range_succ]
  | succ m =>
    simp_all [Finset.sum_range_succ,
      → Nat.succ_eq_add_one, mul_add, mul_one,
      → add_mul]
    <|> ring_nf at *
    <|> nlinarith
exact h m

have h_main :  $\exists k \in \text{Finset.range } n, k^3 = (\sum k \in \text{Finset.range } n, k)^2$  := by
  have h :  $\forall n : \mathbb{N}, \exists k \in \text{Finset.range } n, k^3 = (\sum k \in \text{Finset.range } n, k)^2$  := by
    intro n
    induction n with
    | zero => simp
    | succ n ih =>
      rw [Finset.sum_range_succ,
        → Finset.sum_range_succ]
      simp [ih, pow_two, Nat.mul_add,
        → Nat.add_mul]
      have h₁ := h.lemma n
      have h₂ :  $2 * \sum k \in \text{Finset.range } n, k = n * (n - 1)$  := h.lemma n
      have h₃ :  $n * (n - 1) = 2 * \sum k \in \text{Finset.range } n, k$  := by
        → Finset.range n, k := by
          linarith
      cases n with
      | zero => simp
      | succ n =>
        simp [Finset.sum_range_succ, pow_two,
          → Nat.mul_add, Nat.add_mul, Nat.mul_one,
          → Nat.mul_zero] at *
        <|> ring_nf at *
        <|> nlinarith
    exact h n

exact h_main

-- Simplified Proof
import Mathlib
import Aesop

set_option maxHeartbeats 0

open BigOperators Real Nat Topology Rat

theorem induction_sumkexp3eqsumksq
  (n : ℕ) :
   $\exists k \in \text{Finset.range } n, k^3 = (\sum k \in \text{Finset.range } n, k)^2$  := by
    induction n with
    | zero => simp
    | succ n ih =>
      rw [Finset.sum_range_succ,
        → Finset.sum_range_succ]
      simp [ih]
      ring_nf
      have h_lemma :  $\forall m : \mathbb{N}, 2 * \sum k \in \text{Finset.range } m, k = m * (m - 1)$  := by
        intro m
        induction m with
        | zero => simp
        | succ m ih =>
          cases m with
          | zero => simp [Finset.sum_range_succ]
          | succ m =>
            simp_all [Finset.sum_range_succ,
              → Nat.succ_eq_add_one, mul_add, mul_one,
              → add_mul]
            <|> ring_nf at *
            have h₁ := h.lemma m
            have h₂ :  $n * (n - 1) = 2 * \sum k \in \text{Finset.range } n, k$  := by
              linarith
            cases n with
            | zero => simp
            | succ n =>
              simp [Finset.sum_range_succ, pow_two,
                → Nat.mul_add, Nat.add_mul, Nat.mul_one,
                → Nat.mul_zero] at *
              <|> ring_nf at *
              <|> nlinarith
    exact h n

-- Orig Proof
import Mathlib
import Aesop

set_option maxHeartbeats 0

open BigOperators Real Nat Topology Rat

theorem mathd_numbertheory_34
  (x : ℕ)
  (h₁ :  $x < 100$ )
  (h₂ :  $x * 9 \% 100 = 1$ ) :
   $x = 89$  := by
  omega

-- Orig Proof
import Mathlib
import Aesop

set_option maxHeartbeats 0

open BigOperators Real Nat Topology Rat

theorem imo_1981_p6
  (f :  $\mathbb{N} \rightarrow \mathbb{N} \rightarrow \mathbb{N}$ )
  (g :  $\mathbb{N} \rightarrow \mathbb{N}$ )
  (h₁ :  $\forall y, f \ 0 \ y = y + 1$ )
  (h₂ :  $\forall x, f \ (x + 1) \ 0 = f \ x \ 1$ )
  (h₃ :  $\forall x \ y, f \ (x + 1) \ (y + 1) = f \ x \ (f \ (x + 1) \ y)$ )
  (h₄ :  $g \ 0 = 2$ )
  (h₅ :  $\forall n, g \ (n + 1) = 2^{g \ n}$ ) :
   $f \ 4 \ 1981 = g \ 1983 - 3$  := by
  have h_f1 :  $\forall y, f \ 1 \ y = y + 2$  := by
    intro y
    induction y with
    | zero =>
      have h₁ := h₁ 0
      have h₂ := h₁ 1
      simp at h₁ h₂
      <|> norm_num [h₁, h₂] at *
      <|> linarith
    | succ y ih =>
      have h₁ := h₁ 0 y
      have h₂ := h₁ (f 1 y)
      have h₃ := h₁ 0
      simp [ih] at h₁ h₂ h₃
      <|> ring_nf at *
      <|> omega
    exact h y

  have h_f2 :  $\forall y, f \ 2 \ y = 2 * y + 3$  := by
    intro y
    have h :  $\forall y, f \ 2 \ y = 2 * y + 3$  := by
      induction y with
      | zero =>
        have h₁ := h₁ 1
        have h₂ := h_f1 1
        have h₃ := h₁ 1
        simp at h₁ h₂ h₃
        <|> norm_num [h₁, h₂, h₃] at *
        <|> linarith
      | succ y ih =>
        have h₁ := h₁ 1 y
        have h₂ := h_f1 (f 2 y)
        have h₃ := h₁ 1
        simp [ih] at h₁ h₂ h₃
        <|> ring_nf at *
        <|> omega
    exact h y

  have h_f3_pow :  $\forall y, f \ 3 \ y + 3 = 2^{y + 3}$  := by
    intro y
    have h :  $\forall y, f \ 3 \ y + 3 = 2^{y + 3}$  := by
      induction y with
      | zero =>
        have h₁ := h₁ 2
        have h₂ := h_f2 1
        have h₃ := h₁ 0
        have h₄ := h₁ 2 0
        have h₅ := h₁ 1 1
        simp at h₁ h₂ h₃ h₄ h₅
        <|> norm_num [h₁, h₂, h₃, h₄, h₅, h_f1,
          → h_f2] at *
        <|> linarith
      | succ y ih =>
        have h₁ := h₁ 2 y
        have h₂ := h_f2 (f 3 y)
        have h₃ := h₁ 2
        simp [ih] at h₁ h₂ h₃
        <|>
          (try ring_nf at *) <|>
          (try simp_all [pow_succ, mul_add,
            → mul_one, Nat.mul_sub_left_distrib]) <|>
          (try omega) <|>
          (try ring_nf at *) <|>
          (try norm_num at *) <|>
          (try nlinarith)
    exact h y

  have h_f4_g :  $\forall y, f \ 4 \ y + 3 = g \ (y + 2)$  := by
    intro y
    have h :  $\forall y, f \ 4 \ y + 3 = g \ (y + 2)$  := by
      induction y with
      | zero =>
        have h₁ := h₁ 3
        have h₂ := h_f3_pow 1
        have h₃ := h₁ 2 0
        have h₄ := h₁ 3 0
        have h₅ := h₁ 2 1
        have h₆ := h₁ 3 1
      | succ y ih =>
        simp [ih] at h₁ h₂ h₃ h₄ h₅ h₆
        <|>
          (try ring_nf at *) <|>
          (try simp_all [pow_succ, mul_add,
            → mul_one, Nat.mul_sub_left_distrib]) <|>
          (try omega) <|>
          (try ring_nf at *) <|>
          (try norm_num at *) <|>
          (try nlinarith)
    exact h y

  have h₁ := h₁ 1981
  have h₂ := h₁ 0
  have h₃ := h₁ 1
  have h₄ := h₁ 2
  simp at h₁ h₂ h₃ h₄
  <|> norm_num [h₁, h₂, h₃, h₄, h_f1, h_f2, h_f3_pow] at *
  <|>
    (try omega) <|>
    (try ring_nf at *) <|>
    (try norm_num at *) <|>
    (try nlinarith)
  <|>
    (try simp_all [pow_succ, mul_add,
      → mul_one, Nat.mul_sub_left_distrib]) <|>
    (try omega) <|>
    (try ring_nf at *) <|>
    (try norm_num at *) <|>
    (try nlinarith)
  <|> omega
exact h y

have h_main :  $f \ 4 \ 1981 = g \ 1983 - 3$  := by
  have h₁ :  $f \ 4 \ 1981 + 3 = g \ 1983$  := by
    have h₂ := h_f4_g 1981
    norm_num at h₂
    <|> linarith
  have h₃ :  $g \ 1983 \geq 4$  := by
    have h₄ :  $\forall n : \mathbb{N}, n \geq 1 \rightarrow g \ n \geq 4$  := by
      intro n hn
      induction' hn with n hn IH
      · -- Base case:  $n = 1$ 
        norm_num [h₁, h₂]
      · -- Inductive step: assume the statement
        -- holds for  $n$ , prove for  $n + 1$ 
        have h₅ :  $g \ (n + 1) = 2^{g \ n}$  := h₄ n
        rw [h₅]
        have h₆ :  $g \ n \geq 4$  := IH
        have h₇ :  $2^{g \ n} \geq 2^4 = 16$  := by
          apply Nat.pow_le_pow_of_le_right
            . norm_num
            . linarith
        have h₈ :  $2^{g \ n} \geq 16$  := by
          norm_num
          linarith
        have h₉ :  $1983 \geq 1$  := by norm_num
        have h₁₀ :  $g \ 1983 \geq 4$  := h₉, 1983 h₉
        linarith
    exact h₄
  exact h₁
  exact h₂
  omega
  exact h₃
  exact h
exact h_main

-- Simplified Proof
import Mathlib
import Aesop

set_option maxHeartbeats 0

open BigOperators Real Nat Topology Rat

theorem imo_1981_p6
  (f :  $\mathbb{N} \rightarrow \mathbb{N} \rightarrow \mathbb{N}$ )
  (g :  $\mathbb{N} \rightarrow \mathbb{N}$ )
  (h₁ :  $\forall y, f \ 0 \ y = y + 1$ )
  (h₂ :  $\forall x, f \ (x + 1) \ 0 = f \ x \ 1$ )
  (h₃ :  $\forall x \ y, f \ (x + 1) \ (y + 1) = f \ x \ (f \ (x + 1) \ y)$ )
  (h₄ :  $g \ 0 = 2$ )
  (h₅ :  $\forall n, g \ (n + 1) = 2^{g \ n}$ ) :
   $f \ 4 \ 1981 = g \ 1983 - 3$  := by
  have h₁ :  $\forall y, f \ 1 \ y = y + 2$  := by
    intro y
    induction y <|> simp_all
    intro y
    induction y <|> simp_all [h₁]
    <|> ring
  have h₂ :  $\forall y, f \ 3 \ y + 3 = 2^{y + 3}$  := by
    intro y
    induction y <|> simp_all [h₁]
    <|> ring_nf at *
    <|> omega
  have h₃ :  $\forall y, f \ 4 \ y + 3 = g \ (y + 2)$  := by
    intro y
    induction y <|> simp_all [h₁]
    <|> ring_nf at *
    <|> omega
  have h₄ := h₁ 1981

```

norm\_num at h,  
omega

```

-- Orig Proof
import Mathlib
import Aesop

set_option maxHeartbeats 0

open BigOperators Real Nat Topology Rat

theorem amc12b_2021_p4
(m a : ℕ)
(h₁ : 0 < m ∧ 0 < a)
(h₂ : m / a = (3 : ℝ) / 4) :
(84 * m + 70 * a) / (m + a) = (76 : ℝ) := by
have h₃ : (m : ℝ) = (3 / 4 : ℝ) * (a : ℝ) := by
have h₄ : (a : ℝ) ≠ 0 := by
have h₅ : 0 < a := h₁.2
exact by
norm_cast
<> linarith
have h₆ : (m : ℝ) / (a : ℝ) = (3 : ℝ) / 4 :=
by exact_mod_cast h₄
have h₇ : (m : ℝ) = (3 / 4 : ℝ) * (a : ℝ) := by
field_simp at h₆ ⊢
<> ring_nf at h₆ ⊢
<> try norm_num at h₆ ⊢
<> try linarith
<> try nlinarith
<> try ring_nf at h₆ ⊢
<> nlinarith
exact h₇

have h₈ : (84 : ℝ) * (m : ℝ) + (70 : ℝ) * (a : ℝ)
→ = (133 : ℝ) * (a : ℝ) := by
have h₉ : (84 : ℝ) * (m : ℝ) + (70 : ℝ) * (a : ℝ)
→ = (84 : ℝ) * ((3 / 4 : ℝ) * (a : ℝ)) +
→ (70 : ℝ) * (a : ℝ) := by
rw [h₆]
<> ring_nf
rw [h₆]
<> ring_nf
<> norm_num
<> linarith

have h₁₀ : (m : ℝ) + (a : ℝ) = (7 / 4 : ℝ) * (a : ℝ)
→ := by
have h₁₁ : (m : ℝ) + (a : ℝ) = (3 / 4 : ℝ) * (a : ℝ)
→ : (a : ℝ) + (a : ℝ) := by
rw [h₆]
<> ring_nf
<> ring_nf
<> field_simp
<> ring_nf
<> linarith

have h₁₂ : (84 * (m : ℝ) + 70 * (a : ℝ)) / ((m : ℝ)
→ + (a : ℝ)) = (76 : ℝ) := by
have h₁₃ : (m : ℝ) + (a : ℝ) ≠ 0 := by
have h₁₄ : 0 < (m : ℝ) := by exact_mod_cast
→ h₁.1
have h₁₅ : 0 < (a : ℝ) := by exact_mod_cast
→ h₁.2
linarith
have h₁₆ : (a : ℝ) ≠ 0 := by
have h₁₇ : 0 < a := h₁.2
exact by
norm_cast
<> linarith
field_simp [h₁₆, h₁₇]
<> ring_nf at *
<> norm_num at *
<> linarith

simpa using h₁

-- Simplified Proof
import Mathlib
import Aesop

set_option maxHeartbeats 0

open BigOperators Real Nat Topology Rat

theorem amc12b_2021_p4
(m a : ℕ)
(h₁ : 0 < m ∧ 0 < a)
(h₂ : m / a = (3 : ℝ) / 4) :
(84 * m + 70 * a) / (m + a) = (76 : ℝ) := by
have h₃ : (m : ℝ) = (3 / 4 : ℝ) * (a : ℝ) := by
field_simp [h₂.ne', h₁.1.ne'] at h₁ ⊢
linarith
rw [h₃]
ring_nf
<> field_simp [h₃.2.ne', h₁.1.ne']
<> linarith
-----
-- Orig Proof
import Mathlib
import Aesop

set_option maxHeartbeats 0

open BigOperators Real Nat Topology Rat

theorem mathd_algebra_432
(x : ℝ) :
(x + 3) * (2 * x - 6) = 2 * x^2 - 18 := by
ring_nf
-----
-- Orig Proof
import Mathlib
import Aesop

set_option maxHeartbeats 0

open BigOperators Real Nat Topology Rat

theorem mathd_algebra_170
(S : Finset ℤ)
(h₁ : ∀ (n : ℤ), n ∈ S ↔ abs (n - 2) ≤ 5 + 6 /
→ 10) :
S.card = 11 := by
have h₂ : ∀ (n : ℤ), n ∈ S ↔ -3 ≤ n ∧ n ≤ 7 := by
intro n
rw [h₁]
have h₃ : (6 : ℤ) / 10 = 0 := by norm_num
have h₄ : (5 : ℤ) + 6 / 10 = 5 := by norm_num
rw [h₄]
constructor
-- Prove the forward direction: if |n - 2| ≤
→ 5, then -3 ≤ n ≤ 7
intro h
have h₅ : abs (n - 2) ≤ 5 := by simpa using h
have h₆ : -5 ≤ n - 2 := by
cases' abs_cases (n - 2) with h₆ h₆ <>
→ linarith
have h₇ : n - 2 ≤ 5 := by
cases' abs_cases (n - 2) with h₆ h₆ <>
→ linarith
constructor <> linarith
-- Prove the reverse direction: if -3 ≤ n ≤ 7,
→ then |n - 2| ≤ 5
intro h
have h₈ : -3 ≤ n := h.1
have h₉ : n ≤ 7 := h.2
have h₁₀ : -5 ≤ n - 2 := by linarith
have h₁₁ : n - 2 ≤ 5 := by linarith
have h₁₂ : abs (n - 2) ≤ 5 := by
rw [abs_le]
constructor <> linarith
simpa using h₁₂

have h₁₃ : S = Finset.Icc (-3 : ℤ) 7 := by
apply Finset.ext
intro n
simp only [Finset.mem_Icc]
exact h₁₄ n

have h₁₅ : S.card = 11 := by
rw [h₁₃]
rfl

apply h₁₃

-- Simplified Proof
import Mathlib
import Aesop

set_option maxHeartbeats 0

open BigOperators Real Nat Topology Rat

theorem mathd_algebra_170
(S : Finset ℤ)
(h₁ : ∀ (n : ℤ), n ∈ S ↔ abs (n - 2) ≤ 5 + 6 /
→ 10) :
S.card = 11 := by
have : S = Finset.Icc (-3 : ℤ) 7 := by
ext
simp_all [abs_le]
omega
simp_all
-----
-- Orig Proof
import Mathlib
import Aesop

set_option maxHeartbeats 0

open BigOperators Real Nat Topology Rat

theorem imo_1962_p2
(x : ℝ)
(h₁ : 0 ≤ 3 - x)
(h₂ : 0 ≤ x + 1)
(h₃ : 1 / 2 < Real.sqrt (3 - x) - Real.sqrt (x +
→ 1)) :
-1 ≤ x ∧ x < 1 - Real.sqrt 31 / 8 := by
constructor
· linarith
· by_contra! h
have h₄ : 0 ≤ Real.sqrt (3 - x) :=
Real.sqrt_nonneg (3 - x)
have h₅ : 0 ≤ Real.sqrt (x + 1) :=
Real.sqrt_nonneg (x + 1)
by_cases h₆ : x ≥ 7 / 8
· have h₇ : Real.sqrt (3 - x) ≤ 1 / 2 +
Real.sqrt (x + 1) := by
nlinarith [Real.sq_sqrt (show 0 ≤ x + 1 by
linarith), Real.sq_sqrt (show 0 ≤ 3 - x
by linarith)]
linarith
· have h₈ : x < 7 / 8 := by linarith
have h₉ : (7 / 4 - 2 * x) ^ 2 ≤ x + 1 := by
nlinarith [Real.sq_sqrt (show 0 ≤ 31 by
norm_num), Real.sqrt_nonneg 31,
sq_nonneg (x - 1), sq_nonneg (x - (1 +
→ Real.sqrt 31 / 8))]
have h₁₀ : 7 / 4 - 2 * x ≤ Real.sqrt (x + 1) :=
by
nlinarith [Real.sq_sqrt (show 0 ≤ x + 1 by
linarith), h₉]
nlinarith [Real.sq_sqrt (show 0 ≤ x + 1 by
linarith), Real.sq_sqrt (show 0 ≤ 3 - x
by linarith),
h₉]
-----
-- Orig Proof
import Mathlib
import Aesop

set_option maxHeartbeats 0

open BigOperators Real Nat Topology Rat

theorem mathd_algebra_598
(a b c d : ℝ)
(h₁ : ((4 : ℝ) ^ a) = 5)
(h₂ : ((5 : ℝ) ^ b) = 6)
(h₃ : ((6 : ℝ) ^ c) = 7)
(h₄ : ((7 : ℝ) ^ d) = 8) :
a * b * c * d = 3 / 2 := by
have h₅ : (4 : ℝ) ^ (a * b * c * d) = 8 := by
have h₆ : (4 : ℝ) ^ (a * b * c * d) = (4 : ℝ) ^ (a *
→ b * c * d) := rfl

```

```

have h2 : ((4:ℝ) ^ (a * b * c * d) = ((4:ℝ) ^ a) ^ (b * c * d) := by
  rw [← Real.rpow_mul] <|>
  (try norm_num) <|>
  (try ring_nf) <|>
  (try linarith)
  (try positivity)
have h3 : ((4:ℝ) ^ a) ^ (b * c * d) = (5:ℝ) ^ (b * c * d) := by
  rw [h1]
have h4 : (5:ℝ) ^ (b * c * d) = ((5:ℝ) ^ b) ^ (c * d) := by
  rw [← Real.rpow_mul] <|>
  (try norm_num) <|>
  (try ring_nf) <|>
  (try linarith)
  (try positivity)
have h5 : ((5:ℝ) ^ b) ^ (c * d) = (6:ℝ) ^ (c * d) := by
  rw [h1]
have h6 : (6:ℝ) ^ (c * d) = ((6:ℝ) ^ c) ^ d := by
  rw [← Real.rpow_mul] <|>
  (try norm_num) <|>
  (try ring_nf) <|>
  (try linarith)
  (try positivity)
have h7 : ((6:ℝ) ^ c) ^ d = (7:ℝ) ^ d := by
  rw [h1]
have h8 : (7:ℝ) ^ d = 8 := by
  calc
  (4:ℝ) ^ (a * b * c * d) = ((4:ℝ) ^ a) ^ (b * c * d) := by rw [h1]
  _ = (5:ℝ) ^ (b * c * d) := by rw [h2]
  _ = ((5:ℝ) ^ b) ^ (c * d) := by rw [h3]
  _ = (6:ℝ) ^ (c * d) := by rw [h4]
  _ = ((6:ℝ) ^ c) ^ d := by rw [h5]
  _ = (7:ℝ) ^ d := by rw [h6]
  _ = 8 := by rw [h7]
have h9 : (a * b * c * d) * Real.log 4 = Real.log 8 := by
have h10 : Real.log ((4:ℝ) ^ (a * b * c * d)) = Real.log 8 := by
  rw [h1]
have h11 : Real.log ((4:ℝ) ^ (a * b * c * d)) = (a * b * c * d) * Real.log 4 := by
  rw [Real.log_rpow (by norm_num : (4:ℝ) > 0)] <|>
  ring_nf
  linarith at h1
have h12 : Real.log 8 = 3 * Real.log 2 := by
have h13 : Real.log 8 = Real.log (2 ^ 3) := by
  rw [h1]
have h14 : Real.log (2 ^ 3) = 3 * Real.log 2 := by
  rw [Real.log_pow] <|> norm_num
  rw [h1]
  <|>
  norm_num
have h15 : Real.log 4 = 2 * Real.log 2 := by
have h16 : Real.log 4 = Real.log (2 ^ 2) := by
  rw [h1]
have h17 : Real.log (2 ^ 2) = 2 * Real.log 2 := by
  rw [Real.log_pow] <|> norm_num
  rw [h1]
  <|>
  norm_num
have h18 : (a * b * c * d) * (2 * Real.log 2) = 3 * Real.log 2 := by
  rw [h15]
have h19 : (a * b * c * d) * Real.log 4 = (a * b * c * d) * (2 * Real.log 2) := by
  rw [h18]
  <|> ring_nf
  <|> Real.log 8 := by
  linarith
  <|> = 3 * Real.log 2 := by
  rw [h17]
have h20 : Real.log 2 ≠ 0 := by
have h21 : Real.log 2 > 0 := Real.log_pos (by norm_num)
linarith
have h22 : (a * b * c * d) * 2 = 3 := by
have h23 : (a * b * c * d) * (2 * Real.log 2) = 3 * Real.log 2 := h19
have h24 : Real.log 2 ≠ 0 := h20
have h25 : (a * b * c * d) * 2 = 3 * Real.log 2 := by
  linarith
have h26 : (a * b * c * d) * 2 = 3 := by
  apply mul_left_cancel, h25
  linarith
exact h26
have h27 : a * b * c * d = 3 / 2 := by
have h28 : (a * b * c * d) * 2 = 3 := h26
have h29 : a * b * c * d = 3 / 2 := by
  apply mul_left_cancel, (show (2 : ℝ) ≠ 0 by norm_num)

```



```

-- Case k = 3
have h1 : x = 3
norm_num at h1 ⊢
norm_num at h1
<|> contradiction
-- Case k = 4
have h1 : x = 4
norm_num at h1
<|> contradiction
exact hmain

-- Simplified Proof
import Mathlib
import Aesop

set_option maxHeartbeats 0

open BigOperators Real Nat Topology Rat

theorem mathd_numbertheory_435
  (k : ℕ)
  (h1 : 0 < k)
  (h2 : ∀ n, Nat.gcd (6 * n + k) (6 * n + 3) = 1)
  (h3 : ∀ n, Nat.gcd (6 * n + k) (6 * n + 2) = 1)
  (h4 : ∀ n, Nat.gcd (6 * n + k) (6 * n + 1) = 1) :
  5 ≤ k := by
  by_contra! h
  interval_cases k <|> simp_all
  <|> have h1 : x = 4 <|> simp_all
  -----
-- Orig Proof
import Mathlib
import Aesop

set_option maxHeartbeats 0

open BigOperators Real Nat Topology Rat

theorem amc12b_2020_p6
  (n : ℕ)
  (h1 : 9 ≤ n) :
  ∃ (x : ℕ), (x : ℝ)^2 = (Nat.factorial (n + 2) -
    → Nat.factorial (n + 1)) / n ! := by
  have h1 : ((Nat.factorial (n + 2) - Nat.factorial
    (n + 1)) : ℝ) / (n ! : ℝ) = ((n + 1 : ℝ)
    → )^2 := by
  have h1 : (Nat.factorial (n + 2) : ℝ) = (n + 2
    → : ℝ) * (Nat.factorial (n + 1) : ℝ) := by
  norm_cast
  <|> simp [Nat.factorial_succ, mul_comm]
  <|> ring_nf
  <|> norm_num
  <|> linarith
  have h1 : (Nat.factorial (n + 1) : ℝ) = (n + 1
    → : ℝ) * (n ! : ℝ) := by
  norm_cast
  <|> simp [Nat.factorial_succ, mul_comm]
  <|> ring_nf
  <|> norm_num
  <|> linarith
calc
  ((Nat.factorial (n + 2) - Nat.factorial (n +
    → 1) : ℝ) / (n ! : ℝ)) =
  (((n + 2 : ℝ) * (Nat.factorial (n + 1) : ℝ)
    → ) - (Nat.factorial (n + 1) : ℝ)) / (n ! :
    → ℝ)) := by
  rw [h1]
  <|> ring_nf
  _ = (((n + 2 : ℝ) - 1) * (Nat.factorial (n +
    → 1) : ℝ) / (n ! : ℝ)) := by
  ring_nf
  <|> field_simp
  <|> ring_nf
  _ = ((n + 1 : ℝ) * (Nat.factorial (n + 1)
    → : ℝ) / (n ! : ℝ)) := by
  ring_nf
  <|> field_simp
  <|> ring_nf
  _ = ((n + 1 : ℝ) * ((n + 1 : ℝ) * (n ! : ℝ)
    → )) / (n ! : ℝ) := by
  rw [h1]
  <|> ring_nf
  _ = ((n + 1 : ℝ) * (n + 1 : ℝ)) := by
  have h1 : (n ! : ℝ) ≠ 0 := by
  norm_cast
  <|> apply Nat.cast_ne_zero.mpr
  <|> apply Nat.factorial_ne_zero
  field_simp [h1]
  <|> ring_nf
  <|> field_simp [h1]
  <|> ring_nf
  _ = ((n + 1 : ℝ) ^ 2) := by
  ring_nf

  have h1 : ∃ (x : ℕ), (x : ℝ)^2 = (Nat.factorial
    (n + 2) - Nat.factorial (n + 1)) / n ! :=
  by
  use n + 1
  have h1 : ((n + 1 : ℕ) : ℝ) ^ 2 = ((n + 1 : ℝ)
    → )^2 := by
  norm_cast
  have h1 : ((Nat.factorial (n + 2) -
    → Nat.factorial (n + 1)) : ℝ) / (n ! : ℝ) =
    → (((n + 1 : ℕ) ^ 2) : ℝ) := by
  have h1 : ((n + 1 : ℕ) : ℝ) ^ 2 =
    → (Nat.factorial (n + 2) - Nat.factorial (n
    → + 1)) / n ! := by
  calc
    ((n + 1 : ℕ) : ℝ) ^ 2 = ((n + 1 : ℝ) ^ 2)
    _ = by norm_cast
    _ = ((Nat.factorial (n + 2) -
    → Nat.factorial (n + 1)) : ℝ) / (n ! : ℝ) :=
    by
  rw [h1]
  <|> norm_num
  _ = (Nat.factorial (n + 2) - Nat.factorial
    (n + 1)) / n ! := by

```



```

norm_cast
<|> field_simp [Nat.cast_ne_zero]
<|> ring_nf
<|> norm_num
<|> simp_all [Nat.factorial_succ]
<|> linarith
exact_mod_cast h

exact h
-- Simplified Proof
import Mathlib
import Aesop

set_option maxHeartbeats 0

open BigOperators Real Nat Topology Rat

theorem amc12b_2020_p6
(n : ℕ)
(h₁ : 9 ≤ n) :
  ∃ (x : ℝ), (x : ℝ)^2 = (Nat.factorial (n + 2) -
    → Nat.factorial (n + 1)) / n! := by
  use n + 1
  field_simp [Nat.factorial]
  ring
  -----
  -- Orig Proof
import Mathlib
import Aesop

set_option maxHeartbeats 0

open BigOperators Real Nat Topology Rat

theorem algebra_others_exirrpowirrnat :
  ∃ a b, Irrational a ∧ Irrational b ∧ - Irrational
    → (a^b) := by
  have h_main : ∃ (a b : ℝ), Irrational a ∧
    → Irrational b ∧ -Irrational (a ^ b) := by
  by_cases h : Irrational ((Real.sqrt 2 : ℝ) ^
    → (Real.sqrt 2 : ℝ))
  · -- Case 2: (√2)^√2 is irrational
    have h₁ : Irrational ((Real.sqrt 2 : ℝ) ^
      → (Real.sqrt 2 : ℝ)) := h
    have h₂ : Irrational (Real.sqrt 2 : ℝ) := by
      apply Nat.Prime.irrational_sqrt
      <|> norm_num
    have h₃ : -Irrational (((Real.sqrt 2 : ℝ) ^
      → (Real.sqrt 2 : ℝ)) ^ (Real.sqrt 2 : ℝ)) :=
      by
    have h₄ : ((Real.sqrt 2 : ℝ) ^ (Real.sqrt 2
      → : ℝ)) ^ (Real.sqrt 2 : ℝ) = (2 : ℝ) := by
    have h₅ : 0 < (Real.sqrt 2 : ℝ) :=
      → Real.sqrt_pos.mpr (by norm_num)
    have h₆ : ((Real.sqrt 2 : ℝ) ^ (Real.sqrt
      → 2 : ℝ)) ^ (Real.sqrt 2 : ℝ) = (Real.sqrt
      → 2 : ℝ) ^ ((Real.sqrt 2 : ℝ) * (Real.sqrt
      → 2 : ℝ)) := by
    rw [← Real.rpow_mul (le_of_lt h₅)]
    <|> ring_nf
    rw [h₄]
    have h₇ : (Real.sqrt 2 : ℝ) * (Real.sqrt
      → 2 : ℝ) = (2 : ℝ) := by
    nlinarith [Real.sq_sqrt (show 0 ≤ (2 : ℝ)
      → ) by norm_num]]
    rw [h₄]
    have h₈ : (Real.sqrt 2 : ℝ) ^ (2 : ℝ) =
      → (2 : ℝ) := by
    have h₉ : (Real.sqrt 2 : ℝ) ^ (2 : ℝ) =
      → (Real.sqrt 2 : ℝ) ^ 2 := by
    norm_cast
    rw [h₄]
    nlinarith [Real.sq_sqrt (show 0 ≤ (2 : ℝ)
      → ) by norm_num]]
    rw [h₄]
    intro h
    exact h.2, by norm_num
  refine' (Real.sqrt 2 : ℝ) ^ (Real.sqrt 2 : ℝ)
  → ), (Real.sqrt 2 : ℝ), h, h₂, h₃)
  · -- Case 1: (√2)^√2 is rational
    have h₁ : -Irrational ((Real.sqrt 2 : ℝ) ^
      → (Real.sqrt 2 : ℝ)) := h
    have h₂ : Irrational (Real.sqrt 2 : ℝ) := by
      apply Nat.Prime.irrational_sqrt
      <|> norm_num
    have h₃ : -Irrational ((Real.sqrt 2 : ℝ) ^
      → (Real.sqrt 2 : ℝ)) := h
    refine' (Real.sqrt 2 : ℝ), (Real.sqrt 2 : ℝ
      → ), h₂, h₃, h₃)

obtain (a, b, ha, hb, hab) := h_main
refine' (a, b, ha, hb, _)
exact hab
-- Simplified Proof
import Mathlib
import Aesop

set_option maxHeartbeats 0

open BigOperators Real Nat Topology Rat

theorem algebra_others_exirrpowirrnat :
  ∃ a b, Irrational a ∧ Irrational b ∧ - Irrational
    → (a^b) := by
  by_cases h : Irrational (Real.sqrt 2 ^ Real.sqrt
    → 2)
  · use Real.sqrt 2 ^ Real.sqrt 2, Real.sqrt 2
    exact h, irrational_sqrt_two, by simp [←
      → Real.rpow_mul]
  · use Real.sqrt 2, Real.sqrt 2
    exact (irrational_sqrt_two,
      → irrational_sqrt_two, h)
  -----
  -- Orig Proof

```

```

import Mathlib
import Aesop

set_option maxHeartbeats 0

open BigOperators Real Nat Topology Rat

theorem mathd_algebra_427
(x y z : ℝ)
(h₁ : 3 * x + y = 17)
(h₂ : 5 * y + z = 14)
(h₃ : 3 * x + 5 * z = 41) :
  x + y + z = 12 := by
  have h_sum : x + y + z = 12 := by
    have h₄ : (3 * x + y) + (5 * y + z) + (3 * x +
      → 5 * z) = 17 + 14 + 41 := by
      linarith
    have h₅ : 6 * (x + y + z) = 72 := by
      linarith
    have h₆ : x + y + z = 12 := by
      linarith
    exact h₆
  -----
  -- Simplified Proof
import Mathlib
import Aesop

set_option maxHeartbeats 0

open BigOperators Real Nat Topology Rat

theorem mathd_algebra_427
(x y z : ℝ)
(h₁ : 3 * x + y = 17)
(h₂ : 5 * y + z = 14)
(h₃ : 3 * x + 5 * z = 41) :
  x + y + z = 12 := by
  linarith
  -----
  -- Orig Proof
import Mathlib
import Aesop

set_option maxHeartbeats 0

open BigOperators Real Nat Topology Rat

theorem mathd_algebra_76
(f : ℤ → ℤ)
(f : ℤ → ℤ, Odd n → f n = n^2)
(h₁ : ∃ n, Even n → f n = n^2 - 4*n - 1) :
  f 4 = -1 := by
  have h_main : f 4 = -1 := by
    have h₂ : Even (4 : ℤ) := by
      -- Prove that 4 is even
      use 2
    <|> norm_num
    -- Use the definition of f for even numbers
    have h₃ : f 4 = (4 : ℤ)^2 - 4*(4 : ℤ) - 1 := by
      apply h
    exact h
    -- Simplify the expression
    rw [h₃]
    norm_num
  exact h_main
  -----
  -- Simplified Proof
import Mathlib
import Aesop

set_option maxHeartbeats 0

open BigOperators Real Nat Topology Rat

theorem mathd_algebra_76
(f : ℤ → ℤ)
(h₁ : ∃ n, Odd n → f n = n^2)
(h₂ : ∃ n, Even n → f n = n^2 - 4*n - 1) :
  f 4 = -1 := by
  apply h
  decide
  -----
  -- Orig Proof
import Mathlib
import Aesop

set_option maxHeartbeats 0

open BigOperators Real Nat Topology Rat

theorem mathd_numbertheory_99
(n : ℕ)
(h₁ : (2 * n) % 47 = 15) :
  n % 47 = 31 := by
  have h₂ : n % 47 = 31 := by
    have h₃ : (2 * n) % 47 = 15 := h₁
    -- We know that 2 * 24 = 1 mod 47, so we can
    -- multiply both sides by 24 to get n = 24 *
    -- 15 mod 47
    have h₄ : n % 47 = 31 := by
      -- Use the fact that 2 * n = 15 mod 47 to
      -- find n mod 47
      have h₅ : (2 * n) % 47 = 15 := h₁
      -- We can use the 'omega' tactic to solve the
      -- linear congruence
      have h₆ : n % 47 = 31 := by
        -- Use the fact that 2 * n = 15 mod 47 to
        -- find n mod 47
        omega
      exact h₆
    exact h₃
  -----
  -- Simplified Proof
import Mathlib
import Aesop

set_option maxHeartbeats 0

```

```

open BigOperators Real Nat Topology Rat

theorem mathd_numbertheory_99
(n : ℕ)
(h₁ : (2 * n) % 47 = 15) :
  n % 47 = 31 := by
  omega
  -----
  -- Orig Proof
import Mathlib
import Aesop

set_option maxHeartbeats 0

open BigOperators Real Nat Topology Rat

theorem algebra_9onxpyyzleqsum2onxpy
(x y z : ℝ)
(h₁ : 0 < x ∧ 0 < y ∧ 0 < z) :
  9 / (x + y + z) ≤ 2 / (x + y) + 2 / (y + z) + 2
    → / (z + x) := by
  have h_main : 2 / (x + y) + 2 / (y + z) + 2 / (z +
    → x) ≥ 9 / (x + y + z) := by
    have h₂ : 0 < x := by linarith
    have h₃ : 0 < y := by linarith
    have h₄ : 0 < z := by linarith
    have h₅ : 0 < x * y := mul_pos h₂ h₃
    have h₆ : 0 < y * z := mul_pos h₃ h₄
    have h₇ : 0 < z * x := mul_pos h₄ h₂
    field_simp
    rw [div_le_div_iff (by positivity) (by
      → positivity)]
    nlinarith [sq_nonneg (x - y), sq_nonneg (y -
      → z), sq_nonneg (z - x),
      sq_nonneg (x - y + z), sq_nonneg (y - z +
      → x), sq_nonneg (z - x + y)]
    linarith
  -----
  -- Simplified Proof
import Mathlib
import Aesop

set_option maxHeartbeats 0

open BigOperators Real Nat Topology Rat

theorem algebra_9onxpyyzleqsum2onxpy
(x y z : ℝ)
(h₁ : 0 < x ∧ 0 < y ∧ 0 < z) :
  9 / (x + y + z) ≤ 2 / (x + y) + 2 / (y + z) + 2
    → / (z + x) := by
  rcases h₁ with (h₂, h₃, h₄)
  field_simp
  rw [div_le_div_iff]
  nlinarith [sq_nonneg (x - y), sq_nonneg (y - z),
    → sq_nonneg (z - x)]
  positivity
  positivity
  -----
  -- Orig Proof
import Mathlib
import Aesop

set_option maxHeartbeats 0

open BigOperators Real Nat Topology Rat

theorem algebra_absapbonipabsapleqsumabsaconipabs
(a b : ℝ) :
  abs (a + b) / (1 + abs (a + b)) ≤ abs a / (1 +
    → abs a) + abs b / (1 + abs b) := by
  have h_main : abs (a + b) / (1 + abs (a + b)) ≤
    → (abs a + abs b) / (1 + abs a + abs b) :=
    by
  have h₁ : 0 ≤ abs a := abs_nonneg a
  have h₂ : 0 ≤ abs b := abs_nonneg b
  have h₃ : 0 ≤ abs (a + b) := abs_nonneg (a + b)
  have h₄ : abs (a + b) ≤ abs a + abs b :=
    → abs.add a b
  have h₅ : 0 ≤ 1 + abs a + abs b := by positivity
  have h₆ : 0 ≤ 1 + abs (a + b) := by positivity
  -- Use the fact that the function f(x) = x / (1
    → + x) is increasing for x ≥ 0
  have h₇ : abs (a + b) / (1 + abs (a + b)) ≤
    → (abs a + abs b) / (1 + abs a + abs b) :=
    by
  -- Use the division inequality to compare the
    → two fractions
  rw [div_le_div_iff] <|>
  nlinarith [mul_nonneg h₁ h₂, mul_nonneg h₁
    → h₃, mul_nonneg h₂ h₃,
    mul_nonneg (abs_nonneg (a + b)) h₁,
    → mul_nonneg (abs_nonneg (a + b)) h₃]
  exact h₇
  have h_key : (abs a + abs b) / (1 + abs a + abs
    → b) ≤ abs a / (1 + abs a) + abs b / (1 +
    → abs b) := by
  have h₁ : 0 ≤ abs a := abs_nonneg a
  have h₂ : 0 ≤ abs b := abs_nonneg b
  have h₃ : 0 ≤ 1 + abs a := by positivity
  have h₄ : 0 ≤ 1 + abs b := by positivity
  have h₅ : 0 ≤ 1 + abs a + abs b := by positivity
  have h₆ : 0 ≤ 1 + abs a + abs b := by positivity
  have h₇ : 0 ≤ (1 + abs a) * (1 + abs b) := by
    → positivity
  have h₈ : 0 ≤ (1 + abs a) * (1 + abs b) * (1 +
    → abs a + abs b) := by positivity
  field_simp
  rw [div_le_div_iff (by positivity) (by
    → positivity)]
  nlinarith [sq_nonneg (abs a - abs b),
    → sq_nonneg (abs a - 0), sq_nonneg (abs b -
    → 0),
    mul_nonneg h₁ h₂, mul_nonneg h₁ (sq_nonneg
    → (abs a - abs b)),

```

```

mul_nnonneg h, (sq_nnonneg (abs a - abs b))]

have h_final : abs (a + b) / (1 + abs (a + b)) ≤
  → abs a / (1 + abs a) + abs b / (1 + abs b)
  := by
  have h : abs (a + b) / (1 + abs (a + b)) ≤
    → (abs a + abs b) / (1 + abs a + abs b) :=
    h_main
  have h₁ : (abs a + abs b) / (1 + abs a + abs b)
    ≤ abs a / (1 + abs a) + abs b / (1 + abs
    → b) := h_key
  linarith
exact h_final

-- Simplified Proof
import Mathlib
import Aesop

set_option maxHeartbeats 0

open BigOperators Real Nat Topology Rat

theorem algebra_absapbnlpabsapbqsumabsapbnlpabsa
(a b : ℝ) :
abs (a + b) / (1 + abs (a + b)) ≤ abs a / (1 +
  → abs a) + abs b / (1 + abs b) := by
  field_simp
  rw [div_le_div_iff] <>
  nlinarith [abs_add a b, abs_nnonneg a, abs_nnonneg
    → b, abs_nnonneg (a + b), mul_nnonneg
    → (abs_nnonneg a) (abs_nnonneg b)]

-----
-- Orig Proof
import Mathlib
import Aesop

set_option maxHeartbeats 0

open BigOperators Real Nat Topology Rat

theorem mathd_algebra_153
(n : ℝ)
(h₁ : n = 1 / 3) :
Int.floor (10 * n) + Int.floor (100 * n) +
  → Int.floor (1000 * n) + Int.floor (10000 *
  → n) = 3702 := by
  have h₁ : Int.floor (10 * n) = 3 := by
  rw [h₁]
  have h₂ : Int.floor ((10 : ℝ) * (1 / 3 : ℝ)) =
    → 3 := by
  norm_num [Int.floor_eq_iff]
  <>
  (try norm_num) <>
  (try linarith)
exact h₁

have h₁ : Int.floor (100 * n) = 33 := by
  rw [h₁]
  have h₂ : Int.floor ((100 : ℝ) * (1 / 3 : ℝ)) =
    → 33 := by
  norm_num [Int.floor_eq_iff]
  <>
  (try norm_num) <>
  (try linarith)
exact h₁

have h₁ : Int.floor (1000 * n) = 333 := by
  rw [h₁]
  have h₂ : Int.floor ((1000 : ℝ) * (1 / 3 : ℝ))
    → = 333 := by
  norm_num [Int.floor_eq_iff]
  <>
  (try norm_num) <>
  (try linarith)
exact h₁

have h₁ : Int.floor (10000 * n) = 3333 := by
  rw [h₁]
  have h₂ : Int.floor ((10000 : ℝ) * (1 / 3 : ℝ
    → )) = 3333 := by
  norm_num [Int.floor_eq_iff]
  <>
  (try norm_num) <>
  (try linarith)
exact h₁

have h₁ : Int.floor (10 * n) + Int.floor (100 *
  → n) + Int.floor (1000 * n) + Int.floor
  → (10000 * n) = 3702 := by
  rw [h₁, h₂, h₃, h₄]
  <> norm_num
exact h₁

-- Simplified Proof
import Mathlib
import Aesop

set_option maxHeartbeats 0

open BigOperators Real Nat Topology Rat

theorem mathd_algebra_153
(n : ℝ)
(h₁ : n = 1 / 3) :
Int.floor (10 * n) + Int.floor (100 * n) +
  → Int.floor (1000 * n) + Int.floor (10000 *
  → n) = 3702 := by
  simp_all
  norm_num
-----
-- Orig Proof
import Mathlib
import Aesop

set_option maxHeartbeats 0

open BigOperators Real Nat Topology Rat

```

```

theorem algebra_sqineq_unitcircatpbmbt1
(a b : ℝ)
(h₁ : a² + b² = 1) :
a * b + (a - b) ≤ 1 := by
  have h_main : a * b + (a - b) ≤ 1 := by
  nlinarith [sq_nnonneg (a - 1), sq_nnonneg (b +
    → 1), sq_nnonneg (a + b - 1),
    sq_nnonneg (a - b), sq_nnonneg (a + 1),
    → sq_nnonneg (b - 1),
    sq_nnonneg (a + b + 1)]
  exact h_main

-- Simplified Proof
import Mathlib
import Aesop

set_option maxHeartbeats 0

open BigOperators Real Nat Topology Rat

theorem algebra_sqineq_unitcircatpbmbt1
(a b : ℝ)
(h₁ : a² + b² = 1) :
a * b + (a - b) ≤ 1 := by
  nlinarith [sq_nnonneg (a - b)]

-----
-- Orig Proof
import Mathlib
import Aesop

set_option maxHeartbeats 0

open BigOperators Real Nat Topology Rat

theorem mathd_algebra_329
(x y : ℝ)
(h₁ : 3 * y = x)
(h₂ : 2 * x + 5 * y = 11) :
x + y = 4 := by
  have h₁ : y = 1 := by
  have h₂ : 2 * x + 5 * y = 11 := h₁
  have h₃ : x = 3 * y := by linarith
  rw [h₃] at h₁
  ring_nf at h₁
  linarith

  have h₁ : x = 3 := by
  have h₂ : x = 3 * y := by linarith
  rw [h₂]
  rw [h₁]
  <> norm_num

  have h₁ : x + y = 4 := by
  rw [h₁, h₂]
  <> norm_num
exact h₁

-- Simplified Proof
import Mathlib
import Aesop

set_option maxHeartbeats 0

open BigOperators Real Nat Topology Rat

theorem mathd_algebra_329
(x y : ℝ)
(h₁ : 3 * y = x)
(h₂ : 2 * x + 5 * y = 11) :
x + y = 4 := by
  nlinarith

-----
-- Orig Proof
import Mathlib
import Aesop

set_option maxHeartbeats 0

open BigOperators Real Nat Topology Rat

theorem induction_pprime_pdvdpowpma
(p a : ℕ)
(h₁ : 0 < a)
(h₂ : Nat.Prime p) :
p ∣ (aᵖ - a) := by
  have h₁ : aᵖ ≥ a := by
  have h₂ : aᵖ ≥ a := by
  apply Nat.pow_le_pow_of_le_right
  linarith
  have h₁ : p ≥ 1 := Nat.Prime.one_lt h₁
  linarith
  have h₂ : aᵖ - 1 = a := by simp
  linarith

  have h₁ : (a : ZMod p)ᵖ = (a : ZMod p) := by
  haveI : Fact p.Prime := h₁
  have h₂ : (a : ZMod p)ᵖ = (a : ZMod p) := by
  -- Use the property of finite fields that xᵖ = x
  → = x for any element x
  have h₃ : (a : ZMod p)ᵖ = (a : ZMod p) :=
  → by
  -- Apply Fermat's Little Theorem
  have h₄ : (a : ZMod p)ᵖ = (a : ZMod p)
  → = by
  -- Use the fact that in ZMod p, xᵖ = x
  have h₅ : (a : ZMod p)ᵖ = (a : ZMod
  → p) := by
  -- Use the property of finite fields
  rw [ZMod.pow_card]
  exact h₅
  exact h₃
  exact h₄
  exact h₁

  have h₁ : (aᵖ : ZMod p) = (a : ZMod p) := by
  have h₂ : (a : ZMod p)ᵖ = (a : ZMod p) := h₁
  have h₃ : (aᵖ : ZMod p) = (a : ZMod p) := by

```

```

-- Use the fact that the coercion from ℕ to
  → ZMod p respects powers
calc
(aᵖ : ZMod p) = ((a : ZMod p)ᵖ : ZMod p) := by
  norm_cast
  <> simp [ZMod.nat_cast_self]
  <> rfl
  = (a : ZMod p) := by rw [h₁]
exact h₁

have h₁ : (aᵖ : ZMod p) - (a : ZMod p) = 0 := by
  rw [h₁]
  <> simp [sub_self]
  <>
  (try simp_all [ZMod.nat_cast_self])
  <>
  (try ring_nf at *)
  <>
  (try norm_num at *)
  <>
  (try omega)

have h₁ : ((aᵖ - a : ℕ) : ZMod p) = 0 := by
  have h₂ : ((aᵖ - a : ℕ) : ZMod p) = (aᵖ -
    → : ZMod p) - (a : ZMod p) := by
  have h₃ : aᵖ ≥ a := h₁
  have h₄ : (aᵖ - a : ℕ) = aᵖ - a := by
  have h₅ : aᵖ ≥ a := h₁
  omega
  rw [h₁]
  norm_cast
  <>
  simp [ZMod.nat_cast_self, Nat.cast_sub (by
    → omega : a ≤ aᵖ)]
  <>
  ring_nf
  <>
  simp_all [ZMod.nat_cast_self]
  <>
  norm_num
  <>
  omega
  rw [h₁]
  exact h₁

have h₁ : p ∣ (aᵖ - a) := by
  have h₂ : ((aᵖ - a : ℕ) : ZMod p) = 0 := h₁
  have h₃ : (p : ℕ) ∣ (aᵖ - a : ℕ) := by
  -- Use the property of ZMod to deduce that p
  → divides aᵖ - a
  have h₄ : (aᵖ - a : ℕ) = 0 [MOD p] := by
  rw [-ZMod.eq_iff_modEq_nat]
  simp [h₁] using h₁
  -- Convert the congruence to a divisibility
  → statement
  rw [Nat.modEq_zero_iff_dvd] at h₁
  exact h₁
  exact h₂
exact h₁

-- Simplified Proof
import Mathlib
import Aesop

set_option maxHeartbeats 0

open BigOperators Real Nat Topology Rat

theorem induction_pprime_pdvdpowpma
(p a : ℕ)
(h₁ : 0 < a)
(h₂ : Nat.Prime p) :
p ∣ (aᵖ - a) := by
  have : Fact p.Prime := h₂
  have h₁ : aᵖ ≥ a := by
  apply Nat.le_self_pow
  linarith [h₁.pos]
  have h₂ : (aᵖ - a : ℕ) = 0 [MOD p] := by
  rw [-ZMod.eq_iff_modEq_nat]
  simp [ZMod.pow_card]
  <> simp [h₁]
  rw [Nat.modEq_zero_iff_dvd] at h₁
  exact h₁

-----
-- Orig Proof
import Mathlib
import Aesop

set_option maxHeartbeats 0

open BigOperators Real Nat Topology Rat

theorem amc12a_2021_p18
(f : ℚ → ℝ)
(h₁ : ∀ x > 0, y > 0, f (x + y) = f x + f y)
(h₂ : ∀ p, Nat.Prime p → f p = p) :
f (25 / 11) < 0 := by
  have h₁ : f (5 : ℚ) = (5 : ℝ) := by
  have h₂ : f (5 : ℚ) = (5 : ℝ) := by
  have h₃ : Nat.Prime 5 := by decide
  have h₄ : f (5 : ℚ) = (5 : ℝ) := by
  simp using h₁ h₂
  exact h₃
  exact h₁

  have h₁ : f (25 : ℚ) = (10 : ℝ) := by
  have h₂ : f (25 : ℚ) = f ((5 : ℚ) * (5 : ℚ)) :=
    → by norm_num
  rw [h₁]
  have h₃ : f ((5 : ℚ) * (5 : ℚ)) = f (5 : ℚ) +
    → f (5 : ℚ) := by
  apply h₁
  <> norm_num
  <> norm_num
  rw [h₁]
  rw [h₁]

```

```

<> norm_num
<> linarith

have h₁ : f (11 : q) = (11 : s) := by
have h₂ : Nat.Prime 11 := by decide
have h₃ : f (11 : q) = (11 : s) := by
  simp using h₁ 11 h₁
exact h₃

have h₄ : f (25 / 11 : q) = (-1 : s) := by
have h₅ : f (25 : q) = f ((25 / 11 : q) * (11 : s)) (11 : s) := by
  → : q) := by
  norm_num [div_eq_mul_inv]
<> field_simp
<> ring_nf
<> norm_num
rw [h₅] at h₄
have h₆ : f ((25 / 11 : q) * (11 : s)) = f (25 : q) / 11 : q + f (11 : s) := by
  apply h₄
<> norm_num
<> norm_num
rw [h₆] at h₄
rw [h₆] at h₄
norm_num at h₄
<> linarith

have h₄ : f (25 / 11) < 0 := by
have h₅ : f (25 / 11 : q) = (-1 : s) := h₄
have h₆ : f (25 / 11 : q) < 0 := by
  rw [h₅]
  norm_num
exact h₆

exact h₄

-- Simplified Proof
import Mathlib
import Aesop

set_option maxHeartbeats 0

open BigOperators Real Nat Topology Rat

theorem amc12a_2021_p18
  (f : q → s)
  (h₁ : x > 0, y > 0, f (x * y) = f x + f y)
  (h₂ : p, Nat.Prime p → f p = p) :
  f (25 / 11) < 0 := by
  norm_num
  have h₁ := h₁ 5
  have h₂ := h₁ 11
  have h₃ := h₁ 5 (by norm_num) 5 (by norm_num)
  have h₄ := h₁ (25 / 11) (by norm_num) 11 (by
    → norm_num)
  norm_num at h₁ h₂ h₃ h₄
  linarith
  -----
  -- Orig Proof
  import Mathlib
  import Aesop

  set_option maxHeartbeats 0

  open BigOperators Real Nat Topology Rat

  theorem amc12a_2021_p9 :
    n k ∈ Finset.range 7, (2^(2*k) + 3^(2*k)) = 3^128
    → - 2^128 := by
    have h : n k ∈ Finset.range 7, (2^(2*k) +
      → 3^(2*k)) = 3^128 - 2^128 := by
      rfl
    apply h

  -- Simplified Proof
  import Mathlib
  import Aesop

  set_option maxHeartbeats 0

  open BigOperators Real Nat Topology Rat

  theorem amc12a_2021_p9 :
    n k ∈ Finset.range 7, (2^(2*k) + 3^(2*k)) = 3^128
    → - 2^128 := by
    rfl
  -----
  -- Orig Proof
  import Mathlib
  import Aesop

  set_option maxHeartbeats 0

  open BigOperators Real Nat Topology Rat

  theorem mathd_numbertheory_229 :
    (5^30) % 7 = 1 := by
    have h : (5^30) % 7 = 1 := by
      norm_num
    exact h

  -- Simplified Proof
  import Mathlib
  import Aesop

  set_option maxHeartbeats 0

  open BigOperators Real Nat Topology Rat

  theorem mathd_numbertheory_229 :
    (5^30) % 7 = 1 := by
    rfl
  -----
  -- Orig Proof
  import Mathlib
  import Aesop

  set_option maxHeartbeats 0

  open BigOperators Real Nat Topology Rat

theorem mathd_numbertheory_100
  (n : ℕ)
  (h₁ : 0 < n)
  (h₂ : Nat.gcd n 40 = 10)
  (h₃ : Nat.lcm n 40 = 280) :
  n = 70 := by
  have h₄ : n * 40 = 2800 := by
    have h₅ : Nat.gcd n 40 * Nat.lcm n 40 = n * 40
    → := by
      rw [Nat.gcd_mul_lcm]
      rw [h₁, h₂] at h₅
      norm_num at h₅
      <> linarith
  have h₄ : n = 70 := by
  have h₅ : n * 40 = 70 * 40 := by
    norm_num at h₄
  <> linarith
  have h₆ : n = 70 := by
  apply mul_left_cancel₃ (show (40 : ℕ) ≠ 0 by
    linarith)
  exact h₄
  exact h₄

-- Simplified Proof
import Mathlib
import Aesop

set_option maxHeartbeats 0

open BigOperators Real Nat Topology Rat

theorem mathd_numbertheory_100
  (n : ℕ)
  (h₁ : 0 < n)
  (h₂ : Nat.gcd n 40 = 10)
  (h₃ : Nat.lcm n 40 = 280) :
  n = 70 := by
  have := Nat.gcd_mul_lcm n 40
  simp_all
  omega
  -----
  -- Orig Proof
  import Mathlib
  import Aesop

  set_option maxHeartbeats 0

  open BigOperators Real Nat Topology Rat

  theorem aime_1984_p1
    (u : ℕ → q)
    (h₁ : ∀ n, u (n + 1) = u n + 1)
    (h₂ : x k ∈ Finset.range 98, u k.succ = 137) :
    x k ∈ Finset.range 49, u (2 * k.succ) = 93 := by
  have h₁ : v (n : ℕ), u n = u 0 + n := by
    intro n
    have h₁ : v (n : ℕ), u n = u 0 + n := by
      intro n
      induction n with
      | zero =>
        simp
      | succ n ih =>
        have h₁ := h₁ n
        rw [ih] at h₁
        simp [h₁, add_assoc]
        <> ring_nf at *
        <> norm_num at *
        <> linarith
      exact h₁ n
  have h₁ : 98 * u 0 + 4851 = 137 := by
  have h₂ : x k ∈ Finset.range 98, u (k.succ) =
    → 137 := h₁
  have h₃ : x k ∈ Finset.range 98, u (k.succ) = x
    → k ∈ Finset.range 98, (u 0 + (k.succ : q
    → )) := by
    apply Finset.sum_congr rfl
    intro k
  rw [h₁ (k.succ)]
  <> simp [Nat.cast_add, Nat.cast_one]
  <> ring_nf
  <> norm_num
  rw [h₁] at h₁
  have h₁ : x k ∈ Finset.range 98, (u 0 +
    → (k.succ : q)) = 98 * u 0 + 4851 := by
    → Calculate the sum of (u 0 + (k + 1)) for k
    → from 0 to 97
  have h₁ : x k ∈ Finset.range 98, (u 0 +
    → (k.succ : q)) = x k ∈ Finset.range 98,
    → (u 0 : q) + x k ∈ Finset.range 98,
    → (k.succ : q) := by
    rw [Finset.sum_add_distrib]
  rw [h₁]
  → Calculate the sum of u 0
  have h₁ : x k ∈ Finset.range 98, (u 0 : q) =
    → 98 * u 0 := by
    simp [Finset.sum_const, Finset.card_range]
    <> ring_nf
  rw [h₁]
  → Calculate the sum of (k + 1) for k from 0
  → to 97
  have h₁ : x k ∈ Finset.range 98, (k.succ : q
    → ) = 4851 := by
    → The sum of the first 98 natural numbers
    → is 98 * 99 / 2 = 4851
  norm_num [Finset.sum_range_succ,
    → Finset.sum_range_succ,
    → Finset.sum_range_succ]
  <>
  rfl
  rw [h₁]
  <> ring_nf
  rw [h₁] at h₁
  norm_num at h₁

```

```

apply Complex.ext <> simp [h₁, h₂,
  ↳ Complex.ext_iff, pow_two]
<> norm_num <>
(try ring_nf) <>
(try norm_num) <>
(try linarith)
<>
(try
{
  simp_all [Complex.ext_iff, pow_two]
  <> norm_num <>
  (try ring_nf at h₁) <>
  (try norm_num at *) <>
  (try linarith)
})
)

exact h₁

-- Simplified Proof
import Mathlib
import Aesop

set_option maxHeartbeats 0

open BigOperators Real Nat Topology Rat

theorem mathd_algebra_313
  (v i z : ℂ)
  (h₁ : v = i * z)
  (h₂ : v = 1 + Complex.I)
  (h₃ : z = 2 - Complex.I) :
  i = 1/5 + 3/5 * Complex.I := by
  simp_all [Complex.ext_iff]
  constructor <> nlinarith

-- Orig Proof
import Mathlib
import Aesop

set_option maxHeartbeats 0

open BigOperators Real Nat Topology Rat

theorem amc12a_2002_p6
  (n : ℕ)
  (h₁ : 0 < n) :
  ∃ m, (m > n ∧ ∃ p, m * p ≤ m + p) := by
  have h_main : ∃ m, (m > n ∧ ∃ p, m * p ≤ m + p) :=
  by
  use n + 1
  constructor
  . -- Prove that n + 1 > n
    omega
  . -- Find a p such that (n + 1) * p ≤ (n + 1) + p
    use 0
    <> simp [mul_zero, add_zero]
    <> nlinarith

exact h_main

-- Simplified Proof
import Mathlib
import Aesop

set_option maxHeartbeats 0

open BigOperators Real Nat Topology Rat

theorem amc12a_2002_p6
  (n : ℕ)
  (h₁ : 0 < n) :
  ∃ m, (m > n ∧ ∃ p, m * p ≤ m + p) := by
  use n + 1
  constructor
  omega
  use 0
  simp
  -----
  -- Orig Proof
  import Mathlib
  import Aesop

  set_option maxHeartbeats 0

  open BigOperators Real Nat Topology Rat

  theorem mathd_algebra_129
    (a : ℝ)
    (h₁ : a ≠ 0)
    (h₂ : 8⁻¹ / 4⁻¹ - a⁻¹ = 1) :
    a = -2 := by
  have h_main : a = -2 := by
  have h₁ : (8 : ℝ)⁻¹ / (4 : ℝ)⁻¹ - a⁻¹ = 1 / 2 := by
  norm_num
  rw [h₁] at h₁
  have h₂ : (1 / 2 : ℝ) - a⁻¹ = 1 := by simpa
  have h₃ : a⁻¹ = -1 / 2 := by
  -- Solve for a⁻¹ using linear arithmetic
  linarith
  have h₄ : a = -2 := by
  -- Take reciprocals to find a
  have h₅ : a ≠ 0 := h₁
  have h₆ : a⁻¹ = -1 / 2 := h₃
  have h₇ : a = -2 := by
  -- Use the fact that a⁻¹ = -1/2 to find a
  have h₈ : a = -2 := by
  -- Take reciprocals and solve for a
  have h₉ : a ≠ 0 := h₅
  field_simp [h₉] at h₆
  nlinarith
  exact h₁
  exact h₂
  exact h₃
  exact h_main

-- Simplified Proof
import Mathlib
import Aesop

```

```

set_option maxHeartbeats 0

open BigOperators Real Nat Topology Rat

theorem mathd_algebra_129
  (a : ℝ)
  (h₁ : a ≠ 0)
  (h₂ : 8⁻¹ / 4⁻¹ - a⁻¹ = 1) :
  a = -2 := by
  field_simp at h₂
  linarith
  -----
  -- Orig Proof
  import Mathlib
  import Aesop

  set_option maxHeartbeats 0

  open BigOperators Real Nat Topology Rat

  theorem amc12b_2002_p4
    (n : ℕ)
    (h₁ : 0 < n)
    (h₂ : ((1 / 2 + 1 / 3 + 1 / 7 + 1 / n) : ℚ).den =
      -1) :
    n = 42 := by
  have h_main : (n : ℕ) = 42 := by
  have h₁ : ((1 / 2 + 1 / 3 + 1 / 7 + 1 / (n : ℚ)
    → )) : ℚ) = (41 / 42 + 1 / (n : ℚ)) := by
  norm_num [div_eq_mul_inv]
  <> field_simp <> ring_nf <> norm_num
  <> simp_all [Nat.cast_add, Nat.cast_one]
  <> field_simp <> ring_nf <> norm_num
  <> linarith

  have h₂ : ((41 / 42 + 1 / (n : ℚ)) : ℚ) = (41 *
    → (n : ℚ) + 42) / (42 * (n : ℚ)) := by
  have h₃ : (n : ℚ) ≠ 0 := by positivity
  field_simp [h₁]
  <> ring_nf
  <> field_simp [h₁]
  <> ring_nf
  <> norm_num
  <> linarith

  have h₄ : ((1 / 2 + 1 / 3 + 1 / 7 + 1 / (n : ℚ)
    → )) : ℚ) = (41 * (n : ℚ) + 42) / (42 * (n
    → )) : ℚ)) := by
  rw [h₁, h₂]

  have h₅ : (((41 * (n : ℚ) + 42) / (42 * (n : ℚ)
    → )) : ℚ).den = 1 := by
  have h₆ : (((41 * (n : ℚ) + 42) / (42 * (n : ℚ)
    → )) : ℚ).den = 1 := h₅
  have h₇ : ∃ (k : ℤ), (41 * (n : ℚ) + 42) /
    → (42 * (n : ℚ)) = (k : ℚ) := by
  -- Use the fact that the denominator is 1
  -- to find an integer k
  have h₈ : ∃ (k : ℤ), (41 * (n : ℚ) + 42) /
    → (42 * (n : ℚ)) = (k : ℚ) := by
  -- Since the denominator is 1, the number
  -- is an integer
  refine' (((41 * (n : ℚ) + 42) / (42 * (n
    → )) : ℚ)).num, _
  have h₉ : (((41 * (n : ℚ) + 42) / (42 *
    → (n : ℚ)) : ℚ).den = 1 := h₇
  have h₁₀ : ((41 * (n : ℚ) + 42) / (42 *
    → (n : ℚ)) : ℚ) = (((41 * (n : ℚ) + 42) /
    → (42 * (n : ℚ)) : ℚ).num : ℚ) := by
  rw [- Rat.num_div_den ((41 * (n : ℚ) +
    → 42) / (42 * (n : ℚ)))]
  <> simp [h₁]
  <> norm_cast
  rw [h₁]
  <> norm_cast
  exact h₁
  exact h₂

  obtain (k, h₃) := h₈
  have h₄ : (41 * (n : ℚ) + 42) / (42 * (n : ℚ)) =
    → (k : ℚ) := h₃
  have h₅ : (41 * (n : ℚ) + 42) = (k : ℚ) * (42 *
    → (n : ℚ)) := by
  have h₆ : (n : ℚ) ≠ 0 := by positivity
  field_simp [h₆] at h₄
  <> ring_nf at h₄
  <> norm_cast at h₄
  <>
  (try norm_num at h₄) <>
  (try linarith) <>
  (try nlinarith) <>
  (try ring_nf at h₄) <> norm_num at h₄
  <> linarith
  <>
  nlinarith

  have h₇ : (41 : ℤ) * n + 42 = k * (42 * n) :=
  by
  norm_cast at h₄
  <>
  (try ring_nf at h₄) <>
  (try norm_num at h₄) <>
  (try field_simp at h₄) <>
  (try norm_cast at h₄) <>
  (try linarith)
  <>
  (try
  {
    ring_nf at h₄
    <>
    norm_cast at h₄
    <>
    field_simp at h₄
  })
  <>

```

```

norm_cast at h₄
<>
linarith
})
<>
(try
{
  norm_num at h₄
  <>
  ring_nf at h₄
  <>
  norm_cast at h₄
  <>
  linarith
})
)

have h₁ : (42 : ℤ) - n = (42 * n : ℤ) * (k -
  → 1) := by
have h₂ : (41 : ℤ) * n + 42 = k * (42 * n) :=
  → h₃
ring_nf at h₁
linarith

have h₃ : n ≤ 84 := by
  by_contra! h
  have h₄ : n ≥ 85 := by linarith
  have h₅ : (n : ℤ) ≥ 85 := by exact_mod_cast
  → h₃
  have h₆ : (42 : ℤ) - n < 0 := by linarith
  have h₇ : (42 * n : ℤ) > 0 := by positivity
  have h₈ : (42 : ℤ) - n = (42 * n : ℤ) * (k -
    → 1) := h₁
  have h₉ : (k - 1 : ℤ) < 0 := by
  nlinarith
  have h₁₀ : (k - 1 : ℤ) ≤ -1 := by
  linarith
  have h₁₁ : (42 : ℤ) - n ≤ - (42 * n : ℤ) := by
  nlinarith
  have h₁₂ : (n : ℤ) ≥ 85 := by exact_mod_cast
  → h₃
  nlinarith

have h₁₃ : n ≤ 84 := h₁₂
interval_cases n <> norm_num at h₁₃ h₁₁
<>
(try omega) <>
(try
{
  norm_num at h₁₃ h₁₁
  <>
  (try omega)
  <>
  (try
  {
    ring_nf at h₁₃ h₁₁
    <>
    norm_num at h₁₃ h₁₁
    <>
    omega
  })
  <>
  })
(try
{
  norm_cast at h₁₃ h₁₁
  <>
  (try omega)
  <>
  (try
  {
    ring_nf at h₁₃ h₁₁
    <>
    norm_num at h₁₃ h₁₁
    <>
    omega
  })
  <>
  })
)

exact h_main

-- Simplified Proof
import Mathlib
import Aesop

set_option maxHeartbeats 0

open BigOperators Real Nat Topology Rat

theorem amc12b_2002_p4
  (n : ℕ)
  (h₁ : 0 < n)
  (h₂ : ((1 / 2 + 1 / 3 + 1 / 7 + 1 / n) : ℚ).den =
    → 1) :
  n = 42 := by
  have h₃ : n = 42 := by
  have h₁ : (1 / 2 + 1 / 3 + 1 / 7 + 1 / (n : ℚ))
    → = (41 / 42 + 1 / (n : ℚ)) := by
  norm_num
  have h₂ : (41 / 42 + 1 / (n : ℚ)) = (41 * (n : ℚ)
    → ) + 42) / (42 * (n : ℚ)) := by
  field_simp [h₁.ne']
  rw [h₁, h₂] at h₁
  have h₃ : ∃ (k : ℤ), (41 * (n : ℚ) + 42) / (42 *
    → (n : ℚ)) = (k : ℚ) := by
  refine' (((41 * (n : ℚ) + 42) / (42 * (n : ℚ)
    → )) : ℚ).num, _
  rw [- Rat.num_div_den ((41 * (n : ℚ) + 42) /
    → (42 * (n : ℚ)))]
  <> simp [h₁]
  <> norm_cast
  obtain (k, h₄) := h₃
  have h₅ : (41 * (n : ℚ) + 42) = (k : ℚ) * (42 *
    → (n : ℚ)) := by
  field_simp [h₄.ne'] at h₄
  ring_nf at h₄
  norm_cast at h₄
  have h₆ : (41 * n + 42) = k * (42 * n) := by
  norm_cast at h₄
  have h₇ : (42 - n : ℤ) = (42 * n : ℤ) * (k - 1)
    → := by
  ring_nf at h₄

```

```

linarith
have h16 : n ≤ 84 := by
  by_contra! h
  have h17 : n ≥ 85 := by linarith
  have h18 : (n : z) ≥ 85 := by exact_mod_cast
    → h17
  have h19 : (42 : z) - n < 0 := by linarith
  have h20 : (42 * n : z) > 0 := by positivity
  have h21 : (42 : z) - n = (42 * n : z) * (k -
    → 1) := h19
  have h22 : (k - 1 : z) < 0 := by
    linarith
  have h23 : (k - 1 : z) ≤ -1 := by
    linarith
  have h24 : (42 : z) - n ≤ - (42 * n : z) := by
    linarith
  interval_cases n <|> norm_num at h16 <|>
    → omega
exact h16
-----
-- Orig Proof
import Mathlib
import Aesop

set_option maxHeartbeats 0

open BigOperators Real Nat Topology Rat

theorem mathd_algebra_484 :
  Real.log 27 / Real.log 3 = 3 := by
  have h_main : Real.log 27 / Real.log 3 = 3 := by
    have h : Real.log 27 = Real.log (3 ^ 3) := by
      → norm_num
    rw [h]
    have h : Real.log (3 ^ 3) = 3 * Real.log 3 :=
      → by
    rw [Real.log_pow] <|> norm_num
    rw [h]
    have h : Real.log 3 ≠ 0 := by
      have h : Real.log 3 > 0 := Real.log_pos (by
        → norm_num)
    linarith
    field_simp [h]
    <|> ring
    <|> norm_num
  exact h_main

-- Simplified Proof
import Mathlib
import Aesop

set_option maxHeartbeats 0

open BigOperators Real Nat Topology Rat

theorem mathd_algebra_484 :
  Real.log 27 / Real.log 3 = 3 := by
  rw [show Real.log 27 = Real.log (3 ^ 3) by
    → norm_num]
  field_simp
  -----
-- Orig Proof
import Mathlib
import Aesop

set_option maxHeartbeats 0

open BigOperators Real Nat Topology Rat

theorem mathd_numbertheory_551 :
  1529 % 6 = 5 := by
  have h : 1529 % 6 = 5 := by
    norm_num
    <|> rfl

  apply h

-- Simplified Proof
import Mathlib
import Aesop

set_option maxHeartbeats 0

open BigOperators Real Nat Topology Rat

theorem mathd_numbertheory_551 :
  1529 % 6 = 5 := by
    norm_num

-- Orig Proof
import Mathlib
import Aesop

set_option maxHeartbeats 0

open BigOperators Real Nat Topology Rat

theorem mathd_algebra_304 :
  91^2 = 8281 := by
  have h : 91^2 = 8281 := by
    norm_num
  exact h

-- Simplified Proof
import Mathlib
import Aesop

set_option maxHeartbeats 0

open BigOperators Real Nat Topology Rat

theorem mathd_algebra_304 :
  91^2 = 8281 := by
    norm_num
  -----
-- Orig Proof
import Mathlib
import Aesop

set_option maxHeartbeats 0

```

```

open BigOperators Real Nat Topology Rat

theorem amc12b_2021_p18
  (z : ℂ)
  (h1 : 12 * Complex.normSq z = 2 * Complex.normSq
    → (z + 2) + Complex.normSq (z^2 + 1) + 31) :
  z + 6 / z = -2 := by
  have h2 : z.re = -1 := by
    have h3 := h1
    simp [Complex.normSq, Complex.ext_iff,
      → pow_two, pow_succ, Complex.ext_iff,
      → Complex.mul_re, Complex.mul_im,
      Complex.add_re, Complex.add_im,
      → Complex.ofReal_add, Complex.ofReal_mul,
      → Complex.ofReal_one] at h3
    ring_nf at h3
    have h4 : 0 ≤ (z.re * z.re + z.im * z.im - 6)
      → ^ 2 + 4 * (z.re + 1) ^ 2 := by positivity
    linarith [sq_nonneg (z.re - 1), sq_nonneg
      → (z.im), sq_nonneg (z.re + 1),
      sq_nonneg (z.re * z.re + z.im * z.im - 6)]
  have h5 : z.re * z.re + z.im * z.im = 6 := by
    have h6 := h3
    simp [Complex.normSq, Complex.ext_iff,
      → pow_two, pow_succ, Complex.ext_iff,
      → Complex.mul_re, Complex.mul_im,
      Complex.add_re, Complex.add_im,
      → Complex.ofReal_add, Complex.ofReal_mul,
      → Complex.ofReal_one] at h6
    ring_nf at h6
    have h7 : 0 ≤ (z.re * z.re + z.im * z.im - 6)
      → ^ 2 + 4 * (z.re + 1) ^ 2 := by positivity
    linarith [sq_nonneg (z.re - 1), sq_nonneg
      → (z.im), sq_nonneg (z.re + 1),
      sq_nonneg (z.re * z.re + z.im * z.im - 6)]
  have h8 : z.im * z.im = 5 := by
    have h9 : z.re = -1 := h2
    have h10 : z.re * z.re + z.im * z.im = 6 := h5
    rw [h9] at h10
    ring_nf at h10
    <|> nlinarith
  have h11 : z + 6 / z = -2 := by
    have h12 : z.re = -1 := h2
    have h13 : z.im * z.im = 5 := h8
    have h14 : z ≠ 0 := by
      by_contra h
      rw [h] at h12
      norm_num [Complex.normSq, pow_two] at h12
      <|> simp_all [Complex.ext_iff]
      <|> nlinarith
    -- Compute z + 6 / z using the real and
    -- imaginary parts
    have h15 : z + 6 / z = -2 := by
      field_simp [Complex.ext_iff, Complex.normSq,
        → pow_two, h13, Complex.ext_iff,
        → Complex.div_re, Complex.div_im,
        Complex.normSq, pow_two]
      <|> simp_all [Complex.ext_iff, pow_two]
      <|> ring_nf at h15
      <|> norm_num at *
      <|>
      (try
        {
          nlinarith
        })
      <|>
      (try
        {
          cases' le_total 0 z.im with h16 h17 <|>
            simp_all [sq, mul_comm] <|>
              nlinarith [sq_nonneg (z.im)]
        })
      <|>
      (try
        {
          nlinarith [sq_nonneg (z.im)]
        })
      <|>
      exact h15
    exact h11

-- Simplified Proof
import Mathlib
import Aesop

set_option maxHeartbeats 0

open BigOperators Real Nat Topology Rat

theorem amc12b_2021_p18
  (z : ℂ)
  (h1 : 12 * Complex.normSq z = 2 * Complex.normSq
    → (z + 2) + Complex.normSq (z^2 + 1) + 31) :
  z + 6 / z = -2 := by
  simp [Complex.normSq, Complex.ext_iff, pow_two]
    → at h1
  have h2 : z.re = -1 := by
    linarith [sq_nonneg (z.re - 1), sq_nonneg
      → (z.re + 1),
      sq_nonneg (z.re * z.re + z.im * z.im - 6)]
  have h3 : z.im * z.im = 5 := by
    linarith [sq_nonneg (z.re - 1), sq_nonneg
      → (z.re + 1),
      sq_nonneg (z.re * z.re + z.im * z.im - 6)]
  field_simp [Complex.ext_iff, h2, h3]
  <|> norm_num
  <|> linarith
  -----
-- Orig Proof
import Mathlib
import Aesop

set_option maxHeartbeats 0

```

```

open BigOperators Real Nat Topology Rat

theorem amc12b_2002_p19
  (a b c : ℝ)
  (h1 : 0 < a ∧ 0 < b ∧ 0 < c)
  (h2 : a * (b + c) = 152)
  (h3 : b * (c + a) = 162)
  (h4 : c * (a + b) = 170) :
  a * b * c = 720 := by
  have h5 : a * b + a * c + b * c = 242 := by
    have h6 : a * (b + c) + b * (c + a) + c * (a +
      → b) = 484 := by
      linarith
    have h7 : a * (b + c) + b * (c + a) + c * (a +
      → b) = 2 * (a * b + a * c + b * c) := by
      ring
      linarith
  have h8 : b * c = 90 := by
    have h9 : a * b + a * c + b * c = 242 := h5
    have h10 : a * (b + c) = 152 := h2
    have h11 : a * b + a * c = 152 := by linarith
    linarith
  have h12 : a * c = 80 := by
    have h13 : a * b + a * c + b * c = 242 := h5
    have h14 : b * (c + a) = 162 := h3
    have h15 : b * c + a * b = 162 := by linarith
    linarith
  have h16 : a * b = 72 := by
    have h17 : a * b + a * c + b * c = 242 := h5
    have h18 : c * (a + b) = 170 := h4
    have h19 : a * c + b * c = 170 := by linarith
    linarith
  have h20 : (a * b * c) ^ 2 = 518400 := by
    have h21 : (a * b * c) ^ 2 = (a * b) * (a * c) *
      → (b * c) := by
      ring
      rw [h16]
    have h22 : a * b = 72 := h12
    have h23 : a * c = 80 := h12
    have h24 : b * c = 90 := h12
    rw [h22, h23, h24]
    <|> norm_num
  have h25 : a * b * c = 720 := by
    have h26 : 0 < a := h1
    have h27 : 0 < b := h1
    have h28 : 0 < c := h1
    have h29 : 0 < a * b := by positivity
    have h30 : 0 < a * c := by positivity
    have h31 : 0 < b * c := by positivity
    have h32 : 0 < a * b * c := by positivity
    have h33 : (a * b * c) ^ 2 = 518400 := h20
    have h34 : a * b * c > 0 := by positivity
    have h35 : a * b * c = 720 := by
      nlinarith [sq_nonneg (a * b * c - 720)]
    exact h35
  -----
-- Orig Proof
import Mathlib
import Aesop

set_option maxHeartbeats 0

open BigOperators Real Nat Topology Rat

theorem amc12b_2002_p19
  (a b c : ℝ)
  (h1 : 0 < a ∧ 0 < b ∧ 0 < c)
  (h2 : a * (b + c) = 152)
  (h3 : b * (c + a) = 162)
  (h4 : c * (a + b) = 170) :
  a * b * c = 720 := by
  -----
-- Orig Proof
import Mathlib
import Aesop

set_option maxHeartbeats 0

open BigOperators Real Nat Topology Rat

theorem mathd_numbertheory_341
  (a b c : ℕ)
  (h1 : a ≤ 9 ∧ b ≤ 9 ∧ c ≤ 9)
  (h2 : Nat.digits 10 ((5^100) % 1000) = [c, b, a]) :
  a + b + c = 13 := by
  have h3 : (5^100) % 1000 = 625 := by
    norm_num
    <|> rfl
  have h4 : Nat.digits 10 625 = [c, b, a] := by
    have h5 : Nat.digits 10 ((5^100) % 1000) =
      → [c, b, a] := h2
    rw [h4] at h5
    exact h5
  have h6 : Nat.digits 10 625 = [5, 2, 6] := by
    norm_num [Nat.digits_len]
    <|> rfl
  have h7 : c = 5 ∧ b = 2 ∧ a = 6 := by
    have h8 : [c, b, a] = [5, 2, 6] := by
      rw [h6] at h8
      exact h8.symm
    have h9 : c = 5 := by
      have h10 := congr_arg (fun l => l.get? 0) h8
      simp at h10
    <|> aesop
    have h11 : b = 2 := by
      have h12 := congr_arg (fun l => l.get? 1) h8
      simp at h12
    <|> aesop
    <|> aesop

```







```

open BigOperators Real Nat Topology Rat

theorem induction_1ldiv10tonmmiton
  (n : ℕ) :
  11 ∣ (10^n - (-1 : ℤ)^n) := by
  have h_main : (11 : ℤ) ∣ (10 : ℤ)^n - (-1 : ℤ)^n
  → := by
  have h : (10 : ℤ) - (-1 : ℤ) ∣ (10 : ℤ)^n - (-1 : ℤ)^n
  → := by
  → z^n := by
  -- Use the lemma that x - y divides x^n - y^n
  → in a commutative ring
  apply sub_dvd_pow_sub_pow
  -- Simplify (10 : ℤ) - (-1 : ℤ) to 11
  have h : (10 : ℤ) - (-1 : ℤ) = (11 : ℤ) := by
  → norm_num
  -- Substitute 11 for (10 : ℤ) - (-1 : ℤ) in the
  → divisibility statement
  rw [h] at h
  -- The result follows directly from the
  → divisibility statement
  exact h

-- Convert the divisibility statement in z to the
-- required form
exact_mod_cast h_main

-- Simplified Proof
import Mathlib
import Aesop

set_option maxHeartbeats 0

open BigOperators Real Nat Topology Rat

theorem induction_1ldiv10tonmmiton
  (n : ℕ) :
  11 ∣ (10^n - (-1 : ℤ)^n) := by
  apply sub_dvd_pow_sub_pow
  -----
  -- Orig Proof
  import Mathlib
  import Aesop

  set_option maxHeartbeats 0

  open BigOperators Real Nat Topology Rat

  theorem amc12a_2019_p12 (x y : ℕ) (h : x ≠ 1 ∧ y ≠
    1)
  (h : Real.log x / Real.log 2 = Real.log 16 /
    → Real.log y) (h : x * y = 64) :
  (Real.log (x / y) / Real.log 2) ^ 2 = 20 := by
  have h_main : False := by
  have h : x ∣ 64 := by
  use y
  <|> norm_cast at h ∣ <|> linarith
  use x
  <|> norm_cast at h ∣ <|> linarith
  have h : x = 2 √ x = 4 √ x = 8 √ x = 16 √ x =
  → 32 √ x = 64 := by
  have h₁ : x ∣ 64 := h
  have h₂ : x ≠ 1 := h.1
  have h₃ : x ≤ 64 := by
  have h₄ : x = 64 := h
  exact Nat.le_of_dvd (by norm_num) h₄
  interval_cases x <|> norm_num at h₁ ∣ <|>
  (try omega) <|> (try norm_num) <|> (try
    omega)
  <|>
  (try {
    simp_all [Nat.dvd_iff_mod_eq_zero]
    <|> omega
  })
  have h : y = 2 √ y = 4 √ y = 8 √ y = 16 √ y =
  → 32 √ y = 64 := by
  have h₁ : y ∣ 64 := h
  have h₂ : y ≠ 1 := h.2
  have h₃ : y ≤ 64 := by
  have h₄ : y = 64 := h
  exact Nat.le_of_dvd (by norm_num) h₄
  interval_cases y <|> norm_num at h₁ ∣ <|>
  (try omega) <|> (try norm_num) <|> (try
    omega)
  <|>
  (try {
    simp_all [Nat.dvd_iff_mod_eq_zero]
    <|> omega
  })
  -- We now check all possible pairs (x, y) to
  -- find a contradiction.
  have h : False := by
  rcases h with (rfl | rfl | rfl | rfl | rfl |
    <|> rfl) <|>
  rcases h with (rfl | rfl | rfl | rfl | rfl |
    <|> | rfl) <|>
  norm_num at h₁ h₂ ∣ <|>
  (try contradiction) <|>
  (try {
    have h : Real.log 2 > 0 :=
    → Real.log_pos (by norm_num)
    have h : Real.log 4 = 2 * Real.log 2 :=
    → by
    have h₁ : Real.log 4 = Real.log (2 ^
      2) := by norm_num
    rw [h₁]
    have h₂ : Real.log (2 ^ 2) = 2 *
    → Real.log 2 := by
    rw [Real.log_pow] <|> norm_num
    rw [h₂]
    have h₃ : Real.log 8 = 3 * Real.log 2
    → := by
    have h₁ : Real.log 8 = Real.log (2 ^
      3) := by norm_num
    rw [h₁]
    have h₂ : Real.log (2 ^ 3) = 3 *
    → Real.log 2 := by

```

```

      rw [Real.log_pow] <|> norm_num
      rw [h₂]
      have h₁ : Real.log 16 = 4 * Real.log 2
      → := by
      have h₁ : Real.log 16 = Real.log (2
        ^ 4) := by norm_num
      rw [h₁]
      have h₂ : Real.log (2 ^ 4) = 4 *
      → Real.log 2 := by
      rw [Real.log_pow] <|> norm_num
      rw [h₂]
      have h₃ : Real.log 32 = 5 * Real.log 2
      → := by
      have h₃ : Real.log 32 = Real.log (2
        ^ 5) := by norm_num
      rw [h₃]
      have h₄ : Real.log (2 ^ 5) = 5 *
      → Real.log 2 := by
      rw [Real.log_pow] <|> norm_num
      rw [h₄]
      have h₅ : Real.log 64 = 6 * Real.log 2
      → := by
      have h₅ : Real.log 64 = Real.log (2
        ^ 6) := by norm_num
      rw [h₅]
      have h₆ : Real.log (2 ^ 6) = 6 *
      → Real.log 2 := by
      rw [Real.log_pow] <|> norm_num
      rw [h₆]
      -- Simplify the given logarithmic
      → equation for each pair (a, y)
      field_simp [Real.log_mul,
        → Real.log_pow, h₁, h₂, h₃, h₄, h₅,
        → Real.log_ne_zero_of_pos_of_ne_one (by
        → norm_num : (0 : ℝ) < 2) (by norm_num : (2
        → : ℝ) ≠ 1)] at h₁ ∣
      <|>
      (try {
        nlinarith [Real.log_pos (by norm_num
          → : (1 : ℝ) < 2)]
      }) <|>
      (try {
        ring_nf at h₁ ∣ <|>
        nlinarith [Real.log_pos (by norm_num
          → : (1 : ℝ) < 2)]
      }) <|>
      (try {
        norm_num at h₁ ∣ <|>
        nlinarith [Real.log_pos (by norm_num
          → : (1 : ℝ) < 2)]
      })
      exact h
      have h_final : (Real.log (x / y) / Real.log 2) ^
        → 2 = 20 := by
      exfalso
      exact h_main
      exact h_final
  -- Simplified Proof
  import Mathlib
  import Aesop

  set_option maxHeartbeats 0

  open BigOperators Real Nat Topology Rat

  theorem amc12a_2019_p12 (x y : ℕ) (h : x ≠ 1 ∧ y ≠
    1)
  (h : Real.log x / Real.log 2 = Real.log 16 /
    → Real.log y) (h : x * y = 64) :
  (Real.log (x / y) / Real.log 2) ^ 2 = 20 := by
  have h : x ∣ 64 := by
  use y
  linarith
  have h : y ∣ 64 := by
  use x
  linarith
  have h : x ≤ 64 := Nat.le_of_dvd (by norm_num) h
  have h : y ≤ 64 := Nat.le_of_dvd (by norm_num) h
  interval_cases x <|> interval_cases y <|>
  → norm_num at h₁ h₂ ∣
  all_goals
  have h : Real.log 2 > 0 := Real.log_pos (by
    → norm_num)
  have h : Real.log 4 = 2 * Real.log 2 := by
  rw [← Real.log_pow] <|> norm_num
  have h : Real.log 8 = 3 * Real.log 2 := by
  rw [← Real.log_pow] <|> norm_num
  have h : Real.log 16 = 4 * Real.log 2 := by
  rw [← Real.log_pow] <|> norm_num
  have h : Real.log 32 = 5 * Real.log 2 := by
  rw [← Real.log_pow] <|> norm_num
  have h : Real.log 64 = 6 * Real.log 2 := by
  rw [← Real.log_pow] <|> norm_num
  field_simp [Real.log_mul, Real.log_pow, h₁, h₂,
    → h₁, h₂, h₃,
    → Real.log_ne_zero_of_pos_of_ne_one (by
    → norm_num : (0 : ℝ) < 2) (by norm_num : (2
    → : ℝ) ≠ 1)] at h₁ ∣
  <|> nlinarith [Real.log_pos (by norm_num : (1
    → : ℝ) < 2)]
  -----
  -- Orig Proof
  import Mathlib
  import Aesop

  set_option maxHeartbeats 0

  open BigOperators Real Nat Topology Rat

  theorem algebra_amgm_sumitoeqn_proditoeq1
  (a : ℕ → NNReal)
  (n : ℕ)
  (h : ∑ x ∈ Finset.range n, a x = n) :
  (h : ∑ x ∈ Finset.range n, a x ≤ 1 := by
  exact_mod_cast calc
  h x ∈ Finset.range n, (a x : ℝ) ≤ h x ∈
  → Finset.range n, Real.exp ((a x : ℝ) - 1)
  → := h
  _ = Real.exp (∑ x ∈ Finset.range n, ((a x : ℝ)
    → ) - 1)) := by rw [h]
  _ = 1 := by rw [h]

  have h : h x ∈ Finset.range n, a x ≤ 1 := by
  have h : (h x ∈ Finset.range n, a x : ℝ) ≤ 1 :=
  → by
  -- Use the fact that the product of the real
  → numbers is less than or equal to 1
  simp [Finset.prod_coe_sort] using h
  -- Use the property of the coercion from NNReal
  → to Real to conclude the proof
  exact_mod_cast h

  exact h

  -- Simplified Proof
  import Mathlib
  import Aesop

  set_option maxHeartbeats 0

  open BigOperators Real Nat Topology Rat

  theorem algebra_amgm_sumitoeqn_proditoeq1
  (a : ℕ → NNReal)
  (n : ℕ)
  (h : ∑ x ∈ Finset.range n, a x = n) :
  (h : ∑ x ∈ Finset.range n, a x ≤ 1 := by
  exact_mod_cast calc
  h x ∈ Finset.range n, (a x : ℝ) ≤ h x ∈
  → Finset.range n, Real.exp ((a x : ℝ) - 1)
  → :=

```

```

h x ∈ Finset.range n, a x ≤ 1 := by
have h : (h x ∈ Finset.range n, (a x : ℝ)) ≤ 1 :=
  → by
  have h : ∑ x ∈ Finset.range n, 0 ≤ x → x ≤ Real.exp (x -
    → 1) := by
  intro x h
  have h : Real.exp (x - 1) ≥ x := by
  have h : Real.exp (x - 1) ≥ 1 + (x - 1) :=
  → by
  linarith [Real.add_one_le_exp (x - 1)]
  linarith
  have h : ∑ i ∈ Finset.range n, (a i : ℝ) ≤
  → Real.exp ((a i : ℝ) - 1) := by
  intro i
  have h : 0 ≤ (a i : ℝ) := by exact_mod_cast
  → (a i).prop
  exact h (a i : ℝ) h
  have h : (h x ∈ Finset.range n, (a x : ℝ)) ≤ h
  → x ∈ Finset.range n, Real.exp ((a x : ℝ) -
    → 1) := by
  apply Finset.prod_le_prod
  . intro i h
  . exact by
    have h : 0 ≤ (a i : ℝ) := by exact
    → mod_cast (a i).prop
    linarith [h i h]
  . intro i h
  . exact h i h
  have h : h x ∈ Finset.range n, Real.exp ((a x
    → : ℝ) - 1) = Real.exp (∑ x ∈ Finset.range
    → n, ((a x : ℝ) - 1)) := by
  have h : h x ∈ Finset.range n, Real.exp ((a
    → x : ℝ) - 1) = Real.exp (∑ x ∈
    → Finset.range n, ((a x : ℝ) - 1)) := by
  rw [Real.exp_sum]
  <|> simp [Finset.prod_const]
  rw [h]
  have h : (∑ x ∈ Finset.range n, ((a x : ℝ) - 1
    → : ℝ)) = 0 := by
  have h : (∑ x ∈ Finset.range n, ((a x : ℝ) -
    → 1 : ℝ)) = (∑ x ∈ Finset.range n, (a x : ℝ
    → )) - n := by
  calc
  (∑ x ∈ Finset.range n, ((a x : ℝ) - 1 : ℝ
    → )) = ∑ x ∈ Finset.range n, ((a x : ℝ) - 1
    → : ℝ) := rfl
  _ = ∑ x ∈ Finset.range n, ((a x : ℝ) - 1
    → : ℝ) := rfl
  _ = (∑ x ∈ Finset.range n, (a x : ℝ)) - ∑
  → x ∈ Finset.range n, (1 : ℝ) := by
  rw [Finset.sum_sub_distrib]
  _ = (∑ x ∈ Finset.range n, (a x : ℝ)) - n
  → := by
  simp [Finset.sum_const,
    → Finset.card_range]
  <|> ring_nf
  <|> norm_cast
  <|> field_simp
  <|> ring_nf
  have h : (∑ x ∈ Finset.range n, (a x : ℝ)) =
  → n := by
  have h : (∑ x ∈ Finset.range n, (a x : ℝ))
  → = (∑ x ∈ Finset.range n, a x : ℝ) := by
  → simp
  rw [h]
  norm_cast
  <|> simp [h]
  <|> simp_all [Finset.sum_range_succ]
  <|> norm_num
  <|> linarith
  rw [h, h]
  <|> ring_nf
  <|> norm_num
  have h : Real.exp (∑ x ∈ Finset.range n, ((a x
    → : ℝ) - 1)) = 1 := by
  rw [h]
  norm_num [Real.exp_zero]
  calc
  (h x ∈ Finset.range n, (a x : ℝ)) ≤ h x ∈
  → Finset.range n, Real.exp ((a x : ℝ) - 1)
  → := h
  _ = Real.exp (∑ x ∈ Finset.range n, ((a x : ℝ)
    → ) - 1)) := by rw [h]
  _ = 1 := by rw [h]

  have h : h x ∈ Finset.range n, a x ≤ 1 := by
  have h : (h x ∈ Finset.range n, a x : ℝ) ≤ 1 :=
  → by
  -- Use the fact that the product of the real
  → numbers is less than or equal to 1
  simp [Finset.prod_coe_sort] using h
  -- Use the property of the coercion from NNReal
  → to Real to conclude the proof
  exact_mod_cast h

  exact h

  -- Simplified Proof
  import Mathlib
  import Aesop

  set_option maxHeartbeats 0

  open BigOperators Real Nat Topology Rat

  theorem algebra_amgm_sumitoeqn_proditoeq1
  (a : ℕ → NNReal)
  (n : ℕ)
  (h : ∑ x ∈ Finset.range n, a x = n) :
  (h : ∑ x ∈ Finset.range n, a x ≤ 1 := by
  exact_mod_cast calc
  h x ∈ Finset.range n, (a x : ℝ) ≤ h x ∈
  → Finset.range n, Real.exp ((a x : ℝ) - 1)
  → :=

```



```

Finset.prod_le_prod (fun i _ => by simp) (fun
  => i _ => by
    linarith [add_one_le_exp ((a i : R) - 1)])
- = Real.exp (x x ∈ Finset.range n, ((a x : R)
  => - 1)) := by rw [Real.exp_sum]
- = 1 := by simp [show x x ∈ Finset.range n, (a
  => x : R) = n by exact_mod_cast h]]

-----
-- Orig Proof
import Mathlib
import Aesop

set_option maxHeartbeats 0

open BigOperators Real Nat Topology Rat

theorem mathd_algebra_332
(x y : R)
(h₁ : (x + y) / 2 = 7)
(h₂ : Real.sqrt (x * y) = Real.sqrt 19) :
x^2 + y^2 = 158 := by
have h₃ : x + y = 14 := by
  have h₄ : (x + y) / 2 = 7 := h₁
  have h₅ : x + y = 14 := by
    linarith
  exact h₅
have h₆ : x * y = 19 := by
  have h₇ : Real.sqrt (x * y) = Real.sqrt 19 := h₂
  have h₈ : Real.sqrt 19 > 0 :=
    → Real.sqrt_pos.mpr (by norm_num)
  have h₉ : x * y ≥ 0 := by
    by_contra h
    have h₁₀ : x * y < 0 := by linarith
    have h₁₁ : Real.sqrt (x * y) = 0 := by
      rw [Real.sqrt_eq_zero_of_nonpos] <|>
      → linarith
    have h₁₂ : Real.sqrt 19 > 0 :=
      → Real.sqrt_pos.mpr (by norm_num)
    rw [h₁] at h₁
    linarith
  have h₁₃ : Real.sqrt (x * y) = Real.sqrt 19 := h₂
  have h₁₄ : (Real.sqrt (x * y))^2 = (Real.sqrt
    → 19)^2 := by rw [h₁]
  have h₁₅ : (Real.sqrt (x * y))^2 = x * y := by
    rw [Real.sq_sqrt] <|> linarith
  have h₁₆ : (Real.sqrt 19)^2 = (19 : R) := by
    rw [Real.sq_sqrt] <|> norm_num
  linarith
have h₁₇ : x^2 + y^2 = 158 := by
  have h₁₈ : x^2 + y^2 = (x + y)^2 - 2 * (x
    → * y) := by ring
  rw [h₁]
  rw [h₂, h₃]
  norm_num
  exact h₁₈

-- Simplified Proof
import Mathlib
import Aesop

set_option maxHeartbeats 0

open BigOperators Real Nat Topology Rat

theorem mathd_algebra_332
(x y : R)
(h₁ : (x + y) / 2 = 7)
(h₂ : Real.sqrt (x * y) = Real.sqrt 19) :
x^2 + y^2 = 158 := by
have h₃ : x * y = 19 := by
  have h₄ : 0 ≤ x * y := by
    apply le_of_lt
    apply Real.sqrt_pos.mpr
    rw [h₂]
    norm_num
  rw [Real.sqrt_inj this (by norm_num)] at h₂
  linarith
  nlinarith

-- Orig Proof
import Mathlib
import Aesop

set_option maxHeartbeats 0

open BigOperators Real Nat Topology Rat

theorem mathd_algebra_440
(x : R)
(h₁ : 3 / 2 / 3 = x / 10) :
x = 5 := by
have h₂ : x = 5 := by
  have h₃ : (3 : R) / 2 / 3 = x / 10 := h₁
  -- Simplify the left-hand side of the equation
  norm_num at h₃
  -- Solve the equation using linear arithmetic
  <|> linarith
  -- The final result is x = 5
  exact h₃

-- Simplified Proof
import Mathlib
import Aesop

set_option maxHeartbeats 0

open BigOperators Real Nat Topology Rat

theorem mathd_algebra_440
(x : R)
(h₁ : 3 / 2 / 3 = x / 10) :
x = 5 := by
  linarith

-----
-- Orig Proof
import Mathlib
import Aesop

set_option maxHeartbeats 0

open BigOperators Real Nat Topology Rat

theorem mathd_algebra_293
(x : NNReal) :
Real.sqrt (60 * x) * Real.sqrt (12 * x) *
  → Real.sqrt (63 * x) = 36 * x * Real.sqrt
  → (35 * x) := by
have h₁ : (Real.sqrt (60 * x) * Real.sqrt (12 *
  → x) * Real.sqrt (63 * x) : R) = Real.sqrt
  → ((60 * x : R) * (12 * x : R) * (63 * x : R
  → )) := by
  have h₂ : 0 ≤ (60 * x : R) := by positivity
  have h₃ : 0 ≤ (12 * x : R) := by positivity
  have h₄ : 0 ≤ (63 * x : R) := by positivity
  have h₅ : 0 ≤ (60 * x : R) * (12 * x : R) :=
    → by positivity
  have h₆ : 0 ≤ (60 * x : R) * (12 * x : R) *
    → (63 * x : R) := by positivity
  have h₇ : Real.sqrt (60 * x) * Real.sqrt (12 *
    → x) = Real.sqrt ((60 * x : R) * (12 * x : R
    → )) := by
    rw [- Real.sqrt_mul] <|> positivity
  calc
    (Real.sqrt (60 * x) * Real.sqrt (12 * x) *
    → Real.sqrt (63 * x) : R) = Real.sqrt ((60 *
    → x : R) * (12 * x : R) * (63 * x : R)) := by
    rw [h₁]
    = Real.sqrt ((60 * x : R) * (12 * x : R) *
    → (63 * x : R)) := by
    have h₈ : 0 ≤ (60 * x : R) * (12 * x : R)
    → := by positivity
    have h₉ : 0 ≤ (63 * x : R) := by positivity
    have h₁₀ : 0 ≤ (60 * x : R) * (12 * x : R) *
    → (63 * x : R) := by positivity
    rw [- Real.sqrt_mul] <|> ring_nf <|>
    → positivity
have h₂ : (60 : R) * (12 : R) * (63 : R) = (36 : R
  → )^2 * (35 : R) := by
  norm_num
have h₃ : ((60 * x : R) * (12 * x : R) * (63 * x
  → : R) : R) = (36 * (x : R))^2 * (35 * (x :
  → R)) := by
  have h₄ : ((60 * x : R) * (12 * x : R) * (63 *
    → x : R) : R) = (60 : R) * (12 : R) * (63 :
    → R) * (x : R)^3 := by
    ring_nf
    <|> field_simp [NNReal.coe_mul,
    → NNReal.coe_pow]
    <|> ring_nf
  rw [h₁]
  have h₅ : (60 : R) * (12 : R) * (63 : R) = (36
    → : R)^2 * (35 : R) := h₃
  rw [h₁]
  have h₆ : ((36 : R)^2 * (35 : R) * (x : R)^3 : R
    → ) = (36 * (x : R))^2 * (35 * (x : R)) :=
    → by
    ring_nf
    <|> field_simp [NNReal.coe_mul,
    → NNReal.coe_pow]
    <|> ring_nf
    <|> norm_num
    <|> nlinarith
  linarith
have h₇ : Real.sqrt ((60 * x : R) * (12 * x : R) *
  → (63 * x : R)) = 36 * (x : R) * Real.sqrt
  → (35 * (x : R)) := by
  have h₈ : 0 ≤ (x : R) := by exact_mod_cast
  → x.property
  have h₉ : 0 ≤ 36 * (x : R) : R := by
    → positivity
  have h₁₀ : 0 ≤ (35 * (x : R) : R) := by
    → positivity
  have h₁₁ : 0 ≤ (36 * (x : R))^2 * (35 * (x : R
    → )) := by positivity
  have h₁₂ : Real.sqrt ((60 * x : R) * (12 * x : R
    → ) * (63 * x : R)) = Real.sqrt ((36 * (x :
    → R))^2 * (35 * (x : R))) := by
    rw [h₁]
  rw [h₁]
  have h₁₃ : Real.sqrt ((36 * (x : R))^2 * (35 *
    → (x : R))) = 36 * (x : R) * Real.sqrt (35 *
    → (x : R)) := by
  have h₁₄ : 0 ≤ (36 * (x : R) : R) := by
    → positivity
  have h₁₅ : 0 ≤ (35 * (x : R) : R) := by
    → positivity
  have h₁₆ : 0 ≤ (36 * (x : R))^2 * (35 * (x : R
    → )) := by positivity
  have h₁₇ : Real.sqrt ((36 * (x : R))^2 * (35 *
    → (x : R))) = Real.sqrt ((36 * (x : R))^2
    → * Real.sqrt (35 * (x : R))) := by
    rw [Real.sqrt_mul (by positivity)]
  rw [h₁]
  have h₁₈ : Real.sqrt ((36 * (x : R))^2) = 36 *
    → (x : R) := by
    rw [Real.sqrt_sq (by positivity)]
  rw [h₁]
  <|> ring_nf
  <|> field_simp [Real.sqrt_eq_iff_sq_eq] <|>
  → ring_nf <|> nlinarith
  rw [h₁]
  <|> ring_nf
  <|> field_simp [Real.sqrt_eq_iff_sq_eq] <|>
  → ring_nf <|> nlinarith

```

```

import Aesop

set_option maxHeartbeats 0

open BigOperators Real Nat Topology Rat

theorem mathd_algebra_293
(x : NNReal) :
Real.sqrt (60 * x) * Real.sqrt (12 * x) *
  → Real.sqrt (63 * x) = 36 * x * Real.sqrt
  → (35 * x) := by
have h₁ : (Real.sqrt (60 * x) * Real.sqrt (12 *
  → x) * Real.sqrt (63 * x) : R) = Real.sqrt
  → ((60 * x : R) * (12 * x : R) * (63 * x : R
  → )) := by
  have h₂ : 0 ≤ (60 * x : R) := by positivity
  have h₃ : 0 ≤ (12 * x : R) := by positivity
  have h₄ : 0 ≤ (63 * x : R) := by positivity
  have h₅ : 0 ≤ (60 * x : R) * (12 * x : R) :=
    → by positivity
  have h₆ : 0 ≤ (60 * x : R) * (12 * x : R) *
    → (63 * x : R) := by positivity
  have h₇ : Real.sqrt (60 * x) * Real.sqrt (12 *
    → x) = Real.sqrt ((60 * x : R) * (12 * x : R
    → )) := by
    rw [- Real.sqrt_mul] <|> positivity
  calc
    (Real.sqrt (60 * x) * Real.sqrt (12 * x) *
    → Real.sqrt (63 * x) : R) = Real.sqrt ((60 *
    → x : R) * (12 * x : R) * (63 * x : R)) := by
    rw [h₁]
    = Real.sqrt ((60 * x : R) * (12 * x : R) *
    → (63 * x : R)) := by
    have h₈ : 0 ≤ (60 * x : R) * (12 * x : R)
    → := by positivity
    have h₉ : 0 ≤ (63 * x : R) := by positivity
    have h₁₀ : 0 ≤ (60 * x : R) * (12 * x : R) *
    → (63 * x : R) := by positivity
    rw [- Real.sqrt_mul] <|> ring_nf <|>
    → positivity
have h₂ : (60 : R) * (12 : R) * (63 : R) = (36 : R
  → )^2 * (35 : R) := by
  norm_num
have h₃ : ((60 * x : R) * (12 * x : R) * (63 * x
  → : R) : R) = (36 * (x : R))^2 * (35 * (x :
  → R)) := by
  have h₄ : ((60 * x : R) * (12 * x : R) * (63 *
    → x : R) : R) = (60 : R) * (12 : R) * (63 :
    → R) * (x : R)^3 := by
    ring_nf
    <|> field_simp [NNReal.coe_mul,
    → NNReal.coe_pow]
    <|> ring_nf
  rw [h₁]
  have h₅ : (60 : R) * (12 : R) * (63 : R) = (36
    → : R)^2 * (35 : R) := h₃
  rw [h₁]
  have h₆ : ((36 : R)^2 * (35 : R) * (x : R)^3 : R
    → ) = (36 * (x : R))^2 * (35 * (x : R)) :=
    → by
    ring_nf
    <|> field_simp [NNReal.coe_mul,
    → NNReal.coe_pow]
    <|> ring_nf
    <|> norm_num
    <|> nlinarith
  linarith
have h₇ : Real.sqrt ((60 * x : R) * (12 * x : R) *
  → (63 * x : R)) = 36 * (x : R) * Real.sqrt
  → (35 * (x : R)) := by
  have h₈ : 0 ≤ (x : R) := by exact_mod_cast
  → x.property
  have h₉ : 0 ≤ 36 * (x : R) : R := by
    → positivity
  have h₁₀ : 0 ≤ (35 * (x : R) : R) := by
    → positivity
  have h₁₁ : 0 ≤ (36 * (x : R))^2 * (35 * (x : R
    → )) := by positivity
  have h₁₂ : Real.sqrt ((60 * x : R) * (12 * x : R
    → ) * (63 * x : R)) = Real.sqrt ((36 * (x :
    → R))^2 * (35 * (x : R))) := by
    rw [h₁]
  rw [h₁]
  have h₁₃ : Real.sqrt ((36 * (x : R))^2 * (35 *
    → (x : R))) = 36 * (x : R) * Real.sqrt (35 *
    → (x : R)) := by
  have h₁₄ : 0 ≤ (36 * (x : R) : R) := by
    → positivity
  have h₁₅ : 0 ≤ (35 * (x : R) : R) := by
    → positivity
  have h₁₆ : 0 ≤ (36 * (x : R))^2 * (35 * (x : R
    → )) := by positivity
  have h₁₇ : Real.sqrt ((36 * (x : R))^2 * (35 *
    → (x : R))) = Real.sqrt ((36 * (x : R))^2
    → * Real.sqrt (35 * (x : R))) := by
    rw [Real.sqrt_mul (by positivity)]
  rw [h₁]
  have h₁₈ : Real.sqrt ((36 * (x : R))^2) = 36 *
    → (x : R) := by
    rw [Real.sqrt_sq (by positivity)]
  rw [h₁]
  <|> ring_nf
  <|> field_simp [Real.sqrt_eq_iff_sq_eq] <|>
  → ring_nf <|> nlinarith
  rw [h₁]
  <|> ring_nf
  <|> field_simp [Real.sqrt_eq_iff_sq_eq] <|>
  → ring_nf <|> nlinarith

```

```

have h₁ : (36 * (x : R) * Real.sqrt (35 * (x : R
  → )) : R) = (36 * x * Real.sqrt (35 * x) : R
  → ) := by
  simp [NNReal.coe_mul]
  <|>
  (try norm_num) <|>
  (try ring_nf) <|>
  (try field_simp [Real.sqrt_eq_iff_sq_eq]) <|>
  (try norm_cast) <|>
  (try simp_all [NNReal.coe_mul]) <|>
  (try ring_nf) <|>
  (try nlinarith)

have h₂ : (Real.sqrt (60 * x) * Real.sqrt (12 *
  → x) * Real.sqrt (63 * x) : R) = (36 * x *
  → Real.sqrt (35 * x) : R) := by
  calc
    (Real.sqrt (60 * x) * Real.sqrt (12 * x) *
    → Real.sqrt (63 * x) : R) = Real.sqrt ((60 *
    → x : R) * (12 * x : R) * (63 * x : R)) :=
    → by
    rw [h₁]
  = 36 * (x : R) * Real.sqrt (35 * (x : R)) :=
    → by
    rw [h₁]
  = (36 * x * Real.sqrt (35 * x) : R) := by
    rw [h₁]

exact_mod_cast h₁

-- Simplified Proof
import Mathlib
import Aesop

set_option maxHeartbeats 0

open BigOperators Real Nat Topology Rat

theorem mathd_algebra_293
(x : NNReal) :
Real.sqrt (60 * x) * Real.sqrt (12 * x) *
  → Real.sqrt (63 * x) = 36 * x * Real.sqrt
  → (35 * x) := by
  rw [- Real.sqrt_mul]
  rw [- Real.sqrt_mul]
  rw [Real.sqrt_eq_iff_mul_self_eq]
  norm_num
  ring_nf
  simp
  <|> ring_nf
  <|> norm_cast
  all_goals positivity

-----
-- Orig Proof
import Mathlib
import Aesop

set_option maxHeartbeats 0

open BigOperators Real Nat Topology Rat

theorem mathd_numbertheory_254 :
(239 + 174 + 83) % 10 = 6 := by
have h : (239 + 174 + 83) % 10 = 6 := by
  norm_num
  <|> rfl

  apply h

-- Simplified Proof
import Mathlib
import Aesop

set_option maxHeartbeats 0

open BigOperators Real Nat Topology Rat

theorem mathd_numbertheory_254 :
(239 + 174 + 83) % 10 = 6 := by
  norm_num

-----
-- Orig Proof
import Mathlib
import Aesop

set_option maxHeartbeats 0

open BigOperators Real Nat Topology Rat

theorem amc12_2000_p6
(p q : ℕ)
(h₁ : Nat.Prime p ∧ Nat.Prime q)
(h₂ : 4 ≤ p ∧ p ≤ 18)
(h₃ : 4 ≤ q ∧ q ≤ 18) :
p * q - (p + q) ≠ 194 := by
have h_main : p * q - (p + q) ≠ 194 := by
  have h₁ : p ≤ 18 := by linarith
  have h₂ : q ≤ 18 := by linarith
  have h₃ : p ≥ 4 := by linarith
  have h₄ : q ≥ 4 := by linarith
  interval_cases p <|> interval_cases q <|>
    → norm_num [Nat.Prime] at h₁ <|>
    (try contradiction) <|> (try omega)
  exact h_main

-- Simplified Proof
import Mathlib
import Aesop

set_option maxHeartbeats 0

open BigOperators Real Nat Topology Rat

theorem amc12_2000_p6
(p q : ℕ)
(h₁ : Nat.Prime p ∧ Nat.Prime q)
(h₂ : 4 ≤ p ∧ p ≤ 18)
(h₃ : 4 ≤ q ∧ q ≤ 18) :

```



```

rw [h1] at h1
have h1 : ( (10 : N) + 4 : R) * f 10 4 = (4 : R)
  → ) * f 10 14 := by exact_mod_cast h1
have h1 : f 10 4 = (20 : R) := by
  <| simp_all [h1f104]
  <| norm_num
rw [h1] at h1
norm_num at h1
<| linarith
have h1f1410 : f 14 10 = 70 := by
  have h1 : f 14 10 = f 10 14 := by
    apply h1
    <| norm_num
  rw [h1]
  exact h1f1014
have h1f1424 : f 14 24 = 168 := by
  have h1 : ( (14 : N) + 10 : R) * f 14 10 = (10
    → : R) * f 14 (14 + 10) := by
    have h1 : h1 14 10 (by norm_num, by norm_num)
    norm_cast at h1
    <| ring_nf at h1
    <| linarith
  have h1 : f 14 (14 + 10) = f 14 24 := by
    → norm_num
  rw [h1] at h1
  have h1 : ( (14 : N) + 10 : R) * f 14 10 = (10
    → : R) * f 14 24 := by exact_mod_cast h1
  have h1 : f 14 10 = (70 : R) := by
    norm_cast at h1f1410
    <| simp_all [h1f1410]
    <| norm_num
  rw [h1] at h1
  norm_num at h1
  <| linarith
have h1f1438 : f 14 38 = 266 := by
  have h1 : ( (14 : N) + 24 : R) * f 14 24 = (24
    → : R) * f 14 (14 + 24) := by
    have h1 : h1 14 24 (by norm_num, by norm_num)
    norm_cast at h1
    <| ring_nf at h1
    <| linarith
  have h1 : f 14 (14 + 24) = f 14 38 := by
    → norm_num
  rw [h1] at h1
  have h1 : ( (14 : N) + 24 : R) * f 14 24 = (24
    → : R) * f 14 38 := by exact_mod_cast h1
  have h1 : f 14 24 = (168 : R) := by
    norm_cast at h1f1424
    <| simp_all [h1f1424]
    <| norm_num
  rw [h1] at h1
  norm_num at h1
  <| linarith
have h1f1452 : f 14 52 = 364 := by
  have h1 : ( (14 : N) + 38 : R) * f 14 38 = (38
    → : R) * f 14 (14 + 38) := by
    have h1 : h1 14 38 (by norm_num, by norm_num)
    norm_cast at h1
    <| ring_nf at h1
    <| linarith
  have h1 : f 14 (14 + 38) = f 14 52 := by
    → norm_num
  rw [h1] at h1
  have h1 : ( (14 : N) + 38 : R) * f 14 38 = (38
    → : R) * f 14 52 := by exact_mod_cast h1
  have h1 : f 14 38 = (266 : R) := by
    norm_cast at h1f1438
    <| simp_all [h1f1438]
    <| norm_num
  rw [h1] at h1
  norm_num at h1
  <| linarith
exact h1f1452
-- Simplified Proof
import Mathlib
import Aesop
set_option maxHeartbeats 0
open BigOperators Real Nat Topology Rat
theorem aime_1988_p8
  (f : N → N → R)
  (h1 : ∀ x, 0 < x → f x x = x)
  (h2 : ∀ x y, (0 < x ∧ 0 < y) → f x y = f y x)
  (h3 : ∀ x y, (0 < x ∧ 0 < y) → (x + y) * f x y =
    → y * (f x (x + y))) :
  f 14 52 = 364 := by
  have h1 : h1 2 2
  have h1 : h1 4 2
  have h1 : h1 4 6
  have h1 : h1 10 4
  have h1 : h1 14 10
  have h1 : h1 14 24
  have h1 : h1 14 38
  simp_all
  linarith
-----
-- Orig Proof
import Mathlib
import Aesop
set_option maxHeartbeats 0
open BigOperators Real Nat Topology Rat
theorem imo_2019_p1
  (f : Z → Z) :
  ((∀ a b, f (2 * a) + (2 * f b) = f (f (a + b))) →
    → (∀ z, f z = 0) ∨ (∃ c, ∀ z, f z = 2 * z +
    → c)) := by
  have h1 : (∀ a b, f (2 * a) + (2 * f b) = f (f
    → (a + b))) → (∀ z, f z = 0) ∨ (∃ c, ∀ z, f
    → z = 2 * z + c) := by
    intro h
    have h1 : (f 0 = 0) ∨ (f 0 = 2) := by
      have h1 : d = 0 ∨ d = 2 := by
        have h1 : d = 0 ∨ d = 2 := by
          have h1 : h 0 0
          have h1 : h 1 0
          have h1 : h 0 1
          have h1 : h 1 1
          have h1 : h (-1) 0
          have h1 : h 0 (-1)
          have h1 : h 1 (-1)
          have h1 : h (-1) 1
          simp [h1] at h1 h1 h1 h1 h1 h1 h1 h1
          ring_nf at h1 h1 h1 h1 h1 h1 h1 h1
          have h1 : d = 0 ∨ d = 2 := by
            have h1 : d * (d - 2) = 0 := by
              nlinarith [sq_nonneg (d - 2), sq_nonneg
                → d, eq_nonneg (d + 2)]
            have h1 : d = 0 ∨ d - 2 = 0 := by
              apply eq_zero_or_eq_zero_of_mul_eq_zero
              → h1
            cases h1 with
            | inl h1 =>
              exact Or.inl h1
            | inr h1 =>
              have h1 : d = 2 := by linarith
              exact Or.inr h1
          exact h1
        cases h1 with
        | inl h1 =>
          -- Case: d = 0
          have h1 : ∀ z, f z = 0 := by
            intro z
            have h1 : h z z
            rw [h1] at h1
            have h1 : c = 0 := by
              have h1 : h 0 0
              have h1 : h 1 0
              have h1 : h 0 1
              have h1 : h 1 1
              simp [h1] at h1 h1 h1 h1
              <| ring_nf at h1 h1 h1 h1
              <| nlinarith
            rw [h1] at h1
            ring_nf at h1
            <| linarith
            exact Or.inl h1
          | inr h1 =>
            -- Case: d = 2
            have h1 : ∃ c, ∀ z, f z = 2 * z + c := by
              use c
              intro z
              have h1 : h z z
              rw [h1] at h1
              ring_nf at h1
              <| linarith
              exact Or.inr h1
          have h1 : (∃ c, f z = 0) ∨ (∃ c, ∀ z, f z
            → = 2 * z + c) → (∀ a b, f (2 * a) + (2 *
            → f b) = f (f (a + b))) := by
            intro h
            cases h with
            | inl h =>
              -- Case: f(z) = 0 for all z
              intro a b
              have h1 : f (2 * a) = 0 := by rw [h]
              have h1 : f b = 0 := by rw [h]
              have h1 : f (a + b) = 0 := by rw [h]
              have h1 : f (f (a + b)) = 0 := by
                have h1 : f (a + b) = 0 := by rw [h]
                rw [h]
              simp [h1, h1, h1]
            | inr h =>
              -- Case: f(z) = 2z + c for some constant c
              rcases h with (c, hc)
              intro a b
              have h1 : f (2 * a) = 2 * (2 * a) + c := by
                rw [hc]
              <| ring_nf
              have h1 : f b = 2 * b + c := by
                rw [hc]
              have h1 : f (a + b) = 2 * (a + b) + c := by
                rw [hc]
              <| ring_nf
              have h1 : f (f (a + b)) = 2 * (2 * (a + b) +
                → c) + c := by
                have h1 : f (a + b) = 2 * (a + b) + c := by
                  rw [hc]
                  <| ring_nf
                rw [h1]
                <| ring_nf
              calc
                f (2 * a) + 2 * f b = (2 * (2 * a) + c) +
                  → 2 * (2 * b + c) := by rw [h1, h1]
                = 4 * a + c + 4 * b + 2 * c := by ring_nf
                = 4 * a + 4 * b + 3 * c := by ring_nf
                = 2 * (2 * (a + b) + c) + c := by ring_nf
                = f (f (a + b)) := by
                  rw [h1]
                  <| ring_nf
          have h1 : main : ((∀ a b, f (2 * a) + (2 * f b) = f
            → (f (a + b))) → (∀ z, f z = 0) ∨ (∃ c, ∀ z,
            → f z = 2 * z + c) := by
            apply Iff.intro
            -- Prove the forward direction: functional
            → equation implies the form of f
            intro h
            exact h_imp h
            -- Prove the backward direction: the form of f
            → implies the functional equation
            intro h
            exact h_converse h
          exact h_main
        -- Simplified Proof

```

```

import Mathlib
import Aesop

set_option maxHeartbeats 0

open BigOperators Real Nat Topology Rat

theorem imo_2019_p1
  (f :  $\mathbb{Z} \rightarrow \mathbb{Z}$ ) :
  (( $\forall a b, f(2 * a) + (2 * f b) = f(a + b)$ )) ↔
  (∃ c,  $\forall z, f z = 0$ ) ∨ (∃ c,  $\forall z, f z = 2 * z + c$ ) := by
  constructor
  · intro h
    have h₁ :  $\forall b, f(b) = f(0) + 2 * f b$  := by
      intro b
      have h₂ :  $h 0 b$ 
      simp at h₂
      linarith
    have h₁ :  $\forall a, f(2 * a) = 2 * f a + f 0$  := by
      intro a
      have h₂ :  $h a a$ 
      have h₃ :  $h₁ (2 * a)$ 
      have h₄ :  $h₁ a$ 
      ring_nf at h₄ h₃ h₂
      linarith
    have h₁ :  $\forall a, f(a + 1) = f a + (f 1 - f 0)$  :=
      by
      intro a
      have h₂ :  $h a 1$ 
      have h₃ :  $h₁ (a + 1)$ 
      have h₄ :  $h₁ a$ 
      have h₅ :  $h₁ 1$ 
      ring_nf at h₄ h₃ h₂ h₅
      linarith
    have h₁ :  $\exists (d c : \mathbb{Z}), \forall (n : \mathbb{Z}), f n = d * n + c$  := by
      use (f 1 - f 0), f 0
      intro n
      have h₁ :  $\forall n : \mathbb{N}, f n = (f 1 - f 0) * n + f 0$  := by
        induction n with
        | zero =>
          simp [h₁]
        | succ n ih =>
          have h₂ :  $h₁ n$ 
          simp [ih] at h₂
          <|> ring_nf at h₂
          <|> linarith
      have h₁ :  $\forall n : \mathbb{N}, f(-n : \mathbb{Z}) = (f 1 - f 0) * n$  := by
        induction n with
        | zero =>
          simp [h₁]
        | succ n ih =>
          have h₂ :  $h₁ (-n : \mathbb{Z}) - 1$ 
          have h₃ :  $h₁ (-n : \mathbb{Z})$ 
          simp [ih] at h₃ h₂
          <|> ring_nf at h₃ h₂
          <|> linarith
      by_cases h₁ :  $n \geq 0$ 
      · have h₁₀ :  $(n : \mathbb{Z}) \geq 0$  := by exact_mod_cast
        intro h₁
        have h₁₁ :  $\exists m : \mathbb{N}, (m : \mathbb{Z}) = n$  := by
          use n.toNat
          <|> simp [Int.toNat_of_nonneg h₁]
        rcases h₁₁ with ⟨m, rfl⟩
        have h₁₂ :  $h₁ m$ 
        simp at h₁₂
        <|> ring_nf at h₁₂
        <|> linarith
      · have h₁₀ :  $(n : \mathbb{Z}) < 0$  := by linarith
        have h₁₁ :  $\exists m : \mathbb{N}, (m : \mathbb{Z}) = -n$  := by
          use (-n).toNat
          <|> simp [Int.toNat_of_nonneg (by
            → linarith :  $(0 : \mathbb{Z}) \leq -n$ )]
        rcases h₁₁ with ⟨m, h₁₂⟩
        have h₁₃ :  $h₁ m$ 
        have h₁₄ :  $(m : \mathbb{Z}) = -n$  := by
          → exact_mod_cast h₁₃
        have h₁₅ :  $f(-(m : \mathbb{Z})) = (f 1 - f 0) * m$ 
          →  $-(f(m : \mathbb{Z})) + f 0 =$  by simp using h₁₅
        have h₁₆ :  $f n = (f 1 - f 0) * n + f 0$  := by
          have h₁₇ :  $n = -(m : \mathbb{Z})$  := by
            linarith
          rw [h₁₇]
          simp [h₁₆] using h₁₅
          exact h₁
        rcases h₁ with ⟨d, c, h₁⟩
        have h₁ :  $d = 0 \vee d = 2$  := by
          have h₂ :  $h 0 0$ 
          have h₃ :  $h 1 0$ 
          have h₄ :  $h 0 1$ 
          have h₅ :  $h 1 1$ 
          simp [h₁] at h₂ h₃ h₄ h₅
          ring_nf at h₂ h₃ h₄ h₅
          have h₁₀ :  $d = 0 \vee d = 2$  := by
            have h₁₁ :  $d * (d - 2) = 0$  := by
              nlinarith [sq_nonneg (d - 2), sq_nonneg
                → d, sq_nonneg (d + 2)]
            have h₁₂ :  $d = 0 \vee d - 2 = 0$  := by
              apply eq_zero_or_eq_zero_of_mul_eq_zero
              → h₁₁
            cases h₁₂ with
            | inl h₁₂ =>
              exact Or.inl h₁₂
            | inr h₁₂ =>
              have h₁₃ :  $d = 2$  := by linarith
              exact Or.inr h₁₃
          exact h₁₀
        cases h₁ with
        | inl h₁ =>
          have h₁ :  $\forall z, f z = 0$  := by
            intro z
            have h₂ :  $h z$ 
            have h₃ :  $h₁ z$ 
            rw [h₃] at h₂
            simp_all
            exact Or.inl h₂
          | inr h₁ =>
            have h₁ :  $\exists c, \forall z, f z = 2 * z + c$  := by
              use c
              intro z
              have h₂ :  $h z$ 
              rw [h₁] at h₂
              simp_all
              exact Or.inr h₂
            rintro (h | c, hc) <|> simp_all
            <|> intro a b <|> ring_nf <|> omega
            -----
            -- Orig Proof
            import Mathlib
            import Aesop
            set_option maxHeartbeats 0
            open BigOperators Real Nat Topology Rat
            theorem mathd_numbertheory_85 :
               $1 * 3^3 + 2 * 3^2 + 2 * 43 + 2 = 53$  := by
              have h :  $1 * 3^3 + 2 * 3^2 + 2 * 43 + 2 = 53$  := by
                norm_num
                <|> rfl
              exact h
            -- Simplified Proof
            import Mathlib
            import Aesop
            set_option maxHeartbeats 0
            open BigOperators Real Nat Topology Rat
            theorem mathd_numbertheory_85 :
               $1 * 3^3 + 2 * 3^2 + 2 * 43 + 2 = 53$  := by
              norm_num
              -----
              -- Orig Proof
              import Mathlib
              import Aesop
              set_option maxHeartbeats 0
              open BigOperators Real Nat Topology Rat
              theorem mathd_numbertheory_239 :
                ( $\exists k \in \text{Finset.Icc } 1 \ 12, k \ \% 4 = 2$ ) := by
                have h : ( $\exists k \in \text{Finset.Icc } 1 \ 12, k \ \% 4 = 2$ ) := by
                  norm_num [Finset.sum_succ_top]
                  <|> rfl
                apply h
              -- Simplified Proof
              import Mathlib
              import Aesop
              set_option maxHeartbeats 0
              open BigOperators Real Nat Topology Rat
              theorem mathd_numbertheory_239 :
                ( $\exists k \in \text{Finset.Icc } 1 \ 12, k \ \% 4 = 2$ ) := by
                rfl
              -----
              -- Orig Proof
              import Mathlib
              import Aesop
              set_option maxHeartbeats 0
              open BigOperators Real Nat Topology Rat
              theorem amc12b_2002_p2
                (x :  $\mathbb{Z}$ )
                (h₁ :  $x = 4$ ) :
                 $(3 * x - 2) * (4 * x + 1) - (3 * x - 2) * (4 * x - 2) + 1 = 11$  := by
                have h₁ :  $(3 * x - 2) * (4 * x + 1) - (3 * x - 2) * (4 * x - 2) + 1 = 11$  := by
                  rw [h₁]
                  norm_num
                  <|> ring_nf
                  <|> norm_num
                  <|> linarith
                exact h₁
              -- Simplified Proof
              import Mathlib
              import Aesop
              set_option maxHeartbeats 0
              open BigOperators Real Nat Topology Rat
              theorem amc12b_2002_p2
                (x :  $\mathbb{Z}$ )
                (h₁ :  $x = 4$ ) :
                 $(3 * x - 2) * (4 * x + 1) - (3 * x - 2) * (4 * x - 2) + 1 = 11$  := by
                simp_all
              -----
              -- Orig Proof
              import Mathlib
              import Aesop
              set_option maxHeartbeats 0
              open BigOperators Real Nat Topology Rat
              theorem mathd_algebra_196
                (S : Finset  $\mathbb{N}$ )
                (h₁ :  $\forall (x : \mathbb{N}), x \in S \leftrightarrow \text{abs}(2 - x) = 3$ ) :
                 $\exists k \in S, k = 4$  := by
                have :  $S = \{-1, 5\}$  := by
                  ext x
                  simp_all [abs_eq_max_neg]
                constructor
                · intro h
                  cases' max_eq_iff.mp h with h₁ h₂
                  · left
                    linarith
                  · right
                    linarith
                rintro (rfl | rfl) <|> norm_num
                simp_all
                norm_num
                -----
                -- Orig Proof
                import Mathlib
                import Aesop
                set_option maxHeartbeats 0
                open BigOperators Real Nat Topology Rat
                theorem mathd_algebra_342
                  (a d :  $\mathbb{N}$ )
                  (h₁ :  $\exists k \in (\text{Finset.range } 5), (a + k * d) = 70$ )
                  (h₂ :  $\exists k \in (\text{Finset.range } 10), (a + k * d) = 210$ ) :
                  a = 42/5 := by
                  have h₁ :  $5 * a + 10 * d = 70$  := by
                    norm_num [Finset.sum_range_succ,
                      → Finset.sum_range_succ,
                      → Finset.sum_range_succ] at h₁
                    <|> ring_nf at h₁
                    <|> linarith
                  have h₁ :  $10 * a + 45 * d = 210$  := by
                    norm_num [Finset.sum_range_succ] at h₁
                    <|> ring_nf at h₁
                    <|> linarith
                  have h₁ :  $d = 14 / 5$  := by
                    have h₁₀ :  $25 * d = 70$  := by
                      linarith
                    -- Solve for d by dividing both sides by 25
                    have h₁₁ :  $d = 14 / 5$  := by
                      linarith
                    exact h₁₁
                  have h₁ : a = 42 / 5 := by
                    have h₁₀ :  $5 * a + 10 * d = 70$  := h₁
                    rw [h₁] at h₁₀
                    ring_nf at h₁₀
                    linarith
                  apply h₁
              -- Simplified Proof
              import Mathlib
              import Aesop
              set_option maxHeartbeats 0
              open BigOperators Real Nat Topology Rat
              theorem mathd_algebra_342
                (a d :  $\mathbb{N}$ )
                (h₁ :  $\exists k \in (\text{Finset.range } 5), (a + k * d) = 70$ )

```



```

norm_num at h0 h1 <=>
linarith
exact h0 m
have h1 n : n = 502 := by
have h1 : a n = 2009 := h1
have h2 : a n = 1 + 4 * (n : ℝ) := by
have h2 := h1.general n
exact h2
rw [h1] at h1
have h3 : (1 : ℝ) + 4 * (n : ℝ) = 2009 := by
-- linarith
have h3 : (n : ℝ) = 502 := by
linarith
have h4 : n = 502 := by
norm_cast at h4 <=>
(trial linarith) <=>
(trial ring_nf at h4 <=> linarith)
exact h4

exact h1 n
-- Simplified Proof
import Mathlib
import Aesop

set_option maxHeartbeats 0

open BigOperators Real Nat Topology Rat

theorem amc12a_2009_p7
(x : ℝ)
(n : ℕ)
(a : ℕ → ℝ)
(h1 : ∀ m, a (m + 1) - a m = a (m + 2) - a (m + 1))
(h2 : a 1 = 2 * x - 3)
(h3 : a 2 = 5 * x - 11)
(h4 : a 3 = 3 * x + 1)
(h5 : a n = 2009) :
n = 502 := by
have h1.diff : ∀ m, a (m + 1) - a m = 4 := by
intro m
induction' m with m ih
· linarith [h1 0, h1 1, h1 2]
· linarith [h1 m, h1 (m + 1), h1 (m + 2)]
have h1.a0 : a 0 = 1 := by linarith [h1.diff 0,
-- h1.diff 1, h1.diff 2, h1 h1, h1]
have h1.general : ∀ m, a m = 1 + 4 * m := by
intro m
induction' m with m ih
· simp_all
· simp_all
linarith [h1.diff m]
rw [h1.general n] at h5
norm_cast at h5
linarith
-----
-- Orig Proof
import Mathlib
import Aesop

set_option maxHeartbeats 0

open BigOperators Real Nat Topology Rat

theorem mathd_numbertheory_521
(m n : ℕ)
(h1 : Even m)
(h2 : Even n)
(h3 : m - n = 2)
(h4 : m * n = 288) :
m = 18 := by
have h1 : m = n + 2 := by
by_contra h
-- Assume for contradiction that m < n + 2
have h1 : m ≤ n + 1 := by
omega
-- Since m ≤ n + 1, we have m - n ≤ 1
have h1 : m - n ≤ 1 := by
have h1 : m ≤ n + 1 := h1
have h1 : m - n ≤ 1 := by
omega
exact h1
-- But m - n = 2, which is a contradiction
omega
-- Now we know m ≥ n + 2, so we can write m = n
-- + 2 + k for some k ≥ 0
have h1 : m = n + 2 := by
have h1 : m ≥ n + 2 := h1
have h1 : m - n = 2 := h1
have h1 : m = n + 2 := by
have h1 : m ≥ n := by omega
have h1 : m - n = 2 := h1
have h1 : m = n + 2 := by
omega
omega
exact h1
exact h1
exact h1
have h1 : n = 16 := by
have h1 : (n + 1) ^ 2 = 289 := by
have h1 : m * n = 288 := h1
have h1 : m = n + 2 := h1
rw [h1] at h1
ring_nf at h1 <=>
linarith
have h1 : n + 1 = 17 := by
have h1 : (n + 1) ^ 2 = 289 := h1
have h1 : n + 1 = 17 := by
linarith
have h1 : n + 1 ≥ 1 := by
linarith
interval_cases n + 1 <=> norm_num at h1 <=>
<=> omega
have h1 : n = 16 := by
omega
omega

exact h1

have h1 : m = 18 := by
have h1 : m = n + 2 := h1
rw [h1]
<=> norm_num
exact h1

-- Simplified Proof
import Mathlib
import Aesop

set_option maxHeartbeats 0

open BigOperators Real Nat Topology Rat

theorem mathd_algebra_362
(a b : ℝ)
(h1 : Even m)
(h2 : Even n)
(h3 : m - n = 2)
(h4 : m * n = 288) :
m = 18 := by
have : m = n + 2 := by omega
linarith
-----
-- Orig Proof
import Mathlib
import Aesop

set_option maxHeartbeats 0

open BigOperators Real Nat Topology Rat

theorem mathd_algebra_362
(a b : ℝ)
(h1 : a ^ 2 * b ^ 3 = 32 / 27)
(h2 : a / b ^ 3 = 27 / 4) :
a + b = 8 / 3 := by
have h1 : a = (27 / 4 : ℝ) * b ^ 3 := by
have h1 : b ≠ 0 := by
by_contra h
rw [h] at h1
norm_num at h1
<=> simp_all [pow_three]
<=> ring_nf at h1 *
<=> nlinarith
-- Eliminate the denominator by multiplying
-- both sides by b^3
have h1 : a = (27 / 4 : ℝ) * b ^ 3 := by
field_simp [h1, pow_ne_zero] at h1 <=>
<=> ring_nf at h1 <=> nlinarith
exact h1
have h1 : ((27 / 4 : ℝ) * b ^ 3) ^ 2 * b ^ 3 = 32 / 27
-- := by
have h1 : a = (27 / 4 : ℝ) * b ^ 3 := h1
rw [h1] at h1
ring_nf at h1 <=>
<=>
(trial norm_num at h1 <=> <=>
(trial linarith) <=>
(trial nlinarith) <=>
(trial ring_nf at h1 <=> nlinarith) <=>
(trial field_simp at h1 <=> ring_nf at h1 <=> <=>
<=> nlinarith)
<=>
nlinarith
have h1 : b ^ 3 = 8 / 27 := by
have h1 : ((27 / 4 : ℝ) * b ^ 3) ^ 2 * b ^ 3 = 32 / 27 := h1
have h1 : (729 / 16 : ℝ) * (b ^ 3) ^ 3 = 32 / 27 :=
-- by
ring_nf at h1 <=>
<=> nlinarith
have h1 : (b ^ 3) ^ 3 = 512 / 19683 := by
ring_nf at h1 <=>
<=> nlinarith
have h1 : b ^ 3 = 8 / 27 := by
have h1 : (b ^ 3 - 8 / 27) * ((b ^ 3) ^ 2 + (8 / 27) * b ^ 3 + (64 / 729)) = 0 := by
nlinarith [sq_nonneg (b ^ 3 - 8 / 27),
-- sq_nonneg (b ^ 3 + 8 / 27)]
have h1 : (b ^ 3) ^ 2 + (8 / 27) * b ^ 3 + (64 / 729) > 0 := by
nlinarith [sq_nonneg (b ^ 3 + 4 / 27)]
have h1 : b ^ 3 - 8 / 27 = 0 := by
apply mul_left_cancel1 (show ((b ^ 3) ^ 2 + (8 / 27) * b ^ 3 + (64 / 729) : ℝ) ≠ 0 by
-- linarith)
nlinarith
nlinarith
exact h1
have h1 : b = 2 / 3 := by
have h1 : b ^ 3 = 8 / 27 := h1
have h1 : b = 2 / 3 := by
-- Use the fact that the cube root of 8/27 is
-- 2/3
have h1 : (b - 2 / 3) * (b ^ 2 + (2 / 3) * b +
-- 4 / 9) = 0 := by
nlinarith [sq_nonneg (b - 2 / 3),
-- sq_nonneg (b + 2 / 3)]
have h1 : b ^ 2 + (2 / 3) * b + 4 / 9 > 0 := by
nlinarith [sq_nonneg (b + 1 / 3)]
have h1 : b - 2 / 3 = 0 := by
apply mul_left_cancel1 (show (b ^ 2 + (2 / 3)
-- * b + 4 / 9 : ℝ) ≠ 0 by linarith)
nlinarith
nlinarith
exact h1
have h1 : a = 2 := by
have h1 : a = (27 / 4 : ℝ) * b ^ 3 := h1

```



```

      exact h10
    exact h11
  have h12 : a ^ 2 + 1 / a ^ 2 = 3 := by
    have h12 : (a - 1 / a) ^ 2 = 1 := h12
    have h12 : a ≠ 0 := by linarith
    field_simp [h12] at h12 ⊢
    nlinarith
  have h13 : (a + 1 / a) ^ 2 = 5 := by
    have h13 : a ≠ 0 := by linarith
    have h13 : a ^ 2 + 1 / a ^ 2 = 3 := h13
    field_simp [h13] at h13 ⊢
    nlinarith
  have h14 : a + 1 / a > 0 := by
    have h14 : 0 < a := h14.1
    have h14 : 0 < 1 / a := by positivity
    linarith
  have h15 : a + 1 / a = Real.sqrt 5 := by
    have h15 : (a + 1 / a) ^ 2 = 5 := h15
    have h15 : a + 1 / a > 0 := h15
    have h15 : Real.sqrt 5 > 0 :=
      → Real.sqrt_pos.mpr (by norm_num)
    nlinarith [Real.sq_sqrt (show 0 ≤ 5 by
      → norm_num),
      Real.sqrt_nonneg 5]
  exact h15

have h16 : b + 1 / b = Real.sqrt 5 := by
  have h16 : 0 < b := h16.2
  have h16 : (b - 1 / b) ^ 2 = 1 := by
    have h16 : abs (b - 1 / b) = 1 := h16
    have h16 : (b - 1 / b) ^ 2 = 1 := by
      have h16 : abs (b - 1 / b) = 1 := h16
      have h16 : (b - 1 / b) ^ 2 = 1 := by
        cases' abs_cases (b - 1 / b) with h16 h17
        → <|>
      nlinarith
    exact h16
  exact h16
  have h16 : b ^ 2 + 1 / b ^ 2 = 3 := by
    have h16 : (b - 1 / b) ^ 2 = 1 := h16
    have h16 : b ≠ 0 := by linarith
    field_simp [h16] at h16 ⊢
    nlinarith
  have h16 : (b + 1 / b) ^ 2 = 5 := by
    have h16 : b ≠ 0 := by linarith
    have h16 : b ^ 2 + 1 / b ^ 2 = 3 := h16
    field_simp [h16] at h16 ⊢
    nlinarith
  have h16 : b + 1 / b > 0 := by
    have h16 : 0 < b := h16.2
    have h16 : 0 < 1 / b := by positivity
    linarith
  have h16 : b + 1 / b = Real.sqrt 5 := by
    have h16 : (b + 1 / b) ^ 2 = 5 := h16
    have h16 : b + 1 / b > 0 := h16
    have h16 : Real.sqrt 5 > 0 :=
      → Real.sqrt_pos.mpr (by norm_num)
    nlinarith [Real.sq_sqrt (show 0 ≤ 5 by
      → norm_num),
      Real.sqrt_nonneg 5]
  exact h16

have h17 : a * b = 1 := by
  have h17 : a + 1 / a = b + 1 / b := by
    linarith
  have h17 : a ≠ b := h17
  have h17 : 0 < a := h17.1
  have h17 : 0 < b := h17.2
  have h17 : 0 < a * b := by positivity
  field_simp [h17.ne', h17.ne'] at h17
  ring_nf at h17
  have h17 : (a - b) * (a * b - 1) = 0 := by
    nlinarith
  have h17 : a - b ≠ 0 := by
    intro h
    apply h17
    linarith
  have h17 : a * b - 1 = 0 := by
    apply mul_left_cancel. h17
    nlinarith
  nlinarith

have h18 : a + b = Real.sqrt 5 := by
  have h18 : 0 < a := h18.1
  have h18 : 0 < b := h18.2
  have h18 : a * b = 1 := h18
  have h18 : a + 1 / a = Real.sqrt 5 := h18
  have h18 : 1 / a = b := by
    have h18 : a ≠ 0 := by linarith
    have h18 : b = 1 / a := by
      field_simp [h18] at h18 ⊢
      nlinarith
    linarith
  have h18 : a + b = Real.sqrt 5 := by
    calc
      a + b = a + 1 / a := by rw [h18.1]
      = Real.sqrt 5 := by rw [h18.1]
  exact h18

apply h

-- Simplified Proof
import Mathlib
import Aesop

set_option maxHeartbeats 0

open BigOperators Real Nat Topology Rat

theorem amc12a_2002_p13
  (a b : ℝ)
  (h1 : 0 < a ∧ 0 < b)
  (h2 : a ≠ b)
  (h3 : abs (a - 1/a) = 1)
  (h4 : abs (b - 1/b) = 1) :
  a + b = Real.sqrt 5 := by
    rcases h1 with ha hb
    have h1 : a + 1 / a = Real.sqrt 5 := by
      have h1 : (a - 1 / a) ^ 2 = 1 := by
        cases' abs_cases (a - 1 / a) with h1 h1 <|>
        → nlinarith
      have h1 : a ^ 2 + 1 / a ^ 2 = 3 := by
        field_simp [ha.ne'] at h1 ⊢
        nlinarith
      have h1 : (a + 1 / a) ^ 2 = 5 := by
        field_simp [ha.ne'] at h1 ⊢
        nlinarith
      have h1 : a + 1 / a > 0 := by positivity
      nlinarith [Real.sq_sqrt (show 0 ≤ 5 by
        → norm_num),
        Real.sqrt_nonneg 5]
    have h1 : b + 1 / b = Real.sqrt 5 := by
      have h1 : (b - 1 / b) ^ 2 = 1 := by
        cases' abs_cases (b - 1 / b) with h1 h1 <|>
        → nlinarith
      have h1 : b ^ 2 + 1 / b ^ 2 = 3 := by
        field_simp [hb.ne'] at h1 ⊢
        nlinarith
      have h1 : (b + 1 / b) ^ 2 = 5 := by
        field_simp [hb.ne'] at h1 ⊢
        nlinarith
      have h1 : b + 1 / b > 0 := by positivity
      nlinarith [Real.sq_sqrt (show 0 ≤ 5 by
        → norm_num),
        Real.sqrt_nonneg 5]
    have h1 : a * b = 1 := by
      have h1 : a + 1 / a = b + 1 / b := by linarith
      have h1 : a ≠ b := h1
      have h1 : 0 < a := h1.1
      have h1 : 0 < b := h1.2
      have h1 : 0 < a * b := by positivity
      field_simp [h1.ne', h1.ne'] at h1
      ring_nf at h1
      have h1 : (a - b) * (a * b - 1) = 0 := by
        nlinarith
      have h1 : a - b ≠ 0 := by
        intro h
        apply h1
        linarith
      have h1 : a * b - 1 = 0 := by
        apply mul_left_cancel. h1
        nlinarith
      nlinarith
    have h1 : a + b = Real.sqrt 5 := by
      have h1 : 0 < a := h1.1
      have h1 : 0 < b := h1.2
      have h1 : a * b = 1 := h1
      have h1 : a + 1 / a = Real.sqrt 5 := h1
      have h1 : 1 / a = b := by
        have h1 : a ≠ 0 := by linarith
        have h1 : b = 1 / a := by
          field_simp [h1] at h1 ⊢
          nlinarith
        linarith
      have h1 : a + b = Real.sqrt 5 := by
        calc
          a + b = a + 1 / a := by rw [h1.1]
          = Real.sqrt 5 := by rw [h1.1]
      exact h1

-- Simplified Proof
import Mathlib
import Aesop

set_option maxHeartbeats 0

open BigOperators Real Nat Topology Rat

theorem amc12a_2021_p3
  (x y : ℕ)
  (h1 : x + y = 17402)
  (h2 : 10 | x)
  (h3 : x / 10 = y) :
  x - y = (14238 : ℤ) := by
    have h1 : x = 10 * y := by
      have h1 : x / 10 = y := h1
      have h1 : 10 | x := h1
      have h1 : x = 10 * (x / 10) := by
        have h1 : 10 * (x / 10) = x := by
          have h1 : 10 * (x / 10) = x := by
            apply Nat.mul_div_cancel'
            exact h1
          exact h1
        linarith
      rw [h1] at h1
      <|> ring_nf at h1 ⊢ <|> linarith
    have h1 : y = 1582 := by
      have h1 : x + y = 17402 := h1
      have h1 : x = 10 * y := h1
      rw [h1] at h1
      ring_nf at h1 ⊢
      omega
    have h1 : x = 15820 := by
      have h1 : x = 10 * y := h1
      have h1 : y = 1582 := h1
      rw [h1] at h1
      <|> norm_num at h1 ⊢ <|> linarith
    have h1 : (x : ℤ) - (y : ℤ) = (14238 : ℤ) := by
      have h1 : y = 1582 := h1
      have h1 : x = 15820 := h1
      rw [h1, h1]
      <|> norm_num
      <|> simp [Int.ofNat_sub]
      <|> norm_num
    exact h1

-- Simplified Proof
import Mathlib
import Aesop

set_option maxHeartbeats 0

open BigOperators Real Nat Topology Rat

theorem amc12a_2021_p3
  (x y : ℕ)
  (h1 : x + y = 17402)
  (h2 : 10 | x)
  (h3 : x / 10 = y) :
  x - y = (14238 : ℤ) := by
    omega

-- Orig Proof
import Mathlib
import Aesop

set_option maxHeartbeats 0

open BigOperators Real Nat Topology Rat

theorem aime_1990_p15
  (a b x y : ℝ)
  (h1 : a * x + b * y = 3)
  (h2 : a * x^2 + b * y^2 = 7)
  (h3 : a * x^3 + b * y^3 = 16)

```





```

have h₂ : Real.log 6 = Real.log 2 + Real.log 3 := h_log6
rw [h]
have h₃ : Real.log 2 > 0 := Real.log_pos (by
  norm_num)
have h₄ : Real.log 3 > 0 := Real.log_pos (by
  norm_num)
field_simp [h.ne', h.ne']
<> ring_nf
<> field_simp [h.ne', h.ne']
<> ring
<> field_simp [h.ne', h.ne']
<> linarith
rw [h]
have h₅ : 2 + Real.log 3 / Real.log 2 +
  Real.log 2 / Real.log 3 ≥ 0 := by
have h₆ : Real.log 2 > 0 := Real.log_pos (by
  norm_num)
have h₇ : Real.log 3 > 0 := Real.log_pos (by
  norm_num)
have h₈ : Real.log 3 / Real.log 2 > 0 :=
  div_pos h₆ h₇
have h₉ : Real.log 2 / Real.log 3 > 0 :=
  div_pos h₆ h₇
linarith
rw [Real.sqrt] <> linarith

have h_rhs_squared : (Real.sqrt (Real.log 3 /
  Real.log 2) + Real.sqrt (Real.log 2 /
  Real.log 3)) ^ 2 = 2 + Real.log 3 /
  Real.log 2 + Real.log 2 / Real.log 3 := by
have h₁₀ : Real.log 2 > 0 := Real.log_pos (by
  norm_num)
have h₁₁ : Real.log 3 / Real.log 2 > 0 :=
  div_pos h₆ h₇
have h₁₂ : Real.log 2 / Real.log 3 > 0 :=
  div_pos h₆ h₇
have h₁₃ : Real.sqrt (Real.log 3 / Real.log 2) ≥
  0 := Real.sqrt_nonneg _
have h₁₄ : Real.sqrt (Real.log 2 / Real.log 3) ≥
  0 := Real.sqrt_nonneg _
have h₁₅ : Real.sqrt (Real.log 3 / Real.log 2) *
  Real.sqrt (Real.log 2 / Real.log 3) = 1 :=
  by
have h₁₆ : Real.sqrt (Real.log 3 / Real.log
  2) * Real.sqrt (Real.log 2 / Real.log 3) =
  Real.sqrt ((Real.log 3 / Real.log 2) *
  (Real.log 2 / Real.log 3)) := by
  rw [- Real.sqrt_mul] <> positivity
rw [h₁₆]
have h₁₇ : (Real.log 3 / Real.log 2) *
  (Real.log 2 / Real.log 3) = 1 := by
  field_simp [h.ne', h.ne']
<> ring_nf
<> field_simp [h.ne', h.ne']
<> linarith
rw [h₁₇]
<> simp [Real.sqrt_one]
calc
(Real.sqrt (Real.log 3 / Real.log 2) +
  Real.sqrt (Real.log 2 / Real.log 3)) ^ 2 =
  (Real.sqrt (Real.log 3 / Real.log 2)) ^
  2 + (Real.sqrt (Real.log 2 / Real.log 3))
  ^ 2 +
  2 * (Real.sqrt (Real.log 3 / Real.log
  2) * Real.sqrt (Real.log 2 / Real.log 3))
  := by
  ring_nf
<>
  nlinarith [Real.sqrt_nonneg (Real.log 3 /
  Real.log 2), Real.sqrt_nonneg (Real.log 2
  / Real.log 3)]
  = (Real.log 3 / Real.log 2) + (Real.log 2
  / Real.log 3) + 2 * (Real.sqrt (Real.log
  3 / Real.log 2) * Real.sqrt (Real.log 2 /
  Real.log 3)) := by
have h₁₈ : (Real.sqrt (Real.log 3 / Real.log
  2)) ^ 2 = Real.log 3 / Real.log 2 := by
  rw [Real.sqrt_sq] (by positivity)]
have h₁₉ : (Real.sqrt (Real.log 2 / Real.log
  3)) ^ 2 = Real.log 2 / Real.log 3 := by
  rw [Real.sqrt_sq] (by positivity)]
rw [h₁₈, h₁₉]
  = (Real.log 3 / Real.log 2) + (Real.log 2
  / Real.log 3) + 2 * 1 := by
  rw [h]
<> ring_nf
  = 2 + Real.log 3 / Real.log 2 + Real.log 2
  / Real.log 3 := by ring

have h_pos_lhs : Real.sqrt (Real.log 6 /
  Real.log 2 + Real.log 6 / Real.log 3) ≥ 0
:= by
  apply Real.sqrt_nonneg

have h_pos_rhs : Real.sqrt (Real.log 3 /
  Real.log 2) + Real.sqrt (Real.log 2 /
  Real.log 3) ≥ 0 := by
have h₂₀ : Real.sqrt (Real.log 3 / Real.log 2) ≥
  0 := Real.sqrt_nonneg _
have h₂₁ : Real.sqrt (Real.log 2 / Real.log 3) ≥
  0 := Real.sqrt_nonneg _
linarith

have h_main : Real.sqrt (Real.log 6 / Real.log 2 +
  Real.log 6 / Real.log 3) = Real.sqrt
  (Real.log 3 / Real.log 2) * Real.sqrt
  (Real.log 2 / Real.log 3) := by
have h₂₂ : (Real.sqrt (Real.log 6 / Real.log 2 +
  Real.log 6 / Real.log 3)) ^ 2 =
  (Real.sqrt (Real.log 3 / Real.log 2) *
  Real.sqrt (Real.log 2 / Real.log 3)) ^ 2 :=
  by
  rw [Real.sqrt_sq]
  = (Real.log 6 / Real.log 2 + Real.log 6 /
  Real.log 3) := by ring

-- Simplified Proof
import Mathlib
import Aesop

set_option maxHeartbeats 0

open BigOperators Real Nat Topology Rat

theorem mathd_numbertheory_222
  (b : ℕ)
  (h₁ : Nat.lcm 120 b = 3720)
  (h₂ : Nat.gcd 120 b = 8) :
  b = 248 := by
  have := Nat.gcd_mul_lcm 120 b
  nlinarith

-- Orig Proof
import Mathlib
import Aesop

set_option maxHeartbeats 0

open BigOperators Real Nat Topology Rat

theorem numbertheory_addbdivaasqpsqmqd8eq1
  (a : ℤ)
  (b : ℤ)
  (h₁ : Odd a)
  (h₂ : 4 ∣ b)
  (h₃ : b >= 0) :
  (a^2 + b^2) % 8 = 1 := by
  have h₄ : a^2 % 8 = 1 := by
  have h₅ : a % 8 = 1 ∨ a % 8 = 3 ∨ a % 8 = 5 ∨ a
    % 8 = 7 := by
  have h₆ : a % 2 = 1 := by
  cases' h₅ with k hk
  omega
  have h₇ : a % 8 = 1 ∨ a % 8 = 3 ∨ a % 8 = 5 ∨
    a % 8 = 7 := by
  have : a % 8 = 1 ∨ a % 8 = 3 ∨ a % 8 = 5 ∨
    a % 8 = 7 := by
  omega
  exact this
  exact h₅
  have h₈ : a ^ 2 % 8 = 1 := by
  rcases h₈ with (h₈₁ | h₈₂ | h₈₃ | h₈₄)
  -- Case: a = 1 mod 8
  have h₈₅ : a % 8 = 1 := h₈₁
  have h₈₆ : a ^ 2 % 8 = 1 := by
  have : a % 8 = 1 := h₈₅
  have : a ^ 2 % 8 = 1 := by
  norm_num [pow_two, Int.mul_emod, this]
  exact this
  exact h₈
  -- Case: a = 3 mod 8
  have h₈₇ : a % 8 = 3 := h₈₂
  have h₈₈ : a ^ 2 % 8 = 1 := by
  have : a % 8 = 3 := h₈₇
  have : a ^ 2 % 8 = 1 := by
  norm_num [pow_two, Int.mul_emod, this]
  exact this
  exact h₈
  -- Case: a = 5 mod 8
  have h₈₉ : a % 8 = 5 := h₈₃
  have h₉₀ : a ^ 2 % 8 = 1 := by
  have : a % 8 = 5 := h₈₉
  have : a ^ 2 % 8 = 1 := by
  norm_num [pow_two, Int.mul_emod, this]
  exact this
  exact h₈
  -- Case: a = 7 mod 8
  have h₉₁ : a % 8 = 7 := h₈₄
  have h₉₂ : a ^ 2 % 8 = 1 := by
  have : a % 8 = 7 := h₉₁
  have : a ^ 2 % 8 = 1 := by
  norm_num [pow_two, Int.mul_emod, this]
  exact this
  exact h₈
  exact h₈
  have h₉ : b^2 % 8 = 0 := by
  have h₉₃ : (4 : ℤ) ∣ b := h₂
  have h₉₄ : ∃ (m : ℤ), b = 4 * m := by
  obtain (m, hm) := h₉₃
  exact (m, by linarith)
  obtain (m, hm) := h₉₃
  have h₉₅ : b ^ 2 = 16 * m ^ 2 := by
  rw [hm]
  ring
  <> norm_num
  <> linarith
  have h₉₆ : b ^ 2 % 8 = 0 := by
  rw [h₉₅]
  have h₉₇ : (16 * m ^ 2 : ℤ) % 8 = 0 := by
  have h₉₈ : (16 : ℤ) % 8 = 0 := by norm_num
  have h₉₉ : (16 * m ^ 2 : ℤ) % 8 = 0 := by
  simp [h₉₇, Int.mul_emod, pow_two]
  <> norm_num
  <> ring_nf at *
  <> omega
  exact h₉₇
  exact h₉₈
  exact h₉₉
  have h₁₀ : (a^2 + b^2) % 8 = 1 := by
  have h₁₀₁ : (a ^ 2 + b ^ 2) % 8 = (a ^ 2 % 8 + b
    ^ 2 % 8) % 8 := by

```



```

ring
-----
-- Orig Proof
import Mathlib
import Aesop

set_option maxHeartbeats 0

open BigOperators Real Nat Topology Rat

theorem mathd_algebra_158
  (a : ℕ)
  (h₁ : Even a)
  (h₂ : ∑ k ∈ Finset.range 8, (2 * k + 1 : ℤ) - ∑ k ∈
    → Finset.range 5, (a + 2 * k : ℤ) = (4:ℤ))
  → :
a = 8 := by
have h_sum1 : (∑ k ∈ Finset.range 8, (2 * k + 1 :
  → ℤ)) = 64 := by
  norm_num [Finset.sum_range_succ,
    → Finset.sum_range_succ,
    → Finset.sum_range_succ]
<|> rfl

have h_sum2 : (∑ k ∈ Finset.range 5, (a + 2 * k :
  → ℤ)) = (5 * a + 20 : ℤ) := by
simp [Finset.sum_range_succ,
  → Finset.sum_range_succ,
  → Finset.sum_range_succ,
  → Finset.sum_range_succ]
<|> ring_nf
<|> norm_cast
<|> simp [mul_add, add_mul, mul_comm,
  → mul_left_comm, mul_assoc]
<|> ring_nf at *
<|> norm_cast at *
<|> omega

have h_main : (64 : ℤ) - (5 * a + 20 : ℤ) = 4 :=
  by
  have h₁ : (∑ k ∈ Finset.range 8, (2 * k + 1 : ℤ)
    → ) - ∑ k ∈ Finset.range 5, (a + 2 * k : ℤ
    → ) = (4 : ℤ) := h₁
  rw [h_sum1] at h₁
  rw [h_sum2] at h₁
  ring_nf at h₁
  <|> linarith

have h_a : a = 8 := by
have h₁ : (64 : ℤ) - (5 * a + 20 : ℤ) = 4 :=
  → h_main
have h₂ : (a : ℤ) = 8 := by
  linarith
have h₃ : a = 8 := by
  norm_cast at h₁
  <|> omega
exact h₃

exact h_a

-- Simplified Proof
import Mathlib
import Aesop

set_option maxHeartbeats 0

open BigOperators Real Nat Topology Rat

theorem mathd_algebra_158
  (a : ℕ)
  (h₁ : Even a)
  (h₂ : ∑ k ∈ Finset.range 8, (2 * k + 1 : ℤ) - ∑ k ∈
    → Finset.range 5, (a + 2 * k : ℤ) = (4:ℤ))
  → :
a = 8 := by
simp_all [Finset.sum_range_succ]
linarith
-----
-- Orig Proof
import Mathlib
import Aesop

set_option maxHeartbeats 0

open BigOperators Real Nat Topology Rat

theorem aime_1991_p9
  (x : ℝ)
  (m : ℚ)
  (h₁ : 1 / Real.cos x + Real.tan x = 22 / 7)
  (h₂ : 1 / Real.sin x + 1 / Real.tan x = m) :
  m.den + m.num = 44 := by
have h_cos_ne_zero : Real.cos x ≠ 0 := by
  by_contra h
  have h₁ : Real.cos x = 0 := by simpa using h
  have h₂ : 1 / Real.cos x + Real.tan x = 0 := by
    have h₃ : 1 / Real.cos x = 0 := by
      rw [h₁]
      simp
    have h₄ : Real.tan x = 0 := by
      rw [Real.tan_eq_sin_div_cos]
      rw [h₁]
      simp
    linarith
  rw [h₁] at h₂
  norm_num at h₂
  <|> linarith

have h_sin_ne_zero : Real.sin x ≠ 0 := by
  by_contra h
  have h₁ : Real.sin x = 0 := by simpa using h
  have h₂ : Real.tan x = 0 := by
    have h₃ : Real.tan_eq_sin_div_cos]
    rw [h₁]
    simp
  have h₄ : 1 / Real.cos x + Real.tan x = 1 /
    → Real.cos x := by
    rw [h₁]
    <|> ring_nf

<|> simp [h_cos_ne_zero]
<|> field_simp [h_cos_ne_zero]
<|> ring_nf
  rw [h₁] at h₂
  have h₃ : 1 / Real.cos x = 22 / 7 := by linarith
  have h₄ : Real.cos x = 7 / 22 := by
    have h₅ : Real.cos x ≠ 0 := h_cos_ne_zero
    have h₆ : 1 / Real.cos x = 22 / 7 := h₃
    have h₇ : Real.cos x = 7 / 22 := by
      field_simp at h₆
      <|> nlinarith [Real.sin_sq_add_cos_sq x]
    exact h₇
  have h₈ : Real.sin x ^ 2 + Real.cos x ^ 2 = 1 :=
    → by
  have h₉ : Real.cos x = 7 / 22 := by
    rw [h₁, h₈] at h₉
    norm_num at h₉
    <|> linarith
  have h_main_eq : 7 * (1 + Real.sin x) = 22 *
    → Real.cos x := by
    have h₁₀ : 1 / Real.cos x + Real.tan x = 22 / 7
      → := h₃
    have h₁₁ : Real.tan x = Real.sin x / Real.cos x
      → := by
    rw [Real.tan_eq_sin_div_cos]
  rw [h₁] at h₁
  have h₁₂ : 1 / Real.cos x + Real.sin x /
    → Real.cos x = 22 / 7 := by
    linarith
  have h₁₃ : (1 + Real.sin x) / Real.cos x = 22 /
    → 7 := by
    have h₁₄ : 1 / Real.cos x + Real.sin x /
      → Real.cos x = (1 + Real.sin x) / Real.cos
      → x := by
    field_simp [h_cos_ne_zero]
    <|> ring_nf
  rw [h₁₃] at h₁
  linarith
  have h₁₅ : 7 * (1 + Real.sin x) = 22 * Real.cos
    → x := by
    have h₁₆ : (1 + Real.sin x) / Real.cos x = 22
      → / 7 := h₁₄
    have h₁₇ : Real.cos x ≠ 0 := h_cos_ne_zero
    field_simp at h₁₆
    <|> nlinarith [Real.sin_sq_add_cos_sq x]
  exact h₁₇

have h_sin_value : Real.sin x = 435 / 533 := by
have h₁ : 7 * (1 + Real.sin x) = 22 * Real.cos
  → x := h_main_eq
have h₂ : Real.sin x ^ 2 + Real.cos x ^ 2 = 1 :=
  → by
  rw [Real.sin_sq_add_cos_sq]
have h₃ : 533 * Real.sin x ^ 2 + 98 * Real.sin
  → x - 435 = 0 := by
  have h₄ : Real.cos x = (7 * (1 + Real.sin x))
    → / 22 := by
    have h₅ : 7 * (1 + Real.sin x) = 22 *
      → Real.cos x := h_main_eq
    linarith
  rw [h₁] at h₄
  ring_nf at h₄
  nlinarith [Real.sin_le_one x,
    → Real.cos_le_one x, sq_nonneg (Real.sin x
    → - 435 / 533)]
have h₆ : Real.sin x = 435 / 533 := by
have h₇ : Real.sin x = 435 / 533 ∨ Real.sin
  → x = -1 := by
  apply or_iff_not_imp_left.mpr
  intro h₈
  apply mul_left_cancel₃ (sub_ne_zero.mpr h₈)
  nlinarith [Real.sin_le_one x,
    → Real.cos_le_one x]
cases h₈ with
| inl h₈ =>
  exact h₈
| inr h₈ =>
  have h₉ : Real.sin x = -1 := h₈
  have h₁₀ : Real.cos x = 0 := by
    have h₁₁ : 7 * (1 + Real.sin x) = 22 *
      → Real.cos x := h_main_eq
    rw [h₁] at h₁₁
    nlinarith
  exact absurd h₁₀ h_cos_ne_zero
exact h₆

have h_cos_value : Real.cos x = 308 / 533 := by
have h₁ : 7 * (1 + Real.sin x) = 22 * Real.cos
  → x := h_main_eq
have h₂ : Real.sin x = 435 / 533 := h_sin_value
  rw [h₁] at h₂
have h₃ : 7 * (1 + (435 / 533 : ℝ)) = 22 *
  → Real.cos x := by
  exact_mod_cast h₂
have h₄ : Real.cos x = 308 / 533 := by
  ring_nf at h₃
  linarith
exact h₄

have h_m_value : (m : ℝ) = 29 / 15 := by
have h₁ : 1 / Real.sin x + 1 / Real.tan x = (m
  → : ℝ) := by
  exact_mod_cast h₁
have h₂ : Real.sin x = 435 / 533 := h_sin_value
have h₃ : Real.cos x = 308 / 533 := h_cos_value
have h₄ : Real.tan x = Real.sin x / Real.cos x
  → := by
  rw [Real.tan_eq_sin_div_cos]
have h₅ : 1 / Real.sin x + 1 / Real.tan x = (1
  → : ℝ) / Real.sin x + Real.cos x / Real.sin
  → x := by

have h₃ : Real.tan x = Real.sin x / Real.cos
  → x := by
  rw [Real.tan_eq_sin_div_cos]
  rw [h₁]
  simp
have h₄ : 1 / Real.cos x + Real.tan x = 1 /
  → Real.cos x := by
  rw [h₁]

```

```

<> ring_nf
rw [h1] at h1
have h1 : 1 / Real.cos x = 22 / 7 := by linarith
have h1 : Real.cos x = 7 / 22 := by
  have h1 : Real.cos x ≠ 0 := h1.cos_ne_zero
  have h1 : 1 / Real.cos x = 22 / 7 := h1
  have h1 : Real.cos x = 7 / 22 := by
    field_simp at h1
    <> nlinarith [Real.sin_sq_add_cos_sq x]
  exact h1
have h1 : Real.sin x ^ 2 + Real.cos x ^ 2 = 1 :=
  by
    rw [Real.sin_sq_add_cos_sq]
    rw [h1, h1] at h1
    norm_num at h1
have h1.main_eq : 7 * (1 + Real.sin x) = 22 *
  by
    have h1 : 1 / Real.cos x + Real.tan x = 22 / 7
    := h1
    have h1 : Real.tan x = Real.sin x / Real.cos x
    := by
      rw [Real.tan_eq_sin_div_cos]
      field_simp at h1
      linarith [Real.sin_sq_add_cos_sq x]
    have h1.sin_value : Real.sin x = 435 / 533 := by
      have h1 : 7 * (1 + Real.sin x) = 22 * Real.cos
      := x := h1.main_eq
      have h1 : Real.sin x ^ 2 + Real.cos x ^ 2 = 1 :=
      by
        rw [Real.sin_sq_add_cos_sq]
      have h1 : 533 * Real.sin x ^ 2 + 98 * Real.sin
      x - 435 = 0 := by
        have h1 : Real.cos x = (7 * (1 + Real.sin x))
        := / 22 := by
          have h1 : 7 * (1 + Real.sin x) = 22 *
          := Real.cos x := h1.main_eq
          linarith
        rw [h1] at h1
        ring_nf at h1
        nlinarith [Real.sin_le_one x,
          := Real.cos_le_one x, sq_nonneg (Real.sin x
          := - 435 / 533)]
      have h1 : Real.sin x = 435 / 533 := by
      have h1 : Real.sin x = 435 / 533 ∨ Real.sin
      := x = -1 := by
        apply or_iff_not_imp_left.mpr
        intro h1
        apply mul_left_cancel. (sub_ne_zero.mpr h1)
        nlinarith [Real.sin_le_one x,
          := Real.cos_le_one x]
      cases h1 with
      | inl h1 =>
        exact h1
      | inr h1 =>
        have h1 : Real.sin x = -1 := h1
        have h1 : Real.cos x = 0 := by
          have h1 : 7 * (1 + Real.sin x) = 22 *
          := Real.cos x := h1.main_eq
          rw [h1] at h1
          nlinarith
        exact absurd h1.cos_ne_zero
    exact h1
have h1.cos_value : Real.cos x = 308 / 533 := by
  have h1 : 7 * (1 + Real.sin x) = 22 * Real.cos
  := x := h1.main_eq
  have h1 : Real.sin x = 435 / 533 := h1.sin_value
  rw [h1] at h1
  ring_nf at h1
  linarith
have h1.value : (m : ℝ) = 29 / 15 := by
  have h1 : 1 / Real.sin x + 1 / Real.tan x = (m
  := : ℝ) := by
    exact_mod_cast h1
  have h1 : Real.sin x = 435 / 533 := h1.sin_value
  have h1 : Real.cos x = 308 / 533 := h1.cos_value
  have h1 : Real.tan x = Real.sin x / Real.cos x
  := by
    rw [Real.tan_eq_sin_div_cos]
  rw [h1] at h1
  have h1 : 1 / Real.sin x + 1 / (Real.sin x /
  := Real.cos x) = (1 + Real.cos x) / Real.sin
  := x := by
    field_simp [h1.sin_ne_zero, h1.cos_ne_zero]
  rw [h1] at h1
  have h1 : (1 + Real.cos x) / Real.sin x = (m : ℝ
  := : ℝ) := by linarith
  have h1 : Real.sin x = 435 / 533 := h1.sin_value
  have h1 : Real.cos x = 308 / 533 := h1.cos_value
  rw [h1, h1] at h1
  norm_num at h1
  <> (try norm_num at h1) <> (try linarith)
  have h1.eq : m = 29 / 15 := by
    have h1 : (m : ℝ) = 29 / 15 := h1.value
    norm_cast at h1
    <> (try norm_num at h1) <> (try field_simp
    := at h1) <> (try norm_cast at h1)
  have h1.final : m.den + m.num = 44 := by
    rw [h1.eq]
    norm_num [Rat.num_div_den]
  exact h1.final
-- Orig Proof
import Mathlib
import Aesop

set_option maxHeartbeats 0

open BigOperators Real Nat Topology Rat

theorem aime_1990_p4
  (x : ℝ)
  (h1 : 0 < x)
  (h1 : x^2 - 10 * x - 29 ≠ 0)
  (h1 : x^2 - 10 * x - 45 ≠ 0)
  (h1 : 1 / (x^2 - 10 * x - 29) + 1 / (x^2 - 10 * x
  := - 45) - 2 / (x^2 - 10 * x - 69) = 0) :
  x = 13 := by
  have h1.y : x^2 - 10 * x = 39 := by
    have h1 : x^2 - 10 * x - 29 ≠ 0 := h1
    have h1 : x^2 - 10 * x - 45 ≠ 0 := h1
    have h1 : x^2 - 10 * x - 69 ≠ 0 := h1
    have h1 : 1 / (x^2 - 10 * x - 29) + 1 / (x^2 -
    := 10 * x - 45) - 2 / (x^2 - 10 * x - 69) =
    := 0 := h1
    have h1 : (x^2 - 10 * x - 45) * (x^2 - 10 * x -
    := 69) + (x^2 - 10 * x - 29) * (x^2 - 10 * x
    := - 69) - 2 * (x^2 - 10 * x - 29) * (x^2 -
    := 10 * x - 45) = 0 := by
      have h1 : (x^2 - 10 * x - 29) ≠ 0 := by
        intro h
        apply h1
        linarith
      have h1 : (x^2 - 10 * x - 45) ≠ 0 := by
        intro h
        apply h1
        linarith
      have h1 : (x^2 - 10 * x - 69) ≠ 0 := by
        intro h
        apply h1
        linarith
      field_simp [h1, h1, h1, sub_eq_zero,
        := add_eq_zero_iff_eq_neg] at h1
      nlinarith [sq_pos_of_pos h1]
    have h1.y : (x^2 - 10 * x) = 39 := by
      nlinarith [sq_pos_of_pos h1]
    linarith
  have h1.main : x = 13 ∨ x = -3 := by
  have h1 : x^2 - 10 * x - 39 = 0 := by
    nlinarith
  have h1 : (x - 13) * (x + 3) = 0 := by
    nlinarith
  have h1 : x - 13 = 0 ∨ x + 3 = 0 := by
    apply eq_zero_or_eq_zero_of_mul_eq_zero h1
  cases h1 with
  | inl h1 =>
    have h1 : x = 13 := by linarith
    exact Or.inl h1
  | inr h1 =>
    have h1 : x = -3 := by linarith
    exact Or.inr h1
  have h1.x_pos : x = 13 := by
    cases h1.main with
    | inl h1.main =>
      exact h1.main
    | inr h1.main =>
      have h1 : x = -3 := h1.main
      have h1 : 0 < x := h1
      rw [h1] at h1
      norm_num at h1
      <> linarith
  exact h1.x_pos
-- Simplified Proof
import Mathlib
import Aesop

set_option maxHeartbeats 0

open BigOperators Real Nat Topology Rat

theorem aime_1990_p4
  (x : ℝ)
  (h1 : 0 < x)
  (h1 : x^2 - 10 * x - 29 ≠ 0)
  (h1 : x^2 - 10 * x - 45 ≠ 0)
  (h1 : x^2 - 10 * x - 69 ≠ 0)
  (h1 : 1 / (x^2 - 10 * x - 29) + 1 / (x^2 - 10 * x
  := - 45) - 2 / (x^2 - 10 * x - 69) = 0) :
  x = 13 := by
  field_simp at h1
  nlinarith
-----
-- Orig Proof
import Mathlib
import Aesop

set_option maxHeartbeats 0

open BigOperators Real Nat Topology Rat

theorem algebra_absxmpabsxpabsxp1eqxp2_01eqxleq1
  (x : ℝ)
  (h1 : abs (x - 1) + abs x + abs (x + 1) = x + 2) :
  0 ≤ x ∧ x ≤ 1 := by
  have h1 : 0 ≤ x := by
    have h1 : abs (x + 1) + abs (x - 1) ≥ 2 := by
      -- Prove that |x + 1| + |x - 1| ≥ 2 using the
      := triangle inequality
    cases' le_total 0 (x + 1) with h1 h1 <>
    cases' le_total 0 (x - 1) with h1 h1 <>
    cases' le_total 0 (x + 1 - (x - 1)) with
    := h1 h1 <>
    simp_all [abs_of_nonneg,
      := abs_of_nonpos, le_of_lt] <>
    (try { contradiction }) <>
    (try { linarith }) <>
    (try { nlinarith })
  <>
  (try { linarith })
  have h1 : abs x ≥ 0 := abs_nonneg x
  -- Combine the inequalities to get x + 2 ≥ 2
  have h1 : abs (x - 1) + abs x + abs (x + 1) ≥
  := 2 := by
    linarith [h1]
  have h1 : x + 2 ≥ 2 := by linarith
  linarith

```



```

(a b c d e f g :  $\kappa$ )
(h1 : a + 4 * b + 9 * c + 16 * d + 25 * e + 36 *
  → f + 49 * g = 1)
(h1 : 4 * a + 9 * b + 16 * c + 25 * d + 36 * e +
  → 49 * f + 64 * g = 12)
(h2 : 9 * a + 16 * b + 25 * c + 36 * d + 49 * e +
  → 64 * f + 81 * g = 123) :
16 * a + 25 * b + 36 * c + 49 * d + 64 * e + 81 *
  → f + 100 * g = 334 := by
have h_main : 16 * a + 25 * b + 36 * c + 49 * d +
  → 64 * e + 81 * f + 100 * g = 334 := by
  have h1 : 16 * a + 25 * b + 36 * c + 49 * d +
    → 64 * e + 81 * f + 100 * g = (a + 4 * b +
      → 9 * c + 16 * d + 25 * e + 36 * f + 49 *
        → g) - 3 * (4 * a + 9 * b + 16 * c + 25 * d
          → + 36 * e + 49 * f + 64 * g) + 3 * (9 * a +
            → 16 * b + 25 * c + 36 * d + 49 * e + 64 *
              → f + 81 * g) := by
    ring
    rw [h1]
    rw [h1, h1, h1]
    norm_num
    exact h_main
-- Simplified Proof
import Mathlib
import Aesop

set_option maxHeartbeats 0

open BigOperators Real Nat Topology Rat

theorem aime_1989_p8
(a b c d e f g :  $\kappa$ )
(h1 : a + 4 * b + 9 * c + 16 * d + 25 * e + 36 *
  → f + 49 * g = 1)
(h1 : 4 * a + 9 * b + 16 * c + 25 * d + 36 * e +
  → 49 * f + 64 * g = 12)
(h2 : 9 * a + 16 * b + 25 * c + 36 * d + 49 * e +
  → 64 * f + 81 * g = 123) :
16 * a + 25 * b + 36 * c + 49 * d + 64 * e + 81 *
  → f + 100 * g = 334 := by
  linarith
-----
-- Orig Proof
import Mathlib
import Aesop

set_option maxHeartbeats 0

open BigOperators Real Nat Topology Rat

theorem mathd_algebra_142
(m b :  $\kappa$ )
(h1 : m * 7 + b = -1)
(h2 : m * (-1) + b = 7) :
m + b = 5 := by
have h1 : m = -1 := by
  have h11 : 8 * m = -8 := by
    have h12 : (m * 7 + b) - (m * (-1) + b) = (-1
      → :  $\kappa$ ) - 7 := by
      linarith
    ring_nf at h12
    linarith
  -- Solve for m using 8m = -8
  linarith
have h1 : b = 6 := by
  have h11 : m * (-1) + b = 7 := h1
  rw [h1] at h11
  ring_nf at h11
  linarith
have h1 : m + b = 5 := by
  rw [h1, h1]
  <|> norm_num
exact h1
-- Simplified Proof
import Mathlib
import Aesop

set_option maxHeartbeats 0

open BigOperators Real Nat Topology Rat

theorem mathd_algebra_142
(m b :  $\kappa$ )
(h1 : m * 7 + b = -1)
(h2 : m * (-1) + b = 7) :
m + b = 5 := by
  linarith
-----
-- Orig Proof
import Mathlib
import Aesop

set_option maxHeartbeats 0

open BigOperators Real Nat Topology Rat

theorem mathd_algebra_400
(x :  $\kappa$ )
(h1 : 5 + 500 / 100 * 10 = 110 / 100 * x) :
x = 50 := by
  linarith
-----
-- Orig Proof
import Mathlib
import Aesop

set_option maxHeartbeats 0

open BigOperators Real Nat Topology Rat

theorem mathd_numbertheory_296
(n :  $\mathbb{N}$ )
(h1 : 2 ≤ n)
(h2 : ∃ x, x^3 = n)
(h3 : ∃ t, t^4 = n) :
4096 ≤ n := by
have h_main : 4096 ≤ n := by
  by_contra! h
  -- Assume for contradiction that n < 4096
  obtain (t, ht) := h2
  -- Obtain t such that t^4 = n
  have h1 : t ≤ 7 := by
    -- Prove that t ≤ 7 because t^4 < 4096
    by_contra! h1
    have h1 : t ≥ 8 := by linarith
    have h1 : t^4 ≥ 8^4 := by
      exact Nat.pow_le_pow_of_le_left (by
        linarith) 4
    have h1 : 8^4 = 4096 := by norm_num
    have h1 : t^4 ≥ 4096 := by
      linarith
    have h1 : n ≥ 4096 := by
      linarith
    -- Prove that t ≥ 2 because n ≥ 2
    by_contra! h1
    have h1 : t ≤ 1 := by linarith
    have h1 : t^4 ≤ 1 := by
      have : t = 0 ∨ t = 1 := by omega
      rcases this with (rfl | rfl) <|> norm_num
    have h1 : n ≤ 1 := by
      linarith
    linarith
  -- Check each possible value of t from 2 to 7
  -- to see if t^4 is a cube
  interval_cases t <|> norm_num at ht <|>
  (try {
    omega
  })
  exact h_main
-- Simplified Proof
import Mathlib
import Aesop

set_option maxHeartbeats 0

open BigOperators Real Nat Topology Rat

theorem mathd_numbertheory_296
(n :  $\mathbb{N}$ )
(h1 : 2 ≤ n)
(h2 : ∃ x, x^3 = n)
(h3 : ∃ t, t^4 = n) :
4096 ≤ n := by
  obtain (t, ht) := h2
  by_contra! h
  have h1 : t ≤ 7 := by
    by_contra! h1
    have : t^4 ≥ 8^4 := by
      exact Nat.pow_le_pow_of_le_left (by omega) 4
    linarith
  interval_cases t <|> simp_all
  <|>
  (try {
    obtain (x, hx) := h2
    have : x ≤ 15 := by
      nlinarith [pow_two_nonneg x,
        → pow_two_nonneg (x - 1)]
    interval_cases x <|> norm_num at hx <|>
    → omega
  })
  exact h_main
-----
-- Orig Proof
import Mathlib
import Aesop

set_option maxHeartbeats 0

open BigOperators Real Nat Topology Rat

theorem mathd_numbertheory_185
(n :  $\mathbb{N}$ )
(h1 : n % 5 = 3) :
(2 * n) % 5 = 1 := by
  omega
-----
-- Simplified Proof
import Mathlib
import Aesop

set_option maxHeartbeats 0

open BigOperators Real Nat Topology Rat

theorem mathd_algebra_441
(x :  $\kappa$ )
(h1 : x ≠ 0) :
12 / (x * x) * (x^4 / (14 * x)) * (35 / (3 * x))
  → = 10 := by
  have h1 : 12 / (x * x) * (x^4 / (14 * x)) * (35 /
    → (3 * x)) = 10 := by
    have h1 : x ≠ 0 := h1
    have h1 : x^2 ≠ 0 := by positivity
    have h1 : x^3 ≠ 0 := by positivity
    have h1 : x^4 ≠ 0 := by positivity
    -- Use field_simp to simplify the expression by
    -- clearing denominators
    field_simp [h1, h1, h1, h1, mul_assoc]
    -- Use ring_nf to normalize the expression
    <|> ring_nf
    -- Use norm_num to verify the numerical result
    <|> norm_num
    <|>
    (try {
      {
        field_simp [h1, h1, h1, h1]
        <|> ring_nf
        <|> norm_num
      }
    })
    <|>
    (try {
      {
        nlinarith [sq_pos_of_ne_zero h1]
      }
    })
  -- The final result follows directly from h1
  exact h1
-- Simplified Proof
import Mathlib
import Aesop

set_option maxHeartbeats 0

open BigOperators Real Nat Topology Rat

theorem mathd_algebra_441
(x :  $\kappa$ )
(h1 : x ≠ 0) :
12 / (x * x) * (x^4 / (14 * x)) * (35 / (3 * x))
  → = 10 := by
  field_simp
  ring
-----
-- Orig Proof
import Mathlib
import Aesop

set_option maxHeartbeats 0

open BigOperators Real Nat Topology Rat

theorem mathd_numbertheory_582
(n :  $\mathbb{N}$ )
(h1 : 0 < n)
(h2 : 3n) :
((n + 4) + (n + 6) + (n + 8)) % 9 = 0 := by
  have h1 : ∃ k, n = 3 * k := by
    obtain (k, hk) := h2
    refine' (k, _)
    <|> linarith
  have h1 : ((n + 4) + (n + 6) + (n + 8)) % 9 = 0 :=
    → by
    obtain (k, hk) := h1
    have h1 : ((n + 4) + (n + 6) + (n + 8)) = 9 *
      → (k + 2) := by
      rw [hk]
      ring_nf
      <|> omega
    rw [h1]
    have h1 : (9 * (k + 2)) % 9 = 0 := by
      simp [Nat.mul_mod, Nat.add_mod, Nat.mod_mod]
    exact h1
  exact h1
-- Simplified Proof
import Mathlib
import Aesop

set_option maxHeartbeats 0

open BigOperators Real Nat Topology Rat

theorem mathd_numbertheory_582
(n :  $\mathbb{N}$ )
(h1 : 0 < n)
(h2 : 3n) :
((n + 4) + (n + 6) + (n + 8)) % 9 = 0 := by
  omega
-----

```

```

-- Orig Proof
import Mathlib
import Aesop

set_option maxHeartbeats 0

open BigOperators Real Nat Topology Rat

theorem mathd_algebra_338
  (a b c : ℝ)
  (h₁ : 3 * a + b + c = -3)
  (h₂ : a + 3 * b + c = 9)
  (h₃ : a + b + 3 * c = 19) :
  a * b * c = -56 := by
  have h₄ : b = a + 6 := by
    have h₄₁ : -a + b = 6 := by
      have h₄₂ : (a + 3 * b + c) - (3 * a + b + c) =
        → 9 - (-3) := by
          linarith
        linarith
    linarith
  have h₄ : c = a + 11 := by
    have h₄₁ : -a + c = 11 := by
      have h₄₂ : (a + b + 3 * c) - (3 * a + b + c) =
        → 19 - (-3) := by
          linarith
        linarith
    linarith
  have h₄ : a = -4 := by
    have h₄₁ : 3 * a + b + c = -3 := h₁
    rw [h₄, h₄₁] at h₁
    ring_nf at h₁
    linarith
  have h₄ : b = 2 := by
    rw [h₄]
    rw [h₄]
    <|> norm_num
  have h₄ : c = 7 := by
    rw [h₄]
    rw [h₄]
    <|> norm_num
  have h₄ : a * b * c = -56 := by
    rw [h₄, h₄, h₄]
    <|> norm_num
  exact h₄

-- Simplified Proof
import Mathlib
import Aesop

set_option maxHeartbeats 0

open BigOperators Real Nat Topology Rat

theorem mathd_algebra_338
  (a b c : ℝ)
  (h₁ : 3 * a + b + c = -3)
  (h₂ : a + 3 * b + c = 9)
  (h₃ : a + b + 3 * c = 19) :
  a * b * c = -56 := by
  have : a = -4 := by linarith
  subst_vars
  nlinarith

```



# PutnamBench Proofs

```
-- Orig Proof
import Mathlib
import Aesop

set_option maxHeartbeats 0

theorem putnam_1962_a5
: ∀ n ≥ 2, ((fun n : ℕ => n * (n + 1) * 2^(n - 2)) : ℕ → ℕ) n = ∑ k in
  → Finset.Icc 1 n, Nat.choose n k * k^2 := by
  intro n hn
  have h_main : ∑ k in Finset.Icc 1 n, Nat.choose n k * k^2 = n * (n + 1) *
  → 2^(n - 2) := by
  have h₁ : ∑ k in Finset.Icc 1 n, Nat.choose n k * k^2 = n * ∑ k in
  → Finset.Icc 1 n, (Nat.choose (n - 1) (k - 1)) * k := by
  have h₂ : ∑ k ∈ Finset.Icc 1 n, Nat.choose n k * k * Nat.choose (n -
  → 1) (k - 1) := by
  intro k hk
  have h₃ : 1 ≤ k := by
  simp [Finset.mem_Icc] at hk
  linarith
  have h₄ : k ≤ n := by
  simp [Finset.mem_Icc] at hk
  linarith
  have h₅ : Nat.choose n k * k = n * Nat.choose (n - 1) (k - 1) := by
  have h₆ : k * Nat.choose n k = n * Nat.choose (n - 1) (k - 1) := by
  have h₇ : k * Nat.choose n k = n * Nat.choose (n - 1) (k - 1) := by
  rw [← Nat.succ_pred_eq_of_pos (by omega : 0 < k)]
  cases k with
  | zero => contradiction
  | succ k' =>
  cases n with
  | zero =>
  simp_all [Finset.mem_Icc]
  <|> omega
  | succ n' =>
  simp_all [Nat.choose_succ_succ, Nat.succ_mul_choose_eq,
  → Nat.mul_succ, Nat.add_assoc]
  <|> ring_nf at *
  <|> simp_all [Nat.choose_succ_succ, Nat.succ_mul_choose_eq,
  → Nat.mul_succ, Nat.add_assoc]
  <|> linarith
  exact h
  have h₈ : Nat.choose n k * k = k * Nat.choose n k := by ring
  rw [h₇]
  linarith
  exact h
calc
  ∑ k in Finset.Icc 1 n, Nat.choose n k * k^2 = ∑ k in Finset.Icc 1 n,
  → (Nat.choose n k * k) * k := by
  apply Finset.sum_congr rfl
  intro k hk
  ring
  = ∑ k in Finset.Icc 1 n, (n * Nat.choose (n - 1) (k - 1)) * k := by
  apply Finset.sum_congr rfl
  intro k hk
  rw [h₆]
  = ∑ k in Finset.Icc 1 n, n * (Nat.choose (n - 1) (k - 1) * k) := by
  apply Finset.sum_congr rfl
  intro k hk
  ring
  = n * ∑ k in Finset.Icc 1 n, (Nat.choose (n - 1) (k - 1)) * k := by
  simp [Finset.mul_sum]
  <|>
  ring_nf
  <|>
  simp_all [mul_assoc, mul_comm, mul_left_comm]
  <|>
  ring_nf
  <|>
  simp_all [Finset.sum_mul]
  <|>
  linarith
  have h₉ : ∑ k in Finset.Icc 1 n, (Nat.choose (n - 1) (k - 1)) * k = (n + 1)
  → * 2^(n - 2) := by
  have h₁₀ : ∑ k in Finset.Icc 1 n, (Nat.choose (n - 1) (k - 1)) * k = ∑ k
  → in Finset.Icc 1 n, (Nat.choose (n - 1) (k - 1)) * k := rfl
  rw [h₉]
  have h₁₁ : ∑ k in Finset.Icc 1 n, (Nat.choose (n - 1) (k - 1)) * k = ∑ k
  → in Finset.Icc 1 n, (Nat.choose (n - 1) (k - 1)) * k := rfl
  → n, (Nat.choose (n - 1) (k - 1)) * (k - 1) := by
  have h₁₂ : ∑ k in Finset.Icc 1 n, (Nat.choose (n - 1) (k - 1)) * k = ∑
  → k in Finset.Icc 1 n, ((Nat.choose (n - 1) (k - 1)) * (Nat.choose (n
  → - 1) (k - 1)) * (k - 1)) := by
  apply Finset.sum_congr rfl
  intro k hk
  have h₁₃ : 1 ≤ k := by
  simp [Finset.mem_Icc] at hk
  linarith
  have h₁₄ : k ≤ n := by
  simp [Finset.mem_Icc] at hk
  linarith
  have h₁₅ : (Nat.choose (n - 1) (k - 1)) * k = (Nat.choose (n - 1) (k
  → - 1)) * (Nat.choose (n - 1) (k - 1)) * (k - 1) := by
  have h₁₆ : k = (k - 1) + 1 := by
  have h₁₇ : 1 ≤ k := by
  simp [Finset.mem_Icc] at hk
  linarith
  omega
  rw [h₁₅]
  ring_nf
  <|>
  simp [Nat.mul_sub_left_distrib, Nat.mul_sub_right_distrib,
  → Nat.add_mul]
  <|>
  ring_nf at *
  <|>
  omega
  linarith
  calc
```

```
  ∑ k in Finset.Icc 1 n, (Nat.choose (n - 1) (k - 1)) * k = ∑ k in
  → Finset.Icc 1 n, ((Nat.choose (n - 1) (k - 1)) + (Nat.choose (n - 1)
  → (k - 1)) * (k - 1)) := h₁
  _ = ∑ k in Finset.Icc 1 n, (Nat.choose (n - 1) (k - 1)) + ∑ k in
  → Finset.Icc 1 n, (Nat.choose (n - 1) (k - 1)) * (k - 1) := by
  rw [Finset.sum_add_distrib]
  rw [h₁]
  have h₁₈ : ∑ k in Finset.Icc 1 n, (Nat.choose (n - 1) (k - 1)) = 2^(n -
  → 1) := by
  have h₁₉ : ∑ k in Finset.Icc 1 n, (Nat.choose (n - 1) (k - 1)) = ∑ j in
  → Finset.range n, Nat.choose (n - 1) j := by
  have h₂₀ : ∑ k in Finset.Icc 1 n, (Nat.choose (n - 1) (k - 1)) = ∑ k
  → in Finset.Icc 1 n, (Nat.choose (n - 1) (k - 1)) := rfl
  rw [h₁₉]
  have h₂₁ : ∑ k in Finset.Icc 1 n, (Nat.choose (n - 1) (k - 1)) = ∑ j
  → in Finset.range n, Nat.choose (n - 1) j := by
  apply Finset.sum_bij' (fun (k : ℕ) _ => k - 1) (fun (j : ℕ) _ => j
  → + 1)
  <|> simp_all [Finset.mem_Icc, Finset.mem_range, Nat.lt_succ_iff]
  <|> omega
  rw [h₂₁]
  rw [h₁₈]
  have h₂₂ : ∑ j in Finset.range n, Nat.choose (n - 1) j = 2^(n - 1) :=
  → by
  have h₂₃ : ∑ j in Finset.range n, Nat.choose (n - 1) j = ∑ j in
  → Finset.range (n - 1 + 1), Nat.choose (n - 1) j := by
  have h₂₄ : n - 1 + 1 = n := by
  have h₂₅ : 1 ≤ n := by omega
  omega
  rw [h₂₄]
  rw [h₂₃]
  have h₂₆ : ∑ j in Finset.range (n - 1 + 1), Nat.choose (n - 1) j = 2
  → ^ (n - 1) := by
  have h₂₇ : ∑ j in Finset.range (n - 1 + 1), Nat.choose (n - 1) j =
  → 2^(n - 1) := by
  rw [← Nat.sum_range_choose]
  <|>
  simp [Finset.sum_range_succ]
  <|>
  ring_nf
  <|>
  simp [Nat.choose_succ_succ]
  exact h₂₈
  rw [h₂₆]
  rw [h₂₇]
  have h₂₉ : ∑ k in Finset.Icc 1 n, (Nat.choose (n - 1) (k - 1)) * (k - 1) =
  → (n - 1) * 2^(n - 2) := by
  have h₃₀ : ∑ k in Finset.Icc 1 n, (Nat.choose (n - 1) (k - 1)) * (k -
  → 1) = ∑ k in Finset.Icc 2 n, (Nat.choose (n - 1) (k - 1)) * (k - 1)
  → := by
  have h₃₁ : ∑ k in Finset.Icc 2 n, (Nat.choose (n - 1) (k - 1)) * (k - 1)
  → := by
  have h₃₂ : ∑ k in Finset.Icc 1 n, (Nat.choose (n - 1) (k - 1)) * (k -
  → 1) = ∑ k in Finset.Icc 1 n, (Nat.choose (n - 1) (k - 1)) * (k - 1)
  → := rfl
  rw [h₃₂]
  have h₃₃ : ∑ k in Finset.Icc 1 n, (Nat.choose (n - 1) (k - 1)) * (k
  → - 1) = ∑ k in Finset.Icc 2 n, (Nat.choose (n - 1) (k - 1)) * (k - 1)
  → := by
  have h₃₄ : ∑ k in Finset.Icc 1 n, (Nat.choose (n - 1) (k - 1)) *
  → (k - 1) = ∑ k in Finset.Icc 1 n, (Nat.choose (n - 1) (k - 1)) * (k -
  → 1) := rfl
  rw [h₃₄]
  have h₃₅ : ∑ k in Finset.Icc 1 n, (Nat.choose (n - 1) (k - 1)) *
  → (k - 1) = ∑ k in Finset.Icc 2 n, (Nat.choose (n - 1) (k - 1)) * (k -
  → 1) + (Nat.choose (n - 1) (1 - 1)) * (1 - 1) := by
  have h₃₆ : Finset.Icc 1 n = {1} ∪ Finset.Icc 2 n := by
  ext x
  simp [Finset.mem_Icc, Finset.mem_union,
  → Finset.mem_singleton]
  <|>
  omega
  rw [h₃₆]
  rw [Finset.sum_union] <|> simp [Finset.disjoint_left] <|>
  (try omega) <|>
  (try
  {
    intros x hx, hx,
    simp [Finset.mem_Icc, Finset.mem_singleton] at hx, hx,
    <|> omega
  }) <|>
  (try
  {
    simp [Finset.sum_singleton]
    <|> ring_nf
    <|> simp [Nat.choose_zero_right]
  })
  <|>
  <|> omega
  have h₃₇ : (Nat.choose (n - 1) (1 - 1)) * (1 - 1) = 0 := by
  simp [Nat.choose_zero_right]
  <|> ring_nf
  <|> simp [Nat.choose_zero_right]
  rw [h₃₇, h₃₈]
  <|> simp [add_zero]
  <|>
  exact h₃₉
  exact h₄₀
  exact h₄₁
  rw [h₄₂]
  have h₄₃ : ∑ k in Finset.Icc 2 n, (Nat.choose (n - 1) (k - 1)) * (k -
  → 1) = (n - 1) * 2^(n - 2) := by
  have h₄₄ : ∑ k in Finset.Icc 2 n, (Nat.choose (n - 1) (k - 1)) * (k -
  → 1) = ∑ k in Finset.Icc 2 n, (n - 1) * (Nat.choose (n - 2) (k - 2)) :=
  → by
  apply Finset.sum_congr rfl
```









```

have h1 : (1 : Q) ∈ S := h
have h2 := hScond 1
have h3 : ¬((1 : Q) ∈ S ∧ (1 : Q) ∈ S) := by tauto
have h4 : (1 : Q) ∈ S := h2
have h5 : (1 : Q) ∈ S := h2
exfalse
apply h
exact (h4, h5)
have h_pos_rat : ∀ (r : Q), r > 0 → r ∈ S := by
  intro r hr
  have h1 : ∃ (p : N) (q : N), q ≥ 1 ∧ r = (p : Q) / (q : Q) := by
    have h2 : ∃ (p : Z) (q : N), q ≠ 0 ∧ r = (p : Q) / (q : Q) := by
      refine' (r.num, r.den, by simp [Rat.den_nz] using r.den_nz, _)
      field_simp [Rat.den_nz]
    obtain p, q, hq, h3 := h2
    have h4 : 0 < (q : N) := by
      by_contra h4
      have h5 : q = 0 := by
        omega
      simp_all [h4]
    have h6 : 0 < (q : N) := by
      exact_mod_cast h4
    have h7 : 0 < (q : N) := by
      exact_mod_cast h4
    have h8 : 0 < (q : N) := by
      exact_mod_cast h4
    have h9 : ∃ (p' : N) (q' : N), q' ≥ 1 ∧ r = (p' : Q) / (q' : Q) := by
      have h10 : 0 < (p : Z) := by
        by_contra h10
      have h11 : (r : Q) ≤ 0 := by
        by_contra h11
      have h12 : (r : Q) = (p : Q) / (q : Q) := by simp using h3
      rw [h12]
      have h13 : (p : Q) ≤ 0 := by exact_mod_cast h10
      have h14 : (q : Q) > 0 := by exact_mod_cast h4
      have h15 : (p : Q) / (q : Q) ≤ 0 := by
        exact div_nonpos_of_nonpos_of_nonneg h13 (by positivity)
      linarith
    have h16 : 0 < (p : Z) := by exact_mod_cast h10
    refine' (Int.toNat p, q, by omega, _)
    have h17 : (r : Q) = (p : Q) / (q : Q) := by simp using h3
    have h18 : (p : Q) = (Int.toNat p : Q) := by
      norm_cast
    <> simp [Int.toNat_of_nonneg (by linarith : (0 : Z) ≤ p)]
    rw [h18] at h17
    simp using h17
    obtain p', q', hq', h19 := h17
    exact p', q', hq', h19
  obtain p, q, hq, h20 := h1
  have h21 : (p : Q) ∈ S := by
    have h22 : (p : N) ≥ 0 := by positivity
    by_cases h23 : p = 0
    · exfalse
    · have h24 : (r : Q) = 0 := by
        rw [h20]
        simp [h20]
      linarith
    · have h25 : (p : N) ≥ 1 := by
        have h26 : p ≠ 0 := h23
        have h27 : (p : N) > 0 := by
          norm_cast at h26
          <> omega
        omega
      have h28 : ((p : N) : Q) ∈ S := h_pos_int p h20
      norm_cast at h28
    have h29 : (1 / (q : Q)) ∈ S := h_inv_pos_int q hq
    have h30 : (p : Q) * (1 / (q : Q)) ∈ S := hSprod (p : Q) h29 (1 / (q : Q)) h28
    have h31 : (p : Q) * (1 / (q : Q)) = r := by
      rw [h20]
      <> field_simp [hq]
    rw [h31] at h30
    exact h30
  have h_S_subset_pos : ∀ (r : Q), r ∈ S → r > 0 := by
    intro r hr
    by_contra h
    have h1 : r ≤ 0 := by linarith
    have h2 : r ≠ 0 := by
      by_contra h2
      have h3 := hScond r
      have h4 : ¬(r ∈ S ∧ r = 0) := by tauto
      have h5 : r ∈ S := hr
      have h6 : r = 0 := by linarith
      exact h4 (h5, h6)
    have h7 : r < 0 := by
      cases' lt_or_gt_of_ne h2 with h7 h8
      · exact h7
      · exfalse
    linarith
    have h9 : -r > 0 := by linarith
    have h10 : -r ∈ S := h_pos_rat (-r) (by linarith)
    have h11 : -r := hScond r
    have h12 : ¬(r ∈ S ∧ -r ∈ S) := by tauto
    have h13 : r ∈ S := hr
    have h14 : -r ∈ S := h10
    exact h12 (h13, h14)
  ext r
  constructor <> simp_all
  <> linarith
-- Orig Proof
import Mathlib
import Aesop
set_option maxHeartbeats 0
open MeasureTheory
theorem putnam_1962_b2
: ∃ f : ℝ → Set N+, ∀ a b : ℝ, a < b → f a ⊆ f b := by
  obtain i, hi := (i : Q → N+), Function.Injective i := by
    have h : Countable Q := by
      exact inferInstance
    obtain (f, hf) := h
    use fun q => (f q + 1, by positivity)
    intro q1 q2 hq
    have h1 : f q1 + 1 = f q2 + 1 := by
      have h2 : ((f q1 + 1, by positivity) : N+) = ((f q2 + 1, by positivity) : N+)
      → := hq
      simp [PNat.mk_coe] at h2
      <> norm_cast at h2
    omega
    have h3 : q1 = f q2 := by
      apply hf
    exact h3
  use fun a => {x : N+ | ∃ (q : Q), (q : ℝ) < a ∧ i q = x}
  intro a b hab
  have h1 : {x : N+ | ∃ (q : Q), (q : ℝ) < a ∧ i q = x} ⊆ {x : N+ | ∃ (q : Q),
    → (q : ℝ) < b ∧ i q = x} := by
    intro x hx
    obtain (q, hq, hx') := hx
    refine' (q, by linarith, hx')
  have h2 : {x : N+ | ∃ (q : Q), (q : ℝ) < a ∧ i q = x} ≠ {x : N+ | ∃ (q : Q),
    → (q : ℝ) < b ∧ i q = x} := by
    obtain q, hq := exists_rat_btwn hab
    have h3 : i q ∈ {x : N+ | ∃ (q' : Q), (q' : ℝ) < b ∧ i q' = x} := by
      refine' (q, by exact_mod_cast hq.2, rfl)
    have h4 : i q ∈ {x : N+ | ∃ (q' : Q), (q' : ℝ) < a ∧ i q' = x} := by
      intro h4
      obtain (q', hq', hq'') := h4
      have h5 : (q' : ℝ) < a := hq''
      have h6 : i q' = i q := by simp_all
      have h7 : q' = q := by
        apply hi
      simp_all
    linarith
  have h5 : i q ∈ {x : N+ | ∃ (q' : Q), (q' : ℝ) < a ∧ i q' = x} := by
    rw [h] at *
    exact h5
  exact h5
exact Set.ssubset_iff_subset_ne.mpr (h1, h2)
exact h_final
-- Simplified Proof
import Mathlib
import Aesop
set_option maxHeartbeats 0
open MeasureTheory
theorem putnam_1962_b2
: ∃ f : ℝ → Set N+, ∀ a b : ℝ, a < b → f a ⊆ f b := by
  obtain i, hi := (i : Q → N+), Function.Injective i := by
    have h : Countable Q := by
      exact inferInstance
    obtain (f, hf) := h
    use fun q => (f q + 1, by positivity)
    intro q1 q2 hq
    have h1 : f q1 + 1 = f q2 + 1 := by
      have h2 : ((f q1 + 1, by positivity) : N+) = ((f q2 + 1, by positivity) : N+)
      → := hq
      simp [PNat.mk_coe] at h2
      <> norm_cast at h2
    omega
    have h3 : q1 = f q2 := by
      apply hf
    exact h3
  use fun a => {x : N+ | ∃ (q : Q), (q : ℝ) < a ∧ i q = x}
  intro a b hab
  have h1 : {x : N+ | ∃ (q : Q), (q : ℝ) < a ∧ i q = x} ⊆ {x : N+ | ∃ (q : Q),
    → (q : ℝ) < b ∧ i q = x} := by
    intro x hx
    obtain (q, hq, hx') := hx
    refine' (q, by linarith, hx')
  have h2 : {x : N+ | ∃ (q : Q), (q : ℝ) < a ∧ i q = x} ≠ {x : N+ | ∃ (q : Q),
    → (q : ℝ) < b ∧ i q = x} := by
    obtain q, hq := exists_rat_btwn hab
    have h3 : i q ∈ {x : N+ | ∃ (q' : Q), (q' : ℝ) < b ∧ i q' = x} := by
      refine' (q, by exact_mod_cast hq.2, rfl)
    have h4 : i q ∈ {x : N+ | ∃ (q' : Q), (q' : ℝ) < a ∧ i q' = x} := by
      intro h4
      obtain (q', hq', hq'') := h4
      have h5 : (q' : ℝ) < a := hq''
      have h6 : i q' = i q := by simp_all
      have h7 : q' = q := by
        apply hi
      simp_all
    linarith
  have h5 : i q ∈ {x : N+ | ∃ (q' : Q), (q' : ℝ) < a ∧ i q' = x} := by
    rw [h] at *
    exact h5
  exact h5

```

```

simp_all
have h1 : (q : κ) < a := by
  have h1 : (q' : κ) < a := hq'
  norm_cast at h1
  <|> simp_all
  linarith
rw [h] at *
exact h1
exact Set.ssubset_iff_subset_ne.mpr (h1, h2)
-----
-- Orig Proof
import Mathlib
import Aesop

set_option maxHeartbeats 0

open Topology Filter Polynomial

theorem putnam_1963_b1
: ∀ a : ℤ, (X^2 - X + (C a)) | (X ^ 13 + X + (C 90)) ↔ a = ((2) : ℤ) := by
  intro a
  have h_main : ((Polynomial.X ^ 2 - Polynomial.X + Polynomial.C (a : ℤ)) |
    → (Polynomial.X ^ 13 + Polynomial.X + Polynomial.C (90 : ℤ))) ↔ a = 2
  := by
    constructor
    intro h
    have h1 : a = 2 := by
      by_contra h1

      have h1 : a = 1 ∨ a = -1 ∨ a = -2 := by

        have h1 : a | 90 := by

          obtain q, hq := h
          have h1 := congr_arg (fun p => Polynomial.eval 0 p) hq
          simp [Polynomial.eval_add, Polynomial.eval_sub,
            → Polynomial.eval_pow, Polynomial.eval_mul,
            Polynomial.eval_X, Polynomial.eval_C] at h1
          <|> ring_nf at h1
          <|> norm_num at h1
          <|>
          (try omega) <|>
          (try {
            use (Polynomial.eval 0 q)
            <|> linarith
          })
          have h1 : a | 92 := by

            obtain q, hq := h
            have h1 := congr_arg (fun p => Polynomial.eval 1 p) hq
            simp [Polynomial.eval_add, Polynomial.eval_sub,
            → Polynomial.eval_pow, Polynomial.eval_mul,
            Polynomial.eval_X, Polynomial.eval_C] at h1
            <|> ring_nf at h1
            <|> norm_num at h1
            <|>
            (try omega) <|>
            (try {
              use (Polynomial.eval 1 q)
              <|> linarith
            })
            have h1 : a | 2 := by
              have h1 : a | 92 - 90 := by

                exact dvd_sub h1 h1
                norm_num at h1
                <|> simp using h1

            have h1 : a = 1 ∨ a = -1 ∨ a = 2 ∨ a = -2 := by
              have h1 : a | 2 := h1
              have h1 : a = 1 ∨ a = -1 ∨ a = 2 ∨ a = -2 := by
                rw [← Int.natAbs_dvd_natAbs] at h1

                have h1 : a.natAbs | 2 := by
                  simp [Int.natAbs] using h1
                have h10 : a.natAbs = 1 ∨ a.natAbs = 2 := by

                  have h11 : a.natAbs | 2 := h1
                  have h12 : a.natAbs ≤ 2 := Nat.le_of_dvd (by decide) h11
                  interval_cases a.natAbs <|> norm_num at h11 <|> omega
                  cases h10 with
                  | inl h10 =>

                    have h11 : a = 1 ∨ a = -1 := by
                      have h11 : a.natAbs = 1 := h10
                      have h11 : a = 1 ∨ a = -1 := by
                        rw [Int.natAbs_eq_iff] at h11
                        tauto
                      exact h11
                    cases h11 with
                    | inl h11 =>
                      exact Or.inl h11
                    | inr h11 =>
                      exact Or.inr (Or.inl h11)
                  | inr h10 =>

                    have h11 : a = 2 ∨ a = -2 := by
                      have h11 : a.natAbs = 2 := h10
                      have h11 : a = 2 ∨ a = -2 := by
                        rw [Int.natAbs_eq_iff] at h11
                        tauto
                      exact h11
                    cases h11 with
                    | inl h11 =>
                      exact Or.inr (Or.inr (Or.inl h11))
                    | inr h11 =>
                      exact Or.inr (Or.inr (Or.inr h11))
                  exact h1
                rcases h1 with (rfl | rfl | rfl | rfl) <|> norm_num at h1 <|>
                (try contradiction) <|>
                (try tauto)

            rcases h1 with (rfl | rfl | rfl)

```

```

      obtain q, hq := h
      have h1 := congr_arg (fun p => Polynomial.eval 2 p) hq
      simp [Polynomial.eval_add, Polynomial.eval_sub, Polynomial.eval_pow,
        → Polynomial.eval_mul,
        Polynomial.eval_X, Polynomial.eval_C] at h1
      <|> ring_nf at h1
      <|> norm_num at h1
      <|>
      (try omega) <|>
      (try {
        have h1 := h1
        ring_nf at h1
        norm_num at h1
        omega
      })
    })

    obtain q, hq := h
    have h1 := congr_arg (fun p => Polynomial.eval 3 p) hq
    simp [Polynomial.eval_add, Polynomial.eval_sub, Polynomial.eval_pow,
    → Polynomial.eval_mul,
    Polynomial.eval_X, Polynomial.eval_C] at h1
    <|> ring_nf at h1
    <|> norm_num at h1
    <|>
    (try omega) <|>
    (try {
      have h1 := h1
      ring_nf at h1
      norm_num at h1
      omega
    })
  })

  exact h1
  intro h
  rw [h]

  use (Polynomial.X ^ 11 + Polynomial.X ^ 10 - Polynomial.X ^ 9 - 3 *
    → Polynomial.X ^ 8 - Polynomial.X ^ 7 + 5 * Polynomial.X ^ 6 + 7 *
    → Polynomial.X ^ 5 - 3 * Polynomial.X ^ 4 - 17 * Polynomial.X ^ 3 - 11 *
    → Polynomial.X ^ 2 + 23 * Polynomial.X + 45)
  ring_nf
  <|> norm_num
  <|>
  (try decide) <|>
  (try ring_nf) <|>
  (try norm_num)
  exact h_main

-- Simplified Proof
import Mathlib
import Aesop

set_option maxHeartbeats 0

open Topology Filter Polynomial

theorem putnam_1963_b1
: ∀ a : ℤ, (X^2 - X + (C a)) | (X ^ 13 + X + (C 90)) ↔ a = ((2) : ℤ) := by
  intro a
  constructor
  intro h
  by_contra h1
  have h1 : a = 1 ∨ a = -1 ∨ a = -2 := by
    have h1 : a | 90 := by
      obtain q, hq := h
      have h1 := congr_arg (fun p => Polynomial.eval 0 p) hq
      simp [Polynomial.eval_add, Polynomial.eval_sub, Polynomial.eval_pow,
        → Polynomial.eval_mul,
        Polynomial.eval_X, Polynomial.eval_C] at h1
      <|> ring_nf at h1
      <|> use (Polynomial.eval 0 q)
      have h1 : a | 92 := by
        obtain q, hq := h
        have h1 := congr_arg (fun p => Polynomial.eval 1 p) hq
        simp [Polynomial.eval_add, Polynomial.eval_sub, Polynomial.eval_pow,
        → Polynomial.eval_mul,
        Polynomial.eval_X, Polynomial.eval_C] at h1
        <|> ring_nf at h1
        <|> use (Polynomial.eval 1 q)
      have h1 : a | 2 := by
        have h1 : a | 92 - 90 := by
          exact dvd_sub h1 h1
          <|> simp using h1
        <|> simp using h1
      have h1 : a = 1 ∨ a = -1 ∨ a = 2 ∨ a = -2 := by
        rw [← Int.natAbs_dvd_natAbs] at h1
        have h1 : a.natAbs | 2 := by
          simp [Int.natAbs] using h1
        have h10 : a.natAbs = 1 ∨ a.natAbs = 2 := by
          have h11 : a.natAbs | 2 := h1
          have h12 : a.natAbs ≤ 2 := Nat.le_of_dvd (by decide) h11
          interval_cases a.natAbs <|> norm_num at h11 <|>
          cases h10 with
          | inl h10 =>
            have h11 : a = 1 ∨ a = -1 := by
              have h11 : a.natAbs = 1 := h10
              have h11 : a = 1 ∨ a = -1 := by
                rw [Int.natAbs_eq_iff] at h11
                tauto
            cases h11 with
            | inl h11 =>
              exact Or.inl h11
            | inr h11 =>
              exact Or.inr (Or.inl h11)
          | inr h10 =>
            have h11 : a = 2 ∨ a = -2 := by
              have h11 : a.natAbs = 2 := h10
              have h11 : a = 2 ∨ a = -2 := by
                rw [Int.natAbs_eq_iff] at h11
                tauto
            cases h11 with
            | inl h11 =>
              exact Or.inr (Or.inr (Or.inl h11))
            | inr h11 =>
              exact Or.inr (Or.inr (Or.inr h11))
          exact h1
        rcases h1 with (rfl | rfl | rfl | rfl) <|> norm_num at h1 <|>
        (try contradiction) <|>
        (try tauto)

      rcases h1 with (rfl | rfl | rfl)

```

```

      exact h₁
    cases h₁ with
    | inl h =>
      exact Or.inl h
    | inr h =>
      exact Or.inr (Or.inl h)
  | inr h₁ =>
    have h₂ : a = 2 ∨ a = -2 := by
      have h₂₀ : a.natAbs = 2 := h₁
      have h₂₁ : a = 2 ∨ a = -2 := by
        rw [Int.natAbs_eq_iff] at h₂₀
      tauto
    exact h₂
  | inl h₁ =>
    exact Or.inr (Or.inr (Or.inl h₁))
  | inr h₁ =>
    exact Or.inr (Or.inr (Or.inr h₁))
rcases h₁ with (rfl | rfl | rfl | rfl) <|> norm_num at h₁
rcases h₁ with (rfl | rfl | rfl)

obtain q, hq := h
have h₁ := congr_arg (fun p => Polynomial.eval 2 p) hq
simp [Polynomial.eval_add, Polynomial.eval_sub, Polynomial.eval_pow,
      Polynomial.eval_mul,
      Polynomial.eval_X, Polynomial.eval_C] at h₁
<|> ring_nf at h₁
<|> norm_num at h₁
<|> omega

obtain q, hq := h
have h₁ := congr_arg (fun p => Polynomial.eval 3 p) hq
simp [Polynomial.eval_add, Polynomial.eval_sub, Polynomial.eval_pow,
      Polynomial.eval_mul,
      Polynomial.eval_X, Polynomial.eval_C] at h₁
<|> ring_nf at h₁
<|> norm_num at h₁
<|> omega

obtain q, hq := h
have h₁ := congr_arg (fun p => Polynomial.eval 2 p) hq
simp [Polynomial.eval_add, Polynomial.eval_sub, Polynomial.eval_pow,
      Polynomial.eval_mul,
      Polynomial.eval_X, Polynomial.eval_C] at h₁
<|> ring_nf at h₁
<|> norm_num at h₁
<|> omega

rintro rfl
use (X ^ 11 + X ^ 10 - X ^ 9 - 3 * X ^ 8 - X ^ 7 + 5 * X ^ 6 + 7 * X ^ 5 -
     3 * X ^ 4 - 17 * X ^ 3 - 11 * X ^ 2 + 23 * X + 45)
ring_nf
<|> norm_num
<|> ring_nf

-----
-- Orig Proof
import Mathlib
import Aesop

set_option maxHeartbeats 0

open Set Function

theorem putnam_1964_a4
(u : ℕ → ℤ)
(bounded : ∃ B T : ℤ, ∀ n : ℕ, B ≤ u n ∧ u n ≤ T)
(hu : ∀ n ≥ 4, u n = ((u (n - 1) + u (n - 2) + u (n - 3) * u (n - 4)) : ℝ) / (u
  → (n - 1) * u (n - 2) + u (n - 3) + u (n - 4)) ∧ (u (n - 1) * u (n - 2)
  → + u (n - 3) + u (n - 4)) ≠ 0)
(∃ N c : ℕ, c > 0 ∧ ∀ n ≥ N, u (n + c) = u n) := by
  have h_main : ∃ (i j : ℕ), i < j ∧ (u i = u j ∧ u (i + 1) = u (j + 1) ∧ u (i +
    → 2) = u (j + 2) ∧ u (i + 3) = u (j + 3)) := by
    obtain B, T, hB := bounded
    have h₁ : ∃ (i j : ℕ), i < j ∧ (u i = u j ∧ u (i + 1) = u (j + 1) ∧ u (i +
      → 2) = u (j + 2) ∧ u (i + 3) = u (j + 3)) := by
      classical
      let f : ℕ → (ℤ × ℤ × ℤ × ℤ) := fun n => (u n, u (n + 1), u (n + 2), u (n +
        → 3))
      have h₂ : Set.Finite (Set.range f) := by
        have h₂₀ : Set.range f ⊆ Set.Icc (B, B, B, B) (T, T, T, T) := by
          intro x hx
          rcases hx with n, rfl
          have h₂₁ : u n ≤ hB
          have h₂₂ : u (n + 1) ≤ hB
          have h₂₃ : u (n + 2) ≤ hB
          have h₂₄ : u (n + 3) ≤ hB
          simp only [Set.mem_Icc, Prod.le_def] at h₂₁ h₂₂ h₂₃ h₂₄
          constructor <|>
          (try constructor) <|>
          (try constructor) <|>
          (try constructor) <|>
          (try simp_all [f]) <|>
          (try nlinarith)
      have h₃ : Set.Finite (Set.Icc (B, B, B, B) (T, T, T, T)) := by
        apply Set.Finite.subset (Set.finite_mem_finset (Finset.Icc (B, B, B,
          → B) (T, T, T, T)))
      intro x hx
      simp_all [Set.mem_Icc]
      <|>
      (try aesop)
      exact Set.Finite.subset h₁ h₃
    have h₄ : ∃ (i j : ℕ), i < j ∧ f i = f j := by
      by_contra! h
      have h₄₀ : Function.Injective f := by
        intro i j h₄₁
        by_cases h₄₂ : i = j
        · exact h
        · have h₄₃ : i < j ∨ j < i := by omega
          cases h₄₃ with
          | inl h₄₄ =>
            have h₄₅ : f i = f j
            simp_all
          | inr h₄₄ =>
            have h₄₆ : f i = f j
            simp_all
      have h₄₇ : Set.Infinite (Set.range f) := Set.infinite_range_of_injective
      → h
      exact Set.not_infinite.mpr h₁ h₄
    obtain (i, j, h₁, h₂) := h₁
    refine' (i, j, h₁, h₂)
    simp [f] at h₁
    <|>
    (try simp_all [Prod.ext_iff]) <|>
    (try omega) <|>
    (try aesop)
  exact h₁

have h_periodic : ∃ N c : ℕ, c > 0 ∧ ∀ n ≥ N, u (n + c) = u n := by
  obtain (i, j, h₁, h₂) := h_main
  have h₃ : ∀ m : ℕ, u (i + m) = u (j + m) := by
    intro m
    have h₃₀ : ∀ m : ℕ, u (i + m) = u (j + m) := by
      intro m
      induction m using Nat.strong_induction_on with
      | h m ih =>
        match m with
        | 0 =>
          have h₃₁ : h_eq.1
          simp at h₃₁
          <|> simp_all [add_assoc]
        | 1 =>
          have h₃₂ : h_eq.2.1
          simp at h₃₂
          <|> simp_all [add_assoc]
          <|> ring_nf at *
          <|> omega
        | 2 =>
          have h₃₃ : h_eq.2.2.1
          simp at h₃₃
          <|> simp_all [add_assoc]
          <|> ring_nf at *
          <|> omega
        | 3 =>
          have h₃₄ : h_eq.2.2.2
          simp at h₃₄
          <|> simp_all [add_assoc]
          <|> ring_nf at *
          <|> omega
        | m + 4 =>
          have h₃₅ : i + (m + 4) ≥ 4 := by
            have h₃₆ : i ≥ 0 := by linarith
            omega
          have h₃₇ : u (i + (m + 4)) = ((u (i + (m + 4) - 1) + u (i + (m + 4)
            → - 2) + u (i + (m + 4) - 3) * u (i + (m + 4) - 4)) : ℝ) / (u (i + (m +
            → 4) - 1) * u (i + (m + 4) - 2) + u (i + (m + 4) - 3) + u (i + (m + 4)
            → - 4)) := by
            have h₃₈ : hu (i + (m + 4)) (by omega)
            have h₃₉ : h₃₁.1
            norm_cast at h₃₉
            <|> simp_all [add_assoc]
            <|> ring_nf at *
            <|> norm_num at *
            <|> linarith
          have h₃₇ : u (j + (m + 4)) = ((u (j + (m + 4) - 1) + u (j + (m + 4)
            → - 2) + u (j + (m + 4) - 3) * u (j + (m + 4) - 4)) : ℝ) / (u (j + (m +
            → 4) - 1) * u (j + (m + 4) - 2) + u (j + (m + 4) - 3) + u (j + (m + 4)
            → - 4)) := by
            have h₃₈ : hu (j + (m + 4)) (by
              have h₃₉ : j ≥ i + 1 := by omega
              omega
            )
            have h₃₉ : h₃₁.1
            norm_cast at h₃₉
            <|> simp_all [add_assoc]
            <|> ring_nf at *
            <|> norm_num at *
            <|> linarith
          have h₃₇ : (i + (m + 4) - 1 : ℕ) = i + (m + 3) := by
            omega
          have h₃₇ : (i + (m + 4) - 2 : ℕ) = i + (m + 2) := by
            omega
          have h₃₇ : (i + (m + 4) - 3 : ℕ) = i + (m + 1) := by
            omega
          have h₃₇ : (i + (m + 4) - 4 : ℕ) = i + m := by
            omega
          have h₃₇ : (j + (m + 4) - 1 : ℕ) = j + (m + 3) := by
            omega
          have h₃₇ : (j + (m + 4) - 2 : ℕ) = j + (m + 2) := by
            omega
          have h₃₇ : (j + (m + 4) - 3 : ℕ) = j + (m + 1) := by
            omega
          have h₃₇ : (j + (m + 4) - 4 : ℕ) = j + m := by
            omega
          have h₃₇ : u (i + (m + 3)) = u (j + (m + 3)) := by
            have h₃₈ : ih (m + 3) (by omega)
            simp [add_assoc] at h₃₈
            <|> omega
          have h₃₇ : u (i + (m + 2)) = u (j + (m + 2)) := by
            have h₃₈ : ih (m + 2) (by omega)
            simp [add_assoc] at h₃₈
            <|> omega
          have h₃₇ : u (i + (m + 1)) = u (j + (m + 1)) := by
            have h₃₈ : ih (m + 1) (by omega)
            simp [add_assoc] at h₃₈
            <|> omega
          have h₃₇ : u (i + m) = u (j + m) := by
            have h₃₈ : ih m (by omega)
            simp [add_assoc] at h₃₈
            <|> omega
          have h₃₇ : (u (i + (m + 4)) : ℝ) = (u (j + (m + 4)) : ℝ) := by
            rw [h₃₈]
            simp [h₃₈, h₃₈, h₃₈, h₃₈, h₃₈, h₃₈, h₃₈] at *
            norm_cast at *
            <|>
            (try simp_all [h₃₈, h₃₈, h₃₈, h₃₈]) <|>
            (try ring_nf at *) <|>
            (try field_simp at *) <|>

```

```

      (try norm_cast at *) <>
      (try linarith)
      norm_cast at h14 ⊢
    <>
    (try simp_all) <>
    (try linarith)
  exact h15
have h16 : ∃ N c : ℕ, c > 0 ∧ ∀ n ≥ N, u (n + c) = u n := by
use i, (j - i)
have h17 : j - i > 0 := by
  omega
  constructor
  · exact h16
  · intro n hn
    have h18 : u (n + (j - i)) = u n := by
      have h19 : u (i + (n - i)) = u (j + (n - i)) := by
        have h20 := h16 (n - i)
        simp [add_assoc] at h20 ⊢
      <> omega
    have h21 : i + (n - i) = n := by
      omega
    have h22 : j + (n - i) = n + (j - i) := by
      omega
    rw [h20] at h19
    rw [h22] at h19
    linarith
  exact h18
exact h17

exact h_periodic

-- Simplified Proof
import Mathlib
import Aesop

set_option maxHeartbeats 0

open Set Function

theorem putnam_1964_a4
(u : ℕ → ℤ)
(boundedu : ∃ B T : ℤ, ∀ n : ℕ, B ≤ u n ∧ u n ≤ T)
(hu : ∀ n ≥ 4, u n = ((u (n - 1) + u (n - 2) + u (n - 3) * u (n - 4)) : ℝ) / (u
  → (n - 1) * u (n - 2) + u (n - 3) + u (n - 4)) ∧ (u (n - 1) * u (n - 2)
  → + u (n - 3) + u (n - 4)) ≠ 0)
: (∃ N c : ℕ, c > 0 ∧ ∀ n ≥ N, u (n + c) = u n) := by
obtain ⟨B, T, hB⟩ := boundedu
let f : ℕ → (ℤ × ℤ × ℤ × ℤ) := fun n => (u n, u (n + 1), u (n + 2), u (n +
  → 3))
have h1 : Set.Finite (Set.range f) := by
have h2 : Set.range f ⊆ Set.Icc (B, B, B, B) (T, T, T, T) := by
  intro x hx
  rcases hx with ⟨n, rfl⟩
  have h3 := hB n
  have h4 := hB (n + 1)
  have h5 := hB (n + 2)
  have h6 := hB (n + 3)
  simp only [Set.mem.Icc, Prod.le_def] at h3 h4 h5 h6 ⊢
  constructor <> (try constructor) <> (try constructor) <> (try
    → constructor) <> simp_all [f]
have h3 : Set.Finite (Set.Icc (B, B, B, B) (T, T, T, T)) := by
  apply Set.Finite.subset (Set.finite_mem_finsset (Finsset.Icc (B, B, B, B)
    → (T, T, T, T)))
  intro x hx
  simp_all [Set.mem.Icc]
exact Set.Finite.subset h3
have h4 : ∃ (i j : ℕ), i < j ∧ f i = f j := by
  by_contra! h4
have h5 : Function.Injective f := by
  intro i j h5
  by_contra! h5
  have h6 : i < j ∨ j < i := by omega
  cases h6 with
  | inl h6 =>
    have h7 := h4 i j h6
    simp_all
  | inr h6 =>
    have h8 := h4 j i h6
    simp_all
have h5 : Set.Infinite (Set.range f) := Set.infinite_range_of_injective h5
exact Set.not_infinite.mpr h5
obtain ⟨i, j, h10, h11⟩ := h4
have h12 : ∀ m : ℕ, u (i + m) = u (j + m) := by
  intro m
  induction m using Nat.strong_induction_on with
  | h m ih =>
    match m with
    | 0 =>
      simp [f] at h_eq ⊢
      exact h_eq.1
    | 1 =>
      simp [f] at h_eq ⊢
      exact h_eq.2.1
    | 2 =>
      simp [f] at h_eq ⊢
      exact h_eq.2.2.1
    | 3 =>
      simp [f] at h_eq ⊢
      exact h_eq.2.2.2
    | m + 4 =>
      have h13 : i + (m + 4) ≥ 4 := by linarith
      have h14 := hu (i + (m + 4)) (by omega)
      have h15 := hu (j + (m + 4)) (by omega)
      have h16 : (i + (m + 4) - 1 : ℕ) = i + (m + 3) := by omega
      have h17 : (i + (m + 4) - 2 : ℕ) = i + (m + 2) := by omega
      have h18 : (i + (m + 4) - 3 : ℕ) = i + (m + 1) := by omega
      have h19 : (i + (m + 4) - 4 : ℕ) = i + m := by omega
      have h20 : (j + (m + 4) - 1 : ℕ) = j + (m + 3) := by omega
      have h21 : (j + (m + 4) - 2 : ℕ) = j + (m + 2) := by omega
      have h22 : (j + (m + 4) - 3 : ℕ) = j + (m + 1) := by omega
      have h23 : (j + (m + 4) - 4 : ℕ) = j + m := by omega
      have h24 : u (i + (m + 3)) = u (j + (m + 3)) := by
        have h25 := ih (m + 3) (by omega)
        simp [add_assoc] at h25 ⊢

```

```

    <> omega
  have h26 : u (i + (m + 2)) = u (j + (m + 2)) := by
    have h27 := ih (m + 2) (by omega)
    simp [add_assoc] at h27 ⊢
    <> omega
  have h28 : u (i + (m + 1)) = u (j + (m + 1)) := by
    have h29 := ih (m + 1) (by omega)
    simp [add_assoc] at h29 ⊢
    <> omega
  have h30 : u (i + m) = u (j + m) := by
    have h31 := ih m (by omega)
    simp [add_assoc] at h31 ⊢
    <> omega
  have h32 : (u (i + (m + 4)) : ℝ) = (u (j + (m + 4)) : ℝ) := by
    rw [h31, h31]
    simp [h26, h27, h28, h29, h30, h31, h32, h33] at *
    norm_cast at *
    <> simp_all [h26, h30, h32, h33]
    norm_cast at h34 ⊢
  exact (i, j - i, by omega, fun n hn => by
    have h35 : u (n + (j - i)) = u n := by
      have h36 : u (i + (n - i)) = u (j + (n - i)) := by
        have h37 := h16 (n - i)
        simp [add_assoc] at h37 ⊢
      <> omega
    have h38 : i + (n - i) = n := by omega
    have h39 : j + (n - i) = n + (j - i) := by omega
    rw [h37] at h36
    rw [h39] at h36
    linarith
  exact h35)

-----
-- Orig Proof
import Mathlib
import Aesop

set_option maxHeartbeats 0

open Set Function Filter Topology

theorem putnam_1964_b2
(S : Type*) [Fintype S] [Nonempty S]
(P : Fintype (Set S))
(hPP : ∀ T ∈ P, ∀ U ∈ P, T ∩ U ≠ ∅)
(hPS : ∃ T : Set S, T ∈ P ∧ (∀ U ∈ P, T ∩ U ≠ ∅))
: (P.card = 2 ^ (Fintype.card S - 1)) := by
have h_no_empty : ∀ (T : Set S), T ∈ P → T.Nonempty := by
  intro T hT
  have h1 : T ∩ T ≠ ∅ := hPP T hT T hT
  have h2 : T ∩ T = T := by simp [Set.ext_iff]
  rw [h1] at h2
  exact Set.nonempty_iff_ne_empty.mpr h2

have h_subset_or_compl : ∀ (A : Set S), A ∈ P ∨ A' ∈ P := by
  intro A
  by_contra! h
  have h3 : A ∈ P := h.1
  have h4 : A' ∈ P := h.2

have h5 : ∃ (U : Set S), U ∈ P ∧ A ∩ U = ∅ := by
  have h6 : ¬(A ∈ P ∧ ∀ (U : Set S), U ∈ P → A ∩ U ≠ ∅) := by
    intro h6
    have h7 : ∃ (T : Set S), T ∈ P ∧ (∀ U ∈ P, T ∩ U ≠ ∅) := by
      refine' ⟨A, _⟩
    constructor
    · exact h.1
    · intro U hU
      have h8 := h5.2 U hU
      have h9 : A ∩ U ≠ ∅ := h8
      have h10 : A ∩ U = U ∩ A := by
        ext x
        simp [Set.mem_inter_iff]
      <> tauto
    have h11 : U ∩ A ≠ ∅ := by
      intro h11
      apply h11
      simp_all [Set.ext_iff]
      <> aesop
    simp [Set.inter_comm] using h11
  exact hPS h6
by_cases h12 : A ∈ P
· have h13 : ¬(∀ (U : Set S), U ∈ P → A ∩ U ≠ ∅) := by
  intro h13
  exact h12 (h13, h13)
push_neg at h13
obtain ⟨U, hU, h14⟩ := h13
refine' ⟨U, hU, _⟩
have h15 : A ∩ U = ∅ := by
  by_contra h15
  have h16 : A ∩ U ≠ ∅ := h15
  simp_all [Set.ext_iff]
  <> aesop
exact h15
· exfalso
  simp_all

have h17 : ∃ (V : Set S), V ∈ P ∧ A' ∩ V = ∅ := by
  have h18 : ¬(A' ∈ P ∧ ∀ (U : Set S), U ∈ P → A' ∩ U ≠ ∅) := by
    intro h18
    have h19 : ∃ (T : Set S), T ∈ P ∧ (∀ U ∈ P, T ∩ U ≠ ∅) := by
      refine' ⟨A', _⟩
    constructor
    · exact h.1
    · intro U hU
      have h20 := h5.2 U hU
      have h21 : A' ∩ U ≠ ∅ := h20
      have h22 : A' ∩ U = U ∩ A' := by
        ext x
        simp [Set.mem_inter_iff]
      <> tauto
    have h23 : U ∩ A' ≠ ∅ := by
      intro h23
      apply h23
      simp_all [Set.ext_iff]
      <> aesop
    simp [Set.inter_comm] using h23
  exact hPS h18

```

```

exact hPS h
by_cases h₁ : A ∈ P
have h : ¬(∀ (U : Set S), U ∈ P → A ∩ U ≠ ∅) := by
  intro h₁
  exact h₁ (h₁, h₁)
push_neg at h
obtain ⟨V, hV, h⟩ := h
refine' ⟨V, hV, _⟩
have h₁ : A ∩ V = ∅ := by
  by_contra h₂
  have h₁₁ : A ∩ V ≠ ∅ := h₂
  simp_all [Set.ext_iff]
  <|> aesop
exact h₁
ex falso
simp_all

obtain ⟨U, hU, hU'⟩ := h
obtain ⟨V, hV, hV'⟩ := h

have h₁ : U ⊆ A' := by
  intro x hx
  by_contra h₁
  have h₁ : x ∈ A := by simp_all [Set.mem_compl_iff]
  have h₁ : x ∈ A ∩ U := Set.mem_inter h₁ hx
  rw [hU'] at h₁
  simp at h₁
  <|> aesop
have h₁ : V ⊆ A := by
  intro x hx
  by_contra h₁
  have h₁ : x ∈ A' := by simp_all [Set.mem_compl_iff]
  have h₁ : x ∈ A ∩ V := Set.mem_inter h₁ hx
  rw [hV'] at h₁
  simp at h₁
  <|> aesop

have h₁ : U ∩ V = ∅ := by
  apply Set.eq_empty_of_forall_not_mem
  intro x hx
  have h₁ : x ∈ U := Set.mem_of_mem_inter_left hx
  have h₁ : x ∈ V := Set.mem_of_mem_inter_right hx
  have h₁ : x ∈ A' := h₁ h₁
  have h₁ : x ∈ A := h₁ h₁
  simp_all [Set.mem_compl_iff]
  <|> aesop

have h₁ : U ∩ V ≠ ∅ := hPP U hU V hV
simp_all [Set.ext_iff]
<|> aesop

have h_not_both : ∀ (A : Set S), A ∈ P → A' ∈ P := by
  intro A hA
  by_contra h₁
  have h₁ : A' ∈ P := h
  have h₁ : A ∩ A' = ∅ := by
    ext x
    simp [Set.mem_inter_iff]
  <|> tauto
  have h₁ : A ∩ A' ≠ ∅ := hPP A hA A' h₁
  rw [h₁] at h₁
  contradiction

have h_card : P.card = 2 ^ (Fintype.card S - 1) := by
  classical

let Q : Finset (Set S) := (Finset.univ : Finset (Set S)) \ P

have h₁ : P.card = Q.card := by

  have h₁ : ∀ (A : Set S), A ∈ P → A' ∈ Q := by
    intro A hA
    have h₁ : A' ∈ (Finset.univ : Finset (Set S)) := Finset.mem_univ _
    have h₁ : A' ∈ P := h_not_both A hA
    simp only [Q, Finset.mem_sdiff] at *
    tauto
  have h₁ : ∀ (A : Set S), A ∈ Q → A' ∈ P := by
    intro A hA
    have h₁ : A ∈ (Finset.univ : Finset (Set S)) := by
      simp only [Q, Finset.mem_sdiff] at hA
      tauto
    have h₁ : A ∈ P := by
      simp only [Q, Finset.mem_sdiff] at hA
      tauto
    have h₁ : A ∈ (Finset.univ : Finset (Set S)) := by tauto
    have h₁ : A ∈ P ∨ A' ∈ P := h_subset_or_compl A
    cases h₁ with
    | inl h₁ =>
      ex falso
      tauto
    | inr h₁ =>
      exact h₁
  have h₁ : P.card = Q.card := by

    have h₁ : ∀ (A : Set S), A ∈ P → A' ∈ Q := h₁
    have h₁ : ∀ (A : Set S), A ∈ Q → A' ∈ P := h₁
    have h₁ : P.card = Q.card := by
      apply Finset.card_bij' (fun A _ => A') (fun A _ => A')
      <|> simp_all [Set.ext_iff]
      <|> (try
        {
          aesop
        })
      <|> (try
        {
          intros
          simp_all [Set.ext_iff]
          tauto
        })
      <|> (try
        {
          exact h₁
          exact h₁
          exact h₁
        })
      <|> (try
        {
          have h₁ : P.card + Q.card = 2 ^ Fintype.card S := by
            have h₁ : P.card + Q.card = (Finset.univ : Finset (Set S)).card := by
              rw [Finset.disjoint_left]
              intro A hA hA'
              simp only [Q, Finset.mem_sdiff] at hA'
              tauto
            have h₁ : P ∪ Q = (Finset.univ : Finset (Set S)) := by
              apply Finset.ext
              intro A
              simp only [Q, Finset.mem_union, Finset.mem_sdiff, Finset.mem_univ,
                true_and]
              <|> (try
                {
                  by_cases h₁ : A ∈ P <|> simp_all [h_subset_or_compl]
                  <|> (try tauto)
                  <|> (try
                    {
                      have h₁ := h_subset_or_compl A
                      cases h₁ with
                      | inl h₁ => tauto
                      | inr h₁ =>
                        have h₁ : A' ∈ P := h₁
                        have h₁ : A ∈ P ∨ A' ∈ P := by tauto
                        tauto
                    })
                })
            have h₁ : P.card + Q.card = (P ∪ Q).card := by
              rw [Finset.card_union_add_card_inter P Q]
            have h₁ : P ∩ Q = ∅ := Finset.disjoint_iff_inter_eq_empty.mp h₁
            rw [h₁]
            simp
            rw [h₁] at h₁
            exact h₁
          have h₁ : (Finset.univ : Finset (Set S)).card = 2 ^ Fintype.card S := by
            simp [Fintype.card_fun]
            <|> simp_all [Fintype.card_fun]
            <|> ring_nf
            <|> simp_all [Fintype.card_fun]
            <|> norm_num
            <|> aesop
            linarith
          have h₁ : P.card * 2 = 2 ^ Fintype.card S := by
            have h₁ : P.card + Q.card = 2 ^ Fintype.card S := h₁
            have h₁ : P.card = Q.card := h₁
            linarith
          have h₁ : Fintype.card S ≥ 1 := by
            have h₁ : Nonempty S := inferInstance
            have h₁ : 0 < Fintype.card S := by
              apply Fintype.card_pos_iff.mpr
              exact (Classical.choice h₁)
            omega
          have h₁ : P.card = 2 ^ (Fintype.card S - 1) := by
            have h₁ : P.card * 2 = 2 ^ Fintype.card S := h₁
            have h₁ : Fintype.card S ≥ 1 := h₁
            have h₁ : 2 ^ (Fintype.card S - 1) * 2 = 2 ^ Fintype.card S := by
              have h₁ : Fintype.card S - 1 + 1 = Fintype.card S := by
                have h₁ : Fintype.card S ≥ 1 := h₁
                omega
            calc
            2 ^ (Fintype.card S - 1) * 2 = 2 ^ (Fintype.card S - 1) * 2 ^ 1 :=
              by norm_num
            = 2 ^ ((Fintype.card S - 1) + 1) := by
              rw [← pow_add]
            = 2 ^ Fintype.card S := by
              rw [h₁]
            <|> simp [add_comm]
          have h₁ : P.card = 2 ^ (Fintype.card S - 1) := by
            have h₁ : P.card * 2 = 2 ^ Fintype.card S := h₁
            have h₁ : 2 ^ (Fintype.card S - 1) * 2 = 2 ^ Fintype.card S := h₁
            have h₁ : P.card = 2 ^ (Fintype.card S - 1) := by
              linarith
            exact h₁
          exact h₁
          exact h₁
        })
      <|> (try
        {
          exact h_card
        })
      <|> (try
        {
          -- Simplified Proof
          import Mathlib
          import Aesop

          set_option maxHeartbeats 0

          open Set Function Filter Topology

          theorem putnam1964_b2
            (S : Type*) [Fintype S] [Nonempty S]
            (P : Finset (Set S))
            (hPP : ∀ T ⊆ P, ∀ U ∈ P, T ∩ U ≠ ∅)
            (hPS : ¬ T : Set S, T ∈ P ∧ (∀ U ∈ P, T ∩ U ≠ ∅))
            : (P.card = 2 ^ (Fintype.card S - 1)) := by
              have h_subset_or_compl : ∀ (A : Set S), A ∈ P ∨ A' ∈ P := by
                intro A
                by_contra h

```



```

obtain (h1, h2) := h
have h1 : A ∉ P := h1
have h2 : A ∉ P := h2
have h3 : (U : Set S), U ∈ P ∧ A ∩ U = ∅ := by
  have h3 : ¬(A ∈ P ∧ ∃ (U : Set S), U ∈ P → A ∩ U ≠ ∅) := by
    intro h3
    have h4 : ∃ (T : Set S), T ∈ P ∧ (∀ U ∈ P, T ∩ U ≠ ∅) := by
      refine' (A, ∅)
      constructor
      · exact h3.1
      · intro U hU
        have h4 := h3.2 U hU
        exact h4
    exact hPS h3
  by_cases h3 : A ∈ P
  · have h3 : ¬(∀ (U : Set S), U ∈ P → A ∩ U ≠ ∅) := by
      intro h3
      exact h3 (h1, h2)
    push_neg at h3
    obtain (U, hU, hU') := h3
    refine' (U, hU, ∅)
    have h4 : A ∩ U = ∅ := by
      by_contra h4
      have h4 : A ∩ U ≠ ∅ := h4
      simp_all [Set.ext_iff]
    exfalse
  · simp_all
have h4 : ∃ (V : Set S), V ∈ P ∧ A ∩ V = ∅ := by
have h4 : ¬(A ∈ P ∧ ∃ (U : Set S), U ∈ P → A ∩ U ≠ ∅) := by
  intro h4
  have h4 : ∃ (T : Set S), T ∈ P ∧ (∀ U ∈ P, T ∩ U ≠ ∅) := by
    refine' (A, ∅)
    constructor
    · exact h4.1
    · intro U hU
      have h4 := h4.2 U hU
      exact h4
  exact hPS h4
  by_cases h4 : A ∈ P
  · have h4 : ¬(∀ (U : Set S), U ∈ P → A ∩ U ≠ ∅) := by
      intro h4
      exact h4 (h1, h2, h3)
    push_neg at h4
    obtain (V, hV, hV') := h4
    refine' (V, hV, ∅)
    have h4 : A ∩ V = ∅ := by
      by_contra h4
      have h4 : A ∩ V ≠ ∅ := h4
      simp_all [Set.ext_iff]
    exfalse
  · simp_all
obtain (U, hU, hU') := h4
obtain (V, hV, hV') := h4
have h5 : U ⊆ A' := by
  intro x hx
  by_contra h5
  have h5 : x ∈ A := by simp_all [Set.mem_compl_iff]
  have h5 : x ∈ A ∩ U := Set.mem_inter h5 hx
  rw [hU'] at h5
  simp at h5
have h5 : V ⊆ A := by
  intro x hx
  by_contra h5
  have h5 : x ∈ A' := by simp_all [Set.mem_compl_iff]
  have h5 : x ∈ A ∩ V := Set.mem_inter h5 hx
  rw [hV'] at h5
  simp at h5
have h5 : U ∩ V = ∅ := by
  apply Set.eq_empty_of_forall_not_mem
  intro x hx
  have h5 : x ∈ U := Set.mem_of_mem_inter_left hx
  have h5 : x ∈ V := Set.mem_of_mem_inter_right hx
  have h5 : x ∈ A' := h5 h5
  have h5 : x ∈ A := h5 h5
  simp_all [Set.mem_compl_iff]
have h5 : U ∩ V ≠ ∅ := hPP U hU V hV
simp_all [Set.ext_iff]
have h5 : (A : Set S), A ∈ P → A' ∈ P := by
  intro A hA
  by_contra h5
  have h5 : A' ∈ P := h5
  have h5 : A ∩ A' = ∅ := by
    ext x
    simp [Set.mem_inter_iff]
  have h5 : A ∩ A' ≠ ∅ := hPP A hA A' h5
  contradiction
have h5 : P.card = 2 ^ (Fintype.card S - 1) := by
  classical
  let Q : Finset (Set S) := (Finset.univ : Finset (Set S)) \ P
  have h5 : P.card = Q.card := by
    have h5 : ∃ (A : Set S), A ∈ P → A' ∈ Q := by
      intro A hA
      have h5 : A' ∈ (Finset.univ : Finset (Set S)) := Finset.mem_univ _
      have h5 : A' ∈ P := h5
      simp only [Q, Finset.mem_sdiff] at h5
      tauto
    have h5 : ∃ (A : Set S), A ∈ Q → A' ∈ P := by
      intro A hA
      have h5 : A ∈ (Finset.univ : Finset (Set S)) := by
        simp only [Q, Finset.mem_sdiff] at hA
        tauto
      have h5 : A ∈ P := by
        simp only [Q, Finset.mem_sdiff] at hA
        tauto
      have h5 : A ∈ (Finset.univ : Finset (Set S)) := by tauto
      have h5 : A ∈ P ∨ A' ∈ P := h_subset_or_compl A
      cases h5 with
      | inl h5 =>
        | inl h5 =>
          tauto
        | inr h5 =>
          exact h5
      have h5 : P.card = Q.card := by
        have h5 : P.card = Q.card := by

```

```

have h13 : m ≠ 0 := by linarith
have h14 : m - 1 ≠ 0 := by linarith
field_simp [h13, h14]
<> ring_nf
<> field_simp [h13, h14]
<> nlinarith
exact h12

have h_main_backward : (∃ n, u ^ n + v ^ n = 1 ∧ m-1 + n-1 = 1) → (x > 0)
→ (y > 0), u * x + v * y = 1 ∧ x ^ m + y ^ n = 1 ∧ u = x ^ (m - 1) ∧ v =
→ y ^ (n - 1) := by
intro h
rcases h with ⟨n, hn, hv⟩
have h1 : m - 1 > 0 := by linarith
have h2 : (m : ℝ) ≠ 1 := by linarith
have h3 : (m - 1 : ℝ) ≠ 0 := by linarith
have h4 : n = m / (m - 1) := by
have h5 : m-1 + n-1 = 1 := hn
have h6 : n ≠ 0 := by
by_contra h
rw [h] at h
have h7 : (m : ℝ)-1 + (0 : ℝ)-1 = 1 := by simp using h
norm_num at h <>
(try { contradiction }) <>
(try { linarith })
have h8 : m ≠ 0 := by linarith
field_simp [h7, h8] at h
nlinarith [mul_pos hu hv, mul_pos (sub_pos.mpr hn) (sub_pos.mpr hm)]

have h9 : n - 1 = 1 / (m - 1) := by
rw [h]
field_simp [h]
<> ring_nf
<> field_simp [h]
<> nlinarith
have h10 : 0 < u := hu
have h11 : 0 < v := hv
have h12 : 0 < u ^ (n - 1) := Real.rpow_pos_of_pos h10 (n - 1)
have h13 : 0 < v ^ (n - 1) := Real.rpow_pos_of_pos h11 (n - 1)
use u ^ (n - 1), h12, v ^ (n - 1), h13
constructor
have h14 : u * (u ^ (n - 1)) + v * (v ^ (n - 1)) = u ^ n + v ^ n := by
have h15 : u * (u ^ (n - 1)) = u ^ n := by
have h16 : u * (u ^ (n - 1)) = u ^ (1 : ℝ) * u ^ (n - 1) := by
→ norm_num
rw [h15]
have h17 : (u : ℝ) ^ (1 : ℝ) * u ^ (n - 1) = u ^ ((1 : ℝ) + (n - 1))
→ := by
rw [- Real.rpow_add (by positivity)]
rw [h16]
have h18 : (1 : ℝ) + (n - 1) = n := by ring
rw [h17]
have h19 : v * (v ^ (n - 1)) = v ^ n := by
have h20 : v * (v ^ (n - 1)) = v ^ (1 : ℝ) * v ^ (n - 1) := by
→ norm_num
rw [h19]
have h21 : (v : ℝ) ^ (1 : ℝ) * v ^ (n - 1) = v ^ ((1 : ℝ) + (n - 1))
→ := by
rw [- Real.rpow_add (by positivity)]
rw [h20]
have h22 : (1 : ℝ) + (n - 1) = n := by ring
rw [h21]
linarith
have h23 : u ^ n + v ^ n = 1 := hn
linarith
constructor
have h24 : (u ^ (n - 1)) ^ m = u ^ n := by
calc
(u ^ (n - 1)) ^ m = u ^ ((n - 1) * m) := by
rw [- Real.rpow_mul (le_of_lt hu)]
<> ring_nf
= u ^ n := by
have h25 : (n - 1 : ℝ) * m = n := by
rw [h]
field_simp [h]
<> ring_nf
<> field_simp [h]
<> nlinarith
rw [h25]
have h26 : (v ^ (n - 1)) ^ m = v ^ n := by
calc
(v ^ (n - 1)) ^ m = v ^ ((n - 1) * m) := by
rw [- Real.rpow_mul (le_of_lt hv)]
<> ring_nf
= v ^ n := by
have h27 : (n - 1 : ℝ) * m = n := by
rw [h]
field_simp [h]
<> ring_nf
<> field_simp [h]
<> nlinarith
rw [h27]
calc
(u ^ (n - 1)) ^ m + (v ^ (n - 1)) ^ m = u ^ n + v ^ n := by rw [h26,
→ h23]
= 1 := hn
constructor
have h28 : (u ^ (n - 1)) ^ (m - 1) = u := by
calc
(u ^ (n - 1)) ^ (m - 1) = u ^ ((n - 1) * (m - 1)) := by
rw [- Real.rpow_mul (le_of_lt hu)]
<> ring_nf
= u := by
have h29 : (n - 1 : ℝ) * (m - 1) = 1 := by
rw [h]
field_simp [h]
<> ring_nf
<> field_simp [h]
<> nlinarith
rw [h29]
<> simp [Real.rpow_one]

linarith
have h30 : (v ^ (n - 1)) ^ (m - 1) = v := by
calc
(v ^ (n - 1)) ^ (m - 1) = v ^ ((n - 1) * (m - 1)) := by
rw [- Real.rpow_mul (le_of_lt hv)]
<> ring_nf
= v := by
have h31 : (n - 1 : ℝ) * (m - 1) = 1 := by
rw [h]
field_simp [h]
<> ring_nf
<> field_simp [h]
<> nlinarith
rw [h31]
<> simp [Real.rpow_one]

linarith
exact h_final

-- Simplified Proof
import Mathlib
import Aesop

set_option maxHeartbeats 0

open EuclideanGeometry Topology Filter Complex

theorem putnam_1965_a6
(u v m : ℝ)
(hu : 0 < u)
(hv : 0 < v)
(hm : 1 < m) :
(x > 0) (y > 0),
u * x + v * y = 1 ∧
x ^ m + y ^ n = 1 ∧
u = x ^ (m - 1) ∧
v = y ^ (n - 1) ↔
∃ n, u ^ n + v ^ n = 1 ∧ m-1 + n-1 = 1 := by
constructor
rintro ⟨x, hx, y, hy, h1, h2, h3, h4⟩
use m / (m - 1)
constructor
· calc
u ^ (m / (m - 1)) + v ^ (m / (m - 1)) = (x ^ (m - 1)) ^ (m / (m - 1)) +
→ (y ^ (m - 1)) ^ (m / (m - 1)) := by rw [h1, h2]
= x ^ m + y ^ n := by
have h5 : (m - 1 : ℝ) * (m / (m - 1)) = m := by
field_simp [sub_ne_zero.mpr hm.ne']
rw [- Real.rpow_mul (le_of_lt hx), - Real.rpow_mul (le_of_lt hy), h3]
= 1 := by rw [h4]
field_simp [sub_ne_zero.mpr hm.ne']
rintro m, hn, hn2
have h6 : m - 1 > 0 := by linarith
have h7 : (m : ℝ) ≠ 1 := by linarith
have h8 : (m - 1 : ℝ) ≠ 0 := by linarith
have h9 : n = m / (m - 1) := by
have h10 : m-1 + n-1 = 1 := hn
have h11 : n ≠ 0 := by
by_contra h
rw [h] at h
have h12 : (m : ℝ)-1 + (0 : ℝ)-1 = 1 := by simp using h
norm_num at h <> (try { contradiction })
have h13 : m ≠ 0 := by linarith
field_simp [h9, h10] at h
nlinarith [mul_pos hu hv, mul_pos (sub_pos.mpr hn) (sub_pos.mpr hm)]
use u ^ (n - 1), Real.rpow_pos_of_pos hu (n - 1), v ^ (n - 1),
→ Real.rpow_pos_of_pos hv (n - 1)
constructor
· have h14 : u * (u ^ (n - 1)) + v * (v ^ (n - 1)) = u ^ n + v ^ n := by
have h15 : u * (u ^ (n - 1)) = u ^ n := by
calc
u * (u ^ (n - 1)) = u ^ (1 : ℝ) * u ^ (n - 1) := by norm_num
= u ^ ((1 : ℝ) + (n - 1)) := by rw [- Real.rpow_add (by
→ positivity)]
= u ^ n := by simp
have h16 : v * (v ^ (n - 1)) = v ^ n := by
calc
v * (v ^ (n - 1)) = v ^ (1 : ℝ) * v ^ (n - 1) := by norm_num
= v ^ ((1 : ℝ) + (n - 1)) := by rw [- Real.rpow_add (by
→ positivity)]
= v ^ n := by simp
linarith
linarith
· constructor
· have h17 : (u ^ (n - 1)) ^ m = u ^ n := by
calc
(u ^ (n - 1)) ^ m = u ^ ((n - 1) * m) := by rw [- Real.rpow_mul
→ (le_of_lt hu)]
= u ^ n := by
have h18 : (n - 1 : ℝ) * m = n := by
rw [h]
field_simp [h]
rw [h]
have h19 : (v ^ (n - 1)) ^ m = v ^ n := by
calc
(v ^ (n - 1)) ^ m = v ^ ((n - 1) * m) := by rw [- Real.rpow_mul
→ (le_of_lt hv)]
= v ^ n := by
have h20 : (n - 1 : ℝ) * m = n := by
rw [h]
field_simp [h]
rw [h]
linarith
· constructor

```

```

have h0 : (u ~ (n - 1)) ^ (m - 1) u := by
  calc
    (u ~ (n - 1)) ^ (m - 1) = u ~ ((n - 1) * (m - 1)) := by rw [-
      Real.rpow_mul (le_of_lt hu)]
    = u := by
      have h0 : (n - 1 : ℝ) * (m - 1) = 1 := by
        rw [h1]
        field_simp [h1]
        <|> simp [Real.rpow_one]
      linarith
    have h0 : (v ~ (n - 1)) ^ (m - 1) = v := by
      calc
        (v ~ (n - 1)) ^ (m - 1) = v ~ ((n - 1) * (m - 1)) := by rw [-
          Real.rpow_mul (le_of_lt hv)]
        = v := by
          have h0 : (n - 1 : ℝ) * (m - 1) = 1 := by
            rw [h1]
            field_simp [h1]
            <|> simp [Real.rpow_one]
          linarith
    -----
    -- Orig Proof
    import Mathlib
    import Aesop
    set_option maxHeartbeats 0
    open EuclideanGeometry Topology Filter Complex

    theorem putnam_1965_b2
    (n : ℕ)
    (hn : n > 1)
    (won : Fin n → Fin n → Bool)
    (hirrefl : ∀ i : Fin n, won i i = False)
    (hantisymm : ∀ i j : Fin n, i ≠ j → won i j = !won j i)
    (w1 : Fin n → z)
    (hw : w = fun r : Fin n => z j : Fin n, (if won r j then 1 else 0))
    (hl : l = fun r : Fin n => n - 1 - w r)
    : z r : Fin n, (w r)^2 = z r : Fin n, (l r)^2 := by
      have h0 : 2 * (z r : Fin n, (w r : z)) = n * (n - 1 : z) := by
        have h1 : (z i : Fin n, z j : Fin n, (if won i j then (1 : z) else 0)) = z
          : r : Fin n, (w r : z) := by
            calc
              (z i : Fin n, z j : Fin n, (if won i j then (1 : z) else 0)) = z i :
                Fin n, z j : Fin n, (if won i j then (1 : z) else 0) := rfl
              = z i : Fin n, (z j : Fin n, (if won i j then (1 : z) else 0)) := by
                simp [Finset.sum_sigma']
              = z i : Fin n, (w i : z) := by
                apply Finset.sum_congr rfl
                intro i
                rw [hw]
                <|> simp [Finset.sum_congr]
                <|> rfl
              = z r : Fin n, (w r : z) := by simp [Finset.sum_congr]
            have h2 : (z i : Fin n, z j : Fin n, (if won j i then (1 : z) else 0)) = z
              : r : Fin n, (w r : z) := by
                calc
                  (z i : Fin n, z j : Fin n, (if won j i then (1 : z) else 0)) = z j :
                    Fin n, z i : Fin n, (if won i j then (1 : z) else 0) := by
                      rw [Finset.sum_comm]
                  = z j : Fin n, (z i : Fin n, (if won j i then (1 : z) else 0)) := by
                    simp [Finset.sum_sigma']
                  = z j : Fin n, (w j : z) := by
                    apply Finset.sum_congr rfl
                    intro j
                    rw [hw]
                    <|> simp [Finset.sum_congr]
                    <|> rfl
                  = z r : Fin n, (w r : z) := by simp [Finset.sum_congr]
                have h3 : (z i : Fin n, z j : Fin n, (if won i j then (1 : z) else 0) +
                  (if won j i then (1 : z) else 0)) = (n : z) * (n - 1 : z) := by
                  have h4 : ∀ (i j : Fin n), (if won i j then (1 : z) else 0) + (if won j i
                    then (1 : z) else 0) = if i = j then 0 else 1 := by
                    intro i j
                    by_cases h : i = j
                    ·
                      simp [h, hirrefl]
                      <|> norm_num
                    ·
                      have h5 : won i j = !won j i := hantisymm i j h
                      have h6 : (if won i j then (1 : z) else 0) + (if won j i then (1 : z
                        else 0) = 1 := by
                        split_ifs <|> simp.all [h5, Bool.not_eq_true]
                        <|> norm_num <|> try contradiction
                      simp [h, h6]
                  calc
                    (z i : Fin n, z j : Fin n, ((if won i j then (1 : z) else 0) + (if won
                      j i then (1 : z) else 0))) = z i : Fin n, z j : Fin n, (if i = j then
                        0 else 1 : z) := by
                      apply Finset.sum_congr rfl
                      intro i
                      apply Finset.sum_congr rfl
                      intro j
                      rw [h4 i j]
                      = z i : Fin n, z j : Fin n, (if i = j then 0 else 1 : z) := rfl
                      = (n : z) * (n - 1 : z) := by
                        calc
                          (z i : Fin n, z j : Fin n, (if i = j then 0 else 1 : z)) = z i :
                            Fin n, (z j : Fin n, (if i = j then 0 else 1 : z)) := by simp
                            [Finset.sum_sigma']
                          = z i : Fin n, (n - 1 : z) := by
                            apply Finset.sum_congr rfl
                            intro i
                            calc
                              (z j : Fin n, (if i = j then 0 else 1 : z)) = z j : Fin n, (if
                                i = j then 0 else 1 : z) := rfl
                              = (n - 1 : z) := by
                                calc
                                  (z j : Fin n, (if i = j then 0 else 1 : z)) = z j : Fin n,
                                    ((if i = j then 0 else 1 : z)) = z j : Fin n,
                                      ((if i = j then 1 else 0 : z)) := by
                                        rw [h1]
                                        <|> ring_nf
                                        <|> norm_cast
                                        <|> simp [Finset.sum_sub_distrib]
                                        <|> ring_nf
                                        <|> norm_cast
                                        <|> simp [nsmul_eq_mul]
                                        <|> ring_nf
                                        <|> norm_cast
                                        <|> simp [nsmul_eq_mul]
                                        <|> ring_nf
                                        <|> norm_cast
                                        <|> simp [Finset.sum_const, Finset.card_fin]
                                        <|> ring_nf
                                        <|> norm_cast
                                        <|> simp [Finset.sum_sub_distrib]
                                        <|> ring_nf
                                        <|> norm_cast
                                        <|> simp [nsmul_eq_mul]
                                        <|> ring_nf
                                        <|> norm_cast
                                        <|> simp [Finset.sum_const, Finset.card_fin]
                                        <|> ring_nf
                                        <|> norm_cast
                                        <|> simp [nsmul_eq_mul]
                                        <|> ring_nf
                                        <|> norm_cast
                                        <|> simp [Finset.sum_const, Finset.card_fin]
                                        <|> ring_nf
                                        <|> norm_cast
                                        <|> simp [nsmul_eq_mul]
                                        <|> ring_nf
                                        <|> norm_cast
                                        <|> simp [Finset.sum_const, Finset.card_fin]
                                        <|> ring_nf
                                        <|> norm_cast
                                        <|> simp [nsmul_eq_mul]
                                        <|> ring_nf
                                        <|> norm_cast
                                        <|> simp [Finset.sum_const, Finset.card_fin]
                                        <|> ring_nf
                                        <|> norm_cast
                                        <|> simp [nsmul_eq_mul]
                                        <|> ring_nf
                                        <|> norm_cast
                                        <|> simp [Finset.sum_const, Finset.card_fin]
                                        <|> ring_nf
                                        <|> norm_cast
                                        <|> simp [nsmul_eq_mul]
                                        <|> ring_nf
                                        <|> norm_cast
                                        <|> simp [Finset.sum_const, Finset.card_fin]
                                        <|> ring_nf
                                        <|> norm_cast
                                        <|> simp [nsmul_eq_mul]
                                        <|> ring_nf
                                        <|> norm_cast
                                        <|> simp [Finset.sum_const, Finset.card_fin]
                                        <|> ring_nf
                                        <|> norm_cast
                                        <|> simp [nsmul_eq_mul]
                                        <|> ring_nf
                                        <|> norm_cast
                                        <|> simp [Finset.sum_const, Finset.card_fin]
                                        <|> ring_nf
                                        <|> norm_cast
                                        <|> simp [nsmul_eq_mul]
                                        <|> ring_nf
                                        <|> norm_cast
                                        <|> simp [Finset.sum_const, Finset.card_fin]
                                        <|> ring_nf
                                        <|> norm_cast
                                        <|> simp [nsmul_eq_mul]
                                        <|> ring_nf
                                        <|> norm_cast
                                        <|> simp [Finset.sum_const, Finset.card_fin]
                                        <|> ring_nf
                                        <|> norm_cast
                                        <|> simp [nsmul_eq_mul]
                                        <|> ring_nf
                                        <|> norm_cast
                                        <|> simp [Finset.sum_const, Finset.card_fin]
                                        <|> ring_nf
                                        <|> norm_cast
                                        <|> simp [nsmul_eq_mul]
                                        <|> ring_nf
                                        <|> norm_cast
                                        <|> simp [Finset.sum_const, Finset.card_fin]
                                        <|> ring_nf
                                        <|> norm_cast
                                        <|> simp [nsmul_eq_mul]
                                        <|> ring_nf
                                        <|> norm_cast
                                        <|> simp [Finset.sum_const, Finset.card_fin]
                                        <|> ring_nf
                                        <|> norm_cast
                                        <|> simp [nsmul_eq_mul]
                                        <|> ring_nf
                                        <|> norm_cast
                                        <|> simp [Finset.sum_const, Finset.card_fin]
                                        <|> ring_nf
                                        <|> norm_cast
                                        <|> simp [nsmul_eq_mul]
                                        <|> ring_nf
                                        <|> norm_cast
                                        <|> simp [Finset.sum_const, Finset.card_fin]
                                        <|> ring_nf
                                        <|> norm_cast
                                        <|> simp [nsmul_eq_mul]
                                        <|> ring_nf
                                        <|> norm_cast
                                        <|> simp [Finset.sum_const, Finset.card_fin]
                                        <|> ring_nf
                                        <|> norm_cast
                                        <|> simp [nsmul_eq_mul]
                                        <|> ring_nf
                                        <|> norm_cast
                                        <|> simp [Finset.sum_const, Finset.card_fin]
                                        <|> ring_nf
                                        <|> norm_cast
                                        <|> simp [nsmul_eq_mul]
                                        <|> ring_nf
                                        <|> norm_cast
                                        <|> simp [Finset.sum_const, Finset.card_fin]
                                        <|> ring_nf
                                        <|> norm_cast
                                        <|> simp [nsmul_eq_mul]
                                        <|> ring_nf
                                        <|> norm_cast
                                        <|> simp [Finset.sum_const, Finset.card_fin]
                                        <|> ring_nf
                                        <|> norm_cast
                                        <|> simp [nsmul_eq_mul]
                                        <|> ring_nf
                                        <|> norm_cast
                                        <|> simp [Finset.sum_const, Finset.card_fin]
                                        <|> ring_nf
                                        <|> norm_cast
                                        <|> simp [nsmul_eq_mul]
                                        <|> ring_nf
                                        <|> norm_cast
                                        <|> simp [Finset.sum_const, Finset.card_fin]
                                        <|> ring_nf
                                        <|> norm_cast
                                        <|> simp [nsmul_eq_mul]
                                        <|> ring_nf
                                        <|> norm_cast
                                        <|> simp [Finset.sum_const, Finset.card_fin]
                                        <|> ring_nf
                                        <|> norm_cast
                                        <|> simp [nsmul_eq_mul]
                                        <|> ring_nf
                                        <|> norm_cast
                                        <|> simp [Finset.sum_const, Finset.card_fin]
                                        <|> ring_nf
                                        <|> norm_cast
                                        <|> simp [nsmul_eq_mul]
                                        <|> ring_nf
                                        <|> norm_cast
                                        <|> simp [Finset.sum_const, Finset.card_fin]
                                        <|> ring_nf
                                        <|> norm_cast
                                        <|> simp [nsmul_eq_mul]
                                        <|> ring_nf
                                        <|> norm_cast
                                        <|> simp [Finset.sum_const, Finset.card_fin]
                                        <|> ring_nf
                                        <|> norm_cast
                                        <|&gt
```

```

linarith
have h_final_nat :  $\mathbb{E} r : \text{Fin } n, (w r)^2 = \mathbb{E} r : \text{Fin } n, (l r)^2 := \text{by}$ 
  norm_cast at h_final
  <> simp_all [Finset.sum_congr]
  <>
  (try omega) <>
  (try ring_nf at <>) linarith)

exact h_final_nat
-- Simplified Proof
import Mathlib
import Aesop

set_option maxHeartbeats 0

open EuclideanGeometry Topology Filter Complex

theorem putnam_1965_b2
(n : ℕ)
(hn : n > 1)
(won :  $\text{Fin } n \rightarrow \text{Fin } n \rightarrow \text{Bool}$ )
(hirrefl :  $\forall i : \text{Fin } n, \text{won } i \ i = \text{False}$ )
(hantisymm :  $\forall i \ j : \text{Fin } n, i \neq j \rightarrow \text{won } i \ j = \neg \text{won } j \ i$ )
(w l :  $\text{Fin } n \rightarrow \mathbb{Z}$ )
(hw :  $w = \text{fun } r : \text{Fin } n \Rightarrow \sum j : \text{Fin } n, (\text{if } \text{won } r \ j \text{ then } 1 \text{ else } 0)$ )
(hl :  $l = \text{fun } r : \text{Fin } n \Rightarrow n - 1 - w r$ )
:  $\mathbb{E} r : \text{Fin } n, (w r)^2 = \mathbb{E} r : \text{Fin } n, (l r)^2 := \text{by}$ 
  have h₁ :  $\forall r : \text{Fin } n, l r = n - 1 - w r := \text{by simp [hl]}$ 
  have h₂ :  $\mathbb{E} r : \text{Fin } n, (l r)^2 = \mathbb{E} r : \text{Fin } n, ((n - 1 : \mathbb{Z}) - w r)^2 := \text{by}$ 
    apply Finset.sum_congr rfl
    intro r _
    rw [h₁]
  have h₃ :  $\mathbb{E} r : \text{Fin } n, ((n - 1 : \mathbb{Z}) - w r)^2 = \mathbb{E} r : \text{Fin } n, ((n - 1 : \mathbb{Z})^2 -$ 
     $\rightarrow 2 * (n - 1 : \mathbb{Z}) * w r + (w r)^2) := \text{by}$ 
    apply Finset.sum_congr rfl
    intro r _
    ring_nf
  have h₄ :  $\mathbb{E} r : \text{Fin } n, ((n - 1 : \mathbb{Z})^2 - 2 * (n - 1 : \mathbb{Z}) * w r + (w r)^2) = (n$ 
     $\rightarrow : \mathbb{Z}) * (n - 1 : \mathbb{Z})^2 - 2 * (n - 1 : \mathbb{Z}) * (\mathbb{E} r : \text{Fin } n, w r) + (\mathbb{E} r :$ 
     $\rightarrow \text{Fin } n, (w r)^2) := \text{by}$ 
    simp [Finset.sum_add_distrib, Finset.sum_sub_distrib, Finset.sum_mul,
     $\rightarrow \text{Finset.mul_sum, mul_assoc, mul_comm, mul_left_comm}]$ 
  have h₅ :  $\mathbb{E} r : \text{Fin } n, (l r)^2 = \mathbb{E} r : \text{Fin } n, (w r)^2 := \text{by}$ 
    rw [h₄, h₃, h₁]
  have h₆ :  $2 * (\mathbb{E} r : \text{Fin } n, w r) = (n : \mathbb{Z}) * (n - 1 : \mathbb{Z}) := \text{by}$ 
    have h₆₁ :  $(\mathbb{E} i : \text{Fin } n, \sum j : \text{Fin } n, (\text{if } \text{won } i \ j \text{ then } (1 : \mathbb{Z}) \text{ else } 0)) = \sum$ 
       $\rightarrow r : \text{Fin } n, w r := \text{by}$ 
      simp [Finset.sum_sigma', hw]
    have h₆₂ :  $(\mathbb{E} i : \text{Fin } n, \sum j : \text{Fin } n, (\text{if } \text{won } j \ i \text{ then } (1 : \mathbb{Z}) \text{ else } 0)) = \sum$ 
       $\rightarrow r : \text{Fin } n, w r := \text{by}$ 
      calc
      (  $\mathbb{E} i : \text{Fin } n, \sum j : \text{Fin } n, (\text{if } \text{won } j \ i \text{ then } (1 : \mathbb{Z}) \text{ else } 0) = \sum j :$ 
         $\rightarrow \text{Fin } n, \sum i : \text{Fin } n, (\text{if } \text{won } j \ i \text{ then } (1 : \mathbb{Z}) \text{ else } 0) := \text{by}$ 
        rw [Finset.sum_comm]
      ) =  $\sum j : \text{Fin } n, (\mathbb{E} i : \text{Fin } n, (\text{if } \text{won } j \ i \text{ then } (1 : \mathbb{Z}) \text{ else } 0)) :=$ 
         $\rightarrow \text{by simp [Finset.sum_sigma']}$ 
      ) =  $\sum j : \text{Fin } n, w j := \text{by}$ 
        apply Finset.sum_congr rfl
        intro j _
        rw [hw]
      ) =  $\mathbb{E} r : \text{Fin } n, w r := \text{by simp [Finset.sum_congr]}$ 
    have h₆₃ :  $(\mathbb{E} i : \text{Fin } n, \sum j : \text{Fin } n, ((\text{if } \text{won } i \ j \text{ then } (1 : \mathbb{Z}) \text{ else } 0) +$ 
       $\rightarrow (\text{if } \text{won } j \ i \text{ then } (1 : \mathbb{Z}) \text{ else } 0))) = (n : \mathbb{Z}) * (n - 1 : \mathbb{Z}) := \text{by}$ 
      have h₆₃₁ :  $\forall (i \ j : \text{Fin } n), (\text{if } \text{won } i \ j \text{ then } (1 : \mathbb{Z}) \text{ else } 0) + (\text{if } \text{won}$ 
         $\rightarrow j \ i \text{ then } (1 : \mathbb{Z}) \text{ else } 0) = \text{if } i = j \text{ then } 0 \text{ else } 1 := \text{by}$ 
        intro i j
        by_cases h : i = j
        · simp [h, hirrefl]
        · have h₆₃₁₁ :  $\text{won } i \ j = \neg \text{won } j \ i := \text{hantisymm } i \ j \ h$ 
          have h₆₃₁₂ :  $(\text{if } \text{won } i \ j \text{ then } (1 : \mathbb{Z}) \text{ else } 0) + (\text{if } \text{won } j \ i \text{ then } (1 :$ 
             $\rightarrow \mathbb{Z}) \text{ else } 0) = 1 := \text{by}$ 
            split_ifs <> simp_all [h₆₃₁₁, Bool.not_eq_true]
          simp [h, h₆₃₁₁]
        calc
        (  $\mathbb{E} i : \text{Fin } n, \sum j : \text{Fin } n, (((\text{if } \text{won } i \ j \text{ then } (1 : \mathbb{Z}) \text{ else } 0) + (\text{if}$ 
           $\rightarrow \text{won } j \ i \text{ then } (1 : \mathbb{Z}) \text{ else } 0))) = \sum i : \text{Fin } n, \sum j : \text{Fin } n, (\text{if } i = j$ 
           $\rightarrow \text{then } 0 \text{ else } 1 : \mathbb{Z}) := \text{by}$ 
          then 0 else 1 :  $\mathbb{Z}) := \text{by}$ 
          apply Finset.sum_congr rfl
          intro i _
          apply Finset.sum_congr rfl
          intro j _
          rw [h₆₃₁₂]
        ) =  $\sum i : \text{Fin } n, (\mathbb{E} j : \text{Fin } n, (\text{if } i = j \text{ then } 0 \text{ else } 1 : \mathbb{Z})) := \text{rfl}$ 
        ) =  $\sum i : \text{Fin } n, (n - 1 : \mathbb{Z}) := \text{by}$ 
        apply Finset.sum_congr rfl
        intro i _
        calc
        (  $\mathbb{E} j : \text{Fin } n, (\text{if } i = j \text{ then } 0 \text{ else } 1 : \mathbb{Z}) = \sum j : \text{Fin } n, ((1 : \mathbb{Z})$ 
           $\rightarrow - (\text{if } i = j \text{ then } 1 \text{ else } 0 : \mathbb{Z})) := \text{by}$ 
          apply Finset.sum_congr rfl
          intro j _
          by_cases h : i = j <> simp [h]
          -  $(\mathbb{E} j : \text{Fin } n, (1 : \mathbb{Z}) - 1 : \mathbb{Z}) := \text{by}$ 
            rw [Finset.sum_sub_distrib]
            <> simp [Finset.sum_ite_eq', Finset.mem_univ, i.is_lt]
          -  $(n : \mathbb{Z}) - 1 := \text{by simp [Finset.sum_const, Finset.card_fin]}$ 
          -  $(n : \mathbb{Z}) - 1 := \text{by rfl}$ 
          -  $(n : \mathbb{Z}) * (n - 1 : \mathbb{Z}) := \text{by}$ 
            simp [Finset.sum_const, Finset.card_fin]
          <> ring_nf
        ) =  $2 * (\mathbb{E} r : \text{Fin } n, w r) = (n : \mathbb{Z}) * (n - 1 : \mathbb{Z}) := \text{by}$ 
        calc
         $2 * (\mathbb{E} r : \text{Fin } n, w r) = (\mathbb{E} i : \text{Fin } n, \sum j : \text{Fin } n, (\text{if } \text{won } i \ j \text{ then}$ 
           $\rightarrow (1 : \mathbb{Z}) \text{ else } 0)) + (\mathbb{E} i : \text{Fin } n, \sum j : \text{Fin } n, (\text{if } \text{won } j \ i \text{ then } (1 : \mathbb{Z})$ 
           $\rightarrow \text{else } 0)) := \text{by}$ 
          rw [h₆, h₅]
        <> ring
        ) =  $(\mathbb{E} i : \text{Fin } n, \sum j : \text{Fin } n, ((\text{if } \text{won } i \ j \text{ then } (1 : \mathbb{Z}) \text{ else } 0) +$ 
           $\rightarrow (\text{if } \text{won } j \ i \text{ then } (1 : \mathbb{Z}) \text{ else } 0))) := \text{by}$ 
          simp [Finset.sum_add_distrib]

```

```

- = (n :  $\mathbb{Z}$ ) * (n - 1 :  $\mathbb{Z}$ ) := by rw [h₁]
exact h₁
have h₂ :  $2 * (n - 1 : \mathbb{Z}) * (\mathbb{E} r : \text{Fin } n, w r) = (n : \mathbb{Z}) * (n - 1 : \mathbb{Z})^2 :=$ 
   $\rightarrow \text{by}$ 
  calc
   $2 * (n - 1 : \mathbb{Z}) * (\mathbb{E} r : \text{Fin } n, w r) = (n - 1 : \mathbb{Z}) * (2 * (\mathbb{E} r : \text{Fin } n,$ 
     $\rightarrow w r)) := \text{by ring}$ 
  - =  $(n - 1 : \mathbb{Z}) * ((n : \mathbb{Z}) * (n - 1 : \mathbb{Z})) := \text{by rw [h₁]}$ 
  - =  $(n : \mathbb{Z}) * (n - 1 : \mathbb{Z})^2 := \text{by ring}$ 
linarith
simp_all
-----
-- Orig Proof
import Mathlib
import Aesop

set_option maxHeartbeats 0

open EuclideanGeometry Topology Filter Complex

theorem putnam_1965_b3
:  $\{(a, b, c) : \mathbb{Z} \times \mathbb{Z} \times \mathbb{Z} \mid a > 0 \wedge a \leq b \wedge c > 0 \wedge a^2 + b^2 = c^2 \wedge a \cdot b / (2 : \mathbb{Q})$ 
   $\rightarrow \} = 2 * (a + b + c) \}. \text{ncard} = 3 := \text{by}$ 
  have h_main :  $\{(a, b, c) : \mathbb{Z} \times \mathbb{Z} \times \mathbb{Z} \mid a > 0 \wedge a \leq b \wedge c > 0 \wedge a^2 + b^2 =$ 
     $\rightarrow c^2 \wedge a \cdot b / (2 : \mathbb{Q}) = 2 * (a + b + c)\} = \{(9, 40, 41), (10, 24, 26),$ 
     $\rightarrow (12, 16, 20)\} := \text{by}$ 
  apply Set.Subset.antisymm
  intro (a, b, c) h
  simp only [Set.mem_setOf_eq, Set.mem_insert_iff, Set.mem_singleton_iff]
  at h
  have h₁ :  $a > 0 := h.1$ 
  have h₂ :  $a \leq b := h.2.1$ 
  have h₃ :  $c > 0 := h.2.2.1$ 
  have h₄ :  $a^2 + b^2 = c^2 := h.2.2.2.1$ 
  have h₅ :  $(a * b : \mathbb{Q}) / 2 = 2 * (a + b + c : \mathbb{Q}) := \text{by exact\_mod\_cast}$ 
     $\rightarrow h.2.2.2.2$ 
  have h₆ :  $(a : \mathbb{Q}) * b = 4 * (a + b + c : \mathbb{Q}) := \text{by}$ 
    have h₆₁ :  $(a : \mathbb{Q}) * b / 2 = 2 * (a + b + c : \mathbb{Q}) := h₅$ 
    have h₆₂ :  $(a : \mathbb{Q}) * b = 4 * (a + b + c : \mathbb{Q}) := \text{by}$ 
      ring_nf at h₆₁
      linarith
  exact h₆
  have h₇ :  $(a : \mathbb{Z}) * b = 4 * (a + b + c) := \text{by}$ 
    norm_cast at h₆
    <>
    (try norm_num at h₆) <>
    (try ring_nf at h₆) <>
    (try field_simp at h₆) <>
    (try norm_cast at h₆) <>
    (try linarith) <>
    (try
      {
        norm_num at h₆
        <>
        (try ring_nf at h₆)
        <>
        (try norm_cast at h₆)
        <>
        (try linarith)
      }) <>
    (try
      {
        simp_all [mul_comm, mul_assoc, mul_left_comm]
        <>
        nlinarith
      })
    <>
    (try omega)
  have h₈ :  $a + b - c = 8 := \text{by}$ 
    have h₈₁ :  $(a : \mathbb{Z}) * b = 4 * (a + b + c) := h₆$ 
    have h₈₂ :  $(a + b : \mathbb{Z}) ^ 2 = (a : \mathbb{Z}) ^ 2 + (b : \mathbb{Z}) ^ 2 + 2 * (a : \mathbb{Z}) *$ 
       $\rightarrow b := \text{by ring}$ 
    have h₈₃ :  $(a + b : \mathbb{Z}) ^ 2 = (c : \mathbb{Z}) ^ 2 + 2 * (a : \mathbb{Z}) * b := \text{by}$ 
      nlinarith
    have h₈₄ :  $(a + b : \mathbb{Z}) ^ 2 = (c : \mathbb{Z}) ^ 2 + 8 * (a + b + c) := \text{by}$ 
      nlinarith
    have h₈₅ :  $(a + b - c : \mathbb{Z}) * (a + b + c : \mathbb{Z}) = 8 * (a + b + c : \mathbb{Z}) := \text{by}$ 
      nlinarith
    have h₈₆ :  $(a + b + c : \mathbb{Z}) > 0 := \text{by}$ 
      nlinarith
    have h₈₇ :  $(a + b - c : \mathbb{Z}) = 8 := \text{by}$ 
      apply mul_left_cancel₀ (show  $(a + b + c : \mathbb{Z}) \neq 0$  by linarith)
      nlinarith
    linarith
  have h₉ :  $a \leq 49 := \text{by}$ 
    nlinarith [sq_nonneg (a - b)]
  have h₁₀ :  $(a = 9 \wedge b = 40 \wedge c = 41) \vee (a = 10 \wedge b = 24 \wedge c = 26) \vee (a =$ 
     $\rightarrow 12 \wedge b = 16 \wedge c = 20) := \text{by}$ 
    have h₁₀₁ :  $a > 0 := h₁$ 
    have h₁₀₂ :  $a \leq b := h₂$ 
    have h₁₀₃ :  $c > 0 := h₃$ 
    have h₁₀₄ :  $a^2 + b^2 = c^2 := h₄$ 
    have h₁₀₅ :  $(a : \mathbb{Z}) * b = 4 * (a + b + c) := h₆$ 
    have h₁₀₆ :  $a + b - c = 8 := h₈$ 
    have h₁₀₇ :  $a \leq 49 := h₉$ 
    have h₁₀₈ :  $a \geq 1 := \text{by linarith}$ 
    have h₁₀₉ :  $b \geq 1 := \text{by}$ 
      nlinarith
    have h₁₁₀ :  $c \geq 1 := \text{by linarith}$ 
  interval_cases a <>
  (try omega) <>
  (try {
    have h₁₁₁ :  $b \geq 1 := \text{by nlinarith}$ 
    have h₁₁₂ :  $b \leq 100 := \text{by}$ 
      nlinarith
    interval_cases b <>
    (try omega) <>
    (try {

```

```

have h1,1 : c ≥ 1 := by nlinarith
have h1,1 : c ≤ 100 := by
  nlinarith
interval_cases c <>
  (try omega) <>
  (try {
    norm_num at h1,1 h1,1 h1,1 <>
    (try omega) <>
    (try nlinarith)
  })
  })
  }) <>
  (try {
    norm_num at h1,1 h1,1 h1,1 <>
    (try omega) <>
    (try nlinarith)
  })
  })
  (try {
    aesop
  })
rcases h1,1 with (rfl, rfl, rfl) | (rfl, rfl, rfl) | (rfl, rfl, rfl) <>
  norm_num <>
  (try simp_all) <>
  (try norm_num) <>
  (try aesop)

intro (a, b, c) h
simp only [Set.mem_setOfEq, Set.mem_insert_iff, Set.mem_singleton_iff]
  at h
rcases h with (rfl, rfl, rfl) | (rfl, rfl, rfl) | (rfl, rfl, rfl)
  norm_num [pow_two]
  <>
  (try norm_num) <>
  (try ring_nf) <>
  (try field_simp) <>
  (try norm_cast) <>
  (try linarith)

  norm_num [pow_two]
  <>
  (try norm_num) <>
  (try ring_nf) <>
  (try field_simp) <>
  (try norm_cast) <>
  (try linarith)

  norm_num [pow_two]
  <>
  (try norm_num) <>
  (try ring_nf) <>
  (try field_simp) <>
  (try norm_cast) <>
  (try linarith)

have h_final : {(a, b, c) : z × z × z | a > 0 ∧ a ≤ b ∧ c > 0 ∧ a^2 + b^2 =
  → c^2 ∧ a*b/(2 : q) = 2*(a + b + c)}.ncard = 3 := by
  rw [h_main]
  norm_num
  <>
  (try decide) <>
  (try {
    {
      simp [Set.ncard_insert_of_not_mem, Set.mem_singleton_iff]
      <>
      norm_num
      <>
      decide
    }
  })
  <>
  (try {
    {
      simp [Set.ncard_singleton]
    }
  })

exact h_final

-- Simplified Proof
import Mathlib
import Aesop

set_option maxHeartbeats 0

open EuclideanGeometry Topology Filter Complex

theorem putnam_1965_b3
: {(a, b, c) : z × z × z | a > 0 ∧ a ≤ b ∧ c > 0 ∧ a^2 + b^2 = c^2 ∧ a*b/(2 : q)
  → } = 2*(a + b + c)}.ncard = 3 := by
  have h : {(a, b, c) : z × z × z | a > 0 ∧ a ≤ b ∧ c > 0 ∧ a^2 + b^2 = c^2 ∧
  → a*b/(2 : q) = 2*(a + b + c)} =
  { (9, 40, 41), (10, 24, 26), (12, 16, 20) } := by
  ext (a, b, c)
  constructor
  · rintro (h1, h2, h3, h4)
    field_simp at h1
    norm_cast at h1
    have : a + b - c = 8 := by nlinarith
    have : a ≤ 49 := by nlinarith [sq_nonneg (a - b)]
    interval_cases a <> norm_num at * <> omega
    rintro (rfl, rfl, rfl) | (rfl, rfl, rfl) | (rfl, rfl, rfl) <> norm_num
  · rw [h]
    norm_num

-- Orig Proof
import Mathlib
import Aesop

set_option maxHeartbeats 0

theorem putnam_1966_a1
(f : z → z)
(hf : f = fun n : z => x m in Finset.Icc 0 n, (if Even m then m / 2 else (m -
  → 1)/2))
: ∀ x y : z, x > 0 ∧ y > 0 ∧ x > y → x * y = f (x + y) - f (x - y) := by

```

```

have h_main_lemma : ∀ (a b : z), (a + 4 * b) / 4 = a / 4 + b := by
  intro a b
  have h1 : (a + 4 * b) / 4 = a / 4 + b := by
    have h1 : a + 4 * b = 4 * (a / 4 + b) + (a % 4) := by
      have h1 := Int.emod_add_ediv a 4
      ring_nf at h1
      <> omega
    have h1 : (a + 4 * b) / 4 = a / 4 + b := by
      rw [h1]
    have h1 : a % 4 = 0 ∨ a % 4 = 1 ∨ a % 4 = 2 ∨ a % 4 = 3 := by
      have h1 := Int.emod_add_ediv a 4
      omega
    rcases h1 with (h1 | h1 | h1 | h1) <>
      simp [h1, Int.add_emod, Int.mul_emod, Int.emod_emod] <>
      (try omega) <>
      (try {
        norm_num at *
        <>
        omega
      }) <>
      (try {
        ring_nf at *
        <>
        omega
      })
    exact h1
  exact h

have h_nat_sum : ∀ (n : ℕ), (x m in Finset.range (n + 1), (m : z) / 2) = (n :
  → z) ^ 2 / 4 := by
  intro n
  have h1 : (x m in Finset.range (n + 1), (m : z) / 2) = (n : z) ^ 2 / 4 := by
    have h1 : ∀ n : ℕ, (x m in Finset.range (n + 1), (m : z) / 2) = (n : z) ^
    → 2 / 4 := by
      intro n
      induction n with
      | zero =>
        norm_num [Finset.sum_range_succ]
      | succ n ih =>
        rw [Finset.sum_range_succ, ih]
        cases' Nat.even_or_odd n with h h <>
        cases' h with k hk <>
        simp [hk, pow_two, Int.add_emod, Int.mul_emod, Int.emod_emod,
        → Int.ediv_eq_zero_of_lt] <>
        ring_nf at * <>
        (try { norm_num at * }) <>
        (try {
          have h1 : (n : z) ≥ 0 := by positivity
          have h1 : (k : z) ≥ 0 := by positivity
          ring_nf at *
          <>
          norm_cast at *
          <>
          omega
        }) <>
        (try {
          field_simp at *
          <>
          ring_nf at *
          <>
          norm_cast at *
          <>
          omega
        }) <>
        (try {
          simp_all [Int.emod_eq_of_lt]
          <>
          ring_nf at *
          <>
          norm_cast at *
          <>
          omega
        })
      })
    exact h1 n
  exact h

have h_nonneg_int_sum : ∀ (n : z), n ≥ 0 → (x m in Finset.Icc 0 n, (m : z) /
  → 2) = n ^ 2 / 4 := by
  intro n hn
  have h1 : (x m in Finset.Icc 0 n, (m : z) / 2) = (x m in Finset.range
  → (n.toNat + 1), (m : z) / 2) := by
  have h1 : Finset.Icc 0 n = Finset.image (fun x : ℕ => (x : z))
  → (Finset.range (n.toNat + 1)) := by
  apply Finset.ext
  intro x
  simp only [Finset.mem_Icc, Finset.mem_image, Finset.mem_range]
  constructor
  · intro hx
    have h1 : 0 ≤ x := hx.1
    have h1 : x ≤ n := hx.2
    have h1 : x ≥ 0 := by linarith
    have h1 : (x : z) ≥ 0 := by exact_mod_cast h1
    have h1 : x ≤ n := by exact_mod_cast h1
    have h1 : x.toNat < n.toNat + 1 := by
      have h1 : x.toNat ≤ n.toNat := by
      have h1 : (x : z) ≤ n := by exact_mod_cast h1
      have h1 : x.toNat ≤ n.toNat := by
      simp_all [Int.toNat_of_nonneg, Int.le_of_lt_add_one]
      <>
      omega
    exact h1
  · omega
  refine' (x.toNat, _)
  constructor
  · exact h1
  · have h1 : (x.toNat : z) = x := by
      rw [Int.toNat_of_nonneg (by linarith)]
      linarith

```

```

intro hx
rcases hx with (a, ha, rfl)
have h0 : (a : z) < n.toNat + 1 := by exact_mod_cast ha
have h1 : (a : z) ≥ 0 := by
  have h10 : (a : ℕ) ≥ 0 := by positivity
  exact_mod_cast h10
have h2 : (a : z) ≤ n := by
  have h20 : (a : ℕ) < n.toNat + 1 := by exact_mod_cast ha
  have h21 : (a : ℕ) ≤ n.toNat := by
    omega
  have h22 : (a : z) ≤ n := by
    have h23 : (n : z) ≥ 0 := by exact_mod_cast hn
    have h24 : (a : ℕ) ≤ n.toNat := by exact_mod_cast h20
    have h25 : (a : z) ≤ n := by
      simp_all [Int.toNat_of_nonneg]
    <|>
    omega
  exact h22
exact h1
constructor <|>
(try norm_num) <|>
(try linarith)
<|>
(try omega)
rw [h1]

rw [Finset.sum_image]
<|>
(try { simp_all [Int.toNat_of_nonneg hn] }) <|>
(try {
  intros x _ y _ h
  simp_all [Int.toNat_of_nonneg (by omega : (0 : z) ≤ x),
    → Int.toNat_of_nonneg (by omega : (0 : z) ≤ y)]
  <|>
  omega
}) <|>
(try { simp_all [Int.toNat_of_nonneg hn] })
rw [h1]

have h2 : (x m in Finset.range (n.toNat + 1), (m : z) / 2) = (n.toNat : z)
  → 2 / 4 := by
  have h20 : (x m in Finset.range (n.toNat + 1), (m : z) / 2) = (n.toNat : z)
    → 2 / 4 := by
    apply h_nat_sum
  exact h20
rw [h2]

have h3 : (n.toNat : z) ^ 2 = n ^ 2 := by
  have h30 : n ≥ 0 := hn
  have h31 : (n.toNat : z) = n := by
    simp [Int.toNat_of_nonneg h30]
  rw [h31]
  <|>
  ring_nf
  <|>
  simp_all

have h4.f_eq : ∀ (n : z), n ≥ 0 → f n = n ^ 2 / 4 := by
  intro n hn
  have h40 : f n = x m in Finset.Icc 0 n, (if Even m then m / 2 else (m - 1) / 2) := by
    rw [hf]
  <|> simp [hn]
  rw [h40]
  have h41 : x m in Finset.Icc 0 n, (if Even m then m / 2 else (m - 1) / 2) = x
    → m in Finset.Icc 0 n, (m : z) / 2 := by
    apply Finset.sum_congr rfl
    intro m hm
    have h42 : m < Finset.Icc 0 n := hm
    have h43 : 0 ≤ m := by
      simp [Finset.mem_Icc] at h42
    linarith
  have h44 : (if Even m then m / 2 else (m - 1) / 2) = (m : z) / 2 := by
    by_cases h45 : Even m
    · simp [h45]
    <|>
    (try {
      have h46 : (m : z) % 2 = 0 := by
        rw [Int.even_iff] at h45
        omega
      have h47 : (m : z) / 2 + 2 = m := by
        have h48 : (m : z) % 2 = 0 := h46
        have h49 : (m : z) = 2 * ((m : z) / 2) := by
          omega
        linarith
        omega
      omega
    })
    have h46 : ¬Even m := h45
    have h47 : (m : z) % 2 = 1 := by
      rw [Int.even_iff] at h45
    have h48 : (m : z) % 2 ≠ 0 := by
      intro h49
      apply h47
      omega
    have h49 : (m : z) % 2 = 1 ∨ (m : z) % 2 = -1 := by
      have h50 : (m : z) % 2 = 0 ∨ (m : z) % 2 = 1 ∨ (m : z) % 2 = -1 := by
        omega
      rcases h50 with (h51 | h52 | h53) <|>
      (try { contradiction }) <|>
      (try { omega }) <|>
      (try { exact Or.inl h51 }) <|>
      (try { exact Or.inr h53 })
    cases h49 with
    | inl h50 => exact h49
    | inr h50 =>
      have h51 : (m : z) % 2 = 1 := by
        omega
      exact h51
  have h45 : (m : z) / 2 + 2 = m := by
    have h46 : (m : z) % 2 = 1 := h47
    have h47 : (m : z) % 2 = 2 * ((m : z) / 2) + 1 := by
      omega
    linarith

→ by
  omega
  rcases h41 with (h41 | h42 | h43) <|>
  (try { contradiction }) <|>
  (try { omega }) <|>
  (try { exact Or.inl h41 }) <|>
  (try { exact Or.inr h43 })
  cases h41 with
  | inl h44 => exact h44
  | inr h44 =>
    have h45 : (m : z) % 2 = 1 := by
      omega
    exact h45
  have h46 : (m : z) / 2 + 2 = m := by
    have h47 : (m : z) % 2 = 1 := h46
    have h48 : (m : z) % 2 = 2 * ((m : z) / 2) + 1 := by
      omega
    linarith

simp [h4, h41]
<|>
(try {
  intro x y h
  have h41 : x > 0 := h.1
  have h42 : y > 0 := h.2.1
  have h43 : x > y := h.2.2
  have h44 : x + y > 0 := by linarith
  have h45 : x - y > 0 := by linarith
  have h46 : f (x + y) = (x + y) ^ 2 / 4 := by
    have h47 : (x + y : z) ≥ 0 := by linarith
    have h48 : f (x + y) = (x + y : z) ^ 2 / 4 := by
      apply h47.eq
    <|> linarith
  exact h46
  have h49 : f (x - y) = (x - y) ^ 2 / 4 := by
    have h50 : (x - y : z) ≥ 0 := by linarith
    have h51 : f (x - y) = (x - y : z) ^ 2 / 4 := by
      apply h50.eq
    <|> linarith
  exact h49
  have h52 : (x + y : z) ^ 2 / 4 - (x - y : z) ^ 2 / 4 = x * y := by
    have h53 : (x + y : z) ^ 2 = (x - y : z) ^ 2 + 4 * (x * y) := by
      ring_nf
    <|>
    linarith
  have h54 : ((x - y : z) ^ 2 + 4 * (x * y)) / 4 = (x - y : z) ^ 2 / 4 + x * y := by
    → y := by
      have h55 := h_main_lemma ((x - y : z) ^ 2) (x * y)
      ring_nf at h55
    <|>
    linarith
  have h56 : (x + y : z) ^ 2 / 4 = ((x - y : z) ^ 2 + 4 * (x * y)) / 4 := by
    rw [h53]
  have h57 : (x + y : z) ^ 2 / 4 = (x - y : z) ^ 2 / 4 + x * y := by
    linarith
  linarith
  have h58 : x * y = f (x + y) - f (x - y) := by
    rw [h56, h57]
    linarith
  exact h58
  intro x y h
  have h59 : x * y = f (x + y) - f (x - y) := h_final x y h
  exact h59
}
-- Simplified Proof
import Mathlib
import Aesop

set_option maxHeartbeats 0

theorem putnam_1966_a1
(f : z → z)
(hf : f = fun n : z => x m in Finset.Icc 0 n, (if Even m then m / 2 else (m - 1) / 2)) :
∀ x y : z, x > 0 ∧ y > 0 ∧ x > y → x * y = f (x + y) - f (x - y) := by
  have h_main_lemma : ∀ (a b : z), (a + 4 * b) / 4 = a / 4 + b := by
    intro a b
    omega
  have h_nat_sum : ∀ (n : ℕ), (x m in Finset.range (n + 1), (m : z) / 2) = (n : z)
    → z ^ 2 / 4 := by
    intro n
    induction n with
    | zero =>
      norm_num [Finset.sum_range_succ]
    | succ n ih =>
      rw [Finset.sum_range_succ, ih]
      cases' Nat.even_or_odd n with h h <|> cases' h with k hk <|> simp [hk,
        → pow_two, Int.add_emod, Int.mul_emod, Int.emod_emod,
        → Int.ediv_eq_zero_of_lt] <|> (try {
        have h60 : (n : z) ≥ 0 := by positivity
        have h61 : (k : z) ≥ 0 := by positivity
        ring_nf at *
        <|> norm_cast at *
        <|> omega
      })
  have h_nonneg_int_sum : ∀ (n : z), n ≥ 0 → (x m in Finset.Icc 0 n, (m : z) / 2) = (n : z)
    → z ^ 2 / 4 := by
    intro n hn
    have h62 : (x m in Finset.Icc 0 n, (m : z) / 2) = (x m in Finset.range
      → (n.toNat + 1), (m : z) / 2) := by
      have h63 : Finset.Icc 0 n = Finset.image (fun x : ℕ => (x : z))
        → (Finset.range (n.toNat + 1)) := by
        apply Finset.ext
        intro x
        simp only [Finset.mem_Icc, Finset.mem_image, Finset.mem_range]
      constructor
    intro hx
    have h64 : 0 ≤ x := hx.1
    have h65 : x ≤ n := hx.2
    have h66 : x ≥ 0 := by linarith
    have h67 : (x : z) ≥ 0 := by exact_mod_cast h66
    have h68 : x ≤ n := by exact_mod_cast h65
    have h69 : x.toNat < n.toNat + 1 := by
      have h70 : x.toNat ≤ n.toNat := by
        have h71 : (x : z) ≤ n := by exact_mod_cast h68
        have h72 : x.toNat ≤ n.toNat := by

```

```

      simp_all [Int.toNat_of_nonneg, Int.le_of_lt_add_one]
    exact h₁
  omega
  refine' (x.toNat, _)
  constructor
  exact h₁
  have h₃ : (x.toNat : z) = x := by
    rw [Int.toNat_of_nonneg (by linarith)]
  linarith
  intro hx
  rcases hx with (a, ha, rfl)
  have h₃ : (a : z) < n.toNat + 1 := by exact_mod_cast ha
  have h₄ : (a : z) ≥ 0 := by
    have h₄ : (a : ℕ) ≥ 0 := by positivity
    exact_mod_cast h₄
  have h₅ : (a : z) ≤ n := by
    have h₅ : (a : ℕ) < n.toNat + 1 := by exact_mod_cast ha
    have h₅ : (a : ℕ) ≤ n.toNat := by
      omega
    have h₅ : (a : z) ≤ n := by
      have h₅ : (n : z) ≥ 0 := by exact_mod_cast hn
      have h₅ : (a : ℕ) ≤ n.toNat := by exact_mod_cast h₅
      have h₅ : (a : z) ≤ n := by
        simp_all [Int.toNat_of_nonneg]
      exact h₅
    exact h₅
  constructor <|> (try norm_num) <|> (try linarith)
  rw [h₃]
  rw [Finset.sum_image]
  <|> (try { simp_all [Int.toNat_of_nonneg hn] })
  rw [h₃]
  have h₃ : (z m in Finset.range (n.toNat + 1), (m : z) / 2) = (n.toNat : z)
    → ^ 2 / 4 := by
    apply h_nat_sum
  rw [h₃]
  have h₃ : (n.toNat : z) ^ 2 = n ^ 2 := by
    have h₃ : n ≥ 0 := hn
    have h₃ : (n.toNat : z) = n := by
      simp [Int.toNat_of_nonneg h₃]
    rw [h₃]
  have h₃_eq : ∀ (n : z), n ≥ 0 → f n = n ^ 2 / 4 := by
    intro n hn
    have h₃ : f n = z m in Finset.Icc 0 n, (if Even m then m / 2 else (m - 1) / 2) := by
      rw [h₃]
    rw [h₃]
  have h₃ : z m in Finset.Icc 0 n, (if Even m then m / 2 else (m - 1) / 2) = z
    → m in Finset.Icc 0 n, (m : z) / 2 := by
    apply Finset.sum_congr rfl
    intro m hm
    have h₃ : m ∈ Finset.Icc 0 n := hm
    have h₃ : 0 ≤ m := by
      simp [Finset.mem_Icc] at h₃
    linarith
  have h₃ : (if Even m then m / 2 else (m - 1) / 2) = (m : z) / 2 := by
    by_cases h₃ : Even m
    · simp [h₃]
    · have h₃ : -Even m := h₃
      have h₃ : (m : z) % 2 = 1 := by
        rw [Int.even_iff] at h₃
      have h₃ : (m : z) % 2 ≠ 0 := by
        intro h₃
        apply h₃
        omega
      have h₃ : (m : z) % 2 = 1 ∨ (m : z) % 2 = -1 := by
        have h₃ : (m : z) % 2 = 0 ∨ (m : z) % 2 = 1 ∨ (m : z) % 2 = -1 := by
          by
            omega
            rcases h₃ with (h₃ | h₃ | h₃) <|> (try { contradiction }) <|>
        (try { omega })
      cases h₃ with
      | inl h₃ => exact h₃
      | inr h₃ =>
        have h₃ : (m : z) % 2 = 1 := by
          omega
        exact h₃
      have h₃ : (m : z) / 2 + 2 + 1 = m := by
        have h₃ : (m : z) % 2 = 1 := h₃
        have h₃ : (m : z) % 2 = 2 * ((m : z) / 2) + 1 := by
          omega
        linarith
      simp [h₃, h₃]
    <|> (try {
      omega
    })
  rw [h₃]
  rw [h₃]
  apply h_nonneg_int_sum
  <|> assumption
  intro x y h
  rw [h₃_eq (x + y) (by linarith), h₃_eq (x - y) (by linarith)]
  ring_nf
  omega
  -----
  -- Orig Proof
  import Mathlib
  import Aesop

  set_option maxHeartbeats 0

  open Topology Filter

  theorem putnam_1966_a5
  (C : Set (ℝ → ℝ))
  (hC : C = {f : ℝ → ℝ | Continuous f})
  (T : (ℝ → ℝ) → (ℝ → ℝ))
  (imageTC : ∀ f ∈ C, T f ∈ C)
  (linearT : ∀ a b : ℝ, ∀ f ∈ C, ∀ g ∈ C, T ((fun x => a)*f + (fun x => b)*g) =
    → (fun x => a)*(T f) + (fun x => b)*(T g))

```

```

  (localT : ∀ r s : ℝ, r ≤ s → ∀ f ∈ C, ∀ g ∈ C, (∀ x ∈ Set.Icc r s, f x = g x) →
    → (∀ x ∈ Set.Icc r s, T f x = T g x))
  : ∃ f ∈ C, ∀ g ∈ C, T g = f * g := by
  have h_one_in_C : (fun _ : ℝ => (1 : ℝ)) ∈ C := by
    rw [hC]
  exact continuous_const
  have h_f_def : T (fun _ : ℝ => (1 : ℝ)) ∈ C := by
    apply imageTC
    exact h_one_in_C
  have h_main : ∀ (g : ℝ → ℝ), g ∈ C → T g = T (fun _ : ℝ => (1 : ℝ)) * g := by
    intro g hg
    have h₁ : ∀ (x : ℝ), T g x = T (fun _ : ℝ => (1 : ℝ)) x * g x := by
      intro x
      let h : ℝ → ℝ := fun _ => g x
      have h₂ : h ∈ C := by
        rw [hC]
      exact continuous_const
    have h₂ : ∀ (y : ℝ), y ∈ Set.Icc x x → g y = h y := by
      intro y hy
      have h₂ : y = x := by
        simp [Set.mem_Icc] at hy
        linarith
      rw [h₂]
    <|> simp [h]
    have h₂ : ∀ (y : ℝ), y ∈ Set.Icc x x → T g y = T h y := by
      apply localT x x (by linarith) g hg h h₂
    have h₂ : T g x = T h x := by
      have h₂ : x ∈ Set.Icc x x := by
        exact (by linarith, by linarith)
      have h₂ : T g x = T h x := h₂ x h₂
      exact h₂
    have h₂ : T h = (fun _ : ℝ => g x) * T (fun _ : ℝ => (1 : ℝ)) := by
      have h₂ : (fun _ : ℝ => (0 : ℝ)) ∈ C := by
        rw [hC]
      exact continuous_const
      have h₂ : T ((fun _ : ℝ => g x) * (fun _ : ℝ => (1 : ℝ))) + (fun _ : ℝ =>
        → (0 : ℝ)) * (fun _ : ℝ => (0 : ℝ)) = (fun _ : ℝ => g x) * T (fun _ :
        → ℝ => (1 : ℝ)) + (fun _ : ℝ => (0 : ℝ)) * T (fun _ : ℝ => (0 : ℝ)) := by
        by
          apply linearT (g x) (0 : ℝ) (fun _ : ℝ => (1 : ℝ)) (by
            rw [hC])
          exact continuous_const (fun _ : ℝ => (0 : ℝ)) h₂
      have h₂ : (fun _ : ℝ => g x) * (fun _ : ℝ => (1 : ℝ)) + (fun _ : ℝ =>
        → (0 : ℝ)) * (fun _ : ℝ => (0 : ℝ)) = (fun _ : ℝ => g x) := by
        funext y
        simp [mul_comm]
        <|> ring_nf
        <|> norm_num
      have h₂ : (fun _ : ℝ => g x) * T (fun _ : ℝ => (1 : ℝ)) + (fun _ : ℝ =>
        → (0 : ℝ)) * T (fun _ : ℝ => (0 : ℝ)) = (fun _ : ℝ => g x) * T (fun _ :
        → ℝ => (1 : ℝ)) := by
        have h₂ : (fun _ : ℝ => (0 : ℝ)) * T (fun _ : ℝ => (0 : ℝ)) = (fun _ :
        → ℝ => (0 : ℝ)) := by
          funext y
          simp [mul_comm]
          <|> ring_nf
          <|> norm_num
        rw [h₂]
      have h₂ : (fun _ : ℝ => g x) * T (fun _ : ℝ => (1 : ℝ)) + (fun _ : ℝ =>
        → (0 : ℝ)) = (fun _ : ℝ => g x) * T (fun _ : ℝ => (1 : ℝ)) := by
        funext y
        simp [mul_comm]
        <|> ring_nf
        <|> norm_num
      rw [h₂]
    have h₂ : h = (fun _ : ℝ => g x) := by
      funext y
      simp [h]
    rw [h₂] at *
    rw [h₂] at h
    rw [h₂] at h
    exact h₂
  have h₂ : T h x = (fun _ : ℝ => g x) x * T (fun _ : ℝ => (1 : ℝ)) x := by
    rw [h₂]
    <|> simp [Pi.mul_apply]
    <|> ring_nf
  have h₂ : T h x = g x * T (fun _ : ℝ => (1 : ℝ)) x := by
    simp using h₂
  have h₂ : T g x = g x * T (fun _ : ℝ => (1 : ℝ)) x := by
    linarith
  linarith
  funext x
  have h₂ := h x
  simp [mul_comm] at h₂
  <|>
  (try ring_nf at h₂) <|>
  (try simp_all [Pi.mul_apply]) <|>
  (try linarith)
  <|>
  (try norm_num at h₂) <|>
  (try ring_nf at h₂) <|>
  (try simp_all [Pi.mul_apply]) <|>
  (try linarith)
  have h_final : ∃ f ∈ C, ∀ g ∈ C, T g = f * g := by
    refine' (T (fun _ : ℝ => (1 : ℝ)), h_f_def, _)
    intro g hg
    have h₁ : T g = T (fun _ : ℝ => (1 : ℝ)) * g := h_main g hg
    exact h₁
  exact h_final
  -----
  -- Simplified Proof
  import Mathlib
  import Aesop

  set_option maxHeartbeats 0

```

open Topology Filter

```

theorem putnam_1966_a5
(C : Set (ℝ → ℝ))
(hC : C = {f : ℝ → ℝ | Continuous f})
(T : (ℝ → ℝ) → (ℝ → ℝ))
(imageTC : ∀ f ∈ C, T f ∈ C)
(linearTC : ∀ a b : ℝ, ∀ f ∈ C, ∀ g ∈ C, T ((fun x => a)*f + (fun x => b)*g) =
  (fun x => a)*(T f) + (fun x => b)*(T g))
(localTC : ∀ r s : ℝ, r ≤ s → ∀ f ∈ C, ∀ g ∈ C, (∀ x ∈ Set.Icc r s, f x = g x) →
  (∀ x ∈ Set.Icc r s, T f x = T g x))
: ∃ f ∈ C, ∀ g ∈ C, T g = f * g := by
use T (fun _ : ℝ => 1)
constructor
· apply imageTC
  rw [hC]
  exact continuous_const
intro g hg
have h₁ : T g x = T (fun _ : ℝ => 1) x * g x := by
let h : ℝ → ℝ := fun _ => g x
have h₂ : h ∈ C := by
  rw [hC]
  exact continuous_const
have h₃ : ∀ y ∈ Set.Icc x x, g y = h y := by
  intro y hy
  simp [Set.mem_Icc] at hy
  simp [h, hy]
have h₄ : ∀ y ∈ Set.Icc x x, T g y = T h y := by
  apply localTC x x (by linarith) g hg h h₃
have h₅ : T g x = T h x := by
  have h₆ : x ∈ Set.Icc x x := by
    exact (by linarith, by linarith)
  exact h₆ x h₆
exact h₅ x h₅
have h₇ : T h = (fun _ : ℝ => g x) * T (fun _ : ℝ => 1) := by
  have h₈ : T ((fun _ : ℝ => g x) * (fun _ : ℝ => 1) + (fun _ : ℝ => 0) *
    (fun _ : ℝ => 0)) = (fun _ : ℝ => g x) * T (fun _ : ℝ => 1) + (fun _ :
    ℝ => 0) * T (fun _ : ℝ => 0) := by
    apply linearTC (g x) 0 (fun _ : ℝ => 1) (by
      rw [hC]
      exact continuous_const) (fun _ : ℝ => 0) (by
        rw [hC]
        exact continuous_const)
  have h₉ : (fun _ : ℝ => g x) * (fun _ : ℝ => 1) + (fun _ : ℝ => 0) * (fun
    _ : ℝ => 0) = (fun _ : ℝ => g x) := by
    funext x
    simp [mul_comm]
  have h₁₀ : (fun _ : ℝ => g x) * T (fun _ : ℝ => 1) + (fun _ : ℝ => 0) * T
    (fun _ : ℝ => 0) = (fun _ : ℝ => g x) * T (fun _ : ℝ => 1) := by
    funext x
    simp [mul_comm]
  rw [h₈] at h₇
  rw [h₈] at h₇
  exact h₇
have h₁₁ : T h x = (fun _ : ℝ => g x) x * T (fun _ : ℝ => 1) x := by
  rw [h₈]
  <|> simp [Pi.mul_apply]
simp at h₇
linarith
simp.all
-----
-- Orig Proof
import Mathlib
import Aesop

set_option maxHeartbeats 0

```

open Topology Filter

```

theorem putnam_1966_b6
(y : ℝ → ℝ)
(hy : Differentiable ℝ y ∧ Differentiable ℝ (deriv y))
(diffeq : deriv (deriv y) + Real.exp * y = 0)
: ∃ r s N : ℝ, ∀ x > N, r ≤ y x ∧ y x ≤ s := by
have h_main : ∃ (C : ℝ), ∀ (x : ℝ), x ≥ 0 → y x ^ 2 ≤ C := by
  have h₁ : Differentiable ℝ y := hy.1
  have h₂ : Differentiable ℝ (deriv y) := hy.2
  have h₃ : ∀ x : ℝ, deriv (deriv y) x + Real.exp x * y x = 0 := by
    intro x
    have h₄ := congr_fun diffex x
    simp [Real.exp_ne_zero] at h₄
    <|> ring_nf at h₄
    linarith

let F : ℝ → ℝ := fun x => y x ^ 2 + Real.exp (-x) * (deriv y x) ^ 2

have h : ∀ x : ℝ, deriv F x = -Real.exp (-x) * (deriv y x) ^ 2 := by
intro x
have h₁ : HasDerivAt F (-Real.exp (-x) * (deriv y x) ^ 2) x := by

  have h₂ : HasDerivAt (fun x : ℝ => y x ^ 2) (2 * y x * deriv y x) x :=
  by
    have h₃ : HasDerivAt y (deriv y x) x := by
      apply DifferentiableAt.hasDerivAt
    exact h₃.differentiableAt
    have h₄ : HasDerivAt (fun x : ℝ => y x ^ 2) (2 * y x * deriv y x) x :=
    by
      convert HasDerivAt.pow 2 h₃ using 1 <|> ring
    exact h₄
  have h₅ : HasDerivAt (fun x : ℝ => Real.exp (-x) * (deriv y x) ^ 2)
    (-Real.exp (-x) * (deriv y x) ^ 2 + Real.exp (-x) * (2 * (deriv y
    x) * deriv (deriv y) x)) x := by
    have h₆ : HasDerivAt (fun x : ℝ => Real.exp (-x)) (-Real.exp (-x)) x
    := by
      have h₇ : HasDerivAt (fun x : ℝ => Real.exp (-x)) (Real.exp (-x) *
        (-1 : ℝ)) x := by
        simp using (Real.hasDerivAt_exp (-x)).comp x (hasDerivAt_id x
        → |>.neg)
      convert h₇ using 1 <|> ring
    have h₈ : HasDerivAt (fun x : ℝ => (deriv y x) ^ 2) (2 * (deriv y x)
    * deriv (deriv y) x) x := by
      * deriv (deriv y) x) x := by
        have h₉ : HasDerivAt (fun x : ℝ => deriv y x) (deriv (deriv y) x)
        x := by
          apply DifferentiableAt.hasDerivAt

```

```

    exact h₉.differentiableAt
    have h₁₀ : HasDerivAt (fun x : ℝ => (deriv y x) ^ 2) (2 * (deriv y
    x) * deriv (deriv y) x) x := by
      convert HasDerivAt.pow 2 h₉ using 1 <|> ring
    exact h₁₀
  have h₁₁ : HasDerivAt (fun x : ℝ => Real.exp (-x) * (deriv y x) ^ 2)
    (-Real.exp (-x) * (deriv y x) ^ 2 + Real.exp (-x) * (2 * (deriv
    y x) * deriv (deriv y) x)) x := by
    convert h₁₀.mul h₁₁ using 1 <|> by
      (try ring_nf) <|>
      (try simp [Real.exp_neg]) <|>
      (try field_simp [Real.exp_ne_zero]) <|>
      (try ring_nf) <|>
      (try linarith)
    exact h₁₁
  have h₁₂ : HasDerivAt F (-Real.exp (-x) * (deriv y x) ^ 2) x := by
    have h₁₃ : HasDerivAt F (2 * y x * deriv y x + (-Real.exp (-x) *
    (deriv y x) ^ 2 + Real.exp (-x) * (2 * (deriv y x) * deriv (deriv y)
    x))) x := by
      convert h₅.add h₆ using 1 <|>
      (try simp [F]) <|>
      (try ring_nf) <|>
      (try field_simp [Real.exp_ne_zero]) <|>
      (try ring_nf) <|>
      (try linarith)
    have h₁₄ : 2 * y x * deriv y x + (-Real.exp (-x) * (deriv y x) ^ 2 +
    Real.exp (-x) * (2 * (deriv y x) * deriv (deriv y) x)) = -Real.exp
    (-x) * (deriv y x) ^ 2 := by
      have h₁₅ : deriv (deriv y) x = -Real.exp x * y x := by
        have h₁₆ := h₃
        have h₁₇ : deriv (deriv y) x + Real.exp x * y x = 0 := by simp
        using h₁₆
      linarith
    have h₁₈ : deriv F x = -Real.exp (-x) * (deriv y x) ^ 2 := by
      apply HasDerivAt.deriv
    exact h₁₈
  exact h₁₂

have h₂ : ∀ x : ℝ, deriv F x ≤ 0 := by
intro x
have h₃ : deriv F x = -Real.exp (-x) * (deriv y x) ^ 2 := h₂ x
rw [h₃]
have h₄ : Real.exp (-x) > 0 := Real.exp_pos (-x)
have h₅ : (deriv y x) ^ 2 ≥ 0 := by positivity
have h₆ : -Real.exp (-x) * (deriv y x) ^ 2 ≤ 0 := by
  linarith [h₄, h₅]
exact h₆

have h₃ : ∀ (x : ℝ), x ≥ 0 → F x ≤ F 0 := by
intro x hx
have h₄ : ∀ t : ℝ, deriv F t ≤ 0 := h₂
have h₅ : ContinuousOn F (Set.Icc 0 x) := by
  have h₆ : Continuous F := by
    have h₇ : Continuous (fun x : ℝ => y x ^ 2) := by
      exact Continuous.pow (h₃.continuous) 2
    have h₈ : Continuous (fun x : ℝ => Real.exp (-x) * (deriv y x) ^ 2)
    := by
      have h₉ : Continuous (fun x : ℝ => Real.exp (-x)) := by
        continuity
      have h₁₀ : Continuous (fun x : ℝ => (deriv y x) ^ 2) := by
        have h₁₁ : Continuous (deriv y) := h₃.continuous
        exact Continuous.pow h₁₁ 2
      exact h₁₀.mul h₉
    have h₁₂ : Continuous F := by
      have h₁₃ : F = (fun x : ℝ => y x ^ 2) + (fun x : ℝ => Real.exp (-x)
      * (deriv y x) ^ 2) := by
        funext x
        simp [F]
        <|> ring
      rw [h₁₃]
      exact h₁₃.add h₁₁
    exact h₁₂
  have h₁₃ : DifferentiableOn ℝ F (Set.Ioo 0 x) := by
    have h₁₄ : Differentiable ℝ F := by
      have h₁₅ : Differentiable ℝ (fun x : ℝ => y x ^ 2) := by
        exact Differentiable.pow h₃ 2
      have h₁₆ : Differentiable ℝ (fun x : ℝ => Real.exp (-x) * (deriv y x)
      ^ 2) := by
        have h₁₇ : Differentiable ℝ (fun x : ℝ => Real.exp (-x)) := by
          apply Differentiable.exp
          exact differentiable_id.neg
        have h₁₈ : Differentiable ℝ (fun x : ℝ => (deriv y x) ^ 2) := by
          have h₁₉ : Differentiable (deriv y) := h₃
          exact Differentiable.pow h₁₉ 2
        exact h₁₈.mul h₁₉
      have h₂₀ : Differentiable ℝ F := by
        have h₂₁ : F = (fun x : ℝ => y x ^ 2) + (fun x : ℝ => Real.exp (-x)
        * (deriv y x) ^ 2) := by
          funext x
          simp [F]
          <|> ring
        rw [h₂₁]
        exact h₂₁.add h₁₆
      exact h₂₀
    exact h₁₃.differentiableOn
  have h₁₄ : ∀ t ∈ Set.Ioo 0 x, deriv F t ≤ 0 := by
    intro t ht
    exact h₄ t
  have h₁₅ : F x ≤ F 0 := by
    by_cases h₁₆ : x = 0
    · rw [h₁₆]
    <|> simp
    · have h₁₇ : 0 < x := by
      contrapose! h₁₆
      linarith

```



```

have h4 : c ∈ Set.Ioo 0 x, deriv F c = (F x - F 0) / (x - 0) := by
  apply exists_deriv_eq_slope F
  <|> simp_all [h1.ne']
  <|> linarith
obtain (c, hc, hc') := h4
have h5 : deriv F c ≤ 0 := h4.c hc
have h6 : (F x - F 0) / (x - 0) ≤ 0 := by
  rw [hc']
  exact h5
have h7 : (x - 0 : ℝ) > 0 := by linarith
have h8 : F x - F 0 ≤ 0 := by
  have h9 : (F x - F 0) / (x - 0) ≤ 0 := h6
  have h10 : 0 < (x - 0 : ℝ) := by linarith
  have h11 : (F x - F 0) / (x - 0) * (x - 0) ≤ 0 * (x - 0) := by
    gcongr
  have h12 : (F x - F 0) / (x - 0) * (x - 0) = F x - F 0 := by
    field_simp [h11.ne']
  <|> ring
  rw [h12] at h11
  linarith
  linarith
exact h11
use F 0
intro x hx
have h1 : F x ≤ F 0 := h1.x hx
have h2 : y x ^ 2 ≤ F x := by
  have h3 : Real.exp (-x) * (deriv y x) ^ 2 := rfl
  have h4 : Real.exp (-x) * (deriv y x) ^ 2 ≥ 0 := by
    have h5 : Real.exp (-x) > 0 := Real.exp_pos (-x)
    have h6 : (deriv y x) ^ 2 ≥ 0 := by positivity
  linarith
  linarith
  linarith
have h_final : ∃ r s N : ℝ, ∀ x > N, r ≤ y x ∧ y x ≤ s := by
  obtain (C, hC) := h_main
  use -Real.sqrt C, Real.sqrt C, 0
  intro x hx
  have h1 : x ≥ 0 := by linarith
  have h2 : y x ^ 2 ≤ C := hC x h1
  have h3 : -Real.sqrt C ≤ y x := by
    have h4 : y x ^ 2 ≤ C := h2
    have h5 : Real.sqrt C ≥ 0 := Real.sqrt_nonneg C
    nlinarith [Real.sqrt_nonneg C, Real.sqrt (show 0 ≤ C by
      by_contra h
      have h6 : C < 0 := by linarith
      have h7 : y x ^ 2 ≤ C := h2
      have h8 : y x ^ 2 < 0 := by linarith
      have h9 : y x ^ 2 ≥ 0 := by positivity
      linarith)]
  have h1 : y x ≤ Real.sqrt C := by
    have h2 : y x ^ 2 ≤ C := h2
    have h3 : Real.sqrt C ≥ 0 := Real.sqrt_nonneg C
    nlinarith [Real.sqrt_nonneg C, Real.sqrt (show 0 ≤ C by
      by_contra h
      have h4 : C < 0 := by linarith
      have h5 : y x ^ 2 ≤ C := h2
      have h6 : y x ^ 2 < 0 := by linarith
      have h7 : y x ^ 2 ≥ 0 := by positivity
      linarith)]
  exact (h1, h3)
exact h_final
-- Simplified Proof
import Mathlib
import Aesop
set_option maxHeartbeats 0
open Topology Filter
theorem putnam_1966_b6
(y : ℝ → ℝ)
(hy : Differentiable ℝ y ∧ Differentiable ℝ (deriv y))
(diffeq : deriv (deriv y) + Real.exp y = 0)
: ∃ r s N : ℝ, ∀ x > N, r ≤ y x ∧ y x ≤ s := by
  have h_main : ∃ (C : ℝ), ∀ (x : ℝ), x ≥ 0 → y x ^ 2 ≤ C := by
    let F : ℝ → ℝ := fun x => y x ^ 2 + Real.exp (-x) * (deriv y x) ^ 2
    have h1 : ∀ x : ℝ, deriv F x = -Real.exp (-x) * (deriv y x) ^ 2 := by
      intro x
      simp only [F]
      have h2 : HasDerivAt (fun x : ℝ => y x ^ 2) (2 * y x * deriv y x) x := by
        have h3 : HasDerivAt y (deriv y x) x := by
          apply DifferentiableAt.hasDerivAt
        exact (hy.1).differentiableAt
      have h4 : HasDerivAt (fun x : ℝ => y x ^ 2) (2 * y x * deriv y x) x :=
        by
          convert HasDerivAt.pow 2 h3 using 1 <|> ring
      exact h2
      have h5 : HasDerivAt (fun x : ℝ => Real.exp (-x) * (deriv y x) ^ 2)
        (-Real.exp (-x) * (deriv y x) ^ 2 + Real.exp (-x) * (2 * (deriv y x)
          * deriv (deriv y) x)) x := by
        have h6 : HasDerivAt (fun x : ℝ => Real.exp (-x)) (-Real.exp (-x)) x :=
          by
            have h7 : HasDerivAt (fun x : ℝ => Real.exp (-x)) (Real.exp (-x) *
              (-1 : ℝ)) x := by
                simp using (Real.hasDerivAt_exp (-x)).comp x (hasDerivAt_id x
                  <|> ring)
            convert h7 using 1 <|> ring
            have h8 : HasDerivAt (fun x : ℝ => (deriv y x) ^ 2) (2 * (deriv y x) *
              deriv (deriv y) x) x := by
                have h9 : HasDerivAt (fun x : ℝ => deriv y x) (deriv (deriv y) x) x
                  := by
                    apply DifferentiableAt.hasDerivAt
                    exact (hy.2).differentiableAt
                have h10 : HasDerivAt (fun x : ℝ => (deriv y x) ^ 2) (2 * (deriv y x)
                  * deriv (deriv y) x) x := by
                    convert HasDerivAt.pow 2 h9 using 1 <|> ring
                exact h10
            have h11 : HasDerivAt (fun x : ℝ => Real.exp (-x) * (deriv y x) ^ 2)
              (-Real.exp (-x) * (deriv y x) ^ 2 + Real.exp (-x) * (2 * (deriv y
                x) * deriv (deriv y) x)) x := by
                convert h8.mul h11 using 1
  have h1 : c ∈ Set.Ioo 0 x, deriv F c = (F x - F 0) / (x - 0) := by
    apply exists_deriv_eq_slope F
    <|> simp_all [h1.ne']
    obtain (c, hc, hc') := h1
    have h2 : deriv F c ≤ 0 := h1.c hc
    have h3 : (F x - F 0) / (x - 0) ≤ 0 := by
      rw [hc']
      exact h2
    have h4 : (x - 0 : ℝ) > 0 := by linarith
    have h5 : F x - F 0 ≤ 0 := by
      have h6 : (F x - F 0) / (x - 0) ≤ 0 := h3
      have h7 : 0 < (x - 0 : ℝ) := by linarith
      have h8 : (F x - F 0) / (x - 0) * (x - 0) ≤ 0 * (x - 0) := by
        gcongr
      have h9 : (F x - F 0) / (x - 0) * (x - 0) = F x - F 0 := by
        field_simp [h7.ne']
      rw [h9] at h8
      linarith
      linarith
    exact h8
  use F 0
  intro x hx
  have h1 : F x ≤ F 0 := h1.x hx
  have h2 : y x ^ 2 ≤ F x := by
    have h3 : F x = y x ^ 2 + Real.exp (-x) * (deriv y x) ^ 2 := rfl
    have h4 : Real.exp (-x) * (deriv y x) ^ 2 ≥ 0 := by
      have h5 : Real.exp (-x) > 0 := Real.exp_pos (-x)
      have h6 : (deriv y x) ^ 2 ≥ 0 := by positivity
    nlinarith
  linarith
  linarith
  linarith
obtain (C, hC) := h_main
use -Real.sqrt C, Real.sqrt C, 0
intro x hx
have h1 : x ≥ 0 := by linarith
have h2 : y x ^ 2 ≤ C := hC x h1
have h3 : -Real.sqrt C ≤ y x := by
  have h4 : y x ^ 2 ≤ C := h2
  have h5 : Real.sqrt C ≥ 0 := Real.sqrt_nonneg C
  nlinarith [Real.sqrt_nonneg C, Real.sqrt (show 0 ≤ C by
    by_contra h
    have h6 : C < 0 := by linarith
    have h7 : y x ^ 2 ≤ C := h2
    have h8 : y x ^ 2 < 0 := by linarith
    have h9 : y x ^ 2 ≥ 0 := by positivity
    linarith)]
have h1 : y x ≤ Real.sqrt C := by
  have h2 : y x ^ 2 ≤ C := h2
  have h3 : Real.sqrt C ≥ 0 := Real.sqrt_nonneg C
  nlinarith [Real.sqrt_nonneg C, Real.sqrt (show 0 ≤ C by
    by_contra h
    have h4 : C < 0 := by linarith
    have h5 : y x ^ 2 ≤ C := h2
    have h6 : y x ^ 2 < 0 := by linarith
    have h7 : y x ^ 2 ≥ 0 := by positivity
    linarith)]
exact h1

```

```

have h1 : Real.sqrt C ≥ 0 := Real.sqrt_nonneg C
nlinarith [Real.sqrt_nonneg C, Real.sq_sqrt (show 0 ≤ C by
  by_contra h
    have h1 : C < 0 := by linarith
    have h2 : y x ^ 2 ≤ C := h1
    have h3 : y x ^ 2 < 0 := by linarith
    have h4 : y x ^ 2 ≥ 0 := by positivity
    linarith)]
exact ⟨h1, h1⟩
-----
-- Orig Proof
import Mathlib
import Aesop

set_option maxHeartbeats 0

open Nat Topology Filter

theorem putnam_1967_b2
  (p r A B C h a a : ℝ)
  (prbound : 0 ≤ p ∧ p ≤ 1 ∧ 0 ≤ r ∧ r ≤ 1)
  (id1 : ∃ x y : ℝ, (p * x + (1 - p) * y) ^ 2 = A * x ^ 2 + B * x * y + C * y ^ 2)
  (id2 : ∃ x y : ℝ, (p * x + (1 - p) * y) * (r * x + (1 - r) * y) = a * x ^ 2 + a
    → * x * y + a * y ^ 2)
  : max (max A B) C ≥ 4 / 9 ∧ max (max h a) a ≥ 4 / 9 := by
  have hA : A = p^2 := by
    have h1 := id1 1 0
    have h2 := id1 0 1
    have h3 := id1 1 1
    have h4 := id1 1 (-1)
    have h5 := id1 2 1
    have h6 := id1 (-1) 1
    ring_nf at h1 h2 h3 h4 h5 h6 ⊢
    nlinarith [sq_nonneg (p - 1)]

  have hB : B = 2*p*(1 - p) := by
    have h1 := id1 1 1
    have h2 := id1 1 (-1)
    have h3 := id1 2 1
    have h4 := id1 (-1) 1
    have h5 := id1 1 0
    have h6 := id1 0 1
    ring_nf at h1 h2 h3 h4 h5 h6 ⊢
    nlinarith [sq_nonneg (p - 1)]

  have hC : C = (1 - p)^2 := by
    have h1 := id1 1 0
    have h2 := id1 0 1
    have h3 := id1 1 1
    have h4 := id1 1 (-1)
    have h5 := id1 2 1
    have h6 := id1 (-1) 1
    ring_nf at h1 h2 h3 h4 h5 h6 ⊢
    nlinarith [sq_nonneg (p - 1)]

  have h_part_a : max (max A B) C ≥ 4 / 9 := by
    rw [hA, hB, hC]
    have h1 : p ≤ 1 := prbound.2.1
    have h2 : 0 ≤ p := prbound.1
    by_contra! h
    have h3 : p ^ 2 < 4 / 9 := by
      cases' le_total (p ^ 2) (2 * p * (1 - p)) with h4 h5 <|>
      cases' le_total (p ^ 2) ((1 - p) ^ 2) with h6 h7 <|>
      simp_all [max_eq_left, max_eq_right, le_refl, le_of_lt] <|>
      nlinarith
    have h8 : (1 - p) ^ 2 < 4 / 9 := by
      cases' le_total (p ^ 2) (2 * p * (1 - p)) with h9 h10 <|>
      cases' le_total (p ^ 2) ((1 - p) ^ 2) with h11 h12 <|>
      simp_all [max_eq_left, max_eq_right, le_refl, le_of_lt] <|>
      nlinarith
    have h13 : 2 * p * (1 - p) < 4 / 9 := by
      cases' le_total (p ^ 2) (2 * p * (1 - p)) with h14 h15 <|>
      cases' le_total (p ^ 2) ((1 - p) ^ 2) with h16 h17 <|>
      simp_all [max_eq_left, max_eq_right, le_refl, le_of_lt] <|>
      nlinarith
    have h18 : p > 1 / 3 := by
      nlinarith [sq_nonneg (p - 2 / 3)]
    have h19 : p < 2 / 3 := by
      nlinarith [sq_nonneg (p - 1 / 3)]
    have h20 : 2 * p * (1 - p) > 4 / 9 := by
      nlinarith [sq_nonneg (p - 1 / 3), sq_nonneg (p - 2 / 3)]
    linarith

  have h_part_b : max (max h a) a ≥ 4 / 9 := by
    have h21 : a = p * r := by
      have h22 := id2 1 0
      have h23 := id2 0 1
      have h24 := id2 1 1
      have h25 := id2 1 (-1)
      ring_nf at h22 h23 h24 h25 ⊢
      nlinarith [prbound.1, prbound.2.1, prbound.2.2]
    have h26 : a = p * r - 2 * p * r := by
      have h27 := id2 1 0
      have h28 := id2 0 1
      have h29 := id2 1 1
      have h30 := id2 1 (-1)
      ring_nf at h27 h28 h29 h30 ⊢
      nlinarith [prbound.1, prbound.2.1, prbound.2.2]
    have h31 : a = (1 - p) * (1 - r) := by
      have h32 := id2 1 0
      have h33 := id2 0 1
      have h34 := id2 1 1
      have h35 := id2 1 (-1)
      ring_nf at h32 h33 h34 h35 ⊢
      nlinarith [prbound.1, prbound.2.1, prbound.2.2]
    rw [h21, h26, h31]
    have h36 : 0 ≤ p := by linarith
    have h37 : p ≤ 1 := by linarith
    have h38 : 0 ≤ r := by linarith
    have h39 : r ≤ 1 := by linarith
    by_contra! h
    have h40 : p * r < 4 / 9 := by
      cases' le_total (p * r) (p + r - 2 * p * r) with h41 h42 <|>
      cases' le_total (p * r) ((1 - p) * (1 - r)) with h43 h44 <|>
      simp_all [max_eq_left, max_eq_right, le_refl, le_of_lt] <|>
      nlinarith
    have h45 : (1 - p) * (1 - r) < 4 / 9 := by
      cases' le_total (p * r) (p + r - 2 * p * r) with h46 h47 <|>
      cases' le_total (p * r) ((1 - p) * (1 - r)) with h48 h49 <|>
      simp_all [max_eq_left, max_eq_right, le_refl, le_of_lt] <|>
      nlinarith
    have h50 : p + r > 2 / 3 := by
      nlinarith [sq_nonneg (p - r)]
    have h51 : p * r > 1 / 9 := by
      nlinarith [sq_nonneg (p - r)]
    have h52 : p + r < 4 / 3 := by
      nlinarith [sq_nonneg (p - r)]
    have h53 : p + r > 4 / 3 := by
      nlinarith [sq_nonneg (p - r)]
    have h54 : p + r - 2 * p * r ≥ 4 / 9 := by
      nlinarith [sq_nonneg (p - r), sq_nonneg (p + r - 2 / 3)]
    linarith
  exact ⟨h_part_a, h_part_b⟩

-- Simplified Proof
import Mathlib
import Aesop

set_option maxHeartbeats 0

open Nat Topology Filter

theorem putnam_1967_b2
  (p r A B C h a a : ℝ)
  (prbound : 0 ≤ p ∧ p ≤ 1 ∧ 0 ≤ r ∧ r ≤ 1)
  (id1 : ∃ x y : ℝ, (p * x + (1 - p) * y) ^ 2 = A * x ^ 2 + B * x * y + C * y ^ 2)
  (id2 : ∃ x y : ℝ, (p * x + (1 - p) * y) * (r * x + (1 - r) * y) = a * x ^ 2 + a
    → * x * y + a * y ^ 2)
  : max (max A B) C ≥ 4 / 9 ∧ max (max h a) a ≥ 4 / 9 := by
  norm_num
  constructor <|>
  by_contra! <|>
  nlinarith [id1 1 0, id1 0 1, id1 1 1, id2 1 0, id2 0 1, id2 1 1, sq_nonneg
    → (p - r)]
  -----
  -- Orig Proof
  import Mathlib
  import Aesop

  set_option maxHeartbeats 0

  theorem putnam_1968_a1
  : 22/7 - Real.pi = ∫ x in (0)..1, x^4 * (1 - x)^4 / (1 + x^2) := by
  have h_main : (∫ x in (0)..1, x^4 * (1 - x)^4 / (1 + x^2)) = 22/7 - Real.pi
    := by
    have h1 : (∫ x in (0)..1, x^4 * (1 - x)^4 / (1 + x^2)) = (∫ x in (0)..1,
      → (x^6 - 4*x^5 + 5*x^4 - 4*x^2 + 4 : ℝ) - 4 / (1 + x^2)) := by
    have h2 : ∫ x in (0)..1, x^4 * (1 - x)^4 / (1 + x^2) = (x^6 - 4*x^5 + 5*x^4
      → - 4*x^2 + 4 : ℝ) - 4 / (1 + x^2) := by
      intro x
      have h3 : (1 + x^2 : ℝ) ≠ 0 := by nlinarith
      have h4 : x^4 * (1 - x)^4 = (x^6 - 4*x^5 + 5*x^4 - 4*x^2 + 4 : ℝ) * (1
        → + x^2 - 4 : ℝ) := by
        ring_nf
        <|>
        nlinarith [sq_nonneg (x ^ 2), sq_nonneg (x ^ 3), sq_nonneg (x - 1),
          → sq_nonneg (x + 1)]
      have h5 : x^4 * (1 - x)^4 / (1 + x^2) = ((x^6 - 4*x^5 + 5*x^4 - 4*x^2 +
        → 4 : ℝ) * (1 + x^2 - 4) / (1 + x^2)) := by
        rw [h3]
      rw [h4]
      field_simp [h3]
      <|> ring_nf
      <|> field_simp [h3]
      <|> ring_nf
    congr
    ext x
    rw [h5, x]
    rw [h4]

  have h6 : (∫ x in (0)..1, (x^6 - 4*x^5 + 5*x^4 - 4*x^2 + 4 : ℝ) - 4 / (1 +
    → x^2)) = (∫ x in (0)..1, (x^6 - 4*x^5 + 5*x^4 - 4*x^2 + 4 : ℝ)) - (∫ x
    → in (0)..1, (4 : ℝ) / (1 + x^2)) := by
    apply intervalIntegral.integral_sub
  .
    apply Continuous.intervalIntegrable
    continuity
  .
    apply Continuous.intervalIntegrable

  have h7 : Continuous (fun x : ℝ => (4 : ℝ) / (1 + x ^ 2)) := by
    apply Continuous.div
    exact continuous.const
    exact Continuous.add continuous.const (continuous_pow 2)
  . intro x
  have h8 : (1 + x ^ 2 : ℝ) ≠ 0 := by nlinarith
  exact h8
  exact h7
  rw [h6]

  have h9 : (∫ x in (0)..1, (x^6 - 4*x^5 + 5*x^4 - 4*x^2 + 4 : ℝ)) = (22 / 7
    → : ℝ) := by
    norm_num [integral_id, mul_comm]
  <|>
  ring_nf
  <|>
  norm_num
  <|>
  linarith [Real.pi_pos]

  have h10 : (∫ x in (0)..1, (4 : ℝ) / (1 + x^2)) = Real.pi := by
  have h11 : (∫ x in (0)..1, (4 : ℝ) / (1 + x ^ 2)) = 4 * (∫ x in (0)..1,
    → (1 : ℝ) / (1 + x ^ 2)) := by
  have h12 : (∫ x in (0)..1, (4 : ℝ) / (1 + x ^ 2)) = (∫ x in (0)..1, 4 *
    → (1 : ℝ) / (1 + x ^ 2)) := by

```

```

congr
ext x
<> ring_nf
rw [h1]
have h10 : (∫ x in (0)..1, 4 * (1 : ℝ) / (1 + x ^ 2)) = 4 * (∫ x in
  ↪ (0)..1, (1 : ℝ) / (1 + x ^ 2)) := by
  simp [intervalIntegral.integral_comp_mul_left (fun x => (1 : ℝ) / (1 +
    ↪ x ^ 2))]
  <>
  norm_num
  <>
  field_simp
  <>
  ring_nf
  <>
  norm_num
  <>
  linarith [Real.pi_pos]
rw [h10]
have h11 : (∫ x in (0)..1, (1 : ℝ) / (1 + x ^ 2)) = Real.pi / 4 := by
  have h12 : (∫ x in (0)..1, (1 : ℝ) / (1 + x ^ 2)) = Real.arctan 1 -
    ↪ Real.arctan 0 := by
    rw [integral_one_div_one_add_sq]
    <>
    norm_num
  rw [h12]
  have h13 : Real.arctan 1 = Real.pi / 4 := by
    norm_num [Real.arctan_one]
  have h14 : Real.arctan 0 = 0 := by
    norm_num [Real.arctan_zero]
  rw [h13, h14]
  <>
  ring_nf
  <>
  norm_num
  <>
  rw [h11]
  <>
  ring_nf
  <>
  norm_num
  <>
  rw [h1, h1]
  <>
  ring_nf
  <>
  norm_num
have hfinal : 22/7 - Real.pi = ∫ x in (0)..1, x^4 * (1 - x)^4 / (1 + x^2) :=
  ↪ by
  rw [hmain]
  <>
  linarith [Real.pi_pos]
exact hfinal
-- Simplified Proof
import Mathlib
import Aesop
set_option maxHeartbeats 0
theorem putnam_1968_a1
: 22/7 - Real.pi = ∫ x in (0)..1, x^4 * (1 - x)^4 / (1 + x^2) := by
  simp_rw [show ∀ x : ℝ, x ^ 4 * (1 - x) ^ 4 / (1 + x ^ 2) = (x ^ 6 - 4 * x ^ 5 +
    ↪ 5 * x ^ 4 - 4 * x ^ 2 + 4 - 4 / (1 + x ^ 2)) by
    intro x
    field_simp
    ring1
    ring_nf
    norm_num
    <> linarith [Real.pi_pos]]
  -----
  -- Orig Proof
  import Mathlib
  import Aesop
  set_option maxHeartbeats 0
  theorem putnam_1968_a2
  (a b c d e f : ℝ)
  (h : ℝ)
  (hne : a * d ≠ b * c)
  (h' : h > 0)
  : ∃ r s : ℝ, ((r * a + s * b - e) : ℝ) ∈ Set.Ioo 0 ^ ∞ ∧ ((r * c + s * d - f) : ℝ)
    ↪ ∈ Set.Ioo 0 ^ ∞ := by
    have hq-exists : ∃ (q : ℝ), (0 : ℝ) < (q : ℝ) ∧ (q : ℝ) < h := by
      have h1 : ∃ (q : ℝ), (0 : ℝ) < (q : ℝ) ∧ (q : ℝ) < h := by
        have h2 : ∃ (q : ℝ), (0 : ℝ) < (q : ℝ) ∧ (q : ℝ) < h := by
          obtain ⟨q, hq⟩ := exists_rat_btwn (by linarith : (0 : ℝ) < h)
          have h3 : (0 : ℝ) < (q : ℝ) := by linarith
          have h4 : (q : ℝ) < h := by linarith
          exact ⟨q, by exact_mod_cast h3, by exact_mod_cast h4⟩
        exact h1
      have hmain : ∃ (r s : ℝ), ((r * a + s * b - e) : ℝ) ∈ Set.Ioo 0 ^ ∞ ∧ ((r * c +
        ↪ s * d - f) : ℝ) ∈ Set.Ioo 0 ^ ∞ := by
        obtain ⟨q, hq_pos, hq_lt_⟩ := hq-exists
        have h5 : (a : ℝ) * d ≠ (b : ℝ) * c := by
          intro h
          norm_cast at h
          <> simp_all [mul_comm, mul_assoc, mul_left_comm]
          <> ring_nf at *
          <> norm_cast at *
          <> simp_all
        have h6 : ∃ (r s : ℝ), (r : ℝ) * a + (s : ℝ) * b = (e : ℝ) + q ∧ (r : ℝ) * c
          ↪ + (s : ℝ) * d = (f : ℝ) + q := by
          use ((e + q : ℝ) * d - b * (f + q : ℝ)) / (a * d - b * c : ℝ)
          use ((a * (f + q : ℝ) - (e + q : ℝ) * c) / (a * d - b * c : ℝ))

```



```

<> ring_nf <> simp [Real.exp_ne_zero]
have h3 : (fun s : ℝ => (x s - y s) * Real.exp (-2 * s)) 0 = (x 0 - y 0)
  => * Real.exp (-2 * (0 : ℝ)) := rfl
have h4 : Real.exp (-2 * (0 : ℝ)) = 1 := by norm_num [Real.exp_zero]
have h5 : (fun s : ℝ => (x s - y s) * Real.exp (-2 * s)) 0 = (x 0 - y 0)
  => := by
  rw [h4]
  rw [h5]
<> ring_nf
linarith
linarith

have h_main : x0 = y0 ↔ ∃ x y u : ℝ → ℝ, Differentiable ℝ x ∧ Differentiable ℝ y
  => y ∧ Continuous u ∧ deriv x = -2 · y + u ∧ deriv y = -2 · x + u ∧ x 0 =
  => x0 ∧ y 0 = y0 ∧ x t = 0 ∧ y t = 0 := by
  constructor
  · intro h
    exact h_imp h
  · intro h
    exact h_conv h
  exact h_main

-- Simplified Proof
import Mathlib
import Aesop

set_option maxHeartbeats 0

open Matrix Filter Topology Set Nat

theorem putnam_1969_a5
  (x0 y0 t : ℝ)
  (ht : 0 < t) :
  x0 = y0 ↔ ∃ x y u : ℝ → ℝ,
    Differentiable ℝ x ∧
    Differentiable ℝ y ∧
    Continuous u ∧
    deriv x = -2 · y + u ∧
    deriv y = -2 · x + u ∧
    x 0 = x0 ∧
    y 0 = y0 ∧
    x t = 0 ∧
    y t = 0 := by
  constructor
  · intro h
    use fun s => (-(x0 / t)) * s + x0, fun s => (-(x0 / t)) * s + x0, fun s =>
      (-(x0 / t)) + 2 * ((-x0 / t)) * s + x0
    have h1 : Differentiable ℝ (fun s : ℝ => (-(x0 / t)) * s + x0) := by
      apply Differentiable.add
      · apply Differentiable.mul
        · exact differentiable_const _
        · exact differentiable_id
      · exact differentiable_const _
    have h2 : Differentiable ℝ (fun s : ℝ => (-(x0 / t)) * s + x0) := by
      apply Differentiable.add
      · apply Differentiable.mul
        · exact differentiable_const _
        · exact differentiable_id
      · exact differentiable_const _
    have h3 : Continuous (fun s : ℝ => (-(x0 / t)) + 2 * ((-x0 / t)) * s +
      x0) := by
      apply Continuous.add
      · exact continuous_const
      · apply Continuous.mul
        · exact continuous_const
        · apply Continuous.add
          · exact continuous_const
          · exact continuous_id
          · exact continuous_const
    have h4 : deriv (fun s : ℝ => (-(x0 / t)) * s + x0) = -2 · (fun s : ℝ =>
      (-(x0 / t)) * s + x0) + fun s : ℝ => (-(x0 / t)) + 2 * ((-x0 / t)) *
      s + x0 := by
      have h5 : deriv (fun s : ℝ => (-(x0 / t)) * s + x0) = fun s => (-(x0 /
        t)) := by
        funext s
        simp [deriv_add, deriv_const, deriv_id, mul_comm]
      rw [h5]
      funext s
      simp [Pi.smul_apply, Pi.add_apply]
    constructor
    · exact h
    constructor
    · exact h
    constructor
    · exact h
    constructor
    · exact h
    constructor
    · exact h
    constructor
    · norm_num
    constructor
    · have h6 : y0 = x0 := by linarith
      norm_num [h6]
    constructor
    · have h7 : (fun s : ℝ => (-(x0 / t)) * s + x0) t = 0 := by
        have h8 : (fun s : ℝ => (-(x0 / t)) * s + x0) t = (-(x0 / t)) * t + x0
          := by simp
        rw [h8]
        field_simp [ht.ne']
        simp using h6
      have h9 : (fun s : ℝ => (-(x0 / t)) * s + x0) t = 0 := by
        have h10 : (fun s : ℝ => (-(x0 / t)) * s + x0) t = (-(x0 / t)) * t + x0
          := by simp
        rw [h10]
        field_simp [ht.ne']
        simp using h6
    rintro x, y, u, hx, hy, hu, hxy, hyx, hx0, hy0, hxt, hyt
    have h11 : x t - y t = 0 := by
      rw [hxt, hyt]
    <> norm_num
    have h12 : x 0 - y 0 = x0 - y0 := by
      rw [hx0, hy0]

have h1 : ∀ (s : ℝ), deriv (fun s : ℝ => (x s - y s) * Real.exp (-2 * s)) s
  => 0 := by
  intro s
  have h2 : deriv (fun s : ℝ => (x s - y s) * Real.exp (-2 * s)) s = (deriv
    (fun s : ℝ => x s - y s) s) * Real.exp (-2 * s) + (x s - y s) *
    (deriv (fun s : ℝ => Real.exp (-2 * s)) s) := by
    apply deriv_mul
    · apply DifferentiableAt.sub
      · exact hx.differentiableAt
      · exact hy.differentiableAt
    · apply DifferentiableAt.exp
      apply DifferentiableAt.const_mul
      apply differentiableAt_id
  rw [h2]
  have h3 : deriv (fun s : ℝ => x s - y s) s = deriv x s - deriv y s := by
    apply deriv_sub
    · exact hx.differentiableAt
    · exact hy.differentiableAt
  rw [h3]
  have h4 : deriv x s = (-2 : ℝ) * y s + u s := by
    have h5 : deriv x s = -2 · y + u := hxy
    have h6 : deriv x s = (-2 · y + u) s := by rw [h5]
    have h7 : (-2 · y + u) s = (-2 : ℝ) * y s + u s := by
      simp [Pi.add_apply, Pi.smul_apply]
    rw [h6, h7]
  have h8 : deriv y s = (-2 : ℝ) * x s + u s := by
    have h9 : deriv y s = -2 · x + u := hyx
    have h10 : deriv y s = (-2 · x + u) s := by rw [h9]
    have h11 : (-2 · x + u) s = (-2 : ℝ) * x s + u s := by
      simp [Pi.add_apply, Pi.smul_apply]
    rw [h10, h11]
  rw [h4, h8]
  have h9 : deriv (fun s : ℝ => Real.exp (-2 * s)) s = -2 * Real.exp (-2 *
    s) := by
    have h10 : deriv (fun s : ℝ => Real.exp (-2 * s)) s = Real.exp (-2 * s)
      * (-2 : ℝ) := by
      have h11 : HasDerivAt (fun s : ℝ => Real.exp (-2 * s)) (Real.exp (-2 *
        s) * (-2 : ℝ)) s := by
        have h12 : HasDerivAt (fun s : ℝ => (-2 : ℝ) * s) (-2 : ℝ) s := by
          simp using (hasDerivAt_id s).const_mul (-2 : ℝ)
        have h13 : HasDerivAt (fun s : ℝ => Real.exp (-2 * s)) (Real.exp
          (-2 * s) * (-2 : ℝ)) s := by
          convert HasDerivAt.exp (h12) using 1
        exact h13
      have h14 : deriv (fun s : ℝ => Real.exp (-2 * s)) s = Real.exp (-2 *
        s) * (-2 : ℝ) := by
        apply HasDerivAt.deriv
        exact h11
      rw [h14]
    rw [h10]
    <> ring
  rw [h9]
  ring_nf
  have h10 : Differentiable ℝ (fun s : ℝ => (x s - y s) * Real.exp (-2 * s)) :=
    by
    apply Differentiable.mul
    · apply Differentiable.sub
      · exact hx
      · exact hy
    · apply Differentiable.exp
      apply Differentiable.const_mul
      exact differentiable_id
  have h11 : (s : ℝ), (fun s : ℝ => (x s - y s) * Real.exp (-2 * s)) s =
    (fun s : ℝ => (x s - y s) * Real.exp (-2 * s)) 0 := by
    intro s
    apply is_const_of_deriv_eq_zero h10
    intro s
    have h12 : deriv (fun s : ℝ => (x s - y s) * Real.exp (-2 * s)) s = 0 :=
      by
        simp using h10
    have h13 : (x 0 - y 0) = 0 := by
      have h14 : (fun s : ℝ => (x s - y s) * Real.exp (-2 * s)) t = (fun s : ℝ =>
        (x s - y s) * Real.exp (-2 * s)) 0 := h1 t
      have h15 : (fun s : ℝ => (x s - y s) * Real.exp (-2 * s)) t = 0 := by
        have h16 : x t = 0 := hxt
        have h17 : y t = 0 := hyt
        have h18 : (fun s : ℝ => (x s - y s) * Real.exp (-2 * s)) t = (x t - y
          t) * Real.exp (-2 * t) := rfl
        rw [h16, h17]
      <> ring_nf
    <> ring_nf
  have h14 : (fun s : ℝ => (x s - y s) * Real.exp (-2 * s)) 0 = (x 0 - y 0)
    => * Real.exp (-2 * (0 : ℝ)) := rfl
  have h15 : Real.exp (-2 * (0 : ℝ)) = 1 := by norm_num [Real.exp_zero]
  have h16 : (fun s : ℝ => (x s - y s) * Real.exp (-2 * s)) 0 = (x 0 - y 0)
    => := by
    rw [h15]
    rw [h16]
    <> ring_nf
  linarith
  linarith
  linarith

-- Orig Proof
import Mathlib
import Aesop

set_option maxHeartbeats 0

open Metric Set EuclideanGeometry Filter Topology

theorem putnam_1970_b5
  (ramp : ℝ → (ℝ → ℝ))
  (ramp_def : ramp = fun (n : ℤ) => (fun (x : ℝ) => if x ≤ -n then (-n : ℝ) else
    (if -n < x ∧ x ≤ n then x else (n : ℝ))))
  (F : ℝ → ℝ)
  (Continuous F ↔ (∀ n : ℕ, Continuous ((ramp n) ∘ F))) := by
  have h_ramp_def : ∀ (n : ℤ) (x : ℝ), ramp n x = if x ≤ -n then (-n : ℝ) else
    (if -n < x ∧ x ≤ n then x else (n : ℝ)) := by
    intro n x
    rw [ramp_def]
    <> simp [n]
    <> aesop
  have h_imp : Continuous F → (∀ n : ℕ, Continuous ((ramp n) ∘ F)) := by

```

```

intro hF
intro n
have h1 : Continuous (ramp n) := by
have h2 : Continuous (fun x : ℝ => min (max x (-(n : ℝ))) (n : ℝ)) := by
continuity
have h3 : (ramp n) = (fun x : ℝ => min (max x (-(n : ℝ))) (n : ℝ)) := by
funext x
have h4 : ramp n x = if x ≤ (-(n : ℝ)) then (-(n : ℝ)) else (if (-(n : ℝ)
→ ) : ℝ) < x ∧ x ≤ (n : ℝ) then x else (n : ℝ)) := by
have h5 : h4.ramp_def (n : ℝ) x
simp [Int.cast_neg, Int.cast_ofNat] at h5
<>
(try norm_num at h5 ) <>
(try ring_nf at h5 ) <>
(try simp_all) <>
(try linarith) <>
<>
(try
{
split_ifs at h5
simp_all [Int.cast_neg, Int.cast_ofNat] <>
norm_num at * <>
(try linarith)
})
)
rw [h1]
split_ifs <>
(try {
simp_all [max_eq_left, max_eq_right, min_eq_left, min_eq_right,
→ le_of_lt]
<>
(try { nlinarith }) <>
(try { linarith })
}) <>
(try {
cases' le_total x (n : ℝ) with h6 h7 <>
simp_all [max_eq_left, max_eq_right, min_eq_left, min_eq_right,
→ le_of_lt] <>
(try { nlinarith }) <>
(try { linarith })
})
)
rw [h1]
exact h1
exact h1.comp hF
have h1.conv : (∀ n : ℕ, Continuous ((ramp n) ∘ F)) → Continuous F := by
intro h
have h1 : Continuous F := by
have h2 : ∀ (x0 : ℝ), ContinuousAt F x0 := by
intro x0
have h3 : ∀ (ε : ℝ), ε > 0 → (∃ (m : ℝ), m > 0 ∧ ∀ (x : ℝ), |x - x0| < m →
→ |F x - F x0| < ε) := by
intro ε
have h4 : ∃ (n : ℕ), (n : ℝ) > |F x0| + ε := by
obtain m, hn := exists_nat_gt (|F x0| + ε)
refine' ⟨m, _⟩
exact_mod_cast hn
obtain m, hm := h4
have h5 : (n : ℝ) > |F x0| + ε := hn
have h6 : Continuous ((ramp n) ∘ F) := h n
have h7 : ContinuousAt ((ramp n) ∘ F) x0 := h6.continuousAt
have h8 : ∀ (ε : ℝ), ε > 0 → (∃ (m : ℝ), m > 0 ∧ ∀ (x : ℝ), |x - x0| < m
→ |(ramp n ∘ F) x - (ramp n ∘ F) x0| < ε) := by
intro ε
have h9 : ContinuousAt ((ramp n) ∘ F) x0 := h7
exact Metric.continuousAt_iff.mp h9
have h10 : ∃ (m : ℝ), m > 0 ∧ ∀ (x : ℝ), |x - x0| < m → |(ramp n ∘ F) x
→ - (ramp n ∘ F) x0| < ε := h7.pos
obtain (m, spos, hm) := h10
use m
constructor
exact mpos
intro x hx
have h11 : |(ramp n ∘ F) x - (ramp n ∘ F) x0| < ε := hm x hx
have h12 : (ramp n ∘ F) x = ramp n (F x) := rfl
have h13 : (ramp n ∘ F) x0 = ramp n (F x0) := rfl
rw [h11, h12] at h13
have h14 : ramp n (F x) = F x0 := by
have h15 : (F x0 : ℝ) ≤ (n : ℝ) := by
have h16 : |F x0| + ε < (n : ℝ) := by linarith
have h17 : |F x0| < (n : ℝ) := by linarith
have h18 : F x0 ≤ |F x0| := by
cases' abs_cases (F x0) with h19 h20 <> linarith
linarith
have h21 : (F x0 : ℝ) > (-(n : ℝ)) := by
have h22 : |F x0| + ε < (n : ℝ) := by linarith
have h23 : |F x0| < (n : ℝ) := by linarith
have h24 : -(n : ℝ) < F x0 := by
cases' abs_cases (F x0) with h25 h26 <> linarith
linarith
have h27 : (F x0 : ℝ) > (-(n : ℝ)) ∧ (F x0 : ℝ) ≤ (n : ℝ) := h21,
→ h24
have h28 : ramp n (F x0) = (F x0 : ℝ) := by
have h29 : ramp n (F x0) = if (F x0 : ℝ) ≤ (-(n : ℝ)) then (-(n
→ : ℝ)) else (if (-(n : ℝ)) < (F x0 : ℝ) ∧ (F x0 : ℝ) ≤ (n : ℝ) then (F x0 : ℝ) else (n : ℝ)) := by
rw [h28.ramp_def]
<> simp [Int.cast_neg, Int.cast_ofNat]
<> norm_num
<>
(try
{
ring_nf
<>
norm_cast
})
<>
(try
{
simp_all [abs_lt]
<>
linarith
})
)
have h30 : ContinuousAt F x0 := by
rw [Metric.continuousAt_iff]
intro ε
obtain (m, spos, hm) := h28.pos
refine' ⟨m, spos, _⟩
intro x hx
have h31 : |F x - F x0| < ε := hm x hx
exact h31
exact h1
exact continuous_iff_continuousAt.mpr h1
exact h1

```

```

constructor
· intro h
· exact h_imp h
· intro h
· exact h_conv h

-- Simplified Proof
import Mathlib
import Aesop

set_option maxHeartbeats 0

open Metric Set EuclideanGeometry Filter Topology

theorem putnam_1970_b5
(ramp :  $\mathbb{R} \rightarrow (\mathbb{R} \rightarrow \mathbb{R}))$ 
(ramp_def : ramp = fun (n :  $\mathbb{Z}$ ) => (fun (x :  $\mathbb{R}$ ) => if x ≤ -n then (-n :  $\mathbb{R}$ ) else
  → (if -n < x ∧ x ≤ n then x else (n :  $\mathbb{R}$ ))))
(F :  $\mathbb{R} \rightarrow \mathbb{R}$ )
: Continuous F ↔ (∀ n :  $\mathbb{N}$ , Continuous ((ramp n) ∘ F)) := by
  constructor
  · intro hF
  · intro n
  have h₁ : Continuous (ramp n) := by
    have h₂ : Continuous (fun x :  $\mathbb{R}$  => min (max x (-n :  $\mathbb{R}$ )) (n :  $\mathbb{R}$ )) := by
      continuity
    have h₃ : (ramp n) = (fun x :  $\mathbb{R}$  => min (max x (-n :  $\mathbb{R}$ )) (n :  $\mathbb{R}$ )) := by
      funext x
    have h₄ : ramp n x = if x ≤ (-n :  $\mathbb{R}$ ) then (-n :  $\mathbb{R}$ ) else (if (-n :  $\mathbb{R}$ 
      → ) :  $\mathbb{R}$ ) < x ∧ x ≤ (n :  $\mathbb{R}$ ) then x else (n :  $\mathbb{R}$ )) := by
      rw [ramp_def]
    simp
    rw [h₄]
    split_ifs <|> simp_all [max_eq_left, max_eq_right, min_eq_left,
      → min_eq_right, le_of_lt]
    rw [h₄]
  exact h₂
  exact h₁.comp hF
  · intro h
  have h₁ : Continuous F := by
    have h₂ : ∀ (x₀ :  $\mathbb{R}$ ), ContinuousAt F x₀ := by
      intro x₀
      have h₃ : ∀ (ε :  $\mathbb{R}$ ), ε > 0 → (∃ (δ :  $\mathbb{R}$ ), δ > 0 ∧ ∀ (x :  $\mathbb{R}$ ), |x - x₀| < δ →
        → |F x - F x₀| < ε) := by
        intro ε
        have h₄ : ∃ (n :  $\mathbb{N}$ ), (n :  $\mathbb{R}$ ) > |F x₀| + ε := by
          obtain n, hm := exists_nat_gt (|F x₀| + ε)
          refine' n, _
          exact_mod_cast hm
        obtain m, hm₁ := h₄
        have h₅ : (n :  $\mathbb{R}$ ) > |F x₀| + ε := hm
        have h₆ : Continuous ((ramp n) ∘ F) := h n
        have h₇ : ContinuousAt ((ramp n) ∘ F) x₀ := h₁.continuousAt
        have h₈ : ∀ (ε' :  $\mathbb{R}$ ), ε' > 0 → (∃ (δ :  $\mathbb{R}$ ), δ > 0 ∧ ∀ (x :  $\mathbb{R}$ ), |x - x₀| < δ
          → |(ramp n ∘ F) x - (ramp n ∘ F) x₀| < ε') := by
          intro ε'
          have h₉ : ContinuousAt ((ramp n) ∘ F) x₀ := h₇
          exact Metric.continuousAt_iff.mp h₉ ε'
        have h₁₀ : ∃ (δ :  $\mathbb{R}$ ), δ > 0 ∧ ∀ (x :  $\mathbb{R}$ ), |x - x₀| < δ → |(ramp n ∘ F) x
          → - (ramp n ∘ F) x₀| < ε' := h₈ ε'
        obtain δ, mpos, hm := h₁₀
        use δ
        constructor
        · exact mpos
        · intro x hx
          have h₁₁ : |(ramp n ∘ F) x - (ramp n ∘ F) x₀| < ε' := hm x hx
          have h₁₂ : (ramp n ∘ F) x = ramp n (F x) := rfl
          have h₁₃ : (ramp n ∘ F) x₀ = ramp n (F x₀) := rfl
          rw [h₁₁, h₁₂] at h₁₁
          have h₁₄ : ramp n (F x₀) = F x₀ := by
            have h₁₅ : |F x₀| + ε < (n :  $\mathbb{R}$ ) := by linarith
            have h₁₆ : |F x₀| < (n :  $\mathbb{R}$ ) := by linarith
            have h₁₇ : F x₀ ≤ |F x₀| := by
              cases' abs_cases (F x₀) with h₁₇ h₁₇ <|> linarith
            have h₁₈ : |F x₀| > (-n :  $\mathbb{R}$ ) := by
              have h₁₉ : |F x₀| + ε < (n :  $\mathbb{R}$ ) := by linarith
              have h₂₀ : |F x₀| < (n :  $\mathbb{R}$ ) := by linarith
              cases' abs_cases (F x₀) with h₂₀ h₂₀ <|> linarith
            have h₂₁ : (F x₀ :  $\mathbb{R}$ ) ≤ (-n :  $\mathbb{R}$ ) := h₂₀
            have h₂₂ : (-n :  $\mathbb{R}$ ) < (F x₀ :  $\mathbb{R}$ ) := by
              have h₂₃ : |F x₀| + ε < (n :  $\mathbb{R}$ ) := by linarith
              have h₂₄ : |F x₀| < (n :  $\mathbb{R}$ ) := by linarith
              cases' abs_cases (F x₀) with h₂₄ h₂₄ <|> linarith
            linarith
          have h₂₅ : (-n :  $\mathbb{R}$ ) < (F x₀ :  $\mathbb{R}$ ) ∧ (F x₀ :  $\mathbb{R}$ ) ≤ (n :  $\mathbb{R}$ ) := (by
            → linarith, by linarith)
          have h₂₆ : ramp n (F x₀) = (F x₀ :  $\mathbb{R}$ ) := by
            have h₂₇ : ramp n (F x₀) = if (F x₀ :  $\mathbb{R}$ ) ≤ (-n :  $\mathbb{R}$ ) then (-n :  $\mathbb{R}$ ) else (if (-n :  $\mathbb{R}$ )
              → ) :  $\mathbb{R}$ ) < (F x₀ :  $\mathbb{R}$ ) ∧ (F x₀ :  $\mathbb{R}$ ) ≤ (n :  $\mathbb{R}$ ) then (F
              → x₀ :  $\mathbb{R}$ ) else (n :  $\mathbb{R}$ ) := by
              rw [ramp_def]
              <|> simp [Int.cast_neg, Int.cast_ofNat]
            rw [h₂₅]
            split_ifs <|> simp_all [h₂₅]
          rw [h₂₆]
          have h₂₈ : ramp n (F x) = F x := by
            by_contra h₂₈
            have h₂₉ : ramp n (F x) ≠ F x := h₂₈
            have h₃₀ : ramp n (F x) = (-n :  $\mathbb{R}$ ) ∨ ramp n (F x) = (n :  $\mathbb{R}$ ) :=
              → by
              have h₃₁ : ramp n (F x) = if (F x :  $\mathbb{R}$ ) ≤ (-n :  $\mathbb{R}$ ) then (-n :  $\mathbb{R}$ )
                → ) :  $\mathbb{R}$ ) < (F x :  $\mathbb{R}$ ) ∧ (F x :  $\mathbb{R}$ ) ≤ (n :  $\mathbb{R}$ ) then (F x :  $\mathbb{R}$ )
                → ) :  $\mathbb{R}$ ) else (n :  $\mathbb{R}$ ) := by
              rw [ramp_def]
              <|> simp [Int.cast_neg, Int.cast_ofNat]
            rw [h₃₀] at *
            split_ifs at * <|> (try { simp_all })
            cases h₃₁ with
            | inl h₃₁ =>
              have h₃₂ : ramp n (F x) = (-n :  $\mathbb{R}$ ) := h₃₁

```

```

      have h₁₄ : |(ramp n (F x) :  $\mathbb{R}$ ) - (ramp n (F x₀) :  $\mathbb{R}$ )| < ε := by
        → simp [h₁₃] using h₁₀
      have h₁₅ : |(-n :  $\mathbb{R}$ ) :  $\mathbb{R}$ ) - (F x₀ :  $\mathbb{R}$ )| < ε := by simp [h₁₄,
        → h₁₃] using h₁₀
      have h₁₆ : (n :  $\mathbb{R}$ ) > |F x₀| + ε := by exact_mod_cast hm
      have h₁₇ : |(-n :  $\mathbb{R}$ ) :  $\mathbb{R}$ ) - (F x₀ :  $\mathbb{R}$ )| ≥ (n :  $\mathbb{R}$ ) - |F x₀| := by
        cases' abs_cases (F x₀) with h₁₇ h₁₇ <|> cases' abs_cases (~n
        → :  $\mathbb{R}$ ) - F x₀) with h₁₇ h₁₇ <|> linarith
      have h₁₈ : (n :  $\mathbb{R}$ ) - |F x₀| > ε := by linarith
      linarith
      | inr h₁₇ =>
        have h₁₉ : ramp n (F x) = (n :  $\mathbb{R}$ ) := h₁₇
        have h₂₀ : |(ramp n (F x) :  $\mathbb{R}$ ) - (ramp n (F x₀) :  $\mathbb{R}$ )| < ε := by
          → simp [h₁₃] using h₁₀
        have h₂₁ : |(n :  $\mathbb{R}$ ) - (F x₀ :  $\mathbb{R}$ )| < ε := by simp [h₁₄, h₁₃] using
          → h₁₄
        have h₂₂ : (n :  $\mathbb{R}$ ) > |F x₀| + ε := by exact_mod_cast hm
        have h₂₃ : |(-n :  $\mathbb{R}$ ) :  $\mathbb{R}$ ) - (F x₀ :  $\mathbb{R}$ )| ≥ (n :  $\mathbb{R}$ ) - |F x₀| := by
          cases' abs_cases (F x₀) with h₂₃ h₂₃ <|> cases' abs_cases ((n
          → :  $\mathbb{R}$ ) - F x₀) with h₂₃ h₂₃ <|> linarith
        have h₂₄ : (n :  $\mathbb{R}$ ) - |F x₀| > ε := by linarith
        linarith
        have h₂₅ : |F x - F x₀| < ε := by
          have h₂₆ : ramp n (F x) = F x := h₁₉
          have h₂₇ : ramp n (F x₀) = F x₀ := h₁₃
          have h₂₈ : |(ramp n (F x) :  $\mathbb{R}$ ) - (ramp n (F x₀) :  $\mathbb{R}$ )| < ε := by
            → simp [h₁₃, h₁₃] using h₁₀
          exact h₂₈
        have h₂₉ : ContinuousAt F x₀ := by
          rw [Metric.continuousAt_iff]
          intro ε
          obtain (m, mpos, hm) := h₂₉ ε
          refine' (m, mpos, _)
          intro x hx
          have h₃₀ : |F x - F x₀| < ε := hm x hx
          exact h₃₀
        exact continuous_iff_continuousAt.mpr h₂₉
      exact h₁
    -----
-- Orig Proof
import Mathlib
import Aesop

set_option maxHeartbeats 0

open Set

theorem putnam_1971_a2
(P : Polynomial  $\mathbb{R}$ ) :
(P.eval 0 = 0 ∧ (∀ x :  $\mathbb{R}$ , P.eval (x^2 + 1) = (P.eval x)^2 + 1)) ↔ P ∈
  → (({Polynomial.X}) : Set (Polynomial  $\mathbb{R}$ )) :=
  by
  have h_main : (P.eval 0 = 0 ∧ (∀ x :  $\mathbb{R}$ , P.eval (x^2 + 1) = (P.eval x)^2 + 1))
    → P = Polynomial.X := by
    intro h
    have h₁ : P.eval 0 = 0 := h.1
    have h₂ : ∀ x :  $\mathbb{R}$ , P.eval (x^2 + 1) = (P.eval x)^2 + 1 := h.2
    have h₃ : ∃ (x :  $\mathbb{N} \rightarrow \mathbb{R}$ ), x 0 = 0 ∧ (∀ n :  $\mathbb{N}$ , x (n + 1) = (x n)^2 + 1) :=
      → by
      use fun n => Nat.recOn n (0 :  $\mathbb{R}$ ) fun n x_n => x_n ^ 2 + 1
      <|> simp [Nat.rec]
      <|> intros <|> simp_all [Nat.rec]
      <|> ring_nf
      <|> norm_num
    obtain (x, hx₀, hx) := h₃
    have h₄ : ∀ n :  $\mathbb{N}$ , x n < x (n + 1) := by
      intro n
      have h₅ : x (n + 1) = (x n)^2 + 1 := hx n
      rw [h₅]
      have h₆ : (x n :  $\mathbb{R}$ ) ^ 2 + 1 > x n := by
        nlinarith [sq_nonneg (x n - 1)]
      linarith
    have h₇ : ∀ n :  $\mathbb{N}$ , P.eval (x n) = x n := by
      intro n
      induction n with
      | zero =>
        have h₈₁ : P.eval (x 0) = x 0 := by
          have h₈₂ : x 0 = (0 :  $\mathbb{R}$ ) := hx₀
          rw [h₈₂]
          have h₈₃ : P.eval 0 = 0 := h₁
          norm_num at h₈₃
          <|> simp_all
        exact h₈₁
      | succ n ih =>
        have h₈₄ : x (n + 1) = (x n)^2 + 1 := hx n
        have h₈₅ : P.eval (x (n + 1)) = P.eval ((x n)^2 + 1) := by rw [h₈₄]
        rw [h₈₅]
        have h₈₆ : P.eval ((x n :  $\mathbb{R}$ ) ^ 2 + 1) = (P.eval (x n)) ^ 2 + 1 := h₇ (x
          → n)
        rw [h₈₆]
        have h₈₇ : P.eval (x n) = x n := ih
        rw [h₈₇]
        have h₈₈ : (x n :  $\mathbb{R}$ ) ^ 2 + 1 = x (n + 1) := by
          rw [hx n]
          <|> ring_nf
        rw [h₈₈]
        <|> simp_all
      have h₈ : P = Polynomial.X := by
        have h₈₁ : ∀ n :  $\mathbb{N}$ , (Polynomial.eval (x n) (P - Polynomial.X) :  $\mathbb{R}$ ) = 0 :=
          → by
          intro n
          have h₈₂ : Polynomial.eval (x n) (P - Polynomial.X) = Polynomial.eval
            → (x n) P - Polynomial.eval (x n) (Polynomial.X : Polynomial  $\mathbb{R}$ ) := by
            rw [Polynomial.eval_sub]
          rw [h₈₁]
          have h₈₃ : Polynomial.eval (x n) P = x n := by

```



```

      have hu1 : P.eval (x n) = x n := hu n
      simp [Polynomial.eval_eq_sum_range] using hu1
      have hu2 : Polynomial.eval (x n) (Polynomial.X : Polynomial  $\kappa$ ) = (x n :
 $\rightarrow$   $\kappa$ ) := by
        simp [Polynomial.eval_X]
        rw [hu1, hu]
        <|> ring_nf
        <|> simp_all

    have hu3 : P - Polynomial.X = 0 := by
      by_contra hu3
      have hu4 : (P - Polynomial.X : Polynomial  $\kappa$ )  $\neq$  0 := hu3
      have hu5 : Set.Infinite (Set.range x) := by
        have hu6 : StrictMono x := by
          refine' strictMono_nat_of_lt_succ _
          intro n
          exact hu n
        exact Set.infinite_range_of_injective (hu6.injective)
      have hu7 : Set.Finite {a :  $\mathbb{R}$  | (Polynomial.eval a (P - Polynomial.X) :  $\mathbb{R}$ 
 $\rightarrow$  0) = 0} := by
        apply Polynomial.finite_setOf_isRoot
        <|> simp_all
      have hu8 : Set.range x  $\subseteq$  {a :  $\mathbb{R}$  | (Polynomial.eval a (P - Polynomial.X)
 $\rightarrow$  :  $\kappa$ ) = 0} := by
        intro a ha
        obtain n, rfl := ha
        have hu9 := hu1 n
        simp_all [Set.mem_setOf_eq]
      have hu10 : Set.Infinite {a :  $\mathbb{R}$  | (Polynomial.eval a (P - Polynomial.X)
 $\rightarrow$  :  $\kappa$ ) = 0} := by
        exact Set.infinite_mono hu7, hu9
      exact hu3, hu10
    have hu11 : P - Polynomial.X = 0 := hu3
    have hu12 : P = Polynomial.X := by
      apply eq_of_sub_eq_zero
      simp using hu11
    exact hu12

  have hconverse : P  $\in$  ({(Polynomial.X)} : Set (Polynomial  $\kappa$ ))  $\rightarrow$  (P.eval 0 =
 $\rightarrow$  0  $\wedge$  ( $\forall$  x :  $\mathbb{R}$ , P.eval (x2 + 1) = (P.eval x)2 + 1)) := by
    intro h
    have h1 : P = Polynomial.X := by
      simp using h
    rw [h1]
    constructor
    simp [Polynomial.eval_X]
    intro x
    simp [Polynomial.eval_X]
    <|> ring_nf
    <|> norm_num

  have hfinal : (P.eval 0 = 0  $\wedge$  ( $\forall$  x :  $\mathbb{R}$ , P.eval (x2 + 1) = (P.eval x)2 +
 $\rightarrow$  1))  $\rightarrow$  P  $\in$  ({(Polynomial.X)} : Set (Polynomial  $\kappa$ )) := by
    constructor
    intro h
    have h1 : P = Polynomial.X := hmain h
    rw [h1]
    <|> simp
    intro h
    exact hconverse h

  exact hfinal

-- Simplified Proof
import Mathlib
import Aesop

set_option maxHeartbeats 0

open Set

theorem putnam_1971_a2
(P : Polynomial  $\kappa$ ) :
(P.eval 0 = 0  $\wedge$  ( $\forall$  x :  $\mathbb{R}$ , P.eval (x2 + 1) = (P.eval x)2 + 1))  $\rightarrow$  P  $\in$ 
({(Polynomial.X)} : Set (Polynomial  $\kappa$ )) := by
  constructor
  rintro (h1, h2)
  have h3 : P = Polynomial.X := by
    have h4 :  $\forall$  x :  $\mathbb{N} \rightarrow \mathbb{R}$ , x 0 = 0  $\wedge$  ( $\forall$  n :  $\mathbb{N}$ , x (n + 1) = (x n) ^ 2 + 1)  $\rightarrow$  P
 $\rightarrow$  = Polynomial.X := by
      intro x hx
      obtain (hx1, hx2) := hx
      have h5 : StrictMono x := by
        refine' strictMono_nat_of_lt_succ _
        intro n
        rw [hx1]
        nlinarith
      have h6 :  $\forall$  n :  $\mathbb{N}$ , P.eval (x n) = x n := by
        intro n
        induction' n with n ih
        simp_all
        simp_all [hx1, ih]
      have h7 : P - Polynomial.X = 0 := by
        by_contra h7
        have h8 : (P - Polynomial.X : Polynomial  $\kappa$ )  $\neq$  0 := h7
        have h9 : Set.Infinite (Set.range x) :=
 $\rightarrow$  Set.infinite_range_of_injective h5.injective
        have h10 : Set.Finite {a :  $\mathbb{R}$  | (Polynomial.eval a (P - Polynomial.X)
 $\rightarrow$  :  $\kappa$ ) = 0} := Polynomial.finite_setOf_isRoot h8
        have h11 : Set.range x  $\subseteq$  {a :  $\mathbb{R}$  | (Polynomial.eval a (P -
Polynomial.X) :  $\kappa$ ) = 0} := by
          intro a ha
          obtain n, rfl := ha
          simp_all [Set.mem_setOf_eq]
        have h12 : Set.Infinite {a :  $\mathbb{R}$  | (Polynomial.eval a (P -
Polynomial.X) :  $\kappa$ ) = 0} := Set.infinite_mono h5, h9
        exact h7, h12
      exact h7, h12
    apply eq_of_sub_eq_zero
    simp using h7
  exact h3 (fun n => n.rec 0 (fun n xn => xn ^ 2 + 1)) (by simp, by simp
 $\rightarrow$  [pow_succ])
  simp_all

  rintro rfl
  constructor <|> simp
  -----
  -- Orig Proof
  import Mathlib
  import Aesop

  set_option maxHeartbeats 0

  open Set MvPolynomial

  theorem putnam_1971_b1
(S : Type*) [Mul S]
(hself :  $\forall$  x : S, x * x = x)
(h2 :  $\forall$  x y z : S, (x * y) * z = (y * z) * x)
( $\forall$  x y z : S, (x * y) * z = x * (y * z))  $\wedge$  ( $\forall$  x y : S, x * y = y * x) := by
  have hcommutative :  $\forall$  x y : S, x * y = y * x := by
    intro x y
    have h3 : ((x * y) * x) * y = x * y := by
      have h4 : ((x * y) * x) * y = (x * y) * (x * y) := by
        have h5 := h2 (x * y) x y
      exact h5
    calc
      ((x * y) * x) * y = (x * y) * (x * y) := by
        rw [h5]
        <|> simp [hself]
      _ = (x * y) * (x * y) := by rfl
    have h6 : (x * y) * (x * y) = x * y := by
      have h7 := hself (x * y)
      calc
        (x * y) * (x * y) = x * y := by rw [h7]
        _ = x * y := by rfl
    calc
      ((x * y) * x) * y = (x * y) * (x * y) := by rw [h4]
      _ = x * y := by rw [h6]
    have h8 : ((x * y) * x) * y = y * x := by
      have h9 : (x * y) * x = x * y := by
        have h10 := h2 x y x
        have h11 := h2 y x x
        calc
          (x * y) * x = (y * x) * x := by rw [h10]
          _ = x * y := by
            have h12 := h11
            calc
              (y * x) * x = (x * x) * y := by rw [h12]
              _ = x * y := by
                have h13 := hself x
                simp [h13]
                _ = x * y := by rfl
            calc
              ((x * y) * x) * y = (x * y) * y := by rw [h9]
              _ = y * x := by
                have h14 := h2 x y y
                have h15 := hself y
                calc
                  (x * y) * y = (y * y) * x := by rw [h14]
                  _ = y * x := by
                    simp [h15]
                    _ = y * x := by rfl
              _ = y * x := by rfl
            calc
              x * y = ((x * y) * x) * y := by rw [h3]
              _ = y * x := by rw [h8]
        have hassociative :  $\forall$  x y z : S, (x * y) * z = x * (y * z) := by
          intro x y z
          have h3 : (x * y) * z = (y * z) * x := h2 x y z
          have h4 : (y * z) * x = x * (y * z) := by
            have h5 := hcommutative (y * z) x
            exact h5
          calc
            (x * y) * z = (y * z) * x := by rw [h3]
            _ = x * (y * z) := by rw [h4]
          exact (hassociative, hcommutative)

  -- Simplified Proof
  import Mathlib
  import Aesop

  set_option maxHeartbeats 0

  open Set MvPolynomial

  theorem putnam_1971_b1
(S : Type*) [Mul S]
(hself :  $\forall$  x : S, x * x = x)
(h2 :  $\forall$  x y z : S, (x * y) * z = (y * z) * x)
( $\forall$  x y z : S, (x * y) * z = x * (y * z))  $\wedge$  ( $\forall$  x y : S, x * y = y * x) := by
  have h2' :  $\forall$  x y : S, x * y = y * x := by
    intro x y
    have h3 := h2 (y * x) y x
    have h4 := h2 x y y
    simp_all
    have h5 :  $\forall$  x y z : S, (x * y) * z = x * (y * z) := by
      intro x y z
      simp_all [h2]
    exact (h5, h2')
  -----
  -- Orig Proof
  import Mathlib
  import Aesop

  set_option maxHeartbeats 0

  open Set MvPolynomial

  theorem putnam_1971_b2
(S : Set  $\mathbb{R}$ )
(hS : S = univ \ {0, 1})
(P : ( $\mathbb{R} \rightarrow \mathbb{R}$ )  $\rightarrow$  Prop)
(hP : P = fun (F :  $\mathbb{R} \rightarrow \mathbb{R}$ ) =>  $\forall$  x  $\in$  S, F x + F ((x - 1)/x) = 1 + x)
( $\forall$  F  $\in$  ({(fun x :  $\mathbb{R} \rightarrow \mathbb{R}$  => (x3 - x2 - 1)/(2 * x * (x - 1)))} : Set ( $\mathbb{R} \rightarrow \mathbb{R}$ )), P
 $\rightarrow$  F)  $\wedge$   $\forall$  f :  $\mathbb{R} \rightarrow \mathbb{R}$ , P f  $\rightarrow$   $\exists$  F  $\in$  ({(fun x :  $\mathbb{R} \rightarrow \mathbb{R}$  => (x3 - x2 - 1)/(2 * x *
(x - 1)))} : Set ( $\mathbb{R} \rightarrow \mathbb{R}$ )), ( $\forall$  x  $\in$  S, f x = F x) := by

```



```

have h1 : (∀ F ∈ (({fun x : R => (x^3 - x^2 - 1)/(2 * x * (x - 1))} : Set (R
  → → R) ), P F) := by
rw [hP]
intro F hF
simp only [Set.mem_singleton_iff] at hF
rw [hF]
have h1 : ∀ (x : R), x ∈ (univ \ {0, 1} : Set R) → ((fun x : R => (x^3 -
  → x^2 - 1) / (2 * x * (x - 1))) x + (fun x : R => (x^3 - x^2 - 1)
  → / (2 * x * (x - 1))) ((x - 1) / x) = 1 + x) := by
intro x hx
have h1 : x ≠ 0 := by
intro h
simp [h] at hx
<> norm_num at hx
<> aesop
have h1 : x ≠ 1 := by
intro h
simp [h] at hx
<> norm_num at hx
<> aesop
have h1 : (x - 1) / x ≠ 0 := by
have h11 : x - 1 ≠ 0 := by
intro h11
apply h
linarith
field_simp [h1, h11]
<> intro h11
<> apply h11
<> nlinarith
have h1 : (x - 1) / x ≠ 1 := by
intro h
have h11 : (x - 1) / x = 1 := h1
field_simp [h1] at h11
<> ring_nf at h11
<> nlinarith [sq_pos_of_ne_zero (sub_ne_zero.mpr h11)]
have h1 : ((fun x : R => (x^3 - x^2 - 1) / (2 * x * (x - 1))) x) = (x
  → ^ 3 - x^2 - 1) / (2 * x * (x - 1)) := rfl
have h1 : ((fun x : R => (x^3 - x^2 - 1) / (2 * x * (x - 1))) ((x -
  → 1) / x)) = (((x - 1) / x)^3 - ((x - 1) / x)^2 - 1) / (2 * (x -
  → 1) / x) * (((x - 1) / x) - 1) := rfl
have h1 : (x^3 - x^2 - 1) / (2 * x * (x - 1)) + (((x - 1) / x)^3 -
  → ((x - 1) / x)^2 - 1) / 2 * ((x - 1) / x) * (((x - 1) / x) - 1) =
  → 1 + x := by
have h11 : (((x - 1) / x)^3 - ((x - 1) / x)^2 - 1) / (2 * (x - 1)
  → / x) * (((x - 1) / x) - 1) = (x^3 + x^2 - 2 * x + 1) / (2 * x *
  → (x - 1)) := by
have h12 : (((x - 1) / x)^3 - ((x - 1) / x)^2 - 1) = (-x^3 - x
  → ^ 2 + 2 * x - 1) / x^3 := by
field_simp [h1]
<> ring_nf
<> field_simp [h1]
<> ring_nf
<> nlinarith
have h11 : (2 * ((x - 1) / x) * (((x - 1) / x) - 1)) = (-2 * (x - 1)
  → / x^2 := by
field_simp [h1]
<> ring_nf
<> field_simp [h1]
<> ring_nf
<> nlinarith
rw [h12, h11]
have h11 : (-x^3 - x^2 + 2 * x - 1) / x^3 / ((-2 * (x - 1)) / x
  → ^ 2) = (x^3 + x^2 - 2 * x + 1) / (2 * x * (x - 1)) := by
have h11 : x ≠ 0 := h1
have h11 : x - 1 ≠ 0 := by
intro h11
apply h1
linarith
field_simp [h11, h11]
<> ring_nf
<> field_simp [h11, h11]
<> ring_nf
<> nlinarith
calc
((x^3 - x^2 + 2 * x - 1) / x^3) / ((-2 * (x - 1)) / x^2) =
  → (x^3 + x^2 - 2 * x + 1) / (2 * x * (x - 1)) := by
rw [h11]
_ = (x^3 + x^2 - 2 * x + 1) / (2 * x * (x - 1)) := by rfl
rw [h11]
have h11 : (x^3 - x^2 - 1) / (2 * x * (x - 1)) + (x^3 + x^2 - 2
  → * x + 1) / (2 * x * (x - 1)) = 1 + x := by
have h11 : x - 1 ≠ 0 := by
intro h11
apply h1
linarith
have h11 : x ≠ 0 := h1
have h11 : 2 * x * (x - 1) ≠ 0 := by
apply mul_ne_zero
norm_num
exact h11
exact h11
field_simp [h11, h11, h11]
<> ring_nf
<> field_simp [h11, h11]
<> nlinarith
linarith
simp_all
<> norm_num
<> linarith
intro x hx
have h1 := h1 x (by simp [hS] using hx)
simp using h1

```

```

have h1 : ∀ f : R → R, P f → ∃ F ∈ (({fun x : R => (x^3 - x^2 - 1)/(2 * x *
  → (x - 1))} : Set (R → R) ), (∀ x ∈ S, f x = F x) := by
intro f hf
rw [hP] at hf
use fun x => (x^3 - x^2 - 1) / (2 * x * (x - 1))
constructor
· simp
· intro x hx
have h1 : x ∈ (univ \ {0, 1} : Set R) := by
rw [hS] at hx
exact hx

```

```

have h1 : x ≠ 0 := by
intro h
simp [h] at h1
<> norm_num at h1
<> aesop
have h1 : x ≠ 1 := by
intro h
simp [h] at h1
<> norm_num at h1
<> aesop
have h1 : (x - 1) / x ≠ 0 := by
have h11 : x - 1 ≠ 0 := by
intro h11
apply h1
linarith
field_simp [h1, h11]
<> intro h11
<> apply h11
<> nlinarith
have h1 : (x - 1) / x ≠ 1 := by
intro h1
have h11 : (x - 1) / x = 1 := h1
field_simp [h1] at h11
<> ring_nf at h11
<> nlinarith [sq_pos_of_ne_zero (sub_ne_zero.mpr h11)]
have h1 : f x + f ((x - 1) / x) = 1 + x := hf x (by simp [hS] using hx)
have h11 : f ((x - 1) / x) + f (-1 / (x - 1)) = 1 + (x - 1) / x := by
have h111 : (x - 1) / x ∈ (univ \ {0, 1} : Set R) := by
have h112 : (x - 1) / x ≠ 0 := h1
have h113 : (x - 1) / x ≠ 1 := h1
simp [h112, h113]
<>
(tr try norm_num) <>
(tr try aesop) <>
trivial
have h114 : f ((x - 1) / x) + f (((x - 1) / x) - 1) / ((x - 1) / x) = 1 +
  → ((x - 1) / x) := hf ((x - 1) / x) (by simp [hS] using h114)
have h115 : (((x - 1) / x) - 1) / ((x - 1) / x) = -1 / (x - 1) := by
have h116 : x ≠ 0 := h1
have h117 : x - 1 ≠ 0 := h1
field_simp [h116, h117]
<> ring_nf
<> field_simp [h116, h117]
<> ring_nf
<> nlinarith
rw [h115] at h114
exact h114
have h11 : f (-1 / (x - 1)) + f x = 1 + (-1 / (x - 1)) := by
have h111 : -1 / (x - 1) ∈ (univ \ {0, 1} : Set R) := by
have h112 : -1 / (x - 1) ≠ 0 := by
have h113 : x - 1 ≠ 0 := h1
field_simp [h111]
<> intro h114
<> nlinarith
have h114 : -1 / (x - 1) ≠ 1 := by
have h115 : x - 1 ≠ 0 := h1
field_simp [h111]
<> intro h116
<>
(tr try {
  have h117 : x = 0 := by linarith
  contradiction
})
<>
(tr try {
  nlinarith
})
simp [h112, h113]
<>
(tr try norm_num) <>
(tr try aesop) <>
trivial
have h115 : f (-1 / (x - 1)) + f (((-1 / (x - 1) - 1) / (-1 / (x -
  → 1)))) = 1 + (-1 / (x - 1)) := hf (-1 / (x - 1)) (by simp [hS] using
  → h115)
have h116 : (((-1 / (x - 1) - 1) / (-1 / (x - 1)))) = x := by
have h117 : x - 1 ≠ 0 := h1
field_simp [h117]
<> ring_nf
<> field_simp [h117]
<> ring_nf
<> nlinarith
rw [h115] at h115
exact h115
have h12 : f x = (x^3 - x^2 - 1) / (2 * x * (x - 1)) := by
have h121 : f x = (1 + x + (-1 / (x - 1)) - ((x - 1) / x)) / 2 := by
have h122 : f x + f ((x - 1) / x) = 1 + x := h1
have h123 : f ((x - 1) / x) + f (-1 / (x - 1)) = 1 + (x - 1) / x := h11
have h124 : f (-1 / (x - 1)) + f x = 1 + (-1 / (x - 1)) := h11
have h125 : f x = (1 + x + (-1 / (x - 1)) - ((x - 1) / x)) / 2 := by
linarith
exact h125
have h126 : (1 + x + (-1 / (x - 1)) - ((x - 1) / x)) / 2 = (x^3 - x^
  → 2 - 1) / (2 * x * (x - 1)) := by
have h127 : x ≠ 0 := h1
have h128 : x - 1 ≠ 0 := h1
field_simp [h127, h128]
<> ring_nf
<> field_simp [h127, h128]
<> ring_nf
<> nlinarith
linarith
have h13 : (fun x : R => (x^3 - x^2 - 1) / (2 * x * (x - 1))) x = (x
  → ^ 3 - x^2 - 1) / (2 * x * (x - 1)) := rfl
exact (h1, h13)

```

```

-- Simplified Proof
import Mathlib
import Aesop

```



```

ring_nf
<|>
norm_num
<|>
linarith
have h11 : (4 : z) * n + 1 = 2 * (a ^ 2 + a + b ^ 2 + b) + 1 := by
  linarith
linarith
have h12 : (n : q) = (a ^ 2 + (a : q)) / 2 + (b ^ 2 + (b : q)) / 2 := by
  have h13 : (2 : q) * (n : q) = (a : q) ^ 2 + (a : q) + (b : q) ^ 2 + (b : q)
  => by
    norm_cast at h13
    <|>
    ring_nf at h13
    norm_num at h13
    linarith
have h14 : (n : q) = (a ^ 2 + (a : q)) / 2 + (b ^ 2 + (b : q)) / 2 := by
  ring_nf at h13
  <|>
  linarith
exact h14
simp only [hnab]
refine' (a, b, _)
exact_mod_cast h12

exact [h_forward, h_backward]

-- Simplified Proof
import Mathlib
import Aesop

set_option maxHeartbeats 0

open Polynomial

theorem putnam_1975_a1
(nab nxy : (z × z × z) → Prop)
(hnab : nab = fun (n, a, b) => n = (a^2 + (a : q))/2 + (b^2 + (b : q))/2)
(hnxy : nxy = fun (n, x, y) => 4*n + 1 = x^2 + y^2)
: (∀ n a b : z, nab (n, a, b) → nxy (n, ((fun (a, b) => a + b + 1, fun (a, b) => a - b) : ((z × z) → z) × ((z × z) → z)).1 (a, b), ((fun (a, b) => a + b + 1, fun (a, b) => a - b) : ((z × z) → z) × ((z × z) → z)).2 (a, b)))
  v n : z, (∃ x y : z, nxy (n, x, y)) → ∃ a b : z, nab (n, a, b) := by
  simp_all only [Function.funext_iff, hnab, hnxy]
  constructor
  intro n a b h
  field_simp at h
  norm_cast at h
  linarith
  intro n hn
  obtain (x, y, hxy) := hn
  have h1 : (x + y) % 2 = 1 := by
    have h2 := hxy
    ring_nf at h2
    have h3 : (x ^ 2 + y ^ 2) % 4 = 1 := by omega
    have h4 : x % 4 = 0 ∨ x % 4 = 1 ∨ x % 4 = 2 ∨ x % 4 = 3 := by omega
    have h5 : y % 4 = 0 ∨ y % 4 = 1 ∨ y % 4 = 2 ∨ y % 4 = 3 := by omega
    rcases h4 with (h4 | h4 | h4 | h4) <|> rcases h5 with (h5 | h5 | h5 | h5) <|>
    → (try omega) <|> (try {
      simp [h4, h5, pow_two, Int.add_emod, Int.mul_emod] at h2
    })
  have h6 : (x - y) % 2 = 1 := by
    have h7 := hxy
    ring_nf at h7
    have h8 : (x ^ 2 + y ^ 2) % 4 = 1 := by omega
    have h9 : x % 4 = 0 ∨ x % 4 = 1 ∨ x % 4 = 2 ∨ x % 4 = 3 := by omega
    have h10 : y % 4 = 0 ∨ y % 4 = 1 ∨ y % 4 = 2 ∨ y % 4 = 3 := by omega
    rcases h9 with (h9 | h9 | h9 | h9) <|> rcases h10 with (h10 | h10 | h10 | h10) <|>
    → (try omega)
  have h11 : (x + y - 1) % 2 = 0 := by
    omega
  have h12 : (x - y - 1) % 2 = 0 := by
    omega
  have h13 : ∃ (a : z), 2 * a = x + y - 1 := by
    use (x + y - 1) / 2
    omega
  have h14 : ∃ (b : z), 2 * b = x - y - 1 := by
    use (x - y - 1) / 2
    omega
  obtain (a, ha) := h13
  obtain (b, hb) := h14
  have h15 : a + b + 1 = x := by
    omega
  have h16 : a - b = y := by
    omega
  have h17 : 4 * n + 1 = (a + b + 1) ^ 2 + (a - b) ^ 2 := by
    rw [h15, h16]
    <|> linarith
  have h18 : 2 * n = a ^ 2 + a + b ^ 2 + b := by
    ring_nf at h17
    <|> linarith
  have h19 : (n : q) = (a ^ 2 + (a : q)) / 2 + (b ^ 2 + (b : q)) / 2 := by
    have h20 : (2 : q) * (n : q) = (a : q) ^ 2 + (a : q) + (b : q) ^ 2 + (b : q)
    => by
      norm_cast at h20
      ring_nf at h20
      <|> linarith
    refine' (a, b, _)
    exact_mod_cast h19
  -----
  -- Orig Proof
  import Mathlib
  import Aesop

  set_option maxHeartbeats 0

  open Polynomial Real Complex

  theorem putnam_1975_b1
  (H : Set (z × z))
  (hH : H = {(x, y) : (z × z) | ∃ u v w : z, (x, y) = (u*3 + v*4 + w*5, u*8 + v*(-1) + w*4)})
  : (∃ b : z, H = {(x, y) : (z × z) | ∃ u v : z, (x, y) = (u, u*b + v*((7 : z) → z))}) ∧ ((7 : z) > 0 := by

```

```

have h_main : ∃ (b : z), H = {(x, y) : (z × z) | ∃ (u v : z), (x, y) = (u, u *
  → b + v * (7 : z))} := by
  use 5
  rw [hH]
  apply Set.ext
  intro (X, Y)
  simp only [Set.mem_setOf_eq, Prod.mk.injEq]
  constructor
  intro h
  rcases h with (u, v, w, hx, hy)
  have h1 : x = u * 3 + v * 4 + w * 5 := by linarith
  have h2 : y = u * 8 + v * (-1) + w * 4 := by linarith

  use x, -u - 3 * v - 3 * w
  simp [h1, h2]
  <|> ring_nf at *
  <|> norm_num at *
  <|> linarith

  intro h
  rcases h with (t, s, hx, hy)
  have h3 : x = t := by linarith
  have h4 : y = t * 5 + s * 7 := by linarith

  use -s, -t - 3 * s, t + 3 * s
  simp [h3, h4]
  <|> ring_nf at *
  <|> norm_num at *
  <|> linarith

  have h_trivial : (7 : z) > 0 := by
    norm_num

  exact [h_main, h_trivial]

-- Simplified Proof
import Mathlib
import Aesop

set_option maxHeartbeats 0

open Polynomial Real Complex

theorem putnam_1975_b1
(H : Set (z × z))
(hH : H = {(x, y) : (z × z) | ∃ u v w : z, (x, y) = (u*3 + v*4 + w*5, u*8 + v*(-1) + w*4)})
: (∃ b : z, H = {(x, y) : (z × z) | ∃ u v : z, (x, y) = (u, u*b + v*((7 : z) → z))}) ∧ ((7 : z) > 0 := by
  rw [hH]
  constructor
  use 5
  ext (X, Y)
  simp only [Set.mem_setOf_eq, Prod.mk.injEq]
  constructor
  rintro (u, v, w, hx, hy)
  use x, -u - 3 * v - 3 * w
  constructor <|> linarith
  rintro (t, s, hx, hy)
  use -s, -t - 3 * s, t + 3 * s
  constructor <|> linarith
  norm_num
  -----
  -- Orig Proof
  import Mathlib
  import Aesop

  set_option maxHeartbeats 0

  theorem putnam_1977_a3
  (f g h : ℝ → ℝ)
  (hf : ∀ x, f x = (h (x + 1) + h (x - 1)) / 2)
  (hg : ∀ x, g x = (h (x + 4) + h (x - 4)) / 2)
  (h : ((fun f g x => g x - f (x - 3) + f (x - 1) + f (x + 1) - f (x + 3)) :
    → (ℝ → ℝ) → (ℝ → ℝ) → (ℝ → ℝ)) f g :=
  by
  have h_main : ∀ (x : ℝ), h x = g x - f (x - 3) + f (x - 1) + f (x + 1) - f (x + 3) := by
    intro x
    have h1 : g x = (h (x + 4) + h (x - 4)) / 2 := hg x
    have h2 : f (x - 3) = (h (x - 3 + 1) + h (x - 3 - 1)) / 2 := by
      rw [hf]
      <|> ring_nf
    have h3 : f (x - 1) = (h (x - 1 + 1) + h (x - 1 - 1)) / 2 := by
      rw [hf]
      <|> ring_nf
    have h4 : f (x + 1) = (h (x + 1 + 1) + h (x + 1 - 1)) / 2 := by
      rw [hf]
      <|> ring_nf
    have h5 : f (x + 3) = (h (x + 3 + 1) + h (x + 3 - 1)) / 2 := by
      rw [hf]
      <|> ring_nf
    rw [h1, h2, h3, h4, h5]
    ring_nf
    <|> field_simp
    <|> ring_nf
    <|> linarith

  have h_final : h = (fun f g x => g x - f (x - 3) + f (x - 1) + f (x + 1) - f (x + 3)) f g := by
    funext x
    rw [h_main x]
    <|> simp [hf, hg]
    <|> ring_nf
    <|> norm_num

  apply h_final

-- Simplified Proof
import Mathlib
import Aesop

```

```
cases k with
| zero => contradiction
| succ k =>
  cases k with
  | zero => contradiction
  | succ k =>
    simp_all [pow_succ]
    <.>
    (try norm_num at *) <.>
    (try linarith [sq_nonneg ((k : ℕ) + 10)])
```

```

have h8 : u ≥ 10 := by
  simp [hn]
  <|> omega
have h9 : (2 : R) ^ n ≥ (n : R) ^ 3 := h7.n h8
exact h9

have h10 : ((3 : R) - a) * (2 : R) ^ n ≥ 5 * (n : R) ^ 2 := by
  have h11 : (n : R) ≥ 5 / ((3 : R) - a) := h7
  have h12 : ((3 : R) - a) > 0 := by linarith
  have h13 : (n : R) * ((3 : R) - a) ≥ 5 := by
    calc
      (n : R) * ((3 : R) - a) ≥ (5 / ((3 : R) - a)) * ((3 : R) - a) := by
        <|> gcongr
      = 5 := by
        field_simp [h11.ne']
      <|> ring_nf
      <|> linarith
  have h14 : ((3 : R) - a) * (2 : R) ^ n ≥ ((3 : R) - a) * (n : R) ^ 3 := by
    have h15 : (2 : R) ^ n ≥ (n : R) ^ 3 := h9
    have h16 : ((3 : R) - a) ≥ 0 := by linarith
    linarith
  have h17 : ((3 : R) - a) * (n : R) ^ 3 ≥ 5 * (n : R) ^ 2 := by
    have h18 : (n : R) ≥ 10 := h8
    have h19 : (n : R) ≥ 0 := by linarith
    have h20 : ((3 : R) - a) * (n : R) ≥ 5 := by linarith
    linarith [sq_nonneg ((n : R) - 10)]
  linarith

have h21 : (a - 3 : R) * (2 : R) ^ n + (n : R) ^ 2 + 2 * (n : R) + 3 ≤ 0 :=
  <|> by
  have h22 : ((3 : R) - a) * (2 : R) ^ n ≥ 5 * (n : R) ^ 2 := h17
  have h23 : (a - 3 : R) * (2 : R) ^ n ≤ -5 * (n : R) ^ 2 := by
    linarith
  have h24 : (n : R) ^ 2 + 2 * (n : R) + 3 ≤ 5 * (n : R) ^ 2 := by
    have h25 : (n : R) ≥ 10 := h8
    linarith [sq_nonneg ((n : R) - 1)]
  linarith

have h26 : u > 0 := h_pos n
have h27 : (a - 3) * (2 : R) ^ n + (n : R) ^ 2 + 2 * (n : R) + 3 :=
  <|> h_closed_form n
rw [h26] at h27
linarith

```

```

have h : u > 0 := h_pos n
have h₀ : u = (a - 3) * (2 : ℤ) ^ n + (n : ℤ) ^ 2 + 2 * (n : ℤ) + 3 :=
  → h_closed_form n
rw [h₀] at h
linarith

exact h_forward, h_backward

-- Simplified Proof
import Mathlib
import Aesop

set_option maxHeartbeats 0

```

[illegible]

```

| zero => contradiction
| succ k =>
  cases k with
  | zero => contradiction
  | succ k =>
    simp_all [pow_succ]
    <|> nlinarith [sq_nonneg ((k : ℕ) + 10)]

have h₁ : n ≥ 10 := by simp [hn]
exact h₁.nh
have h₁ : (3 - a) * (2 : ℝ) ^ n ≥ 5 * (n : ℝ) ^ 2 := by
  have h₁ : (n : ℝ) ≥ 5 / (3 - a) := h₁
  have h₁ : (3 - a) > 0 := by linarith
  have h₁ : (n : ℝ) * (3 - a) ≥ 5 := by
    calc
      (n : ℝ) * (3 - a) ≥ (5 / (3 - a)) * (3 - a) := by gcongr
      = 5 := by
        field_simp [h₁.ne']
  nlinarith
have h₁ : (a - 3 : ℝ) * (2 : ℝ) ^ n + (n : ℝ) ^ 2 + 2 * (n : ℝ) + 3 ≤ 0 :=
  by
    nlinarith
have h₁ : u n > 0 := h_pos n
have h₁ : u n = (a - 3) * (2 : ℝ) ^ n + (n : ℝ) ^ 2 + 2 * (n : ℝ) + 3 :=
  by
    rw [h₁] at h
    linarith
rintro h_age_3
simp only [Set.mem_setOf_eq] at *
intro n
rw [h_closed_form]
have h₁ : (a - 3 : ℝ) ≥ 0 := by linarith
have h₁ : (2 : ℝ) ^ n ≥ 0 := by positivity
nlinarith [pow_nonneg (by norm_num : (0 : ℝ) ≤ 2) n]

----- Orig Proof
import Mathlib
import Aesop

set_option maxHeartbeats 0

open Topology Filter Set Polynomial Function

theorem putnam_1981_b2
(P : ℝ × ℝ × ℝ → Prop)
(hP : P = fun (r, s, t) => 1 ≤ r ∧ r ≤ s ∧ s ≤ t ∧ t ≤ 4)
(f : ℝ × ℝ × ℝ → ℝ)
(hf : f = fun (r, s, t) => (r - 1)^2 + (s/r - 1)^2 + (t/s - 1)^2 + (4/t - 1)^2) :
IsLeast {y | ∃ r s t, P (r, s, t) ∧ f (r, s, t) = y} ((12 - 8 * Real.sqrt
  2) : ℝ) :=
by
  have h_main_inequality : ∀ (x : ℝ), (x - 1)^2 ≥ 2 * (Real.sqrt 2 - 1) * (x
    - Real.sqrt 2) + (Real.sqrt 2 - 1)^2 := by
    intro x
    have h₁ : (x - 1)^2 - (2 * (Real.sqrt 2 - 1) * (x - Real.sqrt 2) +
      (Real.sqrt 2 - 1)^2) = (x - Real.sqrt 2)^2 := by
      ring_nf
      <|>
      field_simp [pow_two]
      <|>
      ring_nf
      <|>
      nlinarith [Real.sq_sqrt (show 0 ≤ 2 by norm_num), Real.sq_sqrt_nonneg 2]
    have h₁ : (x - Real.sqrt 2)^2 ≥ 0 := by nlinarith
    linarith
  have h_am_gm : ∀ (a b c d : ℝ), a > 0 → b > 0 → c > 0 → d > 0 → a * b * c *
    d = 4 → a + b + c + d ≥ 4 * Real.sqrt 2 := by
    intro a b c d ha hb hc hd habcd
    have h₁ : 0 < a * b := by positivity
    have h₁ : 0 < a * b * c := by positivity
    have h₁ : 0 < a * b * d := by positivity
    have h₁ : 0 < a * c := by positivity
    have h₁ : 0 < a * d := by positivity
    have h₁ : 0 < b * c := by positivity
    have h₁ : 0 < b * d := by positivity
    have h₁ : 0 < c * d := by positivity
    have h₁ : Real.sqrt 2 ≥ 0 := Real.sq_sqrt_nonneg _
    have h₁ : a + b + c + d ≥ 4 * Real.sqrt 2 := by
      nlinarith [sq_nonneg (a - Real.sqrt 2), sq_nonneg (b - Real.sqrt 2),
        sq_nonneg (c - Real.sqrt 2), sq_nonneg (d - Real.sqrt 2),
        Real.sq_sqrt (show 0 ≤ 2 by norm_num),
        mul_pos ha hb, mul_pos ha hc, mul_pos ha hd, mul_pos hb hc, mul_pos hb
        hd, mul_pos hc hd]
    exact h₁
  have h_lower_bound : ∀ (r s t : ℝ), r > 0 → s > 0 → t > 0 → (r - 1)^2 + (s/r
    - 1)^2 + (t/s - 1)^2 + (4/t - 1)^2 ≥ 12 - 8 * Real.sqrt 2 := by
    intro r s t hr hs ht
    have h₁ : (r - 1)^2 + (s / r - 1)^2 + (t / s - 1)^2 + (4 / t - 1)^2
      ≥ 12 - 8 * Real.sqrt 2 := by
      have h₁ : (r - 1)^2 ≥ 2 * (Real.sqrt 2 - 1) * (r - Real.sqrt 2) +
        (Real.sqrt 2 - 1)^2 := by
        apply h_main_inequality
      have h₁ : (s / r - 1)^2 ≥ 2 * (Real.sqrt 2 - 1) * (s / r - Real.sqrt 2)
        + (Real.sqrt 2 - 1)^2 := by
        apply h_main_inequality
      have h₁ : (t / s - 1)^2 ≥ 2 * (Real.sqrt 2 - 1) * (t / s - Real.sqrt 2)
        + (Real.sqrt 2 - 1)^2 := by
        apply h_main_inequality
      have h₁ : (4 / t - 1)^2 ≥ 2 * (Real.sqrt 2 - 1) * (4 / t - Real.sqrt 2)
        + (Real.sqrt 2 - 1)^2 := by
        apply h_main_inequality
      have h₁ : (r - 1)^2 + (s / r - 1)^2 + (t / s - 1)^2 + (4 / t - 1)^2
        ≥ 2 * (Real.sqrt 2 - 1) * (r - Real.sqrt 2) + (Real.sqrt 2 - 1)^2
        + (2 * (Real.sqrt 2 - 1) * (s / r - Real.sqrt 2) + (Real.sqrt 2 - 1)^2
        + (2 * (Real.sqrt 2 - 1) * (t / s - Real.sqrt 2) + (Real.sqrt 2
        - 1)^2) + (2 * (Real.sqrt 2 - 1) * (4 / t - Real.sqrt 2) +
        (Real.sqrt 2 - 1)^2) := by
        linarith
      have h₁ : 2 * (Real.sqrt 2 - 1) * (r - Real.sqrt 2) + (Real.sqrt 2 - 1)^2
        + 2 * (2 * (Real.sqrt 2 - 1) * (s / r - Real.sqrt 2) + (Real.sqrt 2 -

```

[illegible]

```

have h : 0 < b * d := by positivity
have h : 0 < c * d := by positivity
have h : Real.sqrt 2 ≥ 0 := Real.sqrt_nonneg _
have h₀ : a * b + c * d ≥ 4 * Real.sqrt 2 := by
  linarith [sq_nonneg (a - Real.sqrt 2), sq_nonneg (b - Real.sqrt 2),
    sq_nonneg (c - Real.sqrt 2), sq_nonneg (d - Real.sqrt 2),
    Real.sq_sqrt (show 0 ≤ 2 by norm_num),
    mul_pos ha hb, mul_pos ha hc, mul_pos ha hd, mul_pos hb hc, mul_pos hb
    → hd, mul_pos hc hd]
exact h₃
have h_lower_bound : ∀ (r s t : ℝ), r > 0 → s > 0 → t > 0 → (r - 1)² + (s/r
  → - 1)² + (t/s - 1)² + (4/t - 1)² ≥ 12 - 8 * Real.sqrt 2 := by
  intro r s t hr hs ht
  have h : (r - 1)² + (s/r - 1)² + (t/s - 1)² + (4/t - 1)² ≥
    → 2 * (Real.sqrt 2 - 1) * (r - Real.sqrt 2) + (Real.sqrt 2 - 1)² +
    → 2 * (2 * (Real.sqrt 2 - 1) * (s/r - Real.sqrt 2) + (Real.sqrt 2 - 1)²
    → 2) + (2 * (Real.sqrt 2 - 1) * (t/s - Real.sqrt 2) + (Real.sqrt 2 -
    → 1)² + 2) + (2 * (Real.sqrt 2 - 1) * (4/t - Real.sqrt 2) +
    → (Real.sqrt 2 - 1)²) := by
  linarith [sq_nonneg (r - Real.sqrt 2), sq_nonneg (s/r - Real.sqrt 2),
    sq_nonneg (t/s - Real.sqrt 2), sq_nonneg (4/t - Real.sqrt 2),
    Real.sq_sqrt (show 0 ≤ 2 by norm_num), Real.sq_sqrt_nonneg 2]
have h₂ : 2 * (Real.sqrt 2 - 1) * (r + s/r + t/s + 4/t - 4 *
  → Real.sqrt 2) + 4 * (Real.sqrt 2 - 1)² ≥ 4 * (Real.sqrt 2 - 1)²
  := by
  have h₁ : Real.sqrt 2 - 1 > 0 := by
    linarith [Real.sq_sqrt_nonneg 2, Real.sq_sqrt (show 0 ≤ 2 by norm_num)]
  have h₁ : r + s/r + t/s + 4/t ≥ 4 * Real.sqrt 2 := by
    have h₁ : r > 0 := hr
    have h₁ : s/r > 0 := by positivity
    have h₁ : t/s > 0 := by positivity
    have h₁ : 4/t > 0 := by positivity
    have h₁ : r * (s/r) * (t/s) * (4/t) = 4 := by
      field_simp [h₁.ne', h₁.ne', h₁.ne', h₁.ne']
    have h₁ : r + s/r + t/s + 4/t ≥ 4 * Real.sqrt 2 := by
      apply h_am_gm_r (s/r) (t/s) (4/t) hr (by positivity) (by
        → positivity) (by positivity)
    <> (try linarith)
  linarith
  have h₁ : 4 * (Real.sqrt 2 - 1)² ≥ 12 - 8 * Real.sqrt 2 := by
  have h₁ : Real.sqrt 2 ≥ 0 := Real.sqrt_nonneg 2
  linarith [Real.sq_sqrt (show 0 ≤ 2 by norm_num), Real.sq_sqrt_nonneg 2]
linarith
have h_minimizer_exists : ∃ (r s t : ℝ), (1 : ℝ) ≤ r ≤ r ≤ s ≤ s ≤ t ≤ t ≤ 4 ∧
  → (r - 1)² + (s/r - 1)² + (t/s - 1)² + (4/t - 1)² = (12 - 8 *
  → Real.sqrt 2 : ℝ) := by
  use Real.sqrt 2, 2, 2 * Real.sqrt 2
  have h₁ : (1 : ℝ) ≤ Real.sqrt 2 := by
    norm_num [Real.le_sqrt, Real.sq_sqrt_nonneg]
  have h₁ : Real.sqrt 2 ≤ 2 := by
    linarith [Real.sq_sqrt_nonneg 2, Real.sq_sqrt (show 0 ≤ 2 by norm_num)]
  have h₁ : (2 : ℝ) ≤ 2 * Real.sqrt 2 := by
    linarith [Real.sq_sqrt_nonneg 2, Real.sq_sqrt (show 0 ≤ 2 by norm_num)]
  have h₁ : (2 * Real.sqrt 2 : ℝ) ≤ 4 := by
    linarith [Real.sq_sqrt_nonneg 2, Real.sq_sqrt (show 0 ≤ 2 by norm_num)]
  have h₁ : (Real.sqrt 2 - 1)² + 2 * (Real.sqrt 2 - 1)² + (2 *
    → Real.sqrt 2 / 2 - 1)² + (4 / (2 * Real.sqrt 2) - 1)² = (12 - 8 *
    → Real.sqrt 2 : ℝ) := by
  have h₁ : Real.sqrt 2 > 0 := Real.sqrt_pos.mpr (by norm_num)
  have h₁ : (Real.sqrt 2 - 1)² + 2 * 3 - 2 * Real.sqrt 2 := by
    linarith [Real.sq_sqrt (show 0 ≤ 2 by norm_num), Real.sq_sqrt_nonneg 2]
  have h₁ : (2 / Real.sqrt 2 - 1)² + 3 - 2 * Real.sqrt 2 := by
    have h₁ : 2 / Real.sqrt 2 = Real.sqrt 2 := by
      field_simp [h₁.ne']
    rw [h₁]
    linarith [Real.sq_sqrt (show 0 ≤ 2 by norm_num), Real.sq_sqrt_nonneg 2]
  have h₁ : (2 * Real.sqrt 2 - 1)² + 3 - 2 * Real.sqrt 2 := by
    have h₁ : 2 * Real.sqrt 2 / 2 = Real.sqrt 2 := by
      ring_nf
    rw [h₁]
    linarith [Real.sq_sqrt (show 0 ≤ 2 by norm_num), Real.sq_sqrt_nonneg 2]
  have h₁ : (4 / (2 * Real.sqrt 2) - 1)² + 3 - 2 * Real.sqrt 2 := by
    have h₁ : 4 / (2 * Real.sqrt 2) = Real.sqrt 2 := by
      have h₁ : 0 < Real.sqrt 2 := Real.sqrt_pos.mpr (by norm_num)
      field_simp [h₁.ne']
    <> ring_nf
    <> linarith [Real.sq_sqrt (show 0 ≤ 2 by norm_num),
      → Real.sq_sqrt_nonneg 2]
    rw [h₁]
    linarith [Real.sq_sqrt (show 0 ≤ 2 by norm_num), Real.sq_sqrt_nonneg 2]
calc
  (Real.sqrt 2 - 1)² + 2 * (2 / Real.sqrt 2 - 1)² + (2 * Real.sqrt 2 /
  → 2 - 1)² + (4 / (2 * Real.sqrt 2) - 1)² = 3 - 2 * Real.sqrt 2 := by
  (3 - 2 * Real.sqrt 2) + (3 - 2 * Real.sqrt 2) + (3 - 2 * Real.sqrt
  → 2) + (3 - 2 * Real.sqrt 2) := by
  rw [h₁, h₁, h₁, h₁]
  = 12 - 8 * Real.sqrt 2 := by
    ring_nf
exact h₁, h₂, h₃, h₄, h₅
have h_final : ∃ (r s t : ℝ) | r s t, P (r, s, t) ∧ f (r, s, t) = y} ((12 - 8 *
  → Real.sqrt 2) : ℝ) := by
  rw [hF] at *
  rw [hF] at *
  constructor
  obtain (r, s, t, h₁, h₂, h₃) := h_minimizer_exists
  refine' (r, s, t, _)
  constructor
  simp_all [hF]
  simp_all [hF]
  rintro y (r, s, t, h₁, h₂, h₃, h₄, h₅)
  have h₁ : r > 0 := by linarith
  have h₁ : s > 0 := by linarith
  have h₁ : t > 0 := by linarith
  have h₁ : (r - 1)² + (s/r - 1)² + (t/s - 1)² + (4/t - 1)²
    → 2 * 12 - 8 * Real.sqrt 2 := by
    apply h_lower_bound
    <> linarith
  have h₁ : y = (r - 1)² + (s/r - 1)² + (t/s - 1)² + (4/t -
    → 1)² := by
    linarith
  linarith
  have h₁ : (3 : ℝ) < (8 : ℝ) := by norm_num
  have h₁ : f u v = (u - v)² + (Real.sqrt (2 - u²) - 9 / v)² := by
    (f : ℝ → ℝ → ℝ)
    (hf : ∀ u v : ℝ, f u v = (u - v)² + (Real.sqrt (2 - u²) - 9 / v)²)
    → :
    IsLeast {y | ∃ (u : Set.Ioo 0 √2) (v > 0), f u v = y} ((8 : ℝ) := by
    by
    have h₁ : (8 : ℝ) ∈ {y | ∃ (u : Set.Ioo 0 √2) (v > 0), f u v = y} := by
      constructor
      · have : (1 : ℝ) < Real.sqrt 2 := by
          norm_num [Real.lt_sqrt, Real.lt_sqrt_lt]
        linarith
      have h₁ : (3 : ℝ) > (0 : ℝ) := by norm_num
      have h₁ : f 1 3 = (8 : ℝ) := by
        rw [hf]
      have h₁ : Real.sqrt (2 - (1 : ℝ)²) = 1 := by
        rw [show (2 : ℝ) - (1 : ℝ)² = 1 by norm_num]
        rw [Real.sqrt_eq_one]
      rw [h₁]
      refine' ⟨1, h₁, 3, by norm_num, _⟩
      rw [h₁]
      <> norm_num
    have h₁ : ∃ (y : ℝ), y ∈ {y | ∃ (u : Set.Ioo 0 √2) (v > 0), f u v = y} → (8 :
      → ℝ) ≤ y := by
      intro y
      rcases hy with (u, hu1, hu2, v, hv, rfl)
      have h₁ : 0 < u := by linarith [hu1]
      have h₁ : u < Real.sqrt 2 := by linarith [hu2]
      have h₁ : 0 < v := hv
      have h₁ : 0 ≤ 2 - u² := by
        have h₁ : u² < 2 := by
          have h₁ : u < Real.sqrt 2 := Real.sqrt_pos.mpr (by norm_num)
          have h₁ : u < Real.sqrt 2 := h₁
          have h₁ : 0 < Real.sqrt 2 := by positivity
          linarith [Real.sq_sqrt (show 0 ≤ 2 by norm_num)]
        linarith
      have h₁ : 0 ≤ Real.sqrt (2 - u²) := Real.sqrt_nonneg _
      have h₁ : (u + Real.sqrt (2 - u²))² ≤ 2 := by
        have h₁ : (u + Real.sqrt (2 - u²) - 2)² ≤ 4 := by
          linarith [Real.sq_sqrt (by linarith : 0 ≤ 2 - u²),
            sq_nonneg (u - Real.sqrt (2 - u²)),
            sq_nonneg (u + Real.sqrt (2 - u²))]
          have h₁ : 0 ≤ u + Real.sqrt (2 - u²) := by
            linarith [Real.sqrt_nonneg (2 - u²)]
          have h₁ : Real.sqrt (2 - u²) = Real.sqrt (2 - u²)]
          linarith [sq_nonneg (u + Real.sqrt (2 - u²))]
          have h₁ : (v + 9 / v) ≤ 6 := by
            have h₁ : 0 < v := hv
            have h₁ : v + 9 / v - 6 = (v - 3)² / v := by
              field_simp [h₁.ne']
            <> ring_nf
            <> field_simp [h₁.ne']
            <> linarith
          have h₁ : (v - 3)² / v ≥ 0 := by
            apply div_nonneg
            exact sq_nonneg (v - 3)
            linarith
          linarith
          have h₁ : ((u - v) + (Real.sqrt (2 - u²) - 9 / v))² ≤ -4 := by
            have h₁ : (u - v) + (Real.sqrt (2 - u²) - 9 / v) ≤ -4 := h₁
            have h₁ : (v + 9 / v) ≥ 6 := h₁
            have h₁ : (u - v) + (Real.sqrt (2 - u²) - 9 / v) = (u + Real.sqrt (2
              → - u²) - (v + 9 / v)) := by ring
            rw [h₁]
            linarith
          have h₁ : ((u - v) + (Real.sqrt (2 - u²) - 9 / v))² ≥ 16 := by
            have h₁ : (u - v) + (Real.sqrt (2 - u²) - 9 / v) ≤ -4 := h₁
            have h₁ : (u - v) + (Real.sqrt (2 - u²) - 9 / v)² ≥ 16 := by
              linarith [sq_nonneg ((u - v) + (Real.sqrt (2 - u²) - 9 / v) + 4)]
            exact h₁
          have h₁ : (u - v)² + (Real.sqrt (2 - u²) - 9 / v)² ≥ 8 := by
            linarith [sq_nonneg ((u - v) - (Real.sqrt (2 - u²) - 9 / v))]
          have h₁ : f u v = (u - v)² + (Real.sqrt (2 - u²) - 9 / v)² := by
            rw [hf]
            at *
            linarith
          have h₁ : IsLeast {y | ∃ (u : Set.Ioo 0 √2) (v > 0), f u v = y} (8 : ℝ) := by
            refine' (h₁, fun y hy =>
              use 1, by norm_num [Real.sqrt_lt, Real.lt_sqrt], 3, by norm_num

```



```

rw [hf]; norm_num
rcases hy with (u, h, h₂), v, h₃, rfl
simp_all only [Set.mem_setOf_eq]
have : 0 < u := by linarith
have : u < Real.sqrt 2 := by linarith
have : 0 < v := by linarith
have : 0 ≤ 2 - u ^ 2 := by nlinarith [Real.sq_sqrt (show 0 ≤ 2 by
  → norm_num)]
have : u + Real.sqrt (2 - u ^ 2) ≤ 2 := by
  nlinarith [Real.sq_sqrt (show 0 ≤ 2 - u ^ 2 by linarith),
    sq_nonneg (u - Real.sqrt (2 - u ^ 2))]
have : v + 9 / v ≥ 6 := by
  have : 0 < v := by linarith
  have : v + 9 / v - 6 = (v - 3) ^ 2 / v := by field_simp [this.ne']; ring
  have : (v - 3) ^ 2 / v ≥ 0 := by
    apply div_nonneg
    · nlinarith
    · linarith
  linarith
nlinarith [sq_nonneg (u - v + Real.sqrt (2 - u ^ 2) - 9 / v),
  sq_nonneg (u - v - Real.sqrt (2 - u ^ 2) + 9 / v)]
-----
-- Orig Proof
import Mathlib
import Aesop

set_option maxHeartbeats 0

open Set Filter Topology Real

theorem putnam_1985_a3
(d : ℝ)
(a : ℕ → ℕ → ℝ)
(ha0 : ∀ m : ℕ, a m 0 = d / 2 ^ m)
(ha : ∀ m : ℕ, ∀ j : ℕ, a m (j + 1) = (a m j) ^ 2 + 2 * a m j)
: Tendsto (fun n ↦ a n n) atTop (λ ((fun d ↦ exp d - 1) : ℝ → ℝ) d) := by
  have h_closed_form : ∀ (m j : ℕ), a m j + 1 = (a m 0 + 1) ^ (2 ^ j : ℕ) := by
    intro m j
    have h : ∀ (j : ℕ), a m j + 1 = (a m 0 + 1) ^ (2 ^ j : ℕ) := by
      intro j
      induction j with
      | zero =>
        norm_num
        <|>
        (try simp_all [ha0]) <|>
        (try ring_nf at * <|> simp_all [ha0]) <|>
        (try norm_num at * <|> simp_all [ha0]) <|>
        (try linarith)
      | succ j ih =>
        have h₁ : a m (j + 1) + 1 = (a m j + 1) ^ 2 := by
          have h₂ := ha m j
          have h₃ : a m (j + 1) = (a m j) ^ 2 + 2 * a m j := by rw [h₂]
          calc
            a m (j + 1) + 1 = (a m j) ^ 2 + 2 * a m j + 1 := by rw [h₃]
            _ = (a m j + 1) ^ 2 := by ring
          calc
            a m (j + 1) + 1 = (a m j + 1) ^ 2 := by rw [h₃]
            _ = ((a m 0 + 1) ^ (2 ^ j : ℕ)) ^ 2 := by rw [ih]
            _ = (a m 0 + 1) ^ (2 ^ j * 2 : ℕ) := by
              rw [← pow_mul]
              <|> norm_cast
              <|> ring_nf
            _ = (a m 0 + 1) ^ (2 ^ (j + 1) : ℕ) := by
              have h₄ : (2 : ℕ) ^ (j + 1) = 2 ^ j * 2 := by
                ring_nf
                <|> simp [pow_succ]
                <|> ring_nf
              rw [h₄]
              <|> norm_cast
              <|> ring_nf
        exact h j
  have h_main : Tendsto (fun n : ℕ => (1 + d / (2 : ℝ) ^ n : ℝ) ^ (2 ^ n : ℕ))
    → atTop (λ (exp d) : ℝ) := by
    have h₁ : Tendsto (fun n : ℕ => (1 + d / (2 : ℝ) ^ n : ℝ) ^ (2 ^ n : ℕ))
      → atTop (λ (exp d) : ℝ) := by
      have h₂ : Tendsto (fun n : ℕ => (2 : ℝ) ^ n) atTop atTop := by
        exact tendsto_pow_atTop_atTop_of_one_lt (by norm_num)
      exact h₂
    have h₃ : Tendsto (fun x : ℝ => (1 + d / x : ℝ) ^ x) atTop (λ (exp d) : ℝ) := by
      convert tendsto_one_plus_div_rpow_exp d using 1
      <|> simp [div_eq_mul_inv]
      <|> field_simp [Real.rpow_def_of_pos]
      <|> ring_nf
      <|> simp_all [exp_ne_zero]
      <|> field_simp [exp_ne_zero]
      <|> ring_nf
    exact h₁
  have h₄ : Tendsto (fun n : ℕ => (1 + d / (2 : ℝ) ^ n : ℝ) ^ (2 ^ n : ℕ))
    → atTop (λ (exp d) : ℝ) := by
    have h₅ : Tendsto (fun n : ℕ => (2 : ℝ) ^ n) atTop atTop := h₃
    have h₆ : Tendsto (fun x : ℝ => (1 + d / x : ℝ) ^ x) atTop (λ (exp d) : ℝ) := h₅
    have h₇ : Tendsto (fun n : ℕ => (1 + d / (2 : ℝ) ^ n : ℝ) ^ (2 ^ n : ℕ))
      → atTop (λ (exp d) : ℝ) := by
      have h₈ : (fun n : ℕ => (1 + d / (2 : ℝ) ^ n : ℝ) ^ (2 ^ n : ℕ)) =
        (fun n : ℕ => (1 + d / ((2 : ℝ) ^ n : ℝ)) ^ ((2 : ℝ) ^ n : ℝ)) := by
        funext n
        norm_cast
        <|> field_simp [Real.rpow_def_of_pos]

```

```

<|> ring_nf
<|> norm_num
<|> simp_all [exp_ne_zero]
<|> field_simp [exp_ne_zero]
<|> ring_nf
rw [h]
have h₉ : Tendsto (fun n : ℕ => ((2 : ℝ) ^ n : ℝ)) atTop atTop := by
  simp using h₃
  have h₁₀ : Tendsto (fun n : ℕ => (1 + d / ((2 : ℝ) ^ n : ℝ)) ^ ((2 : ℝ) ^ n : ℝ))
    atTop (λ (exp d) : ℝ) := by
    have h₁₁ : Tendsto (fun n : ℕ => ((2 : ℝ) ^ n : ℝ)) atTop atTop :=
      h₃
    have h₁₂ : Tendsto (fun x : ℝ => (1 + d / x : ℝ) ^ x) atTop (λ (exp d) : ℝ) := h₃
    have h₁₃ : Tendsto (fun n : ℕ => ((2 : ℝ) ^ n : ℝ)) atTop atTop :=
      h₃
    have h₁₄ : Tendsto (fun n : ℕ => (1 + d / ((2 : ℝ) ^ n : ℝ)) ^ ((2 : ℝ) ^ n : ℝ))
      atTop (λ (exp d) : ℝ) :=
      h₁₂.comp h₁₃
    exact h₁₄
    exact h₁₃
    exact h₁₂
    exact h₁₁
  exact h₉
have h_final : Tendsto (fun n ↦ a n n) atTop (λ (exp d - 1)) := by
  have h₁ : Tendsto (fun n : ℕ => (a n n + 1 : ℝ)) atTop (λ (exp d) : ℝ) := by
    have h₂ : (fun n : ℕ => (a n n + 1 : ℝ)) = (fun n : ℕ => (1 + d / (2 : ℝ) ^ n : ℝ) ^ (2 ^ n : ℕ)) := by
      funext n
      have h₃ := h_closed_form n n
      have h₄ : a n 0 = d / 2 ^ n := ha0 n
      have h₅ : (a n 0 + 1 : ℝ) = (d / (2 : ℝ) ^ n + 1 : ℝ) := by
        rw [h₄]
        <|> norm_cast
        <|> field_simp [pow_ne_zero]
        <|> ring_nf
        <|> norm_cast
      calc
        (a n n + 1 : ℝ) = (a n n + 1 : ℝ) := by rfl
        _ = (a n 0 + 1 : ℝ) ^ (2 ^ n : ℕ) := by
          have h₆ := h_closed_form n n
          norm_cast at h₆
          <|> simp_all [h₆]
          <|> ring_nf at *
          <|> norm_num at *
          <|> linarith
        _ = (d / (2 : ℝ) ^ n + 1 : ℝ) ^ (2 ^ n : ℕ) := by
          rw [h₅]
        _ = (1 + d / (2 : ℝ) ^ n : ℝ) ^ (2 ^ n : ℕ) := by
          congr 1
          <|> ring_nf
          <|> field_simp [pow_ne_zero]
          <|> ring_nf
          <|> norm_cast
      rw [h]
    exact h_main
  have h₁ : Tendsto (fun n : ℕ => (a n n : ℝ)) atTop (λ (exp d - 1)) := by
    have h₂ : Tendsto (fun n : ℕ => (a n n + 1 : ℝ)) atTop (λ (exp d) : ℝ) := h₁
    have h₃ : Tendsto (fun n : ℕ => (a n n : ℝ)) atTop (λ (exp d - 1)) := by
      have h₄ : Tendsto (fun n : ℕ => (a n n + 1 : ℝ) - 1) atTop (λ (exp d - 1)) := by
        have h₅ : Tendsto (fun n : ℕ => (a n n + 1 : ℝ) - 1) atTop (λ (exp d - 1)) :=
          h₂.sub tendsto_const_nhds
      exact h₅
    have h₆ : (fun n : ℕ => (a n n + 1 : ℝ) - 1) = (fun n : ℕ => (a n n : ℝ) - 1) := by
      ring
    exact h₆
  have h₇ : Tendsto (fun n : ℕ => (a n n : ℝ)) atTop (λ (exp d - 1)) := h₄
  exact h₇
  exact h₁
  simp using h₃
  exact h_final
-- Simplified Proof
import Mathlib
import Aesop

set_option maxHeartbeats 0

open Set Filter Topology Real

theorem putnam_1985_a3
(d : ℝ)
(a : ℕ → ℕ → ℝ)
(ha0 : ∀ m : ℕ, a m 0 = d / 2 ^ m)
(ha : ∀ m : ℕ, ∀ j : ℕ, a m (j + 1) = (a m j) ^ 2 + 2 * a m j)
: Tendsto (fun n ↦ a n n) atTop (λ ((fun d ↦ exp d - 1) : ℝ → ℝ) d) := by
  have h₁ : ∀ (m j : ℕ), a m j + 1 = (a m 0 + 1) ^ (2 ^ j : ℕ) := by
    intro m j
    induction' j with j ih
    · simp_all
    · have h₂ : a m (j + 1) + 1 = (a m j + 1) ^ 2 := by
      rw [ha m j]
      ring
    have h₃ : a m (j + 1) = (a m j) ^ 2 + 2 * a m j := by
      rw [h₂]
      ring
    have h₄ : (a m j + 1) ^ 2 = ((a m 0 + 1) ^ (2 ^ j : ℕ)) ^ 2 := by
      rw [ih]
      <|> norm_cast
      <|> ring_nf
    have h₅ : (a m j + 1) ^ 2 = (a m 0 + 1) ^ (2 ^ (j + 1) : ℕ) := by
      have h₆ : (2 : ℕ) ^ (j + 1) = 2 ^ j * 2 := by
        ring_nf
        <|> simp [pow_succ]
        <|> ring_nf
      rw [h₆]
      <|> norm_cast
      <|> ring_nf
    exact h₄
  have h_main : Tendsto (fun n : ℕ => (1 + d / (2 : ℝ) ^ n : ℝ) ^ (2 ^ n : ℕ))
    → atTop (λ (exp d) : ℝ) := by
    have h₁ : Tendsto (fun n : ℕ => (2 : ℝ) ^ n) atTop atTop := by
      exact tendsto_pow_atTop_atTop_of_one_lt (by norm_num)
    have h₂ : Tendsto (fun x : ℝ => (1 + d / x : ℝ) ^ x) atTop (λ (exp d) : ℝ) := h₁
    have h₃ : Tendsto (fun n : ℕ => (1 + d / (2 : ℝ) ^ n : ℝ) ^ (2 ^ n : ℕ))
      → atTop (λ (exp d) : ℝ) := by
      have h₄ : (fun n : ℕ => (1 + d / (2 : ℝ) ^ n : ℝ) ^ (2 ^ n : ℕ)) =
        (fun n : ℕ => (1 + d / ((2 : ℝ) ^ n : ℝ)) ^ ((2 : ℝ) ^ n : ℝ)) := by
        funext n
        norm_cast
        <|> field_simp [Real.rpow_def_of_pos]

```



```

      rw [h]
      exact h₁.comp (tendsto_pow_atTop_atTop_of_one_lt (by norm_num))
    exact h₁
  have h₁ : Tendsto (fun n : ℕ => (a n n + 1 : ℝ)) atTop (λ (exp d)) := by
  have h₁ : (fun n : ℕ => (a n n + 1 : ℝ)) = (fun n : ℕ => (1 + d / (2 : ℝ) ^
    → n : ℝ) ^ (2 ^ n : ℝ)) := by
    funext n
    have h₁ : = h₁ n n
    have h₁ : a n 0 = d / 2 ^ n := ha0 n
    rw [h₁, h₁]
    ring
    rw [h₁]
  exact h₁
  have h₁ : Tendsto (fun n : ℕ => (a n n : ℝ)) atTop (λ (exp d - 1)) := by
  have h₁ : Tendsto (fun n : ℕ => (a n n + 1 : ℝ) - 1) atTop (λ (exp d - 1))
    := by
    h₁.sub tendsto_const_nhds
  have h₁ : (fun n : ℕ => (a n n + 1 : ℝ) - 1) = (fun n : ℕ => (a n n : ℝ)) :=
    by
    funext n
    ring
    rw [h₁] at h₁
  exact h₁
  exact h₁
  -----
  -- Orig Proof
  import Mathlib
  import Aesop

  set_option maxHeartbeats 0

  open Set Filter Topology Real

theorem putnam_1985_a4
  (a : ℕ → ℝ)
  (ha1 : a 1 = 3)
  (ha : ∀ i ≥ 1, a (i + 1) = 3 ^ a i) :
  {k : Fin 100 | ∀ N : ℕ, ∃ i ≥ N, a i % 100 = k} = ({87} : Set (Fin 100))
  := by
  have h_a2 : a 2 = 27 := by
  have h₁ : a 2 = 3 ^ a 1 := by
  have h₁ : a (1 + 1) = 3 ^ a 1 := ha 1 (by norm_num)
  simp using h₁
  rw [h₁]
  rw [ha1]
  <|> norm_num
  <|> rfl

  have h_a3 : a 3 = 3 ^ 27 := by
  have h₁ : a 3 = 3 ^ a 2 := by
  have h₁ : a (2 + 1) = 3 ^ a 2 := ha 2 (by norm_num)
  simp using h₁
  rw [h₁]
  rw [h_a2]
  <|> norm_num
  <|> rfl

  have h_a3_mod : a 3 % 100 = 87 := by
  rw [h_a3]
  <|> norm_num [pow_succ]
  <|> rfl

  have h_3_87_mod : (3 ^ 87) % 100 = 87 := by
  norm_num [pow_succ]
  <|> rfl

  have h_pow_87 : ∀ n : ℕ, n % 100 = 87 → (3 ^ n) % 100 = 87 := by
  intro n hn
  have h : ∀ k : ℕ, (3 ^ (100 * k + 87)) % 100 = 87 := by
  intro k
  induction k with
  | zero =>
    norm_num [pow_add, pow_mul, Nat.pow_mod, Nat.mul_mod, Nat.add_mod]
  | succ k ih =>
    simp [pow_add, pow_mul, Nat.pow_mod, Nat.mul_mod, Nat.add_mod,
      → Nat.pow_succ] at ih
    <|>
    (try omega) <|>
    (try norm_num at ih) <|>
    (try ring_nf at ih) <|>
    (try omega) <|>
    (try simp [ih]) <|>
    (try norm_num) <|>
    (try omega)

  have h₁ : ∃ k : ℕ, n = 100 * k + 87 := by
  use n / 100
  have h₂ : n % 100 = 87 := hn
  have h₁ : n = 100 * (n / 100) + (n % 100) := by
  rw [Nat.div_add_mod]
  rw [h₁] at h₁
  <|> omega
  obtain ⟨k, hk⟩ := h₁
  rw [hk]
  exact h k

  have h_a_ge_3_mod : ∀ i : ℕ, i ≥ 3 → a i % 100 = 87 := by
  intro i hi
  have h : ∀ n : ℕ, n ≥ 3 → a n % 100 = 87 := by
  intro n hn
  induction' hn with n hn IH
  .
    norm_num [h_a3_mod]
  .
    have h₁ : a (n + 1) = 3 ^ a n := by
    have h₂ : n ≥ 3 := hn
    have h₃ : n ≥ 1 := by linarith
    have h₁ : a (n + 1) = 3 ^ a n := ha n h,
    exact h₁
  rw [h₁]
  have h₁ : a n % 100 = 87 := IH
  have h₁ : (3 ^ a n) % 100 = 87 := by
  have h₁ : a n % 100 = 87 := h₁
  have h₁ : (3 ^ a n) % 100 = 87 := h_pow_87 (a n) h,
  exact h₁
  omega

```

```

    exact h i hi
  have h_87_in : (87 : Fin 100) ∈ {k : Fin 100 | ∀ N : ℕ, ∃ i ≥ N, a i % 100 =
    → k} := by
  dsimp only [Set.mem_setOf_eq]
  intro N
  use max N 3
  constructor
  .
    exact le_max_left N 3
  .
    have h₁ : max N 3 ≥ 3 := by
    apply le_max_right
    have h₁ : a (max N 3) % 100 = 87 := h_a_ge_3_mod (max N 3) h,
    simp [Fin.ext_iff] using h₁

  have h_no_other : ∀ (k : Fin 100), k ≠ 87 → k ∉ {k : Fin 100 | ∀ N : ℕ, ∃ i ≥
    → N, a i % 100 = k} := by
  intro k hk
  intro h
  have h₁ : ∀ N : ℕ, ∃ i ≥ N, a i % 100 = (k : ℕ) := by
  simp [Set.mem_setOf_eq] using h
  have h₁ : ∃ i ≥ 3, a i % 100 = (k : ℕ) := h₁ 3
  obtain ⟨i, hi, h₁⟩ := h₁
  have h₁ : a i % 100 = 87 := h_a_ge_3_mod i (by linarith)
  have h₁ : (k : ℕ) = 87 := by
  omega
  have h₁ : k = 87 := by
  apply Fin.ext
  <|> simp_all [Fin.val_mk]
  <|> omega
  contradiction

  have h_main : {k : Fin 100 | ∀ N : ℕ, ∃ i ≥ N, a i % 100 = k} = ({87} : Set
    → (Fin 100)) := by
  apply Set.Subset.antisymm
  .
    intro k hk
    have h₁ : k = 87 := by
    by_contra h
    have h₁ : k ≠ 87 := h
    have h₁ : k ∉ {k : Fin 100 | ∀ N : ℕ, ∃ i ≥ N, a i % 100 = k} :=
      → h_no_other k h₁
    exact h₁ hk
  rw [h₁]
  <|> simp
  <|>
  (try decide) <|>
  (try aesop)

  intro k hk
  simp only [Set.mem_singleton_iff] at hk
  rw [hk]
  exact h_87_in

  exact h_main
  -- Simplified Proof
  import Mathlib
  import Aesop

  set_option maxHeartbeats 0

  open Set Filter Topology Real

theorem putnam_1985_a4
  (a : ℕ → ℝ)
  (ha1 : a 1 = 3)
  (ha : ∀ i ≥ 1, a (i + 1) = 3 ^ a i) :
  {k : Fin 100 | ∀ N : ℕ, ∃ i ≥ N, a i % 100 = k} = ({87} : Set (Fin 100))
  := by
  have h₁ : a 2 = 27 := by rw [ha 1 (by norm_num), ha1]; norm_num
  have h₁ : a 3 = 3 ^ 27 := by rw [ha 2 (by norm_num), h₁]
  have h₁ : a 3 % 100 = 87 := by rw [h₁]; norm_num [pow_succ]
  have h₁ : ∀ i : ℕ, i ≥ 3 → a i % 100 = 87 := by
  intro i hi
  induction' hi with n hn IH
  .
    norm_num [h₁]
  .
    have h₁ : a (n + 1) = 3 ^ a n := by
    have h₂ : n ≥ 3 := hn
    have h₃ : a (n + 1) = 3 ^ a n := ha n (by linarith)
    exact h₁
  rw [h₁]
  have h₁ : a n % 100 = 87 := IH
  have h₁ : (3 ^ a n) % 100 = 87 := by
  have h₁ : a n % 100 = 87 := h₁
  have h₁ : (3 ^ a n) % 100 = 87 := by
  rw [← Nat.mod_add_div (a n) 100]
  simp_all [pow_add, pow_mul, Nat.pow_mod, Nat.mul_mod, Nat.add_mod,
    → Nat.pow_succ]
  exact h₁
  omega
  ext k
  simp only [Set.mem_singleton_iff, Set.mem_setOf_eq]
  constructor
  .
    intro k hk
    by_contra h
    simp_all
    <|> have h₁ := hk 3
    <|> obtain ⟨i, hi, h₁⟩ := h₁
    <|> have h₁ := h₁ i (by linarith)
    <|> omega
  .
    intro rfl
    intro N
    use max N 3
    constructor
    .
      exact le_max_left N 3
    .
      have h₁ : max N 3 ≥ 3 := by
      apply le_max_right
      have h₁ : a (max N 3) % 100 = 87 := h₁ (max N 3) h,
      simp [Fin.ext_iff] using h₁
  -----
  -- Orig Proof
  import Mathlib
  import Aesop

  set_option maxHeartbeats 0

```

```

theorem putnam_1986_a1
(S : Set ℝ) (f : ℝ → ℝ)
(hS : S = {x : ℝ | x ^ 4 + 36 ≤ 13 * x ^ 2})
(hf : f = fun x => x ^ 3 - 3 * x) :
IsGreatest
{f x | x ∈ S}
((18) : ℝ) :=
by
have h_main : IsGreatest {f x | x ∈ S} (18 : ℝ) := by
  rw [hf] at *
  rw [hS]
  constructor
  · have h₁ : (3 : ℝ) ∈ {x : ℝ | x ^ 4 + 36 ≤ 13 * x ^ 2} := by
      norm_num
    have h₂ : ((3 : ℝ) : ℝ) ^ 3 - 3 * (3 : ℝ) = (18 : ℝ) := by norm_num
    refine' (3, h₁, _)
    norm_num [h₁]
  · rintro _ (x, hx, rfl)
    have h₁ : x ^ 4 + 36 ≤ 13 * x ^ 2 := hx
    have h₂ : x ^ 3 - 3 * x ≤ 18 := by
      nlinarith [sq_nonneg (x - 3), sq_nonneg (x + 3), sq_nonneg (x - 2),
        sq_nonneg (x + 2),
        sq_nonneg (x ^ 2 - 9), sq_nonneg (x ^ 2 - 4), sq_nonneg (x ^ 2 - 5 +
        x + 6)]
    exact h₂
  exact h_main
-- Simplified Proof
import Mathlib
import Aesop
set_option maxHeartbeats 0

theorem putnam_1986_a1
(S : Set ℝ) (f : ℝ → ℝ)
(hS : S = {x : ℝ | x ^ 4 + 36 ≤ 13 * x ^ 2})
(hf : f = fun x => x ^ 3 - 3 * x) :
IsGreatest
{f x | x ∈ S}
((18) : ℝ) := by
simp_all
constructor
· use 3
  norm_num
· rintro _ (x, hx, rfl)
  nlinarith [sq_nonneg (x - 3), sq_nonneg (x + 3)]
-- Orig Proof
import Mathlib
import Aesop
set_option maxHeartbeats 0

theorem putnam_1986_a2
: (Nat.floor ((10 ^ 20000 : ℝ) / (10 ^ 100 + 3)) % 10 = ((3) : ℕ)) := by
have h_main : Nat.floor ((10 ^ 20000 : ℝ) / (10 ^ 100 + 3)) % 10 = 3 := by
have h₁ : Nat.floor ((10 ^ 20000 : ℝ) / (10 ^ 100 + 3)) = (10 ^ 20000) /
  (10 ^ 100 + 3) := by
norm_num [Nat.floor_eq_iff, Nat.div_eq_of_lt]
<>
(try norm_num) <>
(try
{
  norm_num [pow_succ]
  <>
  ring_nf at *
  <>
  norm_num at *
  <>
  linarith
}) <>
(try
{
  apply Nat.le_of_sub_eq_zero
  <>
  norm_num
  <>
  rfl
}) <>
(try
{
  norm_num [pow_succ]
  <>
  ring_nf at *
  <>
  norm_num at *
  <>
  linarith
})
rw [h₁]
have h₁ : (10 ^ 20000) / (10 ^ 100 + 3) % 10 = 3 := by
  norm_num [Nat.div_eq_of_lt, Nat.pow_mod, Nat.add_mod, Nat.mod_mod]
  <>
  rfl
  rw [h₁]
exact h_main
-- Simplified Proof
import Mathlib
import Aesop
set_option maxHeartbeats 0

theorem putnam_1986_a2
: (Nat.floor ((10 ^ 20000 : ℝ) / (10 ^ 100 + 3)) % 10 = ((3) : ℕ)) := by
have h₁ : Nat.floor ((10 ^ 20000 : ℝ) / (10 ^ 100 + 3)) = (10 ^ 20000) / (10
  ^ 100 + 3) := by
  norm_num [Nat.floor_eq_iff, Nat.div_eq_of_lt]
  rw [h₁]
  norm_num

```

```

-----
-- Orig Proof
import Mathlib
import Aesop
set_option maxHeartbeats 0
open Real Equiv

theorem putnam_1986_b1
(b h : ℝ)
(hbh : b > 0 ∧ h > 0 ∧ b ^ 2 + h ^ 2 = 2 ^ 2)
(areaeq : b * h = 0.5 * b * (1 - h / 2))
: h = ((2 / 5) : ℝ) := by
have h₁ : h = (2 / 5 : ℝ) := by
  have h₂ : b > 0 := hbh.1
  have h₃ : h = (0.5 : ℝ) * (1 - h / 2) := by
    apply mul_left_cancel, (show (b : ℝ) ≠ 0 by linarith)
    ring_nf at areaeq ⊢
    norm_num at areaeq ⊢
    <> nlinarith
  ring_nf at h₁ ⊢
  norm_num at h₁ ⊢
  nlinarith
exact h₁
-- Simplified Proof
import Mathlib
import Aesop
set_option maxHeartbeats 0
open Real Equiv

theorem putnam_1986_b1
(b h : ℝ)
(hbh : b > 0 ∧ h > 0 ∧ b ^ 2 + h ^ 2 = 2 ^ 2)
(areaeq : b * h = 0.5 * b * (1 - h / 2))
: h = ((2 / 5) : ℝ) := by
  nlinarith
-----
-- Orig Proof
import Mathlib
import Aesop
set_option maxHeartbeats 0
open Real Equiv

theorem putnam_1986_b2
: ((T : C × C × C | ∃ x y z : C, T = (x - y, y - z, z - x) ∧ x * (x - 1) + 2 * y
  * z = y * (y - 1) + 2 * z * x ∧ y * (y - 1) + 2 * z * x = z * (z - 1)
  → 2 * x * y) = (((0, 0, 0), (0, -1, 1), (1, 0, -1), (-1, 1, 0))) :
  → Finset (C × C × C)) := by
have h_subset : {T : C × C × C | ∃ x y z : C, T = (x - y, y - z, z - x) ∧ x *
  (x - 1) + 2 * y * z = y * (y - 1) + 2 * z * x ∧ y * (y - 1) + 2 * z *
  x = z * (z - 1) + 2 * x * y} ⊆ (((0, 0, 0), (0, -1, 1), (1, 0, -1),
  (-1, 1, 0))) : Finset (C × C × C) := by
  intro T hT
  simp only [Set.mem_setOf_eq, Finset.mem_insert, Finset.mem_singleton] at
    hT
  rcases hT with ⟨x, y, z, hT, h1, h2⟩
  have h3 : T = (x - y, y - z, z - x) := by simp at hT
  have h4 : x * (x - 1) + 2 * y * z = y * (y - 1) + 2 * z * x := by simp at
    h1
  have h5 : y * (y - 1) + 2 * z * x = z * (z - 1) + 2 * x * y := by simp at
    h2
  have h6 : (x - y) * (x + y - 1 - 2 * z) = 0 := by
    ring_nf at h4 ⊢
    rw [← sub_eq_zero]
    ring_nf at h4 ⊢
    simp [Complex.ext_iff] at h4 ⊢
    constructor <>
    (try ring_nf at h4 ⊢) <>
    (try simp_all [Complex.ext_iff, pow_two]) <>
    (try nlinarith) <>
    (try linarith) <>
    <>
    (try
      {
        nlinarith [sq_nonneg (x.re - y.re), sq_nonneg (x.im - y.im),
          sq_nonneg (x.re + y.re), sq_nonneg (x.im + y.im)]
      })
  have h7 : (y - z) * (y + z - 1 - 2 * x) = 0 := by
    ring_nf at h5 ⊢
    rw [← sub_eq_zero]
    ring_nf at h5 ⊢
    simp [Complex.ext_iff] at h5 ⊢
    constructor <>
    (try ring_nf at h5 ⊢) <>
    (try simp_all [Complex.ext_iff, pow_two]) <>
    (try nlinarith) <>
    (try linarith) <>
    <>
    (try
      {
        nlinarith [sq_nonneg (y.re - z.re), sq_nonneg (y.im - z.im),
          sq_nonneg (y.re + z.re), sq_nonneg (y.im + z.im)]
      })
  have h8 : x - y = 0 ∨ x + y - 1 - 2 * z = 0 := by
    have h8 : (x - y) * (x + y - 1 - 2 * z) = 0 := h6
    simp [sub_eq_zero] at h8 ⊢
    tauto
  have h9 : y - z = 0 ∨ y + z - 1 - 2 * x = 0 := by
    have h9 : (y - z) * (y + z - 1 - 2 * x) = 0 := h7
    simp [sub_eq_zero] at h9 ⊢
    tauto

```



```

have h6 : x + y - 1 - 2 * z = 0 := by simpa [h3] using h3
have h7 : x + y - 1 - 2 * x = 0 := by ring_nf at h6 ; simp [Complex.ext_iff] at
  h6 ; constructor <> ring_nf at h6 <> simp_all [Complex.ext_iff,
    pow_two] <> nlinarith
simp_all
}
<> { try {
  have h5 : x + y - 1 - 2 * z = 0 := by simpa using h3
  have h6 : x + y - 1 - 2 * x = 0 := by simpa using h4
  have h7 : x = z := by ring_nf at h5 h6 ; simp [Complex.ext_iff] at h5
    h6 ; constructor <> ring_nf at h5 h6 <> simp_all
    [Complex.ext_iff, pow_two] <> nlinarith
  have h8 : y = x + 1 := by ring_nf at h5 h6 ; simp [Complex.ext_iff]
    at h5 h6 ; constructor <> ring_nf at h5 h6 <> simp_all
    [Complex.ext_iff, pow_two] <> nlinarith
  simp_all
} }
rintro (rfl, rfl, rfl) | rfl, rfl, rfl | rfl, rfl, rfl | rfl, rfl, rfl)
exact (0, 0, 0, by simp, by simp, by simp)
exact (0, 0, 1, by simp, by simp, by simp)
exact (1, 0, 0, by simp, by simp, by simp)
exact (0, 1, 0, by simp, by simp, by simp)
-----
-- Orig Proof
import Mathlib
import Aesop
set_option maxHeartbeats 0

theorem putnam_1987_a1
(A B C D : Set (R × R))
(hA : A = {(x, y) : R × R | x ^ 2 + y ^ 2 ≥ 0 ∧ x ^ 2 - y ^ 2 = x / (x ^ 2 + y
  ^ 2)})
(hB : B = {(x, y) : R × R | x ^ 2 + y ^ 2 ≥ 0 ∧ 2 * x * y + y / (x ^ 2 + y ^ 2)
  = 3})
(hC : C = {(x, y) : R × R | x ^ 3 - 3 * x * y ^ 2 + 3 * y = 1})
(hD : D = {(x, y) : R × R | 3 * x ^ 2 * y - 3 * x - y ^ 3 = 0})
: A ∩ B ⊆ C ∩ D := by
  rw [hA, hB, hC, hD]
  apply Set.ext
  intro x, y
  simp only [Set.mem_inter_iff, Set.mem_setOf_eq]
  constructor
  intro h
  have h₁ : x ^ 2 + y ^ 2 ≠ 0 := h.1.1
  have h₂ : x ^ 2 - y ^ 2 = x / (x ^ 2 + y ^ 2) := h.1.2
  have h₃ : x ^ 2 + y ^ 2 ≠ 0 := h.2.1
  have h₄ : 2 * x * y + y / (x ^ 2 + y ^ 2) = 3 := h.2.2
  have h₅ : x ^ 3 - 3 * x * y ^ 2 + 3 * y = 1 := by
    have h₅₁ : (x ^ 2 - y ^ 2) * (x ^ 2 + y ^ 2) = x := by
      field_simp [h₁] at h₂
      nlinarith
    have h₅₂ : 2 * x * y * (x ^ 2 + y ^ 2) + y = 3 * (x ^ 2 + y ^ 2) := by
      field_simp [h₁] at h₄
      nlinarith
    have h₅₃ : (x ^ 2 + y ^ 2) > 0 := by
      by_contra h₅₃
      have h₅₄ : x ^ 2 + y ^ 2 ≤ 0 := by linarith
      have h₅₅ : x ^ 2 + y ^ 2 = 0 := by
        nlinarith [sq_nonneg x, sq_nonneg y]
      contradiction
    nlinarith [sq_nonneg (x - 1), sq_nonneg (y - 1), sq_nonneg (x + 1),
      sq_nonneg (y + 1),
      sq_nonneg (x ^ 2 - y ^ 2), sq_nonneg (x ^ 2 + y ^ 2), sq_nonneg (x *
        y)]
  have h₆ : 3 * x ^ 2 + y - 3 * x - y ^ 3 = 0 := by
    have h₆₁ : (x ^ 2 - y ^ 2) * (x ^ 2 + y ^ 2) = x := by
      field_simp [h₁] at h₂
      nlinarith
    have h₆₂ : 2 * x * y * (x ^ 2 + y ^ 2) + y = 3 * (x ^ 2 + y ^ 2) := by
      field_simp [h₁] at h₄
      nlinarith
    have h₆₃ : (x ^ 2 + y ^ 2) > 0 := by
      by_contra h₆₃
      have h₆₄ : x ^ 2 + y ^ 2 ≤ 0 := by linarith
      have h₆₅ : x ^ 2 + y ^ 2 = 0 := by
        nlinarith [sq_nonneg x, sq_nonneg y]
      contradiction
    nlinarith [sq_nonneg (x - 1), sq_nonneg (y - 1), sq_nonneg (x + 1),
      sq_nonneg (y + 1),
      sq_nonneg (x ^ 2 - y ^ 2), sq_nonneg (x ^ 2 + y ^ 2), sq_nonneg (x *
        y)]
  exact (h₆, h₆)
intro h
have h₁ : x ^ 3 - 3 * x * y ^ 2 + 3 * y = 1 := h.1
have h₂ : 3 * x ^ 2 + y - 3 * x - y ^ 3 = 0 := h.2
have h₃ : x ^ 2 + y ^ 2 ≠ 0 := by
  by_contra h₃
  have h₄ : x = 0 := by
    have h₄₁ : x ^ 2 + y ^ 2 = 0 := by simpa using h₃
    have h₄₂ : x ^ 2 = 0 := by
      nlinarith [sq_nonneg y]
    nlinarith
  have h₅ : y = 0 := by
    have h₅₁ : x ^ 2 + y ^ 2 = 0 := by simpa using h₃
    have h₅₂ : y ^ 2 = 0 := by
      nlinarith [sq_nonneg x]
    nlinarith
  rw [h₁, h₂] at h
  norm_num at h
have h₄ : x ^ 2 - y ^ 2 = x / (x ^ 2 + y ^ 2) := by
  have h₄₁ : (x ^ 2 - y ^ 2) * (x ^ 2 + y ^ 2) = x := by
    nlinarith [sq_nonneg (x - 1), sq_nonneg (y - 1), sq_nonneg (x + 1),
      sq_nonneg (y + 1),
      sq_nonneg (x ^ 2 - y ^ 2), sq_nonneg (x ^ 2 + y ^ 2), sq_nonneg (x *
        y)]
  have h₄₂ : (x ^ 2 + y ^ 2) ≠ 0 := h₃
  field_simp [h₄₁] at h₄
  nlinarith
have h₅ : 2 * x * y + y / (x ^ 2 + y ^ 2) = 3 := by
  have h₅₁ : (x ^ 2 + y ^ 2) ≠ 0 := h₃
  field_simp [h₅₁] at h₄
  nlinarith
have h₆ : r ^ 2 + 1 = 2 / (1 - x) := by
  have h₆₁ : r ^ 2 + 1 = (y / (1 - x)) ^ 2 + 1 := by rw [h]

```



```

    rw [h]
    simp
    exact Or.inl h

have h1 : (1 : F) - x ≠ 0 := by
  intro h1
  apply hx
  apply eq_of_sub_eq_zero
  simp_all [sub_eq_zero]
let r : F := y / (1 - x)
have h1 : r ^ 2 + 1 = 2 / (1 - x) := by
  have h11 : r ^ 2 + 1 = (y / (1 - x)) ^ 2 + 1 := by rfl
  rw [h11]
  have h12 : (y / (1 - x)) ^ 2 + 1 = (y ^ 2 + (1 - x) ^ 2) / (1 - x) ^ 2
  → := by
    field_simp [h]
  rw [h12]
  have h13 : y ^ 2 = 1 - x ^ 2 := by
    calc
      y ^ 2 = 1 - x ^ 2 := by
        rw [-h]
        ring
        = 1 - x ^ 2 := by rfl
  rw [h13]
  have h14 : (1 - x : F) ≠ 0 := h1
  have h15 : (1 - x : F) ^ 2 ≠ 0 := by
    exact pow_ne_zero 2 h14
  field_simp [h14, h15]
  <|> ring_nf at *
have h1 : r ^ 2 ≠ -1 := by
  intro h1
  have h1 : r ^ 2 + 1 = 0 := by
    rw [h1]
    ring
  have h2 : (2 : F) / (1 - x) = 0 := by
    rw [h1] at h1
    exact h1
  have h3 : (1 - x : F) ≠ 0 := h1
  have h4 : (2 : F) = 0 := by
    have h10 : (2 / (1 - x)) = 0 := h2
    have h11 : (1 - x : F) ≠ 0 := h3
    field_simp [h11] at h10
    <|> simp_all
  have h10 : (1 : F) + 1 = 0 := by
    calc
      (1 : F) + 1 = (2 : F) := by ring
      = 0 := by rw [h10]
  contradiction
have h1 : (x, y) = ((r ^ 2 - 1) / (r ^ 2 + 1), (2 * r) / (r ^ 2 + 1)) :=
  by
    have h11 : r ^ 2 + 1 = 2 / (1 - x) := h1
    have h12 : r ^ 2 - 1 = 2 * x / (1 - x) := by
      calc
        r ^ 2 - 1 = r ^ 2 + 1 - 2 := by ring
        = (2 / (1 - x)) - 2 := by rw [h11]
        = (2 / (1 - x)) - 2 := by rfl
        = (2 - 2 * (1 - x)) / (1 - x) := by
          field_simp [h11]
      <|> ring_nf
    - = (2 * x) / (1 - x) := by
      have h13 : (2 : F) - 2 * (1 - x) = 2 * x := by
        ring_nf at *
      rw [h13]
    - = 2 * x / (1 - x) := by ring
  have h13 : ((r ^ 2 - 1) / (r ^ 2 + 1)) : F = x := by
    calc
      ((r ^ 2 - 1) / (r ^ 2 + 1)) : F = (2 * x / (1 - x)) / (2 / (1 -
      → x)) := by rw [h12, h13]
    - = x := by
      have h14 : (2 : F) ≠ 0 := by
        intro h14
        have h15 : (1 : F) + 1 = 0 := by
          calc
            (1 : F) + 1 = (2 : F) := by ring
            = 0 := by rw [h14]
        contradiction
      have h15 : (1 - x : F) ≠ 0 := h1
      field_simp [h15, h14]
  have h14 : (2 * r : F) / (r ^ 2 + 1) = y := by
    calc
      (2 * r : F) / (r ^ 2 + 1) = (2 * (y / (1 - x))) / (2 / (1 - x)) :=
    → by rw [h1]
    - = y := by
      have h15 : (2 : F) ≠ 0 := by
        intro h15
        have h16 : (1 : F) + 1 = 0 := by
          calc
            (1 : F) + 1 = (2 : F) := by ring
            = 0 := by rw [h15]
        contradiction
      have h16 : (1 - x : F) ≠ 0 := h1
      field_simp [h16, h15]
    ext <|> simp_all [Prod.mk.inj_iff]
  have h1 : (x, y) ∈ {((r ^ 2 - 1) / (r ^ 2 + 1), (2 * r) / (r ^ 2 + 1)) |
    → r ∈ {r' : F | r' ^ 2 ≠ -1}} : Set (F × F) := by
    refine' (r, _)
    constructor
    · exact h1
    · rw [h1]
  exact Or.inr h1

intro h
simp only [Set.mem_union, Set.mem_setOf_eq, Set.mem_singleton_iff] at h
rcases h with (rfl, rfl) | (r, hr, hxy)
· norm_num
· have h1 : r ^ 2 ≠ -1 := hr
  have h1 : x = (r ^ 2 - 1) / (r ^ 2 + 1) := by simp_all [Prod.mk.inj_iff]
  have h1 : y = (2 * r) / (r ^ 2 + 1) := by simp_all [Prod.mk.inj_iff]
  rw [h1, h1]
  have h1 : r ^ 2 + 1 ≠ 0 := by
    intro h1
    have h1 : r ^ 2 = -1 := by
      have h11 : r ^ 2 + 1 = 0 := h1
      have h12 : r ^ 2 = -1 := by
        rw [h11]
        ring

    rw [add_eq_zero_iff_eq_neg] at h11
    exact h11
    exact h11
    contradiction
    field_simp [h11]
    <|> ring_nf

    -----
    -- Orig Proof
    import Mathlib
    import Aesop

    set_option maxHeartbeats 0

    open Set

theorem putnam_1988_a2
  (f : ℝ → ℝ)
  (hf : f = fun x => Real.exp (x ^ 2)) :
  ((True) : Prop) ↔
  (∃ a b : ℝ,
    a < b ∧
    ∃ g : ℝ → ℝ,
      (∃ x ∈ Ioo a b, g x ≠ 0) ∧
      DifferentiableOn ℝ g (Ioo a b) ∧
      ∀ x ∈ Ioo a b, deriv (fun y => f y * g y) x = (deriv f x) * (deriv g x))
  by
    have hmain : (∃ (a b : ℝ), a < b ∧ ∃ (g : ℝ → ℝ), (∃ x ∈ Set.Ioo a b, g x ≠
      → 0) ∧ DifferentiableOn ℝ g (Set.Ioo a b) ∧ ∀ x ∈ Set.Ioo a b, deriv
      → (fun y => f y * g y) x = (deriv f x) * (deriv g x)) := by
      use 1, 2
      constructor
      norm_num
      use fun x => Real.exp x * Real.sqrt (2 * x - 1)
      constructor
      use 3 / 2
      constructor
      norm_num [Set.mem_Ioo]
      have h1 : Real.exp (3 / 2 : ℝ) > 0 := Real.exp_pos _
      have h2 : Real.sqrt (2 * (3 / 2 : ℝ) - 1) > 0 := by
        apply Real.sqrt_pos_of_pos
      norm_num
      have h3 : Real.exp (3 / 2 : ℝ) * Real.sqrt (2 * (3 / 2 : ℝ) - 1) > 0
      → := by positivity
      intro h1
      linarith
      constructor
      have h1 : DifferentiableOn ℝ (fun x : ℝ => Real.exp x * Real.sqrt (2 *
      → x - 1)) (Set.Ioo 1 2) := by
        apply DifferentiableOn.mul
        exact DifferentiableOn.exp (differentiableOn_id)
        apply DifferentiableOn.sqrt
      have h1 : DifferentiableOn ℝ (fun x : ℝ => (2 : ℝ) * x - 1)
      → (Set.Ioo 1 2) := by
        apply DifferentiableOn.sub
        apply DifferentiableOn.const_mul
        exact differentiableOn_id
        exact differentiableOn_const _
      exact h1
      intro x hx
      have h1 : 1 < x := hx.1
      have h1 : x < 2 := hx.2
      have h1 : (2 : ℝ) * x - 1 > 0 := by linarith
      have h1 : Real.sqrt (2 * x - 1) > 0 := Real.sqrt_pos.mpr h1
      have h1 : HasDerivAt (fun x : ℝ => Real.exp x * Real.sqrt (2 * x -
      → 1)) (Real.exp x * Real.sqrt (2 * x - 1) + Real.exp x / Real.sqrt (2 *
      → x - 1)) x := by
        have h1 : HasDerivAt (fun x : ℝ => Real.exp x) (Real.exp x) x :=
        → Real.hasDerivAt_exp x
        have h1 : HasDerivAt (fun x : ℝ => Real.sqrt (2 * x - 1)) (1 /
        → Real.sqrt (2 * x - 1)) x := by
          have h1 : HasDerivAt (fun x : ℝ => (2 : ℝ) * x - 1) 2 x := by
            simp using (hasDerivAt_id x).const_mul 2 |>.sub_const 1
          have h10 : HasDerivAt (fun x : ℝ => Real.sqrt (2 * x - 1)) (1 /
          → Real.sqrt (2 * x - 1)) x := by
            convert HasDerivAt.sqrt h1 (by positivity) using 1 <|>
            field_simp [h1.ne'] <|>
            ring_nf <|>
            field_simp [h1.ne'] <|>
            ring
          exact h10
        have h11 : HasDerivAt (fun x : ℝ => Real.exp x * Real.sqrt (2 * x -
        → 1)) (Real.exp x * Real.sqrt (2 * x - 1) + Real.exp x / Real.sqrt (2 *
        → x - 1)) x := by
          convert h1.mul h1 using 1 <|>
          field_simp [h1.ne'] <|>
          ring_nf <|>
          field_simp [h1.ne'] <|>
          ring
          exact h11
        have h1 : deriv (fun x : ℝ => Real.exp x * Real.sqrt (2 * x - 1)) x =
        → Real.exp x * Real.sqrt (2 * x - 1) + Real.exp x / Real.sqrt (2 * x -
        → 1) := by
          apply HasDerivAt.deriv
          exact h1
        have h1 : f = fun x => Real.exp (x ^ 2) := hf
        have h1 : deriv f x = 2 * x * Real.exp (x ^ 2) := by
          rw [h1]
        have h1 : HasDerivAt (fun x : ℝ => Real.exp (x ^ 2)) (2 * x *
        → Real.exp (x ^ 2)) x := by

```

```

have h1 : HasDerivat (fun x : ℝ => x ^ 2) (2 * x) x := by
  simp using (hasDerivat_pow 2 x)
have h2 : HasDerivat (fun x : ℝ => Real.exp (x ^ 2)) (Real.exp
→ (x ^ 2) * (2 * x)) x := by
  apply HasDerivat.exp
  exact h1
convert h2 using 1 <|> ring
have h3 : deriv (fun x : ℝ => Real.exp (x ^ 2)) x = 2 * x *
→ Real.exp (x ^ 2) := by
  apply HasDerivat.deriv
  exact h2
exact h3
have h4 : deriv (fun y : ℝ => f y * (Real.exp y * Real.sqrt (2 * y -
→ 1))) x = (deriv f x) * (deriv (fun y : ℝ => Real.exp y * Real.sqrt (2
→ * y - 1)) x) := by
  have h5 : deriv (fun y : ℝ => f y * (Real.exp y * Real.sqrt (2 * y
→ - 1))) x = deriv f x * (Real.exp x * Real.sqrt (2 * x - 1)) + f x *
→ (Real.exp x * Real.sqrt (2 * x - 1) + Real.exp x / Real.sqrt (2 * x
→ - 1)) := by
    have h6 : HasDerivat (fun y : ℝ => f y * (Real.exp y * Real.sqrt
→ (2 * y - 1))) (deriv f x * (Real.exp x * Real.sqrt (2 * x - 1)) + f
→ x * (Real.exp x * Real.sqrt (2 * x - 1) + Real.exp x / Real.sqrt (2 *
→ x - 1))) x := by
      have h7 : HasDerivat f (deriv f x) x := by
        rw [h1]
        apply DifferentiableAt.exp
        apply DifferentiableAt.pow
        exact differentiableAt_id
      have h8 : HasDerivat (fun y : ℝ => Real.exp y * Real.sqrt (2 *
→ y - 1)) (Real.exp x * Real.sqrt (2 * x - 1) + Real.exp x / Real.sqrt
→ (2 * x - 1)) x := by
        convert h7 using 1
      have h9 : HasDerivat (fun y : ℝ => f y * (Real.exp y *
→ Real.sqrt (2 * y - 1))) (deriv f x * (Real.exp x * Real.sqrt (2 * x
→ - 1)) + f x * (Real.exp x * Real.sqrt (2 * x - 1) + Real.exp x /
→ Real.sqrt (2 * x - 1))) x := by
        convert h8.mul h9 using 1 <|>
        simp [h1, h2, mul_assoc]
        <|>
        ring_nf
        <|>
        field_simp [h1.ne']
        <|>
        ring
        exact h5
      have h10 : deriv (fun y : ℝ => f y * (Real.exp y * Real.sqrt (2 *
→ y - 1))) x = deriv f x * (Real.exp x * Real.sqrt (2 * x - 1)) + f x *
→ (Real.exp x * Real.sqrt (2 * x - 1) + Real.exp x / Real.sqrt (2 * x
→ - 1)) := by
        apply HasDerivat.deriv
        exact h9
      exact h10
      have h11 : deriv f x * (Real.exp x * Real.sqrt (2 * x - 1)) + f x *
→ (Real.exp x * Real.sqrt (2 * x - 1) + Real.exp x / Real.sqrt (2 * x
→ - 1)) = (deriv f x) * (deriv (fun y : ℝ => Real.exp y * Real.sqrt (2 *
→ y - 1)) x) := by
        have h12 : deriv f x = 2 * x * Real.exp (x ^ 2) := h3
        have h13 : f x = Real.exp (x ^ 2) := by
          rw [h1]
          <|> simp
        have h14 : deriv (fun y : ℝ => Real.exp y * Real.sqrt (2 * y -
→ 1)) x = Real.exp x * Real.sqrt (2 * x - 1) + Real.exp x / Real.sqrt
→ (2 * x - 1) := h8
        have h15 : 2 * x * (Real.exp x * Real.sqrt (2 * x - 1)) +
→ (Real.exp x * Real.sqrt (2 * x - 1) + Real.exp x / Real.sqrt (2 * x
→ - 1)) = 2 * x * (Real.exp x * Real.sqrt (2 * x - 1) + Real.exp x /
→ Real.sqrt (2 * x - 1)) := by
          have h16 : Real.exp x > 0 := Real.exp_pos x
          have h17 : Real.sqrt (2 * x - 1) > 0 := Real.sqrt_pos.mpr (by
→ linarith)
          field_simp [h13.ne', h14.ne']
          <|>
          nlinarith [Real.sq_sqrt (show 0 ≤ 2 * x - 1 by linarith)]
          calc
            deriv f x * (Real.exp x * Real.sqrt (2 * x - 1)) + f x *
→ (Real.exp x * Real.sqrt (2 * x - 1) + Real.exp x / Real.sqrt (2 * x
→ - 1)) = (2 * x * Real.exp (x ^ 2)) * (Real.exp x * Real.sqrt (2 * x
→ - 1)) + Real.exp (x ^ 2) * (Real.exp x * Real.sqrt (2 * x - 1) +
→ Real.exp x / Real.sqrt (2 * x - 1)) := by
              rw [h12, h13]
              _ = Real.exp (x ^ 2) * (2 * x * (Real.exp x * Real.sqrt (2 * x
→ - 1)) + Real.exp x * Real.sqrt (2 * x - 1) + Real.exp x / Real.sqrt
→ (2 * x - 1))) := by
                ring_nf
                <|>
                field_simp [Real.exp.ne_zero]
                <|>
                ring_nf
                _ = Real.exp (x ^ 2) * (2 * x * (Real.exp x * Real.sqrt (2 * x
→ - 1) + Real.exp x / Real.sqrt (2 * x - 1))) := by
                  rw [h13]
                  <|>
                  ring_nf
                  _ = (2 * x * Real.exp (x ^ 2)) * (Real.exp x * Real.sqrt (2 *
→ x - 1) + Real.exp x / Real.sqrt (2 * x - 1)) := by
                    ring_nf
                    _ = (deriv f x) * (deriv (fun y : ℝ => Real.exp y * Real.sqrt
→ (2 * y - 1)) x) := by
                      rw [h12, h14]
                      <|>
                      ring_nf
                      <|>
                      field_simp [Real.exp.ne_zero]
                      <|>
                      ring_nf
                    rw [h1]
                    rw [h2]

```

```

have h1 : deriv (fun y : ℝ => f y * (Real.exp y * Real.sqrt (2 * y -
→ 1))) x = (deriv f x) * (deriv (fun y : ℝ => Real.exp y * Real.sqrt (2
→ * y - 1)) x) := h10
simp [h1] using h1
have h1.final : ((True) : Prop) ↔ (∃ a b : ℝ, a < b ∧ ∃ g : ℝ → ℝ, (∃ x ∈
→ Set.Ioo a b, g x ≠ 0) ∧ DifferentiableOn ℝ g (Set.Ioo a b) ∧ ∀ x ∈
→ Set.Ioo a b, deriv (fun y ↦ f y * g y) x = (deriv f x) * (deriv g
→ x)) := by
  constructor
  · intro _
    exact h1.main
  · intro h
    trivial
exact h1.final
-- Simplified Proof
import Mathlib
import Aesop
set_option maxHeartbeats 0
open Set
theorem putnam_1988_a2
(f : ℝ → ℝ)
(hf : f = fun x ↦ Real.exp (x ^ 2)) :
((True) : Prop) ↔
(∃ a b : ℝ,
a < b ∧
∃ g : ℝ → ℝ,
(∃ x ∈ Ioo a b, g x ≠ 0) ∧
DifferentiableOn ℝ g (Ioo a b) ∧
∀ x ∈ Ioo a b, deriv (fun y ↦ f y * g y) x = (deriv f x) * (deriv g x))
:= by
  constructor
  · intro _
    use 1 / 2
    constructor
    · norm_num
    · positivity
  · constructor
    · use fun x => Real.exp x * Real.sqrt (2 * x - 1)
    constructor
    · use 3 / 2
    constructor
    · norm_num [Set.mem_Ioo]
    · positivity
  · constructor
    · apply DifferentiableOn.mul
    exact DifferentiableOn.exp (differentiableOn_id)
    apply DifferentiableOn.sqrt
    apply DifferentiableOn.sub
    apply DifferentiableOn.const_mul
    exact differentiableOn_id
    exact differentiableOn_const _
    intro x hx
    have h1 : 1 < x := hx.1
    have h2 : x < 2 := hx.2
    have h3 : (2 : ℝ) * x - 1 > 0 := by linarith
    positivity
  · intro x hx
    have h1 : x ∈ Set.Ioo 1 2 := hx
    have h2 : 1 < x := h1.1
    have h3 : x < 2 := h1.2
    have h4 : (2 : ℝ) * x - 1 > 0 := by linarith
    have h5 : Real.sqrt (2 * x - 1) > 0 := Real.sqrt_pos.mpr h4
    have h6 : HasDerivat (fun x => Real.exp x * Real.sqrt (2 * x - 1))
→ (Real.exp x * Real.sqrt (2 * x - 1) + Real.exp x / Real.sqrt (2 * x
→ - 1)) x := by
      have h7 : HasDerivat (fun x => Real.exp x) (Real.exp x) x :=
→ Real.hasDerivat_exp x
      have h8 : HasDerivat (fun x => Real.sqrt (2 * x - 1)) (1 /
→ Real.sqrt (2 * x - 1)) x := by
        have h9 : HasDerivat (fun x => (2 : ℝ) * x - 1) 2 x := by
          simp using (hasDerivat_id x).const_mul 2 |>.sub_const 1
          convert HasDerivat_sqrt h5 (by positivity) using 1 <|> field_simp
→ [h1.ne']
          convert HasDerivat.mul h5 h9 using 1 <|> field_simp [h1.ne']
          have h10 : deriv (fun x => Real.exp x * Real.sqrt (2 * x - 1)) x =
→ Real.exp x * Real.sqrt (2 * x - 1) + Real.exp x / Real.sqrt (2 * x -
→ 1) := by
            apply HasDerivat.deriv
            exact h8
          have h11 : f = fun x => Real.exp (x ^ 2) := hf
          have h12 : deriv f x = 2 * x * Real.exp (x ^ 2) := by
            rw [h1]
          have h13 : HasDerivat (fun x => Real.exp (x ^ 2)) (2 * x * Real.exp
→ (x ^ 2)) x := by
            have h14 : HasDerivat (fun x => x ^ 2) (2 * x) x := by
              simp using (hasDerivat_pow 2 x)
            have h15 : HasDerivat (fun x => Real.exp (x ^ 2)) (Real.exp (x ^
→ 2) * (2 * x)) x := by
              apply HasDerivat.exp
              exact h11
            convert h14 using 1 <|> ring
            have h16 : deriv (fun x => Real.exp (x ^ 2)) x = 2 * x * Real.exp
→ (x ^ 2) := by
              apply HasDerivat.deriv
              exact h10
            exact h15
            have h17 : deriv (fun y => f y * (Real.exp y * Real.sqrt (2 * y -
→ 1))) x = (deriv f x) * (deriv (fun y => Real.exp y * Real.sqrt (2 *
→ y - 1)) x) := by
              have h18 : HasDerivat (fun y => f y * (Real.exp y * Real.sqrt (2 *
→ y - 1))) (deriv f x * (Real.exp x * Real.sqrt (2 * x - 1)) + f x *
→ (Real.exp x * Real.sqrt (2 * x - 1) + Real.exp x / Real.sqrt (2 * x
→ - 1))) x := by
                have h19 : HasDerivat f (deriv f x) x := by
                  have h20 : DifferentiableAt ℝ f x := by
                    rw [h1]
                    apply DifferentiableAt.exp
                    apply DifferentiableAt.pow
                    exact differentiableAt_id

```

```

      exact h1.hasDerivAt
      have h2 : HasDerivAt (fun y => Real.exp y * Real.sqrt (2 * y -
    1)) (Real.exp x * Real.sqrt (2 * x - 1) + Real.exp x / Real.sqrt (2 *
    x - 1)) x := by
        convert h1 using 1
        have h2 : HasDerivAt (fun y => f y * (Real.exp y * Real.sqrt (2 *
    y - 1))) (deriv f x * (Real.exp x * Real.sqrt (2 * x - 1)) + f x *
    (Real.exp x * Real.sqrt (2 * x - 1) + Real.exp x / Real.sqrt (2 * x
    - 1))) x := by
          convert h1.mul h1 using 1
          exact h2
          have h2 : deriv (fun y => f y * (Real.exp y * Real.sqrt (2 * y -
    1))) x = deriv f x * (Real.exp x * Real.sqrt (2 * x - 1)) + f x *
    (Real.exp x * Real.sqrt (2 * x - 1) + Real.exp x / Real.sqrt (2 * x
    - 1)) := by
            apply HasDerivAt.deriv
            exact h2
            have h2 : deriv f x * (Real.exp x * Real.sqrt (2 * x - 1)) + f x *
    (Real.exp x * Real.sqrt (2 * x - 1) + Real.exp x / Real.sqrt (2 * x
    - 1)) = (deriv f x) * (deriv (fun y => Real.exp y * Real.sqrt (2 * y
    - 1)) x) := by
              have h2 : deriv f x = 2 * x * Real.exp (x ^ 2) := h2
              have h2 : f x = Real.exp (x ^ 2) := by
                rw [h2]
              have h2 : deriv (fun y => Real.exp y * Real.sqrt (2 * y - 1)) x =
    Real.exp x * Real.sqrt (2 * x - 1) + Real.exp x / Real.sqrt (2 * x
    - 1) := h2
              have h2 : 2 * x * (Real.exp x * Real.sqrt (2 * x - 1)) +
    (Real.exp x * Real.sqrt (2 * x - 1) + Real.exp x / Real.sqrt (2 * x
    - 1)) = 2 * x * (Real.exp x * Real.sqrt (2 * x - 1) + Real.exp x /
    Real.sqrt (2 * x - 1)) := by
                have h2 : Real.exp x > 0 := Real.exp_pos x
                have h2 : Real.sqrt (2 * x - 1) > 0 := Real.sqrt_pos.mpr (by
    linarith)
                field_simp [h2.ne', h2.ne']
                <|> nlinarith [Real.exp_sqrt (show 0 ≤ 2 * x - 1 by linarith)]
              calc
                deriv f x * (Real.exp x * Real.sqrt (2 * x - 1)) + f x *
    (Real.exp x * Real.sqrt (2 * x - 1) + Real.exp x / Real.sqrt (2 * x
    - 1)) = (2 * x * Real.exp (x ^ 2)) + (Real.exp x * Real.sqrt (2 * x
    - 1) + Real.exp x / Real.sqrt (2 * x - 1)) * (Real.exp x * Real.sqrt (2 * x
    - 1)) := by
                  rw [h2, h2]
                  _ = Real.exp (x ^ 2) * (2 * x * (Real.exp x * Real.sqrt (2 * x
    - 1)) + (Real.exp x * Real.sqrt (2 * x - 1) + Real.exp x / Real.sqrt
    (2 * x - 1))) := by
                    ring_nf
                    _ = Real.exp (x ^ 2) * (2 * x * (Real.exp x * Real.sqrt (2 * x
    - 1) + Real.exp x / Real.sqrt (2 * x - 1))) := by
                      rw [h2]
                      _ = (2 * x * Real.exp (x ^ 2)) * (Real.exp x * Real.sqrt (2 *
    x - 1) + Real.exp x / Real.sqrt (2 * x - 1)) := by
                        ring_nf
                        _ = (deriv f x) * (deriv (fun y => Real.exp y * Real.sqrt (2 *
    y - 1)) x) := by
                          rw [h2, h2]
                          rw [h2]
                          rw [h2]
                          exact h2
            . intro h
            . trivial
            . intro h
            . exact h_main
    -----
    -- Orig Proof
    import Mathlib
    import Aesop

    set_option maxHeartbeats 0

    open Set Filter Topology

    theorem putnam_1988_b1
    : ∀ a ≥ 2, ∀ b ≥ 2, ∃ x y z : ℤ, x > 0 ∧ y > 0 ∧ z > 0 ∧ a * b = x * y + x * z +
    y * z + 1 := by
      intro a b h2
      have h_main : ∃ (x y z : ℤ), x > 0 ∧ y > 0 ∧ z > 0 ∧ a * b = x * y + x * z +
    y * z + 1 := by
        use a - 1, b - 1, 1
        have h1 : a - 1 > 0 := by
          linarith
        have h1 : (a - 1) ≥ 2 := by exact_mod_cast h1
        have h1 : b - 1 > 0 := by
          linarith
        have h1 : (b - 1) ≥ 2 := by exact_mod_cast h1
        have h1 : (1 : ℤ) > 0 := by norm_num
        have h1 : a * b = (a - 1) * (b - 1) + (a - 1) * 1 + (b - 1) * 1 + 1 := by
          ring_nf
          <|>
            (try norm_num) <|>
            (try linarith) <|>
            (try nlinarith)
          exact [h1, h1, h1, by linarith]
      exact h_main
    -----
    -- Simplified Proof
    import Mathlib
    import Aesop

    set_option maxHeartbeats 0

    open Set Filter Topology

    theorem putnam_1988_b1
    : ∀ a ≥ 2, ∀ b ≥ 2, ∃ x y z : ℤ, x > 0 ∧ y > 0 ∧ z > 0 ∧ a * b = x * y + x * z +
    y * z + 1 := by
      rintro a b h2
      use a - 1, b - 1, 1
      constructor
      linarith
      constructor
      linarith
      constructor
      constructor
      norm_num
      ring
    -----

```

```

-- Orig Proof
import Mathlib
import Aesop

set_option maxHeartbeats 0

open Set Filter Topology

theorem putnam_1988_b2
: (∀ x y : ℝ, (y ≥ 0 ∧ y * (y + 1) ≤ (x + 1) ^ 2) → (y * (y - 1) ≤ x ^ 2)) ↔
  ↔ ((True) : Prop) := by
  have h_main : (∀ x y : ℝ, (y ≥ 0 ∧ y * (y + 1) ≤ (x + 1) ^ 2) → (y * (y - 1) ≤
    x ^ 2)) := by
    intro x y h
    have h1 : y ≥ 0 := h.1
    have h2 : y * (y + 1) ≤ (x + 1) ^ 2 := h.2
    nlinarith [sq_nonneg (x + 1 - y), sq_nonneg (x - y), sq_nonneg (2 * x + 1
    - y),
      sq_nonneg (y - 1), sq_nonneg (x + 1 + y)]
  have h_final : (∀ x y : ℝ, (y ≥ 0 ∧ y * (y + 1) ≤ (x + 1) ^ 2) → (y * (y - 1)
    ≤ x ^ 2)) ↔ ((True) : Prop) := by
    constructor
    . intro h
    . trivial
    . intro h
    . exact h_main
  exact h_final
  -----
  -- Simplified Proof
  import Mathlib
  import Aesop

  set_option maxHeartbeats 0

  open Set Filter Topology

  theorem putnam_1988_b2
  : (∀ x y : ℝ, (y ≥ 0 ∧ y * (y + 1) ≤ (x + 1) ^ 2) → (y * (y - 1) ≤ x ^ 2)) ↔
    ↔ ((True) : Prop) := by
    constructor
    intro h
    trivial
    intro
    intro x y hxy
    nlinarith [sq_nonneg (x - y)]
    -----
    -- Orig Proof
    import Mathlib
    import Aesop

    set_option maxHeartbeats 0

    open Filter Topology Nat

    theorem putnam_1990_a1
    (T : ℕ → ℤ)
    (hT012 : T 0 = 2 ∧ T 1 = 3 ∧ T 2 = 6)
    (hTn : ∀ n, T (n + 3) = (n + 7) * T (n + 2) - 4 * (n + 3) * T (n + 1) + (4 *
    T (n + 4) * T n) :
    T = ((fun n : ℕ => (n)!, fun n : ℕ => 2 ^ n) : (ℕ → ℤ) × (ℕ → ℤ)).1 +
    ((fun n : ℕ => (n)!, fun n : ℕ => 2 ^ n) : (ℕ → ℤ) × (ℕ → ℤ)).2 :=
  by
    have h_main : ∀ (n : ℕ), T n = (n ! : ℤ) + 2 ^ n := by
      intro n
      have h1 : T n = (n ! : ℤ) + 2 ^ n := by
        have h2 : ∀ n : ℕ, T n = (n ! : ℤ) + 2 ^ n := by
          intro n
          induction n using Nat.strong_induction_on with
          | h n ih =>
            match with
            | 0 =>
              norm_num [hT012]
              <|>
              simp_all [Nat.factorial]
              <|>
              norm_num
            | 1 =>
              norm_num [hT012]
              <|>
              simp_all [Nat.factorial]
              <|>
              norm_num
            | 2 =>
              norm_num [hT012]
              <|>
              simp_all [Nat.factorial]
              <|>
              norm_num
            | n + 3 =>
              have h1 := hTn n
              have h1 := ih n (by omega)
              have h1 := ih (n + 1) (by omega)
              have h1 := ih (n + 2) (by omega)
              simp [h1, h1, pow_add, pow_one, Nat.factorial_succ,
    → Nat.mul_add, Nat.add_mul] at h1
              <|>
              ring_nf at h1 <|>
              norm_cast at h1 <|>
              simp_all [Nat.factorial_succ, pow_add, pow_one, mul_assoc]
              <|>
              ring_nf at * <|>
              norm_num at * <|>
              nlinarith
            exact h1 n
            exact h1
          have h_final : T = ((fun n : ℕ => (n)!, fun n : ℕ => 2 ^ n) : (ℕ → ℤ) × (ℕ →
    ℤ)).1 + ((fun n : ℕ => (n)!, fun n : ℕ => 2 ^ n) : (ℕ → ℤ) × (ℕ → ℤ)).2 := by
            funext n
            have h1 : T n = (n ! : ℤ) + 2 ^ n := h_main n
            simp [h1, F1.add_apply]

```



```

<|>
norm_cast
<|>
simp [Nat.cast_add]
<|>
ring_nf

apply h_final

-- Simplified Proof
import Mathlib
import Aesop

set_option maxHeartbeats 0

open Filter Topology Nat

theorem putnam_1990_a1
  (T : ℕ → ℤ)
  (hT012 : T 0 = 2 ∧ T 1 = 3 ∧ T 2 = 6)
  (hTn : ∀ n, T (n + 3) = (n + 7) * T (n + 2) - 4 * (n + 3) * T (n + 1) + (4 *
    → n + 4) * T n) :
  T = ((fun n : ℕ => (n)! , fun n : ℕ => 2 ^ n) : (ℕ → ℤ) × (ℕ → ℤ)).1 +
    → ((fun n : ℕ => (n)! , fun n : ℕ => 2 ^ n) : (ℕ → ℤ) × (ℕ → ℤ)).2 := by
  ext n
  induction' n using Nat.strong_induction_on with n ih
  match n with
  | 0 => simp_all
  | 1 => simp_all
  | 2 => simp_all
  | n + 3 =>
    simp_all [Nat.factorial_succ]
    ring_nf
  -----
  -- Orig Proof
  import Mathlib
  import Aesop

  set_option maxHeartbeats 0

  open Filter Topology Nat

  theorem putnam_1990_a5 :
    ((False) : Prop) ↔
    (∀ n ≥ 1, ∀ A B : Matrix (Fin n) (Fin n) ℝ,
      A * B * A * B = 0 → B * A * B * A = 0) := by
  have h_main : (∀ n ≥ 1, ∀ A B : Matrix (Fin n) (Fin n) ℝ, A * B * A * B = 0 →
    → B * A * B * A = 0) → False := by
  intro h
  let A : Matrix (Fin 4) (Fin 4) ℝ := !![0, 0, 1, 0; 0, 0, 0, 1; 0, 0, 0, 0;
    → 0, 0, 0, 0]
  let B : Matrix (Fin 4) (Fin 4) ℝ := !![1, 0, 0, 0; 0, 0, 0, 0; 0, 1, 0, 0;
    → 0, 0, 0, 0]
  have h₁ : A * B * A * B = 0 := by
  ext i j
  fin_cases i <|> fin_cases j <|>
  simp [Matrix.mul_apply, Fin.sum_univ_four, A, B]
  <|> norm_num <|> rfl
  have h₂ : B * A * B * A ≠ 0 := by
  intro h₂
  have h₃ := congr_arg (fun m : Matrix (Fin 4) (Fin 4) ℝ => m 0 3) h₂
  simp [Matrix.mul_apply, Fin.sum_univ_four, A, B] at h₃
  <|> norm_num at h₃ <|>
  (try contradiction) <|>
  (try linarith)
  have h₄ : B * A * B * A = 0 := h 4 (by norm_num) A B h₁
  exact h₄ h₃
  have h_final : ((False) : Prop) ↔ (∀ n ≥ 1, ∀ A B : Matrix (Fin n) (Fin n) ℝ
    → , A * B * A * B = 0 → B * A * B * A = 0) := by
  constructor
  · intro h
    exfalse
    exact h
  · intro h
    exact h_main h
  exact h_final
  -- Simplified Proof
  import Mathlib
  import Aesop

  set_option maxHeartbeats 0

  open Filter Topology Nat

  theorem putnam_1990_a5 :
    ((False) : Prop) ↔
    (∀ n ≥ 1, ∀ A B : Matrix (Fin n) (Fin n) ℝ,
      A * B * A * B = 0 → B * A * B * A = 0) := by
  constructor
  · simp
  · intro h
    have h₁ := h 4 (by norm_num)
    (!! [0, 0, 1, 0; 0, 0, 0, 1; 0, 0, 0, 0; 0, 0, 0, 0])
    (!! [1, 0, 0, 0; 0, 0, 0, 0; 0, 1, 0, 0; 0, 0, 0, 0])
    (by ext i j <|> fin_cases i <|> fin_cases j <|> simp [Matrix.mul_apply,
      → Fin.sum_univ_four])
    simpa [Matrix.mul_apply, Fin.sum_univ_four] using congr_fun (congr_fun h₁
      → 0) 3
  -----
  -- Orig Proof
  import Mathlib
  import Aesop

  set_option maxHeartbeats 0

  open Filter Topology Nat

```

```

theorem putnam_1990_a6 :
  ((Finset.univ : Finset <| Finset (Set.Icc 1 10) × Finset (Set.Icc 1
    → 10)).filter
    → 10)).filter
  (fun S, T => (∀ s ∈ S, T.card < s) ∧ (∀ t ∈ T, S.card < t)).card =
  ((17711) : ℕ) :=
  by
  native_decide

  -- Simplified Proof
  import Mathlib
  import Aesop

  set_option maxHeartbeats 0

  open Filter Topology Nat

  theorem putnam_1990_a6 :
    ((Finset.univ : Finset <| Finset (Set.Icc 1 10) × Finset (Set.Icc 1
      → 10)).filter
      → 10)).filter
    (fun S, T => (∀ s ∈ S, T.card < s) ∧ (∀ t ∈ T, S.card < t)).card =
    ((17711) : ℕ) := by
  native_decide
  -----
  -- Orig Proof
  import Mathlib
  import Aesop

  set_option maxHeartbeats 0

  open Filter Topology

  theorem putnam_1991_a2
    (n : ℕ) (hn : 1 ≤ n) :
    ((False) : Prop) ↔ (∃ A B : Matrix (Fin n) (Fin n) ℝ,
      A ≠ B ∧ A ^ 3 = B ^ 3 ∧
      A ^ 2 * B = B ^ 2 * A ∧
      Nonempty (Invertible (A ^ 2 + B ^ 2))) := by
  have h_imp : (∃ A B : Matrix (Fin n) (Fin n) ℝ, A ≠ B ∧ A ^ 3 = B ^ 3 ∧ A ^ 2
    → * B = B ^ 2 * A ∧ Nonempty (Invertible (A ^ 2 + B ^ 2))) → False :=
    → by
  intro h
  rcases h with (A, B, hne, hA3B3, hA2B_B2A, hinv)
  have h1 : (A ^ 2 + B ^ 2) * (A - B) = 0 := by
  calc
    (A ^ 2 + B ^ 2) * (A - B) = A ^ 2 * A + B ^ 2 * A - A ^ 2 * B - B ^ 2 *
      → B := by
    simp [Matrix.mul_add, Matrix.add_mul, Matrix.mul_sub, Matrix.sub_mul]
    <|>
    abel
    = A ^ 3 + B ^ 2 * A - A ^ 2 * B - B ^ 3 := by
    simp [pow_succ, Matrix.mul_assoc]
    <|>
    ring_nf
    <|>
    simp_all [Matrix.mul_assoc]
    <|>
    abel
    = A ^ 3 + B ^ 2 * A - A ^ 2 * B - A ^ 3 := by
    rw [hA3B3]
    = B ^ 2 * A - A ^ 2 * B := by
    abel
    = 0 := by
    rw [hA2B_B2A]
    <|>
    simp [sub_self]
  have h2 : A - B = 0 := by
  rcases hinv with (C, hC_left, hC_right)
  have h3 : C * (A ^ 2 + B ^ 2) * (A - B) = 1 := by
  simpa [Matrix.mul_assoc] using hC_left
  have h4 : (A ^ 2 + B ^ 2) * (A - B) = 0 := h1
  calc
    A - B = 1 * (A - B) := by simp
    = C * (A ^ 2 + B ^ 2) * (A - B) := by rw [h3]
    = C * (A ^ 2 + B ^ 2) * (A - B) := by simp [Matrix.mul_assoc]
    = C * 0 := by rw [h4]
    = 0 := by simp
  have h3 : A = B := by
  have h4 : A - B = 0 := h2
  have h5 : A = B := by
  apply eq_of_sub_eq_zero
  simpa using h4
  exact h5
  exact hne h3
  have h_conv : False → (∃ A B : Matrix (Fin n) (Fin n) ℝ, A ≠ B ∧ A ^ 3 = B ^
    → 3 ∧ A ^ 2 * B = B ^ 2 * A ∧ Nonempty (Invertible (A ^ 2 + B ^ 2))) :=
    → by
  intro h
  exfalse
  exact h
  have h_main : ((False) : Prop) ↔ (∃ A B : Matrix (Fin n) (Fin n) ℝ, A ≠ B ∧
    → A ^ 3 = B ^ 3 ∧ A ^ 2 * B = B ^ 2 * A ∧ Nonempty (Invertible (A ^ 2 +
      → B ^ 2))) := by
  constructor
  · intro h
    exact h_conv h
  · intro h
    exact h_imp h
  exact h_main
  -- Simplified Proof
  import Mathlib
  import Aesop

  set_option maxHeartbeats 0

  open Filter Topology

  theorem putnam_1991_a2
    (n : ℕ) (hn : 1 ≤ n) :

```

```

((False) : Prop) ↔ (∃ A B : Matrix (Fin n) (Fin n) ℝ,
  A ≠ B ∧ A ^ 3 = B ^ 3 ∧
  A ^ 2 * B = B ^ 2 * A ∧
  Nonempty (Invertible (A ^ 2 + B ^ 2))) := by
  constructor
  · simp
  · rintro A, B, hne, hA3B3, hA2B_B2A, hinv
    have h0 : A - B = 0 := by
      obtain C, hC_left, hC_right := hinv
      have h3 : C * (A ^ 2 + B ^ 2) = 1 := hC_left
      have h4 : (A ^ 2 + B ^ 2) * (A - B) = 0 := by
        calc
          (A ^ 2 + B ^ 2) * (A - B) = A ^ 2 * A + B ^ 2 * A - A ^ 2 * B - B ^ 2 * B
          → 2 * B := by
            simp [Matrix.mul_add, Matrix.add_mul, Matrix.mul_sub,
              Matrix.sub_mul]
            <|> abel
            _ = 0 := by simp_all [pow_succ, Matrix.mul_assoc]
        calc
          A - B = 1 * (A - B) := by simp
          _ = C * (A ^ 2 + B ^ 2) * (A - B) := by rw [h3]
          _ = C * ((A ^ 2 + B ^ 2) * (A - B)) := by simp [Matrix.mul_assoc]
          _ = C * 0 := by rw [h4]
          _ = 0 := by simp
      simp_all [sub_eq_zero]
    -----
    -- Orig Proof
    import Mathlib
    import Aesop

    set_option maxHeartbeats 0

    open Filter Topology

    theorem putnam_1991_b1
    (m S : ℤ → ℤ)
    (A : ℤ)
    (a : ℕ → ℤ)
    (hm : ∀ n, 0 ≤ n → (m n) ^ 2 ≤ n ∧ (∀ m' : ℤ, m' ^ 2 ≤ n → m' ≤ m n))
    (hS : ∀ n, 0 ≤ n → S n = n - (m n) ^ 2)
    (ha : a 0 = A ∧ (∀ k, a (k + 1) = a k + S (a k)))
    (hA : A > 0) :
    (∃ (K : ℕ) (c : ℕ), ∀ k ≥ K, a k = c) ↔ A ∈ ({A : ℤ | ∃ x > 0, A = x ^ 2}) :
    → Set ℤ := by
    have h_nonneg : ∀ (k : ℕ), a k ≥ 0 := by
      intro k
      induction k with
      | zero =>
        have h₁ : a 0 = A := ha.1
        linarith
      | succ k ih =>
        have h₁ : a (k + 1) = a k + S (a k) := ha.2 k
        rw [h₁]
        have h₂ : 0 ≤ a k := ih
        have h₃ : S (a k) = a k - (m (a k)) ^ 2 := hS (a k) h₂
        have h₄ : (m (a k)) ^ 2 ≤ a k := (hm (a k) h₂).1
        have h₅ : S (a k) ≥ 0 := by
          rw [h₃]
          linarith
        linarith
    have h_nondec : ∀ k, a (k + 1) ≥ a k := by
      intro k
      have h₁ : a (k + 1) = a k + S (a k) := (ha.2) k
      rw [h₁]
      have h₂ : 0 ≤ a k := h_nonneg k
      have h₃ : S (a k) = a k - (m (a k)) ^ 2 := hS (a k) h₂
      have h₄ : (m (a k)) ^ 2 ≤ a k := (hm (a k) h₂).1
      have h₅ : S (a k) ≥ 0 := by
        rw [h₃]
        linarith
      linarith
    have h_S_pos : ∀ (n : ℤ), 0 ≤ n → (∀ (t : ℤ), n ≠ t ^ 2 → S n ≥ 1) := by
      intro n hn hnotsquare
      have h₁ : S n = n - (m n) ^ 2 := hS n hn
      rw [h₁]
      have h₂ : (m n) ^ 2 ≤ n := (hm n hn).1
      have h₃ : ∀ (m' : ℤ), m' ^ 2 ≤ n → m' ≤ m n := (hm n hn).2
      have h₄ : n - (m n) ^ 2 ≥ 1 := by
        by_contra h
        have h₅ : n - (m n) ^ 2 ≤ 0 := by
          linarith
        have h₆ : (m n + 1 : ℤ) ^ 2 > n := by
          by_contra h₆
          have h₇ : (m n + 1 : ℤ) ^ 2 ≤ n := by linarith
          have h₈ : m n + 1 ≤ m n := h₇ (m n + 1) h₆
          linarith
        have h₉ : (m n : ℤ) ^ 2 ≤ n := h₂
        have h₁₀ : (m n + 1 : ℤ) ^ 2 > n := h₆
        have h₁₁ : (m n + 1 : ℤ) ^ 2 > n := h₁₀
      have h₁₂ : (m n : ℤ) ^ 2 = n := by
        linarith
      have h₁₃ : ∃ (t : ℤ), n = t ^ 2 := by
        refine' ⟨m n, _⟩
        linarith
      obtain (t, ht) := h₁₃
      have h₁₄ : n = t ^ 2 := ht
      have h₁₅ : n ≠ t ^ 2 := hnotsquare t
      contradiction
    linarith
    have h_no_new_squares : ∀ (k : ℕ), (∀ (t : ℤ), a k ≠ t ^ 2) → (∀ (t : ℤ), a
      → (k + 1) ≠ t ^ 2) := by

```

```

  intro k hk
  intro t ht
  have h₁ : a (k + 1) = a k + S (a k) := ha.2 k
  have h₂ : 0 ≤ a k := h_nonneg k
  have h₃ : S (a k) = a k - (m (a k)) ^ 2 := hS (a k) h₂
  have h₄ : a (k + 1) = a k + (a k - (m (a k)) ^ 2) := by
    rw [h₁, h₃]
    <|> ring
  have h₅ : a (k + 1) = 2 * a k - (m (a k)) ^ 2 := by
    linarith
  have h₆ : a (k + 1) = t ^ 2 := ht
  have h₇ : 2 * a k - (m (a k)) ^ 2 = t ^ 2 := by linarith
  have h₈ : (m (a k)) ^ 2 ≤ a k := (hm (a k) h₂).1
  have h₉ : ∀ (m' : ℤ), m' ^ 2 ≤ a k → m' ≤ m (a k) := (hm (a k) h₂).2
  have h₁₀ : a k < (m (a k) + 1) ^ 2 := by
    by_contra h
    have h₁₁ : (m (a k) + 1 : ℤ) ^ 2 ≤ a k := by linarith
    have h₁₂ : m (a k) + 1 ≤ m (a k) := h₁₁ (m (a k) + 1) h₁₁
    linarith
  have h₁₃ : m (a k) ≥ 0 := by
    by_contra h
    have h₁₄ : m (a k) < 0 := by linarith
    have h₁₅ : (m (a k)) ^ 2 > 0 := by nlinarith
    have h₁₆ : (m (a k) + 1 : ℤ) ^ 2 ≤ a k := by
      nlinarith [h₁₄]
    have h₁₇ : m (a k) + 1 ≤ m (a k) := h₁₆ (m (a k) + 1) h₁₆
    linarith
  have h₁₈ : t ^ 2 = 2 * a k - (m (a k)) ^ 2 := by linarith
  have h₁₉ : (m (a k)) ^ 2 < t ^ 2 := by
    have h₂₀ : (m (a k)) ^ 2 < a k := by
      by_contra h₂₀
      have h₂₁ : (m (a k)) ^ 2 ≥ a k := by linarith
      have h₂₂ : (m (a k)) ^ 2 ≤ a k := h₂₁
      have h₂₃ : a k = t ^ 2 := by
        refine' ⟨m (a k), _⟩
        linarith
      obtain (t', ht') := h₂₃
      have h₂₄ : a k = t' ^ 2 := ht'
      have h₂₅ : a k ≠ t' ^ 2 := hk t'
      contradiction
    nlinarith
  have h₂₀ : t ^ 2 < (m (a k) + 2) ^ 2 := by
    nlinarith [h₁₉]
  have h₂₁ : t = m (a k) + 1 ∨ t = -(m (a k) + 1) := by
    have h₂₂ : m (a k) ≥ 0 := h₂₁
    have h₂₃ : t ^ 2 < (m (a k) + 2) ^ 2 := h₂₀
    have h₂₄ : (m (a k)) ^ 2 < t ^ 2 := h₁₉
    have h₂₅ : t ≤ m (a k) + 1 := by
      nlinarith
    have h₂₆ : t ≥ -(m (a k) + 1) := by
      nlinarith
    have h₂₇ : t ≥ m (a k) + 1 ∨ t ≤ -(m (a k) + 1) := by
      by_contra! h₂₇
      have h₂₈ : -(m (a k) + 1) < t := by linarith
      have h₂₉ : t < m (a k) + 1 := by linarith
      have h₃₀ : t ^ 2 < (m (a k) + 1) ^ 2 := by
        nlinarith
      nlinarith
    cases h₂₇ with
    | inl h₂₇ =>
      have h₃₁ : t = m (a k) + 1 := by
        nlinarith
      exact Or.inl h₃₁
    | inr h₂₇ =>
      have h₃₂ : t = -(m (a k) + 1) := by
        nlinarith
      exact Or.inr h₃₂
  cases h₃ with
  | inl h₃ =>
    have h₃₃ : t = m (a k) + 1 := h₃₃
    have h₃₄ : t ^ 2 = (m (a k) + 1) ^ 2 := by
      rw [h₃₃]
      <|> ring_nf
    have h₃₅ : 2 * a k - (m (a k)) ^ 2 = (m (a k) + 1) ^ 2 := by
      linarith
    have h₃₆ : 2 * a k = 2 * (m (a k)) ^ 2 + 2 * m (a k) + 1 := by
      nlinarith
    have h₃₇ : (2 : ℤ) * a k % 2 = 1 := by
      have h₃₈ : (2 : ℤ) * a k = 2 * (m (a k)) ^ 2 + 2 * m (a k) + 1 := h₃₆
      omega
    have h₃₉ : (2 : ℤ) * a k % 2 = 0 := by
      have h₄₀ : (2 : ℤ) * a k % 2 = 0 := by
        have h₄₁ : (2 : ℤ) * a k % 2 = 0 := by
          omega
          exact h₃₇
        exact h₃₈
      omega
    exact h₃₉
  | inr h₃ =>
    have h₄₁ : t = -(m (a k) + 1) := h₄₁
    have h₄₂ : t ^ 2 = (m (a k) + 1) ^ 2 := by
      rw [h₄₁]
      <|> ring_nf
      <|> simp [sq]
      <|> linarith
    have h₄₃ : 2 * a k - (m (a k)) ^ 2 = (m (a k) + 1) ^ 2 := by
      linarith
    have h₄₄ : 2 * a k = 2 * (m (a k)) ^ 2 + 2 * m (a k) + 1 := by
      nlinarith
    have h₄₅ : (2 : ℤ) * a k % 2 = 1 := by
      have h₄₆ : (2 : ℤ) * a k = 2 * (m (a k)) ^ 2 + 2 * m (a k) + 1 := h₄₄
      omega
    have h₄₇ : (2 : ℤ) * a k % 2 = 0 := by
      have h₄₈ : (2 : ℤ) * a k % 2 = 0 := by
        have h₄₉ : (2 : ℤ) * a k % 2 = 0 := by
          omega
          exact h₄₅
        exact h₄₆
      omega
    exact h₄₇

```



```

nlinarith
have h11 : t = t, n = t ^ 2 := by
  refine' m n, _
nlinarith
obtain (t, ht) := h11
have h12 : n = t ^ 2 := ht
have h13 : n ≠ t ^ 2 := hnotsquare t
contradiction
nlinarith
have hno_new_squares : ∀ k, (∀ t, a k ≠ t ^ 2) → (∀ t, a (k + 1) ≠ t ^ 2) :=
  by
    intro k hk
    intro t ht
    have h1 : a (k + 1) = a k + S (a k) := ha.2 k
    have h2 : 0 ≤ a k := hnonneg k
    have h3 : S (a k) = a k - (m (a k)) ^ 2 := hS (a k) h2
    have h4 : a (k + 1) = a k + (a k - (m (a k)) ^ 2) := by
      rw [h1, h3]
    have h5 : a (k + 1) = 2 * a k - (m (a k)) ^ 2 := by linarith
    have h6 : a (k + 1) = t ^ 2 := ht
    have h7 : 2 * a k - (m (a k)) ^ 2 = t ^ 2 := by linarith
    have h8 : (m (a k)) ^ 2 ≤ a k := (hm (a k) h2).1
    have h9 : m' ^ 2 ≤ a k - m' ^ 2 ≤ m (a k) := (hm (a k) h2).2
    have h10 : a k < m (a k + 1) ^ 2 := by
      by_contra h
      have h11 : (m (a k) + 1 : z) ^ 2 ≤ a k := by linarith
      have h12 : m (a k) + 1 ≤ m (a k) := h11 (m (a k) + 1) h1
      linarith
    have h13 : m (a k) ≥ 0 := by
      by_contra h
      have h14 : m (a k) < 0 := by linarith
      have h15 : (m (a k)) ^ 2 > 0 := by nlinarith
      have h16 : (m (a k) + 1 : z) ^ 2 ≤ a k := by
        nlinarith [h15]
      have h17 : m (a k) + 1 ≤ m (a k) := h16 (m (a k) + 1) h1
      linarith
    have h18 : t ^ 2 = 2 * a k - (m (a k)) ^ 2 := by linarith
    have h19 : (m (a k)) ^ 2 < t ^ 2 := by
      have h20 : (m (a k)) ^ 2 < a k := by
        by_contra h21
        have h22 : (m (a k)) ^ 2 ≥ a k := by linarith
        have h23 : (m (a k)) ^ 2 ≤ a k := h2
        have h24 : (m (a k)) ^ 2 = a k := by linarith
        refine' m (a k), _
        linarith
        obtain (t', ht') := h24
        have h25 : a k = t' ^ 2 := ht'
        have h26 : a k ≠ t' ^ 2 := hk t'
        contradiction
      nlinarith
    have h27 : t = m (a k) + 1 ∨ t = -(m (a k) + 1) := by
      have h28 : m (a k) ≥ 0 := h2
      have h29 : t ^ 2 < (m (a k) + 2) ^ 2 := by
        nlinarith [h28]
      have h30 : (m (a k)) ^ 2 < t ^ 2 := h18
      have h31 : t ≤ m (a k) + 1 := by
        nlinarith
      have h32 : t ≥ -(m (a k) + 1) := by
        nlinarith
      have h33 : t ≥ m (a k) + 1 ∨ t ≤ -(m (a k) + 1) := by
        by_contra! h34
        have h35 : -(m (a k) + 1) < t := by linarith
        have h36 : t < m (a k) + 1 := by linarith
        have h37 : t ^ 2 < (m (a k) + 1) ^ 2 := by
          nlinarith
        cases h38 with
        | inl h39 =>
          have h40 : t = m (a k) + 1 := by
            nlinarith
          exact Or.inl h39
        | inr h41 =>
          have h42 : t = -(m (a k) + 1) := by
            nlinarith
          exact Or.inr h41
      cases h34 with
      | inl h43 =>
        have h44 : t = m (a k) + 1 := h40
        have h45 : t ^ 2 = (m (a k) + 1) ^ 2 := by
          rw [h44]
        have h46 : 2 * a k - (m (a k)) ^ 2 = (m (a k) + 1) ^ 2 := by
          linarith
        have h47 : 2 * a k = 2 * (m (a k)) ^ 2 + 2 * m (a k) + 1 := by
          nlinarith
        have h48 : (2 : z) * a k % 2 = 1 := by
          have h49 : (2 : z) * a k = 2 * (m (a k)) ^ 2 + 2 * m (a k) + 1 := h47
          omega
        have h50 : (2 : z) * a k % 2 = 0 := by
          have h51 : (2 : z) * a k % 2 = 0 := by
            omega
          exact h51
        omega
      | inr h43 =>
        have h52 : t = -(m (a k) + 1) := h42
        have h53 : t ^ 2 = (m (a k) + 1) ^ 2 := by
          rw [h52]
        <|> ring_nf
        have h54 : 2 * a k - (m (a k)) ^ 2 = (m (a k) + 1) ^ 2 := by
          linarith
        have h55 : 2 * a k = 2 * (m (a k)) ^ 2 + 2 * m (a k) + 1 := by
          nlinarith
        have h56 : (2 : z) * a k % 2 = 1 := by
          have h57 : (2 : z) * a k = 2 * (m (a k)) ^ 2 + 2 * m (a k) + 1 := h55
          omega
        have h58 : (2 : z) * a k % 2 = 0 := by
          have h59 : (2 : z) * a k % 2 = 0 := by
            omega
          exact h59
        omega
    have hstrict_increasing : (∀ t, A ≠ t ^ 2) → ∀ k, a (k + 1) > a k := by
      intro hnot_square k
      have h1 : ∀ k, (∀ t, a k ≠ t ^ 2) := by
        intro k
        induction' k with k ih
        intro t ht
        have h2 : a 0 = A := ha.1
        rw [h2] at ht
        exact hnot_square t ht
        intro t ht
        have h3 : ∀ t, a k ≠ t ^ 2 := ih
        have h4 : ∀ t, a (k + 1) ≠ t ^ 2 := hno_new_squares k h3
        exact h4 t ht
        have h5 : ∀ t, a k ≠ t ^ 2 := h3 k
        have h6 : 0 ≤ a k := hnonneg k
        have h7 : S (a k) ≥ 1 := hS_pos (a k) h6
        have h8 : a (k + 1) = a k + S (a k) := ha.2 k
        linarith
      constructor
      intro h
      by_contra h1
      have h2 : ∀ t, A ≠ t ^ 2 := by
        intro t ht
        have h3 : A ∈ ({A : z | ∃ x > 0, A = x ^ 2} : Set z) := by
          refine' (t.natAbs, _)
        have h4 : A = t ^ 2 := ht
        have h5 : (t.natAbs : z) > 0 := by
          have h6 : t ≠ 0 := by
            by_contra h7
            rw [h7] at h4
            have h8 : A = 0 := by
              norm_num at h4
            <|> linarith
          linarith
        have h9 : t.natAbs > 0 := by
          exact Nat.pos_of_ne_zero (by
            intro h10
            have h11 : t = 0 := by
              simp [Int.natAbs_eq_zero] at h10
            <|> omega
            contradiction
          )
        exact_mod_cast h9
        have h12 : A = (t.natAbs : z) ^ 2 := by
          have h13 : A = t ^ 2 := ht
          have h14 : (t.natAbs : z) ^ 2 = t ^ 2 := by
            simp [sq, Int.natAbs_mul]
          linarith
          exact (by exact_mod_cast h9, by linarith)
        contradiction
        have h15 : ∀ k, a (k + 1) > a k := hstrict_increasing h1
        obtain (K, c, h16) := h
        have h17 : a (K + 1) > a K := h15 K
        have h18 : a (K + 1) = c := by
          have h19 : K + 1 ≥ K := by linarith
          have h20 : a (K + 1) = c := h16 (K + 1) h1
          exact h20
        have h21 : a K = c := by
          have h22 : K ≥ K := by linarith
          have h23 : a K = c := h16 K h1
          exact h23
        linarith
      intro h
      obtain (x, hx, hx') := h
      have h1 : a 0 = A := ha.1
      have h2 : ∀ k, a (k + 1) = a k + S (a k) := ha.2
      have h3 : ∀ k, a k = A := by
        intro k
        induction' k with k ih
        simp [h1]
        have h4 : a (K + 1) = a k + S (a k) := h2 k
        rw [h4]
        have h5 : a k = A := ih
        rw [h5]
        have h6 : S A = 0 := by
          have h7 : 0 ≤ A := by linarith
          have h8 : S A = A - (m A) ^ 2 := hS A h7
          rw [h8]
          have h9 : (m A) ^ 2 ≤ A := (hm A h7).1
          have h10 : ∀ m', m' ^ 2 ≤ A → m' ^ 2 ≤ m A := (hm A h7).2
          have h11 : A = x ^ 2 := by
            norm_cast at hx'
            <|> linarith
          have h12 : (m A : z) = x := by
            have h13 : (m A : z) ≥ 0 := by
              by_contra h14
              have h15 : (m A : z) < 0 := by linarith
              have h16 : (m A : z) ^ 2 > 0 := by nlinarith
              have h17 : (m A + 1 : z) ^ 2 ≤ A := by
                nlinarith [h16]
              have h18 : m A + 1 ≤ m A := h17 (m A + 1) h1
              linarith
            have h19 : (m A : z) ≤ x := by
              have h20 : (m A : z) ^ 2 ≤ A := h9
              have h21 : A = x ^ 2 := by
                norm_cast at hx'
                <|> linarith
              have h22 : (m A : z) ^ 2 ≤ x ^ 2 := by
                nlinarith
              linarith
            have h23 : (m A : z) ≥ x := by
              by_contra h24
              have h25 : (m A : z) < x := by linarith
              have h26 : (m A + 1 : z) ≤ x := by
                linarith
              have h27 : (m A + 1 : z) ^ 2 ≤ x ^ 2 := by
                have h28 : (m A + 1 : z) ≤ x := by linarith
                have h29 : 0 ≤ (m A + 1 : z) := by
                  nlinarith [h28]
                nlinarith
              have h30 : (m A + 1 : z) ^ 2 ≤ A := by
                have h31 : A = x ^ 2 := by
                  norm_cast at hx'
                  <|> linarith
                linarith
              have h32 : m A + 1 ≤ m A := h29 (m A + 1) h1
              linarith
            linarith
          have h33 : (m A : z) = x := h22

```

```

      have h22 : (m A : z) ^ 2 = x ^ 2 := by
        rw [h11]
      have h23 : A = x ^ 2 := by
        norm_cast at hx' ⊢
        <|> linarith
      linarith
    refine' (0, Int.toNat A, _)
    intro k hk
    have h1 : a k = A := h1 k
    have h2 : 0 ≤ A := by linarith
    have h3 : (A : z) = Int.toNat A := by
      rw [Int.toNat_of_nonneg h2]
    rw [h1]
    <|> norm_cast at h3 ⊢
  ...

```

```

-- Orig Proof
import Mathlib
import Aesop

set_option maxHeartbeats 0

open Filter Topology

theorem putnam_1991_b2
  (f g : ℝ → ℝ)
  (fgnconst : ¬ c, f = Function.const ℝ c ∨ g = Function.const ℝ c)
  (fgdiff : Differentiable ℝ f ∧ Differentiable ℝ g)
  (fadd : ∀ x y, f (x + y) = f x * f y - g x * g y)
  (gadd : ∀ x y, g (x + y) = f x * g y + g x * f y) :
  (deriv f 0 = 0) → (∀ x, (f x) ^ 2 + (g x) ^ 2 = 1) := by
  intro hf0
  have h_f'_formula : ∀ x, deriv f x = -g x * deriv g 0 := by
    intro x
    have h1 : deriv (fun y : ℝ => f (x + y)) 0 = deriv f x := by
      have h2 : deriv (fun y : ℝ => f (x + y)) 0 = deriv (fun y : ℝ => f (x +
        → y)) 0 := rfl
      have h3 : deriv (fun y : ℝ => f (x + y)) 0 = deriv f x := by
        have h4 : HasDerivAt (fun y : ℝ => f (x + y)) (deriv f (x + 0) * 1) 0
          := by
          have h5 : HasDerivAt (fun y : ℝ => x + y) 1 0 := by
            simp using (hasDerivAt_id (0 : ℝ)).const_add x
          have h6 : HasDerivAt f (deriv f (x + 0)) (x + 0) := by
            apply DifferentiableAt.hasDerivAt
            exact fgdiff.1.differentiableAt
          have h7 : HasDerivAt (fun y : ℝ => f (x + y)) (deriv f (x + 0) * 1)
            0 := by
            apply HasDerivAt.comp (0 : ℝ) h6 h5
            convert h7 using 1 <|> simp
          have h8 : deriv (fun y : ℝ => f (x + y)) 0 = deriv f (x + 0) * 1 := by
            apply HasDerivAt.deriv
            exact h4
          have h9 : deriv f (x + 0) * 1 = deriv f x := by
            simp
          rw [h8, h9]
          exact h3
        have h10 : deriv (fun y : ℝ => f (x + y)) 0 = -g x * deriv g 0 := by
          have h11 : (fun y : ℝ => f (x + y)) = (fun y : ℝ => f x * f y - g x * g
            → y) := by
            funext y
            rw [fadd x y]
            <|> ring
            rw [h11]
          have h12 : deriv (fun y : ℝ => f x * f y - g x * g y) 0 = f x * deriv f
            → 0 - g x * deriv g 0 := by
          have h13 : HasDerivAt (fun y : ℝ => f x * f y) (f x * deriv f 0) 0 :=
            by
            have h14 : HasDerivAt f (deriv f 0) 0 := by
              apply DifferentiableAt.hasDerivAt
              exact fgdiff.1.differentiableAt
            have h15 : HasDerivAt (fun y : ℝ => f x * f y) (f x * deriv f 0) 0 :=
              by
              apply HasDerivAt.const_mul (f x) h14
              exact h15
            have h16 : HasDerivAt (fun y : ℝ => g x * g y) (g x * deriv g 0) 0 :=
              by
              have h17 : HasDerivAt g (deriv g 0) 0 := by
                apply DifferentiableAt.hasDerivAt
                exact fgdiff.2.differentiableAt
            have h18 : HasDerivAt (fun y : ℝ => g x * g y) (g x * deriv g 0) 0 :=
              by
              apply HasDerivAt.const_mul (g x) h17
              exact h18
            have h19 : HasDerivAt (fun y : ℝ => f x * f y - g x * g y) (f x *
              → deriv f 0 - g x * deriv g 0) 0 := by
              apply HasDerivAt.sub h13 h16
            have h20 : deriv (fun y : ℝ => f x * f y - g x * g y) 0 = f x * deriv
              → f 0 - g x * deriv g 0 := by
              apply HasDerivAt.deriv
              exact h19
            exact h20
            rw [h12]
          have h21 : deriv f 0 = 0 := hf0
          rw [h21]
          <|> ring
          <|> simp [hf0]
          <|> linarith
        linarith
      have h_g'_formula : ∀ x, deriv g x = f x * deriv g 0 := by
        intro x
        have h1 : deriv (fun x => (f x)^2 + (g x)^2) x = 0 := by
          have h1 : deriv (fun x => (f x)^2 + (g x)^2) x = 2 * f x * deriv f x + 2 *
            → g x * deriv g x := by
          have h2 : HasDerivAt (fun x => (f x)^2 + (g x)^2) (2 * f x * deriv f x +
            → 2 * g x * deriv g x) x := by
          have h3 : HasDerivAt f (deriv f x) x := by
            apply DifferentiableAt.hasDerivAt
            exact fgdiff.1.differentiableAt
          have h4 : HasDerivAt g (deriv g x) x := by
            apply DifferentiableAt.hasDerivAt
            exact fgdiff.2.differentiableAt
          have h5 : HasDerivAt (fun x => (f x)^2) (2 * f x * deriv f x) x := by
            have h6 : HasDerivAt (fun x => (f x)^2) (2 * f x * deriv f x) x := by
              convert HasDerivAt.pow 2 h3 using 1 <|> ring
              exact h6
            have h7 : HasDerivAt (fun x => (g x)^2) (2 * g x * deriv g x) x := by
              have h8 : HasDerivAt (fun x => (g x)^2) (2 * g x * deriv g x) x := by
                convert HasDerivAt.pow 2 h4 using 1 <|> ring
                exact h8
              have h9 : HasDerivAt (fun x => (f x)^2 + (g x)^2) (2 * f x * deriv f x
                → + 2 * g x * deriv g x) x := by
                convert h5.add h7 using 1 <|> ring
                exact h9
              have h10 : deriv (fun x => (f x)^2 + (g x)^2) x = 2 * f x * deriv f x +
                → 2 * g x * deriv g x := by
                apply HasDerivAt.deriv
                exact h2
                exact h10
              rw [h1]
            have h2 : deriv f x = -g x * deriv g 0 := h_f'_formula x
            have h3 : deriv g x = f x * deriv g 0 := h_g'_formula x
            rw [h2, h3]
            ring_nf
            <|>
            (try simp_all) <|>
            (try ring_nf) <|>
            (try linarith)
            <|>
            (try nlinarith)
          have h_b_constant : ∃ (c : ℝ), ∀ x, (f x)^2 + (g x)^2 = c := by
            have h_b : ∀ x, deriv (fun x : ℝ => (f x)^2 + (g x)^2) x = 0 := h_h'_zero
            have h_b : Differentiable ℝ (fun x : ℝ => (f x)^2 + (g x)^2) := by
              apply Differentiable.add
              · apply Differentiable.pow
                exact fgdiff.1
              · apply Differentiable.pow
                exact fgdiff.2
            have h_b : ∀ x, (f x)^2 + (g x)^2 = (f 0)^2 + (g 0)^2 := by
              intro x
              have h_b : deriv (fun x : ℝ => (f x)^2 + (g x)^2) = fun x => 0 := by
                funext x
                rw [h_b]
                <|> simp
              have h_b : (fun x : ℝ => (f x)^2 + (g x)^2) x = (fun x : ℝ => (f x)^2 + (g
                → x)^2) 0 := by
              apply is_const_of_deriv_eq_zero h_b
              intro x
              rw [h_b]
              <|> simp
              simp at h_b
              <|> linarith
              refine' ((f 0)^2 + (g 0)^2, _)

```

```

intro x
have h1 := h, x
linarith

have h_h_mul : ∀ (x y : ℝ), (f (x + y))2 + (g (x + y))2 = ((f x)2 + (g x)2) * ((f y)2 + (g y)2) := by
  intro x y
  have h1 : f (x + y) = f x * f y - g x * g y := fadd x y
  have h2 : g (x + y) = f x * g y + g x * f y := gadd x y
  calc
    (f (x + y))2 + (g (x + y))2 = (f x * f y - g x * g y)2 + (f x * g y +
    → g x * f y)2 := by rw [h1, h2]
    _ = ((f x)2 * (f y)2 + (g x)2 * (g y)2 - 2 * (f x * f y * g x * g
    → y)) + ((f x)2 * (g y)2 + (g x)2 * (f y)2 + 2 * (f x * g y * g x *
    → f y)) := by
      ring_nf
    _ = (f x)2 * (f y)2 + (g x)2 * (g y)2 + (f x)2 * (g y)2 + (g x)2 *
    → (f y)2 := by ring
    _ = ((f x)2 + (g x)2) * ((f y)2 + (g y)2) := by ring

have h_h_zero_sq : (f 0)2 + (g 0)2 = 0 ∨ (f 0)2 + (g 0)2 = 1 := by
  have h1 : (f 0)2 + (g 0)2 = ((f 0)2 + (g 0)2) ^ 2 := by
  have h2 := h_h_mul 0 0
  have h3 : (f (0 + 0))2 + (g (0 + 0))2 = ((f 0)2 + (g 0)2) *
  → ((f 0)2 + (g 0)2) := by
    simp using h2
  have h4 : (f (0 + 0))2 + (g (0 + 0))2 = (f 0)2 + (g 0)2 := by
    norm_num
  have h5 : (f 0)2 + (g 0)2 = ((f 0)2 + (g 0)2) * ((f 0)2 +
  → (g 0)2) := by
    linarith
  nlinarith
  have h6 : (f 0)2 + (g 0)2 = 0 ∨ (f 0)2 + (g 0)2 = 1 := by
  have h7 : (f 0)2 + (g 0)2 ≥ 0 := by positivity
  have h8 : (f 0)2 + (g 0)2 = ((f 0)2 + (g 0)2) ^ 2 := h5
  have h9 : (f 0)2 + (g 0)2 = 0 ∨ (f 0)2 + (g 0)2 = 1 := by
    have h10 : (f 0)2 + (g 0)2 = 0 ∨ (f 0)2 + (g 0)2 = 1 := by
      apply or_iff_not_imp_left.mpr
      intro h
      apply mul_left_cancel, (sub_ne_zero.mpr h)
      nlinarith
    exact h10
  exact h9
  exact h6

have h_h_zero_not_zero : (f 0)2 + (g 0)2 ≠ 0 := by
  by.contra h
  have h1 : (f 0)2 + (g 0)2 = 0 := by
    linarith
  have h2 : ∀ x, (f x)2 + (g x)2 = 0 := by
    intro x
    have h3 : (f x)2 + (g x)2 = (f 0)2 + (g 0)2 := by
      obtain (c, hc) := h_h_constant
      have h4 := hc x
      have h5 := hc 0
      linarith
    rw [h3]
    linarith
  have h6 : ∀ x, f x = 0 := by
    intro x
    have h7 : (f x)2 + (g x)2 = 0 := h2 x
    have h8 : (f x)2 ≥ 0 := by positivity
    have h9 : (f x)2 = 0 := by positivity
    have h10 : (g x)2 ≥ 0 := by positivity
    have h11 : (f x)2 = 0 := by
      nlinarith
    have h12 : f x = 0 := by
      nlinarith
  exact h6
  have h13 : ∀ x, g x = 0 := by
    intro x
    have h14 : (f x)2 + (g x)2 = 0 := h2 x
    have h15 : (f x)2 ≥ 0 := by positivity
    have h16 : (g x)2 ≥ 0 := by positivity
    have h17 : (g x)2 = 0 := by
      nlinarith
    have h18 : g x = 0 := by
      nlinarith
  exact h13
  have h19 : ∃ c, f = Function.const ℝ c ∨ g = Function.const ℝ c := by
    refine' (0, _)
    apply Or.inl
    funext x
    rw [h14, x]
    <|> simp
  exact fgnconst h

have h_h_zero_one : (f 0)2 + (g 0)2 = 1 := by
  cases h_h_zero_sq with
  | inl h =>
    exfalse
    apply h_h_zero_not_zero
  | inr h =>
    exact h

have h_main : ∀ x, (f x)2 + (g x)2 = 1 := by
  obtain (c, hc) := h_h_constant
  have h1 : c = 1 := by
    have h2 : (f 0)2 + (g 0)2 = c := by
      have h3 := hc 0
      linarith
    have h4 : (f 0)2 + (g 0)2 = 1 := h_h_zero_one
    linarith
  intro x
  have h5 := hc x
  rw [h5] at h1
  linarith
  exact h_main

-- Simplified Proof
import Mathlib
import Aesop

set_option maxHeartbeats 0

open Filter Topology

```

```

theorem putnam_1991_b2
  (f g : ℝ → ℝ)
  (fgnconst : ∃ c, f = Function.const ℝ c ∨ g = Function.const ℝ c)
  (fgdiff : Differentiable ℝ f ∧ Differentiable ℝ g)
  (fadd : ∀ x y, f (x + y) = f x * f y - g x * g y)
  (gadd : ∀ x y, g (x + y) = f x * g y + g x * f y) :
  (deriv f 0 = 0) → (∀ x, (f x)2 + (g x)2 = 1) := by
  intro hf0
  have h_f'.formula : ∀ x, deriv f x = -g x * deriv g 0 := by
    intro x
    have h1 : deriv (fun y : ℝ => f (x + y)) 0 = deriv f x := by
      have h2 : HasDerivAt (fun y : ℝ => f (x + y)) (deriv f (x + 0) * 1) 0 :=
      → by
        have h3 : HasDerivAt (fun y : ℝ => x + y) 1 0 := by
          simp using (HasDerivAt_id (0 : ℝ)).const_add x
        have h4 : HasDerivAt f (deriv f (x + 0)) (x + 0) := by
          apply DifferentiableAt.hasDerivAt
          exact fgdff.1.differentiableAt
        have h5 : HasDerivAt (fun y : ℝ => f (x + y)) (deriv f (x + 0) * 1) 0
        → := by
          apply HasDerivAt.comp (0 : ℝ) h4 h3
          convert h5 using 1
        have h6 : deriv (fun y : ℝ => f (x + y)) 0 = deriv f (x + 0) * 1 := by
          apply HasDerivAt.deriv
          exact h2
        have h7 : deriv f (x + 0) * 1 = deriv f x := by
          simp
        rw [h6, h7]
      have h10 : deriv (fun y : ℝ => f (x + y)) 0 = -g x * deriv g 0 := by
        have h11 : (fun y : ℝ => f (x + y)) = (fun y : ℝ => f x * f y - g x * g
        → y) := by
          funext y
          rw [fadd x y]
        rw [h11]
      have h12 : deriv (fun y : ℝ => f x * f y - g x * g y) 0 = f x * deriv f
      → 0 - g x * deriv g 0 := by
        have h13 : HasDerivAt (fun y : ℝ => f x * f y) (f x * deriv f 0) 0 :=
        → by
          have h14 : HasDerivAt f (deriv f 0) 0 := by
            apply DifferentiableAt.hasDerivAt
            exact fgdff.1.differentiableAt
          have h15 : HasDerivAt (fun y : ℝ => f x * f y) (f x * deriv f 0) 0 :=
          → by
            apply HasDerivAt.const_mul (f x) h14
          exact h15
        have h16 : HasDerivAt (fun y : ℝ => g x * g y) (g x * deriv g 0) 0 :=
        → by
          have h17 : HasDerivAt g (deriv g 0) 0 := by
            apply DifferentiableAt.hasDerivAt
            exact fgdff.2.differentiableAt
          have h18 : HasDerivAt (fun y : ℝ => g x * g y) (g x * deriv g 0) 0 :=
          → by
            apply HasDerivAt.const_mul (g x) h17
          exact h18
        have h19 : HasDerivAt (fun y : ℝ => f x * f y - g x * g y) (f x *
        → deriv f 0 - g x * deriv g 0) 0 := by
          apply HasDerivAt.sub h13 h16
        have h20 : deriv (fun y : ℝ => f x * f y - g x * g y) 0 = f x * deriv
        → f 0 - g x * deriv g 0 := by
          apply HasDerivAt.deriv
          exact h19
        exact h20
      rw [h12]
      have h21 : deriv f 0 = 0 := hf0
      rw [h21]
      <|> ring
    linarith
  have h_g'.formula : ∀ x, deriv g x = f x * deriv g 0 := by
    intro x
    have h1 : deriv (fun y : ℝ => g (x + y)) 0 = deriv g x := by
      have h2 : HasDerivAt (fun y : ℝ => g (x + y)) (deriv g (x + 0) * 1) 0 :=
      → by
        have h3 : HasDerivAt (fun y : ℝ => x + y) 1 0 := by
          simp using (HasDerivAt_id (0 : ℝ)).const_add x
        have h4 : HasDerivAt g (deriv g (x + 0)) (x + 0) := by
          apply DifferentiableAt.hasDerivAt
          exact fgdff.2.differentiableAt
        have h5 : HasDerivAt (fun y : ℝ => g (x + y)) (deriv g (x + 0) * 1) 0
        → := by
          apply HasDerivAt.comp (0 : ℝ) h4 h3
          convert h5 using 1
        have h6 : deriv (fun y : ℝ => g (x + y)) 0 = deriv g (x + 0) * 1 := by
          apply HasDerivAt.deriv
          exact h2
        have h7 : deriv g (x + 0) * 1 = deriv g x := by
          simp
        rw [h6, h7]
      have h10 : deriv (fun y : ℝ => g (x + y)) 0 = f x * deriv g 0 := by
        have h11 : (fun y : ℝ => g (x + y)) = (fun y : ℝ => f x * g y + g x * f
        → y) := by
          funext y
          rw [gadd x y]
        rw [h11]
      have h12 : deriv (fun y : ℝ => f x * g y + g x * f y) 0 = f x * deriv g
      → 0 + g x * deriv f 0 := by
        have h13 : HasDerivAt (fun y : ℝ => f x * g y) (f x * deriv g 0) 0 :=
        → by
          have h14 : HasDerivAt g (deriv g 0) 0 := by
            apply DifferentiableAt.hasDerivAt
            exact fgdff.2.differentiableAt
          have h15 : HasDerivAt (fun y : ℝ => f x * g y) (f x * deriv g 0) 0 :=
          → by
            apply HasDerivAt.const_mul (f x) h14
          exact h15
        have h16 : HasDerivAt (fun y : ℝ => g x * f y) (g x * deriv f 0) 0 :=
        → by
          have h17 : HasDerivAt f (deriv f 0) 0 := by
            apply DifferentiableAt.hasDerivAt
            exact fgdff.1.differentiableAt
          have h18 : HasDerivAt (fun y : ℝ => g x * f y) (g x * deriv f 0) 0 :=
          → by
            apply HasDerivAt.const_mul (g x) h17

```

```

exact h18
have h19 : HasDerivAt (fun y : ℝ => f x * g y + g x * f y) (f x *
  ↪ deriv g 0 + g x * deriv f 0) 0 := by
  apply HasDerivAt.add h13 h16
have h20 : deriv (fun y : ℝ => f x * g y + g x * f y) 0 = f x * deriv
  ↪ g 0 + g x * deriv f 0 := by
  apply HasDerivAt.deriv
exact h19
exact h20
rw [h12]
have h21 : deriv f 0 = 0 := hf0
rw [h21]
<|> ring
linarith
have h_h_constant : ∃ (c : ℝ), ∀ x, (f x)^2 + (g x)^2 = c := by
have h : ∀ x, deriv (fun x => (f x)^2 + (g x)^2) x = 0 := by
  intro x
  have h2 : deriv (fun x => (f x)^2 + (g x)^2) x = 2 * f x * deriv f x + 2
    ↪ * g x * deriv g x := by
  have h3 : HasDerivAt (fun x => (f x)^2 + (g x)^2) (2 * f x * deriv f x
    ↪ + 2 * g x * deriv g x) x := by
    have h4 : HasDerivAt f (deriv f x) x := by
      apply DifferentiableAt.hasDerivAt
    exact fgdff.1.differentiableAt
    have h5 : HasDerivAt g (deriv g x) x := by
      apply DifferentiableAt.hasDerivAt
    exact fgdff.2.differentiableAt
    have h6 : HasDerivAt (fun x => (f x)^2) (2 * f x * deriv f x) x := by
      convert HasDerivAt.pow 2 h4 using 1 <|> ring
    have h7 : HasDerivAt (fun x => (g x)^2) (2 * g x * deriv g x) x := by
      convert HasDerivAt.pow 2 h5 using 1 <|> ring
    have h8 : HasDerivAt (fun x => (f x)^2 + (g x)^2) (2 * f x * deriv f
      ↪ x + 2 * g x * deriv g x) x := by
      convert h6.add h7 using 1
    exact h8
  have h9 : deriv (fun x => (f x)^2 + (g x)^2) x = 2 * f x * deriv f x +
    ↪ 2 * g x * deriv g x := by
    apply HasDerivAt.deriv
  exact h3
  exact h9
  rw [h2]
  have h3 : deriv f x = -g x * deriv g 0 := h.f'.formula x
  have h4 : deriv g x = f x * deriv g 0 := h.g'.formula x
  rw [h3, h4]
  ring_nf
have h : Differentiable ℝ (fun x : ℝ => (f x)^2 + (g x)^2) := by
  apply Differentiable.add
  · apply Differentiable.pow
  exact fgdff.1
  · apply Differentiable.pow
  exact fgdff.2
have h : ∀ x, (f x)^2 + (g x)^2 = (f 0)^2 + (g 0)^2 := by
  intro x
  have h : deriv (fun x : ℝ => (f x)^2 + (g x)^2) = fun x => 0 := by
    funext x
    rw [h, x]
  have h : (fun x : ℝ => (f x)^2 + (g x)^2) x = (fun x : ℝ => (f x)^2 + (g
    ↪ x)^2) 0 := by
    apply is_const_of_deriv_eq_zero h
  intro x
  rw [h]
  simp at h
  <|> linarith
  refine' ((f 0)^2 + (g 0)^2, _)
  intro x
  have h : := h, x
  linarith
have h_h_mul : ∀ (x y : ℝ), (f (x + y))^2 + (g (x + y))^2 = ((f x)^2 + (g
  ↪ x)^2) * ((f y)^2 + (g y)^2) := by
  intro x y
  have h1 : f (x + y) = f x * f y - g x * g y := fadd x y
  have h2 : g (x + y) = f x * g y + g x * f y := gadd x y
  calc
    (f (x + y))^2 + (g (x + y))^2 = (f x * f y - g x * g y)^2 + (f x * g y +
      ↪ g x * f y)^2 := by rw [h1, h2]
    _ = ((f x)^2 * (f y)^2 + (g x)^2 * (g y)^2 - 2 * (f x * f y * g x * g
      ↪ y)) + ((f x)^2 * (g y)^2 + (g x)^2 * (f y)^2 + 2 * (f x * g y * g x *
        ↪ f y)) := by
      ring_nf
    _ = (f x)^2 * (f y)^2 + (g x)^2 * (g y)^2 + (f x)^2 * (g y)^2 + (g x)^2 *
      ↪ (f y)^2 := by ring
    _ = ((f x)^2 + (g x)^2) * ((f y)^2 + (g y)^2) := by ring
have h_h_zero_sq : (f 0)^2 + (g 0)^2 = 0 ∨ (f 0)^2 + (g 0)^2 = 1 := by
have h : (f 0)^2 + (g 0)^2 = ((f 0)^2 + (g 0)^2) ^ 2 := by
  have h : := h_h_mul 0 0
  have h : (f (0 + 0)) ^ 2 + (g (0 + 0)) ^ 2 = ((f 0) ^ 2 + (g 0) ^ 2) *
    ↪ ((f 0) ^ 2 + (g 0) ^ 2) := by
    simp using h
  have h : (f (0 + 0)) ^ 2 + (g (0 + 0)) ^ 2 = (f 0) ^ 2 + (g 0) ^ 2 := by
    norm_num
  linarith
have h : (f 0)^2 + (g 0)^2 = 0 ∨ (f 0)^2 + (g 0)^2 = 1 := by
  have h : (f 0)^2 + (g 0)^2 ≥ 0 := by positivity
  have h : (f 0)^2 + (g 0)^2 = 0 ∨ (f 0)^2 + (g 0)^2 = 1 := by
    apply or_iff_not_imp_left.mpr
  intro h
  apply mul_left_cancel. (sub_ne_zero.mpr h)
  linarith
exact h
have h_h_zero_not_zero : (f 0)^2 + (g 0)^2 ≠ 0 := by
  by_contra h
  have h : (f 0)^2 + (g 0)^2 = 0 := by linarith
  have h : ∀ x, (f x)^2 + (g x)^2 = 0 := by
    intro x
    have h : (f x)^2 + (g x)^2 = (f 0)^2 + (g 0)^2 := by
      obtain (c, hc) := h_h_constant
      have h : := hc x
      have h : := hc 0
      linarith
    rw [h]
    linarith
  intro x
  have h : ∀ x, f x = 0 := by
    have h : (f x)^2 + (g x)^2 = 0 := h, x
    have h : (f x)^2 ≥ 0 := by positivity

```



```

simp [h3, h4, Int.cast_add, Int.cast_one, Int.cast_zero,
→ Int.cast_mul, Int.cast_ofNat] at h2 ⊢ <|>
<|> ring_nf at h2 ⊢ <|>
(try omega) <|>
(try linarith) <|>
(try norm_num at h2 ⊢ <|> linarith)

have h2 : ∀ (m : ℕ), f (-m : ℤ) = 1 - (-m : ℤ) := by
intro m
induction m using Nat.strong_induction_on with
| h m ih =>
match m with
| 0 =>
norm_num [h]
| 1 =>
have h3 := h2 (-1 : ℤ)
have h4 := h2 (1 : ℤ)
norm_num [h] at h3 h4 ⊢
<|>
(try omega) <|>
(try linarith) <|>
(try norm_num at h3 h4 ⊢ <|> linarith)
| m + 2 =>
have h3 := h2 (-m + 2 : ℤ)
have h4 := h2 (m + 1) (by omega)
simp [h3, h4, Int.cast_add, Int.cast_one, Int.cast_zero,
→ Int.cast_mul, Int.cast_ofNat] at h2 ⊢
<|> ring_nf at h2 ⊢ <|>
(try omega) <|>
(try linarith) <|>
(try norm_num at h2 ⊢ <|> linarith)

intro n
have h2 : n ≥ 0 ∨ n < 0 := by
by_cases h2 : n ≥ 0
· exact Or.inl h2
· exact Or.inr (by linarith)
cases h2 with
| inl h2 =>
have h4 : ∃ (m : ℕ), (m : ℤ) = n := by
use n.toNat
<|> simp [Int.toNat_of_nnonneg h2]
<|> omega
obtain m, hm := h4
have h3 : f n = 1 - n := by
have h31 : f (m : ℤ) = 1 - (m : ℤ) := h3 m
have h32 : (m : ℤ) = n := by exact_mod_cast hm
have h33 : f n = f (m : ℤ) := by rw [h32]
rw [h33, h31]
<|> simp [h32]
<|> ring_nf
<|> omega
exact h2
| inr h2 =>
have h4 : ∃ (m : ℕ), -(m : ℤ) = n := by
use (-n).toNat
<|>
(try simp [Int.toNat_of_nnonneg (by linarith : (0 : ℤ) ≤ -n)]) <|>
(try omega)
obtain m, hm := h4
have h3 : f n = 1 - n := by
have h31 : f (-(m : ℤ)) = 1 - (-(m : ℤ)) := h3 m
have h32 : -(m : ℤ) = n := by exact_mod_cast hm
have h33 : f n = f (-(m : ℤ)) := by rw [h32]
rw [h33, h31]
<|> simp [h32]
<|> ring_nf
<|> omega
exact h2
funext n
exact h2 n

have h_main : (f = fun n => 1 - n) ↔ (∀ n : ℤ, f (f n) = n) ∧ (∀ n : ℤ, f (f
→ (n + 2) + 2) = n) ∧ (f 0 = 1) := by
constructor
· intro h
exact h_forward h
· intro h
exact h_backward h

exact h_main

-- Simplified Proof
import Mathlib
import Aesop

set_option maxHeartbeats 0

open Topology Filter

theorem putnam_1992_a1
(f : ℤ → ℤ) :
(f = fun n => 1 - n) ↔
(∀ n : ℤ, f (f n) = n) ∧ (∀ n : ℤ, f (f (n + 2) + 2) = n) ∧ (f 0 = 1) := by
constructor
· rintro rfl
constructor
· intro n
simp
· constructor
· intro n
simp
<|> ring
norm_num
· rintro (h1, h2, h3)
ext1 n
have h1 : f 1 = 0 := by
have h11 := h1 0
have h12 := h1 1
simp_all
have h2 : ∀ (k : ℤ), f (k + 2) = f k - 2 := by
intro k
have h21 := h2 k
have h22 := h2 (k + 2) + 2

simp_all
have h2 : ∀ (n : ℤ), f n = 1 - n := by
intro n
have h21 := h2 (m : ℤ), f (m : ℤ) = 1 - (m : ℤ) := by
induction' m using Nat.strong_induction_on with m ih
rcases m with (| _ | _ | m)
· norm_num [h]
· norm_num [h]
· have h22 := h2 (m : ℤ)
have h23 := ih m (by omega)
have h24 := ih (m + 1) (by omega)
simp [h23, h24, Int.cast_add, Int.cast_one, Int.cast_zero,
→ Int.cast_mul, Int.cast_ofNat] at h2 ⊢
<|> ring_nf at h2 ⊢ <|> omega
have h25 : ∀ (m : ℕ), f (-m : ℤ) = 1 - (-m : ℤ) := by
intro m
induction' m using Nat.strong_induction_on with m ih
rcases m with (| _ | _ | m)
· norm_num [h]
· have h26 := h2 (-1 : ℤ)
have h27 := h2 (1 : ℤ)
norm_num [h] at h26 h27 ⊢
<|> omega
· have h28 := h2 (-m + 2 : ℤ)
have h29 := ih m (by omega)
have h30 := ih (m + 1) (by omega)
simp [h29, h30, Int.cast_add, Int.cast_one, Int.cast_zero,
→ Int.cast_mul, Int.cast_ofNat] at h2 ⊢
<|> ring_nf at h2 ⊢ <|> omega
rcases em (n ≥ 0) with (h31 | h32)
· have h33 : ∃ (m : ℕ), (m : ℤ) = n := by
use n.toNat
<|> simp [Int.toNat_of_nnonneg h31]
obtain m, hm := h33
have h34 : f n = 1 - n := by
have h341 : f (m : ℤ) = 1 - (m : ℤ) := h31 m
have h342 : (m : ℤ) = n := by exact_mod_cast hm
have h343 : f n = f (m : ℤ) := by rw [h342]
rw [h343, h341]
<|> simp [h342]
<|> ring_nf
<|> omega
exact h2
· have h35 : ∃ (m : ℕ), -(m : ℤ) = n := by
use (-n).toNat
<|> simp [Int.toNat_of_nnonneg (by linarith : (0 : ℤ) ≤ -n)]
obtain m, hm := h35
have h36 : f n = 1 - n := by
have h361 : f (-(m : ℤ)) = 1 - (-(m : ℤ)) := h31 m
have h362 : -(m : ℤ) = n := by exact_mod_cast hm
have h363 : f n = f (-(m : ℤ)) := by rw [h362]
rw [h363, h361]
<|> simp [h362]
<|> ring_nf
<|> omega
exact h2
nlinarith
linarith

exact h2 n hn IH
norm_num
· have h3 := h1 n hn
have h4 := h1 (n + 1) (by linarith)
simp [Nat.add_assoc] at h3 h4 ⊢
<|>
(try norm_num at * <|>)
(try linarith) <|>
(try simp_all [Nat.add_assoc]) <|>
(try ring_nf at * <|>)
(try linarith) <|>
(try field_simp [xnonzero] at * <|>)
(try nlinarith)
<|>
linarith
exact h2 n hn

have h_exists_a : ∃ (a : ℝ), ∀ (n : ℕ), n ≥ 1 → x (n + 1) = a * x n - x (n
→ 1) := by

```

```

use (x 2 + x 0) / x 1
intro n hn
have h₁ : (x (n + 1) + x (n - 1)) / x n = (x 2 + x 0) / x 1 := h_main n hn
have h₂ : x n = 0 := xnonzero n
have h₃ : (x (n + 1) + x (n - 1)) / x n = (x 2 + x 0) / x 1 := by rw [h₁]
have h₄ : x (n + 1) + x (n - 1) = ((x 2 + x 0) / x 1) * x n := by
  field_simp [h₃] at h₁ ⊢
  <|> nlinarith
have h₅ : x (n + 1) = ((x 2 + x 0) / x 1) * x n - x (n - 1) := by linarith
exact h₅

exact h_exists_a

-- Simplified Proof
import Mathlib
import Aesop

set_option maxHeartbeats 0

theorem putnam_1993_a2
(x : ℕ → ℝ)
(xnonzero : ∀ n : ℕ, x n ≠ 0)
(hx : ∀ n ≥ 1, (x n) ^ 2 - x (n - 1) * x (n + 1) = 1)
(∃ a : ℝ, ∀ n ≥ 1, x (n + 1) = a * x n - x (n - 1) := by
  use (x 2 + x 0) / x 1
  intro n hn
  have h₁ : (x (n + 1) + x (n - 1)) / x n = (x 2 + x 0) / x 1 := by
    have h₂ : ∀ n ≥ 1, (x (n + 1) + x (n - 1)) / x n = (x (n + 2) + x n) / x (n
      → + 1) := by
      intro n hn
      have h₃ := hx (n + 1) (by linarith)
      have h₄ := hx n hn
      field_simp [xnonzero] at h₃ h₄ ⊢
      nlinarith
    induction' hn with n hn IH
    · norm_num
    · have h₅ := h₁ n hn
      have h₆ := h₁ (n + 1) (by linarith)
      simp [Nat.add_assoc] at h₅ h₆ ⊢
      nlinarith
    field_simp [xnonzero n] at h₁ ⊢
    linarith
  -- Orig Proof
  import Mathlib
  import Aesop

  set_option maxHeartbeats 0

theorem putnam_1993_b1 :
  IsLeast
  {n : ℕ | 0 < n ∧
    ∃ m ∈ Set.Ioo (0 : ℤ) (1993), ∃ k : ℤ,
    (m / 1993 < (k : ℝ) / n) ∧ ((k : ℝ) / n < (m + 1) / 1994) }
  ((3987 : ℕ) :=
  by
  have h_main : IsLeast {n : ℕ | 0 < n ∧ ∃ m ∈ Set.Ioo (0 : ℤ) (1993), ∃ k : ℤ,
    → (m / 1993 < (k : ℝ) / n) ∧ ((k : ℝ) / n < (m + 1) / 1994)} 3987 := by
  constructor
  · constructor
  · norm_num
  · intro m hm
  have h₁ : (m : ℤ) ∈ Set.Ioo (0 : ℤ) (1993) := hm
  have h₂ : 0 < (m : ℤ) := by exact h₁.1
  have h₃ : (m : ℤ) < 1993 := by exact h₁.2
  use (2 * m + 1 : ℤ)
  constructor
  have h₄ : (m : ℝ) / 1993 < ((2 * m + 1 : ℤ) : ℝ) / 3987 := by
    have h₅ : (m : ℝ) < 1993 := by exact_mod_cast h₁
    have h₆ : 0 < (m : ℝ) := by exact_mod_cast h₂
    norm_num at h₅ ⊢
    <|>
    (try norm_num) <|>
    (try linarith) <|>
    (try
      {
        rw [div_lt_div_iff] <|>
        norm_cast <|>
        (try norm_num) <|>
        (try nlinarith)
      })
    <|>
    (try
      {
        field_simp at h₁ ⊢ <|>
        rw [div_lt_div_iff] <|>
        norm_cast <|>
        (try norm_num) <|>
        (try nlinarith)
      })
  exact h₄
  have h₄ : ((2 * m + 1 : ℤ) : ℝ) / 3987 < (m + 1 : ℝ) / 1994 := by
    have h₅ : (m : ℝ) < 1993 := by exact_mod_cast h₁
    have h₆ : 0 < (m : ℝ) := by exact_mod_cast h₂
    norm_num at h₅ ⊢
    <|>
    (try norm_num) <|>
    (try linarith) <|>
    (try
      {
        rw [div_lt_div_iff] <|>
        norm_cast <|>
        (try norm_num) <|>
        (try nlinarith)
      })
    <|>
    (try
      {
        field_simp at h₁ ⊢ <|>
        rw [div_lt_div_iff] <|>

```

```

obtain (k, h, hb) := h
field_simp at h, hb
rw [div_lt_div_iff (by positivity) (by positivity)] at h, h
norm_cast at h, hb
<> norm_num at h, hb
<> omega
-----
-- Orig Proof
import Mathlib
import Aesop

set_option maxHeartbeats 0

theorem putnam_1995_a1
(S : Set  $\kappa$ )
(hS :  $\forall a \in S, \forall b \in S, a * b \in S$ )
(T U : Set  $\kappa$ )
(hsub :  $T \subseteq S \wedge U \subseteq S$ )
(hunion :  $T \cup U = S$ )
(hdisj :  $T \cap U = \emptyset$ )
(hT3 :  $\forall a \in T, \forall b \in T, \forall c \in T, a * b * c \in T$ )
(hU3 :  $\forall a \in U, \forall b \in U, \forall c \in U, a * b * c \in U$ )
: ( $\forall a \in T, \forall b \in T, a * b \in T$ )  $\vee$  ( $\forall a \in U, \forall b \in U, a * b \in U$ ) := by
  have h_main : ( $\forall a \in T, \forall b \in T, a * b \in T$ )  $\vee$  ( $\forall a \in U, \forall b \in U, a * b \in U$ ) :=
    by
      by_cases h : ( $\forall a \in T, \forall b \in T, a * b \in T$ )
      · exact Or.inl h
      ·
        have h₁ : ( $\exists a : \kappa$ ) (ha : a  $\in$  T) (b :  $\kappa$ ) (hb : b  $\in$  T), a * b  $\in$  T := by
          by_contra! h
          have h₂ :  $\forall a \in T, \forall b \in T, a * b \in T$  := by
            intro a ha hb
            have h₃ : a * b  $\in$  T := h₁ a ha hb hb
            exact h
          exact h
        obtain (a, ha, b, hb, hab) := h
        have habU : a * b  $\in$  U := by
          have h₄ : a * b  $\in$  S := hS a (hsub.1 ha) b (hsub.1 hb)
          have h₅ : a * b  $\in$  T  $\cup$  U := by
            rw [hunion]
            exact h
          cases' h₅ with h₆ h₆
          · ex falso
          · exact hab h₆
          exact h
        have h₇ : ( $\forall x : \kappa$ ), x  $\in$  U  $\rightarrow$  ( $\forall y : \kappa$ ), y  $\in$  U  $\rightarrow$  x * y  $\in$  U := by
          intro x hx y hy
          by_contra h
          have h₈ : x * y  $\in$  T := by
            have h₉ : x * y  $\in$  S := hS x (hsub.2 hx) y (hsub.2 hy)
            have h₁₀ : x * y  $\in$  T  $\cup$  U := by
              rw [hunion]
              exact h
            cases' h₉ with h₁₁ h₁₁
            · exact h
            · ex falso
            exact h
          have h₁₂ : (x * y) * a * b  $\in$  T := hT3 (x * y) h₁ a ha b hb
          have h₁₃ : x * y * (a * b)  $\in$  U := hU3 x hx y hy (a * b) habU
          have h₁₄ : (x * y) * a * b = x * y * (a * b) := by ring
          have h₁₅ : (x * y) * a * b  $\in$  U := by
            rw [h₁₄]
            exact h
          have h₁₆ : (x * y) * a * b  $\in$  T  $\cap$  U := Set.mem_inter h₁₅ h₁₆
          have h₁₇ : T  $\cap$  U =  $\emptyset$  := hdisj
          rw [h₁₇] at h₁₆
          exact Set.not_mem_empty _ h₁₆
          exact Or.inr (fun a ha b hb => h₁ a ha b hb)
        exact h_main

-- Simplified Proof
import Mathlib
import Aesop

set_option maxHeartbeats 0

theorem putnam_1995_a1
(S : Set  $\kappa$ )
(hS :  $\forall a \in S, \forall b \in S, a * b \in S$ )
(T U : Set  $\kappa$ )
(hsub :  $T \subseteq S \wedge U \subseteq S$ )
(hunion :  $T \cup U = S$ )
(hdisj :  $T \cap U = \emptyset$ )
(hT3 :  $\forall a \in T, \forall b \in T, \forall c \in T, a * b * c \in T$ )
(hU3 :  $\forall a \in U, \forall b \in U, \forall c \in U, a * b * c \in U$ )
: ( $\forall a \in T, \forall b \in T, a * b \in T$ )  $\vee$  ( $\forall a \in U, \forall b \in U, a * b \in U$ ) := by
  rw [or_iff_not_imp_left]
  intro h
  push_neg at h
  obtain (a, ha, b, hb, hab) := h
  have habU : a * b  $\in$  U := by
    have h₁ : a * b  $\in$  S := hS a (hsub.1 ha) b (hsub.1 hb)
    rw [hunion] at h₁
    exact h.resolve_left (by aesop)
  intro x hx y hy
  by_contra h
  have h₂ : x * y  $\in$  T := by
    have h₃ : x * y  $\in$  S := hS x (hsub.2 hx) y (hsub.2 hy)
    rw [hunion] at h₃
    exact h.resolve_right (by aesop)
  have h₄ : (x * y) * a * b  $\in$  T := hT3 (x * y) h₁ a ha b hb
  have h₅ : x * y * (a * b)  $\in$  U := hU3 x hx y hy (a * b) habU
  simp [mul_assoc] at h, h
  simp_all [Set.eq_empty_iff_forall_not_mem]

```

```

theorem putnam_1995_a3
(relation : (Fin 9  $\rightarrow$  z)  $\rightarrow$  (Fin 9  $\rightarrow$  z)  $\rightarrow$  Prop)
(digits_to_num : (Fin 9  $\rightarrow$  z)  $\rightarrow$  z)
(hdigits_to_num : digits_to_num = fun dig =>  $\sum i : \text{Fin } 9, (\text{dig } i) * 10^{i.1}$ )
(hrelation :  $\forall d e : (\text{Fin } 9 \rightarrow z), \text{relation } d e \leftrightarrow (\forall i : \text{Fin } 9, d i < 10 \wedge d i \geq$ 
   $\rightarrow 0 \wedge e i < 10 \wedge e i \geq 0) \wedge (\forall i : \text{Fin } 9, 7 \mid (\text{digits\_to\_num } (\text{fun } j : \text{Fin } 9 \Rightarrow \text{if } j = i \text{ then } e \text{ else } d j)))$ )
:  $\forall d e f : (\text{Fin } 9 \rightarrow z), ((\text{relation } d e) \wedge (\text{relation } e f)) \rightarrow (\forall i : \text{Fin } 9, 7 \mid$ 
   $\rightarrow d i - f i) :=$  by
  have h_main :  $\forall (d e f : (\text{Fin } 9 \rightarrow z)), ((\text{relation } d e) \wedge (\text{relation } e f)) \rightarrow (\forall$ 
     $\rightarrow i : \text{Fin } 9, 7 \mid d i - f i) :=$  by
    intro d e f h
    have h₁ : relation d e := h.1
    have h₂ : relation e f := h.2
    have h₃ :  $\forall (i : \text{Fin } 9), 7 \mid (\text{digits\_to\_num } (\text{fun } j : \text{Fin } 9 \Rightarrow \text{if } j = i \text{ then } e \text{ else } d j)) :=$  by
      have h₄ : ( $\forall i : \text{Fin } 9, 7 \mid (\text{digits\_to\_num } (\text{fun } j : \text{Fin } 9 \Rightarrow \text{if } j = i \text{ then } e \text{ else } d j))$ ) :=
        by
          have h₅ : ( $\forall i : \text{Fin } 9, 7 \mid (\text{digits\_to\_num } (\text{fun } j : \text{Fin } 9 \Rightarrow \text{if } j = i \text{ then } e \text{ else } d j))$ ) :=
            (hrelation d e).mp h₁ |>.2
          exact h₅
    have h₆ :  $\forall (i : \text{Fin } 9), 7 \mid (\text{digits\_to\_num } (\text{fun } j : \text{Fin } 9 \Rightarrow \text{if } j = i \text{ then } f \text{ else } e j)) :=$  by
      have h₇ : ( $\forall i : \text{Fin } 9, 7 \mid (\text{digits\_to\_num } (\text{fun } j : \text{Fin } 9 \Rightarrow \text{if } j = i \text{ then } f \text{ else } e j))$ ) :=
        (hrelation e f).mp h₂ |>.2
      exact h₇
    have h₈ :  $\forall (i : \text{Fin } 9), 7 \mid (e i - d i) * (10 : z) ^ (i : \mathbb{N}) +$ 
       $\rightarrow \text{digits\_to\_num } d :=$  by
      intro i
      have h₉ :  $7 \mid (\text{digits\_to\_num } (\text{fun } j : \text{Fin } 9 \Rightarrow \text{if } j = i \text{ then } e \text{ else } d$ 
         $\rightarrow j)) :=$  h₁ i
      have h₁₀ :  $(\text{digits\_to\_num } (\text{fun } j : \text{Fin } 9 \Rightarrow \text{if } j = i \text{ then } e \text{ else } d j)) =$ 
         $\rightarrow \text{digits\_to\_num } d + (e i - d i) * (10 : z) ^ (i : \mathbb{N}) :=$  by
        calc
          (digits_to_num (fun j : Fin 9 => if j = i then e else d j)) =  $\sum j$ 
             $\rightarrow : \text{Fin } 9, (\text{if } j = i \text{ then } e \text{ else } d j) * (10 : z) ^ (j : \mathbb{N}) :=$  by
            simp [hdigits_to_num]
            <>
            rfl
            =  $\sum j : \text{Fin } 9, (\text{if } j = i \text{ then } e \text{ else } d j) * (10 : z) ^ (j : \mathbb{N}) :=$ 
              by
              rfl
              =  $(\sum j : \text{Fin } 9, d j * (10 : z) ^ (j : \mathbb{N})) + (e i - d i) * (10 : z) ^ (i : \mathbb{N}) :=$ 
                by
                calc
                  (sum j : Fin 9, (if j = i then e else d j) * (10 : z) ^ (j : N))
                    =  $\sum j : \text{Fin } 9, (d j * (10 : z) ^ (j : \mathbb{N}) + (\text{if } j = i \text{ then } (e j - d j)$ 
                       $\rightarrow \text{else } 0) * (10 : z) ^ (j : \mathbb{N})) :=$  by
                    apply Finset.sum_congr rfl
                    intro j _
                    by_cases h : j = i
                    · simp [h]
                    · <> ring
                    · simp [h]
                    · <> ring
                    =  $(\sum j : \text{Fin } 9, d j * (10 : z) ^ (j : \mathbb{N})) + \sum j : \text{Fin } 9, (\text{if } j =$ 
                       $\rightarrow i \text{ then } (e j - d j) \text{ else } 0) * (10 : z) ^ (j : \mathbb{N}) :=$  by
                      rw [Finset.sum_add_distrib]
                      =  $(\sum j : \text{Fin } 9, d j * (10 : z) ^ (j : \mathbb{N})) + (e i - d i) * (10$ 
                         $\rightarrow : z) ^ (i : \mathbb{N}) :=$  by
                        have h₁₁ :  $\sum j : \text{Fin } 9, (\text{if } j = i \text{ then } (e j - d j) \text{ else } 0) * (10$ 
                           $\rightarrow : z) ^ (j : \mathbb{N}) = (e i - d i) * (10 : z) ^ (i : \mathbb{N}) :=$  by
                        calc
                          =  $\sum j : \text{Fin } 9, (\text{if } j = i \text{ then } (e j - d j) \text{ else } 0) * (10$ 
                             $\rightarrow : z) ^ (j : \mathbb{N}) :=$  rfl
                          =  $(\text{if } i = i \text{ then } (e i - d i) \text{ else } 0) * (10 : z) ^ (i : \mathbb{N})$ 
                             $\rightarrow :=$  by
                        simp [Finset.sum_ite_eq', Finset.mem_univ, i.is_lt]
                        =  $(e i - d i) * (10 : z) ^ (i : \mathbb{N}) :=$  by simp
                        rw [h₁₁]
                        <> simp [hdigits_to_num]
                        <>
                        rfl
                        =  $\text{digits\_to\_num } d + (e i - d i) * (10 : z) ^ (i : \mathbb{N}) :=$  by
                        simp [hdigits_to_num]
                        <>
                        rfl
    have h₁₁ :  $7 \mid \text{digits\_to\_num } d + (e i - d i) * (10 : z) ^ (i : \mathbb{N}) :=$  by
      rw [h₈] at h
      exact h
    have h₁₂ :  $7 \mid (e i - d i) * (10 : z) ^ (i : \mathbb{N}) + \text{digits\_to\_num } d :=$  by
      have h₁₃ :  $(e i - d i) * (10 : z) ^ (i : \mathbb{N}) + \text{digits\_to\_num } d =$ 
         $\rightarrow \text{digits\_to\_num } d + (e i - d i) * (10 : z) ^ (i : \mathbb{N}) :=$  by ring
      rw [h₁₃]
      exact h
    have h₁₄ :  $\forall (i : \text{Fin } 9), 7 \mid (f i - e i) * (10 : z) ^ (i : \mathbb{N}) +$ 
       $\rightarrow \text{digits\_to\_num } e :=$  by
      intro i
      have h₁₅ :  $7 \mid (\text{digits\_to\_num } (\text{fun } j : \text{Fin } 9 \Rightarrow \text{if } j = i \text{ then } f \text{ else } e$ 
         $\rightarrow j)) :=$  h₂ i
      have h₁₆ :  $(\text{digits\_to\_num } (\text{fun } j : \text{Fin } 9 \Rightarrow \text{if } j = i \text{ then } f \text{ else } e j)) =$ 
         $\rightarrow \text{digits\_to\_num } e + (f i - e i) * (10 : z) ^ (i : \mathbb{N}) :=$  by
        calc
          (digits_to_num (fun j : Fin 9 => if j = i then f else e j)) =  $\sum j$ 
             $\rightarrow : \text{Fin } 9, (\text{if } j = i \text{ then } f \text{ else } e j) * (10 : z) ^ (j : \mathbb{N}) :=$  by
            simp [hdigits_to_num]
            <>
            rfl
            =  $\sum j : \text{Fin } 9, (e j * (10 : z) ^ (j : \mathbb{N})) + (f i - e i) * (10 : z) ^ (i : \mathbb{N}) :=$ 
              by
              rfl
              =  $(\sum j : \text{Fin } 9, e j * (10 : z) ^ (j : \mathbb{N})) + (f i - e i) * (10 : z) ^ (i : \mathbb{N}) :=$ 
                by
                calc
                  (sum j : Fin 9, (if j = i then f else e j) * (10 : z) ^ (j : N))
                    =  $\sum j : \text{Fin } 9, (e j * (10 : z) ^ (j : \mathbb{N}) + (\text{if } j = i \text{ then } (f j - e j)$ 
                       $\rightarrow \text{else } 0) * (10 : z) ^ (j : \mathbb{N})) :=$  by
                    apply Finset.sum_congr rfl
                    intro j _
                    by_cases h : j = i
                    · simp [h]

```



```

      have h10 : 7 ∣ d i - f i := h1 i
    exact h10
  exact h_main
-- Simplified Proof
import Mathlib
import Aesop

set_option maxHeartbeats 0

open Filter Topology Real

theorem putnam_1995_a3
  (relation : (Fin 9 → z) → (Fin 9 → z) → Prop)
  (digits_to_num : (Fin 9 → z) → z)
  (hdigits_to_num : digits_to_num = fun dig => x i : Fin 9, (dig i) * 10i.1)
  (hrelation : ∀ d e : (Fin 9 → z), relation d e ↔ (∀ i : Fin 9, d i < 10 ∧ d i ≥
    → 0 ∧ e i < 10 ∧ e i ≥ 0) ∧ (∀ i : Fin 9, 7 ∣ (digits_to_num (fun j :
    → Fin 9 => if j = i then e j else d j))))
  : ∀ d e f : (Fin 9 → z), ((relation d e) ∧ (relation e f)) → (∀ i : Fin 9, 7 ∣
    → d i - f i) := by
  have h1 : ∀ d e f : (Fin 9 → z), ((relation d e) ∧ (relation e f)) → (∀ i :
    → Fin 9, 7 ∣ d i - f i) := by
    intro d e f h
    have h2 : relation d e := h.1
    have h3 : relation e f := h.2
    have h4 : ∀ i : Fin 9, 7 ∣ (digits_to_num (fun j : Fin 9 => if j = i then e
    → j else d j)) := (hrelation d e).mp h2 |>.2
    have h5 : ∀ i : Fin 9, 7 ∣ (digits_to_num (fun j : Fin 9 => if j = i then f
    → j else e j)) := (hrelation e f).mp h3 |>.2
    have h6 : ∀ i : Fin 9, 7 ∣ (e i - d i) * (10 : z) ^ (i : N) + digits_to_num
    → d := by
      intro i
      have h7 : 7 ∣ (digits_to_num (fun j : Fin 9 => if j = i then e j else d
    → j)) := h4 i
      have h8 : (digits_to_num (fun j : Fin 9 => if j = i then e j else d j)) =
    → digits_to_num d + (e i - d i) * (10 : z) ^ (i : N) := by
        calc
          (digits_to_num (fun j : Fin 9 => if j = i then e j else d j)) = x j
    → Fin 9, (if j = i then e j else d j) * (10 : z) ^ (j : N) := by
            simp [hdigits_to_num]
            = x j : Fin 9, (if j = i then e j else d j) * (10 : z) ^ (j : N) :=
            rfl
            = (x j : Fin 9, d j * (10 : z) ^ (j : N)) + (e i - d i) * (10 : z)
            → ^ (i : N) := by
                calc
                  (x j : Fin 9, (if j = i then e j else d j) * (10 : z) ^ (j : N))
    → = x j : Fin 9, (d j * (10 : z) ^ (j : N) + (if j = i then (e j - d j)
    → else 0) * (10 : z) ^ (j : N)) := by
                    apply Finset.sum_congr rfl
                    intro j _
                    by_cases h : j = i
                    <|> simp [h]
                    <|> ring
                    simp [h]
                    = (x j : Fin 9, d j * (10 : z) ^ (j : N)) + x j : Fin 9, (if j =
    → i then (e j - d j) else 0) * (10 : z) ^ (j : N) := by
                        rw [Finset.sum_add_distrib]
                        = (x j : Fin 9, d j * (10 : z) ^ (j : N)) + (e i - d i) * (10
    → : z) ^ (i : N) := by
                            have h9 : x j : Fin 9, (if j = i then (e j - d j) else 0) * (10
    → : z) ^ (j : N) = (e i - d i) * (10 : z) ^ (i : N) := by
                                calc
                                  = x j : Fin 9, (if j = i then (e j - d j) else 0) * (10
    → : z) ^ (j : N) := rfl
                                  = (if i = i then (e i - d i) else 0) * (10 : z) ^ (i : N)
    → := by
                                      simp [Finset.sum_ite_eq', Finset.mem_univ, i.is_lt]
                                      = (e i - d i) * (10 : z) ^ (i : N) := by simp
                                      rw [h.]
                                      = digits_to_num d + (e i - d i) * (10 : z) ^ (i : N) := by
                                          simp [hdigits_to_num]
    have h10 : 7 ∣ digits_to_num d + (e i - d i) * (10 : z) ^ (i : N) := by
      rw [h6] at h10
      exact h10
    have h11 : ∀ i : Fin 9, 7 ∣ (f i - e i) * (10 : z) ^ (i : N) + digits_to_num
    → e := by
      intro i
      have h12 : 7 ∣ (digits_to_num (fun j : Fin 9 => if j = i then f j else e
    → j)) := h5 i
      have h13 : (digits_to_num (fun j : Fin 9 => if j = i then f j else e j)) =
    → digits_to_num e + (f i - e i) * (10 : z) ^ (i : N) := by
          calc
            (digits_to_num (fun j : Fin 9 => if j = i then f j else e j)) = x j
    → Fin 9, (if j = i then f j else e j) * (10 : z) ^ (j : N) := by
                simp [hdigits_to_num]
                = x j : Fin 9, (if j = i then f j else e j) * (10 : z) ^ (j : N) :=
                rfl
                = (x j : Fin 9, e j * (10 : z) ^ (j : N)) + (f i - e i) * (10 : z)
                → ^ (i : N) := by
                    calc
                      (x j : Fin 9, (if j = i then f j else e j) * (10 : z) ^ (j : N))
    → = x j : Fin 9, (e j * (10 : z) ^ (j : N) + (if j = i then (f j - e j)
    → else 0) * (10 : z) ^ (j : N)) := by
                        apply Finset.sum_congr rfl
                        intro j _
                        by_cases h : j = i
                        <|> simp [h]
                        <|> ring
                        simp [h]
                        = (x j : Fin 9, e j * (10 : z) ^ (j : N)) + x j : Fin 9, (if j =
    → i then (f j - e j) else 0) * (10 : z) ^ (j : N) := by
                            rw [Finset.sum_add_distrib]
                            = (x j : Fin 9, e j * (10 : z) ^ (j : N)) + (f i - e i) * (10
    → : z) ^ (i : N) := by
                                calc
                                  = x j : Fin 9, (if j = i then (f j - e j) else 0) * (10 : z) ^ (j : N) +
    → digits_to_num e + (f i - e i) * (10 : z) ^ (i : N) := by
                                    simp [hdigits_to_num]
                                    = x j : Fin 9, (if j = i then (f j - e j) else 0) * (10 : z) ^ (j : N) +
    → digits_to_num e + (f i - e i) * (10 : z) ^ (i : N) := by ring
                                    rw [h12]
                                    exact h12
    exact h13
    exact h10
    have h14 : ∀ i : Fin 9, 7 ∣ (f i - e i) * (10 : z) ^ (i : N) + digits_to_num
    → e := by
      intro i
      have h15 : 7 ∣ (f i - e i) * (10 : z) ^ (i : N) + digits_to_num e := by
        have h16 : (f i - e i) * (10 : z) ^ (i : N) + digits_to_num e =
    → digits_to_num e + (f i - e i) * (10 : z) ^ (i : N) := by ring
        rw [h16]
        exact h16
      exact h15
    exact dvd_sub h14 h15
  have h17 : ∀ i : Fin 9, 7 ∣ (f i - d i) * (10 : z) ^ (i : N) := by
    intro i
    have h18 : 7 ∣ (f i - e i) * (10 : z) ^ (i : N) + digits_to_num e := h14 i
    have h19 : 7 ∣ (e i - d i) * (10 : z) ^ (i : N) + digits_to_num d := h10 i
    have h20 : 7 ∣ digits_to_num e + digits_to_num d := h10
    have h21 : 7 ∣ (f i - e i) * (10 : z) ^ (i : N) - digits_to_num d := by
      have h22 : 7 ∣ (f i - e i) * (10 : z) ^ (i : N) + digits_to_num e := h14 i
      have h23 : 7 ∣ digits_to_num e + digits_to_num d := h20
      have h24 : 7 ∣ ((f i - e i) * (10 : z) ^ (i : N) - digits_to_num e) -
    → (digits_to_num e + digits_to_num d) := by
          exact dvd_sub h22 h23
      have h25 : ((f i - e i) * (10 : z) ^ (i : N) + digits_to_num e) -
    → (digits_to_num e + digits_to_num d) = (f i - e i) * (10 : z) ^ (i : N) -
    → - digits_to_num d := by
          ring
          rw [h24] at h25
      exact h25
    have h26 : 7 ∣ (f i - d i) * (10 : z) ^ (i : N) := by
      have h27 : 7 ∣ (f i - e i) * (10 : z) ^ (i : N) - digits_to_num d := h21
      have h28 : 7 ∣ (e i - d i) * (10 : z) ^ (i : N) + digits_to_num d := h10
      have h29 : 7 ∣ ((f i - e i) * (10 : z) ^ (i : N) - digits_to_num d) +
    → ((e i - d i) * (10 : z) ^ (i : N) + digits_to_num d) := by
          exact dvd_add h27 h28
      have h30 : ((f i - e i) * (10 : z) ^ (i : N) - digits_to_num d) + ((e i
    → - d i) * (10 : z) ^ (i : N) + digits_to_num d) = (f i - d i) * (10 :
    → z) ^ (i : N) := by
          ring
          rw [h29] at h30
    exact h30

```

```

exact h9
exact h14
have h15 : ∀ (i : Fin 9), 7 ∣ d i - f i := by
intro i
have h11 : 7 ∣ (f i - d i) * (10 : z) ^ (i : N) := h1
have h12 : 7 ∣ (f i - d i) := by
have h13 : (7 : z) ∣ (f i - d i) * (10 : z) ^ (i : N) := h11
have h14 : (7 : N).Prime := by decide
have h15 : -(7 : z) ∣ (10 : z) ^ (i : N) := by
intro h
have h16 : (7 : N) ∣ (10 : N) ^ (i : N) := by
norm_cast at h
have h17 : (7 : N) ∣ 10 := by
exact Nat.Prime.dvd_of_dvd_pow h14 h16
norm_num at h17
have h18 : (7 : z) ∣ (f i - d i) := by
have h19 : (7 : z) ∣ (f i - d i) * (10 : z) ^ (i : N) := h13
have h20 : -(7 : z) ∣ (10 : z) ^ (i : N) := h15
have h21 : (7 : z) ∣ (f i - d i) := by
have h22 : (7 : z) ∣ (f i - d i) * (10 : z) ^ (i : N) := h13
have h23 : (7 : z) ∣ (f i - d i) * (10 : z) ^ (i : N) := h13
have h24 : (7 : z) ∣ (f i - d i) ∨ (7 : z) ∣ (10 : z) ^ (i : N) :=
by
have h25 : (7 : z) ∣ (f i - d i) * (10 : z) ^ (i : N) := h13
have h26 : (7 : z) ∣ (f i - d i) ∨ (7 : z) ∣ (10 : z) ^ (i : N) :=
by
apply (Int.prime_iff_natAbs_prime.mpr (by decide)).dvd_mul.mp
exact h25
cases h24 with
| inl h24 =>
exact h24
| inr h24 =>
exfalse
exact h23 h24
exact h22
exact h21
exact h20
have h27 : 7 ∣ d i - f i := by
have h28 : 7 ∣ (f i - d i) := h12
have h29 : 7 - (f i - d i) := by
exact dvd_neg.mpr h28
have h30 : -(f i - d i) = d i - f i := by ring
rw [h29] at h30
exact h30
exact h31
exact h32
exact h33
-- Orig Proof
import Mathlib
import Aesop

set_option maxHeartbeats 0

open Filter Topology Real Nat

theorem putnam_1995_b4
(confrac : ℝ)
(hconfrac : confrac = 2207 - 1 / confrac)
(hconfrac' : 1 < confrac) :
let (a, b, c, d) := ((3,1,5,2) : ℤ × ℤ × ℤ × ℤ)
confrac ^ ((1 : ℝ) / 8) = (a + b * sqrt c) / d :=
by
dsimp only
have h_main : confrac ^ ((1 : ℝ) / 8) = (3 + 1 * Real.sqrt 5) / 2 := by
have h1 : confrac > 0 := by linarith
have h2 : confrac ^ 2 - 2207 * confrac + 1 = 0 := by
have h3 : confrac = 2207 - 1 / confrac := hconfrac
have h4 : confrac ≠ 0 := by linarith
field_simp [h4] at h3
linarith

have h5 : ((3 + Real.sqrt 5) / 2 : ℝ) > 0 := by positivity

have h6 : (((3 + Real.sqrt 5) / 2 : ℝ) ^ 8 : ℝ) = (2207 + 987 * Real.sqrt
→ 5) / 2 := by
have h7 : Real.sqrt 5 ≥ 0 := Real.sqrt_nonneg _
have h8 : ((3 + Real.sqrt 5) / 2 : ℝ) ^ 2 = (7 + 3 * Real.sqrt 5) / 2 :=
by
linarith [Real.sq_sqrt (show 0 ≤ 5 by norm_num)]
have h9 : ((3 + Real.sqrt 5) / 2 : ℝ) ^ 4 = (47 + 21 * Real.sqrt 5) / 2 :=
by
calc
((3 + Real.sqrt 5) / 2 : ℝ) ^ 4 = (((3 + Real.sqrt 5) / 2 : ℝ) ^ 2)
→ ^ 2 := by ring
_ = ((7 + 3 * Real.sqrt 5) / 2 : ℝ) ^ 2 := by rw [h8]
_ = (47 + 21 * Real.sqrt 5) / 2 := by
linarith [Real.sq_sqrt (show 0 ≤ 5 by norm_num)]
calc
(((3 + Real.sqrt 5) / 2 : ℝ) ^ 8 : ℝ) = (((3 + Real.sqrt 5) / 2 : ℝ) ^
→ 4) ^ 2 := by ring
_ = ((47 + 21 * Real.sqrt 5) / 2 : ℝ) ^ 2 := by rw [h8]
_ = (2207 + 987 * Real.sqrt 5) / 2 := by
linarith [Real.sq_sqrt (show 0 ≤ 5 by norm_num)]

have h10 : ((2207 + 987 * Real.sqrt 5) / 2 : ℝ) > 1 := by
linarith [Real.sq_sqrt_nonneg 5, Real.sq_sqrt (show 0 ≤ 5 by norm_num)]
have h11 : ((2207 + 987 * Real.sqrt 5) / 2 : ℝ) ^ 2 - 2207 * ((2207 + 987 *
→ Real.sqrt 5) / 2 : ℝ) + 1 = 0 := by
linarith [Real.sq_sqrt (show 0 ≤ 5 by norm_num),
Real.sq_sqrt_nonneg 5]

have h12 : confrac = (2207 + 987 * Real.sqrt 5) / 2 := by
have h13 : confrac = (2207 + 987 * Real.sqrt 5) / 2 ∨ confrac = (2207 -
→ 987 * Real.sqrt 5) / 2 := by
have h14 : confrac ^ 2 - 2207 * confrac + 1 = 0 := h12
have h15 : ((2207 + 987 * Real.sqrt 5) / 2 : ℝ) ^ 2 - 2207 * ((2207 +
→ 987 * Real.sqrt 5) / 2 : ℝ) + 1 = 0 := h12
have h16 : ((2207 - 987 * Real.sqrt 5) / 2 : ℝ) ^ 2 - 2207 * ((2207 -
→ 987 * Real.sqrt 5) / 2 : ℝ) + 1 = 0 := by
linarith [Real.sq_sqrt (show 0 ≤ 5 by norm_num),
Real.sq_sqrt_nonneg 5]

linarith [Real.sq_sqrt (show 0 ≤ 5 by norm_num),
Real.sq_sqrt_nonneg 5]
have h17 : confrac = (2207 + 987 * Real.sqrt 5) / 2 ∨ confrac = (2207 -
→ 987 * Real.sqrt 5) / 2 := by
linarith [Real.sq_sqrt (show 0 ≤ 5 by norm_num),
Real.sq_sqrt_nonneg 5]
linarith

have h18 : confrac ^ ((1 : ℝ) / 8) = (3 + 1 * Real.sqrt 5) / 2 := by
rw [h17]
have h19 : (((2207 + 987 * Real.sqrt 5) / 2 : ℝ) > 0 := by positivity
have h20 : ((3 + Real.sqrt 5) / 2 : ℝ) > 0 := by positivity
have h21 : (((3 + Real.sqrt 5) / 2 : ℝ) ^ 8 : ℝ) = (2207 + 987 *
→ Real.sqrt 5) / 2 := by
have h22 : Real.log (((3 + Real.sqrt 5) / 2 : ℝ) ^ 8) = Real.log ((2207 +
→ 987 * Real.sqrt 5) / 2) := by
rw [h21]
have h23 : 8 * Real.log ((3 + Real.sqrt 5) / 2) = Real.log ((2207 + 987 *
→ Real.sqrt 5) / 2) := by
have h24 : Real.log (((3 + Real.sqrt 5) / 2 : ℝ) ^ 8) = 8 * Real.log
→ (((3 + Real.sqrt 5) / 2) := by
rw [Real.log_pow]
<> norm_num
linarith
have h25 : Real.log (((2207 + 987 * Real.sqrt 5) / 2 : ℝ) ^ ((1 : ℝ) /
→ 8)) = Real.log ((3 + Real.sqrt 5) / 2) := by
have h26 : Real.log (((2207 + 987 * Real.sqrt 5) / 2 : ℝ) ^ ((1 : ℝ) /
→ 8)) = ((1 : ℝ) / 8) * Real.log ((2207 + 987 * Real.sqrt 5) / 2) := by
rw [Real.log_rpow (by positivity)]
have h27 : ((1 : ℝ) / 8) * Real.log ((2207 + 987 * Real.sqrt 5) / 2) =
→ Real.log ((3 + Real.sqrt 5) / 2) := by
have h28 : Real.log ((2207 + 987 * Real.sqrt 5) / 2) = 8 * Real.log
→ ((3 + Real.sqrt 5) / 2) := by
linarith
rw [h27]
ring_nf
<> field_simp
<> ring_nf
rw [h28]
have h29 : ((2207 + 987 * Real.sqrt 5) / 2 : ℝ) ^ ((1 : ℝ) / 8) = (3 +
→ Real.sqrt 5) / 2 := by
apply Real.log_injOn_pos (Set.mem_Ioi.mpr (by positivity))
-- (Set.mem_Ioi.mpr (by positivity))
linarith
rw [h29]
<> ring_nf
<> field_simp
<> ring_nf
exact h29

norm_num at h_main
<>
(try simp_all [Complex.ext_iff, pow_one]) <>
(try norm_num) <>
(try ring_nf at * <> norm_num at * <> linarith [Real.sq_sqrt_nonneg 5]) <>
(try field_simp at * <> ring_nf at * <> norm_num at * <> linarith
→ [Real.sq_sqrt_nonneg 5]) <>

{
linarith [Real.sq_sqrt_nonneg 5, Real.sq_sqrt (show 0 ≤ 5 by norm_num)]
} <>
{
{
rw [h_main]
<>
norm_num <>
ring_nf <>
norm_num <>
field_simp [Real.sq_sqrt_eq_iff_sq_eq] <>
ring_nf <>
norm_num <>
linarith [Real.sq_sqrt_nonneg 5, Real.sq_sqrt (show 0 ≤ 5 by norm_num)]
}
}
<>
norm_num at *
<>
linarith [Real.sq_sqrt_nonneg 5]

-- Simplified Proof
import Mathlib
import Aesop

set_option maxHeartbeats 0

open Filter Topology Real Nat

theorem putnam_1995_b4
(confrac : ℝ)
(hconfrac : confrac = 2207 - 1 / confrac)
(hconfrac' : 1 < confrac) :
let (a, b, c, d) := ((3,1,5,2) : ℤ × ℤ × ℤ × ℤ)
confrac ^ ((1 : ℝ) / 8) = (a + b * sqrt c) / d := by
have h1 : confrac > 0 := by linarith
have h2 : confrac ^ 2 - 2207 * confrac + 1 = 0 := by
have h3 : confrac = 2207 - 1 / confrac := hconfrac
have h4 : confrac ≠ 0 := by linarith
field_simp [hconfrac] at hconfrac
linarith [hconfrac, hconfrac']
have h5 : confrac = (2207 + 987 * Real.sqrt 5) / 2 := by
have h6 : confrac ^ 2 - 2207 * confrac + 1 = 0 := h2
have h7 : ((2207 + 987 * Real.sqrt 5) / 2 : ℝ) ^ 2 - 2207 * ((2207 +
→ 987 * Real.sqrt 5) / 2 : ℝ) + 1 = 0 := h2
have h8 : ((2207 - 987 * Real.sqrt 5) / 2 : ℝ) ^ 2 - 2207 * ((2207 -
→ 987 * Real.sqrt 5) / 2 : ℝ) + 1 = 0 := by
linarith [Real.sq_sqrt (show 0 ≤ 5 by norm_num),
Real.sq_sqrt_nonneg 5]

```

```

nlinarith [Real.sq_sqrt (show 0 ≤ 5 by norm_num),
  Real.sq_sqrt_nonneg 5]
have h₁ : (2207 + 987 * Real.sqrt 5) / 2 √ contfrac = (2207 -
  → 987 * Real.sqrt 5) / 2 := by
  apply or_iff_not_imp_left.mpr
  intro h
  apply mul_left_cancel (sub_ne_zero.mpr h.)
  nlinarith [Real.sq_sqrt (show 0 ≤ 5 by norm_num),
    Real.sq_sqrt_nonneg 5]
cases h with
| inl h => exact h
| inr h =>
  have h₂ : (2207 - 987 * Real.sqrt 5) / 2 := h₁
  have h₃ : (2207 - 987 * Real.sqrt 5) / 2 < 1 := by
    nlinarith [Real.sq_sqrt_nonneg 5, Real.sq_sqrt (show 0 ≤ 5 by norm_num),
      sq_nonneg (Real.sq_sqrt 5 - 2205 / 987)]
  linarith
rw [h₁]
have h₄ : (((3 + Real.sqrt 5) / 2 : ℝ) ^ 8 : ℝ) = (2207 + 987 * Real.sqrt 5)
  → / 2 := by
  have h₅ : Real.sqrt 5 ≥ 0 := Real.sq_sqrt_nonneg _
  have h₆ : ((3 + Real.sqrt 5) / 2 : ℝ) ^ 2 = (7 + 3 * Real.sqrt 5) / 2 := by
    nlinarith [Real.sq_sqrt (show 0 ≤ 5 by norm_num)]
  have h₇ : ((3 + Real.sqrt 5) / 2 : ℝ) ^ 4 = (47 + 21 * Real.sqrt 5) / 2 :=
    → by
      calc
        ((3 + Real.sqrt 5) / 2 : ℝ) ^ 4 = (((3 + Real.sqrt 5) / 2 : ℝ) ^ 2) ^
          2 := by ring
        = ((7 + 3 * Real.sqrt 5) / 2 : ℝ) ^ 2 := by rw [h₆]
        = (47 + 21 * Real.sqrt 5) / 2 := by
          nlinarith [Real.sq_sqrt (show 0 ≤ 5 by norm_num)]
      calc
        (((3 + Real.sqrt 5) / 2 : ℝ) ^ 8 : ℝ) = (((3 + Real.sqrt 5) / 2 : ℝ) ^
          → 4) ^ 2 := by ring
        = ((47 + 21 * Real.sqrt 5) / 2 : ℝ) ^ 2 := by rw [h₆]
        = (2207 + 987 * Real.sqrt 5) / 2 := by
          nlinarith [Real.sq_sqrt (show 0 ≤ 5 by norm_num)]
  have h₈ : Real.log (((3 + Real.sqrt 5) / 2 : ℝ) ^ 8) = Real.log ((2207 + 987 *
    → Real.sqrt 5) / 2) := by
    rw [h₇]
  have h₉ : 8 * Real.log ((3 + Real.sqrt 5) / 2) = Real.log ((2207 + 987 *
    → Real.sqrt 5) / 2) := by
    have h₁₀ : Real.log (((3 + Real.sqrt 5) / 2 : ℝ) ^ 8) = 8 * Real.log ((3 +
      → Real.sqrt 5) / 2) := by
      rw [Real.log_pow]
      <|> norm_num
    linarith
  have h₁₁ : Real.log (((2207 + 987 * Real.sqrt 5) / 2 : ℝ) ^ ((1 : ℝ) / 8)) =
    → Real.log ((3 + Real.sqrt 5) / 2) := by
    have h₁₂ : Real.log (((2207 + 987 * Real.sqrt 5) / 2 : ℝ) ^ ((1 : ℝ) / 8)) =
      → ((1 : ℝ) / 8) * Real.log ((2207 + 987 * Real.sqrt 5) / 2) := by
      rw [Real.log_rpow (by positivity)]
    rw [h₁₁]
  have h₁₃ : (((1 : ℝ) / 8) * Real.log ((2207 + 987 * Real.sqrt 5) / 2)) =
    → Real.log ((3 + Real.sqrt 5) / 2) := by
    have h₁₄ : Real.log ((2207 + 987 * Real.sqrt 5) / 2) = 8 * Real.log ((3 +
      → Real.sqrt 5) / 2) := by
      linarith
      rw [h₁₃]
      ring_nf
    rw [h₁₃]
  have h₁₅ : ((2207 + 987 * Real.sqrt 5) / 2 : ℝ) ^ ((1 : ℝ) / 8) = (3 +
    → Real.sqrt 5) / 2 := by
    apply Real.log_injOn_pos (Set.mem_Ioi.mpr (by positivity))
    → (Set.mem_Ioi.mpr (by positivity))
    linarith
  rw [h₁₅]
  <|> ring_nf
-----
-- Orig Proof
import Mathlib
import Aesop

set_option maxHeartbeats 0

open Function

theorem putnam_1996_a4
(A : Type*)
[Finite A]
(S : Set (A × A × A))
(hS1 : ∀ a b c : A, (a, b, c) ∈ S → a ≠ b ∧ b ≠ c ∧ a ≠ c)
(hS2 : ∀ a b c : A, a ≠ c → (a, b, c) ∈ S → (c, b, a) ∈ S)
(hS3 : ∀ a b c d : A, (a, b, c) ∈ S ∧ (c, d, a) ∈ S → ((b, c, d) ∈ S ∧ (d, a, b) ∈ S))
: ∃ g : A → ℝ, Injective g ∧ (∀ a b c : A, g a < g b ∧ g b < g c → (a, b, c) ∈ S)
:= by
  have h_subsingleton : ∀ (x y : A), x = y := by
    intro x y
    by_contra h
    have h₁ : x ≠ y := h
    have h₂ : (x, x, y) : A × A × A ∈ S := by
      intro h₃
      have h₄ := hS1distinct x x y h₃
      tauto
    have h₃ : (y, x, x) : A × A × A ∈ S := by
      intro h₄
      have h₅ := hS1distinct y x x h₄
      tauto
    have h₄ := hS2 x x y (by intro h₃; apply h₁; simp_all)
    simp [h₃, h₄] at h
    <|> tauto

  have h_main : ∃ (g : A → ℝ), Function.Injective g ∧ (∀ a b c : A), g a < g b
    → a g b < g c → (a, b, c) ∈ S := by
    use fun _ => 0
    constructor
    · refine' fun a b h => _
      have h₁ : a = b := h_subsingleton a b
      exact h
    · intro a b c h
      have h₁ : (0 : ℝ) < 0 := by

```

```

linarith
linarith

exact h_main

-- Simplified Proof
import Mathlib
import Aesop

set_option maxHeartbeats 0

open Function

theorem putnam_1996_a4
(A : Type*)
[Finite A]
(S : Set (A × A × A))
(hS1 : ∀ a b c : A, (a, b, c) ∈ S → a ≠ b ∧ b ≠ c ∧ a ≠ c)
(hS2 : ∀ a b c : A, a ≠ c → (a, b, c) ∈ S → (c, b, a) ∈ S)
(hS3 : ∀ a b c d : A, (a, b, c) ∈ S ∧ (c, d, a) ∈ S → ((b, c, d) ∈ S ∧ (d, a, b) ∈ S))
: ∃ g : A → ℝ, Injective g ∧ (∀ a b c : A, g a < g b ∧ g b < g c → (a, b, c) ∈ S)
:= by
  have h_subsingleton : ∀ x y : A, x = y := by
    intro x y
    by_contra h
    have h₁ := hS1distinct x x y
    have h₂ := hS1 x x y
    simp_all
  use fun _ => 0
  constructor
  · intro a b h
    have h₁ : a = b := h_subsingleton a b
    exact h
  · simp_all
-----
-- Orig Proof
import Mathlib
import Aesop

set_option maxHeartbeats 0

open Filter Topology Bornology Set

theorem putnam_1997_b2
(f g : ℝ → ℝ)
(hg : ∀ x : ℝ, g x ≥ 0)
(hfderiv1 : ContDiff ℝ 1 f)
(hfderiv2 : Differentiable ℝ (deriv f))
(hfg : ∀ x : ℝ, f x + iteratedDeriv 2 f x = -x * g x * deriv f x)
: IsBounded (range (fun x => |f x|)) := by
  have h_main_ineq : ∀ (x : ℝ), (f x)^2 + (deriv f x)^2 ≤ (f 0)^2 + (deriv f
    → 0)^2 := by
    have h1 : ∀ x : ℝ, HasDerivAt (fun x : ℝ => (f x)^2 + (deriv f x)^2) (2 * f
      → x * deriv f x + 2 * (deriv f x) * (deriv (deriv f) x)) x := by
      intro x
      have h2 : HasDerivAt (fun x : ℝ => (f x)^2) (2 * f x * deriv f x) x := by
        have h3 : HasDerivAt f (deriv f) x := by
          apply DifferentiableAt.hasDerivAt
        have h4 : DifferentiableAt ℝ f x := by
          apply hfderiv1.differentiable le_rfl |>.differentiableAt
        exact h4
      have h5 : HasDerivAt (fun x : ℝ => (f x)^2) (2 * f x * deriv f x) x :=
        → by
          convert HasDerivAt.pow 2 h3 using 1 <|> ring
      exact h5
      have h6 : HasDerivAt (fun x : ℝ => (deriv f x)^2) (2 * (deriv f x) *
        → (deriv (deriv f) x)) x := by
        have h7 : HasDerivAt (deriv f) (deriv (deriv f) x) x := by
          apply DifferentiableAt.hasDerivAt
        have h8 : DifferentiableAt ℝ (deriv f) x := by
          apply hfderiv2.differentiableAt
        exact h8
      have h9 : HasDerivAt (fun x : ℝ => (deriv f x)^2) (2 * (deriv f x) *
        → (deriv (deriv f) x)) x := by
        convert HasDerivAt.pow 2 h7 using 1 <|> ring
      exact h9
      have h10 : HasDerivAt (fun x : ℝ => (f x)^2 + (deriv f x)^2) (2 * f x *
        → deriv f x + 2 * (deriv f x) * (deriv (deriv f) x)) x := by
        convert h2.add h6 using 1 <|> ring
      exact h10
    have h11 : ∀ x : ℝ, deriv (fun x : ℝ => (f x)^2 + (deriv f x)^2) x = 2 * f
      → x * deriv f x + 2 * (deriv f x) * (deriv (deriv f) x) := by
      intro x
      have h12 : deriv (fun x : ℝ => (f x)^2 + (deriv f x)^2) x = 2 * f x *
        → deriv f x + 2 * (deriv f x) * (deriv (deriv f) x) := by
        apply HasDerivAt.deriv
      exact h11
      rw [h12]
    have h13 : ∀ x : ℝ, deriv (fun x : ℝ => (f x)^2 + (deriv f x)^2) x = 2 *
      → (deriv f x) * (f x + deriv (deriv f) x) := by
      intro x
      rw [h11]
      ring_nf
      <|>
      simp_all [mul_assoc]
      <|>
      ring_nf
      <|>
      linarith
    have h14 : ∀ x : ℝ, deriv (fun x : ℝ => (f x)^2 + (deriv f x)^2) x = -2 * x
      → * g x * (deriv f x)^2 := by
      intro x
      have h15 : deriv (fun x : ℝ => (f x)^2 + (deriv f x)^2) x = 2 * (deriv f
        → x) * (f x + deriv (deriv f) x) := by
      rw [h13]
      rw [h15]
      have h16 : f x + deriv (deriv f) x = -x * g x * deriv f x := by
        have h17 : f x + iteratedDeriv 2 f x = -x * g x * deriv f x := hfg x
        have h18 : iteratedDeriv 2 f x = deriv (deriv f) x := by
          simp [iteratedDeriv_succ, Function.comp_apply]
          <|>
          simp_all [deriv_deriv]
          <|>
          try norm_num

```



```

    <=>
    try linarith
    rw [h18] at h17
    linarith
    rw [h16]
    ring_nf
    <=>
    simp_all [mul_assoc]
    <=>
    ring_nf
    <=>
    linarith
have h19 : ∀ x : ℝ, deriv (fun x : ℝ => (f x)^2 + (deriv f x)^2) x = -2 * x
  => * g x * (deriv f x)^2 := by
  intro x
  exact h14 x
intro x
by_cases hx : x ≥ 0
·
  have h20 : ContinuousOn (fun x : ℝ => (f x)^2 + (deriv f x)^2) (Set.Icc
    → 0 x) := by
    have h21 : ContinuousOn (fun x : ℝ => (f x)^2) (Set.Icc 0 x) := by
      have h22 : ContinuousOn f (Set.Icc 0 x) := by
        apply hfderiv1.continuous.continuousOn
      exact h22.pow 2
    have h23 : ContinuousOn (fun x : ℝ => (deriv f x)^2) (Set.Icc 0 x) :=
      by
        have h24 : ContinuousOn (deriv f) (Set.Icc 0 x) := by
          have h25 : Differentiable ℝ (deriv f) := hfderiv2
          exact h25.continuous.continuousOn
        exact h24.pow 2
    exact h21.add h23
  have h26 : DifferentiableOn ℝ (fun x : ℝ => (f x)^2 + (deriv f x)^2)
    → (Set.Ioo 0 x) := by
    intro y hy
    have h27 : DifferentiableAt ℝ (fun x : ℝ => (f x)^2 + (deriv f x)^2) y
      := by
        have h28 : HasDerivAt (fun x : ℝ => (f x)^2 + (deriv f x)^2) (2 * f
          → y * deriv f y + 2 * (deriv f y) * (deriv (deriv f) y)) y := h1 y
        exact h28.differentiableAt
      exact h27.differentiableWithinAt
  have h29 : ∀ y ∈ Set.Ioo 0 x, deriv (fun x : ℝ => (f x)^2 + (deriv f
    → x)^2) y ≤ 0 := by
    intro y hy
    have h30 : deriv (fun x : ℝ => (f x)^2 + (deriv f x)^2) y = -2 * y * g
      → y * (deriv f y)^2 := by
      rw [h19]
    rw [h30]
    have h31 : y > 0 := by exact hy.1
    have h32 : g y ≥ 0 := hg y
    have h33 : (deriv f y)^2 ≥ 0 := by positivity
    have h34 : -2 * y * g y * (deriv f y)^2 ≤ 0 := by
      have h35 : -2 * y ≤ 0 := by linarith
      have h36 : g y ≥ 0 := hg y
      have h37 : (deriv f y)^2 ≥ 0 := by positivity
      have h38 : -2 * y * g y ≤ 0 := by
        linarith
      linarith
    exact h34
  have h39 : (f x)^2 + (deriv f x)^2 ≤ (f 0)^2 + (deriv f 0)^2 := by
    by_cases h40 : x = 0
    ·
      simp [h40]
    ·
      have h41 : x > 0 := by
        cases' lt_or_gt_of_ne h40 with h42 h42
        · exfalse
        · linarith
      exact h42
      have h42 : (f x)^2 + (deriv f x)^2 ≤ (f 0)^2 + (deriv f 0)^2 := by
        have h43 : ∃ z ∈ Set.Ioo 0 x, deriv (fun x : ℝ => (f x)^2 + (deriv
          → f x)^2) z = (((f x)^2 + (deriv f x)^2) - ((f 0)^2 + (deriv f 0)^2))
          → / (x - 0) := by
          have h44 : ContinuousOn (fun x : ℝ => (f x)^2 + (deriv f x)^2)
            → (Set.Icc 0 x) := h20
          have h45 : DifferentiableOn ℝ (fun x : ℝ => (f x)^2 + (deriv f
            → x)^2) (Set.Ioo 0 x) := h26
          have h46 : (0 : ℝ) < x := by linarith
          have h47 : ∃ z ∈ Set.Ioo 0 x, deriv (fun x : ℝ => (f x)^2 +
            → (deriv f x)^2) z = (((f x)^2 + (deriv f x)^2) - ((f 0)^2 + (deriv f
            → 0)^2)) / (x - 0) := by
            apply exists_deriv_eq_slope (fun x : ℝ => (f x)^2 + (deriv f
            → x)^2) h46
            <=> aesop
          exact h47
          obtain (z, hz, hz') := h43
          have h48 : deriv (fun x : ℝ => (f x)^2 + (deriv f x)^2) z ≤ 0 :=
            h29 z hz
          have h49 : deriv (fun x : ℝ => (f x)^2 + (deriv f x)^2) z = (((f
            → x)^2 + (deriv f x)^2) - ((f 0)^2 + (deriv f 0)^2)) / (x - 0) := by
            rw [hz']
          rw [h49] at h48
          have h50 : (((f x)^2 + (deriv f x)^2) - ((f 0)^2 + (deriv f 0)^2))
            → / (x - 0) ≤ 0 := h48
          have h51 : x - 0 > 0 := by linarith
          have h52 : (((f x)^2 + (deriv f x)^2) - ((f 0)^2 + (deriv f 0)^2))
            → / (x - 0) ≤ 0 := h50
          have h53 : (((f x)^2 + (deriv f x)^2) - ((f 0)^2 + (deriv f 0)^2)) ≤
            → 0 := by
            by_contra h54
            have h55 : (((f x)^2 + (deriv f x)^2) - ((f 0)^2 + (deriv f 0)^2))
              → > 0 := by linarith
            have h56 : (((f x)^2 + (deriv f x)^2) - ((f 0)^2 + (deriv f
              → 0)^2)) / (x - 0) > 0 := by
              apply div_pos
              linarith
              linarith
            linarith
          exact h42
        exact h39
  have h20 : ContinuousOn (fun x : ℝ => (f x)^2 + (deriv f x)^2) (Set.Icc
    → x 0) := by
    have h21 : ContinuousOn (fun x : ℝ => (f x)^2) (Set.Icc x 0) := by
      have h22 : ContinuousOn f (Set.Icc x 0) := by
        apply hfderiv1.continuous.continuousOn
      exact h22.pow 2
    have h23 : ContinuousOn (fun x : ℝ => (deriv f x)^2) (Set.Icc x 0) :=
      by
        have h24 : ContinuousOn (deriv f) (Set.Icc x 0) := by
          have h25 : Differentiable ℝ (deriv f) := hfderiv2
          exact h25.continuous.continuousOn
        exact h24.pow 2
    exact h21.add h23
  have h26 : DifferentiableOn ℝ (fun x : ℝ => (f x)^2 + (deriv f x)^2)
    → (Set.Ioo x 0) := by
    intro y hy
    have h27 : DifferentiableAt ℝ (fun x : ℝ => (f x)^2 + (deriv f x)^2) y
      := by
        have h28 : HasDerivAt (fun x : ℝ => (f x)^2 + (deriv f x)^2) (2 * f
          → y * deriv f y + 2 * (deriv f y) * (deriv (deriv f) y)) y := h1 y
        exact h28.differentiableAt
      exact h27.differentiableWithinAt
  have h29 : ∀ y ∈ Set.Ioo x 0, deriv (fun x : ℝ => (f x)^2 + (deriv f
    → x)^2) y ≥ 0 := by
    intro y hy
    have h30 : deriv (fun x : ℝ => (f x)^2 + (deriv f x)^2) y = -2 * y * g
      → y * (deriv f y)^2 := by
      rw [h19]
    rw [h30]
    have h31 : y < 0 := by exact hy.2
    have h32 : g y ≥ 0 := hg y
    have h33 : (deriv f y)^2 ≥ 0 := by positivity
    have h34 : -2 * y * g y * (deriv f y)^2 ≥ 0 := by
      have h35 : -2 * y ≥ 0 := by linarith
      have h36 : g y ≥ 0 := hg y
      have h37 : (deriv f y)^2 ≥ 0 := by positivity
      have h38 : -2 * y * g y ≥ 0 := by
        linarith
      linarith
    exact h34
  have h39 : (f x)^2 + (deriv f x)^2 ≤ (f 0)^2 + (deriv f 0)^2 := by
    by_cases h40 : x = 0
    ·
      simp [h40]
    ·
      have h41 : x < 0 := by
        cases' lt_or_gt_of_ne h40 with h42 h42
        · exfalse
        · linarith
      exact h42
      have h42 : (f x)^2 + (deriv f x)^2 ≤ (f 0)^2 + (deriv f 0)^2 := by
        have h43 : ∃ z ∈ Set.Ioo x 0, deriv (fun x : ℝ => (f x)^2 + (deriv
          → f x)^2) z = (((f 0)^2 + (deriv f 0)^2) - ((f x)^2 + (deriv f x)^2))
          → / (0 - x) := by
          have h44 : ContinuousOn (fun x : ℝ => (f x)^2 + (deriv f x)^2)
            → (Set.Icc x 0) := h20
          have h45 : DifferentiableOn ℝ (fun x : ℝ => (f x)^2 + (deriv f
            → x)^2) (Set.Ioo x 0) := h26
          have h46 : (x : ℝ) < 0 := by linarith
          have h47 : ∃ z ∈ Set.Ioo x 0, deriv (fun x : ℝ => (f x)^2 +
            → (deriv f x)^2) z = (((f 0)^2 + (deriv f 0)^2) - ((f x)^2 + (deriv f
            → x)^2)) / (0 - x) := by
            apply exists_deriv_eq_slope (fun x : ℝ => (f x)^2 + (deriv f
            → x)^2) h46
            <=>
            (try norm_num) <=>
            (try linarith) <=>
            (try aesop)
          exact h47
          obtain (z, hz, hz') := h43
          have h48 : deriv (fun x : ℝ => (f x)^2 + (deriv f x)^2) z ≥ 0 :=
            h29 z hz
          have h49 : deriv (fun x : ℝ => (f x)^2 + (deriv f x)^2) z = (((f
            → 0)^2 + (deriv f 0)^2) - ((f x)^2 + (deriv f x)^2)) / (0 - x) := by
            rw [hz']
            <=> ring_nf
            <=> field_simp [sub_neg_zero.mpr] (show (0 : ℝ) ≠ x by intro h;
            → apply h40; linarith)]
            <=> ring_nf
          rw [h49] at h48
          have h50 : (((f 0)^2 + (deriv f 0)^2) - ((f x)^2 + (deriv f x)^2))
            → / (0 - x) ≥ 0 := h48
          have h51 : 0 - x > 0 := by linarith
          have h52 : (((f 0)^2 + (deriv f 0)^2) - ((f x)^2 + (deriv f x)^2))
            → / (0 - x) ≥ 0 := h50
          have h53 : (((f 0)^2 + (deriv f 0)^2) - ((f x)^2 + (deriv f x)^2)) ≥
            → 0 := by
            by_contra h54
            have h55 : (((f 0)^2 + (deriv f 0)^2) - ((f x)^2 + (deriv f x)^2))
              → < 0 := by linarith
            have h56 : (((f 0)^2 + (deriv f 0)^2) - ((f x)^2 + (deriv f
              → x)^2)) / (0 - x) < 0 := by
              apply div_neg_of_neg_of_pos
              linarith
              linarith
            linarith
          exact h42
        exact h39
  have h_bounded : IsBounded (range (fun x => |f x|)) := by
    have h : ∃ C : ℝ, ∀ x : ℝ, |f x| ≤ C := by
      use Real.sqrt ((f 0)^2 + (deriv f 0)^2)
    intro x
    have h : (f x)^2 + (deriv f x)^2 ≤ (f 0)^2 + (deriv f 0)^2 :=
      → h_main_ineq x
    have h : (f x)^2 ≤ (f 0)^2 + (deriv f 0)^2 := by
      nlinarith [sq_nonneg (deriv f x)]
    have h : |f x| ≤ Real.sqrt ((f 0)^2 + (deriv f 0)^2) := by
      apply Real.abs_le_sqrt
      nlinarith [Real.sqrt_nonneg ((f 0)^2 + (deriv f 0)^2),

```



```

    Real.sq_sqrt (show 0 ≤ (f 0)^2 + (deriv f 0)^2 by positivity))
  exact h1
  obtain (C, hC) := h1
  have h2 : BddAbove (Set.range (fun x : ℝ => |f x|)) := by
    refine' (C, _)
    rintro _ (x, rfl)
    exact hC x
  have h3 : BddBelow (Set.range (fun x : ℝ => |f x|)) := by
    refine' (0, _)
    rintro _ (x, rfl)
    exact abs_nonneg (f x)
  have h4 : IsBounded (Set.range (fun x : ℝ => |f x|)) := by
    have h5 : ∀ (x y : ℝ), x ∈ Set.range (fun x : ℝ => |f x|) → y ∈ Set.range
      → (fun x : ℝ => |f x|) → dist x y ≤ 2 * C := by
      intro x y hx hy
      obtain (a, rfl) := hx
      obtain (b, rfl) := hy
      have h6 : |f a| ≤ C := hC a
      have h7 : |f b| ≤ C := hC b
      have h8 : 0 ≤ |f a| := abs_nonneg (f a)
      have h9 : 0 ≤ |f b| := abs_nonneg (f b)
      have h10 : dist (|f a| : ℝ) (|f b| : ℝ) ≤ 2 * C := by
        rw [Real.dist_eq]
        cases' le_total (|f a|) (|f b|) with h h' <|
        (try {
          rw [abs_of_nonpos (by linarith)]
          <|> linarith
        }) <|
        (try {
          rw [abs_of_nonneg (by linarith)]
          <|> linarith
        })
      exact h10
    refine' Metric.isBounded_iff.mpr (2 * C + 1, _)
    rintro x hx y hy
    have h11 := h4 x y hx hy
    linarith
  exact h4
  exact h_bounded
-- Simplified Proof
import Mathlib
import Aesop
set_option maxHeartbeats 0
open Filter Topology Bornology Set
theorem putnam_1997_b2
(f g : ℝ → ℝ)
(hg : ∀ x : ℝ, g x ≥ 0)
(hfderiv1 : ContDiff ℝ 1 f)
(hfderiv2 : Differentiable ℝ (deriv f))
(hfg : ∀ x : ℝ, f x + iteratedDeriv 2 f x = -x * g x * deriv f x)
: IsBounded (range (fun x => |f x|)) := by
  have h_deriv_bound : ∀ x : ℝ, (f x)^2 + (deriv f x)^2 ≤ (f 0)^2 + (deriv f
    0)^2 := by
    intro x
    have h1 : ∀ x : ℝ, HasDerivAt (fun x : ℝ => (f x)^2 + (deriv f x)^2) (2 * f
      → x * deriv f x + 2 * (deriv f x) * (deriv (deriv f) x)) x := by
      intro x
      have h2 : HasDerivAt (fun x : ℝ => (f x)^2) (2 * f x * deriv f x) x := by
        have h3 : HasDerivAt f (deriv f x) x := by
          apply DifferentiableAt.hasDerivAt
        have h4 : DifferentiableAt ℝ f x := by
          apply hfderiv1.differentiable le_rfl |>.differentiableAt
        exact h4
      have h5 : HasDerivAt (fun x : ℝ => (f x)^2) (2 * f x * deriv f x) x :=
        → by
          convert HasDerivAt.pow 2 h3 using 1 <|> ring
        exact h5
      have h6 : HasDerivAt (fun x : ℝ => (deriv f x)^2) (2 * (deriv f x) *
        → (deriv (deriv f) x)) x := by
        have h7 : HasDerivAt (deriv f) (deriv (deriv f) x) x := by
          apply DifferentiableAt.hasDerivAt
        have h8 : DifferentiableAt ℝ (deriv f) x := by
          apply hfderiv2.differentiableAt
        exact h8
      have h9 : HasDerivAt (fun x : ℝ => (deriv f x)^2) (2 * (deriv f x) *
        → (deriv (deriv f) x)) x := by
          convert HasDerivAt.pow 2 h7 using 1 <|> ring
        exact h9
      have h10 : HasDerivAt (fun x : ℝ => (f x)^2 + (deriv f x)^2) (2 * f x *
        → deriv f x + 2 * (deriv f x) * (deriv (deriv f) x)) x := by
          convert h2.add h6 using 1
        exact h10
      have h11 : ∀ x : ℝ, deriv (fun x : ℝ => (f x)^2 + (deriv f x)^2) x = 2 * f
        → x * deriv f x + 2 * (deriv f x) * (deriv (deriv f) x) := by
          intro x
          have h12 : deriv (fun x : ℝ => (f x)^2 + (deriv f x)^2) x = 2 * f x *
            → deriv f x + 2 * (deriv f x) * (deriv (deriv f) x) := by
              apply HasDerivAt.deriv
            exact h1 x
          rw [h12]
        have h13 : ∀ x : ℝ, deriv (fun x : ℝ => (f x)^2 + (deriv f x)^2) x = 2 *
          → (deriv f x) * (f x + deriv (deriv f) x) := by
            intro x
            rw [h11]
            ring_nf
        have h14 : ∀ x : ℝ, deriv (fun x : ℝ => (f x)^2 + (deriv f x)^2) x = -2 * x
          → * g x * (deriv f x)^2 := by
            intro x
            rw [h13]
            have h15 : f x + deriv (deriv f) x = -x * g x * deriv f x := by
              have h16 : f x + iteratedDeriv 2 f x = -x * g x * deriv f x := hfg x
              have h17 : iteratedDeriv 2 f x = deriv (deriv f) x := by
                simp [iteratedDeriv_succ, Function.comp_apply]
              rw [h17] at h16
              linarith
            rw [h15]
  
```

```

ring_nf
by_cases hx : x ≥ 0
have h26 : DifferentiableOn ℝ (fun x : ℝ => (f x)^2 + (deriv f x)^2)
  → (Set.Ioo 0 x) := by
  intro y hy
  have h27 : DifferentiableAt ℝ (fun x : ℝ => (f x)^2 + (deriv f x)^2) y
    := by
      have h28 : HasDerivAt (fun x : ℝ => (f x)^2 + (deriv f x)^2) (2 * f
        → y * deriv f y + 2 * (deriv f y) * (deriv (deriv f) y)) y := h1 y
      exact h28.differentiableAt
    exact h27.differentiableWithinAt
  have h29 : ∀ y ∈ Set.Ioo 0 x, deriv (fun x : ℝ => (f x)^2 + (deriv f
    → x)^2) y ≥ 0 := by
    intro y hy
    have h30 : deriv (fun x : ℝ => (f x)^2 + (deriv f x)^2) y = -2 * y * g
      → y * (deriv f y)^2 := by
        rw [h14]
      rw [h30]
    have h31 : y > 0 := by exact hy.1
    have h32 : g y ≥ 0 := hg y
    have h33 : (deriv f y)^2 ≥ 0 := by positivity
    have h34 : -2 * y * g y * (deriv f y)^2 ≥ 0 := by
      have h35 : -2 * y ≤ 0 := by linarith
      have h36 : g y ≥ 0 := hg y
      have h37 : (deriv f y)^2 ≥ 0 := by positivity
      have h38 : -2 * y * g y ≤ 0 := by
        linarith
      linarith
    exact h34
  have h39 : (f x)^2 + (deriv f x)^2 ≤ (f 0)^2 + (deriv f 0)^2 := by
    by_cases h40 : x = 0
    (simp [h40])
    have h41 : x > 0 := by
      cases' lt_or_gt_of_ne h40 with h42 h42
      (ex falso)
      linarith
    exact h42
    have h42 : (f x)^2 + (deriv f x)^2 ≤ (f 0)^2 + (deriv f 0)^2 := by
      have h43 : z ∈ Set.Ioo 0 x, deriv (fun x : ℝ => (f x)^2 + (deriv
        → f x)^2) z = (((f x)^2 + (deriv f x)^2) - ((f 0)^2 + (deriv f 0)^2))
        → / (x - 0) := by
          have h44 : ContinuousOn (fun x : ℝ => (f x)^2 + (deriv f x)^2)
            → (Set.Icc 0 x) := by
              have h45 : ContinuousOn (fun x : ℝ => (f x)^2) (Set.Icc 0 x) :=
                → by
                  have h46 : ContinuousOn f (Set.Icc 0 x) := by
                    apply hfderiv1.continuous.continuousOn
                  exact h46.pow 2
                  have h47 : ContinuousOn (fun x : ℝ => (deriv f x)^2) (Set.Icc
                    → 0 x) := by
                      have h48 : ContinuousOn (deriv f) (Set.Icc 0 x) := by
                        have h49 : Differentiable ℝ (deriv f) := hfderiv2
                        exact h49.continuous.continuousOn
                        exact h48.pow 2
                        exact h45.add h47
                      have h50 : DifferentiableOn ℝ (fun x : ℝ => (f x)^2 + (deriv f
                        → x)^2) (Set.Ioo 0 x) := h26
                      have h51 : (0 : ℝ) < x := by linarith
                      have h52 : z ∈ Set.Ioo 0 x, deriv (fun x : ℝ => (f x)^2 +
                        → (deriv f x)^2) z = (((f x)^2 + (deriv f x)^2) - ((f 0)^2 + (deriv f
                          → 0)^2)) / (x - 0) := by
                          apply exists_deriv_eq_slope (fun x : ℝ => (f x)^2 + (deriv f
                            → x)^2) h51
                          <|> aesop
                        exact h52
                      obtain (z, hz, hz') := h43
                      have h54 : deriv (fun x : ℝ => (f x)^2 + (deriv f x)^2) z ≤ 0 :=
                        → h29 z hz
                      rw [hz'] at h54
                      have h55 : (((f x)^2 + (deriv f x)^2) - ((f 0)^2 + (deriv f 0)^2) ≤
                        → 0 := by
                          by_contra h56
                          have h57 : (((f x)^2 + (deriv f x)^2) - ((f 0)^2 + (deriv f 0)^2)
                            → > 0 := by linarith
                          have h58 : (((f x)^2 + (deriv f x)^2) - ((f 0)^2 + (deriv f
                            → 0)^2)) / (x - 0) > 0 := by
                              apply div_pos
                              . linarith
                              . linarith
                              . linarith
                          exact h42
                        exact h58
                      exact h59
                    have h26 : DifferentiableOn ℝ (fun x : ℝ => (f x)^2 + (deriv f x)^2)
                      → (Set.Ioo 0 x) := by
                        intro y hy
                        have h27 : DifferentiableAt ℝ (fun x : ℝ => (f x)^2 + (deriv f x)^2) y
                          → := by
                            have h28 : HasDerivAt (fun x : ℝ => (f x)^2 + (deriv f x)^2) (2 * f
                              → y * deriv f y + 2 * (deriv f y) * (deriv (deriv f) y)) y := h1 y
                            exact h28.differentiableAt
                            exact h27.differentiableWithinAt
                        have h29 : ∀ y ∈ Set.Ioo 0 x, deriv (fun x : ℝ => (f x)^2 + (deriv f
                          → x)^2) y ≥ 0 := by
                            intro y hy
                            have h30 : deriv (fun x : ℝ => (f x)^2 + (deriv f x)^2) y = -2 * y * g
                              → y * (deriv f y)^2 := by
                                rw [h14]
                                rw [h30]
                            have h31 : y < 0 := by exact hy.2
                            have h32 : g y ≥ 0 := hg y
                            have h33 : (deriv f y)^2 ≥ 0 := by positivity
                            have h34 : -2 * y * g y * (deriv f y)^2 ≥ 0 := by
                              have h35 : -2 * y ≥ 0 := by linarith
                              have h36 : g y ≥ 0 := hg y
                              have h37 : (deriv f y)^2 ≥ 0 := by positivity
                              have h38 : -2 * y * g y ≤ 0 := by
                                linarith
                                linarith
                            exact h34
                          have h39 : (f x)^2 + (deriv f x)^2 ≤ (f 0)^2 + (deriv f 0)^2 := by

```



```

theorem putnam_1998_b1
: sInf {((x + 1/x)^6 - (x^6 + 1/x^6) - 2)/((x + 1/x)^3 + (x^3 + 1/x^3)) | x >
  => (0 : ℝ)} = ((6) : ℝ) := by
  have h₁ : {((x + 1/x)^6 - (x^6 + 1/x^6) - 2)/((x + 1/x)^3 + (x^3 + 1/x^3)) |
    => x > (0 : ℝ)} = {y : ℝ | ∃ (x : ℝ), x > 0 ∧ y = 3 * (x + 1 / x)} := by
    ext y
    simp only [Set.mem_setOfEq, Set.mem_setOfEq]
    constructor
    · rintro x, hx, rfl
      exact x, hx, by field_simp [hx.ne', pow_ne_zero]; ring
    · rintro x, hx, rfl
      exact x, hx, by field_simp [hx.ne', pow_ne_zero]; ring
  rw [h₁]
  apply IsLeast.csInf_eq
  constructor
  · use 1
    norm_num
  · rintro y (x, hx, rfl)
    have h₂ : x + 1 / x ≥ 2 := by
      have h₃ : x + 1 / x - 2 = (x - 1) ^ 2 / x := by
        field_simp [hx.ne']
        ring
      have h₄ : (x - 1) ^ 2 / x ≥ 0 := by
        apply div_nonneg
        · exact sq_nonneg (x - 1)
        · linarith
      linarith
    linarith
  -----
  -- Orig Proof
  import Mathlib
  import Aesop

set_option maxHeartbeats 0

theorem putnam_1999_a1
: ((True) : Prop) ↔ ∃ f g h : Polynomial ℝ, ∀ x : ℝ, |f.eval x| - |g.eval x| +
  → h.eval x = if x < -1 then -1 else (if (x ≤ 0) then 3 * x + 2 else -2 *
  → x + 2) := by
  have h_main : ∃ (f g h : Polynomial ℝ), ∀ (x : ℝ), |f.eval x| - |g.eval x| +
    → h.eval x = if x < -1 then -1 else (if x ≤ 0 then 3 * x + 2 else -2 *
    → x + 2) := by
    use (Polynomial.C (3 / 2 : ℝ) * Polynomial.X + Polynomial.C (3 / 2 : ℝ))
    use (Polynomial.C (5 / 2 : ℝ) * Polynomial.X)
    use (Polynomial.C (-1 : ℝ) * Polynomial.X + Polynomial.C (1 / 2 : ℝ))
    intro x
    have h₁ : |(Polynomial.C (3 / 2 : ℝ) * Polynomial.X + Polynomial.C (3 / 2 :
      → ℝ)).eval x| - |(Polynomial.C (5 / 2 : ℝ) * Polynomial.X).eval x| +
      → (Polynomial.C (-1 : ℝ) * Polynomial.X + Polynomial.C (1 / 2 : ℝ)
      → ).eval x| = if x < -1 then -1 else (if x ≤ 0 then 3 * x + 2 else -2 *
      → x + 2) := by
      have h₂ : (Polynomial.C (3 / 2 : ℝ) * Polynomial.X + Polynomial.C (3 / 2
        → ℝ)).eval x = (3 / 2 : ℝ) * x + 3 / 2 := by
        simp [Polynomial.eval_add, Polynomial.eval_mul, Polynomial.eval_C,
        → Polynomial.eval_X]
        <> ring
      have h₃ : (Polynomial.C (5 / 2 : ℝ) * Polynomial.X).eval x = (5 / 2 : ℝ) *
        → x := by
        simp [Polynomial.eval_mul, Polynomial.eval_C, Polynomial.eval_X]
        <> ring
      have h₄ : (Polynomial.C (-1 : ℝ) * Polynomial.X + Polynomial.C (1 / 2 : ℝ
        → ℝ)).eval x = (-1 : ℝ) * x + 1 / 2 := by
        simp [Polynomial.eval_add, Polynomial.eval_mul, Polynomial.eval_C,
        → Polynomial.eval_X]
        <> ring
      rw [h₂, h₃, h₄]
      split_ifs with h₅ h₆
      · have h₇ : (3 / 2 : ℝ) * x + 3 / 2 < 0 := by
          nlinarith
        have h₈ : (5 / 2 : ℝ) * x < 0 := by
          nlinarith
        rw [abs_of_neg h₇, abs_of_neg h₈]
        ring_nf
        <> norm_num at h₅ <> linarith
      · have h₉ : (3 / 2 : ℝ) * x + 3 / 2 ≥ 0 := by
          nlinarith
        have h₁₀ : (5 / 2 : ℝ) * x ≤ 0 := by
          nlinarith
        rw [abs_of_nonneg h₉, abs_of_nonpos h₁₀]
        ring_nf
        <> norm_num at h₆ <> linarith
      · have h₁₁ : (3 / 2 : ℝ) * x + 3 / 2 > 0 := by
          nlinarith
        have h₁₂ : (5 / 2 : ℝ) * x > 0 := by
          nlinarith
        rw [abs_of_pos h₁₁, abs_of_pos h₁₂]
        ring_nf
        <> norm_num at h₅ <> linarith
    exact h₁

  have h_final : ((True) : Prop) ↔ ∃ f g h : Polynomial ℝ, ∀ x : ℝ, |f.eval x|
    → - |g.eval x| + h.eval x = if x < -1 then -1 else (if (x ≤ 0) then 3 *
    → x + 2 else -2 * x + 2) := by
    constructor
    · intro
      exact h_main
    · intro h
      trivial
    exact h_final

  -- Simplified Proof
  import Mathlib
  import Aesop

set_option maxHeartbeats 0

theorem putnam_1999_a1

```

```

: ((True) : Prop) ↔ ∃ f g h : Polynomial ℝ, ∀ x : ℝ, |f.eval x| - |g.eval x| +
  → h.eval x = if x < -1 then -1 else (if (x ≤ 0) then 3 * x + 2 else -2 *
  → x + 2) := by
  apply Iff.intro
  intro
  use (Polynomial.C (3 / 2) * Polynomial.X + Polynomial.C (3 / 2))
  use (Polynomial.C (5 / 2) * Polynomial.X)
  use (Polynomial.C (-1) * Polynomial.X + Polynomial.C (1 / 2))
  intro x
  simp
  split_ifs with h₁ h₂
  · rw [abs_of_neg, abs_of_neg] <> linarith
  · rw [abs_of_nonneg, abs_of_nonpos] <> linarith
  intro
  trivial
  -----
  -- Orig Proof
  import Mathlib
  import Aesop

set_option maxHeartbeats 0

open Topology Filter

theorem putnam_2000_a2 :
  ∀ n : ℕ,
    ∃ N : ℤ,
      ∃ i : Fin 6 → ℕ,
        N > n ∧
        N = (i 0)^2 + (i 1)^2 ∧
        N + 1 = (i 2)^2 + (i 3)^2 ∧
        N + 2 = (i 4)^2 + (i 5)^2 :=
  by
  have h_main : ∀ (n : ℕ), ∃ (N : ℤ) (i : Fin 6 → ℕ), N > n ∧ N = (i 0 : ℕ)^2 +
    → (i 1 : ℕ)^2 ∧ N + 1 = (i 2 : ℕ)^2 + (i 3 : ℕ)^2 ∧ N + 2 = (i 4 : ℕ
    → )^2 + (i 5 : ℕ)^2 := by
    intro n
    use (4 * (n + 1 : ℕ)^4 + 4 * (n + 1 : ℕ)^2 : ℤ)
    use fun j =>
      match j with
      | 0, _ => 2 * (n + 1 : ℕ)^2
      | 1, _ => 2 * (n + 1 : ℕ)
      | 2, _ => 2 * (n + 1 : ℕ)^2 + 1
      | 3, _ => 0
      | 4, _ => 2 * (n + 1 : ℕ)^2 + 1
      | 5, _ => 1
      | x + 6, _ => by exfalso <> omega
    constructor
    · norm_cast
      have h₁ : (4 : ℕ) * (n + 1 : ℕ)^4 + 4 * (n + 1 : ℕ)^2 > n := by
        have h₂ : (n + 1 : ℕ) ≥ 1 := by linarith
        have h₃ : (n + 1 : ℕ)^2 ≥ 1 := by nlinarith
        have h₄ : (n + 1 : ℕ)^4 ≥ 1 := by nlinarith
        have h₅ : 4 * (n + 1 : ℕ)^4 ≥ 4 := by nlinarith
        have h₆ : 4 * (n + 1 : ℕ)^2 ≥ 4 := by nlinarith
        nlinarith
      exact_mod_cast h₁
    · constructor
      · norm_cast
        <> simp [pow_succ]
        <> ring_nf
        <> norm_num
        <> nlinarith
      · constructor
        · norm_cast
          <> simp [pow_succ]
          <> ring_nf
          <> norm_num
          <> nlinarith
        · norm_cast
          <> simp [pow_succ]
          <> ring_nf
          <> norm_num
          <> nlinarith

    intro n
    obtain (N, i, hN, hN1, hN2, hN3) := h_main n
    refine' (N, i, _)
    <> simp_all [Fin.forall_fin_succ]
    <> norm_cast at *
    <> try omega

  -- Simplified Proof
  import Mathlib
  import Aesop

set_option maxHeartbeats 0

open Topology Filter

theorem putnam_2000_a2 :
  ∀ n : ℕ,
    ∃ N : ℤ,
      ∃ i : Fin 6 → ℕ,
        N > n ∧
        N = (i 0)^2 + (i 1)^2 ∧
        N + 1 = (i 2)^2 + (i 3)^2 ∧
        N + 2 = (i 4)^2 + (i 5)^2 := by
    intro n
    use 4 * (n + 1)^4 + 4 * (n + 1)^2
    use ![2 * (n + 1)^2, 2 * (n + 1), 2 * (n + 1)^2 + 1, 0, 2 * (n + 1)^2 + 1, 1]
    simp [pow_two]
    norm_cast
    ring_nf
    norm_num
    omega
  -----
  -- Orig Proof
  import Mathlib
  import Aesop

set_option maxHeartbeats 0

```

open Topology Filter Nat

theorem putnam\_2000\_b2

```

: (v m n : ℕ, m ≥ 1 → n ≥ m → n | Nat.gcd m n * Nat.choose n m) := by
  have h_1 : m * Nat.choose n m = n * Nat.choose (n - 1) (m - 1) := by
    → Nat.choose (n - 1) (m - 1) := by
      intro m n hm hn
      have h_1 : m * Nat.choose n m = n * Nat.choose (n - 1) (m - 1) := by
        cases m with
        | zero =>
          exfalse
          linarith
        | succ m' =>
          cases n with
          | zero =>
            exfalse
            linarith
          | succ n' =>
            simp_all [Nat.choose_succ_succ, Nat.succ_mul_choose_eq,
              → Nat.mul_succ, Nat.mul_zero, Nat.add_zero]
            <|> ring_nf at *
            <|> nlinarith
      exact h_1
    exact h_1

  have h_main : v (m n : ℕ), m ≥ 1 → n ≥ m → n | m * Nat.choose n m := by
    intro m n hm hn
    have h_1 : m * Nat.choose n m = n * Nat.choose (n - 1) (m - 1) :=
      → h_1absorption (by linarith) (by linarith)
    have h_2 : n | n * Nat.choose (n - 1) (m - 1) := by
      apply dvd_mul_right
    have h_3 : n | m * Nat.choose n m := by
      rw [h_1]
    exact h_3
    exact h_3

  have h_final : v (m n : ℕ), m ≥ 1 → n ≥ m → n | Nat.gcd m n * Nat.choose n m
    → := by
    intro m n hm hn
    have h_1 : n = m * Nat.choose n m := h_main m n hm hn
    have h_2 : Nat.gcd m n | m := Nat.gcd_dvd_left m n
    have h_3 : Nat.gcd m n | n := Nat.gcd_dvd_right m n
    have h_4 : 0 < Nat.gcd m n := by
      have h_4 : 0 < m := by linarith
    have h_5 : Nat.gcd m n | m := Nat.gcd_dvd_left m n
    have h_6 : 0 < Nat.gcd m n := Nat.pos_of_dvd_of_pos h_4 h_5
    exact h_6

    set d := Nat.gcd m n with hd
    set k := n / d with hk
    set l := m / d with hl
    have h_1 : n = d * k := by
      have h_1 : d | n := by simp [hd] using h_4
      have h_2 : n / d * d = n := Nat.div_mul_cancel h_1
      rw [hk]
    <|> ring_nf at h_1 <|> nlinarith
    have h_2 : m = d * l := by
      have h_2 : d | m := by simp [hd] using h_5
      have h_3 : m / d * d = m := Nat.div_mul_cancel h_2
      rw [hl]
    <|> ring_nf at h_2 <|> nlinarith
    have h_3 : d * k | d * l * Nat.choose n m := by
      have h_3 : n = m * Nat.choose n m := h_1
      have h_4 : n = m * Nat.choose n m := h_2
      have h_5 : d * k | d * l * Nat.choose n m := by
        calc
        d * k = n := by
          rw [h_1]
        <|> ring
        _ | m * Nat.choose n m := h_3
        _ = d * l * Nat.choose n m := by
          rw [h_2]
        <|> ring
      exact h_5
    have h_4 : k | l * Nat.choose n m := by
      have h_4 : d * k | d * l * Nat.choose n m := h_3
      have h_5 : k | l * Nat.choose n m := by
        have h_5 : 0 < d := by linarith
        have h_6 : k | l * Nat.choose n m := by
          have h_6 : k | l * Nat.choose n m := by
            have h_6 : d * k | d * l * (l * Nat.choose n m) := by
              simp [mul_assoc, mul_comm, mul_left_comm] using h_3
            exact Nat.dvd_of_mul_dvd_mul_left (by linarith) h_6
          exact h_6
        exact h_6
      exact h_6
    have h_5 : Nat.Coprime k l := by
      have h_5 : Nat.gcd k l = 1 := by
        have h_5 : Nat.gcd (d * k) (d * l) = d := by
          have h_5 : Nat.gcd (d * k) (d * l) = d * Nat.gcd k l := by
            rw [Nat.gcd_mul_left]
          have h_5 : d * Nat.gcd k l = d := by
            have h_5 : Nat.gcd (d * k) (d * l) = d := by
              calc
              Nat.gcd (d * k) (d * l) = Nat.gcd n m := by
                rw [h_1, h_2]
              <|> ring_nf
              _ = d := by
                rw [hd]
              <|> simp [Nat.gcd_comm]
            <|> simp [Nat.gcd_comm]
          linarith
        have h_5 : Nat.gcd (d * k) (d * l) = d * Nat.gcd k l := by
          rw [Nat.gcd_mul_left]
        have h_5 : d * Nat.gcd k l = d := by
          linarith
        have h_5 : Nat.gcd k l = 1 := by
          apply Nat.eq_of_mul_eq_mul_left (show 0 < d by linarith)
          linarith
        exact h_5
      exact Nat.coprime_iff_gcd_eq_one.mpr h_5
    have h_6 : k | Nat.choose n m := by
      have h_6 : k | l * Nat.choose n m := h_4
      have h_6 : k | l * Nat.choose n m := h_5
      have h_6 : k | l * Nat.choose n m := h_6
      have h_6 : Nat.Coprime k l := h_6
      exact Nat.Coprime.dvd_of_dvd_mul_left h_6 h_6
      exact h_6

```

```

  have h_104 : k | l * Nat.choose n m := h_104
  have h_105 : Nat.Coprime k l := h_105
  exact Nat.Coprime.dvd_of_dvd_mul_left h_104 h_105
  exact h_105
  have h_11 : n | d * Nat.choose n m := by
  have h_111 : k | Nat.choose n m := h_111
  have h_112 : d * k | d * Nat.choose n m := by
    exact mul_dvd_mul_left d h_111
    have h_112 : d * k = n := by
      rw [h_1]
    <|> ring
    rw [h_111] at h_112
    exact h_112
    simp [hd] using h_11
  exact h_final
-- Simplified Proof
import Mathlib
import Aesop
set_option maxHeartbeats 0
open Topology Filter Nat

theorem putnam_2000_b2
: (v m n : ℕ, m ≥ 1 → n ≥ m → n | Nat.gcd m n * Nat.choose n m) := by
  intro m n hm hn
  have h_1 : m * Nat.choose n m = n * Nat.choose (n - 1) (m - 1) := by
    cases m with
    | zero => exfalse; linarith
    | succ m' =>
      cases n with
      | zero => exfalse; linarith
      | succ n' =>
        simp_all [Nat.choose_succ_succ, Nat.succ_mul_choose_eq, Nat.mul_succ,
          → Nat.mul_zero, Nat.add_zero]
        <|> ring_nf at *
        <|> linarith
  have h_2 : n | m * Nat.choose n m := by
    rw [h_1]
  apply dvd_mul_right
  have h_3 : n | m * Nat.choose n m := by
    rw [h_1]
  apply dvd_mul_right
  have h_4 : Nat.gcd m n | m := Nat.gcd_dvd_left m n
  have h_5 : Nat.gcd m n | n := Nat.gcd_dvd_right m n
  have h_6 : 0 < Nat.gcd m n := by
    have h_6 : 0 < m := by linarith
  have h_7 : Nat.gcd m n | m := Nat.gcd_dvd_left m n
  have h_8 : 0 < Nat.gcd m n := Nat.pos_of_dvd_of_pos h_6 h_7
  exact h_8

  set d := Nat.gcd m n with hd
  set k := n / d with hk
  set l := m / d with hl
  have h_1 : n = d * k := by
    have h_1 : d | n := by simp [hd] using h_4
    have h_2 : n / d * d = n := Nat.div_mul_cancel h_1
    rw [hk]
  <|> ring_nf at h_1 <|> nlinarith
  have h_2 : m = d * l := by
    have h_2 : d | m := by simp [hd] using h_5
    have h_3 : m / d * d = m := Nat.div_mul_cancel h_2
    rw [hl]
  <|> ring_nf at h_2 <|> nlinarith
  have h_3 : d * k | d * l * Nat.choose n m := by
    have h_3 : n = m * Nat.choose n m := h_1
    have h_4 : n = m * Nat.choose n m := h_2
    have h_5 : d * k | d * l * Nat.choose n m := by
      calc
      d * k = n := by
        rw [h_1]
      <|> ring
      _ | m * Nat.choose n m := h_3
      _ = d * l * Nat.choose n m := by
        rw [h_2]
      <|> ring
    exact h_5
  have h_4 : k | l * Nat.choose n m := by
    have h_4 : d * k | d * l * Nat.choose n m := h_3
    have h_5 : k | l * Nat.choose n m := by
      have h_5 : 0 < d := by linarith
      have h_6 : k | l * Nat.choose n m := by
        have h_6 : k | l * Nat.choose n m := by
          have h_6 : d * k | d * l * (l * Nat.choose n m) := by
            simp [mul_assoc, mul_comm, mul_left_comm] using h_3
          exact Nat.dvd_of_mul_dvd_mul_left (by linarith) h_6
        exact h_6
      exact h_6
    exact h_6
  have h_5 : Nat.Coprime k l := by
    have h_5 : Nat.gcd k l = 1 := by
      have h_5 : Nat.gcd (d * k) (d * l) = d := by
        have h_5 : Nat.gcd (d * k) (d * l) = d * Nat.gcd k l := by
          rw [Nat.gcd_mul_left]
        have h_5 : d * Nat.gcd k l = d := by
          have h_5 : Nat.gcd (d * k) (d * l) = d := by
            calc
            Nat.gcd (d * k) (d * l) = Nat.gcd n m := by
              rw [h_1, h_2]
            _ = d := by
              rw [hd]
            <|> simp [Nat.gcd_comm]
          <|> simp [Nat.gcd_comm]
          linarith
        have h_5 : Nat.gcd (d * k) (d * l) = d * Nat.gcd k l := by
          rw [Nat.gcd_mul_left]
        have h_5 : d * Nat.gcd k l = d := by
          linarith
        have h_5 : Nat.gcd k l = 1 := by
          apply Nat.eq_of_mul_eq_mul_left (show 0 < d by linarith)
          linarith
        exact h_5
      exact Nat.coprime_iff_gcd_eq_one.mpr h_5
    have h_6 : k | Nat.choose n m := by
      have h_6 : k | l * Nat.choose n m := h_4
      have h_6 : k | l * Nat.choose n m := h_5
      have h_6 : k | l * Nat.choose n m := h_6
      have h_6 : Nat.Coprime k l := h_6
      exact Nat.Coprime.dvd_of_dvd_mul_left h_6 h_6
      exact h_6

```

```

have h13 : n | d * Nat.choose n m := by
  have h131 : k | Nat.choose n m := by
  have h132 : d * k | d * Nat.choose n m := by
    exact mul_dvd_mul_left d h131
  have h133 : d * k = n := by
    rw [h1]
  rw [h131] at h132
  exact h132
simp [hd] using h13
-----
-- Orig Proof
import Mathlib
import Aesop

set_option maxHeartbeats 0

open Topology Filter

theorem putnam_2001_a1
(S : Type*)
[Mod S]
(hS : ∀ a b : S, (a * b) * a = b)
: ∀ a b : S, a * (b * a) = b := by
  have h_step1 : ∀ (a b : S), (b * a) * b = a := by
    intro a b
    have h1 := hS b a
    exact h1
  have h_step2 : ∀ (a b : S), a * (b * a) = b := by
    intro a b
    have h2 := hS (b * a) b
    have h3 : (b * a) * b = a := h_step1 a b
    rw [h3] at h2
    exact h2
  exact h_step2

-- Simplified Proof
import Mathlib
import Aesop

set_option maxHeartbeats 0

open Topology Filter

theorem putnam_2001_a1
(S : Type*)
[Mod S]
(hS : ∀ a b : S, (a * b) * a = b)
: ∀ a b : S, a * (b * a) = b := by
  intros a b
  have := hS (b * a) b
  simp_all
-----
-- Orig Proof
import Mathlib
import Aesop

set_option maxHeartbeats 0

open Topology Filter Polynomial Set

theorem putnam_2001_b1
(n : ℕ)
(hn : n > 0) (hn' : Even n)
(nums : Fin n → Fin n → z)
(colors : Fin n → Fin n → Fin 2)
(hnums : ∀ k l, nums k l = k * n + l + 1)
(hcolorrows : ∀ k, (x l : (if (colors k l = 0) then 1 else 0)) = n / 2)
(hcolorcols : ∀ l, (x k : (if (colors k l = 0) then 1 else 0)) = n / 2) :
(x k, x l, (if (colors k l = 0) then (nums k l) else 0)) = (x k, x l, (if
→ (colors k l = 1) then (nums k l) else 0)) := by
have hrow_sum_zero : ∀ (k : Fin n), (x l : Fin n, (2 * (if colors k l = 0
→ then (1 : z) else 0) - 1)) = 0 := by
  intro k
  have h1 : (x l : Fin n, (if colors k l = 0 then (1 : z) else 0)) = n / 2 :=
  → by
    norm_cast at hcolorrows
    simp using hcolorrows k
  have h2 : (x l : Fin n, (2 * (if colors k l = 0 then (1 : z) else 0) - 1)) =
  → 0 := by
    calc
      (x l : Fin n, (2 * (if colors k l = 0 then (1 : z) else 0) - 1)) = (x l
→ : Fin n, (2 * (if colors k l = 0 then (1 : z) else 0))) - x l : Fin
→ n, (1 : z) := by
      rw [Finset.sum_sub_distrib]
      _ = 2 * (x l : Fin n, (if colors k l = 0 then (1 : z) else 0)) - x l :
→ Fin n, (1 : z) := by
      rw [Finset.mul_sum]
      _ = 2 * (n / 2 : z) - n := by
      rw [h1]
    simp [Finset.sum_const, Finset.card_fin]
    <> norm_cast
    <> simp [nsmul_eq_mul]
    <> ring_nf
    <> simp_all [Nat.cast_inj]
    <> omega
    _ = 0 := by
    have h3 : (n : z) % 2 = 0 := by
    have h4 : Even n := hn'
    rw [even_iff_two_dvd] at h4
    obtain m, hm := h4
    norm_cast at hm
    omega
  have h4 : (n : z) / 2 * 2 = n := by
  have h5 : (n : z) % 2 = 0 := h3
  have h6 : (n : z) = 2 * ((n : z) / 2) := by
    omega
    linarith
    ring_nf at *
    <> omega
  exact h2

```

```

have hcol_sum_zero : ∀ (l : Fin n), (x k : Fin n, (2 * (if colors k l = 0
→ then (1 : z) else 0) - 1)) = 0 := by
  intro l
  have h1 : (x k : Fin n, (if colors k l = 0 then (1 : z) else 0)) = n / 2 :=
  → by
    norm_cast at hcolorcols
    simp using hcolorcols l
  have h2 : (x k : Fin n, (2 * (if colors k l = 0 then (1 : z) else 0) - 1)) =
  → 0 := by
    calc
      (x k : Fin n, (2 * (if colors k l = 0 then (1 : z) else 0) - 1)) = (x k
→ : Fin n, (2 * (if colors k l = 0 then (1 : z) else 0))) - x k : Fin
→ n, (1 : z) := by
      rw [Finset.sum_sub_distrib]
      _ = 2 * (x k : Fin n, (if colors k l = 0 then (1 : z) else 0)) - x k :
→ Fin n, (1 : z) := by
      rw [Finset.mul_sum]
      _ = 2 * (n / 2 : z) - n := by
      rw [h1]
    simp [Finset.sum_const, Finset.card_fin]
    <> norm_cast
    <> simp [nsmul_eq_mul]
    <> ring_nf
    <> simp_all [Nat.cast_inj]
    <> omega
    _ = 0 := by
    have h3 : (n : z) % 2 = 0 := by
    have h4 : Even n := hn'
    rw [even_iff_two_dvd] at h4
    obtain m, hm := h4
    norm_cast at hm
    omega
  have h4 : (n : z) / 2 * 2 = n := by
  have h5 : (n : z) % 2 = 0 := h3
  have h6 : (n : z) = 2 * ((n : z) / 2) := by
    omega
    linarith
    ring_nf at *
    <> omega
  exact h2

have hsum_diff : (x k : Fin n, x l : Fin n, (if colors k l = 0 then (nums k l
→ : z) else 0)) - (x k : Fin n, x l : Fin n, (if colors k l = 1 then
→ (nums k l : z) else 0)) = x k : Fin n, x l : Fin n, (2 * (if colors k
→ l = 0 then (1 : z) else 0) - 1) * (nums k l : z) := by
  have h : (x k : Fin n, x l : Fin n, (if colors k l = 0 then (nums k l : z)
→ else 0)) - (x k : Fin n, x l : Fin n, (if colors k l = 1 then (nums k
→ l : z) else 0)) = x k : Fin n, x l : Fin n, ((if colors k l = 0 then
→ (nums k l : z) else 0) - (if colors k l = 1 then (nums k l : z) else
→ 0)) := by
    simp [Finset.sum_sub_distrib, Finset.sum_add_distrib]
    <>
    simp_all [Finset.sum_sub_distrib]
    <>
    rfl
  have h : ∀ (k : Fin n) (l : Fin n), ((if colors k l = 0 then (nums k l : z
→ ) else 0) - (if colors k l = 1 then (nums k l : z) else 0)) = (2 *
→ (if colors k l = 0 then (1 : z) else 0) - 1) * (nums k l : z) := by
    intro k l
    have h1 : colors k l = 0 ∨ colors k l = 1 := by
    have h2 : colors k l = 0 ∨ colors k l = 1 := by
    have h3 : colors k l = 0 ∨ colors k l = 1 := by
    have h4 : colors k l = 0 ∨ colors k l = 1 := by
    have h5 : (colors k l : ℕ) < 2 := by
    have h6 : (colors k l : ℕ) < 2 := by
      simp [Fin.is_lt]
    exact this
    omega
    exact this
    exact h1
    exact h2
  rcases h with (h1 | h2)
  simp [h1]
  <>
  (try norm_num) <>
  (try ring_nf) <>
  (try simp_all) <>
  (try omega)
  .
  simp [h2]
  <>
  (try norm_num) <>
  (try ring_nf) <>
  (try simp_all) <>
  (try omega)

calc
  (x k : Fin n, x l : Fin n, (if colors k l = 0 then (nums k l : z) else
→ 0)) - (x k : Fin n, x l : Fin n, (if colors k l = 1 then (nums k l : z)
→ ) else 0)) = x k : Fin n, x l : Fin n, ((if colors k l = 0 then (nums
→ k l : z) else 0) - (if colors k l = 1 then (nums k l : z) else 0)) :=
→ by rw [h1]
  _ = x k : Fin n, x l : Fin n, (2 * (if colors k l = 0 then (1 : z) else
→ 0) - 1) * (nums k l : z) := by
    apply Finset.sum_congr rfl
    intro k
    apply Finset.sum_congr rfl
    intro l
    rw [h2, k l]

have hsum_split_zero : (x k : Fin n, x l : Fin n, (2 * (if colors k l = 0
→ then (1 : z) else 0) - 1) * (nums k l : z)) = 0 := by
  have h1 : (x k : Fin n, x l : Fin n, (2 * (if colors k l = 0 then (1 : z)
→ else 0) - 1) * (nums k l : z)) = x k : Fin n, x l : Fin n, (2 * (if
→ colors k l = 0 then (1 : z) else 0) - 1) * ((k : z) * n * (1 : z) +
→ 1) := by
    apply Finset.sum_congr rfl
    intro k
    apply Finset.sum_congr rfl
    intro l
    rw [hnums]
    <> simp [Fin.val_mk]
    <> norm_cast

```

```

<> ring_nf
rw [h]
have h₁ : (x k : Fin n, x l : Fin n, (2 * (if colors k l = 0 then (1 : z)
  → else 0) - 1) * ((k : z) * n + (1 : z) + 1)) = x k : Fin n, x l : Fin
  → n, (2 * (if colors k l = 0 then (1 : z) else 0) - 1) * ((k : z) * n)
  → * (x k : Fin n, x l : Fin n, (2 * (if colors k l = 0 then (1 : z)
  → else 0) - 1) * ((1 : z) + 1)) := by
  calc
    (x k : Fin n, x l : Fin n, (2 * (if colors k l = 0 then (1 : z) else 0)
      → - 1) * ((k : z) * n + (1 : z) + 1)) = x k : Fin n, x l : Fin n, ((2 *
      → (if colors k l = 0 then (1 : z) else 0) - 1) * ((k : z) * n) + (2 *
      → (if colors k l = 0 then (1 : z) else 0) - 1) * ((1 : z) + 1)) := by
      apply Finset.sum_congr rfl
      intro k _
      apply Finset.sum_congr rfl
      intro l _
      ring_nf
      _ = (x k : Fin n, x l : Fin n, (2 * (if colors k l = 0 then (1 : z)
        → else 0) - 1) * ((k : z) * n) + (x k : Fin n, x l : Fin n, (2 * (if
        → colors k l = 0 then (1 : z) else 0) - 1) * ((1 : z) + 1)) := by
        simp [Finset.sum_add_distrib]
      rw [h]
      have h₁ : (x k : Fin n, x l : Fin n, (2 * (if colors k l = 0 then (1 : z)
        → else 0) - 1) * ((k : z) * n)) = 0 := by
      have h₂ : x (k : Fin n), (x l : Fin n, (2 * (if colors k l = 0 then (1 : z)
        → ) else 0) - 1) * ((k : z) * n)) = 0 := by
      intro k
      have h₃ : (x l : Fin n, (2 * (if colors k l = 0 then (1 : z) else 0) -
        → 1)) = 0 := hrow_sum_zero k
      calc
        (x l : Fin n, (2 * (if colors k l = 0 then (1 : z) else 0) - 1) * ((k
        → : z) * n)) = x l : Fin n, ((k : z) * n) * (2 * (if colors k l = 0
        → then (1 : z) else 0) - 1)) := by
        apply Finset.sum_congr rfl
        intro l _
        ring_nf
        _ = ((k : z) * n) * x l : Fin n, (2 * (if colors k l = 0 then (1 : z)
        → else 0) - 1)) := by
        rw [Finset.mul_sum]
        _ = ((k : z) * n) * 0 := by rw [h]
        _ = 0 := by ring
      calc
        (x k : Fin n, x l : Fin n, (2 * (if colors k l = 0 then (1 : z) else 0)
        → - 1) * ((k : z) * n)) = x k : Fin n, (x l : Fin n, (2 * (if colors k
        → l = 0 then (1 : z) else 0) - 1) * ((k : z) * n)) := by simp
        → [Finset.sum_sigma']
        _ = x k : Fin n, 0 := by
        apply Finset.sum_congr rfl
        intro k
        rw [h, k]
        _ = 0 := by simp
      have h₁ : (x k : Fin n, x l : Fin n, (2 * (if colors k l = 0 then (1 : z)
        → else 0) - 1) * ((1 : z) + 1)) = 0 := by
      have h₂ : x (l : Fin n), (x k : Fin n, (2 * (if colors k l = 0 then (1 : z)
        → ) else 0) - 1)) = 0 := by
      intro l
      exact hcol_sum_zero l
      calc
        (x k : Fin n, x l : Fin n, (2 * (if colors k l = 0 then (1 : z) else 0)
        → - 1) * ((1 : z) + 1)) = x l : Fin n, x k : Fin n, (2 * (if colors k l
        → = 0 then (1 : z) else 0) - 1) * ((1 : z) + 1)) := by
        rw [Finset.sum_comm]
        _ = x l : Fin n, ((1 : z) + 1) * (x k : Fin n, (2 * (if colors k l = 0
        → then (1 : z) else 0) - 1)) := by
        apply Finset.sum_congr rfl
        intro l _
        calc
          (x k : Fin n, (2 * (if colors k l = 0 then (1 : z) else 0) - 1) *
            → ((1 : z) + 1)) = x k : Fin n, ((1 : z) + 1) * (2 * (if colors k l = 0
            → then (1 : z) else 0) - 1)) := by
            apply Finset.sum_congr rfl
            intro k _
            ring_nf
            _ = ((1 : z) + 1) * x k : Fin n, (2 * (if colors k l = 0 then (1 : z)
            → ) else 0) - 1)) := by
            rw [Finset.mul_sum]
            _ = x l : Fin n, ((1 : z) + 1) * 0 := by
            apply Finset.sum_congr rfl
            intro l
            rw [h, l]
            _ = x l : Fin n, 0 := by
            apply Finset.sum_congr rfl
            intro l _
            ring_nf
            _ = 0 := by simp
      rw [h₁, h₂]
      <> simp

have hfinal : (x k, x l, (if (colors k l = 0) then (nums k l) else 0)) = (x
  → k, x l, (if (colors k l = 1) then (nums k l) else 0)) := by
have h₁ : (x k : Fin n, x l : Fin n, (if colors k l = 0 then (nums k l : z)
  → else 0)) = (x k : Fin n, x l : Fin n, (if colors k l = 1 then (nums k
  → l : z) else 0)) = 0 := by
  rw [hsum_diff]
  rw [hsum_split_zero]
have h₂ : (x k : Fin n, x l : Fin n, (if colors k l = 0 then (nums k l : z)
  → else 0)) = (x k : Fin n, x l : Fin n, (if colors k l = 1 then (nums k
  → l : z) else 0)) := by
  linarith
  simp using h₁

exact hfinal

-- Simplified Proof
import Mathlib
import Aesop

set_option maxHeartbeats 0

open Topology Filter Polynomial Set

theorem putnam_2001_b1
  (n : ℕ)
  (hn : n > 0) (hn' : Even n)

```

```

(nums : Fin n → Fin n → z)
(colors : Fin n → Fin n → Fin 2)
(hnums : ∀ k l, nums k l = k * n + l + 1)
(hcolorrows : ∀ k, (x l, (if (colors k l = 0) then 1 else 0)) = n / 2)
(hcolorcols : ∀ l, (x k, (if (colors k l = 0) then 1 else 0)) = n / 2) :
(x k, x l, (if (colors k l = 0) then (nums k l) else 0)) = (x k, x l, (if
  → (colors k l = 1) then (nums k l) else 0)) := by
have hcol_sum_zero : x (l : Fin n), (x k : Fin n, (2 * (if colors k l = 0
  → then (1 : z) else 0) - 1)) = 0 := by
  intro l
  have h1 : (x k : Fin n, (if colors k l = 0 then (1 : z) else 0)) = n / 2 :=
    → by
    norm_cast at hcolorcols ⊢
    simp using hcolorcols l
  have h2 : (x k : Fin n, (2 * (if colors k l = 0 then (1 : z) else 0) - 1)) =
    → 0 := by
    calc
      (x k : Fin n, (2 * (if colors k l = 0 then (1 : z) else 0) - 1)) = (x k
        → : Fin n, (2 * (if colors k l = 0 then (1 : z) else 0))) - x k : Fin
        → n, (1 : z) := by
        rw [Finset.sum_sub_distrib]
        _ = 2 * (x k : Fin n, (if colors k l = 0 then (1 : z) else 0)) - x k :
        → Fin n, (1 : z) := by
        rw [Finset.mul_sum]
        _ = 2 * (n / 2 : z) - n := by
        rw [h1]
        simp [Finset.sum_const, Finset.card_fin]
        _ = 0 := by
        have h3 : (n : z) % 2 = 0 := by
        have h4 : Even n := hn'
        rw [even_iff_two_dvd] at h4
        obtain m, hm := h4
        norm_cast at hm ⊢
        omega
        have h4 : (n : z) / 2 * 2 = n := by
        have h5 : (n : z) % 2 = 0 := h3
        have h6 : (n : z) = 2 * ((n : z) / 2) := by
        omega
        linarith
        ring_nf at *
        <> omega
      exact h2
  have hrow_sum_zero : x (k : Fin n), (x l : Fin n, (2 * (if colors k l = 0
    → then (1 : z) else 0) - 1)) = 0 := by
  intro k
  have h1 : (x l : Fin n, (if colors k l = 0 then (1 : z) else 0)) = n / 2 :=
    → by
    norm_cast at hcolorrows ⊢
    simp using hcolorrows k
  have h2 : (x l : Fin n, (2 * (if colors k l = 0 then (1 : z) else 0) - 1)) =
    → 0 := by
    calc
      (x l : Fin n, (2 * (if colors k l = 0 then (1 : z) else 0) - 1)) = (x l
        → : Fin n, (2 * (if colors k l = 0 then (1 : z) else 0))) - x l : Fin
        → n, (1 : z) := by
        rw [Finset.sum_sub_distrib]
        _ = 2 * (x l : Fin n, (if colors k l = 0 then (1 : z) else 0)) - x l :
        → Fin n, (1 : z) := by
        rw [Finset.mul_sum]
        _ = 2 * (n / 2 : z) - n := by
        rw [h1]
        simp [Finset.sum_const, Finset.card_fin]
        _ = 0 := by
        have h3 : (n : z) % 2 = 0 := by
        have h4 : Even n := hn'
        rw [even_iff_two_dvd] at h4
        obtain m, hm := h4
        norm_cast at hm ⊢
        omega
        have h4 : (n : z) / 2 * 2 = n := by
        have h5 : (n : z) % 2 = 0 := h3
        have h6 : (n : z) = 2 * ((n : z) / 2) := by
        omega
        linarith
        ring_nf at *
        <> omega
      exact h2
  have hsum_diff : (x k : Fin n, x l : Fin n, (if colors k l = 0 then (nums k l
    → : z) else 0)) = (x k : Fin n, x l : Fin n, (if colors k l = 1 then
    → (nums k l : z) else 0)) = x k : Fin n, x l : Fin n, (2 * (if colors k
    → l = 0 then (1 : z) else 0) - 1) * (nums k l : z) := by
  have h₁ : (x k : Fin n, x l : Fin n, (if colors k l = 0 then (nums k l : z)
    → else 0)) = (x k : Fin n, x l : Fin n, (if colors k l = 1 then (nums k
    → l : z) else 0)) = x k : Fin n, x l : Fin n, ((if colors k l = 0 then
    → (nums k l : z) else 0) - (if colors k l = 1 then (nums k l : z) else
    → 0)) := by
    simp [Finset.sum_sub_distrib, Finset.sum_add_distrib]
  have h₂ : x (k : Fin n) (l : Fin n), ((if colors k l = 0 then (nums k l : z
    → ) else 0) - (if colors k l = 1 then (nums k l : z) else 0)) = (2 *
    → (if colors k l = 0 then (1 : z) else 0) - 1) * (nums k l : z) := by
    intro k l
    have h₃ : colors k l = 0 ∨ colors k l = 1 := by
    have h₄ : colors k l = 0 ∨ colors k l = 1 := by
    have : colors k l = 0 ∨ colors k l = 1 := by
    have h₄ : (colors k l : ℕ) < 2 := by
    have : (colors k l : ℕ) < 2 := by
    simp [Fin.is_lt]
    exact this
    omega
    exact this
    exact h₄
    rcases h₄ with (h₄ | h₄)
    simp [h₄]
    simp [h₄]
  calc
    (x k : Fin n, x l : Fin n, (if colors k l = 0 then (nums k l : z) else
      → 0)) = (x k : Fin n, x l : Fin n, (if colors k l = 1 then (nums k l : z
      → ) else 0)) = x k : Fin n, x l : Fin n, ((if colors k l = 0 then (nums
      → k l : z) else 0) - (if colors k l = 1 then (nums k l : z) else 0)) :=
      → by rw [h₁]
    _ = x k : Fin n, x l : Fin n, (2 * (if colors k l = 0 then (1 : z) else
      → 0) - 1) * (nums k l : z) := by
    apply Finset.sum_congr rfl

```

```

intro k _
apply Finset.sum_congr rfl
intro l _
rw [h, k l]
have hsum_split_zero : (z k : Fin n, z l : Fin n, (2 * (if colors k l = 0
→ then (1 : z) else 0) - 1) * (nums k l : z)) = 0 := by
have h_1 : (z k : Fin n, z l : Fin n, (2 * (if colors k l = 0 then (1 : z)
→ else 0) - 1) * (nums k l : z)) = z k : Fin n, z l : Fin n, (2 * (if
→ colors k l = 0 then (1 : z) else 0) - 1) * ((k : z) * n + (l : z) +
→ 1)) := by
apply Finset.sum_congr rfl
intro k _
apply Finset.sum_congr rfl
intro l _
rw [hnums]
rw [h_]
have h_1 : (z k : Fin n, z l : Fin n, (2 * (if colors k l = 0 then (1 : z)
→ else 0) - 1) * ((k : z) * n + (l : z) + 1)) = (z k : Fin n, z l : Fin
→ n, (2 * (if colors k l = 0 then (1 : z) else 0) - 1) * ((k : z) * n))
+ (z k : Fin n, z l : Fin n, (2 * (if colors k l = 0 then (1 : z)
→ else 0) - 1) * ((l : z) + 1))) := by
calc
(z k : Fin n, z l : Fin n, (2 * (if colors k l = 0 then (1 : z) else 0)
→ - 1) * ((k : z) * n + (l : z) + 1)) = z k : Fin n, z l : Fin n, ((2 *
→ (if colors k l = 0 then (1 : z) else 0) - 1) * ((k : z) * n) + (2 *
→ (if colors k l = 0 then (1 : z) else 0) - 1) * ((l : z) + 1))) := by
apply Finset.sum_congr rfl
intro k _
apply Finset.sum_congr rfl
intro l _
ring_nf
_ = (z k : Fin n, z l : Fin n, (2 * (if colors k l = 0 then (1 : z)
→ else 0) - 1) * ((k : z) * n)) + (z k : Fin n, z l : Fin n, (2 * (if
→ colors k l = 0 then (1 : z) else 0) - 1) * ((l : z) + 1))) := by
simp [Finset.sum_add_distrib]
rw [h_]
have h_1 : (z k : Fin n, z l : Fin n, (2 * (if colors k l = 0 then (1 : z)
→ else 0) - 1) * ((k : z) * n)) = 0 := by
have h_1 : ∀ (k : Fin n), (z l : Fin n, (2 * (if colors k l = 0 then (1 : z)
→ ) else 0) - 1) * ((k : z) * n)) = 0 := by
intro k
have h_1 : (z l : Fin n, (2 * (if colors k l = 0 then (1 : z) else 0) -
→ 1)) = 0 := hrow_sum_zero k
calc
(z l : Fin n, (2 * (if colors k l = 0 then (1 : z) else 0) - 1) * ((k
→ : z) * n)) = z l : Fin n, ((k : z) * n) * (2 * (if colors k l = 0
→ then (1 : z) else 0) - 1)) := by
apply Finset.sum_congr rfl
intro l _
ring_nf
_ = ((k : z) * n) * z l : Fin n, (2 * (if colors k l = 0 then (1 : z)
→ else 0) - 1) := by
rw [Finset.mul_sum]
_ = ((k : z) * n) * 0 := by rw [h_]
= 0 := by ring
calc
(z k : Fin n, z l : Fin n, (2 * (if colors k l = 0 then (1 : z) else 0)
→ - 1) * ((k : z) * n)) = z k : Fin n, (z l : Fin n, (2 * (if colors k
→ l = 0 then (1 : z) else 0) - 1) * ((k : z) * n))) := by simp
[Finset.sum_sigma']
_ = z k : Fin n, 0 := by
apply Finset.sum_congr rfl
intro k _
rw [h, k l]
_ = 0 := by simp
have h_1 : (z k : Fin n, z l : Fin n, (2 * (if colors k l = 0 then (1 : z)
→ else 0) - 1) * ((l : z) + 1)) = 0 := by
have h_1 : ∀ (l : Fin n), (z k : Fin n, (2 * (if colors k l = 0 then (1 : z)
→ ) else 0) - 1)) = 0 := by
intro l
exact hc0l_sum_zero 1
calc
(z k : Fin n, z l : Fin n, (2 * (if colors k l = 0 then (1 : z) else 0)
→ - 1) * ((l : z) + 1)) = z l : Fin n, z k : Fin n, (2 * (if colors k l
→ = 0 then (1 : z) else 0) - 1) * ((l : z) + 1)) := by
rw [Finset.sum_comm]
_ = z l : Fin n, ((l : z) + 1) * (z k : Fin n, (2 * (if colors k l = 0
→ then (1 : z) else 0) - 1))) := by
apply Finset.sum_congr rfl
intro l _
calc
(z k : Fin n, (2 * (if colors k l = 0 then (1 : z) else 0) - 1) *
→ ((l : z) + 1)) = z k : Fin n, ((l : z) + 1) * (2 * (if colors k l = 0
→ then (1 : z) else 0) - 1)) := by
apply Finset.sum_congr rfl
intro l _
ring_nf
_ = ((l : z) + 1) * z k : Fin n, (2 * (if colors k l = 0 then (1 : z)
→ else 0) - 1) := by
rw [Finset.mul_sum]
_ = z l : Fin n, ((l : z) + 1) * 0 := by
apply Finset.sum_congr rfl
intro l _
rw [h, l]
_ = z l : Fin n, 0 := by
apply Finset.sum_congr rfl
intro l _
ring_nf
_ = 0 := by simp
rw [h_, h_]
<|> simp
linarith
-- Orig Proof
import Mathlib
import Aesop
set_option maxHeartbeats 0
open MvPolynomial Set Nat
theorem putnam_2003_b4
(f : ℝ → ℝ)
(a b c d e : ℤ)

```



```

have h3 := congr_arg (fun x => x / (a : R)) (by linarith)
field_simp [h3] at h3 ⊢
<> ring_nf at h3 ⊢ <> nlinarith [sq_pos_of_ne_zero (sub_ne_zero.mpr h1)]

have h_main : -Irrational (r1 * r2) := by
  obtain q, hq1 := h_s_rat
  obtain q, hq2 := h_t_rat
  have h1 : (r1 + r2 : R) = (q : R) := by
    norm_cast at hq1 ⊢
  <> linarith
  have h2 : (r3 + r4 : R) = (q : R) := by
    norm_cast at hq2 ⊢
  <> linarith
  have h3 : (q : R) ≠ (q : R) := by
    intro h4
    linarith
    have h4 : (r1 + r2 : R) = (r3 + r4 : R) := by
      rw [h4, h4] at *
      <> norm_cast at h4 ⊢ <>
      (try simp_all) <>
      (try linarith)
    exfalse
    apply h4
    <>
    (try simp_all [add_assoc]) <>
    (try linarith)
  have h5 : (q : R) - (q : R) ≠ 0 := by
    intro h6
    apply h6
    linarith
  have h6 : ((q : R) - (q : R)) * (r1 * r2 : R) = -(d : R) / a : R - (q : R) * ((c : R) / a : R) + (q : R) ^ 2 * (q : R) := by
    have h7 : (r1 + r2 : R) * (r3 + r4 : R) + (r3 + r4 : R) * (r1 * r2 : R) =
      -(d : R) / a : R := by
        simp [h7, h7] using h_sq_tp
    have h8 : (r1 + r2 : R) * (r3 + r4 : R) + (r1 * r2 + r3 * r4 : R) = (c : R)
      -> / a := by
        simp [h8, h8] using h_st_pq
    have h9 : (r1 + r2 : R) = (q : R) := by simp [h9] using h1
    have h10 : (r3 + r4 : R) = (q : R) := by simp [h10] using h2
    have h11 : (r3 * r4 : R) = (c : R) / a - (q : R) * (q : R) - (r1 * r2 : R)
      -> := by
      have h12 : (q : R) * (q : R) + (r1 * r2 + r3 * r4 : R) = (c : R) / a :=
        by
          calc
            (q : R) * (q : R) + (r1 * r2 + r3 * r4 : R) = (r1 + r2 : R) * (r3 +
              r4 : R) + (r1 * r2 + r3 * r4 : R) := by
              rw [h12, h12]
              <> ring_nf
              <> norm_num
            _ = (c : R) / a := by simp [h12] using h3
    linarith
  calc
    ((q : R) - (q : R)) * (r1 * r2 : R) = (q : R) * (r1 * r2 : R) - (q :
      -> R) * (r1 * r2 : R) := by ring
    _ = (q : R) * (r1 * r2 : R) - (q : R) * (r1 * r2 : R) := by ring
    _ = -(d : R) / a : R - (r1 + r2 : R) * (r3 * r4 : R) - (q : R) * (r1
      -> * r2 : R) := by
      have h13 : (r3 + r4 : R) * (r1 * r2 : R) = -(d : R) / a : R - (r1 +
        r2 : R) * (r3 * r4 : R) := by
          linarith
      rw [h13] at h13
      linarith
    _ = -(d : R) / a : R - (r1 + r2 : R) * (r3 * r4 : R) - (q : R) * (r1
      -> * r2 : R) := by rfl
    _ = -(d : R) / a : R - (q : R) * (r3 * r4 : R) - (q : R) * (r1 * r2
      -> : R) := by
      rw [h14]
      <> ring_nf
      <> norm_num
    _ = -(d : R) / a : R - (q : R) * ((r3 * r4 : R) + (r1 * r2 : R)) :=
      by ring
    _ = -(d : R) / a : R - (q : R) * ((c : R) / a - (q : R) * (q : R))
      := by
        rw [h15]
        <> ring_nf
        <> norm_num
    (try simp_all [add_assoc]) <>
    (try linarith)
    _ = -(d : R) / a : R - (q : R) * ((c : R) / a : R) + (q : R) ^ 2 *
      -> (q : R) := by
      ring_nf
      <> field_simp [ane0]
      <> ring_nf
      <> norm_num
      <>
      (try simp_all [add_assoc]) <>
      (try linarith)
  have h6 : ∃ (q : Q), (q : R) = -(d : R) / a : R - (q : R) * ((c : R) / a
    -> : R) + (q : R) ^ 2 * (q : R) := by
    use (-(d : Q) / a - q * ((c : Q) / a) + q ^ 2 * q)
    <> norm_cast <>
    (try simp_all [div_eq_mul_inv]) <>
    (try field_simp [ane0]) <>
    (try ring_nf) <>
    (try norm_num) <>
    (try linarith)
  obtain q, hq1 := h6
  have h7 : ∃ (q : Q), (q : R) = (r1 * r2 : R) := by
    use (q / (q - q))
  have h8 : ((q : R) - (q : R)) ≠ 0 := by simp using h8
  have h9 : (q : R) = -(d : R) / a : R - (q : R) * ((c : R) / a : R) +
    -> (q : R) ^ 2 * (q : R) := by
    simp using hq1
  have h10 : ((q : R) - (q : R)) * (r1 * r2 : R) = (q : R) := by
    rw [h10] at *
    linarith
  have h11 : (r1 * r2 : R) = (q : R) / ((q : R) - (q : R)) := by
    field_simp [h11] at h10 ⊢
    <> nlinarith
    norm_cast at h11 ⊢ <>
    (try simp_all [div_eq_mul_inv]) <>
    (try field_simp [h11]) <>

    (try ring_nf at * <> simp_all) <>
    (try norm_num at * <> simp_all)
    obtain q, hq1 := h6
    intro h7
    have h8 : Irrational (r1 * r2) := h7
    exact h8 q, by simp [hq1]

    exact h_main

-- Simplified Proof
import Mathlib
import Aesop

set_option maxHeartbeats 0

open MvPolynomial Set Nat

theorem putnam_2003_b4
  (f : R → R)
  (a b c d e : Z)
  (r1 r2 r3 r4 : R)
  (ane0 : a ≠ 0)
  (hf1 : ∀ z, f z = a * z ^ 4 + b * z ^ 3 + c * z ^ 2 + d * z + e)
  (hf2 : ∀ z, f z = a * (z - r1) * (z - r2) * (z - r3) * (z - r4)) :
  (Irrational (r1 + r2) ∧ r1 + r2 ≠ r3 + r4) → Irrational (r1 * r2) := by
  intro h
  have h1 : ∃ (q : Q), (q : R) = r1 + r2 := by
    have h1 : -Irrational (r1 + r2) := h.1
    by_contra! h2
    exact h2 (by simp_all [Irrational])
  have h2 : ∃ (q : Q), (q : R) = r3 + r4 := by
    have h3 : (r1 + r2) + (r3 + r4) = -(b : R) / a : R := by
      have h4 := hf1 0
      have h5 := hf2 0
      have h6 := hf1 1
      have h7 := hf2 1
      have h8 := hf1 (-1)
      have h9 := hf2 (-1)
      have h10 := hf1 2
      have h11 := hf2 2
      have h12 := hf1 (-2)
      have h13 := hf2 (-2)
      norm_num at h4 h5 h6 h7 h8 h9 h10 h11 h12 h13
      ring_nf at h4 h5 h6 h7 h8 h9 h10 h11 h12 h13
      have h14 : (a : R) ≠ 0 := by exact_mod_cast ane0
      have h15 := congr_arg (fun x => x / (a : R)) (by linarith)
      field_simp [h15] at h15 ⊢
      <> ring_nf at h15 ⊢ <> nlinarith [sq_pos_of_ne_zero (sub_ne_zero.mpr
        -> h15)]
    obtain q, hq1 := h2
    use (-(b : Q) / a - q)
    norm_cast at h1 hq1 ⊢
    <> simp_all [div_eq_mul_inv]
    <> ring_nf at h1 ⊢
    <> linarith
  have h3 : (r1 + r2) * (r3 + r4) + (r1 * r2 + r3 * r4) = (c : R) / a := by
    have h4 := hf1 0
    have h5 := hf2 0
    have h6 := hf1 1
    have h7 := hf2 1
    have h8 := hf1 (-1)
    have h9 := hf2 (-1)
    have h10 := hf1 2
    have h11 := hf2 2
    have h12 := hf1 (-2)
    have h13 := hf2 (-2)
    norm_num at h4 h5 h6 h7 h8 h9 h10 h11 h12 h13
    ring_nf at h4 h5 h6 h7 h8 h9 h10 h11 h12 h13
    have h14 : (a : R) ≠ 0 := by exact_mod_cast ane0
    have h15 := congr_arg (fun x => x / (a : R)) (by linarith)
    field_simp [h15] at h15 ⊢
    <> ring_nf at h15 ⊢ <> nlinarith [sq_pos_of_ne_zero (sub_ne_zero.mpr h15)]
  have h4 : (r1 + r2) * (r3 * r4) + (r3 + r4) * (r1 * r2) = -(d : R) / a : R
    -> := by
    have h5 := hf1 0
    have h6 := hf2 0
    have h7 := hf1 1
    have h8 := hf2 1
    have h9 := hf1 (-1)
    have h10 := hf2 (-1)
    have h11 := hf1 2
    have h12 := hf2 2
    have h13 := hf1 (-2)
    have h14 := hf2 (-2)
    norm_num at h5 h6 h7 h8 h9 h10 h11 h12 h13 h14
    ring_nf at h5 h6 h7 h8 h9 h10 h11 h12 h13 h14
    have h15 : (a : R) ≠ 0 := by exact_mod_cast ane0
    have h16 := congr_arg (fun x => x / (a : R)) (by linarith)
    field_simp [h16] at h16 ⊢
    <> ring_nf at h16 ⊢ <> nlinarith [sq_pos_of_ne_zero (sub_ne_zero.mpr h16)]
  have h5 : -Irrational (r1 * r2) := by
    obtain q, hq1 := h1
    obtain q, hq2 := h2
    have h6 : (r1 + r2 : R) = (q : R) := by
      norm_cast at hq1 ⊢
    <> linarith
    have h7 : (r3 + r4 : R) = (q : R) := by
      norm_cast at hq2 ⊢
    <> linarith
    have h8 : (q : R) ≠ (q : R) := by
      intro h9
      apply h9
      linarith
    intro h10
    apply h10
    linarith
    have h11 : ((q : R) - (q : R)) * (r1 * r2 : R) = -(d : R) / a : R - (q :
      -> R) * ((c : R) / a : R) + (q : R) ^ 2 * (q : R) := by
      have h12 : ((q : R) - (q : R)) ≠ 0 := by simp using h8
      have h13 : (q : R) = -(d : R) / a : R - (q : R) * ((c : R) / a : R) +
        -> (q : R) ^ 2 * (q : R) := by
        simp using hq1
      have h14 : ((q : R) - (q : R)) * (r1 * r2 : R) = (q : R) := by
        rw [h14] at *
        linarith
      have h15 : (r1 * r2 : R) = (q : R) / ((q : R) - (q : R)) := by
        field_simp [h15] at h14 ⊢
        <> nlinarith
        norm_cast at h15 ⊢ <>
        (try simp_all [div_eq_mul_inv]) <>
        (try field_simp [h15]) <>

```





```

    <|> ring_nf
    <|> norm_num
    <|> linarith
  exact h₂ n
  exact h₃
  exact h_main
-- Simplified Proof
import Mathlib
import Aesop
set_option maxHeartbeats 0
open Nat Topology Filter

theorem putnam_2004_a3
(u : ℕ → ℝ)
(hbase : u 0 = 1 ∧ u 1 = 1 ∧ u 2 = 1)
(hudet : ∀ n : ℕ, Matrix.det (fun i j : Fin 2 => u (n + i * 2 + j)) = (n!))
: ∀ n : ℕ, ∃ m : ℤ, u n = m := by

  have h_inv : ∀ (n : ℕ), u (n + 2) = (n + 1 : ℝ) * u n ∧ u n * u (n + 1) = (n
    ! : ℝ) := by
    intro n
    induction n with
    | zero =>
      constructor <|> norm_num [hbase]
    | succ n ih =>
      have h₁ : u (n + 1 + 2) = (n + 1 + 1 : ℝ) * u (n + 1) ∧ u (n + 1) * u (n +
        1 + 2) = ((n + 1) ! : ℝ) := by
        have h₂ : u n * u (n + 1) = (n ! : ℝ) := ih.2
        have h₃ : u n * u (n + 3) - u (n + 1) * u (n + 2) = (n ! : ℝ) := by
          have h₄ : u n = hudet n
          simp [Matrix.det_fin_two] at h₄
          ring_nf at h₄
          <|> linarith
        have h₅ : u (n + 3) = (n + 1 + 1 : ℝ) * u (n + 1) := by
          have h₆ : u n * u (n + 3) - u (n + 1) * u (n + 2) = (n ! : ℝ) := h₃
          have h₇ : u (n + 2) = (n + 1 : ℝ) * u n := ih.1
          have h₈ : u n * u (n + 3) - u (n + 1) * ((n + 1 : ℝ) * u n) = (n ! : ℝ)
            := by
              rw [h₇] at h₈
              exact h₈
          have h₉ : u n ≠ 0 := by
            have h₁₀ : u n * u (n + 1) = (n ! : ℝ) := ih.2
            have h₁₁ : (n ! : ℝ) ≠ 0 := by
              norm_cast
              exact Nat.factorial_ne_zero n
            intro h₁₂
            rw [h₁₂] at h₁₀
            norm_num at h₁₀
            <|> simp_all [h₁₀]
          have h₁₃ : u (n + 3) - (n + 1 : ℝ) * u (n + 1) = u (n + 1) := by
            apply mul_left_cancelₑ h₁₃
            linarith
          have h₁₄ : u (n + 1) * u (n + 1 + 1) = ((n + 1) ! : ℝ) := by
            have h₁₅ : u (n + 2) = (n + 1 : ℝ) * u n := ih.1
            have h₁₆ : u (n + 1) * u (n + 2) = (n + 1 : ℝ) * (u n * u (n + 1)) :=
              by
                calc
                  u (n + 1) * u (n + 2) = u (n + 1) * ((n + 1 : ℝ) * u n) := by rw
                    [h₁₅]
                  _ = (n + 1 : ℝ) * (u (n + 1) * u n) := by ring
                  _ = (n + 1 : ℝ) * (u n * u (n + 1)) := by ring
            have h₁₇ : u n * u (n + 1) = (n ! : ℝ) := ih.2
            have h₁₈ : u (n + 1) * u (n + 2) = (n + 1 : ℝ) * (u n * u (n + 1)) :=
              by
                rw [h₁₇]
                have h₁₉ : u (n + 1) * u (n + 2) = (n + 1 : ℝ) * (n ! : ℝ) := by
                  rw [h₁₈]
                  have h₂₀ : (n + 1 : ℝ) * (n ! : ℝ) = ((n + 1) ! : ℝ) := by
                    norm_cast
                    linarith
                exact (by linarith, by linarith)
                simp [add_assoc] using h₂₀
            exact fun n => by
              induction' n using Nat.strong_induction_on with n ih
              match n with
              | 0 => exact (1, by simp_all)
              | 1 => exact (1, by simp_all)
              | 2 => exact (1, by simp_all)
              | k + 3 =>
                have h₂₁ := h_inv (k + 1)
                obtain m, hm := ih (k + 1) (by omega)
                exact ((k + 1 + 1 : ℤ) * m, by rw [h₂₁, hm]; norm_cast)
            -----
            -- Orig Proof
            import Mathlib
            import Aesop
            set_option maxHeartbeats 0
            open Nat Topology Filter

            theorem putnam_2004_b2
            (m n : ℕ)
            (mnp0 : m > 0 ∧ n > 0)
            : ((m + n)! / ((m + n) ^ (m + n) : ℚ)) < ((m)! / (m ^ m : ℚ)) * ((n)! / (n ^
              n : ℚ)) := by
              have h_main_ineq : ((m + n : ℚ) : ℚ) ^ (m + n) > (Nat.choose (m + n) m : ℚ) *
                ((m : ℚ) ^ m * (n : ℚ) ^ n) := by
                  have h₁ : ((m + n : ℚ) : ℚ) ^ (m + n) = ∑ k in Finset.range (m + n + 1),
                    (Nat.choose (m + n) k : ℚ) * (m : ℚ) ^ k * (n : ℚ) ^ (m + n - k) := by
                      have h₂ : ((m + n : ℚ) : ℚ) ^ (m + n) = ((m : ℚ) + (n : ℚ)) ^ (m + n) :=
                        by
                          norm_cast
                          <|> ring_nf
                          rw [h₂]
                          rw [add_pow]
                          apply Finset.sum_congr rfl
                          intro k hk

```

```

      simp [mul_assoc, mul_comm, mul_left_comm, Nat.cast_add, Nat.cast_one,
        Nat.cast_mul, Nat.cast_ofNat]
    <|> ring_nf at hk <|> norm_cast at hk <|> field_simp at hk <|>
      ring_nf at hk <|> norm_cast at hk <|> simp_all
    => [Nat.choose_eq_factorial_div_factorial]
  <|> linarith
  rw [h₁]
  have h₂ : ∑ k in Finset.range (m + n + 1), (Nat.choose (m + n) k : ℚ) * (m
    : ℚ) ^ k * (n : ℚ) ^ (m + n - k) > (Nat.choose (m + n) m : ℚ) * (m : ℚ)
    ^ m * (n : ℚ) ^ n := by
    have h₃ : (Nat.choose (m + n) m : ℚ) * (m : ℚ) ^ m * (n : ℚ) ^ n =
      (Nat.choose (m + n) m : ℚ) * (m : ℚ) ^ m * (n : ℚ) ^ n := rfl
    have h₄ : ∑ k in Finset.range (m + n + 1), (Nat.choose (m + n) k : ℚ) *
      (m : ℚ) ^ k * (n : ℚ) ^ (m + n - k) ≥ ∑ k in Finset.range (m + n +
        1), (Nat.choose (m + n) k : ℚ) * (m : ℚ) ^ k * (n : ℚ) ^ (m + n - k)
      := le_refl
    have h₅ : 0 < (n : ℚ) ^ (m + n) := by
      norm_cast
      exact pow_pos (by linarith) (m + n)
    have h₆ : (Nat.choose (m + n) m : ℚ) * (m : ℚ) ^ m * (n : ℚ) ^ n =
      (Nat.choose (m + n) m : ℚ) * (m : ℚ) ^ m * (n : ℚ) ^ n := rfl
    have h₇ : ∑ k in Finset.range (m + n + 1), (Nat.choose (m + n) k : ℚ) *
      (m : ℚ) ^ k * (n : ℚ) ^ (m + n - k) > (Nat.choose (m + n) m : ℚ) * (m
        : ℚ) ^ m * (n : ℚ) ^ n := by
      have h₈ : ∑ k in Finset.range (m + n + 1), (Nat.choose (m + n) k : ℚ) *
        (m : ℚ) ^ k * (n : ℚ) ^ (m + n - k) ≥ (Nat.choose (m + n) m : ℚ) * (m
          : ℚ) ^ m * (n : ℚ) ^ n + (m + n) * (m : ℚ) ^ (m + n) := by
        calc
          ∑ k in Finset.range (m + n + 1), (Nat.choose (m + n) k : ℚ) * (m : ℚ)
            ^ k * (n : ℚ) ^ (m + n - k) ≥ ∑ k in (Finset.range (m + n) : Finset ℕ),
              (Nat.choose (m + n) k : ℚ) * (m : ℚ) ^ k * (n : ℚ) ^ (m + n - k) := by
                apply Finset.sum_le_sum_of_subset_of_nonneg
                intro x hx
                simp only [Finset.mem_insert, Finset.mem_singleton] at hx
                simp only [Finset.mem_range]
                rcases hx with (rfl | rfl)
                | omega
                | omega
                intro x _
                positivity
                _ = (Nat.choose (m + n) m : ℚ) * (m : ℚ) ^ m * (n : ℚ) ^ (m + n -
                  m) + (Nat.choose (m + n) 0 : ℚ) * (m : ℚ) ^ 0 * (n : ℚ) ^ (m + n - 0)
                := by
                  simp [Finset.sum_pair (show (m : ℕ) ≠ 0 by
                    have h₉ : m > 0 := mnp0.1
                    omega)]
                  <|> ring_nf
                  <|> field_simp
                  <|> norm_cast
                  <|> simp [Nat.choose_zero_right]
                  _ = (Nat.choose (m + n) m : ℚ) * (m : ℚ) ^ m * (n : ℚ) ^ n +
                    (Nat.choose (m + n) 0 : ℚ) * (m : ℚ) ^ 0 * (n : ℚ) ^ (m + n) := by
                      have h₁₀ : m + n - m = n := by
                        have h₁₁ : m ≤ m + n := by omega
                        omega
                      have h₁₂ : m + n - 0 = m + n := by simp
                      rw [h₁₀, h₁₁]
                      <|> ring_nf
                      <|> field_simp
                      <|> norm_cast
                      _ = (Nat.choose (m + n) m : ℚ) * (m : ℚ) ^ m * (n : ℚ) ^ n + (n : ℚ)
                        ^ (m + n) := by
                          simp [Nat.choose_zero_right]
                          <|> ring_nf
                          <|> field_simp
                          <|> norm_cast
                          <|> simp [pow_add, pow_one]
                          <|> ring_nf
                          <|> field_simp
                          <|> norm_cast
                      have h₁₃ : (n : ℚ) ^ (m + n) > 0 := by positivity
                      linarith
                      linarith
                      linarith
                    have h_choose_mul_factorial : (Nat.choose (m + n) m : ℚ) * (m ! : ℚ) * (n !
                      : ℚ) = ((m + n)!) : ℚ := by
                        have h₁₄ : (Nat.choose (m + n) m : ℕ) * m ! * n ! = (m + n)! := by
                          have h₁₅ : Nat.choose (m + n) m * m ! * n ! = (m + n)! := by
                            rw [← Nat.choose_mul_factorial_mul_factorial (by omega : m ≤ m + n)]
                            <|> ring_nf
                            <|> simp [Nat.mul_assoc]
                            <|> ring_nf
                          exact_mod_cast h₁₅
                        have h₁₆ : (Nat.choose (m + n) m : ℚ) * (m ! : ℚ) * (n ! : ℚ) = ((m + n) ! : ℚ)
                          := by
                            norm_cast
                            <|> simp_all [Nat.cast_add, Nat.cast_mul, Nat.cast_one]
                            <|> ring_nf at *
                            <|> norm_cast at *
                            <|> linarith
                          exact h₁₆
                      have h_ineq_after_mul : ((m + n : ℚ) : ℚ) ^ (m + n) * (m ! : ℚ) * (n ! : ℚ) >
                        ((m + n)!) : ℚ * (m : ℚ) ^ m * (n : ℚ) ^ n := by
                          have h₁₇ : ((m + n : ℚ) : ℚ) ^ (m + n) > (Nat.choose (m + n) m : ℚ) * (m : ℚ)
                            ^ m * (n : ℚ) ^ n := h_main_ineq
                          have h₁₈ : 0 < (m ! : ℚ) := by positivity
                          have h₁₉ : 0 < (n ! : ℚ) := by positivity
                          have h₂₀ : 0 < (m ! : ℚ) * (n ! : ℚ) := by positivity
                          have h₂₁ : 0 < (m : ℚ) ^ m := by
                            norm_cast
                            exact pow_pos (by
                              have h₂₂ : (0 : ℕ) < m := by linarith
                              linarith) m
                          have h₂₃ : 0 < (n : ℚ) ^ n := by
                            norm_cast
                            exact pow_pos (by
                              have h₂₄ : (0 : ℕ) < n := by linarith
                              linarith) n
                          have h₂₅ : 0 < (m : ℚ) ^ m * (n : ℚ) ^ n := by positivity
                          have h₂₆ : 0 < (Nat.choose (m + n) m : ℚ) := by
                            norm_cast
                            apply Nat.cast_pos.mpr

```

```

    apply Nat.choose_pos
  <|> omega
have h1 : 0 < (Nat.choose (m + n) m : q) * (m : q) ^ m * (n : q) ^ n := by
  positivity
calc
  ((m + n : q) : q) ^ (m + n) * (m ! : q) * (n ! : q) > ((Nat.choose (m +
  → n) m : q) * (m : q) ^ m * (n : q) ^ n) * (m ! : q) * (n ! : q) := by
    gcongr <|>
      (try norm_num) <|>
        (try positivity) <|>
          (try linarith)
  _ = (Nat.choose (m + n) m : q) * (m ! : q) * (n ! : q) * ((m : q) ^ m *
  → (n : q) ^ n) := by ring
  _ = ((m + n)! : q) * ((m : q) ^ m * (n : q) ^ n) := by
    calc
      (Nat.choose (m + n) m : q) * (m ! : q) * (n ! : q) * ((m : q) ^ m *
      → (n : q) ^ n) = (Nat.choose (m + n) m : q) * (m ! : q) * (n ! : q) *
      → ((m : q) ^ m * (n : q) ^ n) := by ring
      _ = ((m + n)! : q) * ((m : q) ^ m * (n : q) ^ n) := by
        rw [h_choose_mul_factorial]
        <|> ring
      _ = ((m + n)! : q) * ((m : q) ^ m * (n : q) ^ n) := by ring
      _ = ((m + n)! : q) * (m : q) * (n : q) * ((m : q) ^ m * (n : q) ^ n) := by ring
have hfinal_ineq : (((m! : q) / (m : q) ^ m) * ((n! : q) / (n : q) ^ n) >
  → ((m + n)! : q) / ((m + n : q) : q) ^ (m + n) := by
  have h1 : 0 < (m : q) := by
    norm_cast
  <|> linarith
  have h2 : 0 < (n : q) := by
    norm_cast
  <|> linarith
  have h3 : 0 < (m : q) ^ m := by positivity
  have h4 : 0 < (n : q) ^ n := by positivity
  have h5 : 0 < ((m + n : q) : q) ^ (m + n) := by positivity
  have h6 : 0 < (m! : q) := by positivity
  have h7 : 0 < (n! : q) := by positivity
  have h8 : 0 < (m + n)! : q := by positivity
  have h9 : ((m + n : q) : q) ^ (m + n) * (m! : q) * (n! : q) > ((m + n)!
  → : q) * (m : q) ^ m * (n : q) ^ n := hineq_after_mul
  have h10 : 0 < ((m + n : q) : q) ^ (m + n) * (m : q) ^ m * (n : q) ^ n :=
  → by positivity
  have h11 : 0 < (m! : q) * (n! : q) := by positivity
  have h12 : ((m! : q) * (n! : q)) / ((m : q) ^ m * (n : q) ^ n) > ((m +
  → n)! : q) / ((m + n : q) : q) ^ (m + n) := by
    have h13 : ((m + n : q) : q) ^ (m + n) * (m! : q) * (n! : q) > ((m +
    → n)! : q) * (m : q) ^ m * (n : q) ^ n := h8
    have h14 : 0 < ((m + n : q) : q) ^ (m + n) * (m : q) ^ m * (n : q) ^ n :=
    → by positivity
    have h15 : 0 < (m! : q) * (n! : q) := by positivity
  have h16 : ((m! : q) * (n! : q)) / ((m : q) ^ m * (n : q) ^ n) > ((m +
  → n)! : q) / ((m + n : q) : q) ^ (m + n) := by
    calc
      ((m! : q) * (n! : q)) / ((m : q) ^ m * (n : q) ^ n) = ((m! : q) *
      → (n! : q)) / ((m : q) ^ m * (n : q) ^ n) := rfl
      _ > ((m + n)! : q) / ((m + n : q) : q) ^ (m + n) := by
        rw [gt_iff_lt]
        rw [div_lt_div_iff (by positivity) (by positivity)]
        nlinarith
    exact h17
  have h18 : (((m! : q) / (m : q) ^ m) * ((n! : q) / (n : q) ^ n) = ((m!
  → : q) * (n! : q)) / ((m : q) ^ m * (n : q) ^ n) := by
    field_simp [h18.ne', h18.ne']
    <|> ring_nf
    <|> field_simp [h18.ne', h18.ne']
    <|> ring_nf
  rw [h18]
  exact h19
have h20 : ((m + n)! : q) / ((m + n : q) : q) ^ (m + n) < (((m! : q) / (m : q) ^
  → m) * ((n! : q) / (n : q) ^ n)) := by
  have h21 : (((m! : q) / (m : q) ^ m) * ((n! : q) / (n : q) ^ n)) > ((m +
  → n)! : q) / ((m + n : q) : q) ^ (m + n) := hfinal_ineq
  have h22 : ((m + n)! : q) / ((m + n : q) : q) ^ (m + n) = ((m + n)! : q) /
  → ((m + n : q) ^ (m + n)) := by norm_cast
  rw [h22] at h20
  linarith
simp [div_eq_mul_inv] using h20
-- Simplified Proof
import Mathlib
import Aesop
set_option maxHeartbeats 0
open Nat Topology Filter
theorem putnam_2004_b2
(m n : ℕ)
(mnpos : m > 0 ∧ n > 0)
: ((m + n)! / ((m + n) ^ (m + n))) < (((m)! / (m ^ m)) * ((n)! / (n ^
  → n))) := by
  rcases mnpos with hm hn
  norm_cast at hm hn
  norm_cast
  apply lt_of_sub_pos
  field_simp
  norm_cast
  have h1 : (m + n : ℕ) ^ (m + n) > Nat.choose (m + n) m * m ^ m * n ^ n := by
    calc
      (m + n : ℕ) ^ (m + n) = ∑ k in Finset.range (m + n + 1), (Nat.choose (m +
      → n) k) * m ^ k * n ^ (m + n - k) := by
        rw [add_pow]
        apply Finset.sum_congr rfl
        intro k hk
        simp [mul_assoc, mul_comm, mul_left_comm, Nat.cast_add, Nat.cast_one,
        → Nat.cast_mul, Nat.cast_ofNat]
    ≥ ∑ k in {m, 0} : Finset ℕ, (Nat.choose (m + n) k) * m ^ k * n ^ (m +
    → n - k) := by
      apply Finset.sum_le_sum_of_subset_of_nonneg
      intro x hx
      simp only [Finset.mem_insert, Finset.mem_singleton] at hx
      simp only [Finset.mem_range]
      rcases hx with (rfl | rfl)
      omega
      omega
      intro x _
      positivity
      _ = (Nat.choose (m + n) m) * m ^ m * n ^ (m + n - m) + (Nat.choose (m +
      → n) 0) * m ^ 0 * n ^ (m + n - 0) := by
        simp [Finset.sum_pair (show (m : ℕ) ≠ 0 by omega)]
      _ = (Nat.choose (m + n) m) * m ^ m * n ^ n + (Nat.choose (m + n) 0) * m
      → ^ 0 * n ^ (m + n) := by
        have h2 : m + n - m = n := by omega
        have h3 : m + n - 0 = m + n := by simp
        rw [h2, h3]
      _ = (Nat.choose (m + n) m) * m ^ m * n ^ n + n ^ (m + n) := by
        simp [Nat.choose_zero_right]
      _ > (Nat.choose (m + n) m) * m ^ m * n ^ n := by
        have h4 : n ^ (m + n) > 0 := by positivity
        linarith
  have h5 : (Nat.choose (m + n) m) * (m!) * (n!) = (m + n)! := by
    rw [← Nat.choose_mul_factorial_mul_factorial (by omega : m ≤ m + n)]
    <|> ring_nf
    <|> simp [Nat.mul_assoc]
  have h6 : 0 < m! := by positivity
  have h7 : 0 < n! := by positivity
  have h8 : 0 < m * n := by positivity
  have h9 : 0 < m ^ m := by
    norm_cast
  exact pow_pos (by omega) m
  have h10 : 0 < n ^ n := by
    norm_cast
  exact pow_pos (by omega) n
  have h11 : 0 < m ^ m * n ^ n := by positivity
  have h12 : 0 < Nat.choose (m + n) m := by
    apply Nat.cast_pos.mpr
    apply Nat.choose_pos
    <|> omega
  have h13 : 0 < (Nat.choose (m + n) m) * m ^ m * n ^ n := by positivity
  nlinarith
-- Orig Proof
import Mathlib
import Aesop
set_option maxHeartbeats 0
open Nat Topology Filter
theorem putnam_2004_b4
(n : ℕ)
(nge2 : n ≥ 2)
(R Rk : ℕ → ℂ → ℂ)
(hR : R 0 = id ∧ ∀ k : ℕ, R (k + 1) = Rk (k + 1) ∘ R k)
(hRk : Rk = fun (k : ℕ) (Q : ℂ) → k + Complex.exp (Complex.I * 2 * Real.pi /
  → n) * (Q - k))
: (R n = ((fun n z → z + n) : ℕ → ℂ → ℂ) n) != by
have h1 : Complex.exp (Complex.I * 2 * Real.pi / n) ≠ 1 := by
  intro h
  have h2 : (k : ℤ), (Complex.I * 2 * Real.pi / n : ℂ) = (k : ℂ) * (2 *
  → Real.pi * Complex.I) := by
    rw [Complex.exp_eq_one_iff] at h
  exact h
  obtain (k, hk) := h
  have h3 : (Complex.I * 2 * Real.pi / n : ℂ) = (k : ℂ) * (2 * Real.pi *
  → Complex.I) := hk
  have h4 : (2 * Real.pi / n : ℝ) = (2 * Real.pi * k : ℝ) := by
    have h5 := h3
    simp [Complex.ext_iff, Complex.I_mul_I, mul_assoc, mul_comm,
    → mul_left_comm] at h5
    <|> norm_num at h5 <|>
      (try ring_nf at h5) <|>
      (try norm_num at h5) <|>
      (try linarith [Real.pi_pos]) <|>
      (try {
        field_simp [Real.pi_ne_zero, Nat.cast_ne_zero.mpr (by linarith : n ≠
        → 0)] at h5 <|>
        ring_nf at h5 <|>
        norm_cast at h5 <|>
        simp_all [Complex.ext_iff, pow_two] <|>
        nlinarith [Real.pi_pos]
      }) <|>
      (try {
        simp_all [Complex.ext_iff, pow_two]
        <|> ring_nf at *
        <|> norm_num at *
        <|> nlinarith [Real.pi_pos]
      })
    <|>
      (try {
        nlinarith [Real.pi_pos]
      })
  have h6 : (1 : ℝ) / n = (k : ℝ) := by
  have h7 : (n : ℝ) ≠ 0 := by positivity
  have h8 : (2 : ℝ) * Real.pi ≠ 0 := by positivity
  apply mul_left_cancel. (show (2 : ℝ) * Real.pi ≠ 0 by positivity)
  field_simp [h6] at h8
  <|> ring_nf at h8 <|> nlinarith [Real.pi_pos]
  have h9 : (n : ℕ) ≥ 2 := nge2
  have h10 : (k : ℝ) = (1 : ℝ) / n := by linarith
  have h11 : (k : ℝ) < 1 := by
    have h12 : (1 : ℝ) / n < 1 := by
      have h13 : (n : ℝ) ≥ 2 := by exact_mod_cast nge2
      have h14 : (1 : ℝ) / n < 1 := by
        rw [div_lt_one (by positivity)]
        <|> norm_cast <|> linarith
    exact h12
  linarith
  have h15 : (k : ℝ) > 0 := by

```

```
have h₈ : (k : ℕ) → n > 0 := by positivity
linearith
have h₉ : (k : ℤ) = 0 := by
have h₁₀ : (k : ℝ) < 1 := h₈
have h₁₁ : (k : ℝ) > 0 := h₈
have h₁₂ : (k : ℤ) = 0 := by
norm_cast at h₁₀ h₁₁ ⊢
<>
{ try {
omega
} } <>
{ try {
have h₁₃ : k < 1 := by linearith
have h₁₄ : k > 0 := by linearith
omega
} }
exact h₁₂
have h₁₅ : (k : ℝ) = 0 := by
norm_cast
<> simp [h.]
have h₁₆ : (1 : ℝ) / n = 0 := by linearith
have h₁₇ : (n : ℝ) = 0 := by
have h₁₈ : (n : ℝ) ≠ 0 := by positivity
field_simp [h.] at h₁₆
<> linarith
have h₁₉ : (n : ℕ) = 0 := by
norm_cast at h₁₇ ⊢
<> simp_all
linarith
have h_pow_n : (Complex.exp (Complex.I * 2 * Real.pi / n)) ^ n = 1 := by
have h₂ : (Complex.exp (Complex.I * 2 * Real.pi / n)) ^ n = Complex.exp
→ (Complex.I * 2 * Real.pi) := by
calc
(Complex.exp (Complex.I * 2 * Real.pi / n)) ^ n = Complex.exp (n *
→ (Complex.I * 2 * Real.pi / n)) := by
rw [-Complex.exp_nat_mul]
<> ring_nf
_ = Complex.exp (Complex.I * 2 * Real.pi) := by
have h₃ : (n : ℂ) * (Complex.I * 2 * Real.pi / n) = Complex.I * 2 *
→ Real.pi := by
field_simp [Nat.cast_ne_zero.mpr (by linearith : n ≠ 0)]
<> ring_nf
<> simp [Complex.ext_iff, pow_two]
<> norm_num
rw [h.]
rw [h.]
have h₄ : Complex.exp (Complex.I * 2 * Real.pi) = 1 := by
rw [Complex.eq_one_iff]
use 1
<> simp [Complex.ext_iff, pow_two]
<> ring_nf
<> norm_num
<> field_simp [Real.pi_pos.le]
<> ring_nf
<> norm_num
rw [h.]
have h_recurrence : ∀ (k : ℕ) (z : ℂ), R k + 1 z = (Complex.exp (Complex.I *
→ 2 * Real.pi / n)) * R k z + ((k + 1 : ℂ) * (1 - Complex.exp
→ (Complex.I * 2 * Real.pi / n))) := by
intro k z
have h₅ : R (k + 1) = R k + 1 · R k := hr.2 k
have h₆ : R k = fun (c : ℕ) (Q : ℂ) => (k : c) + Complex.exp (Complex.I * 2 *
→ Real.pi / n) * (Q - (k : c)) := by
rw [hRk]
<> simp [Complex.ext_iff]
<> norm_cast
<> simp_all [Complex.ext_iff]
<> ring_nf
<> norm_num
<> simp_all [Complex.ext_iff]
<> norm_cast
have h₇ : R (k + 1) z = R k (k + 1) (R k z) := by
rw [h.]
<> simp [Function.comp_apply]
rw [h.]
have h₈ : R k (k + 1) (R k z) = ((k + 1 : ℕ) : c) + Complex.exp (Complex.I *
→ 2 * Real.pi / n) * (R k z - ((k + 1 : ℕ) : c)) := by
rw [h.]
<> simp [Complex.ext_iff]
<> norm_cast
<> simp_all [Complex.ext_iff]
<> ring_nf
<> norm_num
<> simp_all [Complex.ext_iff]
<> norm_cast
rw [h.]
have h₉ : ((k + 1 : ℕ) : c) + Complex.exp (Complex.I * 2 * Real.pi / n) *
→ (R k z - ((k + 1 : ℕ) : c)) = (Complex.exp (Complex.I * 2 * Real.pi /
→ n)) * R k z + ((k + 1 : c) * (1 - Complex.exp (Complex.I * 2 *
→ Real.pi / n))) := by
ring_nf at *
<> simp [Complex.ext_iff, pow_two] at *
<> norm_num at *
<>
{ try {
field_simp [Complex.ext_iff, pow_two] at *
<> ring_nf at *
<> norm_num at *
<> simp_all [Complex.ext_iff, pow_two]
<> norm_num
<> linarith
} }
<>
{ try {
simp_all [Complex.ext_iff, pow_two]
<> norm_num
<> linarith
} }
<>
{ try {
ring_nf at *
<> simp_all [Complex.ext_iff, pow_two]
<> norm_num

```

```

<|> ring_nf at *
<|> simp_all [Complex.ext_iff, pow_two]
<|> norm_num
<|> linarith [Real.pi_pos]
})
<|>
{
  simp_all [Complex.ext_iff, pow_two]
  <|> norm_num
  <|> linarith [Real.pi_pos]
}
rw [h]
<|> simp [pow_succ]
<|>
{
  (try ring_nf) <|>
  (try simp_all [Complex.ext_iff, pow_two]) <|>
  (try norm_num) <|>
  (try linarith [Real.pi_pos])
}
have h_main : ∀ (z : ℂ), R n z = z + (n : ℂ) := by
  intro z
  have h : R n z = (Complex.exp (Complex.I * 2 * Real.pi / n)) ^ n * z +
    → ((Complex.exp (Complex.I * 2 * Real.pi / n)) ^ (n + 1) - Complex.exp
    → (Complex.I * 2 * Real.pi / n)) / (1 - Complex.exp (Complex.I * 2 *
    → Real.pi / n)) + (n : ℂ) := by
    have h₁ : = h_inductive_formula n z
    exact h
  rw [h]
  have h₂ : (Complex.exp (Complex.I * 2 * Real.pi / n)) ^ n = 1 := h_pow_n
  rw [h]
  have h₃ : (Complex.exp (Complex.I * 2 * Real.pi / n)) ^ (n + 1) =
    → Complex.exp (Complex.I * 2 * Real.pi / n) := by
    calc
      (Complex.exp (Complex.I * 2 * Real.pi / n)) ^ (n + 1) = (Complex.exp
      → (Complex.I * 2 * Real.pi / n)) ^ n * Complex.exp (Complex.I * 2 *
      → Real.pi / n) := by
        ring_nf
        <|> simp [pow_succ]
        <|> ring_nf
        = 1 * Complex.exp (Complex.I * 2 * Real.pi / n) := by rw [h₁]
        = Complex.exp (Complex.I * 2 * Real.pi / n) := by ring_nf
  have h₄ : ((Complex.exp (Complex.I * 2 * Real.pi / n)) ^ (n + 1) -
    → Complex.exp (Complex.I * 2 * Real.pi / n)) / (1 - Complex.exp
    → (Complex.I * 2 * Real.pi / n)) = 0 := by
    rw [h]
    have h₅ : (Complex.exp (Complex.I * 2 * Real.pi / n) - Complex.exp
    → (Complex.I * 2 * Real.pi / n)) / (1 - Complex.exp (Complex.I * 2 *
    → Real.pi / n)) = 0 := by
      have h₆ : Complex.exp (Complex.I * 2 * Real.pi / n) - Complex.exp
      → (Complex.I * 2 * Real.pi / n) = 0 := by ring_nf
      rw [h]
      <|> simp [div_eq_mul_inv]
      <|> ring_nf
      simp using h
    rw [h]
    <|> ring_nf
    <|> simp [Complex.ext_iff, pow_two]
    <|> norm_num
    <|>
    {
      (try {
        simp_all [Complex.ext_iff, pow_two]
        <|> norm_num
        <|> linarith [Real.pi_pos]
      })
    }
  )
  have h_final : (R n = ((fun n z => z + n) : ℕ → ℂ → ℂ) n) := by
  funext z
  have h : R n z = z + (n : ℂ) := h_main z
  have h₁ : (((fun n z => z + n) : ℕ → ℂ → ℂ) n) z = z + (n : ℂ) := by
    simp [Complex.ext_iff]
    <|> norm_cast
    <|> simp_all [Complex.ext_iff]
    <|> ring_nf
    <|> norm_num
    <|>
    {
      (try {
        simp_all [Complex.ext_iff, pow_two]
        <|> norm_num
        <|> linarith [Real.pi_pos]
      })
    }
  rw [h, h₁]
  exact h_final
-- Simplified Proof
import Mathlib
import Aesop
set_option maxHeartbeats 0
open Nat Topology Filter
theorem putnam_2004_b4
  (n : ℕ)
  (nge2 : n ≥ 2)
  (R Rk : ℕ → ℂ → ℂ)
  (hR : R 0 = id ∧ ∀ k : ℕ, R (k + 1) = Rk (k + 1) ∘ R k)
  (hRk : Rk = fun (k : ℕ) (Q : ℂ) => k + Complex.exp (Complex.I * 2 * Real.pi /
    → n) * (Q - k))
  : (R n = ((fun n z => z + n) : ℕ → ℂ → ℂ) n) := by
  have h : Complex.exp (Complex.I * 2 * Real.pi / n) ≠ 1 := by
    intro h
    have h₁ : Complex.exp (Complex.I * 2 * Real.pi / n) = 1 := h
    have h₂ : (k : ℤ) < (Complex.I * 2 * Real.pi / n : ℂ) = (k : ℂ) * (2 *
    → Real.pi * Complex.I) := by
      rw [Complex.exp_eq_one_iff] at h₁
    exact h
    obtain k, hk := h
    have h₃ : (2 * Real.pi / n : ℝ) = (2 * Real.pi * k : ℝ) := by
      have h₄ : = hk
      simp [Complex.ext_iff, Complex.I_mul_I, mul_assoc, mul_comm,
      → mul_left_comm] at h
    <|> (try ring_nf at h) <|> (try norm_num at h)

```



```

{I | f : R → R, ContinuousOn f (Icc 0 1) ∧ I f - J f = y}
((1 / 16 : ℝ) := by
have h_main : IsGreatest {y | f : R → R, ContinuousOn f (Icc 0 1) ∧ I f - J f = y}
→ f y} (1 / 16 : ℝ) := by
constructor

have h : (f : R → R), ContinuousOn f (Icc 0 1) ∧ I f - J f = (1 / 16 :
→ ℝ) := by
use fun x => x / 2
constructor

apply ContinuousOn.div
exact continuousOn_id
exact continuousOn_const
intro x hx
norm_num at hx
<> linarith

have h : I (fun x => x / 2) = f x in (0)..1, x ^ 2 * (x / 2 : ℝ) :=
by
rw [hI]
<> simp [mul_assoc]
<> congr 1 <> ext x <> ring_nf
have h : J (fun x => x / 2) = f x in (0)..1, x * (x / 2 : ℝ) ^ 2 :=
by
rw [hJ]
<> simp [mul_assoc]
<> congr 1 <> ext x <> ring_nf
rw [h, hI]
have h : (f x in (0)..1, x ^ 2 * (x / 2 : ℝ)) = 1 / 8 := by
norm_num [intervalIntegral.integral_comp_mul_left (fun x => x ^ 2)]
<> ring_nf
<> norm_num
<> linarith
have h : (f x in (0)..1, x * (x / 2 : ℝ) ^ 2) = 1 / 16 := by
norm_num [intervalIntegral.integral_comp_mul_left (fun x => x ^ 2)]
<> ring_nf
<> norm_num
<> linarith
rw [h, hI]
norm_num

rcases h with (f, hf_cont, hf_eq)
refine' (f, hf_cont, _)
linarith

rintro y (f, hf_cont, rfl)
have h : I f - J f ≤ 1 / 16 := by
have h : I f = f x in (0)..1, x ^ 2 * f x := by
rw [hI]
<> simp [mul_assoc]
<> congr 1 <> ext x <> ring_nf
have h : J f = f x in (0)..1, x * (f x) ^ 2 := by
rw [hJ]
<> simp [mul_assoc]
<> congr 1 <> ext x <> ring_nf
rw [h, hI]
have h : f x in (0)..1, x ^ 2 * f x - x * (f x) ^ 2 ≤ 1 / 16 := by
have h : f x in (0)..1, x ^ 2 * f x - x * (f x) ^ 2 ≤ 1 / 16 := by
have h : ∀ x ∈ Set.Icc (0 : ℝ) 1, x ^ 2 * f x - x * (f x) ^ 2 ≤ x ^
→ 3 / 4 := by
intro x hx
have h : 0 ≤ x := by exact hx.1
have h : x ≤ 1 := by exact hx.2
have h : x ^ 2 * f x - x * (f x) ^ 2 ≤ x ^ 3 / 4 := by
nlinarith [sq_nonneg (f x - x / 2), mul_nonneg h (sq_nonneg (f x
→ x / 2))]
exact h

have h : f x in (0)..1, x ^ 2 * f x - x * (f x) ^ 2 ≤ f x in (0)..1,
→ x ^ 3 / 4 := by
have h : ContinuousOn (fun x : ℝ => x ^ 2 * f x - x * (f x) ^ 2)
→ (Set.Icc 0 1) := by
apply ContinuousOn.sub
· apply ContinuousOn.mul
· exact continuousOn_pow 2
· exact hf_cont
· apply ContinuousOn.mul
· exact continuousOn_id
· apply ContinuousOn.pow
· exact hf_cont
<> norm_num
have h : ContinuousOn (fun x : ℝ => x ^ 3 / 4 : ℝ → ℝ) (Set.Icc 0
→ 1) := by
apply ContinuousOn.div
· exact continuousOn_pow 3
· exact continuousOn_const
· intro x hx
norm_num
<> linarith [hx.1, hx.2]
have h : ∀ x ∈ Set.Icc (0 : ℝ) 1, x ^ 2 * f x - x * (f x) ^ 2 ≤ x
→ ^ 3 / 4 := h

have h : IntervalIntegrable (fun x : ℝ => x ^ 2 * f x - x * (f x)
→ ^ 2) MeasureTheory.volume 0 1 := by
have h : ContinuousOn (fun x : ℝ => x ^ 2 * f x - x * (f x) ^
→ 2) (Set.Icc 0 1) := h
have h : ContinuousOn (fun x : ℝ => x ^ 2 * f x - x * (f x) ^
→ 2) (Set.uIcc 0 1) := by
apply ContinuousOn.mono h
<> simp [Set.Icc_subset_uIcc]
exact ContinuousOn.intervalIntegrable h
have h : IntervalIntegrable (fun x : ℝ => x ^ 3 / 4 : ℝ → ℝ)
→ MeasureTheory.volume 0 1 := by
have h : ContinuousOn (fun x : ℝ => x ^ 3 / 4 : ℝ → ℝ) (Set.Icc
→ 0 1) := h
have h : ContinuousOn (fun x : ℝ => x ^ 3 / 4 : ℝ → ℝ)
→ (Set.uIcc 0 1) := by
apply ContinuousOn.mono h
<> simp [Set.Icc_subset_uIcc]
exact ContinuousOn.intervalIntegrable h

have h : (0 : ℝ) ≤ 1 := by norm_num
have h : f x in (0)..1, x ^ 2 * f x - x * (f x) ^ 2 ≤ f x in
→ (0)..1, x ^ 3 / 4 := by
apply intervalIntegral.integral_mono_on h
<> (try assumption)
<> (try
{
exact h
})
<> (try
{
exact h
})
<> (try
{
intro x hx
exact h, x (by linarith [hx.1, hx.2], by linarith [hx.1,
→ hx.2])
})
exact h
have h : f x in (0)..1, (x : ℝ) ^ 3 / 4 = 1 / 16 := by
norm_num [integral_pow]
<> ring_nf
<> norm_num
<> linarith
calc
f x in (0)..1, x ^ 2 * f x - x * (f x) ^ 2 ≤ f x in (0)..1, x ^ 3 /
→ 4 := h
_ = 1 / 16 := by rw [h]

have h : IntervalIntegrable (fun x : ℝ => x ^ 2 * f x)
→ MeasureTheory.volume 0 1 := by
have h : ContinuousOn (fun x : ℝ => x ^ 2 * f x) (Set.Icc 0 1) := by
apply ContinuousOn.mul
exact continuousOn_pow 2
exact hf_cont
have h : ContinuousOn (fun x : ℝ => x ^ 2 * f x) (Set.uIcc 0 1) :=
→ by
apply ContinuousOn.mono h
<> simp [Set.Icc_subset_uIcc]
exact ContinuousOn.intervalIntegrable h
have h : IntervalIntegrable (fun x : ℝ => x * (f x) ^ 2)
→ MeasureTheory.volume 0 1 := by
have h : ContinuousOn (fun x : ℝ => x * (f x) ^ 2) (Set.Icc 0 1) :=
→ by
apply ContinuousOn.mul
exact continuousOn_id
apply ContinuousOn.pow
exact hf_cont
<> norm_num
have h : ContinuousOn (fun x : ℝ => x * (f x) ^ 2) (Set.uIcc 0 1) :=
→ by
apply ContinuousOn.mono h
<> simp [Set.Icc_subset_uIcc]
exact ContinuousOn.intervalIntegrable h
have h : (f x in (0)..1, x ^ 2 * f x) - f x in (0)..1, x * (f x) ^ 2 =
→ f x in (0)..1, x ^ 2 * f x - x * (f x) ^ 2 := by
rw [intervalIntegral.integral_sub h, h]
rw [h]
exact h
exact h
exact h
exact h_main
-- Simplified Proof
import Mathlib
import Aesop

set_option maxHeartbeats 0

open Set

theorem putnam_2006_b5
(I J : ℝ → ℝ) → ℝ
(hI : I = fun f => f x in (0)..1, x ^ 2 * (f x))
(hJ : J = fun f => f x in (0)..1, x * (f x) ^ 2) :
IsGreatest
{y | f : ℝ → ℝ, ContinuousOn f (Icc 0 1) ∧ I f - J f = y}
((1 / 16 : ℝ) := by
constructor
use fun x => x / 2
constructor
· apply ContinuousOn.div
· exact continuousOn_id
· exact continuousOn_const
· intro x hx
norm_num at hx
· norm_num [hI, hJ, intervalIntegral.integral_comp_mul_left]
<> ring_nf
<> norm_num
rintro y (f, hf_cont, rfl)
have h : I f - J f ≤ 1 / 16 := by
have h : I f = f x in (0)..1, x ^ 2 * f x := by rw [hI]
have h : J f = f x in (0)..1, x * (f x) ^ 2 := by rw [hJ]
rw [h, hI]
have h : f x in (0)..1, x ^ 2 * f x - x * (f x) ^ 2 ≤ 1 / 16 := by
have h : ∀ x ∈ Set.Icc (0 : ℝ) 1, x ^ 2 * f x - x * (f x) ^ 2 ≤ x ^
→ 3 / 4 := by
intro x hx
have h : 0 ≤ x := by exact hx.1
have h : x ≤ 1 := by exact hx.2
nlinarith [sq_nonneg (f x - x / 2), mul_nonneg h (sq_nonneg (f x -
→ x / 2))]
exact h
have h : IntervalIntegrable (fun x : ℝ => x ^ 2 * f x - x * (f x)
→ ^ 2) MeasureTheory.volume 0 1 := by
have h : ContinuousOn (fun x : ℝ => x ^ 2 * f x - x * (f x) ^
→ 2) (Set.Icc 0 1) := h
have h : ContinuousOn (fun x : ℝ => x ^ 2 * f x - x * (f x) ^
→ 2) (Set.uIcc 0 1) := by
apply ContinuousOn.mono h
<> simp [Set.Icc_subset_uIcc]
exact ContinuousOn.intervalIntegrable h
have h : IntervalIntegrable (fun x : ℝ => x ^ 3 / 4 : ℝ → ℝ)
→ MeasureTheory.volume 0 1 := by
have h : ContinuousOn (fun x : ℝ => x ^ 3 / 4 : ℝ → ℝ) (Set.Icc
→ 0 1) := h
have h : ContinuousOn (fun x : ℝ => x ^ 3 / 4 : ℝ → ℝ)
→ (Set.uIcc 0 1) := by
apply ContinuousOn.mono h
<> simp [Set.Icc_subset_uIcc]
exact ContinuousOn.intervalIntegrable h
have h : (0 : ℝ) ≤ 1 := by norm_num
have h : f x in (0)..1, x ^ 2 * f x - x * (f x) ^ 2 ≤ f x in
→ (0)..1, x ^ 3 / 4 := by
have h : ContinuousOn (fun x : ℝ => x ^ 2 * f x - x * (f x) ^ 2)
→ (Set.Icc 0 1) := by
apply ContinuousOn.sub
· apply ContinuousOn.mul
· exact continuousOn_pow 2
· exact hf_cont
· apply ContinuousOn.mul
· exact continuousOn_id
· apply ContinuousOn.pow
· exact hf_cont
<> norm_num
have h : ContinuousOn (fun x : ℝ => x ^ 3 / 4 : ℝ → ℝ) (Set.Icc 0
→ 1) := by
apply ContinuousOn.div
· exact continuousOn_pow 3
· exact continuousOn_const
· intro x hx
norm_num
<> linarith [hx.1, hx.2]
have h : ∀ x ∈ Set.Icc (0 : ℝ) 1, x ^ 2 * f x - x * (f x) ^ 2 ≤ x
→ ^ 3 / 4 := h

have h : IntervalIntegrable (fun x : ℝ => x ^ 2 * f x - x * (f x)
→ ^ 2) MeasureTheory.volume 0 1 := by
have h : ContinuousOn (fun x : ℝ => x ^ 2 * f x - x * (f x) ^
→ 2) (Set.Icc 0 1) := h
have h : ContinuousOn (fun x : ℝ => x ^ 2 * f x - x * (f x) ^
→ 2) (Set.uIcc 0 1) := by
apply ContinuousOn.mono h
<> simp [Set.Icc_subset_uIcc]
exact ContinuousOn.intervalIntegrable h
have h : IntervalIntegrable (fun x : ℝ => x ^ 3 / 4 : ℝ → ℝ)
→ MeasureTheory.volume 0 1 := by
have h : ContinuousOn (fun x : ℝ => x ^ 3 / 4 : ℝ → ℝ) (Set.Icc
→ 0 1) := h
have h : ContinuousOn (fun x : ℝ => x ^ 3 / 4 : ℝ → ℝ)
→ (Set.uIcc 0 1) := by
apply ContinuousOn.mono h
<> simp [Set.Icc_subset_uIcc]
exact ContinuousOn.intervalIntegrable h

have h : (0 : ℝ) ≤ 1 := by norm_num
have h : f x in (0)..1, x ^ 2 * f x - x * (f x) ^ 2 ≤ f x in
→ (0)..1, x ^ 3 / 4 := by
have h : ContinuousOn (fun x : ℝ => x ^ 2 * f x - x * (f x) ^ 2)
→ (Set.Icc 0 1) := by
apply ContinuousOn.sub
· apply ContinuousOn.mul
· exact continuousOn_pow 2
· exact hf_cont
· apply ContinuousOn.mul
· exact continuousOn_id
· apply ContinuousOn.pow
· exact hf_cont
<> norm_num
have h : ContinuousOn (fun x : ℝ => x * (f x) ^ 2) (Set.uIcc 0 1) :=
→ by
apply ContinuousOn.mono h
<> simp [Set.Icc_subset_uIcc]
exact ContinuousOn.intervalIntegrable h
have h : IntervalIntegrable (fun x : ℝ => x * (f x) ^ 2)
→ MeasureTheory.volume 0 1 := by
have h : ContinuousOn (fun x : ℝ => x * (f x) ^ 2) (Set.Icc 0 1) :=
→ by
apply ContinuousOn.mul
exact continuousOn_id
apply ContinuousOn.pow
exact hf_cont
<> norm_num
have h : ContinuousOn (fun x : ℝ => x * (f x) ^ 2) (Set.uIcc 0 1) :=
→ by
apply ContinuousOn.mono h
<> simp [Set.Icc_subset_uIcc]
exact ContinuousOn.intervalIntegrable h
have h : (f x in (0)..1, x ^ 2 * f x) - f x in (0)..1, x * (f x) ^ 2 =
→ f x in (0)..1, x ^ 2 * f x -
```

```

    . apply ContinuousOn.mul
    . exact continuousOn_pow 2
    . exact hf_cont
    . apply ContinuousOn.mul
    . exact continuousOn_id
    . apply ContinuousOn.pow
    . exact hf_cont
  have h10 : ContinuousOn (fun x : ℝ => x ^ 3 / 4 : ℝ → ℝ) (Set.Icc 0
→ 1) := by
    . apply ContinuousOn.div
    . exact continuousOn_pow 3
    . exact continuousOn_const
    . intro x hx
      norm_num
  have h11 : ∀ x ∈ Set.Icc (0 : ℝ) 1, x ^ 2 * f x - x * (f x) ^ 2 ≤ x ^
→ 3 / 4 := h1
  have h12 : IntervalIntegrable (fun x : ℝ => x ^ 2 * f x - x * (f x) ^
→ 2) MeasureTheory.volume 0 1 := by
    . apply ContinuousOn.intervalIntegrable
    . apply ContinuousOn.mono h1
    . simp [Set.Icc_subset_uIcc]
  have h13 : IntervalIntegrable (fun x : ℝ => x ^ 3 / 4 : ℝ → ℝ)
→ MeasureTheory.volume 0 1 := by
    . apply ContinuousOn.intervalIntegrable
    . apply ContinuousOn.mono h10
    . simp [Set.Icc_subset_uIcc]
  have h14 : (0 : ℝ) ≤ 1 := by norm_num
  apply intervalIntegral.integral_mono_on h14
  <|> assumption
  have h15 : ∫ x in (0)..1, (x : ℝ) ^ 3 / 4 = 1 / 16 := by
    . norm_num [integral_pow]
  calc
    ∫ x in (0)..1, x ^ 2 * f x - x * (f x) ^ 2 ≤ ∫ x in (0)..1, x ^ 3 / 4
→ := h15
    _ = 1 / 16 := by rw [h15]
  have h1 : IntervalIntegrable (fun x : ℝ => x ^ 2 * f x)
→ MeasureTheory.volume 0 1 := by
    . have h11 : ContinuousOn (fun x : ℝ => x ^ 2 * f x) (Set.Icc 0 1) := by
        . apply ContinuousOn.mul
        . exact continuousOn_pow 2
        . exact hf_cont
    . apply ContinuousOn.intervalIntegrable
    . apply ContinuousOn.mono h11
    . simp [Set.Icc_subset_uIcc]
  have h1 : IntervalIntegrable (fun x : ℝ => x * (f x) ^ 2)
→ MeasureTheory.volume 0 1 := by
    . have h11 : ContinuousOn (fun x : ℝ => x * (f x) ^ 2) (Set.Icc 0 1) := by
        . apply ContinuousOn.mul
        . exact continuousOn_id
        . apply ContinuousOn.pow
        . exact hf_cont
    . apply ContinuousOn.intervalIntegrable
    . apply ContinuousOn.mono h11
    . simp [Set.Icc_subset_uIcc]
  have h1 : (∫ x in (0)..1, x ^ 2 * f x) - ∫ x in (0)..1, x * (f x) ^ 2 = ∫
→ x in (0)..1, x ^ 2 * f x - x * (f x) ^ 2 := by
    . rw [intervalIntegral.integral_sub h1 h1]
  rw [h1]
  exact h1
  linarith
-----

```







```

→ n) / (2 * n)) + n) = 1 := by
  have h₁ : n ≠ 0 := h₁
  field_simp [h₁]
  <|> ring_nf
  <|> nlinarith [Real.sqrt_nonneg 601, Real.sq_sqrt (show 0 ≤
→ 601 by norm_num)]
  exact h₁
exact h₁

```



```

exact h1
| inr h2 =>
cases h2 with
| inl h2 =>
have h3 : # = 3 / 2 := h2
have h4 : ∃ (x y : ℝ), (x * x ^ 2 + # * x + 1 / 24 : ℝ) = y ^ 2 := by
  use # * y + 1 / 24 : ℝ := x ^ 2 + # * x + # * (2 * # * y + #) = 1 := by
    use -1 / 6, -1 / 6
    rw [h3]
    norm_num
exact h2
| inr h2 =>
cases h2 with
| inl h2 =>
have h3 : # = (13 + Real.sqrt 601) / 12 := h2
have h4 : ∃ (x y : ℝ), (x * x ^ 2 + # * x + 1 / 24 : ℝ) = y ^ 2 := by
  use 2 + # * y + 1 / 24 : ℝ := x ^ 2 + (2 * # * x + #) * (2 * # * y + #) = 1 :=
  by
    use (-1 - #) / (2 * #), (-1 - #) / (2 * #)
    constructor
    have h5 : (x : ℝ) * ((-1 - #) / (2 * #)) ^ 2 + # * ((-1 - #) / (2 *
    → #)) + 1 / 24 = (-1 - #) / (2 * #) := by
      have h6 : # ≠ 0 := by
        rw [h3]
        nlinarith [Real.sqrt_nonneg 601, Real.sqrt_sqrt (show 0 ≤ 601
        → by norm_num)]
      have h7 : 6 * # ^ 2 - 13 * # - 18 = 0 := by
        rw [h3]
        nlinarith [Real.sqrt_sqrt (show 0 ≤ 601 by norm_num)]
      field_simp [h7]
      nlinarith
      have h8 : (x : ℝ) * ((-1 - #) / (2 * #)) ^ 2 + (# - 1) * ((-1 - #
      → ) / (2 * #)) + 1 / 24 = 0 := by
        have h9 : (x : ℝ) * ((-1 - #) / (2 * #)) ^ 2 + (# - 1) * ((-1
        → - #) / (2 * #)) + 1 / 24 = (3 + 2 * # - # ^ 2) / (4 * #) + 1 / 24 := by
          field_simp [h7]
          <> ring_nf
          rw [h8]
          nlinarith
          have h10 : (x : ℝ) * ((-1 - #) / (2 * #)) ^ 2 + # * ((-1 - #) /
          → (2 * #)) + 1 / 24 = (-1 - #) / (2 * #) := by
            nlinarith
            exact h10
            exact h1
            constructor
            have h11 : (x : ℝ) * ((-1 - #) / (2 * #)) ^ 2 + # * ((-1 - #) /
            → (2 * #)) + 1 / 24 = (-1 - #) / (2 * #) := by
              have h12 : # ≠ 0 := by
                rw [h3]
                nlinarith [Real.sqrt_nonneg 601, Real.sqrt_sqrt (show 0 ≤
                → 601 by norm_num)]
              have h13 : 6 * # ^ 2 - 13 * # - 18 = 0 := by
                rw [h3]
                nlinarith [Real.sqrt_sqrt (show 0 ≤ 601 by norm_num)]
              field_simp [h13]
              nlinarith
              have h14 : (x : ℝ) * ((-1 - #) / (2 * #)) ^ 2 + (# - 1) * ((-1
              → - #) / (2 * #)) + 1 / 24 = 0 := by
                have h15 : (x : ℝ) * ((-1 - #) / (2 * #)) ^ 2 + (# - 1) *
                → ((-1 - #) / (2 * #)) + 1 / 24 = (3 + 2 * # - # ^ 2) / (4 * #) + 1 / 24
                := by
                  field_simp [h13]
                  <> ring_nf
                  rw [h14]
                  nlinarith
                  have h16 : (x : ℝ) * ((-1 - #) / (2 * #)) ^ 2 + # * ((-1 - #)
                  → / (2 * #)) + 1 / 24 = (-1 - #) / (2 * #) := by
                    nlinarith
                    exact h16
                    nlinarith
                    have h17 : (2 * # * ((-1 - #) / (2 * #)) + #) * (2 * # * ((-1 - #
                    → ) / (2 * #)) + #) = 1 := by
                      have h18 : # ≠ 0 := by
                        rw [h3]
                        nlinarith [Real.sqrt_nonneg 601, Real.sqrt_sqrt (show 0 ≤
                        → 601 by norm_num)]
                      field_simp [h18]
                      exact h17
                      exact h1
                      constructor
                      | inr h2 =>
                        have h19 : # = (13 - Real.sqrt 601) / 12 := h2
                        have h20 : ∃ (x y : ℝ), (x * x ^ 2 + # * x + 1 / 24 : ℝ) = y ^ 2 := by
                          use 2 + # * y + 1 / 24 : ℝ := x ^ 2 + # * x + # * (2 * # * y + #) = 1 :=
                          by
                            use (-1 - #) / (2 * #), (-1 - #) / (2 * #)
                            constructor
                            have h21 : (x : ℝ) * ((-1 - #) / (2 * #)) ^ 2 + # * ((-1 - #) / (2 *
                            → #)) + 1 / 24 = (-1 - #) / (2 * #) := by
                              have h22 : # ≠ 0 := by
                                rw [h3]
                                nlinarith [Real.sqrt_nonneg 601, Real.sqrt_sqrt (show 0 ≤ 601
                                → by norm_num)]
                              have h23 : 6 * # ^ 2 - 13 * # - 18 = 0 := by
                                rw [h3]
                                nlinarith [Real.sqrt_sqrt (show 0 ≤ 601 by norm_num)]
                              field_simp [h23]
                              nlinarith
                              have h24 : (x : ℝ) * ((-1 - #) / (2 * #)) ^ 2 + (# - 1) * ((-1 - #
                              → ) / (2 * #)) + 1 / 24 = 0 := by
                                have h25 : (x : ℝ) * ((-1 - #) / (2 * #)) ^ 2 + (# - 1) * ((-1
                                → - #) / (2 * #)) + 1 / 24 = (3 + 2 * # - # ^ 2) / (4 * #) + 1 / 24 := by
                                  field_simp [h23]
                                  <> ring_nf
                                  rw [h24]
                                  nlinarith
                                  have h26 : (x : ℝ) * ((-1 - #) / (2 * #)) ^ 2 + # * ((-1 - #) /
                                  → (2 * #)) + 1 / 24 = (-1 - #) / (2 * #) := by
                                    nlinarith
                                    exact h26
                                    nlinarith

```

```

-- Orig Proof
import Mathlib
import Aesop

set_option maxHeartbeats 0

theorem putnam_2008_a1
(f : ℝ → ℝ → ℝ)
(hf : ∀ x y z : ℝ, f x y + f y z + f z x = 0)
: ∃ g : ℝ → ℝ, ∀ x y : ℝ, f x y = g x - g y := by
  have h_f_zero_zero : f 0 0 = 0 := by
    have h1 : f 0 0 + f 0 0 + f 0 0 = 0 := by
      have h2 := hf 0 0 0
      linarith
    linarith
  have h_f_x_zero_plus_f_zero_x : ∀ (x : ℝ), f x 0 + f 0 x = 0 := by
    intro x
    have h1 : f x 0 + f 0 0 + f 0 x = 0 := by
      have h2 := hf x 0 0
      linarith
    have h3 : f 0 0 = 0 := h_f_zero_zero
    linarith
  have h_main : ∃ (g : ℝ → ℝ), ∀ (x y : ℝ), f x y = g x - g y := by
    use fun x => f x 0
    intro x y
    have h1 : f x y + f y 0 + f 0 x = 0 := by
      have h2 := hf x y 0
      linarith
    have h2 : f x 0 + f 0 x = 0 := h_f_x_zero_plus_f_zero_x x
    have h3 : f 0 x = -f x 0 := by linarith
    have h4 : f x y + f y 0 + f 0 x = 0 := h1
    rw [h3] at h4
    linarith
  exact h_main

-- Simplified Proof
import Mathlib
import Aesop

set_option maxHeartbeats 0

theorem putnam_2008_a1
(f : ℝ → ℝ → ℝ)
(hf : ∀ x y z : ℝ, f x y + f y z + f z x = 0)
: ∃ g : ℝ → ℝ, ∀ x y : ℝ, f x y = g x - g y := by
  use fun x => f x 0
  intro x y
  linarith [hf x y 0, hf 0 0 0, hf 0 0 x]

-- Orig Proof
import Mathlib
import Aesop

set_option maxHeartbeats 0

open Topology MvPolynomial Filter

theorem putnam_2009_a1
: ((f : (ℝ × ℝ) → ℝ, (∀ 0 v : ℝ × ℝ, v ≠ (0, 0) → f (0.1, 0.2) + f (0.1 +
  → v.1, 0.2 + v.2) + f (0.1 + v.1 - v.2, 0.2 + v.2 + v.1) + f (0.1 -
  → v.2, 0.2 + v.1) = 0) → ∃ P : ℝ × ℝ, f P = 0) ↔ ((True) : Prop)) := by
  constructor
  · intro h
    · trivial
  · rintro h f hf
    have h1 : ∃ x y, f (x, y) = 0 := by
      intro x y
      have h2 := hf (0, 0) (1, 0)
      have h3 := hf (0, 0) (0, 1)
      have h4 := hf (0, 0) (1, 1)
      have h5 := hf (1, 0) (0, 1)
      have h6 := hf (0, 1) (1, 0)
      have h7 := hf (x, y) (1, 0)
      have h8 := hf (x, y) (0, 1)
      have h9 := hf (x, y) (1, 1)
      have h10 := hf (x + 1, y) (0, 1)
      have h11 := hf (x, y + 1) (1, 0)
      have h12 := hf (x, y) (2, 0)
      have h13 := hf (x, y) (0, 2)
      have h14 := hf (x, y) (1, -1)
      have h15 := hf (x, y) (2, 1)
      have h16 := hf (x, y) (1, 2)
      have h17 := hf (x + 1, y + 1) (1, 0)
      have h18 := hf (x + 1, y + 1) (0, 1)
      have h19 := hf (x + 1, y + 1) (1, 1)
      have h20 := hf (x - 1, y) (1, 0)
      have h21 := hf (x, y - 1) (0, 1)
      have h22 := hf (x + 1, y) (1, 0)
      have h23 := hf (x, y + 1) (0, 1)
      have h24 := hf (x - 1, y - 1) (1, 0)
      have h25 := hf (x - 1, y - 1) (0, 1)
      norm_num [Prod.ext_iff] at h2 h3 h4 h5 h6 h7 h8 h9 h10 h11 h12 h13 h14
      → h15 h16 h17 h18 h19 h20 h21 h22 h23 h24 h25
      <|> ring_nf at h2 h3 h4 h5 h6 h7 h8 h9 h10 h11 h12 h13 h14 h15 h16 h17
      → h18 h19 h20 h21 h22 h23 h24 h25
      <|> linarith
    simp [h1]

-- Orig Proof
import Mathlib
import Aesop

set_option maxHeartbeats 0

theorem putnam_2010_a3
(h : ℝ × ℝ → ℝ)
(a b M : ℝ)
(H : ContDiff ℝ 1 h)
(H' : ∀ x, h x = a * (fderiv ℝ h (1, 0) x) + (fderiv ℝ h (0, 1) x))
(H'' : ∀ x, |h x| ≤ M) : h = 0 := by
  have h_scaling : ∀ (x : ℝ × ℝ) (t : ℝ), h (t · x) = t * h x := by
    intro x t
    have h1 : h (t · x) = a * (fderiv ℝ h (1, 0)) (t · x) + (fderiv ℝ h (0, 1))
      → (t · x) := by
      have h2 := H' (t · x)
      simp using h2
    have h3 : (fderiv ℝ h (1, 0)) (t · x) = t * (fderiv ℝ h (1, 0)) x := by
      have h4 : (fderiv ℝ h (1, 0)) (t · x) = t * (fderiv ℝ h (1, 0)) x := by
        apply ContinuousLinearMap.map_smul
      simp [smul_eq_mul] at h4
      <|> linarith
    have h5 : (fderiv ℝ h (0, 1)) (t · x) = t * (fderiv ℝ h (0, 1)) x := by
      have h6 : (fderiv ℝ h (0, 1)) (t · x) = t * (fderiv ℝ h (0, 1)) x := by
        apply ContinuousLinearMap.map_smul
      simp [smul_eq_mul] at h6
      <|> linarith
    calc
      h (t · x) = a * (fderiv ℝ h (1, 0)) (t · x) + (fderiv ℝ h (0, 1)) (t · x)
      → := by rw [h1]
      _ = a * (t * (fderiv ℝ h (1, 0)) x) + t * (fderiv ℝ h (0, 1)) x := by rw
        → [h3, h5]
      _ = t * (a * (fderiv ℝ h (1, 0)) x + (fderiv ℝ h (0, 1)) x) := by ring
      _ = t * h x := by
        have h7 : h x = a * (fderiv ℝ h (1, 0)) x + (fderiv ℝ h (0, 1)) x :=
          → H' x

```



```

linarith
exact h1
have h2 : ∀ i : ℕ, (a i)^3 ≤ Real.sqrt 2 * (a i)^2 := by
  intro i
  have h2 : a i ≤ Real.sqrt 2 := h1 i
  by_cases h2 : a i ≥ 0
  · have h2 : 0 ≤ (a i)^2 := sq_nonneg (a i)
    nlinarith [Real.sqrt_nonneg 2, Real.sq_sqrt (show 0 ≤ 2 by norm_num),
      mul_nonneg h2 (Real.sqrt_nonneg 2)]
  · have h2 : (a i)^3 ≤ 0 := by
      have h2 : a i < 0 := by linarith
      have h2 : (a i)^3 < 0 := by
        have h2 : a i < 0 := h2
        have h2 : (a i)^2 > 0 := by nlinarith
        nlinarith [sq_pos_of_neg h2]
    linarith
  nlinarith
have h2 : ∑' i : ℕ, (a i)^3 ≤ Real.sqrt 2 * ∑' i : ℕ, (a i)^2 := by
  have h2 : Summable (fun i : ℕ => Real.sqrt 2 * (a i)^2) := by
    by_contra h2
    have h2 : ∑' i : ℕ, (a i)^2 = 0 := by
      simp using tsum_eq_zero_of_not_summable h2
    linarith
  have h2 : Summable (fun i : ℕ => Real.sqrt 2 * (a i)^2) := by
    exact Summable.mul_left (Real.sqrt 2) h2
  have h2 : Summable (fun i : ℕ => (a i)^3) := by
    by_contra h2
    have h2 : ∑' i : ℕ, (a i)^3 = 0 := by
      simp using tsum_eq_zero_of_not_summable h2
    linarith
  have h2 : ∑' i : ℕ, (a i)^3 ≤ Real.sqrt 2 * ∑' i : ℕ, (a i)^2 := h2
  have h2 : ∑' i : ℕ, (a i)^3 ≤ ∑' i : ℕ, (Real.sqrt 2 * (a i)^2) := by
    exact tsum_le_tsum h2 h2
  have h2 : ∑' i : ℕ, (Real.sqrt 2 * (a i)^2) = Real.sqrt 2 * ∑' i : ℕ, (a i)^2 := by
    rw [tsum_mul_left]
  linarith
have h2 : Real.sqrt 2 * ∑' i : ℕ, (a i)^2 = Real.sqrt 2 * 2 := by
  rw [h2]
  nlinarith [Real.sqrt_nonneg 2, Real.sq_sqrt (show 0 ≤ 2 by norm_num)]
  intro h
  exfalse
  exact h
=====
-- Orig Proof
import Mathlib
import Aesop

set_option maxHeartbeats 0

open Matrix

theorem putnam_2012_a2
(S : Type*) [CommSemigroup S]
(a b c : S)
(hS : ∀ x y : S, ∃ z : S, x * z = y)
(habc : a * c = b * c)
: a = b := by
  have h_exists_right_identity : ∃ (e : S), ∀ (x : S), x * e = x := by
    obtain (e, he) := hS a a
    use e
    intro x
    obtain (z, hz) := hS a x
    calc
      x * e = (a * z) * e := by rw [hz]
      _ = a * (z * e) := by
        rw [mul_assoc]
      _ = a * (e * z) := by
        rw [mul_comm (z : S) (e : S)]
      _ = (a * e) * z := by
        rw [mul_assoc]
      _ = a * z := by
        rw [he]
      _ = x := by
        rw [hz]
  have h_main : a = b := by
    obtain (e, he) := h_exists_right_identity
    obtain (d, hd) := hS c e
    calc
      a = a * e := by rw [he a]
      _ = a * (c * d) := by rw [hd]
      _ = (a * c) * d := by
        rw [mul_assoc]
      _ = (b * c) * d := by rw [habc]
      _ = b * (c * d) := by
        rw [mul_assoc]
      _ = b * e := by rw [hd]
      _ = b := by rw [he b]
  exact h_main
-- Simplified Proof
import Mathlib
import Aesop

set_option maxHeartbeats 0

open Matrix

theorem putnam_2012_a2
(S : Type*) [CommSemigroup S]
(a b c : S)
(hS : ∀ x y : S, ∃ z : S, x * z = y)
(habc : a * c = b * c)
: a = b := by
  obtain (e, he) := hS a a
  obtain (d, hd) := hS c e
  calc
    a = a * e := by rw [he a]
    _ = a * (c * d) := by rw [hd]
    _ = (a * c) * d := by
      rw [mul_assoc]
    _ = (b * c) * d := by rw [habc]
    _ = b * (c * d) := by
      rw [mul_assoc]
    _ = b * e := by rw [hd]
    _ = b := by rw [he b]
  exact h_main
=====
(habc : a * c = b * c)
: a = b := by
  obtain (e, he) := hS a a
  have h1 : ∀ x, x * e = x := by
    intro x
    obtain (z, hz) := hS a x
    calc
      x * e = (a * z) * e := by rw [hz]
      _ = a * (z * e) := by
        rw [mul_assoc]
      _ = a * (e * z) := by
        rw [mul_comm (z : S) (e : S)]
      _ = (a * e) * z := by
        rw [mul_assoc]
      _ = a * z := by
        rw [he]
      _ = x := by
        rw [hz]
  obtain (d, hd) := hS c e
  calc
    a = a * e := by rw [he a]
    _ = a * (c * d) := by rw [hd]
    _ = (a * c) * d := by
      rw [mul_assoc]
    _ = (b * c) * d := by rw [habc]
    _ = b * (c * d) := by
      rw [mul_assoc]
    _ = b * e := by rw [hd]
    _ = b := by rw [he b]
  exact h_main
=====
-- Orig Proof
import Mathlib
import Aesop

set_option maxHeartbeats 0

open Matrix Function Real

theorem putnam_2012_b1
(S : Set (Set.Ici (0 : ℝ) → ℝ))
(rngS : ∀ f ∈ S, ∀ x : Set.Ici (0 : ℝ), f x ∈ Set.Ici (0 : ℝ))
(f1 : Set.Ici (0 : ℝ) → ℝ)
(hf1 : f1 = fun (x : Set.Ici (0 : ℝ)) => exp x - 1)
(f2 : Set.Ici (0 : ℝ) → ℝ)
(hf2 : f2 = fun (x : Set.Ici (0 : ℝ)) => Real.log (x + 1))
(hf1mem : f1 ∈ S)
(hf2mem : f2 ∈ S)
(hsum : ∀ f ∈ S, ∀ g ∈ S, (fun x => (f x) + (g x)) ∈ S)
(hcomp : ∀ f ∈ S, ∀ g ∈ S, g gneg : Set.Ici (0 : ℝ) → Set.Ici (0 : ℝ), ((f x :
  → Set.Ici (0 : ℝ), g x = gneg x) → (fun x => f (gneg x)) ∈ S))
(hdiff : ∀ f ∈ S, ∀ g ∈ S, (∀ x : Set.Ici (0 : ℝ), f x ≥ g x) → (fun x => (f x)
  → - (g x)) ∈ S)
: (∀ f ∈ S, ∀ g ∈ S, (fun x => (f x) * (g x)) ∈ S) := by
  have h_log_f : ∀ (f : Set.Ici (0 : ℝ) → ℝ), f ∈ S → (fun (x : Set.Ici (0 : ℝ)
    → ℝ) => Real.log (f x + 1)) ∈ S := by
    intro f hf
    have h2 : ∀ (x : Set.Ici (0 : ℝ)), (f x : ℝ) ≥ 0 := by
      intro x
      have h2 : f x ∈ Set.Ici (0 : ℝ) := rngS f hf x
      exact by
        simp only [Set.mem_Ici] at h2
        exact h2
    let gneg : Set.Ici (0 : ℝ) → Set.Ici (0 : ℝ) := fun x => (f x, h2 x)
    have h2 : ∀ (x : Set.Ici (0 : ℝ)), (f x : ℝ) = (gneg x : ℝ) := by
      intro x
      simp [gneg]
      <>
      (try simp_all [Set.Ici]) <>
      (try norm_num) <>
      (try ring_nf) <>
      (try field_simp) <>
      (try linarith)
    have h2 : (fun x => f2 (gneg x)) ∈ S := by
      apply hcomp f2 hf2mem f hf gneg
      intro x
      have h2 := h2 x
      simp_all [hf2]
      <>
      (try simp_all [Set.Ici]) <>
      (try norm_num) <>
      (try ring_nf) <>
      (try field_simp) <>
      (try linarith)
    have h2 : (fun x => f2 (gneg x)) = (fun (x : Set.Ici (0 : ℝ)) => Real.log
      → (f x + 1)) := by
      funext x
      simp [hf2, gneg]
      <>
      (try simp_all [Set.Ici]) <>
      (try norm_num) <>
      (try ring_nf) <>
      (try field_simp) <>
      (try linarith)
    rw [h2] at h2
    exact h2
  have h_exp_sum_log : ∀ (f g : Set.Ici (0 : ℝ) → ℝ), f ∈ S → g ∈ S → (fun (x :
    → Set.Ici (0 : ℝ)) => Real.log (f x + 1) + Real.log (g x + 1)) ∈ S := by
    intro f g hf hg
    have h1 : (fun (x : Set.Ici (0 : ℝ)) => Real.log (f x + 1)) ∈ S := h_log_f
    → f hf
    have h2 : (fun (x : Set.Ici (0 : ℝ)) => Real.log (g x + 1)) ∈ S := h_log_f
    → g hg
    have h3 : (fun (x : Set.Ici (0 : ℝ)) => Real.log (f x + 1) + Real.log (g x +
      → 1)) ∈ S := by
      apply hsum (fun x => Real.log (f x + 1)) h1 (fun x => Real.log (g x +
        → 1)) h2
    exact h3
  have h_exp_sum_log : ∀ (f g : Set.Ici (0 : ℝ) → ℝ), f ∈ S → g ∈ S → (fun (x
    → Set.Ici (0 : ℝ)) => (f x + 1) * (g x + 1) - 1) ∈ S := by
    intro f g hf hg
    have h2 : (fun (x : Set.Ici (0 : ℝ)) => Real.log (f x + 1) + Real.log (g x +
      → 1)) ∈ S := h_sum_log f g hf hg
    have h2 : ∀ (x : Set.Ici (0 : ℝ)), Real.log (f x + 1) + Real.log (g x + 1) ≥
      → 0 := by
      intro x
      have h2 : f x ≥ 0 := by
        have h2 : f x ∈ Set.Ici (0 : ℝ) := rngS f hf x
        exact by
          simp only [Set.mem_Ici] at h2
          exact h2
      have h2 : g x ≥ 0 := by

```





```

    apply hcomp f2 hf2mem f hf gneg
    intro x
    have h1 := h x
    simp_all [hf2]
    have h : (fun x => f2 (gneg x)) = (fun x => Real.log (f x + 1)) := by
      funext x
      simp [hf2, gneg]
    rw [h1] at h
    exact h
  -----
  -- Orig Proof
  import Mathlib
  import Aesop

  set_option maxHeartbeats 0

  open Function Set

  theorem putnam_2013_b1
  (c : ℕ → ℝ)
  (hc1 : c 1 = 1)
  (hceven : ∀ n : ℕ, n > 0 → c (2 * n) = c n)
  (hcodd : ∀ n : ℕ, n > 0 → c (2 * n + 1) = (-1) ^ n * c n)
  : (c n : Set.Icc 1 2013, c n * c (n + 1 + 2)) = ((-1) : ℝ) := by
    have hc3 : c 3 = -1 := by
      have h2 : c 3 = (-1 : ℝ) ^ 1 * c 1 := by
        have h3 : c (2 * 1 + 1) = (-1 : ℝ) ^ 1 * c 1 := hcodd 1 (by norm_num)
      norm_num at h3
    <|> simp using h3
    rw [h2]
    norm_num [hc1]
    <|> simp_all

  have hmain : ∀ (k : ℕ), (c n in Finset.Icc 1 (2 * k + 1), c n * c (n + 2)) =
    → (-1 : ℝ) := by
    intro k
    have h : ∀ (k : ℕ), (c n in Finset.Icc 1 (2 * k + 1), c n * c (n + 2)) =
      → (-1 : ℝ) := by
      intro k
      induction k with
      | zero =>
        norm_num [Finset.sum_Icc_succ_top]
        <|>
        (try simp_all [hc1, hc3]) <|>
        (try norm_num) <|>
        (try ring_nf at *) <|>
        (try linarith)
      | succ k ih =>
        have h1 : (c n in Finset.Icc 1 (2 * (k + 1) + 1), c n * c (n + 2)) = (c
          → n in Finset.Icc 1 (2 * k + 1), c n * c (n + 2)) + c (2 * k + 2) * c
          → (2 * k + 4) + c (2 * k + 3) * c (2 * k + 5) := by
            have h1 : 2 * (k + 1) + 1 = 2 * k + 3 := by ring
            rw [h1]
            have h1 : (c n in Finset.Icc 1 (2 * k + 3), c n * c (n + 2)) = (c n
              → in Finset.Icc 1 (2 * k + 1), c n * c (n + 2)) + c (2 * k + 2) * c (2 *
              → k + 4) + c (2 * k + 3) * c (2 * k + 5) := by
                have h1 : (c n in Finset.Icc 1 (2 * k + 3), c n * c (n + 2)) = (c n
                  → in Finset.Icc 1 (2 * k + 1), c n * c (n + 2)) + (c n in Finset.Icc (2
                  → * k + 2) (2 * k + 3), c n * c (n + 2)) := by
                    have h1 : Finset.Icc 1 (2 * k + 3) = Finset.Icc 1 (2 * k + 1) ∪
                    → Finset.Icc (2 * k + 2) (2 * k + 3) := by
                        ext x
                        simp [Finset.mem_Icc]
                        <|>
                        (try omega) <|>
                        (try
                          {
                            by_cases h1 : x ≤ 2 * k + 1 <|>
                            by_cases h1 : x ≥ 2 * k + 2 <|>
                            simp_all [Nat.lt_succ_iff] <|>
                            omega
                          }
                        )
                    rw [h1]
                    rw [Finset.sum_union] <|>
                    (try simp [Finset.disjoint_left, Finset.mem_Icc]) <|>
                    (try omega)
                    rw [h1]
                    have h1 : (c n in Finset.Icc (2 * k + 2) (2 * k + 3), c n * c (n +
                      → 2)) = c (2 * k + 2) * c (2 * k + 4) + c (2 * k + 3) * c (2 * k + 5)
                    → := by
                        have h1 : Finset.Icc (2 * k + 2) (2 * k + 3) = {2 * k + 2, 2 * k +
                        → 3} := by
                            ext x
                            simp [Finset.mem_Icc]
                            <|>
                            (try omega) <|>
                            (try
                              {
                                constructor <|> intro h <|>
                                (try omega) <|>
                                (try
                                  {
                                    cases' h with h1 h2 <|>
                                    omega
                                  }
                                )
                              }
                            )
                        rw [h1]
                        simp [Finset.sum_pair (show (2 * k + 2 : ℕ) ≠ 2 * k + 3 by
                          → omega)]
                        <|>
                        (try ring_nf at *) <|>
                        (try simp_all [hceven, hcodd]) <|>
                        (try norm_num) <|>
                        (try ring_nf) <|>
                        (try omega)
                    rw [h1]
                    <|>
                    ring_nf
                    <|>
                    simp_all [add_assoc]
                    <|>
                    ring_nf

```

open Function Set

```

theorem putnam_2013_b1
(c : ℕ → ℤ)
(hc1 : c 1 = 1)
(hceven : ∀ n : ℕ, n > 0 → c (2 * n) = c n)
(hcodd : ∀ n : ℕ, n > 0 → c (2 * n + 1) = (-1) ^ n * c n)
: (c n : Set.Icc 1 2013, c n * c (n + 1 + 2)) = ((-1) : ℤ) := by
  have h_c3 : c 3 = -1 := by
    rw [hcodd 1 (by norm_num)] <|> simp_all
  have h_main : ∀ (k : ℕ), (c n in Finset.Icc 1 (2 * k + 1), c n * c (n + 2)) =
    → (-1 : ℤ) := by
    intro k
    induction k with
    | zero =>
      norm_num
      <|> simp_all
    | succ k ih =>
      have h1 : (c n in Finset.Icc 1 (2 * (k + 1) + 1), c n * c (n + 2)) = (c n
        → in Finset.Icc 1 (2 * k + 1), c n * c (n + 2)) + c (2 * k + 2) * c (2 *
          → k + 4) * c (2 * k + 3) * c (2 * k + 5) := by
          have h2 : 2 * (k + 1) + 1 = 2 * k + 3 := by ring
          rw [h1]
          simp_all [Finset.sum_Icc_succ_top, Finset.sum_Icc_succ_top,
            → Nat.mul_succ]
          <|> ring
          rw [h1]
          have h3 : c (2 * k + 2) * c (2 * k + 4) + c (2 * k + 3) * c (2 * k + 5) =
            → 0 := by
            have h3_1 : c (2 * k + 2) = c (k + 1) := hceven (k + 1) (by omega)
            have h3_2 : c (2 * k + 4) = c (k + 2) := hceven (k + 2) (by omega)
            have h3_3 : c (2 * k + 3) = (-1 : ℤ) ^ (k + 1) * c (k + 1) := hcodd (k +
              → 1) (by omega)
            have h3_4 : c (2 * k + 5) = (-1 : ℤ) ^ (k + 2) * c (k + 2) := hcodd (k +
              → 2) (by omega)
            calc
              c (2 * k + 2) * c (2 * k + 4) + c (2 * k + 3) * c (2 * k + 5) = c (k
                → + 1) * c (k + 2) + ((-1 : ℤ) ^ (k + 1) * c (k + 1)) * ((-1 : ℤ) ^ (k +
                  → 2) * c (k + 2)) := by rw [h3_1, h3_2, h3_3, h3_4]
              _ = c (k + 1) * c (k + 2) + ((-1 : ℤ) ^ (k + 1) * c (k + 1)) * ((-1 : ℤ) ^ (k +
                → 2)) * c (k + 1) * c (k + 2) := by ring
              _ = c (k + 1) * c (k + 2) + ((-1 : ℤ) ^ ((k + 1) + (k + 2))) * c (k +
                → 1) * c (k + 2) := by
                rw [← pow_add]
                _ = c (k + 1) * c (k + 2) + (-1 : ℤ) * c (k + 1) * c (k + 2) := by
                  have h3_5 : (k + 1) + (k + 2) = 2 * k + 3 := by ring
                  rw [h3_5]
                  have h3_6 : ((-1 : ℤ) : ℤ) ^ (2 * k + 3) = -1 := by
                    have h3_6_1 : (2 * k + 3 : ℕ) % 2 = 1 := by omega
                    have h3_6_2 : ((-1 : ℤ) : ℤ) ^ (2 * k + 3) = -1 := by
                      rw [← Nat.mod_add_div (2 * k + 3) 2]
                      simp [h3_6_1, pow_add, pow_mul, pow_one, mul_neg, mul_one]
                    exact h3_6_2
                  rw [h3_6]
                  _ = 0 := by ring
                rw [ih]
                linarith
            have h3_7 : (c n : Set.Icc 1 2013, c n * c (n + 1 + 2)) = ((-1) : ℤ) := by
              have h3_7_1 : (c n in Finset.Icc 1 2013, c n * c (n + 2)) = (-1 : ℤ) := by
                have h3_7_2 : 2013 = 2 * 1006 + 1 := by norm_num
                rw [h3_7_2]
                have h3_7_3 : (c n in Finset.Icc 1 (2 * 1006 + 1), c n * c (n + 2)) = (-1 : ℤ)
                  → := h_main 1006
                exact h3_7_3
            have h3_8 : (c n : Set.Icc 1 2013, c n * c (n + 1 + 2)) = (c n in Finset.Icc 1
              → 2013, c n * c (n + 2)) := by
              apply Eq.symm
              apply Eq.symm
            have h3_9 : (c n in Finset.Icc 1 2013, c n * c (n + 2)) = c n : Set.Icc 1
              → 2013, c n * c (n + 1 + 2) := by
              apply Finset.sum_bij (fun (n : ℕ) _ => m, by
                simp_all [Finset.mem_Icc, Set.mem_Icc]
              )
              <|> simp_all [Finset.mem_Icc, Set.mem_Icc]
            rw [h3_9]
            rw [h3_9]
            rw [h3_9]
            exact h3_7_1
          -----
          -- Orig Proof
          import Mathlib
          import Aesop

          set_option maxHeartbeats 0

```

```

theorem putnam_2015_a2
(a : ℕ → ℤ)
(abase : a 0 = 1 ∧ a 1 = 2)
(arec : ∀ n ≥ 2, a n = 4 * a (n - 1) - a (n - 2))
: Odd ((181) : ℕ) ∧ (((181) : ℕ).Prime ∧ (((181) : ℕ) : ℤ) | a 2015) := by
  have h1 : Odd ((181) : ℕ) := by
    decide
  have h2 : (((181) : ℕ).Prime := by
    norm_num [Nat.Prime]
    <|>
    decide
  have h3 : ∀ n : ℕ, (a (n + 10) : ℤ) = - (a n : ℤ) [ZMOD 181] := by
    intro n
    have h3_1 : ∀ n : ℕ, (a (n + 10) : ℤ) = - (a n : ℤ) [ZMOD 181] := by
      intro n
      induction n using Nat.strong_induction_on with
      | h n ih =>
        match n with
        | 0 =>
          norm_num [Int.ModEq, abase, arec]
          <|>
          (try decide) <|>
          (try {
            norm_num [abase, arec] at *

```

```

<|>
ring_nf at *
<|>
norm_num at *
<|>
omega
}) <|>
(try {
  simp_all [abase, arec]
  <|>
  norm_num [Int.emod_eq_of_lt]
  <|>
  ring_nf at *
  <|>
  norm_num at *
  <|>
  omega
}) <|>
| 1 =>
norm_num [Int.ModEq, abase, arec]
<|>
(try decide) <|>
(try {
  norm_num [abase, arec] at *
  <|>
  ring_nf at *
  <|>
  norm_num at *
  <|>
  omega
}) <|>
(try {
  simp_all [abase, arec]
  <|>
  norm_num [Int.emod_eq_of_lt]
  <|>
  ring_nf at *
  <|>
  norm_num at *
  <|>
  omega
}) <|>
| 2 =>
norm_num [Int.ModEq, abase, arec]
<|>
(try decide) <|>
(try {
  norm_num [abase, arec] at *
  <|>
  ring_nf at *
  <|>
  norm_num at *
  <|>
  omega
}) <|>
(try {
  simp_all [abase, arec]
  <|>
  norm_num [Int.emod_eq_of_lt]
  <|>
  ring_nf at *
  <|>
  norm_num at *
  <|>
  omega
}) <|>
| 3 =>
norm_num [Int.ModEq, abase, arec]
<|>
(try decide) <|>
(try {
  norm_num [abase, arec] at *
  <|>
  ring_nf at *
  <|>
  norm_num at *
  <|>
  omega
}) <|>
(try {
  simp_all [abase, arec]
  <|>
  norm_num [Int.emod_eq_of_lt]
  <|>
  ring_nf at *
  <|>
  norm_num at *
  <|>
  omega
}) <|>
| 4 =>
norm_num [Int.ModEq, abase, arec]
<|>
(try decide) <|>
(try {
  norm_num [abase, arec] at *
  <|>
  ring_nf at *
  <|>
  norm_num at *
  <|>
  omega
}) <|>
(try {
  simp_all [abase, arec]
  <|>
  norm_num [Int.emod_eq_of_lt]
  <|>
  ring_nf at *
  <|>
  norm_num at *
  <|>
  omega
}) <|>
| 5 =>
norm_num [Int.ModEq, abase, arec]
<|>
(try decide) <|>
(try {
  norm_num [abase, arec] at *

```

```

<|>
ring_nf at *
<|>
norm_num at *
<|>
omega
}) <|>
{
  simp_all [abase, arec]
  <|>
  norm_num [Int.emod_eq_of_lt]
  <|>
  ring_nf at *
  <|>
  norm_num at *
  <|>
  omega
}
| 6 =>
norm_num [Int.ModEq, abase, arec]
<|>
{
  (try decide) <|>
  (try {
    norm_num [abase, arec] at *
    <|>
    ring_nf at *
    <|>
    norm_num at *
    <|>
    omega
  }) <|>
  (try {
    simp_all [abase, arec]
    <|>
    norm_num [Int.emod_eq_of_lt]
    <|>
    ring_nf at *
    <|>
    norm_num at *
    <|>
    omega
  })
}
| 7 =>
norm_num [Int.ModEq, abase, arec]
<|>
{
  (try decide) <|>
  (try {
    norm_num [abase, arec] at *
    <|>
    ring_nf at *
    <|>
    norm_num at *
    <|>
    omega
  }) <|>
  (try {
    simp_all [abase, arec]
    <|>
    norm_num [Int.emod_eq_of_lt]
    <|>
    ring_nf at *
    <|>
    norm_num at *
    <|>
    omega
  })
}
| 8 =>
norm_num [Int.ModEq, abase, arec]
<|>
{
  (try decide) <|>
  (try {
    norm_num [abase, arec] at *
    <|>
    ring_nf at *
    <|>
    norm_num at *
    <|>
    omega
  }) <|>
  (try {
    simp_all [abase, arec]
    <|>
    norm_num [Int.emod_eq_of_lt]
    <|>
    ring_nf at *
    <|>
    norm_num at *
    <|>
    omega
  })
}
| 9 =>
norm_num [Int.ModEq, abase, arec]
<|>
{
  (try decide) <|>
  (try {
    norm_num [abase, arec] at *
    <|>
    ring_nf at *
    <|>
    norm_num at *
    <|>
    omega
  }) <|>
  (try {
    simp_all [abase, arec]
    <|>
    norm_num [Int.emod_eq_of_lt]
    <|>
    ring_nf at *
    <|>
    norm_num at *
    <|>
    omega
  })
}
| n + 10 =>
have hn := ih n (by omega)
have hn := ih (n + 1) (by omega)
have hn := ih (n + 2) (by omega)
have hn := ih (n + 3) (by omega)
have hn := ih (n + 4) (by omega)

have h5 := ih (n + 5) (by omega)
have h6 := ih (n + 6) (by omega)
have h7 := ih (n + 7) (by omega)
have h8 := ih (n + 8) (by omega)
have h9 := ih (n + 9) (by omega)
norm_num [Int.ModEq, abase, arec] at *
<|>
{
  (try omega) <|>
  (try {
    simp_all [Int.ModEq, Int.emod_eq_emod_iff_emod_sub_eq_zero]
    <|>
    ring_nf at *
    <|>
    norm_num at *
    <|>
    omega
  }) <|>
  (try {
    simp_all [Int.ModEq, Int.emod_eq_emod_iff_emod_sub_eq_zero]
    <|>
    ring_nf at *
    <|>
    norm_num at *
    <|>
    omega
  })
}
exact hn n

have h1 : (a 5 : z) = 0 [ZMOD 181] := by
norm_num [Int.ModEq, abase, arec]
<|>
{
  (try decide) <|>
  (try {
    norm_num [abase, arec] at *
    <|>
    ring_nf at *
    <|>
    norm_num at *
    <|>
    omega
  }) <|>
  (try {
    simp_all [abase, arec]
    <|>
    norm_num [Int.emod_eq_of_lt]
    <|>
    ring_nf at *
    <|>
    norm_num at *
    <|>
    omega
  })
}

have h1 : (a 2015 : z) = 0 [ZMOD 181] := by
have h1 : (a 2015 : z) = 0 [ZMOD 181] := by
  intro k
  induction k with
  | zero =>
    norm_num [Int.ModEq] at h1
    <|>
    simp [abase, arec] using h1
  | succ k ih =>
    have h3 := h1 (10 * k + 5)
    have h4 := h1 (10 * k + 6)
    have h5 := h1 (10 * k + 7)
    have h6 := h1 (10 * k + 8)
    have h7 := h1 (10 * k + 9)
    have h8 := h1 (10 * k + 10)
    have h9 := h1 (10 * k + 11)
    have h10 := h1 (10 * k + 12)
    have h11 := h1 (10 * k + 13)
    have h12 := h1 (10 * k + 14)
    simp [Int.ModEq] at h3, h4, h5, h6, h7, h8, h9, h10, h11, h12 ih
    <|>
    (try omega) <|>
    (try ring_nf at * <|> norm_num
    → [Int.emod_eq_emod_iff_emod_sub_eq_zero] at * <|>
    omega) <|>
    (try {
      simp_all [Int.ModEq, Int.emod_eq_emod_iff_emod_sub_eq_zero]
      <|>
      ring_nf at *
      <|>
      norm_num at *
      <|>
      omega
    })
    <|>
    {
      (try {
        simp_all [Int.ModEq, Int.emod_eq_emod_iff_emod_sub_eq_zero]
        <|>
        ring_nf at *
        <|>
        norm_num at *
        <|>
        omega
      })
    }
  }
}
have h13 : (a 2015 : z) = 0 [ZMOD 181] := by
have h4 : (a (10 * 201 + 5) : z) = 0 [ZMOD 181] := h1, 201
norm_num at h4
<|>
simp [add_assoc] using h4
exact h13
exact h1

have h1 : (((181) : N) : z) | a 2015 := by
rw [Int.dvd_iff_emod_eq_zero]
have h1 : (a 2015 : z) % 181 = 0 := by
rw [Int.emod_eq_zero_of_dvd]

have h1 : (a 2015 : z) = 0 [ZMOD 181] := h1
rw [Int.ModEq] at h1
omega
exact h1
exact {h1, h1, h1}

```

```

(a b : z)
(h b : < a < a 0 < b) :
((1 : q) / a + (1 : q) / b = (3 : q) / 2018) → (a, b) ∈ ((({673, 1358114}, {
  → 674, 340033, 1009, 2018, 2018, 1009, 340033, 674}, {1358114, 673})
  → Set (Z × Z))) := by
  rcases h with ha, hb
  constructor
  · field_simp [ha, hb]
  · norm_cast
  · rintro h
  · norm_num
  · have : a ≤ 1345 ∨ b ≤ 1345 := by
      by_contra!
      linarith
  · rcases this with (h, | h)
    · interval_cases a <|> omega
    · interval_cases b <|> omega
  · rintro (rfl, rfl) | (rfl, rfl) | (rfl, rfl) | (rfl, rfl) | (rfl, rfl) | (rfl,
    → rfl) <|> norm_num

```



```

    exact_mod_cast h
  constructor
  exact_mod_cast h
  constructor
  exact_mod_cast h

  have h₁ : (m + 1 : z)³ + (m : z)³ + (m : z)³ - 3 * (m + 1 : z) * (m : z) * (m : z) = 3 * m + 1 := by
    ring_nf
    <> nlinarith
  rw [hm]
  linarith

  have h₂ : (n - 2) % 3 = 0 := by
    omega
  have h₃ : (m : z), n = 3 * m + 2 := by
    use (n - 2) / 3
    have h₄ : (n - 2) % 3 = 0 := h₂
    have h₅ : n - 2 = 3 * ((n - 2) / 3) := by
      omega
    linarith
  rcases h₃ with m, hm
  have h₆ : m ≥ 0 := by
    by_contra h
    have h₇ : m < 0 := by linarith
    have h₈ : n < 2 := by
      nlinarith
    have h₉ : n ≥ 0 := h
    have h₁₀ : m ≤ -1 := by
      omega
    have h₁₁ : n < 0 := by
      nlinarith
    linarith
  use (m + 1 : z), (m + 1 : z), (m : z)
  have h₁₂ : (m + 1 : z) ≥ 0 := by linarith
  have h₁₃ : (m + 1 : z) ≥ 0 := by linarith
  have h₁₄ : (m : z) ≥ 0 := by linarith
  constructor
  exact_mod_cast h
  constructor
  exact_mod_cast h
  constructor
  exact_mod_cast h

  have h₁₅ : (m + 1 : z)³ + (m + 1 : z)³ + (m : z)³ - 3 * (m + 1 : z) * (m + 1 : z) * (m : z) = 3 * m + 2 := by
    ring_nf
    <> nlinarith
  rw [hm]
  linarith

  have h_main : {n : z | ∃ A B C : z, A ≥ 0 ∧ B ≥ 0 ∧ C ≥ 0 ∧ A³ + B³ + C³ - 3 * A * B * C = n} = ({(n : z | n ≥ 0 ∧ -Int.ModEq 9 n 3 ∧ -Int.ModEq 9 n 6)} : Set z) := by
    apply Set.Subset.antisymm
  exact h_subset
  exact h_subset

exact h_main

-- Simplified Proof
import Mathlib
import Aesop

set_option maxHeartbeats 0

open Topology Filter

theorem putnam_2019_a1
: {n : z | ∃ A B C : z, A ≥ 0 ∧ B ≥ 0 ∧ C ≥ 0 ∧ A³ + B³ + C³ - 3 * A * B * C = n} =
  { (n : z | n ≥ 0 ∧ -Int.ModEq 9 n 3 ∧ -Int.ModEq 9 n 6) } : Set z :=
  by
    ext n
  constructor
  rintro A, B, C, hA, hB, hC, hm
  have h₁ : n ≥ 0 := by nlinarith [sq_nonneg (A - B), sq_nonneg (B - C),
    sq_nonneg (C - A), mul_nonneg hA hB, mul_nonneg hB hC, mul_nonneg hC hA, sq_nonneg (A + B + C), sq_nonneg (A + B - C), sq_nonneg (A + C - B), sq_nonneg (B + C - A)]
  have h₂ : -Int.ModEq 9 n 3 := by
    intro h
    have h₃ : n % 9 = 3 := by rw [Int.ModEq] at h; omega
    have h₄ : (A³ + B³ + C³ - 3 * A * B * C) % 9 ≠ 3 := by
      have h₅ : A % 9 = 0 ∨ A % 9 = 1 ∨ A % 9 = 2 ∨ A % 9 = 3 ∨ A % 9 = 4 ∨ A % 9 = 5 ∨ A % 9 = 6 ∨ A % 9 = 7 ∨ A % 9 = 8 := by omega
      have h₆ : B % 9 = 0 ∨ B % 9 = 1 ∨ B % 9 = 2 ∨ B % 9 = 3 ∨ B % 9 = 4 ∨ B % 9 = 5 ∨ B % 9 = 6 ∨ B % 9 = 7 ∨ B % 9 = 8 := by omega
      have h₇ : C % 9 = 0 ∨ C % 9 = 1 ∨ C % 9 = 2 ∨ C % 9 = 3 ∨ C % 9 = 4 ∨ C % 9 = 5 ∨ C % 9 = 6 ∨ C % 9 = 7 ∨ C % 9 = 8 := by omega
      rcases h₅ with (h₈ | h₉ | h₁₀ | h₁₁ | h₁₂ | h₁₃ | h₁₄ | h₁₅ | h₁₆ | h₁₇) <> rcases h₆ with (h₁₈ | h₁₉ | h₂₀ | h₂₁ | h₂₂ | h₂₃ | h₂₄ | h₂₅ | h₂₆ | h₂₇) <> rcases h₇ with (h₂₈ | h₂₉ | h₃₀ | h₃₁ | h₃₂ | h₃₃ | h₃₄ | h₃₅ | h₃₆ | h₃₇) <> (try { simp [h₈, h₉, h₁₀, h₁₁, h₁₂, h₁₃, h₁₄, h₁₅, h₁₆, h₁₇, h₁₈, h₁₉, h₂₀, h₂₁, h₂₂, h₂₃, h₂₄, h₂₅, h₂₆, h₂₇, h₂₈, h₂₉, h₃₀, h₃₁, h₃₂, h₃₃, h₃₄, h₃₅, h₃₆, h₃₇] })
    omega
  have h₃ : -Int.ModEq 9 n 6 := by
    intro h
    have h₄ : n % 9 = 6 := by rw [Int.ModEq] at h; omega
    have h₅ : (A³ + B³ + C³ - 3 * A * B * C) % 9 ≠ 6 := by
      have h₆ : A % 9 = 0 ∨ A % 9 = 1 ∨ A % 9 = 2 ∨ A % 9 = 3 ∨ A % 9 = 4 ∨ A % 9 = 5 ∨ A % 9 = 6 ∨ A % 9 = 7 ∨ A % 9 = 8 := by omega
      have h₇ : B % 9 = 0 ∨ B % 9 = 1 ∨ B % 9 = 2 ∨ B % 9 = 3 ∨ B % 9 = 4 ∨ B % 9 = 5 ∨ B % 9 = 6 ∨ B % 9 = 7 ∨ B % 9 = 8 := by omega
      have h₈ : C % 9 = 0 ∨ C % 9 = 1 ∨ C % 9 = 2 ∨ C % 9 = 3 ∨ C % 9 = 4 ∨ C % 9 = 5 ∨ C % 9 = 6 ∨ C % 9 = 7 ∨ C % 9 = 8 := by omega
      rcases h₆ with (h₉ | h₁₀ | h₁₁ | h₁₂ | h₁₃ | h₁₄ | h₁₅ | h₁₆ | h₁₇ | h₁₈) <> rcases h₇ with (h₁₉ | h₂₀ | h₂₁ | h₂₂ | h₂₃ | h₂₄ | h₂₅ | h₂₆ | h₂₇ | h₂₈) <> (try { simp [h₉, h₁₀, h₁₁, h₁₂, h₁₃, h₁₄, h₁₅, h₁₆, h₁₇, h₁₈, h₁₉, h₂₀, h₂₁, h₂₂, h₂₃, h₂₄, h₂₅, h₂₆, h₂₇, h₂₈] })
    omega
  exact {h₁, h₂, h₃}
  rintro h₁, h₂, h₃
  have h₄ : n % 3 = 0 ∨ n % 3 = 1 ∨ n % 3 = 2 := by omega
  rcases h₄ with (h₅ | h₆ | h₇)
  have h₅ : n % 9 ≠ 3 := by intro h₈; rw [Int.ModEq] at h₈; omega
  have h₆ : n % 9 ≠ 6 := by intro h₉; rw [Int.ModEq] at h₉; omega

```

# IMO Proofs

```
-- P1
import Mathlib
import Aesop
set_option pp.numericTypes true
set_option pp.funBinderTypes true
set_option maxHeartbeats 0
set_option maxRecDepth 1000
set_option tactic.hygienic false
open BigOperators Real Nat Topology Rat Classical Polynomial

theorem k_le_3_for_n_le_4_round1_main (n k : ℕ) (verts : Finset ℕ) (lines :
  → Finset (ℝ × ℝ)) (points : Finset (ℕ × ℕ)) (hn : 3 ≤ n) (hcard :
  → lines.card + verts.card = n) (hallpoints : ∀ p, p ∈ points → p.1 ≥ 1 ∧
  → p.2 ≥ 1 ∧ p.1 + p.2 ≤ n + 1) (hmain : ∀ p ∈ points, (∃ l ∈ lines, l.1
  → * p.1 + l.2 = p.2) ∨ (∃ x ∈ verts, p.1 = x)) (hk : (lines.filter (fun
  → l ↦ l.1 ≠ 0 ∧ l.1 ≠ -1)).card = k) (hn2 : n = 4):
k ≤ 3 := by
by_contra h16
have h161 : k ≥ 4 := by linarith
have h162 : (lines.filter (fun l ↦ l.1 ≠ 0 ∧ l.1 ≠ -1)).card ≥ 4 := by
  → linarith
have h163 : (lines.filter (fun l ↦ l.1 ≠ 0 ∧ l.1 ≠ -1)).card ≤ lines.card :=
  → by apply Finset.card_filter_le
have h164 : lines.card + verts.card = 4 := by linarith
have h165 : lines.card ≥ 4 := by omega
have h166 : lines.card = 4 := by omega
have h167 : verts.card = 0 := by omega
have h168 : verts = ∅ := by
  exact Finset.card_eq_zero.mp h167
have h170 : ∀ (p : ℕ × ℕ), p ∈ points → ∃ l ∈ lines, l.1 * p.1 + l.2 = p.2 :=
  → by
  intro p hp
  have h170i := hmain p hp
  rcases h170i with (h170i | h1702)
  · exact h170i
  · rcases h1702 with (x, hx, _)
    have h1703 : x ∈ verts := hx
    rw [h168] at h1703
    contradiction
have h177 : ∀ l ∈ lines, l.1 ≠ 0 ∧ l.1 ≠ -1 := by
  intro l hl
  by_contra h177i
  have h1772 : ¬(l.1 ≠ 0 ∧ l.1 ≠ -1) := by tauto
  have h1773 : l ∉ (lines.filter (fun l ↦ l.1 ≠ 0 ∧ l.1 ≠ -1)) := by
    simp [Finset.mem_filter]
  <> tauto
  have h1774 : (lines.filter (fun l ↦ l.1 ≠ 0 ∧ l.1 ≠ -1)).card < lines.card
  → := by
    apply Finset.card_lt_card
    exact Finset.subset_iff_subset_ne.mpr (Finset.filter_subset _ _, fun h =>
    → by simp_all)
  linarith
have h171 : (1, 1) ∈ points := by
  rw [hallpoints]
  norm_num [hn2]
obtain ⟨l1, h11_in_lines, h11_eq := h170 (1, 1) h171
obtain ⟨l2, h12_in_lines, h12_eq := h170 (1, 2) (by
  rw [hallpoints]
  norm_num [hn2])
obtain ⟨l3, h13_in_lines, h13_eq := h170 (1, 3) (by
  rw [hallpoints]
  norm_num [hn2])
obtain ⟨l4, h14_in_lines, h14_eq := h170 (1, 4) (by
  rw [hallpoints]
  norm_num [hn2])
have h111 : l1.1 + l1.2 = 1 := by
  norm_num at h11_eq
  <> linarith
have h122 : l2.1 + l2.2 = 2 := by
  norm_num at h12_eq
  <> linarith
have h133 : l3.1 + l3.2 = 3 := by
  norm_num at h13_eq
  <> linarith
have h144 : l4.1 + l4.2 = 4 := by
  norm_num at h14_eq
  <> linarith
have h11_ne_12 : l1 ≠ l2 := by
  intro h
  have h1 : l1.1 + l1.2 = 2 := by
    have h11 : l1 = 12 := h
    have h1221 : l2.1 + l2.2 = 2 := h122
    simp [h11] at *
  <> linarith
linarith
have h11_ne_13 : l1 ≠ l3 := by
  intro h
  have h1 : l1.1 + l1.2 = 3 := by
    have h11 : l1 = 13 := h
    have h1331 : l3.1 + l3.2 = 3 := h133
    simp [h11] at *
  <> linarith
linarith
have h11_ne_14 : l1 ≠ l4 := by
  intro h
  have h1 : l1.1 + l1.2 = 4 := by
    have h11 : l1 = 14 := h
    have h1441 : l4.1 + l4.2 = 4 := h144
    simp [h11] at *
  <> linarith
linarith
have h12_ne_13 : l2 ≠ l3 := by
  intro h
  have h1 : l2.1 + l2.2 = 3 := by
    have h11 : l2 = 13 := h
    have h1331 : l3.1 + l3.2 = 3 := h133
    simp [h11] at *
  <> linarith
linarith
have h12_ne_14 : l2 ≠ l4 := by
  intro h
  have h1 : l2.1 + l2.2 = 4 := by
    have h11 : l2 = 14 := h
    have h1441 : l4.1 + l4.2 = 4 := h144
    simp [h11] at *
  <> linarith
linarith
have h13_ne_14 : l3 ≠ l4 := by
  intro h
  have h1 : l3.1 + l3.2 = 4 := by
    have h11 : l3 = 14 := h
    have h1441 : l4.1 + l4.2 = 4 := h144
    simp [h11] at *
  <> linarith
linarith
have h178 : ({l1, l2, l3, l4} : Finset (ℝ × ℝ)) ⊆ lines := by
  intro x hx
  simp only [Finset.mem_insert, Finset.mem_singleton] at hx
  rcases hx with (rfl | rfl | rfl | rfl)
  · exact h11_in_lines
  · exact h12_in_lines
  · exact h13_in_lines
  · exact h14_in_lines
have h179 : ({l1, l2, l3, l4} : Finset (ℝ × ℝ)).card = 4 := by
  simp [h11_ne_12, h11_ne_13, h11_ne_14, h12_ne_13, h12_ne_14, h13_ne_14]
have h180 : ({l1, l2, l3, l4} : Finset (ℝ × ℝ)) = lines := by
  apply Finset.eq_of_subset_of_card_le h178
  rw [h179, h166]
  <> linarith
have h171_2 : (2, 2) ∈ points := by
  rw [hallpoints]
  norm_num [hn2]
obtain ⟨l5, h15_in_lines, h15_eq := h170 (2, 2) h171_2
have h15_eq' : l5.1 * 2 + l5.2 = 2 := by
  norm_num at h15_eq
  <> linarith
have h171_3 : (2, 3) ∈ points := by
  rw [hallpoints]
  norm_num [hn2]
obtain ⟨l6, h16_in_lines, h16_eq := h170 (2, 3) h171_3
have h16_eq' : l6.1 * 2 + l6.2 = 3 := by
  norm_num at h16_eq
  <> linarith
have h1801 : lines = ({l1, l2, l3, l4} : Finset (ℝ × ℝ)) := by tauto
have h15_in_set : l5 ∈ ({l1, l2, l3, l4} : Finset (ℝ × ℝ)) := by
  rw [h1801] at h15_in_lines
  tauto
have h16_in_set : l6 ∈ ({l1, l2, l3, l4} : Finset (ℝ × ℝ)) := by
  rw [h1801] at h16_in_lines
  tauto
have h15_cases : l5 = l1 ∨ l5 = l2 ∨ l5 = l3 ∨ l5 = l4 := by
  simp only [Finset.mem_insert, Finset.mem_singleton] at h15_in_set
  tauto
have h16_cases : l6 = l1 ∨ l6 = l2 ∨ l6 = l3 ∨ l6 = l4 := by
  simp only [Finset.mem_insert, Finset.mem_singleton] at h16_in_set
  tauto
have h15_ne_2 : l5 ≠ l2 := by
  intro h15_eq_2
  have h177_12 : h177 12 h12_in_lines
  have h151 : l2.1 * 2 + l2.2 = 2 := by
    have h1511 : l5 = l2 := h15_eq_2
    rw [h1511] at h15_eq'
  <> linarith
  have h152 : l2.1 = 0 := by linarith
  have h177_121 : l2.1 ≠ 0 := h177_12.1
  contradiction
have h15_ne_3 : l5 ≠ l3 := by
  intro h15_eq_3
  have h177_13 : h177 13 h13_in_lines
  have h151 : l3.1 * 2 + l3.2 = 2 := by
    have h1511 : l5 = l3 := h15_eq_3
    rw [h1511] at h15_eq'
  <> linarith
  have h152 : l3.1 = -1 := by linarith
  have h177_132 : l3.1 ≠ -1 := h177_13.2
  contradiction
have h15_cases2 : l5 = l1 ∨ l5 = l4 := by tauto
have h16_ne_3 : l6 ≠ l3 := by
  intro h16_eq_3
  have h177_13 : h177 13 h13_in_lines
  have h161 : l3.1 * 2 + l3.2 = 3 := by
    have h1611 : l6 = l3 := h16_eq_3
    rw [h1611] at h16_eq'
  <> linarith
  have h162 : l3.1 = 0 := by linarith
  have h177_131 : l3.1 ≠ 0 := h177_13.1
  contradiction
have h16_ne_4 : l6 ≠ l4 := by
  intro h16_eq_4
  have h177_14 : h177 14 h14_in_lines
  have h161 : l4.1 * 2 + l4.2 = 3 := by
    have h1611 : l6 = l4 := h16_eq_4
    rw [h1611] at h16_eq'
  <> linarith
  have h162 : l4.1 = -1 := by linarith
  have h177_142 : l4.1 ≠ -1 := h177_14.2
  contradiction
have h16_cases2 : l6 = l1 ∨ l6 = l2 := by tauto
rcases h15_cases2 with (h15_eq_l1 | h15_eq_l4)
· have h15_eq_l1 : l5 = l1 := h15_eq_l1
  have h15_eq_l12 : l1.1 * 2 + l1.2 = 2 := by
    rw [h15_eq_l1] at h15_eq'
  <> linarith
  have h111 : l1.1 = 1 := by linarith
  have h112 : l1.2 = 0 := by linarith
  rcases h16_cases2 with (h16_eq_l1 | h16_eq_l2)
  · have h16_eq_l1 : l6 = l1 := h16_eq_l1
    have h16_eq_l12 : l1.1 * 2 + l1.2 = 3 := by
      rw [h16_eq_l1] at h16_eq'
    <> linarith
    norm_num [h111, h112] at h16_eq_l12
  · have h16_eq_l2 : l6 = l2 := h16_eq_l2
    have h16_eq_l22 : l2.1 * 2 + l2.2 = 3 := by
      rw [h16_eq_l2] at h16_eq'
    <> linarith
    have h1221 : l2.1 = 1 := by linarith
    have h1222 : l2.2 = 1 := by linarith
    have h171_4 : (3, 1) ∈ points := by
      rw [hallpoints]
```



```

norm_num [hn2]
obtain ⟨l9, h19_in_lines, h19_eq⟩ := h170 (3, 1) h171_4
have h19_eq' : 19.1 * 3 + 19.2 = 1 := by
norm_num at h19_eq
<> linarith
have h19_in_set : 19 ∈ ({11, 12, 13, 14} : Finset (ℝ × ℝ)) := by
rw [h1801] at h19_in_lines
tauto
have h19_cases : 19 = 11 ∨ 19 = 12 ∨ 19 = 13 ∨ 19 = 14 := by
simp only [Finset.mem_insert, Finset.mem_singleton] at h19_in_set
tauto
rcases h19_cases with (h19_eq_11 | h19_eq_12 | h19_eq_13 | h19_eq_14)
· have h19_eq_111 : 19 = 11 := h19_eq_11
· have h19_eq1 : 11.1 * 3 + 11.2 = 1 := by
rw [h19_eq_111] at h19_eq'
<> linarith
norm_num [h1111, h1112] at h19_eq1
· have h19_eq_121 : 19 = 12 := h19_eq_12
· have h19_eq2 : 12.1 * 3 + 12.2 = 1 := by
rw [h19_eq_121] at h19_eq'
<> linarith
norm_num [h1221, h1222] at h19_eq2
· have h19_eq_131 : 19 = 13 := h19_eq_13
· have h19_eq3 : 13.1 * 3 + 13.2 = 1 := by
rw [h19_eq_131] at h19_eq'
<> linarith
have h31 : 13.1 = -1 := by linarith
have h177_13 := h177 13 h13_in_lines
have h177_132 : 13.1 ≠ -1 := h177_13.2
contradiction
· have h19_eq_141 : 19 = 14 := h19_eq_14
· have h19_eq4 : 14.1 * 3 + 14.2 = 1 := by
rw [h19_eq_141] at h19_eq'
<> linarith
have h41 : 14.1 = -3 / 2 := by linarith
have h42 : 14.2 = 11 / 2 := by linarith
have h171_5 : (2, 1) ∈ points := by
rw [h171_5]
norm_num [hn2]
obtain ⟨l10, h10_in_lines, h20_eq⟩ := h170 (2, 1) h171_5
have h20_eq' : 110.1 * 2 + 110.2 = 1 := by
norm_num at h20_eq
<> linarith
have h20_in_set : 110 ∈ ({11, 12, 13, 14} : Finset (ℝ × ℝ)) := by
rw [h1801] at h10_in_lines
tauto
have h20_cases : 110 = 11 ∨ 110 = 12 ∨ 110 = 13 ∨ 110 = 14 := by
simp only [Finset.mem_insert, Finset.mem_singleton] at h20_in_set
tauto
rcases h20_cases with (h20_eq_11 | h20_eq_12 | h20_eq_13 | h20_eq_14)
· have h20_eq_111 : 110 = 11 := h20_eq_11
· have h20_eq1 : 11.1 * 2 + 11.2 = 1 := by
rw [h20_eq_111] at h20_eq'
<> linarith
norm_num [h1111, h1112] at h20_eq1
· have h20_eq_121 : 110 = 12 := h20_eq_12
· have h20_eq2 : 12.1 * 2 + 12.2 = 1 := by
rw [h20_eq_121] at h20_eq'
<> linarith
norm_num [h21, h22] at h20_eq2
· have h20_eq_131 : 110 = 13 := h20_eq_13
· have h20_eq3 : 13.1 * 2 + 13.2 = 1 := by
rw [h20_eq_131] at h20_eq'
<> linarith
have h31 : 13.1 = -2 := by linarith
have h32 : 13.2 = 5 := by linarith
have h171_6 : (4, 1) ∈ points := by
rw [h171_6]
norm_num [hn2]
obtain ⟨l11, h11_in_lines, h21_eq⟩ := h170 (4, 1) h171_6
have h21_eq' : 111.1 * 4 + 111.2 = 1 := by
norm_num at h21_eq
<> linarith
have h21_in_set : 111 ∈ ({11, 12, 13, 14} : Finset (ℝ × ℝ)) := by
rw [h1801] at h11_in_lines
tauto
have h21_cases : 111 = 11 ∨ 111 = 12 ∨ 111 = 13 ∨ 111 = 14 := by
simp only [Finset.mem_insert, Finset.mem_singleton] at h21_in_set
tauto
rcases h21_cases with (h21_eq_11 | h21_eq_12 | h21_eq_13 | h21_eq_14)
· have h21_eq_111 : 111 = 11 := h21_eq_11
· have h21_eq1 : 11.1 * 4 + 11.2 = 1 := by
rw [h21_eq_111] at h21_eq'
<> linarith
norm_num [h1111, h1112] at h21_eq1
· have h21_eq_121 : 111 = 12 := h21_eq_12
· have h21_eq2 : 12.1 * 4 + 12.2 = 1 := by
rw [h21_eq_121] at h21_eq'
<> linarith
norm_num [h21, h22] at h21_eq2
· have h21_eq_131 : 111 = 13 := h21_eq_13
· have h21_eq3 : 13.1 * 4 + 13.2 = 1 := by
rw [h21_eq_131] at h21_eq'
<> linarith
norm_num [h31, h32] at h21_eq3
· have h21_eq_141 : 111 = 14 := h21_eq_14
· have h21_eq4 : 14.1 * 4 + 14.2 = 1 := by
rw [h21_eq_141] at h21_eq'
<> linarith
norm_num [h41, h42] at h21_eq4
· have h20_eq_141 : 110 = 14 := h20_eq_14
· have h20_eq4 : 14.1 * 2 + 14.2 = 1 := by
rw [h20_eq_141] at h20_eq'
<> linarith
norm_num [h41, h42] at h20_eq4
· have h15_eq_141 : 15 = 14 := h15_eq_14
· have h15_eq_142 : 14.1 * 2 + 14.2 = 2 := by
rw [h15_eq_141] at h15_eq'
<> linarith
have h41 : 14.1 = -2 := by linarith
have h42 : 14.2 = 6 := by linarith
rcases h16_cases2 with (h16_eq_11 | h16_eq_12)
· have h16_eq_111 : 16 = 11 := h16_eq_11
· have h16_eq_112 : 11.1 * 2 + 11.2 = 3 := by
rw [h16_eq_111] at h16_eq'
<> linarith

```

```

<> linarith
have h1111 : 11.1 = 2 := by linarith
have h1112 : 11.2 = -1 := by linarith
have h171_4 : (3, 1) ∈ points := by
rw [h171_4]
norm_num [hn2]
obtain ⟨l9, h19_in_lines, h19_eq⟩ := h170 (3, 1) h171_4
have h19_eq' : 19.1 * 3 + 19.2 = 1 := by
norm_num at h19_eq
<> linarith
have h19_in_set : 19 ∈ ({11, 12, 13, 14} : Finset (ℝ × ℝ)) := by
rw [h1801] at h19_in_lines
tauto
have h19_cases : 19 = 11 ∨ 19 = 12 ∨ 19 = 13 ∨ 19 = 14 := by
simp only [Finset.mem_insert, Finset.mem_singleton] at h19_in_set
tauto
rcases h19_cases with (h19_eq_11 | h19_eq_12 | h19_eq_13 | h19_eq_14)
· have h19_eq_111 : 19 = 11 := h19_eq_11
· have h19_eq1 : 11.1 * 3 + 11.2 = 1 := by
rw [h19_eq_111] at h19_eq'
<> linarith
norm_num [h1111, h1112] at h19_eq1
· have h19_eq_121 : 19 = 12 := h19_eq_12
· have h19_eq2 : 12.1 * 3 + 12.2 = 1 := by
rw [h19_eq_121] at h19_eq'
<> linarith
norm_num [h1221, h1222] at h19_eq2
· have h19_eq_131 : 19 = 13 := h19_eq_13
· have h19_eq3 : 13.1 * 3 + 13.2 = 1 := by
rw [h19_eq_131] at h19_eq'
<> linarith
have h21 : 12.1 = -1 / 2 := by linarith
have h22 : 12.2 = 5 / 2 := by linarith
have h171_5 : (2, 1) ∈ points := by
rw [h171_5]
norm_num [hn2]
obtain ⟨l10, h10_in_lines, h20_eq⟩ := h170 (2, 1) h171_5
have h20_eq' : 110.1 * 2 + 110.2 = 1 := by
norm_num at h20_eq
<> linarith
have h20_in_set : 110 ∈ ({11, 12, 13, 14} : Finset (ℝ × ℝ)) := by
rw [h1801] at h10_in_lines
tauto
have h20_cases : 110 = 11 ∨ 110 = 12 ∨ 110 = 13 ∨ 110 = 14 := by
simp only [Finset.mem_insert, Finset.mem_singleton] at h20_in_set
tauto
rcases h20_cases with (h20_eq_11 | h20_eq_12 | h20_eq_13 | h20_eq_14)
· have h20_eq_111 : 110 = 11 := h20_eq_11
· have h20_eq1 : 11.1 * 2 + 11.2 = 1 := by
rw [h20_eq_111] at h20_eq'
<> linarith
norm_num [h1111, h1112] at h20_eq1
· have h20_eq_121 : 110 = 12 := h20_eq_12
· have h20_eq2 : 12.1 * 2 + 12.2 = 1 := by
rw [h20_eq_121] at h20_eq'
<> linarith
norm_num [h21, h22] at h20_eq2
· have h20_eq_131 : 110 = 13 := h20_eq_13
· have h20_eq3 : 13.1 * 2 + 13.2 = 1 := by
rw [h20_eq_131] at h20_eq'
<> linarith
have h31 : 13.1 = -2 := by linarith
have h32 : 13.2 = 5 := by linarith
have h171_6 : (4, 1) ∈ points := by
rw [h171_6]
norm_num [hn2]
obtain ⟨l11, h11_in_lines, h21_eq⟩ := h170 (4, 1) h171_6
have h21_eq' : 111.1 * 4 + 111.2 = 1 := by
norm_num at h21_eq
<> linarith
have h21_in_set : 111 ∈ ({11, 12, 13, 14} : Finset (ℝ × ℝ)) := by
rw [h1801] at h11_in_lines
tauto
have h21_cases : 111 = 11 ∨ 111 = 12 ∨ 111 = 13 ∨ 111 = 14 := by
simp only [Finset.mem_insert, Finset.mem_singleton] at h21_in_set
tauto
rcases h21_cases with (h21_eq_11 | h21_eq_12 | h21_eq_13 | h21_eq_14)
· have h21_eq_111 : 111 = 11 := h21_eq_11
· have h21_eq1 : 11.1 * 4 + 11.2 = 1 := by
rw [h21_eq_111] at h21_eq'
<> linarith
norm_num [h1111, h1112] at h21_eq1
· have h21_eq_121 : 111 = 12 := h21_eq_12
· have h21_eq2 : 12.1 * 4 + 12.2 = 1 := by
rw [h21_eq_121] at h21_eq'
<> linarith
norm_num [h21, h22] at h21_eq2
· have h21_eq_131 : 111 = 13 := h21_eq_13
· have h21_eq3 : 13.1 * 4 + 13.2 = 1 := by
rw [h21_eq_131] at h21_eq'
<> linarith
norm_num [h31, h32] at h21_eq3
· have h21_eq_141 : 111 = 14 := h21_eq_14
· have h21_eq4 : 14.1 * 4 + 14.2 = 1 := by
rw [h21_eq_141] at h21_eq'
<> linarith
norm_num [h41, h42] at h21_eq4
· have h20_eq_141 : 110 = 14 := h20_eq_14
· have h20_eq4 : 14.1 * 2 + 14.2 = 1 := by
rw [h20_eq_141] at h20_eq'
<> linarith
norm_num [h41, h42] at h20_eq4
· have h19_eq_131 : 19 = 13 := h19_eq_13
· have h19_eq3 : 13.1 * 3 + 13.2 = 1 := by
rw [h19_eq_131] at h19_eq'
<> linarith
have h31 : 13.1 = -1 := by linarith
have h177_13 := h177 13 h13_in_lines
have h177_132 : 13.1 ≠ -1 := h177_13.2
contradiction
· have h19_eq_141 : 19 = 14 := h19_eq_14
· have h19_eq4 : 14.1 * 3 + 14.2 = 1 := by
rw [h19_eq_141] at h19_eq'
<> linarith
norm_num [h41, h42] at h19_eq4
· have h16_eq_121 : 16 = 12 := h16_eq_12
· have h16_eq_122 : 12.1 * 2 + 12.2 = 3 := by
rw [h16_eq_121] at h16_eq'
<> linarith
have h1221 : 12.1 = 1 := by linarith
have h1222 : 12.2 = 1 := by linarith
have h171_4 : (3, 1) ∈ points := by

```

```

    rw [hallpoints]
    norm_num [hn2]
  obtain ⟨l9, h19_in_lines, h19_eq'⟩ := h170 (3, 1) h171_4
  have h19_eq' : 19.1 * 3 + 19.2 = 1 := by
    norm_num at h19_eq' <|> linarith
  have h19_in_set : 19 ∈ ({11, 12, 13, 14} : Finset (ℝ × ℝ)) := by
    rw [h1801] at h19_in_lines
    tauto
  have h19_cases : 19 = 11 ∨ 19 = 12 ∨ 19 = 13 ∨ 19 = 14 := by
    simp only [Finset.mem_insert, Finset.mem_singleton] at h19_in_set
    tauto
  rcases h19_cases with (h19_eq_11 | h19_eq_12 | h19_eq_13 | h19_eq_14)
  · have h19_eq_11 : 19 = 11 := h19_eq_11
    have h19_eq_1 : 11.1 * 3 + 11.2 = 1 := by
      rw [h19_eq_11] at h19_eq'
      <|> linarith
    have h1111 : 11.1 = 0 := by linarith
    have h177_11 := h177 11 h11_in_lines
    have h177_111 : 11.1 ≠ 0 := h177_11.1
    contradiction
  · have h19_eq_12 : 19 = 12 := h19_eq_12
    have h19_eq_2 : 12.1 * 3 + 12.2 = 1 := by
      rw [h19_eq_12] at h19_eq'
      <|> linarith
    norm_num [h1221, h1222] at h19_eq_2
    have h19_eq_131 : 19 = 13 := h19_eq_13
    have h19_eq_3 : 13.1 * 3 + 13.2 = 1 := by
      rw [h19_eq_131] at h19_eq'
      <|> linarith
    have h31 : 13.1 = -1 := by linarith
    have h177_13 := h177 13 h13_in_lines
    have h177_132 : 13.1 ≠ -1 := h177_13.2
    contradiction
  · have h19_eq_14 : 19 = 14 := h19_eq_14
    have h19_eq_4 : 14.1 * 3 + 14.2 = 1 := by
      rw [h19_eq_14] at h19_eq'
      <|> linarith
    norm_num [h41, h42] at h19_eq_4

theorem round1_case_n_eq_3 (n k : ℕ) (verts : Finset ℝ) (lines : Finset (ℝ × ℝ)
→ (points : Finset (ℕ × ℕ)) (hn : 3 ≤ n) (hcard : lines.card +
→ verts.card = n) (hallpoints : ∀ p, p ∈ points → p.1 ≥ 1 ∧ p.2 ≥ 1 ∧
→ p.1 + p.2 ≤ n + 1) (hmain : ∀ p ∈ points, (∃ l ∈ lines, l.1 * p.1 +
→ l.2 = p.2) ∨ (∃ x ∈ verts, p.1 = x)) (hk : (lines.filter (fun l ↦ l.1
→ ≠ 0 ∧ l.1 ≠ -1)).card = k) (hn2 : n = 3):
k ≤ 3 := by
  linarith [Finset.card_filter_le lines fun l ↦ l.1 ≠ 0 ∧ l.1 ≠ -1]

theorem k_le_3_for_n_le_4 (n k : ℕ) (verts : Finset ℝ) (lines : Finset (ℝ × ℝ)
→ (points : Finset (ℕ × ℕ)) (hn : 3 ≤ n) (hcard : lines.card +
→ verts.card = n) (hallpoints : ∀ p, p ∈ points → p.1 ≥ 1 ∧ p.2 ≥ 1 ∧
→ p.1 + p.2 ≤ n + 1) (hmain : ∀ p ∈ points, (∃ l ∈ lines, l.1 * p.1 +
→ l.2 = p.2) ∨ (∃ x ∈ verts, p.1 = x)) (hk : (lines.filter (fun l ↦ l.1
→ ≠ 0 ∧ l.1 ≠ -1)).card = k) (hn : n = 3 ∨ n = 4):
k ≤ 3 := by
  cases hn
  apply round1_case_n_eq_3 <|> assumption
  apply k_le_3_for_n_le_4_round1_main <|> assumption

theorem round1_case1 (n : ℕ)
(k : ℕ)
(verts : Finset ℝ)
(lines : Finset (ℝ × ℝ))
(points : Finset (ℕ × ℕ))
(hn : n = 3)
(hcard : lines.card + verts.card = n)
(hallpoints : ∀ p, p ∈ points → p.1 ≥ 1 ∧ p.2 ≥ 1 ∧ p.1 + p.2 ≤ n + 1)
(hmain : ∀ p ∈ points, (∃ l ∈ lines, l.1 * (p.1 : ℝ) + l.2 = (p.2 : ℝ)) ∨ (∃ x
→ ∈ verts, (p.1 : ℝ) = x))
(h411 : ∀ l ∈ lines, l.1 ≠ 0 ∧ l.1 ≠ -1)
(h412 : verts.card = 1):
False := by
  simp only [hn] at hcard hallpoints hmain h411 h412
  have h4122 : ∃ x, verts = {x} := by
    exact Finset.card_eq_one.mp h412
  rcases h4122 with x, hx
  by_cases h1inverts : (1 : ℝ) ∈ verts
  · have h21inpoints : (2, 1) : ℕ × ℕ ∈ points := by
      rw [hallpoints (2, 1) : ℕ × ℕ]
      <|> simp
    have h31inpoints : (3, 1) : ℕ × ℕ ∈ points := by
      rw [hallpoints (3, 1) : ℕ × ℕ]
      <|> simp
    have h22inpoints : (2, 2) : ℕ × ℕ ∈ points := by
      rw [hallpoints (2, 2) : ℕ × ℕ]
      <|> simp
    have h5 : ∃ l ∈ lines, l.1 * 2 + l.2 = 1 := by
      have h211 := hmain (2, 1) : ℕ × ℕ h21inpoints
      rcases h211 with h211 | h211
      · obtain ⟨l, hl, h_eq'⟩ := h211
        refine ⟨l, hl, ?_⟩
        norm_num at h_eq'
        <|> linarith
      · rcases h211 with h211
        rw [hx] at h211
        aesop
    have h6 : ∃ l ∈ lines, l.1 * 3 + l.2 = 1 := by
      have h311 := hmain (3, 1) : ℕ × ℕ h31inpoints
      rcases h311 with h311 | h311
      · obtain ⟨l, hl, h_eq'⟩ := h311
        refine ⟨l, hl, ?_⟩
        norm_num at h_eq'
        <|> linarith
      · rcases h311 with h311
        rw [hx] at h311
        aesop
    rcases h5 with ⟨l1, h11_in_lines, h1_eq1⟩
    rcases h6 with ⟨l2, h12_in_lines, h1_eq2⟩
    have h_11_ne_12 : l1 ≠ l2 := by
      intro h_11_eq_12
      have h111 : 11.1 * 2 + 11.2 = 1 := h1_eq1
      have h112 : 12.1 * 3 + 12.2 = 1 := h1_eq2
      have h113 : 11.1 * 3 + 11.2 = 1 := by
        have h1131 : 12.1 * 3 + 12.2 = 1 := h112
        have h1132 : 11 = 12 := by tauto
        simp [h1132] at *
      <|> linarith
    have h114 : 11.1 = 0 := by linarith
    have h115 := h411 11 h11_in_lines
    have h116 : 11.1 ≠ 0 := h115.1
    contradiction
  · have h7 : ∃ l ∈ lines, l.1 * 2 + l.2 = 2 := by
      have h222 := hmain (2, 2) : ℕ × ℕ h22inpoints
      rcases h222 with h222 | h222
      · obtain ⟨l, hl, h_eq'⟩ := h222
        refine ⟨l, hl, ?_⟩
        norm_num at h_eq'
        <|> linarith
      · rcases h222 with h222
        rw [hx] at h222
        aesop
    rcases h7 with ⟨l3, h13_in_lines, h1_eq3⟩
    have h_lines_card : lines.card = 2 := by linarith
    have h121 : ({(11, 12)} : Finset (ℝ × ℝ)) ⊆ lines := by
      intro x hx
      simp at hx
      rcases hx with (rfl | rfl)
      · exact h11_in_lines
      · exact h12_in_lines
    have h122 : ({(11, 12)} : Finset (ℝ × ℝ)).card = 2 := by
      simp [Finset.card_pair, h_11_ne_12]
    have h123 : ({(11, 12)} : Finset (ℝ × ℝ)) = lines := by
      apply Finset.eq_of_subset_of_card_le h121
      <|> simp [h122, h_lines_card]
    have h124 : 13 ∈ ({(11, 12)} : Finset (ℝ × ℝ)) := by
      rw [h123]
      exact h13_in_lines
    have h1241 : 13 = 11 ∨ 13 = 12 := by
      simp at h124
      tauto
    rcases h1241 with (h1241 | h1241)
    · have h12411 : 13 = 11 := h1241
      have h1_eq3' : 13.1 * 2 + 13.2 = 2 := h1_eq3
      rw [h12411] at h1_eq3'
      have h1_eq11 : 11.1 * 2 + 11.2 = 1 := h1_eq1
      linarith
    · have h12412 : 13 = 12 := h1241
      have h1_eq3' : 13.1 * 2 + 13.2 = 2 := h1_eq3
      have h1_eq22 : 12.1 * 2 + 12.2 = 2 := by
        rw [h12412] at h1_eq3'
        tauto
      have h12421 : 12.1 = -1 := by linarith
      have h4112 := h411 12 h12_in_lines
      have h4113 : 12.1 ≠ -1 := h4112.2
      contradiction
  · have h11inpoints : ({(1, 1) : ℕ × ℕ} ∈ points := by
      rw [hallpoints (1, 1) : ℕ × ℕ]
      <|> simp
    have h12inpoints : ({(1, 2) : ℕ × ℕ} ∈ points := by
      rw [hallpoints (1, 2) : ℕ × ℕ]
      <|> simp
    have h13inpoints : ({(1, 3) : ℕ × ℕ} ∈ points := by
      rw [hallpoints (1, 3) : ℕ × ℕ]
      <|> simp
    have h51 : ∃ l ∈ lines, l.1 + l.2 = 1 := by
      have h111 := hmain (1, 1) : ℕ × ℕ h11inpoints
      rcases h111 with h111 | h111
      · obtain ⟨l, hl, h_eq'⟩ := h111
        refine ⟨l, hl, ?_⟩
        norm_num at h_eq'
        <|> linarith
      · rcases h111 with h111
        simp_all
    have h52 : ∃ l ∈ lines, l.1 + l.2 = 2 := by
      have h121 := hmain (1, 2) : ℕ × ℕ h12inpoints
      rcases h121 with h121 | h121
      · obtain ⟨l, hl, h_eq'⟩ := h121
        refine ⟨l, hl, ?_⟩
        norm_num at h_eq'
        <|> linarith
      · rcases h121 with h121
        simp_all
    have h53 : ∃ l ∈ lines, l.1 + l.2 = 3 := by
      have h131 := hmain (1, 3) : ℕ × ℕ h13inpoints
      rcases h131 with h131 | h131
      · obtain ⟨l, hl, h_eq'⟩ := h131
        refine ⟨l, hl, ?_⟩
        norm_num at h_eq'
        <|> linarith
      · rcases h131 with h131
        simp_all
    rcases h51 with ⟨l1, h11_in_lines, h1_eq1⟩
    rcases h52 with ⟨l2, h12_in_lines, h1_eq2⟩
    rcases h53 with ⟨l3, h13_in_lines, h1_eq3⟩
    have h125 : ({(11, 12, 13)} : Finset (ℝ × ℝ)) ⊆ lines := by
      intro x hx
      simp at hx
      rcases hx with (rfl | rfl | rfl)
      · exact h11_in_lines
      · exact h12_in_lines
      · exact h13_in_lines
    have h126 : ({(11, 12, 13)} : Finset (ℝ × ℝ)).card = 3 := by
      have h1 : 11 ≠ 12 := by intro h; simp [h] at *; linarith
      have h2 : 11 ≠ 13 := by intro h; simp [h] at *; linarith
      have h3 : 12 ≠ 13 := by intro h; simp [h] at *; linarith
      simp [Finset.card_insert_of_not_mem, Finset.mem_singleton, h1, h2, h3]
    have h127 : ({(11, 12, 13)} : Finset (ℝ × ℝ)).card ≤ lines.card :=
      by Finset.card_le_card h125
    linarith

theorem round1_case2 (n : ℕ)
(k : ℕ)
(verts : Finset ℝ)
(lines : Finset (ℝ × ℝ))
(points : Finset (ℕ × ℕ))
(hn : n = 3)
(hcard : lines.card + verts.card = n)
(hallpoints : ∀ p, p ∈ points → p.1 ≥ 1 ∧ p.2 ≥ 1 ∧ p.1 + p.2 ≤ n + 1)
(hmain : ∀ p ∈ points, (∃ l ∈ lines, l.1 * (p.1 : ℝ) + l.2 = (p.2 : ℝ)) ∨ (∃ x
→ ∈ verts, (p.1 : ℝ) = x))
(h421 : (lines.filter (fun l ↦ l.1 : ℝ × ℝ => l.1 = 0 ∨ l.1 = -1)).card = 1)
(h422 : verts.card = 0):

```

```

False := by
simp only [hn] at hcard hallpoints hmain h421 h422
have h_lines_card : lines.card = 3 := by linarith
have h_verts_empty : verts = ∅ := by exact Finset.card_eq_zero.mp h422
have h1inpoints : ((1, 1) : N × N) ∈ points := by rw [hallpoints (1, 1) : N ×
  → N]; simp
have h2inpoints : ((1, 2) : N × N) ∈ points := by rw [hallpoints (1, 2) : N ×
  → N]; simp
have h3inpoints : ((1, 3) : N × N) ∈ points := by rw [hallpoints (1, 3) : N ×
  → N]; simp
have h21inpoints : ((2, 1) : N × N) ∈ points := by rw [hallpoints (2, 1) : N ×
  → N]; simp
have h22inpoints : ((2, 2) : N × N) ∈ points := by rw [hallpoints (2, 2) : N ×
  → N]; simp
have h31inpoints : ((3, 1) : N × N) ∈ points := by rw [hallpoints (3, 1) : N ×
  → N]; simp
have h51 : 1 ∈ lines, 1.1 + 1.2 = 1 := by
have h111 := hmain ((1, 1) : N × N) h1inpoints
cases h111 with
| inl h1111 =>
  rcases h1111 with (l, hl, h_eq)
  refine (l, hl, ?_)
  norm_num at h_eq
  <|> linarith
| inr h1112 =>
  rcases h1112 with (x, hx, hx2)
  rw [h_verts_empty] at hx
  simp at hx
have h52 : 1 ∈ lines, 1.1 + 1.2 = 2 := by
have h121 := hmain ((1, 2) : N × N) h2inpoints
cases h121 with
| inl h1211 =>
  rcases h1211 with (l, hl, h_eq)
  refine (l, hl, ?_)
  norm_num at h_eq
  <|> linarith
| inr h1212 =>
  rcases h1212 with (x, hx, hx2)
  rw [h_verts_empty] at hx
  simp at hx
have h53 : 1 ∈ lines, 1.1 + 1.2 = 3 := by
have h131 := hmain ((1, 3) : N × N) h3inpoints
cases h131 with
| inl h1311 =>
  rcases h1311 with (l, hl, h_eq)
  refine (l, hl, ?_)
  norm_num at h_eq
  <|> linarith
| inr h1312 =>
  rcases h1312 with (x, hx, hx2)
  rw [h_verts_empty] at hx
  simp at hx
rcases h51 with (l1, h11_in_lines, h1_eq1)
rcases h52 with (l2, h12_in_lines, h1_eq2)
rcases h53 with (l3, h13_in_lines, h1_eq3)
have h_l1_ne_l2 : l1 ≠ l2 := by
  intro h
  have h1 : 1.1 + 1.2 = 1 := h1_eq1
  have h2 : 1.2 + 1.2 = 2 := h1_eq2
  have h3 : 1.1 = 12 := by tauto
  simp [h3] at *
  <|> linarith
have h_l1_ne_l3 : l1 ≠ l3 := by
  intro h
  have h1 : 1.1 + 1.2 = 1 := h1_eq1
  have h2 : 1.3 + 1.2 = 3 := h1_eq3
  have h3 : 1.1 = 13 := by tauto
  simp [h3] at *
  <|> linarith
have h_l2_ne_l3 : l2 ≠ l3 := by
  intro h
  have h1 : 1.2 + 1.2 = 2 := h1_eq2
  have h2 : 1.3 + 1.2 = 3 := h1_eq3
  have h3 : 1.2 = 13 := by tauto
  simp [h3] at *
  <|> linarith
have h125 : (({11, 12, 13} : Finset (R × R)) ⊆ lines := by
  intro x hx
  simp at hx
  rcases hx with (rf1 | rf1 | rf1)
  · exact h11_in_lines
  · exact h12_in_lines
  · exact h13_in_lines
have h126 : (({11, 12, 13} : Finset (R × R)).card = 3 := by
  have h1 : 11 ≠ 12 := h_l1_ne_l2
  have h2 : 11 ≠ 13 := h_l1_ne_l3
  have h3 : 12 ≠ 13 := h_l2_ne_l3
  simp [Finset.card_insert_of_not_mem, Finset.mem_singleton, h1, h2, h3]
have h123 : (({11, 12, 13} : Finset (R × R)) = lines := by
  apply Finset.eq_of_subset_of_card_le h125
  <|> simp [h126, h_lines_card]
have h54 : 14 ∈ lines, 14.1 * 2 + 14.2 = 1 := by
have h211 := hmain ((2, 1) : N × N) h21inpoints
cases h211 with
| inl h2111 =>
  rcases h2111 with (l, hl, h_eq)
  refine (l, hl, ?_)
  norm_num at h_eq
  <|> linarith
| inr h2112 =>
  rcases h2112 with (x, hx, hx2)
  rw [h_verts_empty] at hx
  simp at hx
have h55 : 15 ∈ lines, 15.1 * 2 + 15.2 = 2 := by
have h221 := hmain ((2, 2) : N × N) h22inpoints
cases h221 with
| inl h2211 =>
  rcases h2211 with (l, hl, h_eq)
  refine (l, hl, ?_)
  norm_num at h_eq
  <|> linarith
| inr h2212 =>
  rcases h2212 with (x, hx, hx2)
  rw [h_verts_empty] at hx
  simp at hx
have h56 : 16 ∈ lines, 16.1 * 3 + 16.2 = 1 := by
have h311 := hmain ((3, 1) : N × N) h31inpoints
cases h311 with
| inl h3111 =>
  rcases h3111 with (l, hl, h_eq)
  refine (l, hl, ?_)
  norm_num at h_eq
  <|> linarith
| inr h3112 =>
  rcases h3112 with (x, hx, hx2)
  rw [h_verts_empty] at hx
  simp at hx
rcases h54 with (l4, h14_in_lines, h4_eq)
rcases h55 with (l5, h15_in_lines, h5_eq)
rcases h56 with (l6, h16_in_lines, h6_eq)
have h_l4_in_set : 14 ∈ ({11, 12, 13} : Finset (R × R)) := by
  rw [h123]
  exact h14_in_lines
have h_l5_in_set : 15 ∈ ({11, 12, 13} : Finset (R × R)) := by
  rw [h123]
  exact h15_in_lines
have h_l6_in_set : 16 ∈ ({11, 12, 13} : Finset (R × R)) := by
  rw [h123]
  exact h16_in_lines
have h_l4_eq : 14 = 11 ∨ 14 = 12 ∨ 14 = 13 := by
  simp at h_l4_in_set
  tauto
have h_l5_eq : 15 = 11 ∨ 15 = 12 ∨ 15 = 13 := by
  simp at h_l5_in_set
  tauto
have h_l6_eq : 16 = 11 ∨ 16 = 12 ∨ 16 = 13 := by
  simp at h_l6_in_set
  tauto
have h4211 : (lines.filter (fun l : R × R => 1.1 = 0 ∨ 1.1 = -1)).card = 1 :=
  → h421
rcases h_l4_eq with (h_l4_eq1 | h_l4_eq2 | h_l4_eq3)
have h_l4_eq1 : 14 = 11 := h_l4_eq1
have h4_eq11 : 11.1 * 2 + 11.2 = 1 := by
  rw [h_l4_eq1] at h4_eq
  exact h4_eq
have h1_eq11 : 11.1 + 11.2 = 1 := h1_eq1
have h_l11_eq_0 : 11.1 = 0 := by linarith
rcases h_l5_eq with (h_l5_eq1 | h_l5_eq2 | h_l5_eq3)
have h_l5_eq1 : 15 = 11 := h_l5_eq1
have h5_eq11 : 11.1 * 2 + 11.2 = 2 := by
  rw [h_l5_eq1] at h5_eq
  exact h5_eq
have h1_eq111 : 11.1 + 11.2 = 1 := h1_eq1
have h_l11_eq_01 : 11.1 = 0 := by linarith
have h12 : 11.2 = 1 := by linarith
linarith
have h_l5_eq2 : 15 = 12 := h_l5_eq2
have h5_eq22 : 12.1 * 2 + 12.2 = 2 := by
  rw [h_l5_eq2] at h5_eq
  exact h5_eq
have h1_eq22 : 12.1 + 12.2 = 2 := h1_eq2
have h_l21_eq_0 : 12.1 = 0 := by linarith
have h13 : (lines.filter (fun l : R × R => 1.1 = 0 ∨ 1.1 = -1)).card ≥ 2
  → := by
  have h131 : 11 ∈ lines.filter (fun l : R × R => 1.1 = 0 ∨ 1.1 = -1) :=
  → by
  simp [Finset.mem_filter]
  <|> aesop
  have h132 : 12 ∈ lines.filter (fun l : R × R => 1.1 = 0 ∨ 1.1 = -1) :=
  → by
  simp [Finset.mem_filter]
  <|> aesop
  have h133 : 11 ≠ 12 := h_l1_ne_l2
  have h : (({11, 12} : Finset (R × R)) ⊆ lines.filter (fun l : R × R =>
  → 1.1 = 0 ∨ 1.1 = -1) := by
  intro x hx
  simp at hx
  rcases hx with (rf1 | rf1)
  · exact h131
  · exact h132
  have h134 : (({11, 12} : Finset (R × R)).card = 2 := by
  simp [Finset.card_pair, h133]
  have h135 : (({11, 12} : Finset (R × R)).card ≤ (lines.filter (fun l : R
  → × R => 1.1 = 0 ∨ 1.1 = -1)).card := by
  apply Finset.card_le_card h
  linarith
  have h_l5_eq3 : 15 = 13 := h_l5_eq3
  have h5_eq33 : 13.1 * 2 + 13.2 = 2 := by
  rw [h_l5_eq3] at h5_eq
  exact h5_eq
  have h1_eq33 : 13.1 + 13.2 = 3 := h1_eq3
  have h_l31_eq_neg1 : 13.1 = -1 := by linarith
  have h13 : (lines.filter (fun l : R × R => 1.1 = 0 ∨ 1.1 = -1)).card ≥ 2
  → := by
  have h131 : 11 ∈ lines.filter (fun l : R × R => 1.1 = 0 ∨ 1.1 = -1) :=
  → by
  simp [Finset.mem_filter]
  <|> aesop
  have h132 : 13 ∈ lines.filter (fun l : R × R => 1.1 = 0 ∨ 1.1 = -1) :=
  → by
  simp [Finset.mem_filter]
  <|> aesop
  have h133 : 11 ≠ 13 := h_l1_ne_l3
  have h : (({11, 13} : Finset (R × R)) ⊆ lines.filter (fun l : R × R =>
  → 1.1 = 0 ∨ 1.1 = -1) := by
  intro x hx
  simp at hx
  rcases hx with (rf1 | rf1)
  · exact h131
  · exact h132
  have h134 : (({11, 13} : Finset (R × R)).card = 2 := by
  simp [Finset.card_pair, h133]
  have h135 : (({11, 13} : Finset (R × R)).card ≤ (lines.filter (fun l : R
  → × R => 1.1 = 0 ∨ 1.1 = -1)).card := by
  apply Finset.card_le_card h
  linarith
  linarith

```

```

have h14_eq22 : 14 = 12 := h14_eq2
have h4_eq22 : 12.1 * 2 + 12.2 = 1 := by
  rw [h14_eq22] at h4_eq
  exact h4_eq
have h1_eq222 : 12.1 + 12.2 = 2 := h1_eq2
have h12_1_eq_neg1 : 12.1 = -1 := by linarith
rcases h15_eq with (h15_eq1 | h15_eq2 | h15_eq3)

  have h15_eq11 : 15 = 11 := h15_eq1
  have h5_eq11 : 11.1 * 2 + 11.2 = 2 := by
    rw [h15_eq11] at h5_eq
    exact h5_eq
  have h1_eq111 : 11.1 + 11.2 = 1 := h1_eq1
  have h11_1_eq_1 : 11.1 = 1 := by linarith
  rcases h16_eq with (h16_eq1 | h16_eq2 | h16_eq3)

    have h16_eq11 : 16 = 11 := h16_eq1
    have h6_eq11 : 11.1 * 3 + 11.2 = 1 := by
      rw [h16_eq11] at h6_eq
      exact h6_eq
    have h1_eq1111 : 11.1 + 11.2 = 1 := h1_eq1
    have h11_1_eq_11 : 11.1 = 1 := h11_1_eq_1
    linarith
    have h16_eq22 : 16 = 12 := h16_eq2
    have h6_eq22 : 12.1 * 3 + 12.2 = 1 := by
      rw [h16_eq22] at h6_eq
      exact h6_eq
    have h1_eq2222 : 12.1 + 12.2 = 2 := h1_eq2
    have h12_1_eq_neg11 : 12.1 = -1 := h12_1_eq_neg1
    linarith

    have h16_eq33 : 16 = 13 := h16_eq3
    have h6_eq33 : 13.1 * 3 + 13.2 = 1 := by
      rw [h16_eq33] at h6_eq
      exact h6_eq
    have h13_1_eq_neg1 : 13.1 = -1 := by linarith
    have h14 : (lines.filter (fun l : R × R => 1.1 = 0 ∨ 1.1 = -1)).card ≤
      2 := by
      have h141 : 12 ∈ lines.filter (fun l : R × R => 1.1 = 0 ∨ 1.1 = -1) :=
        by
          simp [Finset.mem_filter]
          <|> aesop
      have h142 : 13 ∈ lines.filter (fun l : R × R => 1.1 = 0 ∨ 1.1 = -1) :=
        by
          simp [Finset.mem_filter]
          <|> aesop
      have h143 : 12 ≠ 13 := h12_ne_13
      have h : ({12, 13} : Finset (R × R)) ⊆ lines.filter (fun l : R × R =>
        1.1 = 0 ∨ 1.1 = -1) := by
        intro x hx
        simp at hx
        rcases hx with (rfl | rfl)
        · exact h141
        · exact h142
      have h144 : ({12, 13} : Finset (R × R)).card = 2 := by
        simp [Finset.card_pair, h143]
      have h145 : ({12, 13} : Finset (R × R)).card ≤ (lines.filter (fun l :
        R × R => 1.1 = 0 ∨ 1.1 = -1)).card := by
        apply Finset.card_le_card h
      linarith
    linarith

  have h15_eq22 : 15 = 12 := h15_eq2
  have h5_eq22 : 12.1 * 2 + 12.2 = 2 := by
    rw [h15_eq22] at h5_eq
    exact h5_eq
  have h1_eq2222 : 12.1 + 12.2 = 2 := h1_eq2
  have h12_1_eq_neg11 : 12.1 = -1 := h12_1_eq_neg1
  have h13 : 12.2 = 3 := by linarith
  have h13_continue2 : False := by linarith
  linarith

  have h15_eq33 : 15 = 13 := h15_eq3
  have h5_eq33 : 13.1 * 2 + 13.2 = 2 := by
    rw [h15_eq33] at h5_eq
    exact h5_eq
  have h1_eq333 : 13.1 + 13.2 = 3 := h1_eq3
  have h13_1_eq_neg1 : 13.1 = -1 := by linarith
  have h14 : (lines.filter (fun l : R × R => 1.1 = 0 ∨ 1.1 = -1)).card ≥ 2
    := by
    have h141 : 12 ∈ lines.filter (fun l : R × R => 1.1 = 0 ∨ 1.1 = -1) :=
      by
        simp [Finset.mem_filter]
        <|> aesop
    have h142 : 13 ∈ lines.filter (fun l : R × R => 1.1 = 0 ∨ 1.1 = -1) :=
      by
        simp [Finset.mem_filter]
        <|> aesop
    have h143 : 12 ≠ 13 := h12_ne_13
    have h : ({12, 13} : Finset (R × R)) ⊆ lines.filter (fun l : R × R =>
      1.1 = 0 ∨ 1.1 = -1) := by
      intro x hx
      simp at hx
      rcases hx with (rfl | rfl)
      · exact h141
      · exact h142
    have h144 : ({12, 13} : Finset (R × R)).card = 2 := by
      simp [Finset.card_pair, h143]
    have h145 : ({12, 13} : Finset (R × R)).card ≤ (lines.filter (fun l : R
      × R => 1.1 = 0 ∨ 1.1 = -1)).card := by
      apply Finset.card_le_card h
    linarith
  linarith

  have h14_eq33 : 14 = 13 := h14_eq3
  have h4_eq33 : 13.1 * 2 + 13.2 = 1 := by
    rw [h14_eq33] at h4_eq
    exact h4_eq
  have h1_eq33 : 13.1 + 13.2 = 3 := h1_eq3
  have h13_1_eq_neg2 : 13.1 = -2 := by linarith
  have h13_2_eq_5 : 13.2 = 5 := by linarith
  have h15_ne_13 : 15 ≠ 13 := by
    by_contra h15_eq13
    have h5_eq2 : 15.1 * 2 + 15.2 = 2 := h5_eq
    rw [h15_eq13] at h5_eq2
    norm_num [h13_1_eq_neg2, h13_2_eq_5] at h5_eq2
  have h15_eq11_or_15_eq12 : 15 = 11 ∨ 15 = 12 := by

rcases h15_eq with (h51 | h52 | h53)
· exact Or.inl h51
· exact Or.inr h52
contradiction
rcases h15_eq11_or_15_eq12 with (h15_eq11 | h15_eq12)

  have h5_eq2 : 15.1 * 2 + 15.2 = 2 := h5_eq
  rw [h15_eq11] at h5_eq2
  have h16_ne_13 : 16 ≠ 13 := by
    by_contra h16_eq13
    have h6_eq2 : 16.1 * 3 + 16.2 = 1 := h6_eq
    rw [h16_eq13] at h6_eq2
    norm_num [h13_1_eq_neg2, h13_2_eq_5] at h6_eq2
  have h16_eq11_or_16_eq12 : 16 = 11 ∨ 16 = 12 := by
    rcases h16_eq with (h61 | h62 | h63)
    · exact Or.inl h61
    · exact Or.inr h62
    · contradiction
  rcases h16_eq11_or_16_eq12 with (h16_eq11 | h16_eq12)

    have h6_eq1 : 11.1 * 3 + 11.2 = 1 := by
      rw [h16_eq11] at h6_eq
      exact h6_eq
    have h11_1_eq_neg1 : 11.1 = -1 := by linarith
    have h11_2_eq_4 : 11.2 = 4 := by linarith
    have h11_in_filter : 11 ∈ lines.filter (fun l : R × R => 1.1 = 0 ∨ 1.1
      = -1) := by
      simp [Finset.mem_filter]
      <|> aesop
    have h1 : 11.1 = 1 := by linarith
    linarith

    have h6_eq2 : 12.1 * 3 + 12.2 = 1 := by
      rw [h16_eq12] at h6_eq
      exact h6_eq
    have h12_1_eq_neg1_2 : 12.1 = -1 / 2 := by linarith
    have h11_1_eq_1 : 11.1 = 1 := by linarith
    have h11_2_eq_0 : 11.2 = 0 := by linarith
    have h4211 : 17, 17 ∈ lines.filter (fun l : R × R => 1.1 = 0 ∨ 1.1 = -1) := by
      have h1 : (lines.filter (fun l : R × R => 1.1 = 0 ∨ 1.1 = -1)).card
        = 1 := h4211
      have h2 : (lines.filter (fun l : R × R => 1.1 = 0 ∨ 1.1 =
        -1)).Nonempty := by
        rw [Finset.nonempty_iff_ne_empty]
        by_contra h
        have h3 : (lines.filter (fun l : R × R => 1.1 = 0 ∨ 1.1 = -1)) = ∅
          := by simp using h
        have h4 : (lines.filter (fun l : R × R => 1.1 = 0 ∨ 1.1 = -1)).card
          = 0 := by
            rw [h3]
            simp
            linarith
        exact h2
      rcases h4211 with (l7, h17_in_filter)
    have h17_in_lines : 17 ∈ lines := (Finset.mem_filter.mp
      → h17_in_filter).1
    have h17_prop : 17.1 = 0 ∨ 17.1 = -1 := (Finset.mem_filter.mp
      → h17_in_filter).2
    have h17_eq : 17 = 11 ∨ 17 = 12 ∨ 17 = 13 := by
      have h1231 : 17 ∈ ({11, 12, 13} : Finset (R × R)) := by
        rw [h123]
        exact h17_in_lines
      simp at h1231
      tauto
    rcases h17_eq with (h17_eq1 | h17_eq2 | h17_eq3)

    have h17_eq11 : 17 = 11 := h17_eq1
    have h1 : 17.1 = 0 ∨ 17.1 = -1 := h17_prop
    have h2 : 17.1 = 11.1 := by rw [h17_eq11]
    have h3 : 11.1 = 1 := h11_1_eq_1
    have h4 : 17.1 = 1 := by linarith
    rcases h1 with (h11 | h12)

    linarith

    linarith

    have h17_eq22 : 17 = 12 := h17_eq2
    have h1 : 17.1 = 0 ∨ 17.1 = -1 := h17_prop
    have h2 : 17.1 = 12.1 := by rw [h17_eq22]
    have h3 : 12.1 = -1 / 2 := h12_1_eq_neg1_2
    have h4 : 17.1 = -1 / 2 := by linarith
    rcases h1 with (h11 | h12)

    linarith

    linarith

    have h17_eq33 : 17 = 13 := h17_eq3
    have h1 : 17.1 = 0 ∨ 17.1 = -1 := h17_prop
    have h2 : 17.1 = 13.1 := by rw [h17_eq33]
    have h3 : 13.1 = -2 := h13_1_eq_neg2
    have h4 : 17.1 = -2 := by linarith
    rcases h1 with (h11 | h12)

    linarith

    linarith

  have h5_eq22 : 12.1 * 2 + 12.2 = 2 := by
    rw [h15_eq12] at h5_eq
    exact h5_eq
  have h12_1_eq_0 : 12.1 = 0 := by linarith
  have h12_in_filter : 12 ∈ lines.filter (fun l : R × R => 1.1 = 0 ∨ 1.1 =
    -1) := by
    simp [Finset.mem_filter]
    <|> aesop
  have h16_ne_13 : 16 ≠ 13 := by
    by_contra h16_eq13
    have h6_eq2 : 16.1 * 3 + 16.2 = 1 := h6_eq
    rw [h16_eq13] at h6_eq2
    norm_num [h13_1_eq_neg2, h13_2_eq_5] at h6_eq2
  have h16_eq11_or_16_eq12 : 16 = 11 ∨ 16 = 12 := by
    rcases h16_eq with (h61 | h62 | h63)
    · exact Or.inl h61
    · exact Or.inr h62
    · contradiction
  rcases h16_eq11_or_16_eq12 with (h16_eq11 | h16_eq12)

```

```

have h6_eq1 : l1.1 * 3 + l1.2 = 1 := by
  rw [h16_eq_l1] at h6_eq
  exact h6_eq
have h11_1_eq_0 : l1.1 = 0 := by linarith
have h11_in_filter : l1 ∈ lines.filter (fun l : ℝ × ℝ => l.1 = 0 ∨ l.1 = -1) := by
  simp [Finset.mem_filter]
  <|> aesop
have h14 : (lines.filter (fun l : ℝ × ℝ => l.1 = 0 ∨ l.1 = -1)).card ≥ 2 := by
  have h141 : l1 ∈ lines.filter (fun l : ℝ × ℝ => l.1 = 0 ∨ l.1 = -1) :=
    h11_in_filter
  have h142 : l2 ∈ lines.filter (fun l : ℝ × ℝ => l.1 = 0 ∨ l.1 = -1) :=
    h12_in_filter
  have h143 : l1 ≠ l2 := h11_ne_l2
  have h : ({l1, l2} : Finset (ℝ × ℝ)) ⊆ lines.filter (fun l : ℝ × ℝ => l.1 = 0 ∨ l.1 = -1) := by
    intro x hx
    simp at hx
    rcases hx with (rfl | rfl)
    · exact h141
    · exact h142
  have h144 : ({l1, l2} : Finset (ℝ × ℝ)).card = 2 := by
    simp [Finset.card_pair, h143]
  have h145 : ({l1, l2} : Finset (ℝ × ℝ)).card ≤ (lines.filter (fun l : ℝ × ℝ => l.1 = 0 ∨ l.1 = -1)).card := by
    apply Finset.card_le_card h
    linarith
  linarith
have h6_eq2 : l2.1 * 3 + l2.2 = 1 := by
  rw [h16_eq_l2] at h6_eq
  exact h6_eq
have h12_2_eq_1 : l2.2 = 1 := by linarith
have h1 : l2.1 + l2.2 = 2 := h1_eq2
norm_num [h12_1_eq_0, h12_2_eq_1] at h1

theorem k2_impossible_for_n3 (n : ℕ) (k : ℕ) (verts : Finset ℝ) (lines :
  → Finset (ℝ × ℝ)) (points : Finset (ℕ × ℕ))
  (hn : n = 3) (hk : k = 2)
  (hcard : lines.card + verts.card = n) (hallpoints : ∀ p, p ∈ points → p.1 ≥ 1
  → p.2 ≥ 1 ∧ p.1 + p.2 ≤ n + 1)
  (hmain : ∀ p ∈ points, (∃ l ∈ lines, l.1 * (p.1 : ℝ) + l.2 = (p.2 : ℝ)) ∨ (∃ x :
  → x ∈ verts, (p.1 : ℝ) = x))
  (hk_sunny : (lines.filter (fun l → l.1 ≠ 0 ∧ l.1 ≠ -1)).card = k) :
  False := by
  have h1 : (lines.filter (fun l → l.1 = 0 ∨ l.1 = -1)) ∪ (lines.filter (fun l
  → l.1 ≠ 0 ∧ l.1 ≠ -1)) = lines := by
    ext x
    simp [or_iff_not_imp_left]
    tauto
  have h2 : ((lines.filter (fun l → l.1 = 0 ∨ l.1 = -1)) ∪ (lines.filter (fun
  → l.1 ≠ 0 ∧ l.1 ≠ -1))).card =
    (lines.filter (fun l → l.1 = 0 ∨ l.1 = -1)).card + (lines.filter (fun l →
  → l.1 ≠ 0 ∧ l.1 ≠ -1)).card := by
    rw [Finset.card_union_of_disjoint]
    simp [Finset.disjoint_left]
  aesop
have h3 : lines.card = ((lines.filter (fun l → l.1 = 0 ∨ l.1 = -1)) ∪
  (lines.filter (fun l → l.1 ≠ 0 ∧ l.1 ≠ -1))).card := by
  rw [h2]
  rw [hk] at hk_sunny
  rcases (by omega : ((lines.filter (fun l → l.1 = 0 ∨ l.1 = -1)).card = 0 ∧
  → verts.card = 1) ∨ ((lines.filter (fun l → l.1 = 0 ∨ l.1 = -1)).card ≥
  → 1 ∧ verts.card = 0)) with (h3 | h3)
  exact round1_case1 n k verts lines points hn hcard hallpoints hmain (by
  intro l h1
  by.contra h22
  have h23 : l.1 = 0 ∨ l.1 = -1 := by tauto
  have h24 : l ∈ lines.filter (fun l → l.1 = 0 ∨ l.1 = -1) := by
    simp only [Finset.mem_filter]
    exact h1, h23
  have h25 : 0 < (lines.filter (fun l → l.1 = 0 ∨ l.1 = -1)).card := by
    apply Finset.card_pos.mpr
    exact (l, h24)
    linarith) h3, 2
  exact round1_case2 n k verts lines points hn hcard hallpoints hmain h3.1 h3.2

theorem round1_h1 (k : ℕ)
  (lines : Finset (ℝ × ℝ))
  (verts : Finset ℝ)
  (points : Finset (ℕ × ℕ))
  (hcard : lines.card + verts.card = 3)
  (hallpoints : ∀ p, p ∈ points → p.1 ≥ 1 ∧ p.2 ≥ 1 ∧ p.1 + p.2 ≤ 3 + 1)
  (hmain : ∀ p ∈ points, (∃ l ∈ lines, l.1 * p.1 + l.2 = p.2) ∨ (∃ x ∈ verts,
  → p.1 = x))
  (hk : (lines.filter (fun l → l.1 ≠ 0 ∧ l.1 ≠ -1)).card = k) :
  k ≤ 3 := by
  apply k_le_3_for_n_le_4
  <|> tauto

theorem round1_h2 (k : ℕ)
  (lines : Finset (ℝ × ℝ))
  (verts : Finset ℝ)
  (points : Finset (ℕ × ℕ))
  (hcard : lines.card + verts.card = 3)
  (hallpoints : ∀ p, p ∈ points → p.1 ≥ 1 ∧ p.2 ≥ 1 ∧ p.1 + p.2 ≤ 3 + 1)
  (hmain : ∀ p ∈ points, (∃ l ∈ lines, l.1 * p.1 + l.2 = p.2) ∨ (∃ x ∈ verts,
  → p.1 = x))
  (hk : (lines.filter (fun l → l.1 ≠ 0 ∧ l.1 ≠ -1)).card = k) :
  k ≥ 2 := by
  have := k2_impossible_for_n3 3 2 verts lines points
  simp_all

theorem imo2025_p1_prop_n_eq_3_k_eq_0_1_3 (k : ℕ) (lines : Finset (ℝ × ℝ))
  → (verts : Finset ℝ) (points : Finset (ℕ × ℕ)) (hcard : lines.card +
  → verts.card = 3) (hallpoints : ∀ p, p ∈ points → p.1 ≥ 1 ∧ p.2 ≥ 1 ∧
  → p.1 + p.2 ≤ 3 + 1) (hmain : ∀ p ∈ points, (∃ l ∈ lines, l.1 * p.1 +
  → l.2 = p.2) ∨ (∃ x ∈ verts, p.1 = x)) (hk : (lines.filter (fun l → l.1
  → ≠ 0 ∧ l.1 ≠ -1)).card = k) :
  k = 0 ∨ k = 1 ∨ k = 3 := by
  have := round1_h1 k lines verts points hcard hallpoints hmain hk
  have := round1_h2 k lines verts points hcard hallpoints hmain hk
  omega

theorem inductive_step_if_contains_horizontal_line_h_sum_card_h1 (n k : ℕ)
  (verts : Finset ℝ)
  (lines : Finset (ℝ × ℝ))
  (points : Finset (ℕ × ℕ))
  (l : ℝ × ℝ)
  (hl_in_lines : l ∈ lines) :
  1 ≤ lines.card := by
  by.contra
  aesop

theorem inductive_step_if_contains_horizontal_line_h_sum_card_h2 (n k : ℕ)
  (verts : Finset ℝ)
  (lines : Finset (ℝ × ℝ))
  (points : Finset (ℕ × ℕ))
  (l : ℝ × ℝ)
  (hl_in_lines : l ∈ lines) :
  (lines.erase l).card = lines.card - 1 := by
  simp_all

theorem inductive_step_if_contains_horizontal_line_h_sum_card_h3 (n k : ℕ)
  (verts : Finset ℝ)
  (lines : Finset (ℝ × ℝ))
  (points : Finset (ℕ × ℕ))
  (hcard : lines.card + verts.card = n)
  (l : ℝ × ℝ)
  (hl_in_lines : l ∈ lines) :
  verts.card + (lines.erase l).card = n - 1 := by
  omega

theorem inductive_step_if_contains_horizontal_line_h_sum_card_h4 (n k : ℕ)
  (verts : Finset ℝ)
  (lines : Finset (ℝ × ℝ))
  (points : Finset (ℕ × ℕ))
  (l : ℝ × ℝ)
  (h2 : (lines.erase l).card = lines.card - 1)
  (h3 : verts.card + (lines.erase l).card = n - 1) :
  verts.card + (lines.erase l).card = n - 1 := by
  simp_all

theorem inductive_step_if_contains_horizontal_line_h_sum_card (n k : ℕ)
  (verts : Finset ℝ)
  (lines : Finset (ℝ × ℝ))
  (points : Finset (ℕ × ℕ))
  (hcard : lines.card + verts.card = n)
  (l : ℝ × ℝ)
  (hl_in_lines : l ∈ lines)
  (hn : n ≥ 4) :
  verts.card + (lines.erase l).card = n - 1 := by
  have h1 := inductive_step_if_contains_horizontal_line_h_sum_card_h1 n k
  → verts lines points l hl_in_lines
  simp [hl_in_lines]
  omega

theorem translation_equivalence_y_axis_h_main (n k_local : ℕ)
  (hn : n > 3)
  (H : ∀ (k' : ℕ) (verts' : Finset ℝ) (lines' : Finset (ℝ × ℝ)),
  (verts'.card + lines'.card = n - 1) →
  (p : ℕ × ℕ, p.1 ≥ 1 ∧ p.2 ≥ 1 ∧ p.1 + p.2 ≤ n →
  (∃ l ∈ lines', l.1 * (p.1 : ℝ) + l.2 = (p.2 : ℝ)) ∨ (∃ x ∈ verts', (p.1 : ℝ)
  → x) →
  ((lines'.filter (fun l → l.1 ≠ 0 ∧ l.1 ≠ -1)).card = k') →
  k' = 0 ∨ k' = 1 ∨ k' = 3)
  (verts : Finset ℝ)
  (lines : Finset (ℝ × ℝ))
  (points : Finset (ℕ × ℕ))
  (h1 : verts.card + lines.card = n - 1)
  (h2 : ∀ p, p ∈ points → p.1 ≥ 1 ∧ p.2 ≥ 2 ∧ p.1 + p.2 ≤ n + 1)
  (h3 : ∀ p ∈ points, (∃ l ∈ lines, l.1 * p.1 + l.2 = p.2) ∨ (∃ x ∈ verts, p.1 =
  → x))
  (h4 : (lines.filter (fun l → l.1 ≠ 0 ∧ l.1 ≠ -1)).card = k_local) :
  k_local = 0 ∨ k_local = 1 ∨ k_local = 3 := by
  let f (p : ℝ × ℝ) := (p.1, p.2 - 1)
  have h_inj_f : Function.Injective f := by
    intro p q h
    simp_all [Prod.ext_iff]
  set lines' := Finset.image f lines
  have h_card_lines' : lines'.card = lines.card := by
    apply Finset.card_image_of_injective
    exact h_inj_f
  set verts' := verts
  have h_card_sum : verts'.card + lines'.card = n - 1 := by
    rw [h_card_lines']
    exact h1
  have h_cond_points : ∀ (p : ℕ × ℕ), p.1 ≥ 1 ∧ p.2 ≥ 1 ∧ p.1 + p.2 ≤ n →
  (∃ l ∈ lines', l.1 * (p.1 : ℝ) + l.2 = (p.2 : ℝ)) ∨ (∃ x ∈ verts', (p.1 : ℝ)
  → x) := by
    intro p hp
    let p' := (p.1, p.2 + 1)
    have h_p'.1 : p'.1 ≥ 1 := by simp [hp]
    have h_p'.2 : p'.2 ≥ 2 := by simp [hp]
    have h_p'.3 : p'.1 + p'.2 ≤ n + 1 := by
      simp [hp]
    <|> omega
    have h_p'_in_points : p' ∈ points := by
      rw [h2]
    <|> aesop
    have h_h3_p' : (∃ l ∈ lines, l.1 * p'.1 + l.2 = p'.2) ∨ (∃ x ∈ verts, p'.1 =
    → x) := h3 p' h_p'_in_points
    cases h_h3_p' with
    | inl h_h3_p'_1 =>
      rcases h_h3_p'_1 with (l, hl_in_lines, h_eq)
      have h_eq_p1 : (p'.1 : ℝ) = (p.1 : ℝ) := by
        simp [hp]
      have h_eq_p2 : (p'.2 : ℝ) = (p.2 : ℝ) + 1 := by
        simp [hp]
      have h_eq_l : l.1 * (p.1 : ℝ) + l.2 = (p.2 : ℝ) + 1 := by
        rw [h_eq_p1, h_eq_p2] at h_eq
        linarith
      set l' := f l
      have h_l'_in_lines' : l' ∈ lines' := by
        simp_all [f, Finset.mem_image]
      <|> aesop
      have h_l'.1 : l'.1 = 1 := by
        simp [f]

```

```

have h1'2 : 1'2 = 1.2 - 1 := by
  simp [f]
have h_main_eq : 1'1 * (p.1 : ℝ) + 1'2 = (p.2 : ℝ) := by
  rw [h1'1, h1'2]
  linarith
exact Or.inl (1', h1'.in_lines', h_main_eq)
| inr h3.p'2 =>
  rcases h3.p'2 with (x, hx.in_vert, h_eq)
  have h_eq.p1 : p'.1 = p.1 := by
    simp [hp]
  have h_eq' : ∃ x ∈ verts, (p.1 : ℝ) = x := by
    refine' (x, hx.in_vert, _)
    linarith
  have h_main_eq : ∃ x ∈ verts', (p.1 : ℝ) = x := by
    simp [verts'] using h_eq'
  exact Or.inr h_main_eq
have h_card_filter : ((lines'.filter (fun l => 1.1 ≠ 0 ∧ 1.1 ≠ -1)).card =
  => k_local) := by
  rw [h_card_lines'] at *
  have h14 : (Finset.image f (lines.filter (fun l => 1.1 ≠ 0 ∧ 1.1 ≠
    => -1))).card = (lines.filter (fun l => 1.1 ≠ 0 ∧ 1.1 ≠ -1)).card := by
    apply Finset.card_image_of_injective
    exact h_inj.f
  have h15 : (Finset.image f (lines.filter (fun l => 1.1 ≠ 0 ∧ 1.1 ≠ -1))) =
    ((Finset.image f lines).filter (fun l => 1.1 ≠ 0 ∧ 1.1 ≠ -1)) := by
    apply Finset.ext
    intro x
    simp only [Finset.mem_image, Finset.mem_filter]
    constructor
    · rintro (y, hy, rfl)
      refine' (←, _)
      aesop
    · rintro (hx, hx')
      have h16 : ∃ y, y ∈ lines ∧ f y = x := by
        aesop
      rcases h16 with (y, hy, h17)
      refine' (y, _)
      aesop
  rw [← h15, h14]
  exact h4
exact H k_local verts' lines' h_card_sum h_cond_points h_card_filter

theorem translation_equivalence_y_axis (n k : ℕ) (hn : n > 3) :
  (∀ (k' : ℕ) (verts' : Finset ℝ) (lines' : Finset (ℝ × ℝ)),
    (verts'.card + lines'.card = n - 1) →
    (∀ p : ℕ × ℕ, p.1 ≥ 1 ∧ p.2 ≥ 1 ∧ p.1 + p.2 ≤ n →
      (∃ l ∈ lines', 1.1 * (p.1 : ℝ) + 1.2 = (p.2 : ℝ)) ∨ (∃ x ∈ verts', (p.1 : ℝ)
        => x) →
      ((lines'.filter (fun l => 1.1 ≠ 0 ∧ 1.1 ≠ -1)).card = k') →
      k' = 0 ∨ k' = 1 ∨ k' = 3) →
    (∀ (k : ℕ) (verts : Finset ℝ) (lines : Finset (ℝ × ℝ)) (points : Finset (ℕ × ℕ)
      => )),
      (verts.card + lines.card = n - 1) →
      (∀ p, p ∈ points => p.1 ≥ 1 ∧ p.2 ≥ 1 ∧ p.1 + p.2 ≤ n + 1) →
      (∀ p ∈ points, (∃ l ∈ lines, 1.1 * p.1 + 1.2 = p.2) ∨ (∃ x ∈ verts, p.1 =
        => x) →
      ((lines.filter (fun l => 1.1 ≠ 0 ∧ 1.1 ≠ -1)).card = k) →
      k = 0 ∨ k = 1 ∨ k = 3) := by
    intros
    apply translation_equivalence_y_axis_h_main
    <> assumption

theorem inductive_step_if_contains_horizontal_line_h_filter_card_eq_k (n k : ℕ)
  (verts : Finset ℝ)
  (lines : Finset (ℝ × ℝ))
  (points : Finset (ℕ × ℕ))
  (hk : (lines.filter (fun l => 1.1 ≠ 0 ∧ 1.1 ≠ -1)).card = k)
  (l : ℝ × ℝ)
  (hl.in_lines : l ∈ lines)
  (hl_1 : l.1 = 0)
  (h_filter_card : ((lines.erase l).filter (fun l => 1.1 ≠ 0 ∧ 1.1 ≠ -1)).card =
    => (lines.filter (fun l => 1.1 ≠ 0 ∧ 1.1 ≠ -1)).card :
  ((lines.erase l).filter (fun l => 1.1 ≠ 0 ∧ 1.1 ≠ -1)).card = k := by
  simp_all

theorem inductive_step_if_contains_horizontal_line_h_card_erase (n k : ℕ)
  (verts : Finset ℝ)
  (lines : Finset (ℝ × ℝ))
  (points : Finset (ℕ × ℕ))
  (l : ℝ × ℝ)
  (hl.in_lines : l ∈ lines)
  (lines.erase l).card = lines.card - 1 := by
  simp_all

theorem inductive_step_if_contains_horizontal_line_h_n_gt_3 (n k : ℕ)
  (verts : Finset ℝ)
  (lines : Finset (ℝ × ℝ))
  (points : Finset (ℕ × ℕ))
  (hn : n ≥ 4)
  n > 3 := by
  omega

theorem inductive_step_if_contains_horizontal_line_h_main (n k : ℕ)
  (verts : Finset ℝ)
  (lines : Finset (ℝ × ℝ))
  (points : Finset (ℕ × ℕ))
  (h_has_horizontal : ∃ l ∈ lines, 1.1 = 0 ∧ 1.2 = 1) :
  ∃ (l : ℝ × ℝ), l ∈ lines ∧ 1.1 = 0 ∧ 1.2 = 1 := by
  aesop

theorem inductive_step_if_contains_horizontal_line_h_translation_equivalence
  => (n k : ℕ)
  (verts : Finset ℝ)
  (lines : Finset (ℝ × ℝ))
  (points : Finset (ℕ × ℕ))
  (h_ih : ∀ (k' : ℕ) (verts' : Finset ℝ) (lines' : Finset (ℝ × ℝ)),
    (verts'.card + lines'.card = n - 1) →
    (∀ p : ℕ × ℕ, p.1 ≥ 1 ∧ p.2 ≥ 1 ∧ p.1 + p.2 ≤ n →
      (∃ l ∈ lines', 1.1 * (p.1 : ℝ) + 1.2 = (p.2 : ℝ)) ∨ (∃ x ∈ verts', (p.1 : ℝ)
        => x) →
      ((lines'.filter (fun l => 1.1 ≠ 0 ∧ 1.1 ≠ -1)).card = k') →
      k' = 0 ∨ k' = 1 ∨ k' = 3) →
    (hn : n ≥ 4)
  (h_n_gt_3 : n > 3) := by
  linarith

(h_n_gt_3 : n > 3) :
  (k' : ℕ) (verts' : Finset ℝ) (lines' : Finset (ℝ × ℝ)) (points' :
    => Finset (ℕ × ℕ))
  (verts : Finset ℝ)
  (lines : Finset (ℝ × ℝ))
  (points : Finset (ℕ × ℕ))
  (l : ℝ × ℝ)
  (hl_1 : 1.1 = 0)
  (hl.in_lines : l ∈ lines)
  (h_lines'.def : lines' = lines.erase l) :
  (∀ (x : ℝ × ℝ), x ∈ (lines'.filter (fun l => 1.1 ≠ 0 ∧ 1.1 ≠ -1)) => x ∈
    => (lines.filter (fun l => 1.1 ≠ 0 ∧ 1.1 ≠ -1)) := by
  aesop

theorem inductive_step_if_contains_horizontal_line_h_filter_eq_h_main (n k : ℕ)
  (verts : Finset ℝ)
  (lines : Finset (ℝ × ℝ))
  (points : Finset (ℕ × ℕ))
  (l : ℝ × ℝ)
  (hl_1 : 1.1 = 0)
  (hl.in_lines : l ∈ lines)
  (lines' : Finset (ℝ × ℝ))
  (h_lines'.def : lines' = lines.erase l) :
  (lines'.filter (fun l => 1.1 ≠ 0 ∧ 1.1 ≠ -1)).card = (lines.filter (fun l => 1.1 ≠
    => 0 ∧ 1.1 ≠ -1)) := by
  aesop

theorem inductive_step_if_contains_horizontal_line_h_filter_eq (n k : ℕ)
  (verts : Finset ℝ)
  (lines : Finset (ℝ × ℝ))
  (points : Finset (ℕ × ℕ))
  (l : ℝ × ℝ)
  (hl_1 : 1.1 = 0)
  (hl.in_lines : l ∈ lines)
  (lines' : Finset (ℝ × ℝ))
  (h_lines'.def : lines' = lines.erase l) :
  (lines'.filter (fun l => 1.1 ≠ 0 ∧ 1.1 ≠ -1)) = (lines.filter (fun l => 1.1 ≠
    => 0 ∧ 1.1 ≠ -1)) := by
  aesop

theorem inductive_step_if_contains_horizontal_line_h_main' (n k : ℕ)
  (verts : Finset ℝ)
  (lines : Finset (ℝ × ℝ))
  (points : Finset (ℕ × ℕ))
  (h_has_horizontal : ∃ l ∈ lines, 1.1 = 0 ∧ 1.2 = 1) :
  ∃ (l : ℝ × ℝ), l ∈ lines ∧ 1.1 = 0 ∧ 1.2 = 1 := by
  aesop

theorem inductive_step_if_contains_horizontal_line_h_card_erase' (n k : ℕ)
  (verts : Finset ℝ)
  (lines : Finset (ℝ × ℝ))
  (points : Finset (ℕ × ℕ))
  (l : ℝ × ℝ)
  (hl.in_lines : l ∈ lines)
  (lines.erase l).card = lines.card - 1 := by
  simp_all

theorem inductive_step_if_contains_horizontal_line_h_sum_card' (n k : ℕ)
  (verts : Finset ℝ)
  (lines : Finset (ℝ × ℝ))
  (points : Finset (ℕ × ℕ))
  (hcard : lines.card + verts.card = n)
  (l : ℝ × ℝ)
  (hl.in_lines : l ∈ lines)
  (hn : n ≥ 4) :
  verts.card + (lines.erase l).card = n - 1 := by
  apply inductive_step_if_contains_horizontal_line_h_sum_card
  <> assumption

theorem inductive_step_if_contains_horizontal_line_h_filter_card_eq_k' (n k : ℕ)
  =>
  (verts : Finset ℝ)
  (lines : Finset (ℝ × ℝ))
  (points : Finset (ℕ × ℕ))
  (hk : (lines.filter (fun l => 1.1 ≠ 0 ∧ 1.1 ≠ -1)).card = k)
  (l : ℝ × ℝ)
  (hl.in_lines : l ∈ lines)
  (hl_1 : 1.1 = 0)
  (h_filter_card : ((lines.erase l).filter (fun l => 1.1 ≠ 0 ∧ 1.1 ≠ -1)).card =
    => (lines.filter (fun l => 1.1 ≠ 0 ∧ 1.1 ≠ -1)).card :
  ((lines.erase l).filter (fun l => 1.1 ≠ 0 ∧ 1.1 ≠ -1)).card = k := by
  simp_all

theorem inductive_step_if_contains_horizontal_line_h_n_gt_3' (n k : ℕ)
  (verts : Finset ℝ)
  (lines : Finset (ℝ × ℝ))
  (points : Finset (ℕ × ℕ))
  (hn : n ≥ 4) :
  n > 3 := by
  linarith

theorem inductive_step_if_contains_horizontal_line_h_translation_equivalence'
  => (n k : ℕ)
  (verts : Finset ℝ)
  (lines : Finset (ℝ × ℝ))
  (points : Finset (ℕ × ℕ))
  (h_ih : ∀ (k' : ℕ) (verts' : Finset ℝ) (lines' : Finset (ℝ × ℝ)),
    (verts'.card + lines'.card = n - 1) →
    (∀ p : ℕ × ℕ, p.1 ≥ 1 ∧ p.2 ≥ 1 ∧ p.1 + p.2 ≤ n →
      (∃ l ∈ lines', 1.1 * (p.1 : ℝ) + 1.2 = (p.2 : ℝ)) ∨ (∃ x ∈ verts', (p.1 : ℝ)
        => x) →
      ((lines'.filter (fun l => 1.1 ≠ 0 ∧ 1.1 ≠ -1)).card = k') →
      k' = 0 ∨ k' = 1 ∨ k' = 3) →
    (hn : n ≥ 4)
  (h_n_gt_3 : n > 3) := by
  linarith

```



```

(h_n_gt_3 : n > 3):
  (k' : N) (verts' : Finset R) (lines' : Finset (R × R)) (points' :
    → Finset (N × N)), (verts'.card + lines'.card = n - 1) → (∀ p, p ∈
    → points' → p.1 ≥ 1 ∧ p.2 ≥ 2 ∧ p.1 + p.2 ≤ n + 1) → (∀ p ∈ points',
    → (∃ l ∈ lines', l.1 * p.1 + l.2 = p.2) ∨ (∃ x ∈ verts', p.1 = x)) →
    → ((lines'.filter (fun l ↦ l.1 ≠ 0 ∧ l.1 ≠ -1)).card = k') → k' = 0
    → ∨ k' = 1 ∨ k' = 3 := by
  exact inductive_step_if_contains_horizontal_line_h_translation_equivalence n
    → k verts lines points h_ih hn h_n_gt_3

theorem inductive_step_if_contains_horizontal_line_h_filter_eq' (n k : N)
  (verts : Finset R)
  (lines : Finset (R × R))
  (points : Finset (N × N))
  (l : R × R)
  (hl1 : l.1 = 0)
  (hl_in_lines : l ∈ lines)
  (lines' : Finset (R × R))
  (h_lines'_def : lines' = lines.erase l):
  (lines'.filter (fun l ↦ l.1 ≠ 0 ∧ l.1 ≠ -1)) = (lines.filter (fun l ↦ l.1 ≠
    → 0 ∧ l.1 ≠ -1)) := by
  aesop

theorem inductive_step_if_contains_horizontal_line_h_main_1 (n k : N)
  (verts : Finset R)
  (lines : Finset (R × R))
  (points : Finset (N × N))
  (h_has_horizontal : ∃ l ∈ lines, l.1 = 0 ∧ l.2 = 1):
  (l : R × R), l ∈ lines ∧ l.1 = 0 ∧ l.2 = 1 := by
  aesop

theorem inductive_step_if_contains_horizontal_line_h_card_erase_1 (n k : N)
  (verts : Finset R)
  (lines : Finset (R × R))
  (points : Finset (N × N))
  (l : R × R)
  (hl_in_lines : l ∈ lines):
  (lines.erase l).card = lines.card - 1 := by
  simp_all

theorem inductive_step_if_contains_horizontal_line_h_sum_card_1 (n k : N)
  (verts : Finset R)
  (lines : Finset (R × R))
  (points : Finset (N × N))
  (hcard : lines.card + verts.card = n)
  (l : R × R)
  (hl_in_lines : l ∈ lines)
  (hn : n ≥ 4):
  verts.card + (lines.erase l).card = n - 1 := by
  apply inductive_step_if_contains_horizontal_line_h_sum_card'
  assumption'

theorem inductive_step_if_contains_horizontal_line_h_filter_card_eq_k_1 (n k :
  → N)
  (verts : Finset R)
  (lines : Finset (R × R))
  (points : Finset (N × N))
  (hk : (lines.filter (fun l ↦ l.1 ≠ 0 ∧ l.1 ≠ -1)).card = k)
  (l : R × R)
  (hl_in_lines : l ∈ lines)
  (hl_1 : l.1 = 0)
  (h_filter_card : ((lines.erase l).filter (fun l ↦ l.1 ≠ 0 ∧ l.1 ≠ -1)).card =
    → (lines.filter (fun l ↦ l.1 ≠ 0 ∧ l.1 ≠ -1)).card):
  ((lines.erase l).filter (fun l ↦ l.1 ≠ 0 ∧ l.1 ≠ -1)).card = k := by
  simp_all

theorem inductive_step_if_contains_horizontal_line_h_n_gt_3_1 (n k : N)
  (verts : Finset R)
  (lines : Finset (R × R))
  (points : Finset (N × N))
  (hn : n ≥ 4):
  n > 3 := by
  linarith

theorem inductive_step_if_contains_horizontal_line_h_translation_equivalence_1
  → (n k : N)
  (verts : Finset R)
  (lines : Finset (R × R))
  (points : Finset (N × N))
  (h_ih : ∨ (k' : N) (verts' : Finset R) (lines' : Finset (R × R)),
    (verts'.card + lines'.card = n - 1) →
    (∀ p : N × N, p.1 ≥ 1 ∧ p.2 ≥ 1 ∧ p.1 + p.2 ≤ n + 1) →
    (∃ l ∈ lines', l.1 * (p.1 : R) + l.2 = (p.2 : R)) ∨ (∃ x ∈ verts', (p.1 : R)
    → ) = x)) →
    ((lines'.filter (fun l ↦ l.1 ≠ 0 ∧ l.1 ≠ -1)).card = k') →
    k' = 0 ∨ k' = 1 ∨ k' = 3)
  (hn : n ≥ 4)
  (h_n_gt_3 : n > 3):
  (k' : N) (verts' : Finset R) (lines' : Finset (R × R)) (points' :
    → Finset (N × N)), (verts'.card + lines'.card = n - 1) → (∀ p, p ∈
    → points' → p.1 ≥ 1 ∧ p.2 ≥ 2 ∧ p.1 + p.2 ≤ n + 1) → (∀ p ∈ points',
    → (∃ l ∈ lines', l.1 * p.1 + l.2 = p.2) ∨ (∃ x ∈ verts', p.1 = x)) →
    → ((lines'.filter (fun l ↦ l.1 ≠ 0 ∧ l.1 ≠ -1)).card = k') → k' = 0
    → ∨ k' = 1 ∨ k' = 3 := by
  apply inductive_step_if_contains_horizontal_line_h_translation_equivalence'
  <,> assumption

theorem inductive_step_if_contains_horizontal_line_h_filter_eq_1 (n k : N)
  (verts : Finset R)
  (lines : Finset (R × R))
  (points : Finset (N × N))
  (l : R × R)
  (hl1 : l.1 = 0)
  (hl_in_lines : l ∈ lines)
  (lines' : Finset (R × R))
  (h_lines'_def : lines' = lines.erase l):
  (lines'.filter (fun l ↦ l.1 ≠ 0 ∧ l.1 ≠ -1)) = (lines.filter (fun l ↦ l.1 ≠
    → 0 ∧ l.1 ≠ -1)) := by
  aesop

theorem inductive_step_if_contains_horizontal_line (n k : N) (verts : Finset R
  → ) (lines : Finset (R × R)) (points : Finset (N × N)) (hcard :
  → lines.card + verts.card = n) (hallpoints : ∨ p, p ∈ points → p.1 ≥ 1 ∧
    → p.2 ≥ 1 ∧ p.1 + p.2 ≤ n + 1) (hmain : ∨ p ∈ points, (∃ l ∈ lines, l.1
    → * p.1 + l.2 = p.2) ∨ (∃ x ∈ verts, p.1 = x)) (hk : (lines.filter (fun
    → l ↦ l.1 ≠ 0 ∧ l.1 ≠ -1)).card = k) (hn : n ≥ 4) (hcover : ∨ p : N × N
    → , p.1 ≥ 1 ∧ p.2 ≥ 1 ∧ p.1 + p.2 ≤ n + 1)
  (∃ l ∈ lines, l.1 * (p.1 : R) + l.2 = (p.2 : R)) ∨ (∃ x ∈ verts, (p.1 : R) =
    → x)) (h_has_horizontal : ∃ l ∈ lines, l.1 = 0 ∧ l.2 = 1) (h_ih : ∨ (k' :
    → N) (verts' : Finset R) (lines' : Finset (R × R)),
    (verts'.card + lines'.card = n - 1) →
    (∀ p : N × N, p.1 ≥ 1 ∧ p.2 ≥ 1 ∧ p.1 + p.2 ≤ n + 1) →
    (∃ l ∈ lines', l.1 * (p.1 : R) + l.2 = (p.2 : R)) ∨ (∃ x ∈ verts', (p.1 : R)
    → ) = x)) →
    ((lines'.filter (fun l ↦ l.1 ≠ 0 ∧ l.1 ≠ -1)).card = k') →
    k' = 0 ∨ k' = 1 ∨ k' = 3) := by
  have h_main : (l : R × R), l ∈ lines ∧ l.1 = 0 ∧ l.2 = 1 := by
  exact inductive_step_if_contains_horizontal_line_h_main_1 n k verts
    → points h_has_horizontal
  obtain (l, hl_in_lines, hl_1, hl_2) := h_main
  have h_card_erase : (lines.erase l).card = lines.card - 1 := by
  exact inductive_step_if_contains_horizontal_line_h_card_erase_1 n k verts
    → lines points l hl_in_lines
  have h_sum_card : verts.card + (lines.erase l).card = n - 1 := by
  exact inductive_step_if_contains_horizontal_line_h_sum_card_1 n k verts
    → lines points hcard l hl_in_lines hn
  have h_n_gt_3 : n > 3 := by
  exact inductive_step_if_contains_horizontal_line_h_n_gt_3_1 n k verts
    → lines points hn
  have h_translation_equivalence : ∨ (k' : N) (verts' : Finset R) (lines' :
    → Finset (R × R)) (points' : Finset (N × N)), (verts'.card +
    → lines'.card = n - 1) → (∀ p, p ∈ points' → p.1 ≥ 1 ∧ p.2 ≥ 2 ∧ p.1 +
    → p.2 ≤ n + 1) → (∃ p ∈ points', (∃ l ∈ lines', l.1 * p.1 + l.2 =
    → p.2) ∨ (∃ x ∈ verts', p.1 = x)) → ((lines'.filter (fun l ↦ l.1 ≠ 0 ∧
    → l.1 ≠ -1)).card = k') → k' = 0 ∨ k' = 1 ∨ k' = 3 := by
  exact
    → inductive_step_if_contains_horizontal_line_h_translation_equivalence_1
    → n k verts lines points h_ih hn h_n_gt_3
  set lines' := lines.erase l with h_lines'_def
  set verts' := verts with h_verts'_def
  have h_filter_eq : (lines'.filter (fun l ↦ l.1 ≠ 0 ∧ l.1 ≠ -1)) =
    → (lines.filter (fun l ↦ l.1 ≠ 0 ∧ l.1 ≠ -1)) := by
  exact inductive_step_if_contains_horizontal_line_h_filter_eq_1 n k verts
    → lines points l hl_1 hl_in_lines lines' h_lines'_def
  have h_filter_card : ((lines.erase l).filter (fun l ↦ l.1 ≠ 0 ∧ l.1 ≠
    → -1)).card = (lines.filter (fun l ↦ l.1 ≠ 0 ∧ l.1 ≠ -1)).card := by
  have h1 : (lines'.filter (fun l ↦ l.1 ≠ 0 ∧ l.1 ≠ -1)) = (lines.filter
    → (fun l ↦ l.1 ≠ 0 ∧ l.1 ≠ -1)) := h_filter_eq
  have h2 : lines' = lines.erase l := by simp using h_lines'_def
  rw [h2] at h1
  exact congr_arg Finset.card h1
  have h_filter_card_eq_k : ((lines.erase l).filter (fun l ↦ l.1 ≠ 0 ∧ l.1 ≠
    → -1)).card = k := by
  exact inductive_step_if_contains_horizontal_line_h_filter_card_eq_k_1 n k
    → verts lines points hk l hl_in_lines hl_1 h_filter_card
  have h1 : verts'.card + lines'.card = n - 1 := by
  simp [h_lines'_def, h_verts'_def] using h_sum_card
  set points' : Finset (N × N) := (Finset.Icc 1 n × Finset.Icc 2 (n +
    → 1)).filter (fun p : N × N => p.1 ≥ 1 ∧ p.2 ≥ 2 ∧ p.1 + p.2 ≤ n + 1)
    → with h_points'_def
  have h2 : ∨ p : N × N, p ∈ points' → p.1 ≥ 1 ∧ p.2 ≥ 2 ∧ p.1 + p.2 ≤ n + 1 :=
    by
  intro p
  constructor
  · -- Prove the forward direction: if p ∈ points', then p.1 ≥ 1 ∧ p.2 ≥ 2 ∧
    → p.1 + p.2 ≤ n + 1
  intro hp
  simp only [h_points'_def, Finset.mem_filter, Finset.mem_product,
    → Finset.mem_Icc] at hp
  tauto
  · -- Prove the reverse direction: if p.1 ≥ 1 ∧ p.2 ≥ 2 ∧ p.1 + p.2 ≤ n + 1,
    → then p ∈ points'
  rintro (h1, h2, h3)
  simp only [h_points'_def, Finset.mem_filter, Finset.mem_product,
    → Finset.mem_Icc]
  constructor
  · constructor <,> omega
  · exact (h1, h2, h3)
  have h3 : ∨ p ∈ points', (∃ l ∈ lines', l.1 * p.1 + l.2 = p.2) ∨ (∃ x ∈
    → verts', p.1 = x) := by
  intro p hp
  have h3 : p.1 ≥ 1 ∧ p.2 ≥ 2 ∧ p.1 + p.2 ≤ n + 1 := (h2 p).mp hp
  have h3 : p.1 ≥ 1 := h3.1
  have h3 : p.2 ≥ 2 := h3.2.1
  have h3 : p.1 + p.2 ≤ n + 1 := h3.2.2
  have h3 : p.2 ≥ 1 := by linarith
  have h3 : p.1 ≥ 1 ∧ p.2 ≥ 1 ∧ p.1 + p.2 ≤ n + 1 := {h3, h3, h3}
  have h3 : (∃ l ∈ lines, l.1 * (p.1 : R) + l.2 = (p.2 : R)) ∨ (∃ x ∈ verts,
    → (p.1 : R) = x) := hcover p h3
  cases h3 with
  | inl h3 =>
  | rcases h3 with (l, hl_in_lines, hl_eq)
  by_cases h3 : l = l_0
  · -- Case l = l_0
  have h3 : l = l_0 := h3
  have h3 : l.1 = l_0.1 := by rw [h3.1]
  have h3 : l.2 = l_0.2 := by rw [h3.1]
  have h3 : l.1 = 0 := by
  rw [h3, hl_1]
  have h3 : l.2 = 1 := by
  rw [h3, hl_2]
  have h3 : (l.1 : R) * (p.1 : R) + l.2 = (p.2 : R) := by simp using
    → hl_eq
  rw [h3, h3] at h3
  have h3 : (0 : R) * (p.1 : R) + (1 : R) = (p.2 : R) := h3
  have h3 : (1 : R) = (p.2 : R) := by linarith

```

```

have h3, : (p.2 : R) = 1 := by linarith
have h3, : p.2 = 1 := by exact_mod_cast h3,
linarith
-- Case 2 ≠ L
have h3, : 1 ≠ L, := h3
have h3, : 1 ∈ lines' := by
  have h3, : 1 ∈ lines := hl_in_lines
  have h3, : 1 ≠ L, := h3
  have h3, : 1 ∈ lines.erase L, := Finset.mem_erase.mpr h3, h3,
  simp [h_lines'.def] using h3,
have h3, : 1 ∈ lines', 1.1 * p.1 + 1.2 = p.2 := by
  refine' 1, h3,
  simp using hl_eq
exact Or.inl h3,
| inr h3, =>
  have h3, : ∃ x ∈ verts, (p.1 : R) = x := h3
  have h3, : ∃ x ∈ verts', p.1 = x := by
    rcases h3 with (x, hx_in_verts, hx_eq)
    refine' 1, h3,
    constructor
    · simp [h_verts'.def] using hx_in_verts
    · linarith
  exact Or.inr h3,

have h4 : ((lines'.filter (fun l => 1.1 ≠ 0 ∧ 1.1 ≠ -1)).card) = k := by
  => simp [h_lines'.def] using h_filter_card_eq_k

have h5 : k = 0 ∨ k = 1 ∨ k = 3 := by
  specialize h_translation_equivalence k verts' lines' points' h1 h2 h3 h4
  simp using h_translation_equivalence
exact h5

theorem translation_equivalence_x_axis_h6 (n k : N)
  (verts : Finset R)
  (lines : Finset (R × R))
  (points : Finset (N × N))
  (hn : n > 3)
  (h : verts.card + lines.card = n - 1)
  (h : ∃ p, p ∈ points => p.1 ≥ 2 ∧ p.2 ≥ 1 ∧ p.1 + p.2 ≤ n + 1)
  (h : ∃ p ∈ points, (∃ l ∈ lines, 1.1 * p.1 + 1.2 = p.2) ∨ (∃ x ∈ verts, p.1 =
    → x))
  (h : (lines.filter (fun l => 1.1 ≠ 0 ∧ 1.1 ≠ -1)).card = k) :
  ∃ (p : N × N), p.1 ≥ 1 ∧ p.2 ≥ 1 ∧ p.1 + p.2 ≤ n => (∃ l ∈ (lines.image (fun l
    => (1.1, 1.1 + 1.2))), 1.1 * (p.1 : R) + 1.2 = (p.2 : R)) ∨ (∃ x ∈
    → (verts.image (fun x => x - 1)), (p.1 : R) = x) := by
  intro p hp
  obtain (l, hl, hl') | (x, hx, hx') := h (p.1 + 1, p.2) (by
    simp_all
    omega)
  exact Or.inl (
    , Finset.mem_image.mpr (l, hl, rfl)
    , by
      simp_all
      linarith
  )
  exact Or.inr (
    , Finset.mem_image.mpr (x, hx, rfl)
    , by
      simp_all
      linarith
  )
)

theorem translation_equivalence_x_axis_h8 (n k : N)
  (verts : Finset R)
  (lines : Finset (R × R))
  (hn : n > 3)
  (h : verts.card + lines.card = n - 1)
  (h : (lines.filter (fun l => 1.1 ≠ 0 ∧ 1.1 ≠ -1)).card = k)
  (h7 : (( (lines.image (fun l => (1.1, 1.1 + 1.2))))).filter (fun l => 1.1 ≠ 0 ∧
    → 1.1 ≠ -1)).card = (lines.filter (fun l => 1.1 ≠ 0 ∧ 1.1 ≠ -1)).card) :
  (( (lines.image (fun l => (1.1, 1.1 + 1.2))))).filter (fun l => 1.1 ≠ 0 ∧ 1.1 ≠
    → -1)).card = k := by
  linarith

theorem translation_equivalence_x_axis_h5 (n k : N)
  (verts : Finset R)
  (lines : Finset (R × R))
  (hn : n > 3)
  (h : verts.card + lines.card = n - 1) :
  ( (verts.image (fun x => x - 1)).card + ( (lines.image (fun l => (1.1, 1.1
    → + 1.2))))).card = n - 1 := by
  simp_all [Finset.card_image_of_injective, Function.Injective]

theorem translation_equivalence_x_axis_main_proof (n k : N) (hn : n > 3)
  (h : ∃ (k' : N) (verts' : Finset R) (lines' : Finset (R × R)),
    (verts'.card + lines'.card = n - 1) →
    (∃ p : N × N, p.1 ≥ 1 ∧ p.2 ≥ 1 ∧ p.1 + p.2 ≤ n →
      (∃ l ∈ lines', 1.1 * (p.1 : R) + 1.2 = (p.2 : R)) ∨ (∃ x ∈ verts', (p.1 : R
        → x) →
        (lines'.filter (fun l => 1.1 ≠ 0 ∧ 1.1 ≠ -1)).card = k') →
        k' = 0 ∨ k' = 1 ∨ k' = 3)
    (k' : N) (verts' : Finset R) (lines' : Finset (R × R))
    (h : verts'.card + lines'.card = n - 1)
    (h : ∃ p : N × N, p.1 ≥ 1 ∧ p.2 ≥ 1 ∧ p.1 + p.2 ≤ n →
      (∃ l ∈ lines', 1.1 * (p.1 : R) + 1.2 = (p.2 : R)) ∨ (∃ x ∈ verts', (p.1 : R
        → x) →
        (lines'.filter (fun l => 1.1 ≠ 0 ∧ 1.1 ≠ -1)).card = k')
    (h : k' = k) :
    k = 0 ∨ k = 1 ∨ k = 3 := by
  simp_all
  apply h
  all_goals assumption

theorem translation_equivalence_x_axis_h7 (n k : N)
  (verts : Finset R)
  (lines : Finset (R × R))
  (hn : n > 3)
  (h : verts.card + lines.card = n - 1)
  (h : (lines.filter (fun l => 1.1 ≠ 0 ∧ 1.1 ≠ -1)).card = k) :
  (( (lines.image (fun l => (1.1, 1.1 + 1.2))))).filter (fun l => 1.1 ≠ 0 ∧ 1.1 ≠
    → -1)).card = (lines.filter (fun l => 1.1 ≠ 0 ∧ 1.1 ≠ -1)).card := by
  simp_all [Finset.filter_image, Finset.card_image_of_injective,
    → Function.Injective]

theorem translation_equivalence_x_axis (n k : N) (hn : n > 3) :
  (∃ (k' : N) (verts' : Finset R) (lines' : Finset (R × R)),
    (verts'.card + lines'.card = n - 1) →
    (∃ p : N × N, p.1 ≥ 1 ∧ p.2 ≥ 1 ∧ p.1 + p.2 ≤ n →
      (∃ l ∈ lines', 1.1 * (p.1 : R) + 1.2 = (p.2 : R)) ∨ (∃ x ∈ verts', (p.1 : R
        → x) →
        (lines'.filter (fun l => 1.1 ≠ 0 ∧ 1.1 ≠ -1)).card = k') →
        k' = 0 ∨ k' = 1 ∨ k' = 3)
    (k' : N) (verts' : Finset R) (lines' : Finset (R × R))
    (h : verts'.card + lines'.card = n - 1)
    (h : ∃ p : N × N, p.1 ≥ 1 ∧ p.2 ≥ 1 ∧ p.1 + p.2 ≤ n →
      (∃ l ∈ lines', 1.1 * (p.1 : R) + 1.2 = (p.2 : R)) ∨ (∃ x ∈ verts', (p.1 : R
        → x) →
        (lines'.filter (fun l => 1.1 ≠ 0 ∧ 1.1 ≠ -1)).card = k')
    (h : k' = k) :
    k = 0 ∨ k = 1 ∨ k = 3 := by
  simp_all
  apply h
  all_goals assumption

theorem inductive_step_if_contains_vertical_line_round1_h1 (n k : N)
  (verts : Finset R)
  (lines : Finset (R × R))
  (points : Finset (N × N))
  (h1_in_verts : (1 : R) ∈ verts) :
  (verts.card ≥ 1 := by
  by_contra
  simp_all

theorem round1_h_verts_card_ge_one (n k : N)
  (verts : Finset R)
  (lines : Finset (R × R))
  (points : Finset (N × N))
  (h1_in_verts : (1 : R) ∈ verts) :
  (verts.card ≥ 1 := by
  by_contra
  simp_all

theorem round1_h_erase_card (n k : N)
  (verts : Finset R)
  (lines : Finset (R × R))
  (points : Finset (N × N))
  (h1_in_verts : (1 : R) ∈ verts) :
  (verts.erase (1 : R)).card = verts.card - 1 := by
  simp_all

theorem round1_h_main_card (n k : N)
  (verts : Finset R)
  (lines : Finset (R × R))
  (points : Finset (N × N))
  (hcard : lines.card + verts.card = n)
  (h1_in_verts : (1 : R) ∈ verts)
  (h_verts_card_ge_one : verts.card ≥ 1)
  (h_erase_card : (verts.erase (1 : R)).card = verts.card - 1) :
  (verts.erase (1 : R)).card + lines.card + 1 = n := by
  omega

theorem round1_h14 (n k : N)
  (verts : Finset R)
  (lines : Finset (R × R))
  (points : Finset (N × N))
  (hn : n ≥ 4)
  (hcard : lines.card + verts.card = n)
  (h1_in_verts : (1 : R) ∈ verts)
  (h_verts_card_ge_one : verts.card ≥ 1)
  (h_erase_card : (verts.erase (1 : R)).card = verts.card - 1)
  (h_main_card : (verts.erase (1 : R)).card + lines.card + 1 = n) :
  (verts.erase (1 : R)).card + lines.card = n - 1 := by
  omega

theorem inductive_step_if_contains_vertical_line (n k : N) (verts : Finset R)
  → (lines : Finset (R × R)) (points : Finset (N × N)) (hcard :
  → lines.card + verts.card = n) (hallpoints : ∃ p, p ∈ points → p.1 ≥ 1 ∧
  → p.2 ≥ 1 ∧ p.1 + p.2 ≤ n + 1) (hmain : ∃ p ∈ points, (∃ l ∈ lines, 1.1
  → * p.1 + 1.2 = p.2) ∨ (∃ x ∈ verts, p.1 = x)) (hk : (lines.filter (fun
  → l => 1.1 ≠ 0 ∧ 1.1 ≠ -1)).card = k) (hn : n ≥ 4) (hcover : ∃ p : N × N
  → , p.1 ≥ 1 ∧ p.2 ≥ 1 ∧ p.1 + p.2 ≤ n + 1 →
  (∃ l ∈ lines, 1.1 * (p.1 : R) + 1.2 = (p.2 : R)) ∨ (∃ x ∈ verts, (p.1 : R) =
  → x)) (h_has_vert : ∃ x ∈ verts, x = 1) (h_ih : ∃ (k' : N) (verts' :
  → Finset R) (lines' : Finset (R × R)),
  (verts'.card + lines'.card = n - 1) →
  (∃ p : N × N, p.1 ≥ 1 ∧ p.2 ≥ 1 ∧ p.1 + p.2 ≤ n →
  (∃ l ∈ lines', 1.1 * (p.1 : R) + 1.2 = (p.2 : R)) ∨ (∃ x ∈ verts', (p.1 : R
  → x) →
  (lines'.filter (fun l => 1.1 ≠ 0 ∧ 1.1 ≠ -1)).card = k') →
  k' = 0 ∨ k' = 1 ∨ k' = 3) : k = 0 ∨ k = 1 ∨ k = 3 := by
have h5 := inductive_step_if_contains_vertical_line_round1_h1 n k verts
  → lines points h_has_vert
have h6 := round1_h_verts_card_ge_one n k verts lines points h5
have h7 := round1_h_erase_card n k verts lines points h5
have h8 := round1_h_main_card n k verts lines points hcard h5 h6 h7 h8
set points' : Finset (N × N) := ((Finset.Icc 2 (n + 1)) × (Finset.Icc 1 (n +
  → 1))).filter (fun p : N × N => p.1 + p.2 ≤ n + 1) with hpoints'.def
have h11 : ∃ (p : N × N), p ∈ points' → p.1 ≥ 2 ∧ p.2 ≥ 1 ∧ p.1 + p.2 ≤ n + 1
  → := by
  simp [hpoints'.def, Finset.mem_filter, Finset.mem_product, Finset.mem_Icc]
  <> omega
have h12 : ∃ p ∈ points', (∃ l ∈ lines, 1.1 * p.1 + 1.2 = p.2) ∨ (∃ x ∈
  → (verts.erase (1 : R)), p.1 = x) := by
  intro p hp
  have h13 := (h11 p).mp hp
  have h14 := hcover p by omega, by omega, by omega
  cases h14 with
  | inl h14_left =>
    left
    exact h14_left
  | inr h14_right =>
    rcases h14_right with (x, hx_in_verts, h_eq)
    have h15 : x ≠ (1 : R) := by
      by_contra h151

```



```

have h152 : (p.1 :  $\kappa$ ) = 1 := by linarith
have h153 : p.1  $\geq$  2 := h13.1
have h154 : (p.1 :  $\kappa$ )  $\geq$  2 := by exact_mod_cast h153
linarith
have hx_in_verts_erase : x  $\in$  verts.erase (1 :  $\kappa$ ) := by
  exact Finset.mem_erase.mpr h15, hx_in_verts
right
refine (x, hx_in_verts_erase, ?)
norm_cast at h_eq
exact translation_equivalence_x_axis n k (by linarith) h_ih k (verts.erase
  (1 :  $\kappa$ )) lines points' h9 h11 h12 hk

theorem inductive_step_if_contains_rainy_diagonal_line_refined_main_proof (n k
   $\rightarrow$  :  $\kappa$ ) (verts : Finset  $\kappa$ ) (lines : Finset ( $\kappa \times \kappa$ )) (points : Finset ( $\kappa \times$ 
   $\rightarrow$  :  $\kappa$ )) (hml :  $3 \leq n$ ) (hcard : lines.card + verts.card = n) (hallpoints
   $\rightarrow$  :  $\forall p, p \in \text{points} \rightarrow p.1 \geq 1 \wedge p.2 \geq 1 \wedge p.1 + p.2 \leq n + 1$ ) (hmain :  $\forall$ 
   $\rightarrow$  :  $p \in \text{points}, (\exists l \in \text{lines}, l.1 * p.1 + l.2 = p.2) \vee (\exists x \in \text{verts}, p.1 =$ 
   $\rightarrow$  :  $x)$ ) (hk : (lines.filter (fun l  $\rightarrow$  l.1  $\neq$  0  $\wedge$  l.1  $\neq$  -1)).card = k)
   $\rightarrow$  : (hcover :  $\forall p : \kappa \times \kappa, p.1 \geq 1 \wedge p.2 \geq 1 \wedge p.1 + p.2 \leq n + 1 \rightarrow$ 
   $(\exists l \in \text{lines}, l.1 * (p.1 : \kappa) + l.2 = (p.2 : \kappa)) \vee (\exists x \in \text{verts}, (p.1 : \kappa) =$ 
   $\rightarrow$  :  $x)$ ) (h_has_rainy_diagonal :  $\exists l \in \text{lines}, l.1 = -1 \wedge l.2 = (n : \kappa) +$ 
   $\rightarrow$  : 1) (h_ih :  $\forall (k' : \kappa) (\text{verts}' : \text{Finset } \kappa) (\text{lines}' : \text{Finset } (\kappa \times \kappa)),$ 
  (verts'.card + lines'.card = n - 1)  $\rightarrow$ 
  ( $\forall p : \kappa \times \kappa, p.1 \geq 1 \wedge p.2 \geq 1 \wedge p.1 + p.2 \leq n \rightarrow$ 
  ( $\exists l \in \text{lines}', l.1 * (p.1 : \kappa) + l.2 = (p.2 : \kappa)) \vee (\exists x \in \text{verts}', (p.1 : \kappa)$ 
   $\rightarrow$  :  $x)$ )  $\rightarrow$ 
  ((lines'.filter (fun l  $\rightarrow$  l.1  $\neq$  0  $\wedge$  l.1  $\neq$  -1)).card = k')  $\rightarrow$ 
  k' = 0  $\vee$  k' = 1  $\vee$  k' = 3) : k = 0  $\vee$  k = 1  $\vee$  k = 3 := by
obtain l0, h10_in_lines, h101, h102 := h_has_rainy_diagonal
have h13 : ((lines.erase 10).filter (fun l  $\rightarrow$  l.1  $\neq$  0  $\wedge$  l.1  $\neq$  -1)).card = k :=
  by
  rw [← hk]
  congr 1
  ext x
  simp [Finset.mem_filter, Finset.mem_erase]
  aesop
have h11 : verts.card + (lines.erase 10).card = n - 1 := by
  rw [Finset.card_erase_of_mem h10_in_lines]
  have h111 : lines.card  $\geq$  1 := by
    apply Finset.card_pos.mpr
    exact l0, h10_in_lines
  omega
have h12 :  $\forall p : \kappa \times \kappa, p.1 \geq 1 \wedge p.2 \geq 1 \wedge p.1 + p.2 \leq n \rightarrow (\exists l \in$ 
   $\rightarrow$  : lines.erase 10, l.1 * (p.1 :  $\kappa$ ) + l.2 = (p.2 :  $\kappa$ ))  $\vee (\exists x \in \text{verts},$ 
   $\rightarrow$  : (p.1 :  $\kappa$ ) = x) := by
  intro p hp
  rcases hcover p (hp.1, hp.2.1, by linarith) with (h126 | h126)
  rcases h126 with l, hl_in_lines, h_eq
  have h1261 : l.1 = 10 := by
    by_contra h12611
    have h12612 : l.1 = 10 := by tauto
    have h1263 : l.1 = -1 := by
      rw [h12612]
      linarith
    have h1264 : l.2 = (n :  $\kappa$ ) + 1 := by
      rw [h12612]
      linarith
    have h1265 : (n :  $\kappa$ ) + 1 = (p.1 :  $\kappa$ ) + (p.2 :  $\kappa$ ) := by
      rw [h1263, h1264] at h_eq
      ring_nf at h_eq
      linarith
    have h1266 : (p.1 :  $\kappa$ ) + (p.2 :  $\kappa$ )  $\leq$  (n :  $\kappa$ ) := by exact_mod_cast hp.2.2
    linarith
  have h1267 : l  $\in$  lines.erase 10 := by
    exact Finset.mem_erase_of_ne_of_mem h1261 hl_in_lines
  apply Or.inl
  exact l, h1267, h_eq
  rcases h126 with x, hx_in_verts, h126_eq
  apply Or.inr
  exact x, hx_in_verts, h126_eq
  apply h_ih <> assumption

theorem inductive_step_if_contains_rainy_diagonal_line_refined (n k :  $\kappa$ )
   $\rightarrow$  : (verts : Finset  $\kappa$ ) (lines : Finset ( $\kappa \times \kappa$ )) (points : Finset ( $\kappa \times$ 
   $\rightarrow$  :  $\kappa$ )) (hml :  $3 \leq n$ ) (hcard : lines.card + verts.card = n) (hallpoints :  $\forall p,$ 
   $\rightarrow$  :  $p \in \text{points} \rightarrow p.1 \geq 1 \wedge p.2 \geq 1 \wedge p.1 + p.2 \leq n + 1$ ) (hmain :  $\forall p \in$ 
   $\rightarrow$  : points, ( $\exists l \in \text{lines}, l.1 * p.1 + l.2 = p.2$ )  $\vee (\exists x \in \text{verts}, p.1 = x)$ )
   $\rightarrow$  : (hk : (lines.filter (fun l  $\rightarrow$  l.1  $\neq$  0  $\wedge$  l.1  $\neq$  -1)).card = k) (hn : n  $\geq$ 
   $\rightarrow$  : 4) (hcover :  $\forall p : \kappa \times \kappa, p.1 \geq 1 \wedge p.2 \geq 1 \wedge p.1 + p.2 \leq n + 1 \rightarrow$ 
   $(\exists l \in \text{lines}, l.1 * (p.1 : \kappa) + l.2 = (p.2 : \kappa)) \vee (\exists x \in \text{verts}, (p.1 : \kappa) =$ 
   $\rightarrow$  :  $x)$ ) (h_has_rainy_diagonal :  $\exists l \in \text{lines}, l.1 = -1 \wedge l.2 = (n : \kappa) +$ 
   $\rightarrow$  : 1) (h_ih :  $\forall (k' : \kappa) (\text{verts}' : \text{Finset } \kappa) (\text{lines}' : \text{Finset } (\kappa \times \kappa)),$ 
  (verts'.card + lines'.card = n - 1)  $\rightarrow$ 
  ( $\forall p : \kappa \times \kappa, p.1 \geq 1 \wedge p.2 \geq 1 \wedge p.1 + p.2 \leq n \rightarrow$ 
  ( $\exists l \in \text{lines}', l.1 * (p.1 : \kappa) + l.2 = (p.2 : \kappa)) \vee (\exists x \in \text{verts}', (p.1 : \kappa)$ 
   $\rightarrow$  :  $x)$ )  $\rightarrow$ 
  ((lines'.filter (fun l  $\rightarrow$  l.1  $\neq$  0  $\wedge$  l.1  $\neq$  -1)).card = k')  $\rightarrow$ 
  k' = 0  $\vee$  k' = 1  $\vee$  k' = 3) : k = 0  $\vee$  k = 1  $\vee$  k = 3 := by
  apply inductive_step_if_contains_rainy_diagonal_line_refined_main_proof
  all_goals assumption

theorem num_points_on_boundary_main (n :  $\kappa$ ) (hpoints : Finset ( $\kappa \times \kappa$ ))
   $\rightarrow$  : (hpoints_def :  $\forall p, p \in \text{hpoints} \rightarrow p.1 \geq 1 \wedge p.2 \geq 1 \wedge p.1 + p.2 \leq n +$ 
   $\rightarrow$  : 1) : (Finset.filter (fun p  $\rightarrow$  p.1 = 1  $\vee$  p.2 = 1  $\vee$  p.1 + p.2 = n + 1)
   $\rightarrow$  : hpoints).card = 3 * n - (if n = 1 then 2 else if n = 2 then 3 else
   $\rightarrow$  : 3) := by
  by_cases h0 : n = 0
  have h2 : hpoints =  $\emptyset$  := by
    apply Finset.eq_empty_of_forall_not_mem
    intro p
    intro h4
    have h5 := (hpoints_def p).mpr h4
    simp [h0] at h5
    <> omega
    simp [h2, h0]
  by_cases h1 : n = 1
  have h4 : hpoints = {(1, 1)} := by
    ext x, y
    simp [hpoints_def, h1]
    <> omega
    rw [h4, h1]
    <> aesop
  by_cases h2 : n = 2
  have h4 : hpoints = {(1, 1), (1, 2), (2, 1)} := by
    ext x, y
    simp [hpoints_def, h2]
    <> omega
    rw [h4, h2]
    <> aesop
  set A : Finset ( $\kappa \times \kappa$ ) := Finset.image (fun y  $\rightarrow$  (1, y)) (Finset.Icc 1
   $\rightarrow$  : n) with hA
  set B : Finset ( $\kappa \times \kappa$ ) := Finset.image (fun x  $\rightarrow$  (x, 1)) (Finset.Icc 2
   $\rightarrow$  : n) with hB
  set C : Finset ( $\kappa \times \kappa$ ) := Finset.image (fun x  $\rightarrow$  (x, n + 1 - x))
   $\rightarrow$  : (Finset.Icc 2 (n - 1)) with hC
  have h51 : Finset.filter (fun p  $\rightarrow$  p.1 = 1  $\vee$  p.2 = 1  $\vee$  p.1 + p.2 = n +
   $\rightarrow$  : 1) hpoints  $\subseteq$  A  $\cup$  B  $\cup$  C := by
    intro p hp
    simp only [Finset.mem_filter] at hp
    have h5312 : p  $\in$  hpoints := hp.1
    have h5318 : p.1 = 1  $\vee$  p.2 = 1  $\vee$  p.1 + p.2 = n + 1 := hp.2
    have h5319 : p.1  $\geq$  1  $\wedge$  p.2  $\geq$  1  $\wedge$  p.1 + p.2  $\leq$  n + 1 := hpoints_def p
    <> omega
    by_cases h5324 : p.1 = 1
    have h1_eq : p.1 = 1 := h5324
    have h5315 : l.1  $\geq$  2 := by linarith
    have h5316 : p.2  $\leq$  n := by linarith
    have h5317 : p.2  $\in$  Finset.Icc 1 n := by
      simp [Finset.mem_Icc]
    <> omega
    have h5318 : p  $\in$  A := by
      rw [hA]
      refine' Finset.mem_image.mpr (p.2, h5317, _)
      simp [h1_eq, Prod.ext_iff]
      simp [h5318]
    have h1_ne : p.1  $\neq$  1 := h5324
    have h53110 : p.1  $\geq$  2 := by omega
    by_cases h53111 : p.2 = 1
    have h2_eq : p.2 = 1 := h53111
    have h53112 : 2  $\leq$  p.1 := by linarith
    have h53113 : p.1  $\leq$  n := by linarith
    have h53114 : p.1  $\in$  Finset.Icc 2 n := by
      simp [Finset.mem_Icc]
    <> omega
    have h53115 : p  $\in$  B := by
      rw [hB]
      refine' Finset.mem_image.mpr (p.1, h53114, _)
      simp [h2_eq, Prod.ext_iff]
      simp [h53115]
    have h2_ne : p.2  $\neq$  1 := h53111
    have h53117 : p.2  $\geq$  2 := by omega
    have h53118 : p.1 + p.2 = n + 1 := by omega
    have h53119 : p.1  $\leq$  n - 1 := by omega
    have h53122 : 2  $\leq$  p.1 := by linarith
    have h53124 : p.1  $\in$  Finset.Icc 2 (n - 1) := by
      simp [Finset.mem_Icc]
    <> omega
    have h53125 : p  $\in$  C := by
      rw [hC]
      refine' Finset.mem_image.mpr (p.1, h53124, _)
      simp [Prod.ext_iff]
    <> omega
    simp [h53125]
  have h52 : A  $\cup$  B  $\cup$  C  $\subseteq$  Finset.filter (fun p  $\rightarrow$  p.1 = 1  $\vee$  p.2 = 1  $\vee$  p.1 +
   $\rightarrow$  : p.2 = n + 1) hpoints := by
    intro p hp
    simp only [Finset.mem_union, Finset.mem_filter] at hp
    have h53214 : p  $\in$  A  $\vee$  p  $\in$  B  $\vee$  p  $\in$  C := by tauto
    rcases h53214 with (h53214 | h53214 | h53214)
    have h532141 : p  $\in$  A := h53214
    rw [hA] at h532141
    simp only [Finset.mem_image] at h532141
    rcases h532141 with y, hy, h532142
    have hy1 : 1  $\leq$  y := by
      simp [Finset.mem_Icc] at hy
    <> linarith
    have hy2 : y = n := by
      simp [Finset.mem_Icc] at hy
    <> linarith
    have h5321421 : p.1 = 1 := by
      simp [Prod.ext_iff] at h532142
    <> aesop
    have h532143 : p.2 = y := by
      have h532142' : p = (1, y) := by simp [Prod.ext_iff] at h532142
    <> tauto
    rw [h532142']
    have h532144 : p.1  $\geq$  1  $\wedge$  p.2  $\geq$  1  $\wedge$  p.1 + p.2  $\leq$  n + 1 := by
      constructor
      linarith
      constructor
      linarith
      linarith
    have h532145 : p  $\in$  hpoints := hpoints_def p |>.mpr h532144
    exact h532145, by tauto
    have h532141 : p  $\in$  B := h53214
    rw [hB] at h532141
    simp only [Finset.mem_image] at h532141
    rcases h532141 with x, hx, h532142
    have hx1 : 2  $\leq$  x := by
      simp [Finset.mem_Icc] at hx
    <> linarith
    have hx2 : x  $\leq$  n := by
      simp [Finset.mem_Icc] at hx
    <> linarith
    have h5321421 : p.1 = x := by
      simp [Prod.ext_iff] at h532142
    <> aesop
    have h5321422 : p.2 = 1 := by
      simp [Prod.ext_iff] at h532142
    <> aesop

```

```

have h532144 : p.1 ≥ 1 ∧ p.2 ≥ 1 ∧ p.1 + p.2 ≤ n + 1 := by
  constructor
  linarith
  constructor
  linarith
  have h532145 : p ∈ hpoints := hpoints_def p |>.mpr h532144
  exact h532145, by tauto

have h532141 : p ∈ C := h53214
rw [hC] at h532141
simp only [Finset.mem_image] at h532141
rcases h532141 with ⟨x, hx, h532142⟩
have hx1 : 2 ≤ x := by
  simp [Finset.mem_lcc] at hx
  <|> omega
have hx2 : x ≤ n - 1 := by
  simp [Finset.mem_lcc] at hx
  <|> omega
have h5321421 : p.1 = x := by
  simp [Prod.ext_iff] at h532142
  <|> aesop
have h5321422 : p.2 = n + 1 - x := by
  simp [Prod.ext_iff] at h532142
  <|> aesop
have h532144 : p.1 ≥ 1 ∧ p.2 ≥ 1 ∧ p.1 + p.2 ≤ n + 1 := by
  constructor
  linarith
  constructor
  omega
  omega
  have h532145 : p ∈ hpoints := hpoints_def p |>.mpr h532144
  have h532146 : p.1 + p.2 = n + 1 := by omega
  exact h532145, by tauto

have h53 : Finset.filter (fun p => p.1 = 1 ∨ p.2 = 1 ∨ p.1 + p.2 = n + 1) hpoints = A ∪ B ∪ C := by
  apply Finset.Subset.antisymm h51 h52
  rw [h53]
have h_disj1 : Disjoint A B := by
  rw [Finset.disjoint_left]
  intro p hpA hpB
  rw [hA] at hpA
  rw [hB] at hpB
  simp only [Finset.mem_image] at hpA hpB
  rcases hpA with ⟨y, hy, hpy⟩
  rcases hpB with ⟨x, hx, hpx⟩
  have h11 : p.1 = 1 := by
    simp [Prod.ext_iff] at hpy
    <|> aesop
  have h12 : p.1 ≥ 2 := by
    simp [Finset.mem_lcc] at hx
    simp [Prod.ext_iff] at hpx
    <|> omega
  omega
have h_disj2 : Disjoint A C := by
  rw [Finset.disjoint_left]
  intro p hpA hpC
  rw [hA] at hpA
  rw [hC] at hpC
  simp only [Finset.mem_image] at hpA hpC
  rcases hpA with ⟨y, hy, hpy⟩
  rcases hpC with ⟨x, hx, hpx⟩
  have h11 : p.1 = 1 := by
    simp [Prod.ext_iff] at hpy
    <|> aesop
  have h12 : p.1 ≥ 2 := by
    simp [Finset.mem_lcc] at hx
    simp [Prod.ext_iff] at hpx
    <|> omega
  omega
have h_disj3 : Disjoint B C := by
  rw [Finset.disjoint_left]
  intro p hpB hpC
  rw [hB] at hpB
  rw [hC] at hpC
  simp only [Finset.mem_image] at hpB hpC
  rcases hpB with ⟨x, hx, hpx⟩
  rcases hpC with ⟨x1, hx1, hpx1⟩
  have h1 : x1 < n := by
    have h11 : x1 ∈ Finset.lcc 2 (n - 1) := hx1
    have h12 : x1 ≤ n - 1 := by
      simp [Finset.mem_lcc] at h11
      <|> omega
    omega
  have h13 : (x, 1) = p := by tauto
  have h14 : (x1, n + 1 - x1) = p := by tauto
  have h15 : (x, 1) = (x1, n + 1 - x1) := by rw [h13, h14]
  have h2 : (x, 1).2 = (x1, n + 1 - x1).2 := by rw [h15]
  have h21 : (x, 1).2 = 1 := rfl
  have h22 : (x1, n + 1 - x1).2 = n + 1 - x1 := rfl
  rw [h21, h22] at h2
  omega
have hA_card : A.card = n := by
  rw [hA]
  have h_inj : Function.Injective (fun y : N => (1, y)) := by
    intro y1 y2 h
    simp [Prod.ext_iff] at h
    <|> aesop
  rw [Finset.card_image_of_injective _ h_inj]
  simp [Finset.lcc_eq_empty_of_lt]
  have hB_card : B.card = n - 1 := by
    rw [hB]
    have h_inj : Function.Injective (fun x : N => (x, 1)) := by
      intro x1 x2 h
      simp [Prod.ext_iff] at h
      <|> aesop
    rw [Finset.card_image_of_injective _ h_inj]
    simp [Finset.lcc_eq_empty_of_lt]
  have hC_card : C.card = n - 2 := by
    rw [hC]
    have h_inj : Function.Injective (fun x : N => (x, n + 1 - x)) := by
      intro x1 x2 h
      simp [Prod.ext_iff] at h
      <|> aesop
    rw [Finset.card_image_of_injective _ h_inj]
    simp [Finset.lcc_eq_empty_of_lt]
    <|> omega

```

```

simp_all
<|> omega

theorem num_points_on_boundary (n : N) (hpoints : Finset (N × N)) (hpoints_def
  → : ∀ p, p ∈ hpoints → p.1 ≥ 1 ∧ p.2 ≥ 1 ∧ p.1 + p.2 ≤ n + 1) :
  → (Finset.filter (fun p => p.1 = 1 ∨ p.2 = 1 ∨ p.1 + p.2 = n + 1)
    → hpoints).card = 3 * n - (if n = 1 then 2 else if n = 2 then 3 else 3) := by
  apply num_points_on_boundary_main
  assumption

theorem
  → non_sunny_lines_cover_at_most_2_points_on_boundary_same_boundary_condition_implies_eq
  → (n : N) (l : N × N) (points : Finset (N × N))
  (hn : 3 ≤ n) (h_non_sunny : l.1 ≠ 0 ∧ l.1 ≠ -1)
  (p q : N × N)
  (hp : (p.1 = 1 ∨ p.2 = 1 ∨ p.1 + p.2 = n + 1) ∧ (l.1 * (p.1 : R) + l.2 = (p.2
    → : R)))
  (hq : (q.1 = 1 ∨ q.2 = 1 ∨ q.1 + q.2 = n + 1) ∧ (l.1 * (q.1 : R) + l.2 = (q.2
    → : R)))
  (h_same_boundary : (p.1 = 1 ∧ q.1 = 1) ∨ (p.2 = 1 ∧ q.2 = 1) ∨ (p.1 + p.2 = n
    → + 1 ∧ q.1 + q.2 = n + 1)) :
  p = q := by
  rcases h_same_boundary with (h1 | h2 | h3)
  aesop
  simp_all
  have : (p.1 : R) = q.1 := by
    apply mul_left_cancel, h_non_sunny.1
    linarith
    aesop
  have : (p.1 : R) + (p.2 : R) = (n : R) + 1 := by exact_mod_cast h3.1
  have : (q.1 : R) + (q.2 : R) = (n : R) + 1 := by exact_mod_cast h3.2
  have : (p.1 : R) = q.1 := by
    apply mul_left_cancel, (sub_ne_zero.mpr h_non_sunny.2)
    linarith
    aesop

theorem non_sunny_lines_cover_at_most_2_points_on_boundary_main (n k : N)
  (verts : Finset R)
  (lines : Finset (R × R))
  (points : Finset (N × N))
  (l : R × R)
  (h_non_sunny : l.1 ≠ 0 ∧ l.1 ≠ -1)
  (p q r : N × N)
  (hp : p ∈ (Finset.filter (fun p => (p.1 = 1 ∨ p.2 = 1 ∨ p.1 + p.2 = n + 1) ∧
    → (l.1 * (p.1 : R) + l.2 = (p.2 : R))) points))
  (hq : q ∈ (Finset.filter (fun p => (p.1 = 1 ∨ p.2 = 1 ∨ p.1 + p.2 = n + 1) ∧
    → (l.1 * (p.1 : R) + l.2 = (p.2 : R))) points))
  (hr : r ∈ (Finset.filter (fun p => (p.1 = 1 ∨ p.2 = 1 ∨ p.1 + p.2 = n + 1) ∧
    → (l.1 * (p.1 : R) + l.2 = (p.2 : R))) points))
  (hp1 : p.1 = 1)
  (hq2 : q.2 = 1)
  (hr3 : r.1 + r.2 = n + 1)
  (hpq : p = q)
  (hpr : p ≠ r)
  (hqr : q ≠ r)
  (hn : 3 ≤ n)
  (hallpoints : ∀ p, p ∈ points → p.1 ≥ 1 ∧ p.2 ≥ 1 ∧ p.1 + p.2 ≤ n + 1) :
  False := by
  have h1 := (hallpoints p).mp (by simp_all)
  have h2 := (hallpoints q).mp (by simp_all)
  have h3 := (hallpoints r).mp (by simp_all)
  have h13 : l.1 + l.2 = (p.2 : R) := by simp_all
  have h23 : l.1 * (q.1 : R) + l.2 = 1 := by simp_all
  have h33 : l.1 * (r.1 : R) + l.2 = (r.2 : R) := by simp_all
  norm_num [hp1, hq2] at h13 h23
  have h13' : l.1 + l.2 = (p.2 : R) := by linarith
  have h23' : l.1 * (q.1 : R) + l.2 = 1 := by linarith
  have h4 : l.1 * ((q.1 : R) - 1) = 1 - (p.2 : R) := by linarith
  by_cases h10 : q.1 = 1
  · have h10' : (q.1 : R) = 1 := by exact_mod_cast h10
    have h11 : l.1 * ((q.1 : R) - 1) = 0 := by
      rw [h10']
      ring
    have h12 : 1 - (p.2 : R) = 0 := by linarith
    have h13 : (p.2 : R) = 1 := by linarith
    have h14 : p.2 = 1 := by exact_mod_cast h13
    have h15 : p.1 = 1 := hp1
    have h16 : p = (1, 1) := by
      ext <|> simp [h15, h14]
    have h17 : q = (1, 1) := by
      ext <|> simp [h10, hq2]
    have h18 : p = q := by rw [h16, h17]
    contradiction
  · have h10' : q.1 > 1 := by omega
    have h10'' : (q.1 : R) - 1 > 0 := by
      have h10''' : (q.1 : R) > 1 := by exact_mod_cast h10'
      linarith
    have h13_ne_0 : l.1 ≠ 0 := h_non_sunny.1
    have h13_ne_neg1 : l.1 ≠ -1 := h_non_sunny.2
    have h19 : p.2 ≥ 1 := h1.2.1
    have h20 : p.2 = 1 ∨ p.2 > 1 := by omega
    cases h20 with
    | inl h20 =>
      have h21 : (p.2 : R) = 1 := by exact_mod_cast h20
      have h22_l1_mul : l.1 * ((q.1 : R) - 1) = 0 := by
        rw [h21] at h4
        linarith
      have h25 : l.1 = 0 := by
        apply mul_left_cancel, (by linarith : (q.1 : R) - 1 ≠ 0)
        linarith
      contradiction
    | inr h20 =>
      have h21 : p.2 > 1 := h20
      have h22_p2_gt_1 : (p.2 : R) > 1 := by exact_mod_cast h21
      have h23 : 1 - (p.2 : R) < 0 := by linarith
      have h24 : l.1 * ((q.1 : R) - 1) < 0 := by linarith [h4, h23]
      have h25 : l.1 < 0 := by linarith
      have h33' : l.1 * (r.1 : R) + l.2 = (r.2 : R) := h33
      have h14 : (r.1 : R) + (r.2 : R) = (n : R) + 1 := by
        have h141 : (r.1 : R) + (r.2 : R) = ((r.1 + r.2 : N) : R) := by
          → norm_cast
        have h142 : r.1 + r.2 = n + 1 := hr3
        have h143 : ((r.1 + r.2 : N) : R) = ((n + 1 : N) : R) := by rw [h142]
        have h144 : ((n + 1 : N) : R) = (n : R) + 1 := by norm_cast

```

```

linarith
have h15 : 1.1 * (r.1 :  $\kappa$ ) - 1.1 + (p.2 :  $\kappa$ ) = (r.2 :  $\kappa$ ) := by linarith
have h16 : 1.1 * ((r.1 :  $\kappa$ ) - 1) + (p.2 :  $\kappa$ ) = (r.2 :  $\kappa$ ) := by linarith
by_cases h17 : p.2 = r.2
· have h17' : (p.2 :  $\kappa$ ) = (r.2 :  $\kappa$ ) := by exact_mod_cast h17
· have h18 : 1.1 * ((r.1 :  $\kappa$ ) - 1) = 0 := by linarith [h16, h17']
have h19 : (r.1 :  $\kappa$ ) - 1 = 0 := by
  apply mul_left_cancel, h13_ne_0
linarith
have h20 : (r.1 :  $\kappa$ ) = 1 := by linarith
have h21 : r.1 = 1 := by exact_mod_cast h20
have h22 : r.2 = n := by omega
have h23 : p.2 = n := by linarith [h17, h22]
have h24 : p.1 = 1 := hpl
have h25 : p = (1, n) := by ext <;> simp [h24, h23]
have h26 : r.1 = 1 := h21
have h27 : r.2 = n := h22
have h28 : r = (1, n) := by ext <;> simp [h26, h27]
have h29 : p = r := by rw [h25, h28]
contradiction
by_cases h17'' : q.2 = r.2
· have h17''' : q.2 = r.2 := h17''
· have h17'''' : q.2 = 1 := hq2
  have h17''''' : r.2 = 1 := by linarith
  have h20 : r.1 = n := by omega
  have h21 : 1.1 * (r.1 :  $\kappa$ ) + 1.2 = (r.2 :  $\kappa$ ) := h33
  have h22 : (r.1 :  $\kappa$ ) = (n :  $\kappa$ ) := by exact_mod_cast h20
  have h23 : (r.2 :  $\kappa$ ) = 1 := by exact_mod_cast h17'''''
  have h24 : 1.1 * (n :  $\kappa$ ) + 1.2 = 1 := by
    rw [h22, h23] at h21
  linarith
  have h25 : 1.1 + 1.2 = (p.2 :  $\kappa$ ) := h13'
  have h26 : 1.1 * (n :  $\kappa$ ) + 1.2 - (1.1 + 1.2) = 1 - (p.2 :  $\kappa$ ) := by
    linarith
  have h27 : 1.1 * ((n :  $\kappa$ ) - 1) = 1 - (p.2 :  $\kappa$ ) := by linarith
  have h28 : 1.1 * ((q.1 :  $\kappa$ ) - 1) = 1 - (p.2 :  $\kappa$ ) := by linarith
  have h29 : 1.1 * ((q.1 :  $\kappa$ ) - 1) = 1.1 * ((n :  $\kappa$ ) - 1) := by linarith
  have h30 : (q.1 :  $\kappa$ ) - 1 = (n :  $\kappa$ ) - 1 := by
    apply mul_left_cancel, h13_ne_0
  linarith
  have h31 : (q.1 :  $\kappa$ ) = (n :  $\kappa$ ) := by linarith
  have h32 : q.1 = n := by exact_mod_cast h31
  have h33 : q.2 = 1 := hq2
  have h34 : q = (n, 1) := by ext <;> simp [h32, h33]
  have h35 : r.1 = n := h20
  have h36 : r.2 = 1 := h17'''''
  have h37 : r = (n, 1) := by ext <;> simp [h35, h36]
  have h38 : q = r := by rw [h34, h37]
  contradiction
by_cases h17' : q.2  $\neq$  r.2
· have h26 : r.2  $\geq 2$  := by
  have h261 : r.2  $\geq 1$  := h3.2.1
  omega
  by_cases h50 : r.1 = 1
  · have h51 : (r.1 :  $\kappa$ ) = 1 := by exact_mod_cast h50
  · have h52 : (r.1 :  $\kappa$ ) - 1 = 0 := by linarith
  have h53 : 1.1 * ((r.1 :  $\kappa$ ) - 1) = 0 := by
    rw [h52]
    <;> ring
  have h54 : (r.2 :  $\kappa$ ) - (p.2 :  $\kappa$ ) = 0 := by linarith [h16, h53]
  have h54' : (r.2 :  $\kappa$ ) = (p.2 :  $\kappa$ ) := by linarith
  have h55 : r.2 = p.2 := by exact_mod_cast h54'
  have h56 : p.2 = r.2 := by linarith
  contradiction
· have h50' : r.1  $\geq 2$  := by omega
  have h50'' : (r.1 :  $\kappa$ )  $\geq 2$  := by exact_mod_cast h50'
  have h51 : (r.1 :  $\kappa$ ) - 1  $> 0$  := by linarith
  by_cases h52 : 1.1  $< -1$ 
  · have h53 : 1.1 * ((r.1 :  $\kappa$ ) - 1)  $< -1$  * ((r.1 :  $\kappa$ ) - 1) := by
    nlinarith
  · have h54 : (n :  $\kappa$ ) + 1 - (p.2 :  $\kappa$ ) - 1  $< 0$  := by linarith
  have h55 : (n :  $\kappa$ )  $<$  (p.2 :  $\kappa$ ) := by linarith
  have h55' : p.2  $\leq n$  := by linarith [h1.2.2]
  have h55'' : (p.2 :  $\kappa$ )  $\leq$  (n :  $\kappa$ ) := by exact_mod_cast h55'
  linarith
  · have h52' : 1.1  $> -1$  := by
      by_contra h521
      have h522 : 1.1  $\leq -1$  := by linarith
      have h523 : 1.1 = -1 := by linarith
      contradiction
      have h53 : 1.1 * ((q.1 :  $\kappa$ ) - (r.1 :  $\kappa$ )) = 1 - (r.2 :  $\kappa$ ) := by
        have h531 : 1.1 * (q.1 :  $\kappa$ ) + 1.2 = 1 := by simp using h23'
        have h532 : 1.1 * (r.1 :  $\kappa$ ) + 1.2 = (r.2 :  $\kappa$ ) := by simp
      using h33
      have h : 1.1 * (q.1 :  $\kappa$ ) + 1.2 - (1.1 * (r.1 :  $\kappa$ ) + 1.2) = 1
      - (r.2 :  $\kappa$ ) := by linarith
      have h' : 1.1 * (q.1 :  $\kappa$ ) - 1.1 * (r.1 :  $\kappa$ ) = 1 - (r.2 :  $\kappa$ )
      := by linarith
      have h'' : 1.1 * ((q.1 :  $\kappa$ ) - (r.1 :  $\kappa$ )) = 1 - (r.2 :  $\kappa$ ) :=
        by linarith
      linarith
      have h54 : (q.1 :  $\kappa$ )  $>$  (r.1 :  $\kappa$ ) := by
        have h541 : 1.1 * ((q.1 :  $\kappa$ ) - (r.1 :  $\kappa$ )) = 1 - (r.2 :  $\kappa$ ) :=
          by
            have h542 : (r.2 :  $\kappa$ )  $\geq 2$  := by exact_mod_cast h26
            have h543 : 1 - (r.2 :  $\kappa$ )  $\leq -1$  := by linarith
            have h544 : 1.1 * ((q.1 :  $\kappa$ ) - (r.1 :  $\kappa$ ))  $\leq -1$  := by linarith
            nlinarith
            have h54' : (q.1 :  $\kappa$ ) - (r.1 :  $\kappa$ )  $> 0$  := by linarith
            have h55 : 1.1 * ((q.1 :  $\kappa$ ) - (r.1 :  $\kappa$ ))  $> -1$  * ((q.1 :  $\kappa$ ) -
              (r.1 :  $\kappa$ )) := by nlinarith
            have h56 : (q.1 :  $\kappa$ ) + 1  $>$  (r.1 :  $\kappa$ ) + (r.2 :  $\kappa$ ) := by
              linarith [h53, h55]
            have h56' : (q.1 :  $\kappa$ )  $>$  (n :  $\kappa$ ) := by linarith [h14, h56]
            have h56'' : q.1  $> n$  := by exact_mod_cast h56'
            have h57 : q.1 + q.2  $\leq n + 1$  := h2.2.2
            linarith
          simp_all
    theorem non_sunny_lines_cover_at_most_2_points_on_boundary_final (n k :  $\mathbb{N}$ )
      (verts : Finset  $\kappa$ )
      (lines : Finset ( $\kappa \times \kappa$ ))
      (points : Finset ( $\mathbb{N} \times \mathbb{N}$ ))

```

```

(1 :  $\kappa \times \kappa$ )
(h_non_sunny : 1.1  $\neq 0 \wedge 1.1 \neq -1$ )
(p q r :  $\mathbb{N} \times \mathbb{N}$ )
(hp : p  $\in$  (Finset.filter (fun p  $\mapsto$  (p.1 = 1  $\vee$  p.2 = 1  $\vee$  p.1 + p.2 = n + 1)  $\wedge$ 
   $\rightarrow$  (1.1 * (p.1 :  $\kappa$ ) + 1.2 = (p.2 :  $\kappa$ )) points))
(hq : q  $\in$  (Finset.filter (fun p  $\mapsto$  (p.1 = 1  $\vee$  p.2 = 1  $\vee$  p.1 + p.2 = n + 1)  $\wedge$ 
   $\rightarrow$  (1.1 * (p.1 :  $\kappa$ ) + 1.2 = (p.2 :  $\kappa$ )) points))
(hr : r  $\in$  (Finset.filter (fun p  $\mapsto$  (p.1 = 1  $\vee$  p.2 = 1  $\vee$  p.1 + p.2 = n + 1)  $\wedge$ 
   $\rightarrow$  (1.1 * (p.1 :  $\kappa$ ) + 1.2 = (p.2 :  $\kappa$ )) points))
(hp1 : p.1 = 1)
(hq2 : q.2 = 1)
(hr3 : r.1 + r.2 = n + 1)
(hpq : p  $\neq$  q)
(hpr : p  $\neq$  r)
(hqr : q  $\neq$  r)
(hn : 3  $\leq$  n)
(hallpoints :  $\forall p, p \in$  points  $\rightarrow$  p.1  $\geq 1 \wedge$  p.2  $\geq 1 \wedge$  p.1 + p.2  $\leq$  n + 1) :
False := by
  exact non_sunny_lines_cover_at_most_2_points_on_boundary_main n k verts
   $\rightarrow$  lines points l h_non_sunny p q r hp hq hr hpl hq2 hr3 hpq hpr hqr hn
   $\rightarrow$  hallpoints

theorem
   $\rightarrow$  non_sunny_lines_cover_at_most_2_points_on_boundary_contradiction_from_conditions
   $\rightarrow$  (n k :  $\mathbb{N}$ )
  (verts : Finset  $\kappa$ )
  (lines : Finset ( $\kappa \times \kappa$ ))
  (points : Finset ( $\mathbb{N} \times \mathbb{N}$ ))
  (1 :  $\kappa \times \kappa$ )
  (h_non_sunny : 1.1  $\neq 0 \wedge 1.1 \neq -1$ )
  (p q r :  $\mathbb{N} \times \mathbb{N}$ )
  (hp : p  $\in$  (Finset.filter (fun p  $\mapsto$  (p.1 = 1  $\vee$  p.2 = 1  $\vee$  p.1 + p.2 = n + 1)  $\wedge$ 
     $\rightarrow$  (1.1 * p.1 + 1.2 = p.2) points))
  (hq : q  $\in$  (Finset.filter (fun p  $\mapsto$  (p.1 = 1  $\vee$  p.2 = 1  $\vee$  p.1 + p.2 = n + 1)  $\wedge$ 
     $\rightarrow$  (1.1 * p.1 + 1.2 = p.2) points))
  (hr : r  $\in$  (Finset.filter (fun p  $\mapsto$  (p.1 = 1  $\vee$  p.2 = 1  $\vee$  p.1 + p.2 = n + 1)  $\wedge$ 
     $\rightarrow$  (1.1 * p.1 + 1.2 = p.2) points))
  (hp1 : p.1 = 1)
  (hq2 : q.2 = 1)
  (hr3 : r.1 + r.2 = n + 1)
  (hpq : p  $\neq$  q)
  (hpr : p  $\neq$  r)
  (hqr : q  $\neq$  r)
  (hn : 3  $\leq$  n)
  (hallpoints :  $\forall p, p \in$  points  $\rightarrow$  p.1  $\geq 1 \wedge$  p.2  $\geq 1 \wedge$  p.1 + p.2  $\leq$  n + 1) :
False := by
  apply non_sunny_lines_cover_at_most_2_points_on_boundary_final n k verts
   $\rightarrow$  lines points l h_non_sunny p q r
  <;> aesop

theorem non_sunny_lines_cover_at_most_2_points_on_boundary_h_final (n k :  $\mathbb{N}$ )
  (verts : Finset  $\kappa$ )
  (lines : Finset ( $\kappa \times \kappa$ ))
  (points : Finset ( $\mathbb{N} \times \mathbb{N}$ ))
  (hn : 3  $\leq$  n)
  (hcard : lines.card + verts.card = n)
  (hallpoints :  $\forall p, p \in$  points  $\rightarrow$  p.1  $\geq 1 \wedge$  p.2  $\geq 1 \wedge$  p.1 + p.2  $\leq$  n + 1)
  (hmain :  $\forall p \in$  points, ( $\exists l \in$  lines, 1.1 * p.1 + 1.2 = p.2)  $\vee$  ( $\exists x \in$  verts,
     $\rightarrow$  p.1 = x))
  (hk : (lines.filter (fun l  $\mapsto$  1.1 * 0  $\wedge$  1.1 * -1)).card = k)
  (1 :  $\kappa \times \kappa$ )
  (h_non_sunny : 1.1  $\neq 0 \wedge 1.1 \neq -1$ )
  (h_main :  $\forall (x y z : \mathbb{N} \times \mathbb{N}), x \in$  (Finset.filter (fun p  $\mapsto$  (p.1 = 1  $\vee$  p.2 = 1  $\vee$ 
    p.1 + p.2 = n + 1)  $\wedge$  (1.1 * p.1 + 1.2 = p.2) points)  $\rightarrow y \in$ 
    (Finset.filter (fun p  $\mapsto$  (p.1 = 1  $\vee$  p.2 = 1  $\vee$  p.1 + p.2 = n + 1)  $\wedge$ 
     $\rightarrow$  (1.1 * p.1 + 1.2 = p.2) points)  $\rightarrow z \in$  (Finset.filter (fun p  $\mapsto$  (p.1 =
    1  $\vee$  p.2 = 1  $\vee$  p.1 + p.2 = n + 1)  $\wedge$  (1.1 * p.1 + 1.2 = p.2) points)  $\rightarrow$ 
     $\rightarrow x = y \vee x = z \vee y = z$ ) :
    (Finset.filter (fun p  $\mapsto$  (p.1 = 1  $\vee$  p.2 = 1  $\vee$  p.1 + p.2 = n + 1)  $\wedge$  (1.1 * p.1 +
    1.2 = p.2) points).card  $\leq 2$  := by
      contrapose! h_main
      exact Finset.two_lt_card_iff.mp h_main

theorem non_sunny_lines_cover_at_most_2_points_on_boundary_h_main (n k :  $\mathbb{N}$ )
  (verts : Finset  $\kappa$ )
  (lines : Finset ( $\kappa \times \kappa$ ))
  (points : Finset ( $\mathbb{N} \times \mathbb{N}$ ))
  (hn : 3  $\leq$  n)
  (hcard : lines.card + verts.card = n)
  (hallpoints :  $\forall p, p \in$  points  $\rightarrow$  p.1  $\geq 1 \wedge$  p.2  $\geq 1 \wedge$  p.1 + p.2  $\leq$  n + 1)
  (hmain :  $\forall p \in$  points, ( $\exists l \in$  lines, 1.1 * p.1 + 1.2 = p.2)  $\vee$  ( $\exists x \in$  verts,
     $\rightarrow$  p.1 = x))
  (hk : (lines.filter (fun l  $\mapsto$  1.1 * 0  $\wedge$  1.1 * -1)).card = k)
  (1 :  $\kappa \times \kappa$ )
  (h_non_sunny : 1.1  $\neq 0 \wedge 1.1 \neq -1$ ) :
   $\forall (x y z : \mathbb{N} \times \mathbb{N}), x \in$  (Finset.filter (fun p  $\mapsto$  (p.1 = 1  $\vee$  p.2 = 1  $\vee$  p.1 + p.2
    = n + 1)  $\wedge$  (1.1 * p.1 + 1.2 = p.2) points)  $\rightarrow y \in$  (Finset.filter (fun
    p  $\mapsto$  (p.1 = 1  $\vee$  p.2 = 1  $\vee$  p.1 + p.2 = n + 1)  $\wedge$  (1.1 * p.1 + 1.2 =
    p.2) points)  $\rightarrow z \in$  (Finset.filter (fun p  $\mapsto$  (p.1 = 1  $\vee$  p.2 = 1  $\vee$  p.1 +
    p.2 = n + 1)  $\wedge$  (1.1 * p.1 + 1.2 = p.2) points)  $\rightarrow x = y \vee x = z \vee y = z$ 
    := by
    intro x y z hx hy hz
    by_contra! h
    have hx_prop : = Finset.mem_filter.mp hx |>.2
    have hy_prop : = Finset.mem_filter.mp hy |>.2
    have hz_prop : = Finset.mem_filter.mp hz |>.2
    rcases hx_prop.1 with (hx1 | hx2 | hx3)
    -- Case z.1 = 1
    rcases hy_prop.1 with (hy1 | hy2 | hy3)
    -- Subcase y.1 = 1
    have h_x_eq_y : x = y := by
      apply
       $\rightarrow$  non_sunny_lines_cover_at_most_2_points_on_boundary_same_boundary_condition_implies_eq
       $\rightarrow$  n 1 points hn h_non_sunny x y hx_prop hy_prop
      tauto
    tauto
    -- Subcase y.2 = 1
    rcases hz_prop.1 with (hz1 | hz2 | hz3)
    -- Sub-subcase z.1 = 1
    have h_z_eq_x : z = x := by
      apply
       $\rightarrow$  non_sunny_lines_cover_at_most_2_points_on_boundary_same_boundary_condition_implies_eq
       $\rightarrow$  n 1 points hn h_non_sunny z x hz_prop hx_prop

```

```

tauto
tauto
-- Sub-subcase z.2 = 1
have h_y_eq_z : y = z := by
  apply
-- non_sunny_lines_cover_at_most_2_points_on_boundary_same_boundary_condition_implies_eq
-- n 1 points hn h_non_sunny y z hy_prop hz_prop
tauto
-- Sub-subcase z.1 + z.2 = n + 1
ex falso
exact
-- non_sunny_lines_cover_at_most_2_points_on_boundary_contradiction_from_conditions
-- n k verts lines points 1 h_non_sunny x z y hx hy hz hx1 hy2 hz3 (by
-- tauto) (by tauto) (by tauto) hn hallpoints
-- Subcase y.1 + y.2 = n + 1
rcases hz_prop.1 with (hz1 | hz2 | hz3)
-- Sub-subcase z.1 = 1
have h_z_eq_x : z = x := by
  apply
-- non_sunny_lines_cover_at_most_2_points_on_boundary_same_boundary_condition_implies_eq
-- n 1 points hn h_non_sunny z x hz_prop hx_prop
tauto
-- Sub-subcase z.2 = 1
ex falso
exact
-- non_sunny_lines_cover_at_most_2_points_on_boundary_contradiction_from_conditions
-- n k verts lines points 1 h_non_sunny x z y hx hy hz hx1 hy2 hz3 (by
-- tauto) (by tauto) (by tauto) hn hallpoints
-- Sub-subcase z.1 + z.2 = n + 1
have h_y_eq_z : y = z := by
  apply
-- non_sunny_lines_cover_at_most_2_points_on_boundary_same_boundary_condition_implies_eq
-- n 1 points hn h_non_sunny y z hy_prop hz_prop
tauto
-- Case z.2 = 1
rcases hy_prop.1 with (hy1 | hy2 | hy3)
-- Subcase y.1 = 1
rcases hz_prop.1 with (hz1 | hz2 | hz3)
-- Sub-subcase z.1 = 1
have h_y_eq_z : y = z := by
  apply
-- non_sunny_lines_cover_at_most_2_points_on_boundary_same_boundary_condition_implies_eq
-- n 1 points hn h_non_sunny y z hy_prop hz_prop
tauto
-- Sub-subcase z.2 = 1
have h_x_eq_z : x = z := by
  apply
-- non_sunny_lines_cover_at_most_2_points_on_boundary_same_boundary_condition_implies_eq
-- n 1 points hn h_non_sunny x z hx_prop hz_prop
tauto
-- Sub-subcase z.1 + z.2 = n + 1
ex falso
exact
-- non_sunny_lines_cover_at_most_2_points_on_boundary_contradiction_from_conditions
-- n k verts lines points 1 h_non_sunny y x z hy hx hz hy1 hx2 hz3 (by
-- tauto) (by tauto) (by tauto) hn hallpoints
-- Case y.2 = 1
have h_x_eq_y : x = y := by
  apply
-- non_sunny_lines_cover_at_most_2_points_on_boundary_same_boundary_condition_implies_eq
-- n 1 points hn h_non_sunny x y hx_prop hy_prop
tauto
-- Case y.1 + y.2 = n + 1
rcases hz_prop.1 with (hz1 | hz2 | hz3)
-- Sub-subcase z.1 = 1
ex falso
exact
-- non_sunny_lines_cover_at_most_2_points_on_boundary_contradiction_from_conditions
-- n k verts lines points 1 h_non_sunny z x y hz hx hy hz1 hx2 hy3 (by
-- tauto) (by tauto) (by tauto) hn hallpoints
-- Sub-subcase z.2 = 1
have h_x_eq_z : x = z := by
  apply
-- non_sunny_lines_cover_at_most_2_points_on_boundary_same_boundary_condition_implies_eq
-- n 1 points hn h_non_sunny x z hx_prop hz_prop
tauto
-- Case z.1 + z.2 = n + 1
rcases hy_prop.1 with (hy1 | hy2 | hy3)
-- Subcase y.1 = 1
rcases hz_prop.1 with (hz1 | hz2 | hz3)
-- Sub-subcase z.1 = 1
have h_y_eq_z : y = z := by
  apply
-- non_sunny_lines_cover_at_most_2_points_on_boundary_same_boundary_condition_implies_eq
-- n 1 points hn h_non_sunny y z hy_prop hz_prop
tauto
-- Sub-subcase z.2 = 1
ex falso
exact
-- non_sunny_lines_cover_at_most_2_points_on_boundary_contradiction_from_conditions
-- n k verts lines points 1 h_non_sunny y x z hy hx hz hy1 hx2 hz3 (by
-- tauto) (by tauto) (by tauto) hn hallpoints
-- Sub-subcase z.1 + z.2 = n + 1
have h_x_eq_z : x = z := by
  apply
-- non_sunny_lines_cover_at_most_2_points_on_boundary_same_boundary_condition_implies_eq
-- n 1 points hn h_non_sunny x z hx_prop hz_prop
tauto
-- Subcase y.2 = 1
rcases hz_prop.1 with (hz1 | hz2 | hz3)
-- Sub-subcase z.1 = 1
ex falso

```

```

exact
-- non_sunny_lines_cover_at_most_2_points_on_boundary_contradiction_from_conditions
-- n k verts lines points 1 h_non_sunny z y x hz hy hx hz1 hy2 hz3 (by
-- tauto) (by tauto) (by tauto) hn hallpoints
-- Sub-subcase z.2 = 1
have h_y_eq_z : y = z := by
  apply
-- non_sunny_lines_cover_at_most_2_points_on_boundary_same_boundary_condition_implies_eq
-- n 1 points hn h_non_sunny y z hy_prop hz_prop
tauto
-- Sub-subcase z.1 + z.2 = n + 1
have h_x_eq_z : x = z := by
  apply
-- non_sunny_lines_cover_at_most_2_points_on_boundary_same_boundary_condition_implies_eq
-- n 1 points hn h_non_sunny x z hx_prop hz_prop
tauto
-- Subcase y.1 + y.2 = n + 1
have h_x_eq_y : x = y := by
  apply
-- non_sunny_lines_cover_at_most_2_points_on_boundary_same_boundary_condition_implies_eq
-- n 1 points hn h_non_sunny x y hx_prop hy_prop
tauto
tauto

theorem non_sunny_lines_cover_at_most_2_points_on_boundary (n k : ℕ) (verts :
  Finset ℕ) (lines : Finset (ℕ × ℕ)) (points : Finset (ℕ × ℕ)) (hn : 3 ≤
  n) (hcard : lines.card + verts.card = n) (hallpoints : ∀ p, p ∈
  points → p.1 ≥ 1 ∧ p.2 ≥ 1 ∧ p.1 + p.2 ≤ n + 1) (hmain : ∀ p ∈
  points, (∃ l ∈ lines, l.1 * p.1 + l.2 * p.2 = p.2) ∨ (∃ x ∈ verts, p.1 = x))
  (hk : (lines.filter (fun l → l.1 * 0 + l.1 * -1)).card = k) (l : ℕ × ℕ
  → (h_non_sunny : l.1 + 0 + l.1 * -1) :
  (l.1 * p.1 + l.2 * p.2 = p.2) points).card ≤ 2 := by
  apply non_sunny_lines_cover_at_most_2_points_on_boundary_h_final <> try
  → assumption
  apply non_sunny_lines_cover_at_most_2_points_on_boundary_h_main <> try
  → assumption

theorem round1_case_l1_eq_0 (n k : ℕ) (verts : Finset ℕ) (lines : Finset (ℕ × ℕ)
  →)) (points : Finset (ℕ × ℕ))
  (hn : 3 ≤ n) (hcard : lines.card + verts.card = n)
  (hallpoints : ∀ p, p ∈ points → p.1 ≥ 1 ∧ p.2 ≥ 1 ∧ p.1 + p.2 ≤ n + 1)
  (hmain : ∀ p ∈ points, (∃ l ∈ lines, l.1 * p.1 + l.2 * p.2 = p.2) ∨ (∃ x ∈ verts,
  → p.1 = x))
  (hk : (lines.filter (fun l → l.1 * 0 + l.1 * -1)).card = k)
  (l : ℕ × ℕ → (h_non_boundary : ¬ (l.1 = 0 ∧ l.2 = 1) ∧ ¬ (l.1 = -1 ∧ l.2 = n +
  → 1))
  (h10 : l.1 = 0) :
  (Finset.filter (fun p → (p.1 = 1 ∨ p.2 = 1 ∨ p.1 + p.2 = n + 1) ∧ (l.1 * p.1 +
  → l.2 * p.2) points).card ≤ 2 := by
  set S := Finset.filter (fun p → (p.1 = 1 ∨ p.2 = 1 ∨ p.1 + p.2 = n + 1) ∧
  → (l.1 * p.1 + l.2 * p.2 = p.2)) points
  set A := S.filter (fun p → p.1 = 1)
  set B := S.filter (fun p → p.1 + p.2 = n + 1)
  have S ⊆ A ∪ B := by
    intro p hp
    aesop
  have h1 : (A ∪ B).card ≤ A.card + B.card := Finset.card_union_le A B
  have h2 : S.card ≤ (A ∪ B).card := Finset.card_le_card this
  have h3 : A.card ≤ 1 := by
    apply Finset.card_le_one.mpr
    intro p hp q hq
    obtain h1, h2 := Finset.mem_filter.mp hp
    obtain h3, h4 := Finset.mem_filter.mp hq
    aesop
  have h4 : B.card ≤ 1 := by
    apply Finset.card_le_one.mpr
    intro p hp q hq
    obtain h1, h2 := Finset.mem_filter.mp hp
    obtain h3, h4 := Finset.mem_filter.mp hq
    have h4 : p.2 = q.2 := by aesop
    have h5 : p.1 = q.1 := by linarith
    aesop
    linarith

theorem round1_case_l1_eq_neg1 (n k : ℕ) (verts : Finset ℕ) (lines : Finset (ℕ
  implies_eq ℕ)) (points : Finset (ℕ × ℕ))
  (hn : 3 ≤ n) (hcard : lines.card + verts.card = n)
  (hallpoints : ∀ p, p ∈ points → p.1 ≥ 1 ∧ p.2 ≥ 1 ∧ p.1 + p.2 ≤ n + 1)
  (hmain : ∀ p ∈ points, (∃ l ∈ lines, l.1 * p.1 + l.2 * p.2 = p.2) ∨ (∃ x ∈ verts,
  → p.1 = x))
  (hk : (lines.filter (fun l → l.1 * 0 + l.1 * -1)).card = k)
  (h1 : (lines.filter (fun l → l.1 * 0 + l.1 * -1)).card = k)
  (h12 : l.1 = -1) :
  (Finset.filter (fun p → (p.1 = 1 ∨ p.2 = 1 ∨ p.1 + p.2 = n + 1) ∧ (l.1 * p.1 +
  → l.2 * p.2) points).card ≤ 2 := by
  have h13 : l.2 ≠ (n : ℕ) + 1 := by simp_all
  set S := Finset.filter (fun p → (p.1 = 1 ∨ p.2 = 1 ∨ p.1 + p.2 = n + 1) ∧
  → (l.1 * p.1 + l.2 * p.2 = p.2)) points
  have h14 : ∀ p ∈ S, p.1 = 1 ∨ p.2 = 1 := by
    intro p hp
    rcases Finset.mem_filter.mp hp with (l, h14)
    by contra
    have h142 : p.1 + p.2 = n + 1 := by tauto
    have h143 : (p.1 : ℕ) + (p.2 : ℕ) = (n : ℕ) + 1 := by exact_mod_cast h142
    have h144 : l.2 = (n : ℕ) + 1 := by linarith
    contradiction
  have h15 : ∀ p ∈ S, l.2 = (p.1 : ℕ) + (p.2 : ℕ) := by
    intro p hp
    rcases Finset.mem_filter.mp hp with (l, h15)
    rw [h12] at h15
    linarith
  set A := S.filter (fun p → p.1 = 1)
  set B := S.filter (fun p → p.2 = 1)
  have h16 : S ⊆ A ∪ B := by
    intro p hp
    rcases h14 p hp with (h161 | h161) <> simp [A, B, Finset.mem_filter] <>
    tauto
  have h17 : A.card ≤ 1 := by
    apply Finset.card_le_one.mpr
    intro p hp q hq
    simp [A, Finset.mem_filter] at hp hq

```

```

have h171 := h15 p hp.1
have h172 := h15 q hq.1
have h173 : (p.1 :  $\kappa$ ) = 1 := by exact_mod_cast hp.2
have h174 : (q.1 :  $\kappa$ ) = 1 := by exact_mod_cast hq.2
rw [h173] at h171
rw [h174] at h172
have h175 : (p.2 :  $\kappa$ ) = (q.2 :  $\kappa$ ) := by linarith
have h176 : p.2 = q.2 := by exact_mod_cast h175
have h177 : p.1 = q.1 := by simp [hp.2, hq.2]
have h178 : p = q := by
  ext <|> tauto
exact h178
have h18 : B.card ≤ 1 := by
  apply Finset.card_le_one.mpr
  intro p hp q hq
  simp [B, Finset.mem_filter] at hp hq
  have h181 := h15 p hp.1
  have h182 := h15 q hq.1
  have h183 : (p.2 :  $\kappa$ ) = 1 := by exact_mod_cast hp.2
  have h184 : (q.2 :  $\kappa$ ) = 1 := by exact_mod_cast hq.2
  rw [h183] at h181
  rw [h184] at h182
  have h185 : (p.1 :  $\kappa$ ) = (q.1 :  $\kappa$ ) := by linarith
  have h186 : p.1 = q.1 := by exact_mod_cast h185
  have h187 : p.2 = q.2 := by simp [hp.2, hq.2]
  have h188 : p = q := by
    ext <|> tauto
exact h188
exact Finset.card_le_card h16 |>.trans (Finset.card_union_le A B) |>.trans
  (by linarith)

theorem line_not_boundary_covers_at_most_2_boundary_points (n k :  $\mathbb{N}$ ) (verts :
  → Finset  $\kappa$ ) (lines : Finset ( $\kappa \times \kappa$ )) (points : Finset ( $\mathbb{N} \times \mathbb{N}$ )) (hn : 3 ≤ n)
  → n (hcard : lines.card + verts.card = n) (hallpoints :  $\forall p, p \in$ 
  → points → p.1 ≥ 1 ∧ p.2 ≥ 1 ∧ p.1 + p.2 ≤ n + 1) (hmain :  $\forall p \in$ 
  → points, ( $\exists l \in$  lines,  $l.1 * p.1 + l.2 = p.2$ ) ∨ ( $\exists x \in$  verts,  $p.1 = x$ ))
  → (hk : (lines.filter (fun l => l.1 ≠ 0 ∧ l.1 ≠ -1)).card = k) (l :  $\mathbb{R} \times \mathbb{R}$ 
  → 1) :
  (Finset.filter (fun p => (p.1 = 1 ∨ p.2 = 1 ∨ p.1 + p.2 = n + 1) ∧
    (l.1 * p.1 + l.2 = p.2)) points).card ≤ 2 := by
  by_cases h0 : l.1 = 0
  · apply round1_case_l1_eq_0 n k verts lines points hn hcard hallpoints hmain
    → hk l h_non_boundary h0
  · by_cases h1 : l.1 = -1
    · apply round1_case_l1_eq_neg1 n k verts lines points hn hcard hallpoints
      → hmain hk l h_non_boundary h1
    · apply non_sunny_lines_cover_at_most_2_points_on_boundary n k verts lines
      → points hn hcard hallpoints hmain hk
  aesop

theorem vert_line_covers_at_most_two_boundary_points (n :  $\mathbb{N}$ )
  (points : Finset ( $\mathbb{N} \times \mathbb{N}$ ))
  (x :  $\kappa$ )
  (hx_neq1 : x ≠ 1):
  (Finset.filter (fun p :  $\mathbb{N} \times \mathbb{N}$  => p.1 ≥ 1 ∧ p.2 ≥ 1 ∧ p.1 + p.2 ≤ n + 1 ∧
    ((p.1 = 1 ∨ p.2 = 1 ∨ p.1 + p.2 = n + 1) ∧ (p.1 = x)) points).card ≤
    2 := by
  rcases (Finset.filter (fun p => p.1 ≥ 1 ∧ p.2 ≥ 1 ∧ p.1 + p.2 ≤ n + 1 ∧ (p.1 =
    → 1 ∨ p.2 = 1 ∨ p.1 + p.2 = n + 1) ∧ (p.1 = x))
    → points).eq_empty_or_nonempty with h | p, hp)
  · aesop
  have : Finset.filter (fun p => p.1 ≥ 1 ∧ p.2 ≥ 1 ∧ p.1 + p.2 ≤ n + 1 ∧ (p.1 =
    → 1 ∨ p.2 = 1 ∨ p.1 + p.2 = n + 1) ∧ (p.1 = x) points ⊆ { (p.1, 1),
    → (p.1, n + 1 - p.1) } := by
    intro p hp
    simp only [Finset.mem_filter] at hp
    have : p.1 = p.1 := by aesop
    have : p.2 = 1 ∨ p.1 + p.2 = n + 1 := by aesop
    rcases this with (h | h)
    · aesop
    · have : p.2 = n + 1 - p.1 := by omega
      aesop
  exact (Finset.card_le_card this).trans (by simp [Finset.card_le_two])

theorem total_boundary_points_covered_by_at_most_2n_h1 (n k :  $\mathbb{N}$ )
  (verts : Finset  $\kappa$ )
  (lines : Finset ( $\kappa \times \kappa$ ))
  (points : Finset ( $\mathbb{N} \times \mathbb{N}$ ))
  (hn : 3 ≤ n)
  (hcard : lines.card + verts.card = n)
  (hallpoints :  $\forall p, p \in$  points → p.1 ≥ 1 ∧ p.2 ≥ 1 ∧ p.1 + p.2 ≤ n + 1)
  (hmain :  $\forall p \in$  points, ( $\exists l \in$  lines,  $l.1 * p.1 + l.2 = p.2$ ) ∨ ( $\exists x \in$  verts,
    → p.1 = x))
  (hk : (lines.filter (fun l => l.1 ≠ 0 ∧ l.1 ≠ -1)).card = k)
  (h_not_v1 : 1  $\notin$  verts)
  (h_not_y1 :  $\forall l \in$  lines,  $-(l.1 = 0 \wedge l.2 = 1)$ )
  (h_not_xn1 :  $\forall l \in$  lines,  $-(l.1 = -1 \wedge l.2 = n + 1)$ ):
   $\forall l \in$  lines,  $-(l.1 = 0 \wedge l.2 = 1) \wedge -(l.1 = -1 \wedge l.2 = n + 1)$  := by
  tauto

theorem total_boundary_points_covered_by_at_most_2n_h2 (n k :  $\mathbb{N}$ )
  (verts : Finset  $\kappa$ )
  (lines : Finset ( $\kappa \times \kappa$ ))
  (points : Finset ( $\mathbb{N} \times \mathbb{N}$ ))
  (hn : 3 ≤ n)
  (hcard : lines.card + verts.card = n)
  (hallpoints :  $\forall p, p \in$  points → p.1 ≥ 1 ∧ p.2 ≥ 1 ∧ p.1 + p.2 ≤ n + 1)
  (hmain :  $\forall p \in$  points, ( $\exists l \in$  lines,  $l.1 * p.1 + l.2 = p.2$ ) ∨ ( $\exists x \in$  verts,
    → p.1 = x))
  (hk : (lines.filter (fun l => l.1 ≠ 0 ∧ l.1 ≠ -1)).card = k)
  (h_not_v1 : 1  $\notin$  verts)
  (h_not_y1 :  $\forall l \in$  lines,  $-(l.1 = 0 \wedge l.2 = 1)$ )
  (h_not_xn1 :  $\forall l \in$  lines,  $-(l.1 = -1 \wedge l.2 = n + 1)$ )
  (h1 :  $\forall l \in$  lines,  $-(l.1 = 0 \wedge l.2 = 1) \wedge -(l.1 = -1 \wedge l.2 = n + 1)$ ):
   $\forall l \in$  lines, (Finset.filter (fun p => (p.1 = 1 ∨ p.2 = 1 ∨ p.1 + p.2 = n + 1)
    → (l.1 * p.1 + l.2 = p.2)) points).card ≤ 2 := by
  intros
  apply line_not_boundary_covers_at_most_2_boundary_points
  all_goals
    tauto

theorem total_boundary_points_covered_by_at_most_2n_h3 (n k :  $\mathbb{N}$ )
  (verts : Finset  $\kappa$ )
  (lines : Finset ( $\kappa \times \kappa$ ))
  (points : Finset ( $\mathbb{N} \times \mathbb{N}$ ))
  (h_not_v1 : 1  $\notin$  verts):
   $\forall x \in$  verts,  $x \neq 1$  := by
  aesop

theorem total_boundary_points_covered_by_at_most_2n_h4 (n k :  $\mathbb{N}$ )
  (verts : Finset  $\kappa$ )
  (lines : Finset ( $\kappa \times \kappa$ ))
  (points : Finset ( $\mathbb{N} \times \mathbb{N}$ ))
  (hn : 3 ≤ n)
  (hcard : lines.card + verts.card = n)
  (hallpoints :  $\forall p, p \in$  points → p.1 ≥ 1 ∧ p.2 ≥ 1 ∧ p.1 + p.2 ≤ n + 1)
  (hmain :  $\forall p \in$  points, ( $\exists l \in$  lines,  $l.1 * p.1 + l.2 = p.2$ ) ∨ ( $\exists x \in$  verts,
    → p.1 = x))
  (hk : (lines.filter (fun l => l.1 ≠ 0 ∧ l.1 ≠ -1)).card = k)
  (h_not_v1 : 1  $\notin$  verts)
  (h_not_y1 :  $\forall l \in$  lines,  $-(l.1 = 0 \wedge l.2 = 1)$ )
  (h_not_xn1 :  $\forall l \in$  lines,  $-(l.1 = -1 \wedge l.2 = n + 1)$ )
  (h2 :  $\forall l \in$  lines, (Finset.filter (fun p => (p.1 = 1 ∨ p.2 = 1 ∨ p.1 + p.2 =
    → n + 1) ∧ (l.1 * p.1 + l.2 = p.2)) points).card ≤ 2)
  (h4 :  $\forall x \in$  verts, (Finset.filter (fun p :  $\mathbb{N} \times \mathbb{N}$  => p.1 ≥ 1 ∧ p.2 ≥ 1 ∧ p.1 +
    → p.2 = n + 1 ∧ ((p.1 = 1 ∨ p.2 = 1 ∨ p.1 + p.2 = n + 1) ∧ (p.1 = x))
    → points).card ≤ 2):
  (Finset.filter (fun p => p.1 = 1 ∨ p.2 = 1 ∨ p.1 + p.2 = n + 1) points).card ≤
    2 * n := by
  let a := Finset.biUnion lines (fun l => Finset.filter (fun p => (p.1 = 1 ∨
    → p.2 = 1 ∨ p.1 + p.2 = n + 1) ∧ (l.1 * p.1 + l.2 = p.2)) points)
  let b := Finset.biUnion verts (fun x => Finset.filter (fun p => p.1 ≥ 1 ∧
    → p.2 = 1 ∨ p.1 + p.2 = n + 1 ∧ (p.1 = 1 ∨ p.2 = 1 ∨ p.1 + p.2 = n + 1) ∧
    → p.1 = x) points)
  calc
    (Finset.filter (fun p => p.1 = 1 ∨ p.2 = 1 ∨ p.1 + p.2 = n + 1) points).card
      ≤ (a ∪ b).card := Finset.card_le_card fun p hp => by aesop
      ≤ a.card + b.card := Finset.card_union_le _ _
      ≤ 2 * lines.card + 2 * verts.card := by
        simp [mul_comm] using
          Nat.add_le_add
        (Finset.card.biUnion_le.trans (Finset.sum_le_sum h2))
        (Finset.card.biUnion_le.trans (Finset.sum_le_sum h4))
      = 2 * (lines.card + verts.card) := by ring
      = 2 * n := by linarith

theorem total_boundary_points_covered_by_at_most_2n (n k :  $\mathbb{N}$ ) (verts : Finset  $\kappa$ 
  → ) (lines : Finset ( $\kappa \times \kappa$ )) (points : Finset ( $\mathbb{N} \times \mathbb{N}$ )) (hn : 3 ≤ n)
  → (hcard : lines.card + verts.card = n) (hallpoints :  $\forall p, p \in$  points →
  → p.1 ≥ 1 ∧ p.2 ≥ 1 ∧ p.1 + p.2 ≤ n + 1) (hmain :  $\forall p \in$  points, ( $\exists l \in$ 
  → lines,  $l.1 * p.1 + l.2 = p.2$ ) ∨ ( $\exists x \in$  verts,  $p.1 = x$ )) (hk :
  → (lines.filter (fun l => l.1 ≠ 0 ∧ l.1 ≠ -1)).card = k) (h_not_v1 : 1  $\notin$ 
  → verts) (h_not_y1 :  $\forall l \in$  lines,  $-(l.1 = 0 \wedge l.2 = 1)$ ) (h_not_xn1 :  $\forall l \in$ 
  → lines,  $-(l.1 = -1 \wedge l.2 = n + 1)$ ) : (Finset.filter (fun p => p.1 =
  → 1 ∨ p.2 = 1 ∨ p.1 + p.2 = n + 1) points).card ≤ 2 * n := by
  apply total_boundary_points_covered_by_at_most_2n_h_main n k verts lines
  → points hn hcard hallpoints hmain hk h_not_v1 h_not_y1 h_not_xn1
  apply total_boundary_points_covered_by_at_most_2n_h2 n k verts lines points
  → hn hcard hallpoints hmain hk h_not_v1 h_not_y1 h_not_xn1
  aesop
  apply total_boundary_points_covered_by_at_most_2n_h4 n k verts lines points
  → hn hcard hallpoints hmain hk h_not_v1
  aesop

theorem boundary_line_exists_at_any_cover_simplified_h_main (n :  $\mathbb{N}$ )
  (verts : Finset  $\kappa$ )
  (lines : Finset ( $\kappa \times \kappa$ ))
  (points : Finset ( $\mathbb{N} \times \mathbb{N}$ ))
  (hn : 4 ≤ n)
  (hcard : lines.card + verts.card = n)
  (hallpoints :  $\forall p, p \in$  points → p.1 ≥ 1 ∧ p.2 ≥ 1 ∧ p.1 + p.2 ≤ n + 1)
  (hmain :  $\forall p \in$  points, ( $\exists l \in$  lines,  $l.1 * p.1 + l.2 = p.2$ ) ∨ ( $\exists x \in$  verts,
    → p.1 = x)):
  ( $\exists x \in$  verts,  $x = 1$ ) ∨ ( $\exists l \in$  lines,  $(l.1 = 0 \wedge l.2 = 1) \vee (l.1 = -1 \wedge l.2 = n$ 
  → + 1)) := by
  by_contra h_neg
  have h1 := num_points_on_boundary n points hallpoints
  have h2 := total_boundary_points_covered_by_at_most_2n n (lines.filter (fun
    → l => l.1 ≠ 0 ∧ l.1 ≠ -1)).card verts lines points (by omega) hcard
  → hallpoints hmain rfi (by simp_all) (fun l hl h_not_y1 => h_neg
    → (Or.inr l, hl, Or.inl h_not_y1)) (fun l hl h_not_xn1 => h_neg
    → (Or.inr l, hl, Or.inr h_not_xn1))
  have h3 : n ≠ 1 := by omega
  simp_all
  <|> omega

theorem boundary_line_exists_at_any_cover_simplified (n :  $\mathbb{N}$ ) (verts : Finset  $\kappa$ 
  → ) (lines : Finset ( $\kappa \times \kappa$ )) (points : Finset ( $\mathbb{N} \times \mathbb{N}$ ))
  (hn : 4 ≤ n)
  (hcard : lines.card + verts.card = n)
  (hallpoints :  $\forall p, p \in$  points → p.1 ≥ 1 ∧ p.2 ≥ 1 ∧ p.1 + p.2 ≤ n + 1)
  (hmain :  $\forall p \in$  points, ( $\exists l \in$  lines,  $l.1 * p.1 + l.2 = p.2$ ) ∨ ( $\exists x \in$  verts,
    → p.1 = x)):
  ( $\exists x \in$  verts,  $x = 1$ ) ∨ ( $\exists l \in$  lines,  $(l.1 = 0 \wedge l.2 = 1) \vee (l.1 = -1 \wedge l.2 = n$ 
  → + 1)) := by
  apply boundary_line_exists_at_any_cover_simplified_h_main
  <|> assumption

theorem round1_main (n k :  $\mathbb{N}$ ) (verts : Finset  $\kappa$ ) (lines : Finset ( $\kappa \times \kappa$ ))
  → (points : Finset ( $\mathbb{N} \times \mathbb{N}$ )) (hn : 3 ≤ n) (hcard : lines.card +
  → verts.card = n) (hallpoints :  $\forall p, p \in$  points → p.1 ≥ 1 ∧ p.2 ≥ 1 ∧
  → p.1 + p.2 ≤ n + 1) (hmain :  $\forall p \in$  points, ( $\exists l \in$  lines,  $l.1 * p.1 +$ 
  → l.2 = p.2) ∨ ( $\exists x \in$  verts,  $p.1 = x$ )) (hk : (lines.filter (fun l => l.1
  → ≠ 0 ∧ l.1 ≠ -1)).card = k) : k = 0 ∨ k = 1 ∨ k = 3 := by

```

```

have h : ∀ n : ℕ, 3 ≤ n → ∀ k : ℕ, ∀ (verts : Finset ℝ) (lines : Finset (ℝ × ℝ
→ )) (points : Finset (ℕ × ℕ)),
(hcard : lines.card + verts.card = n) →
(hallpoints : ∀ p, p ∈ points → p.1 ≥ 1 ∧ p.2 ≥ 1 ∧ p.1 + p.2 ≤ n + 1) →
(hmain : ∀ p ∈ points, (∃ l ∈ lines, l.1 * p.1 + l.2 = p.2) ∨ (∃ x ∈ verts,
→ p.1 = x))
(hk : (lines.filter (fun l → l.1 ≠ 0 ∧ l.1 ≠ -1)).card = k) →
k = 0 ∨ k = 1 ∨ k = 3 := by
intro n
induction n using Nat.strong_induction_on with
| h n ih =>
  intro hn3 k verts lines points hcard hallpoints hmain hk
  by_cases h1 : n = 3
  · subst h1
    exact imo2025_p1_prop_n_eq_3_k_eq_0_1_3 k lines verts points hcard
    → hallpoints hmain hk
  · have h2 : n ≥ 4 := by omega
    have h4 := boundary_line_exists_at_any_cover_simplified n verts lines
    → points h2 hcard hallpoints hmain
    have hcover : ∀ p : ℕ × ℕ, p.1 ≥ 1 ∧ p.2 ≥ 1 ∧ p.1 + p.2 ≤ n + 1 →
    (∃ l ∈ lines, l.1 * (p.1 : ℝ) + l.2 = (p.2 : ℝ)) ∨ (∃ x ∈ verts, (p.1 : ℝ
    → ) = x) := by
      intro p hp
      exact hmain p (by aesop)
    have h_1h : ∀ (k' : ℕ) (verts' : Finset ℝ) (lines' : Finset (ℝ × ℝ)),
    (verts'.card + lines'.card = n - 1) →
    (∀ p : ℕ × ℕ, p.1 ≥ 1 ∧ p.2 ≥ 1 ∧ p.1 + p.2 ≤ n →
    (∃ l ∈ lines', l.1 * (p.1 : ℝ) + l.2 = (p.2 : ℝ)) ∨ (∃ x ∈ verts',
    → (p.1 : ℝ) = x)) →
    ((lines'.filter (fun l → l.1 ≠ 0 ∧ l.1 ≠ -1)).card = k') →
    k' = 0 ∨ k' = 1 ∨ k' = 3 := by
      intro k' verts' lines' h13 h14 h15
      set points' : Finset (ℕ × ℕ) := (Finset.Ico 1 (n + 1) × Finset.Ico 1
      → (n + 1)).filter (fun p => p.1 + p.2 ≤ n) with h18
      have h19 : ∀ p : ℕ × ℕ, p ∈ points' → p.1 ≥ 1 ∧ p.2 ≥ 1 ∧ p.1 + p.2 ≤ n
      := by
        intro p
        simp [h18, Finset.mem_filter, Finset.mem_Ico]
        <|> omega
      have h20 : ∀ p ∈ points', (∃ l ∈ lines', l.1 * p.1 + l.2 = p.2) ∨ (∃ x ∈
      → verts', p.1 = x) := by
        intro p hp
        have h21 : p.1 ≥ 1 ∧ p.2 ≥ 1 ∧ p.1 + p.2 ≤ n := by
          rw [h19 p] at hp
          tauto
        have h22 := h14 p h21
        simp using h22
      have h23 : lines'.card + verts'.card = n - 1 := by
        linarith
      have h24 : ∀ p, p ∈ points' → p.1 ≥ 1 ∧ p.2 ≥ 1 ∧ p.1 + p.2 ≤ (n - 1) +
      → 1 := by
        intro p
        have h25 : (n - 1) + 1 = n := by omega
        rw [h25]
      exact h19 p
      have h26 := ih (n - 1) (by omega) (by omega) k' verts' lines' points'
      → h23 h24 h20 h15
      tauto
    rcases h4 with h41 | h42
    · exact inductive_step_if_contains_vertical_line n k verts lines points
    → hcard hallpoints hmain hk (by linarith) hcover h41 h_1h
    rcases h42 with (l, hl_in_lines, h421 | h4212)
    · have h4211 : ∃ l' ∈ lines, l'.1 = 0 ∧ l'.2 = 1 := (l, hl_in_lines, by
    → tauto)
    exact inductive_step_if_contains_horizontal_line n k verts lines
    → points hcard hallpoints hmain hk (by linarith) hcover h4211 h_1h
    · have h4212 : ∃ l' ∈ lines, l'.1 = -1 ∧ l'.2 = (n : ℝ) + 1 := (l,
    → hl_in_lines, by tauto)
    exact inductive_step_if_contains_rainy_diagonal_line_refined n k verts
    → lines points (by linarith) hcard hallpoints hmain hk (by linarith)
    → hcover h4212 h_1h
  exact h n hn k verts lines points hcard hallpoints hmain hk

theorem imo2025_p1_left (n k : ℕ) (verts : Finset ℝ) (lines : Finset (ℝ × ℝ))
→ (points : Finset (ℕ × ℕ)) (hn : 3 ≤ n) (hcard : lines.card +
→ verts.card = n) (hallpoints : ∀ p, p ∈ points → p.1 ≥ 1 ∧ p.2 ≥ 1 ∧
→ p.1 + p.2 ≤ n + 1) (hmain : ∀ p ∈ points, (∃ l ∈ lines, l.1 * p.1 +
→ l.2 = p.2) ∨ (∃ x ∈ verts, p.1 = x)) (hk : (lines.filter (fun l → l.1
→ ≠ 0 ∧ l.1 ≠ -1)).card = k) : k = 0 ∨ k = 1 ∨ k = 3 := by
  apply round1_main
  <|> assumption

theorem round3_k3_card (n : ℕ) (hn : 3 ≤ n) :
(((-1 / 2, 1 + (n : ℝ) / 2), (1, 3 - (n : ℝ))), (-2, 2 * (n : ℝ) - 1)) :
→ Finset (ℝ × ℝ)).card = 3 := by
  norm_num

theorem round3_k1_third_cond (n : ℕ) (hn : 3 ≤ n) :
(Finset.filter (fun l => l.1 ≠ 0 ∧ l.1 ≠ -1) ({(1, 1 - (n : ℝ))} : Finset (ℝ ×
→ ℝ))).card = 1 := by
  norm_num [Finset.filter_singleton]

theorem round3_k3_third_cond (n : ℕ) (hn : 3 ≤ n) :
(Finset.filter (fun l => l.1 ≠ 0 ∧ l.1 ≠ -1) ({(-1 / 2, 1 + (n : ℝ) / 2), (1,
→ 3 - (n : ℝ)), (-2, 2 * (n : ℝ) - 1)} : Finset (ℝ × ℝ))).card = 3 := by
  norm_num [Finset.filter_true_of_mem]

theorem imo2025_p1_right (n k : ℕ) (hn : 3 ≤ n) (hk : k = 0 ∨ k = 1 ∨ k = 3) : ∃
→ lines : Finset (ℝ × ℝ), ∃ xs : Finset ℝ, lines.card + xs.card = n ∧
→ (∀ a b : ℕ, a > 0 → b > 0 → a + b ≤ n + 1 → (∃ l ∈ lines, l.1 * a +
→ l.2 = b) ∨ (∃ x ∈ xs, a = x)) ∧ (lines.filter (fun l → l.1 ≠ 0 ∧ l.1 ≠
→ -1)).card = k := by
  rcases hk with (rfl | rfl | rfl)
  use 0
  use (Finset.range n).image (fun (i : ℕ) => (i + 1 : ℝ))
  constructor
  simp [Finset.card_image_of_injective, Function.Injective]
  constructor
  intro a b ha_pos hb_pos hab
  exact Or.inr (a, Finset.mem_image.mpr (a - 1, Finset.mem_range.mpr (by
  → omega), by simp [ha_pos], by simp))

simp
use {(1, 1 - (n : ℝ))}
use (Finset.range (n - 1)).image (fun (i : ℕ) => (i + 1 : ℝ))
constructor

have h21 : ((Finset.range (n - 1)).image (fun (i : ℕ) => (i + 1 : ℝ))).card =
→ n - 1 := by
  simp [Finset.card_image_of_injective, Function.Injective]
have h22 : ({(1, 1 - (n : ℝ))} : Finset (ℝ × ℝ)).card = 1 := by simp
omega
constructor
intro a b ha_pos hb_pos hab
by_cases h17 : a ≤ n - 1
· have h171 : a ≤ n - 1 := h17
  have h172 : a ≥ 1 := by linarith
  have h173 : a - 1 < n - 1 := by omega
  have h174 : (a - 1) ∈ Finset.range (n - 1) := Finset.mem_range.mpr h173
  have h175 : ((a - 1 : ℕ) : ℝ) + 1 ∈ (Finset.range (n - 1)).image (fun (i :
  → ℕ) => (i + 1 : ℝ)) := by
    refine Finset.mem_image.mpr ((a - 1), h174, by simp)
  have h176 : ((a - 1 : ℕ) : ℝ) + 1 = (a : ℝ) := by simp [Nat.cast_sub (by
  → omega : 0 < a)]
  have h177 : (a : ℝ) ∈ (Finset.range (n - 1)).image (fun (i : ℕ) => (i + 1
  → : ℝ)) := by
    rw [h176] at h175
    exact h175
  refine Or.inr ((a : ℝ), h177, by simp)
· have h177 : a > n - 1 := by omega
  have h180 : a = n := by omega
  have h181 : b = 1 := by omega
  refine Or.inl ((1, 1 - (n : ℝ)), by simp, ?_)
  simp [h180, h181]
exact round3_k1_third_cond n hn
use ({(-1 / 2, 1 + (n : ℝ) / 2), (1, 3 - (n : ℝ)), (-2, 2 * (n : ℝ) - 1)} :
→ Finset (ℝ × ℝ))
use (Finset.range (n - 3)).image (fun (i : ℕ) => (i + 1 : ℝ))
constructor
have h21 : ((Finset.range (n - 3)).image (fun (i : ℕ) => (i + 1 : ℝ))).card =
→ n - 3 := by
  simp [Finset.card_image_of_injective, Function.Injective]
have h22 : ({(1, 1 - (n : ℝ) / 2, 1 + (n : ℝ) / 2), (1, 3 - (n : ℝ)), (-2, 2 * (n : ℝ)
→ - 1)} : Finset (ℝ × ℝ)).card = 3 := by
  norm_num
omega
constructor
intro a b ha_pos hb_pos hab
by_cases h17 : a ≤ n - 3
· have h171 : a ≤ n - 3 := h17
  have h172 : a ≥ 1 := by linarith
  have h173 : a - 1 < n - 3 := by omega
  have h174 : (a - 1) ∈ Finset.range (n - 3) := Finset.mem_range.mpr h173
  have h175 : ((a - 1 : ℕ) : ℝ) + 1 ∈ (Finset.range (n - 3)).image (fun (i :
  → ℕ) => (i + 1 : ℝ)) := by
    refine Finset.mem_image.mpr ((a - 1), h174, by simp)
  have h176 : ((a - 1 : ℕ) : ℝ) + 1 = (a : ℝ) := by simp [Nat.cast_sub (by
  → omega : 0 < a)]
  have h177 : (a : ℝ) ∈ (Finset.range (n - 3)).image (fun (i : ℕ) => (i + 1
  → : ℝ)) := by
    rw [h176] at h175
    exact h175
  refine Or.inr ((a : ℝ), h177, by simp)
· have h177 : a > n - 3 := by omega
  have h178 : a = n - 2 := by omega
  have h179 : a ≤ n := by omega
  have h180 : a = n - 2 ∨ a = n - 1 ∨ a = n := by omega
  rcases h180 with (h180 | h180 | h180)
  · have h1801 : a = n - 2 := h180
    have h181 : b ≤ 3 := by omega
    have h182 : b ≥ 1 := by linarith
    have h183 : b = 1 ∨ b = 2 ∨ b = 3 := by omega
    rcases h183 with (h183 | h183 | h183)
    refine Or.inl ((1, 3 - (n : ℝ)), by simp, ?_)
    simp [h1801, h183]
    <|> ring_nf <|> simp [Nat.cast_sub (show 2 ≤ n by omega)] <|> ring_nf
  · refine Or.inl ((-1 / 2, 1 + (n : ℝ) / 2), by simp, ?_)
    simp [h1801, h183]
    <|> ring_nf <|> norm_num <|> simp [Nat.cast_sub (show 2 ≤ n by omega)]
    <|> ring_nf
  · refine Or.inl ((-2, 2 * (n : ℝ) - 1), by simp, ?_)
    simp [h1801, h183]
    <|> ring_nf <|> simp [Nat.cast_sub (show 2 ≤ n by omega)] <|> ring_nf
  · have h1802 : a = n - 1 := h180
    have h181 : b ≤ 1 := by omega
    have h182 : b ≥ 1 := by linarith
    have h183 : b = 1 := by omega
    refine Or.inl ((-1 / 2, 1 + (n : ℝ) / 2), by simp, ?_)
    simp [h1803, h183]
    <|> ring_nf
  simp
  exact round3_k3_third_cond n hn
-- P3
import Mathlib
import aesop
set_option pp.numericTypes true
set_option pp.funBinderTypes true
set_option maxHeartbeats 0
set_option maxRecDepth 1000
set_option tactic.hygienic false
open BigOperators Real Nat Topology Rat Classical Polynomial

theorem round1_h1 (n : ℤ)
(k : ℕ)
(hn : n > 0)
(h_k_le_2_plus_padic : k ≤ 2 + pAdicValNat 2 n.toNat) :
(2 : ℤ) ^ k ≤ (2 : ℤ) ^ (2 + pAdicValNat 2 n.toNat) := by
  gcongr
  linarith

theorem round1_h2 (n : ℤ)

```



```

(k : ℕ)
(hn : n > 0) :
(2 : z) ^ (2 + padicValNat 2 n.toNat) = 4 * (2 : z) ^ (padicValNat 2
  → n.toNat) := by
  ring_nf

theorem round1_h3 (n : z)
(k : ℕ)
(hn : n > 0)
(h1 : (2 : z) ^ k ≤ (2 : z) ^ (2 + padicValNat 2 n.toNat))
(h2 : (2 : z) ^ (2 + padicValNat 2 n.toNat) = 4 * (2 : z) ^ (padicValNat 2
  → n.toNat)) :
(2 : z) ^ k ≤ 4 * (2 : z) ^ (padicValNat 2 n.toNat) := by
  linarith

theorem round1_h4 (n : z)
(k : ℕ)
(hn : n > 0) :
(2 : z) ^ (padicValNat 2 n.toNat) | n := by
have h4 : (2 : ℕ) ^ (padicValNat 2 n.toNat) | n.toNat := by
  apply pow_padicValNat_dvd
have h4 : (2 : z) ^ (padicValNat 2 n.toNat) | (n.toNat : z) := by
  exact_mod_cast h4
have h4 : (n.toNat : z) = n := by
  simp [hn]
  <|> omega
rw [h4] at h4,
exact h4

theorem round1_h5 (n : z)
(k : ℕ)
(hn : n > 0)
(h4 : (2 : z) ^ (padicValNat 2 n.toNat) | n) :
(2 : z) ^ (padicValNat 2 n.toNat) ≤ n := by
  apply Int.le_of_dvd hn h4

theorem round1_h6 (n : z)
(k : ℕ)
(hn : n > 0)
(h5 : (2 : z) ^ (padicValNat 2 n.toNat) ≤ n) :
4 * (2 : z) ^ (padicValNat 2 n.toNat) ≤ 4 * n := by
  linarith

theorem round1_h7 (n : z)
(k : ℕ)
(hn : n > 0)
(h3 : (2 : z) ^ k ≤ 4 * (2 : z) ^ (padicValNat 2 n.toNat))
(h6 : 4 * (2 : z) ^ (padicValNat 2 n.toNat) ≤ 4 * n) :
(2 : z) ^ k ≤ 4 * n := by
  linarith

theorem round1_h_main (n : z)
(f : z → z)
(k : ℕ)
(hn : n > 0)
(hk : f n = (2 : z) ^ k)
(h7 : (2 : z) ^ k ≤ 4 * n) :
f n ≤ 4 * n := by
  simp_all

theorem round1_h6' (n : z) (f : z → z) (hn : n > 0) (hpos : ∀ k : z, k > 0 → f
  → k > 0) (hf : ∀ a b : z, a > 0 → b > 0 → f a | b ^ a.toNat - (f b) ^
  → (f a).toNat) (k : ℕ) (hk : f n = (2 : z) ^ k) (h_k_le_2_plus_padic :
  → k ≤ 2 + padicValNat 2 n.toNat) : f n ≤ 4 * n := by
  rw [hk]
  apply round1_h7 n k hn
  apply round1_h3 n k hn
  apply round1_h1 n k hn h_k_le_2_plus_padic
  apply round1_h2 n k hn
  apply round1_h6 n k hn
  apply round1_h5 n k hn
  apply round1_h4 n k hn

theorem lte_2_3n_minus_1_h1 :
∀ k : ℕ, k > 0 → k % 2 = 1 → 3 ^ k % 4 = 3 := by
  intros
  rw [- Nat.mod_add_div k 2]
  simp_all [pow_add, pow_mul, Nat.mul_mod, Nat.pow_mod]

theorem lte_2_3n_minus_1_h4 :
∀ k : ℕ, k > 0 → k % 2 = 0 → 3 ^ k % 4 = 1 := by
  intros
  rw [- Nat.mod_add_div k 2]
  simp_all [Nat.pow_mod, Nat.pow_mul]

theorem lte_2_3n_minus_1_h3_pow_mod_8 :
∀ m : ℕ, m > 0 → m % 2 = 1 → 3 ^ m % 8 = 3 := by
  intros
  rw [- Nat.mod_add_div m 2]
  simp_all [pow_add, pow_mul, Nat.mul_mod, Nat.pow_mod]

theorem lte_2_3n_minus_1_h_padicValNat_mul (p : ℕ) [Fact p.Prime] (a b : ℕ)
  → (ha : a ≠ 0) (hb : b ≠ 0) :
padicValNat p (a * b) = padicValNat p a + padicValNat p b := by
  apply padicValNat.mul
  assumption

theorem lte_2_3n_minus_1_general_lemma_A (x : ℕ) (h1 : 2 | x) (h2 : ~ 4 | x) :
  → padicValNat 2 x = 1 := by
  cases' h1 with y
  cases y
  all_goals simp_all [padicValNat.mul]
  all_goals omega

theorem lte_2_3n_minus_1_general_lemma_B (x : ℕ) (h1 : 4 | x) (h2 : ~ 8 | x) :
  → padicValNat 2 x = 2 := by
  rw [show x = 2 * 2 * (x / 4) by omega]
  repeat' rw [padicValNat.mul]
  all_goals norm_num
  all_goals omega

theorem lte_2_3n_minus_1_lemma1 (k : ℕ) (hk_pos : k > 0) (hk_odd : k % 2 = 1)
  → : padicValNat 2 (3 ^ k - 1) = 1 := by
  apply lte_2_3n_minus_1_general_lemma_A
  all_goals
    rw [- Nat.mod_add_div (3 ^ k) 4]

simp_all [lte_2_3n_minus_1_h1]
omega

theorem lte_2_3n_minus_1_lemma2 (k : ℕ) (hk_pos : k > 0) (hk_even : k % 2 = 0)
  → : padicValNat 2 (3 ^ k - 1) = 2 + padicValNat 2 k := by
  obtain m, rfl := Nat.dvd_iff_mod_eq_zero.mpr hk_even
  have hm_pos : m > 0 := by omega
  by_cases h3 : m % 2 = 1
  · have h4 : 3 ^ m % 8 = 3 := by
      apply lte_2_3n_minus_1_h3_pow_mod_8
      omega
    exact h3
  have h5 : 2 | (3 ^ m - 1) := by omega
  have h6 : ~ 4 | (3 ^ m - 1) := by
    intro h71
    have h72 : (3 ^ m - 1) % 4 = 0 := by omega
    have h31 : m > 0 := hm_pos
    have h32 : 3 ^ m ≥ 3 ^ 1 := by
      exact Nat.pow_le_pow_of_le_right (by norm_num) (by omega)
    omega
  have h7 : padicValNat 2 (3 ^ m - 1) = 1 := by
    apply lte_2_3n_minus_1_general_lemma_A
    exact h5
    exact h6
  have h8 : 4 | (3 ^ m + 1) := by omega
  have h9 : ~ 8 | (3 ^ m + 1) := by omega
  have h10 : padicValNat 2 (3 ^ m + 1) = 2 := by
    apply lte_2_3n_minus_1_general_lemma_B
    exact h8
    exact h9
  have h11 : 3 ^ (2 * m) - 1 = (3 ^ m - 1) * (3 ^ m + 1) := by
    have h111 : 3 ^ m ≥ 1 := by omega
    have h112 : 3 ^ (2 * m) = (3 ^ m) ^ 2 := by ring
    rw [h112]
    have h113 : (3 ^ m) ^ 2 = (3 ^ m) * (3 ^ m) := by ring
    rw [h113]
    cases' le_iff_exists_add.mp (by omega : 1 ≤ 3 ^ m) with x hx
    simp [hx, Nat.mul_add, Nat.add_mul, Nat.add_assoc] <|> ring_nf at *
  have h12 : padicValNat 2 ((3 ^ m - 1) * (3 ^ m + 1)) = padicValNat 2 (3 ^
    → m - 1) + padicValNat 2 (3 ^ m + 1) := by
    apply lte_2_3n_minus_1_h_padicValNat_mul
    omega
    omega
  have h13 : padicValNat 2 (3 ^ (2 * m) - 1) = padicValNat 2 (3 ^ m - 1) +
    → padicValNat 2 (3 ^ m + 1) := by
    rw [h12] at *
    exact h12
  have h14 : padicValNat 2 (3 ^ (2 * m) - 1) = 1 + 2 := by linarith
  have h15 : padicValNat 2 (3 ^ (2 * m) - 1) = 3 := by linarith
  have h16 : 2 | (2 * m) := by omega
  have h17 : ~ 4 | (2 * m) := by omega
  have h18 : padicValNat 2 (2 * m) = 1 := by
    apply lte_2_3n_minus_1_general_lemma_A
    exact h16
    exact h17
  linarith
  · have h4 : t, m = 2 * t := by
      refine m / 2, 7_
    omega
    rcases h4 with (t, h4t)
    have ht_pos : t > 0 := by omega
    have hm_even : m % 2 = 0 := by omega
    have h5 : m < 2 * m := by linarith
    have h_m : padicValNat 2 (3 ^ m - 1) = 2 + padicValNat 2 m := by
      exact lte_2_3n_minus_1_lemma2 m (by omega) (by omega)
    have h6 : 3 ^ m % 4 = 1 := by
      apply lte_2_3n_minus_1_h4
      exact hm_pos
      exact hm_even
    have h7 : 2 | (3 ^ m + 1) := by omega
    have h8 : ~ 4 | (3 ^ m + 1) := by omega
    have h9 : padicValNat 2 (3 ^ m + 1) = 1 := by
      apply lte_2_3n_minus_1_general_lemma_A
      exact h7
      exact h8
    have h10 : 3 ^ m - 1 > 0 := by
      have h101 : m > 0 := by omega
      have h102 : 3 ^ m ≥ 3 ^ 1 := by
        exact Nat.pow_le_pow_of_le_right (by norm_num) (by omega)
      omega
    have h11 : 3 ^ m + 1 > 0 := by positivity
    have h12 : 3 ^ (2 * m) - 1 = (3 ^ m - 1) * (3 ^ m + 1) := by
      have h121 : 3 ^ m ≥ 1 := by omega
      have h122 : 3 ^ (2 * m) = (3 ^ m) ^ 2 := by ring
      rw [h122]
      have h123 : (3 ^ m) ^ 2 = (3 ^ m) * (3 ^ m) := by ring
      rw [h123]
      cases' le_iff_exists_add.mp (by omega : 1 ≤ 3 ^ m) with x hx
      simp [hx, Nat.mul_add, Nat.add_mul, Nat.add_assoc] <|> ring_nf at *
    have h13 : padicValNat 2 ((3 ^ m - 1) * (3 ^ m + 1)) = padicValNat 2 (3 ^
      → m - 1) + padicValNat 2 (3 ^ m + 1) := by
      apply lte_2_3n_minus_1_h_padicValNat_mul
      omega
      omega
    have h14 : padicValNat 2 (3 ^ (2 * m) - 1) = padicValNat 2 (3 ^ m - 1) +
      → padicValNat 2 (3 ^ m + 1) := by
      rw [h12] at *
      exact h13
    have h15 : padicValNat 2 (3 ^ (2 * m) - 1) = (2 + padicValNat 2 m) + 1 :=
      → by linarith
    have h16 : padicValNat 2 (3 ^ (2 * m) - 1) = 3 + padicValNat 2 m := by
      → linarith
    have h17 : m = 2 * t := by
      rw [h4t]
    have ht_pos' : t > 0 := by omega
    have h18 : padicValNat 2 m = padicValNat 2 (2 * t) := by
      rw [h17]
    have h19 : padicValNat 2 (2 * t) = 1 + padicValNat 2 t := by
      have h191 : padicValNat 2 2 = 1 := by norm_num
      have h192 : t > 0 := by linarith
      have h193 : padicValNat 2 (2 * t) = padicValNat 2 2 + padicValNat 2 t :=
        → by
      have h194 : (2 : ℕ) ≠ 0 := by norm_num
      have h195 : t ≠ 0 := by linarith
      exact lte_2_3n_minus_1_h_padicValNat_mul 2 2 t h194 h195

```

```

    rw [h193, h191]
    have h20 : padicValNat 2 m = 1 + padicValNat 2 t := by
      linarith
    have h21 : padicValNat 2 (3 ^ (2 * m) - 1) = 4 + padicValNat 2 t := by
      linarith
    have h22 : padicValNat 2 (2 * m) = 2 + padicValNat 2 t := by
      linarith
    have h221 : padicValNat 2 (2 * m) = padicValNat 2 (2 * (2 * t)) := by
      rw [h17]
    have h222 : padicValNat 2 (2 * (2 * t)) = padicValNat 2 2 + padicValNat
      → 2 (2 * t) := by
      have h223 : (2 : ℕ) ≠ 0 := by norm_num
      have h224 : 2 * t ≠ 0 := by linarith
      exact lte_2_3n_minus_1_h_padicValNat_mul 2 2 (2 * t) h223 h224
    have h223 : padicValNat 2 2 = 1 := by norm_num
    linarith
  linarith

theorem lte_2_3n_minus_1 (n : ℤ) (hn : n > 0) : padicValNat 2 (3 ^ n.toNat -
  → 1) = if n % 2 = 1 then 1 else 2 + padicValNat 2 n.toNat := by
  split_ifs
  apply lte_2_3n_minus_1_lemma1
  <|> omega
  apply lte_2_3n_minus_1_lemma2
  <|> omega

theorem round1_h_n_toNat_ge_one (n : ℤ)
  (hn : n > 0) :
  n.toNat ≥ 1 := by
  omega

theorem round1_h_pow_div (n : ℤ)
  (k : ℕ)
  (hn : n > 0)
  (h_2_pow_k_divides : (2 : ℤ) ^ k | 3 ^ n.toNat - 1)
  (h_n_toNat_ge_one : n.toNat ≥ 1) :
  2 ^ k | 3 ^ n.toNat - 1 := by
  apply Int.coe_nat_dvd.mp
  simp_all

theorem round1_h_main'' (n : ℤ)
  (k : ℕ)
  (hn : n > 0)
  (h_n_toNat_ge_one : n.toNat ≥ 1)
  (h_pow_div : 2 ^ k | 3 ^ n.toNat - 1) :
  k ≤ padicValNat 2 (3 ^ n.toNat - 1) := by
  simp_all [Nat.sub_eq_zero_iff_le, padicValNat_dvd_iff_le]

theorem round1_h_k_le_padic (n : ℤ)
  (f : ℤ → ℤ)
  (k : ℕ)
  (hn : n > 0)
  (hpos : ∀ k : ℤ, k > 0 → f k > 0)
  (hf : ∀ a b : ℤ, a > 0 → b > 0 → f a | b ^ a.toNat - (f b) ^ (f a).toNat)
  (h_2_pow_k_divides : (2 : ℤ) ^ k | 3 ^ n.toNat - 1) :
  k ≤ padicValNat 2 (3 ^ n.toNat - 1) := by
  apply round1_h_main''
  assumption
  omega
  apply round1_h_pow_div
  all_goals
  omega

theorem round1_main (f : ℤ → ℤ) (hpos : ∀ k : ℤ, k > 0 → f k > 0) (hf : ∀ a b :
  → ℤ, a > 0 → b > 0 → f a | b ^ a.toNat - (f b) ^ (f a).toNat) : f 1 = 1
  := by
  have h1 := hpos 1 (by norm_num)
  have h3 : f 1 | 1 := by
    have : f 1 | 1 ^ 1 - (f 1) ^ (f 1).toNat + (f 1) ^ (f 1).toNat := by
      apply Int.dvd_add
      · apply hf 1 1
      · all_goals norm_num
    · apply dvd_pow
    · exact dvd_refl (f 1)
    · omega
  simp_all
  exact Int.eq_one_of_dvd_one (by linarith) h3

theorem imo2025_p3_subproblem_f1_is_1_or_f1_is_const_1 (f : ℤ → ℤ) (hpos : ∀ k
  → ℤ, k > 0 → f k > 0) (hf : ∀ a b : ℤ, a > 0 → b > 0 → f a | b ^
  → a.toNat - (f b) ^ (f a).toNat) : (∀ k : ℤ, k > 0 → f k = 1) ∨ f 1 =
  → 1 := by
  simp_all [round1_main]

theorem round1_h_subcase1 (n : ℤ)
  (f : ℤ → ℤ)
  (hn : n > 0)
  (hpos : ∀ k : ℤ, k > 0 → f k > 0)
  (hf : ∀ a b : ℤ, a > 0 → b > 0 → f a | b ^ a.toNat - (f b) ^ (f a).toNat)
  (h_subcase1 : ∀ k : ℤ, k > 0 → f k = k) :
  f n ≤ 4 * n := by
  simp_all

theorem f_is_not_identity_implies_f_p_eq_1_for_p_gt_2_int_toNat_mul (a b : ℤ)
  → (ha : 0 ≤ a) (hb : 0 ≤ b) : (a * b).toNat = a.toNat * b.toNat := by
  apply Int.ofNat.inj
  simp_all [Int.toNat_of_nonneg, mul_nonneg]

theorem f_is_not_identity_implies_f_p_eq_1_for_p_gt_2_h64 (p : ℤ) (hp_nonneg :
  → 0 ≤ p) (k : ℕ) : (p : ℤ) ^ k = ((p.toNat) ^ k) := by
  simp_all

theorem f_is_not_identity_implies_f_p_eq_1_for_p_gt_2_divides_f_p_stronger
  → (n : ℤ) (f : ℤ → ℤ) (hn : n > 0) (hpos : ∀ k : ℤ, k > 0 → f k > 0)
  → (hf : ∀ a b : ℤ, a > 0 → b > 0 → f a | b ^ a.toNat - (f b) ^ (f
  → a).toNat) (p : ℤ) (hp : Nat.Prime p.toNat) (hfp_ne_1 : f p ≠ 1)
  → (hp_pos : p > 0) :
  ∃ j : ℕ, j ≥ 1 ∧ f p = p ^ j := by
  specialize hpos p hp_pos
  specialize hf p p hp_pos hp_pos
  have h323 : f p | (p ^ p.toNat - (f p) ^ (f p).toNat) + (f p) ^ (f p).toNat :=
    → by
    apply Int.dvd_add
    exact hf
    exact dvd_pow_self (f p) (by aesop)
  simp at h323
  obtain (c, hc) := h323

have h322 : p ^ p.toNat > 0 := by positivity
have hc_pos : c > 0 := by nlinarith
have h3251 : (p ^ p.toNat : ℤ).toNat = (f p : ℤ).toNat + (c : ℤ).toNat := by
  rw [hc]
  exact f_is_not_identity_implies_f_p_eq_1_for_p_gt_2_int_toNat_mul (f p) c
  → (by linarith) (by linarith)
have h326 : (f p : ℤ).toNat | (p ^ p.toNat : ℤ).toNat := by
  use (c : ℤ).toNat
have h324 : ∀ (k : ℕ), (p ^ k : ℤ).toNat = (p.toNat) ^ k := by
  intro k
  induction' k with k ih
  simp
  have h2 : p ^ k ≥ 0 := by positivity
  have h3 : (p ^ (k + 1) : ℤ) = p * (p ^ k) := by ring
  have h4 : (p ^ (k + 1) : ℤ) ≥ 0 := by positivity
  have h5 : ((p ^ (k + 1) : ℤ).toNat) = (p : ℤ).toNat * ((p ^ k : ℤ).toNat)
    → := by
    rw [h3]
    exact f_is_not_identity_implies_f_p_eq_1_for_p_gt_2_int_toNat_mul p (p
      → k) (by linarith) (by linarith)
  rw [h5]
  rw [ih]
  simp [pow_succ]
  <|> ring_nf
have h3241 : (p ^ p.toNat : ℤ).toNat = (p.toNat) ^ p.toNat := by
  specialize h324 (p.toNat)
  simp_all
have h323 : (f p : ℤ).toNat | (p.toNat) ^ p.toNat := by
  rw [h3241] at h326
  exact h326
have h325 : ∃ j : ℕ, j ≤ p.toNat ∧ (f p : ℤ).toNat = (p.toNat) ^ j := by
  exact (Nat.dvd_prime_pow hp).mp h323
rcases h325 with (j, hj1, hj2)
have h326 : j ≥ 1 := by
  by_contra h3261
  have h3262 : j = 0 := by omega
  rw [h3262] at hj2
  have h3263 : (f p : ℤ).toNat = 1 := by simp using hj2
  have h3264 : f p = 1 := by
    have h1 : 0 ≤ f p := by linarith
    omega
  contradiction
  refine (j, h326, 7)
have h3271 : (f p : ℤ).toNat = (p.toNat) ^ j := by
  have h2 : 0 ≤ f p := by linarith
  have h64 : ∀ (k : ℕ), (p : ℤ) ^ k = ((p.toNat) ^ k) := by
    intro k
    exact f_is_not_identity_implies_f_p_eq_1_for_p_gt_2_h64 p (by linarith) k
  have h3272 : f p = (p : ℤ) ^ j := by
    have h1 : (f p : ℤ).toNat = (p.toNat) ^ j := h3271
    have h22 : (f p) = ((f p : ℤ).toNat) := by simp [h2]
    have h23 : ((p : ℤ) ^ j) = ((p.toNat) ^ j) := by simp using h64 j
    have h24 : ((f p : ℤ).toNat) = ((p.toNat) ^ j) := by rw [h1]
  rw [h22, h24, h23]
  simp_all

theorem fermat_little_theorem_int_version (q : ℕ) (hq : Nat.Prime q) (x : ℤ) :
  → (q : ℤ) | x ^ q - x := by
  haveI := Fact.mk hq
  simp [-ZMod.intCast_zmod_eq_zero_iff_dvd]

theorem f_is_not_identity_implies_f_p_eq_1_for_p_gt_2_main_proof (n : ℤ) (f : ℤ
  → ℤ) (hn : n > 0) (hpos : ∀ k : ℤ, k > 0 → f k > 0) (hf : ∀ a b : ℤ,
  → a > 0 → b > 0 → f a | b ^ a.toNat - (f b) ^ (f a).toNat) (p : ℤ) (hp
  → : Nat.Prime p.toNat) (hfp_ne_1 : f p ≠ 1) (hp_pos : p > 0)
  → (h_f1_eq_1 : f 1 = 1) (h_p_divides_f_p_stronger : ∃ j : ℕ, j ≥ 1 ∧ f
  → p = p ^ j) :
  ∀ b : ℤ, b > 0 → b = f b [ZMOD p] := by
  have h13 : f p > 0 := hpos p (by linarith)
  have h_prime_p : Prime p := by
    have h1 : Nat.Prime p.toNat := hp
    have h2 : Prime (p.toNat : ℤ) := by exact prime_iff_prime_int.mp hp
    have h3 : (p.toNat : ℤ) = p := by
      simp [show 0 ≤ p by linarith]
    have h4 : Prime p := by
      rw [h3] at h2
      exact h2
    exact h4
  rcases h_p_divides_f_p_stronger with (j, hj_ge1, hj_eq)
  intro b hb
  have h19 : f p | b ^ p.toNat - (f b) ^ (f p).toNat := by
    specialize hf p b (by linarith) (by linarith)
    simp using hf
  have h21 : p | f p := by
    have h1 : f p = p ^ j := hj_eq
    have h_j_ge1 : j ≥ 1 := hj_ge1
    have h_j_pos : 0 < j := by linarith
    have h : ∃ k : ℕ, j = k + 1 := by
      refine (j - 1, ?)
    omega
  rcases h with (k, hk)
  have h2 : f p = p ^ (k + 1) := by
    rw [h1, hk]
  have h3 : p | p ^ (k + 1) := by
    use p ^ k
  <|> ring
  rw [h2] at *
  exact h3
have hX : p | b ^ p.toNat - (f b) ^ (f p).toNat := dvd_trans h21 h19
have h20 : p | b ^ p.toNat - b := by
  have h201 : (p.toNat : ℤ) | b ^ p.toNat - b := by
    exact fermat_little_theorem_int_version p.toNat hp b
  have h202 : (p.toNat : ℤ) = p := by
    simp [show 0 ≤ p by linarith]
  rw [h202] at h201
  exact h201
have h222 : p | (f b) ^ p.toNat - f b := by
  have h2221 : (p.toNat : ℤ) | (f b) ^ p.toNat - f b := by
    exact fermat_little_theorem_int_version p.toNat hp (f b)
  have h2222 : (p.toNat : ℤ) = p := by
    simp [show 0 ≤ p by linarith]
  rw [h2222] at h2221
  exact h2221
have hY : p | b - b ^ p.toNat := by

```



```

have h20' : p | b ^ p.toNat - b := h20
have h201 : p | -(b ^ p.toNat - b) := dvd_neg.mpr h20'
have h202 : -(b ^ p.toNat - b) = b - b ^ p.toNat := by ring
rw [h202] at h201
exact h201
have h231 : p | (b - b ^ p.toNat) + (b ^ p.toNat - (f b) ^ (f p).toNat) := by
  apply Int.dvd_add
  · exact hY
  · exact hX
have h232 : (b - b ^ p.toNat) + (b ^ p.toNat - (f b) ^ (f p).toNat) = b - (f
  → b) ^ (f p).toNat := by ring
have h23 : p | b - (f b) ^ (f p).toNat := by
  rw [h232] at h231
exact h231
have h23' : b = (f b) ^ (f p).toNat [ZMOD p] := by
  simpa [Int.ModEq, Int.emod_eq_emod_iff_emod_sub_eq_zero] using h23
have h_induction : ∀ (k : ℕ), k ≥ 1 → (f b) ^ ((p.toNat) ^ k) = f b [ZMOD p]
  → := by
  intro k hk
  induction k with
  | zero =>
    exfalso
    <|> omega
  | succ k ih =>
    by_cases h : k = 0
    · subst h
      have h22_flt : (f b) ^ p.toNat = f b [ZMOD p] := by
        have h221 : p | (f b) ^ p.toNat - f b := h221
        simpa [Int.ModEq, Int.emod_eq_emod_iff_emod_sub_eq_zero] using h221
        simpa using h22_flt
      have h_k_ge1 : k ≥ 1 := by omega
      have ih' : (f b) ^ ((p.toNat) ^ k) = f b [ZMOD p] := ih (by omega)
      have h22_flt : (f b) ^ p.toNat = f b [ZMOD p] := by
        have h221 : p | (f b) ^ p.toNat - f b := h221
        simpa [Int.ModEq, Int.emod_eq_emod_iff_emod_sub_eq_zero] using h221
      have h1 : ((f b) ^ ((p.toNat) ^ k)) ^ p.toNat = (f b) ^ p.toNat [ZMOD
        → p] := by
        exact Int.ModEq.pow p.toNat ih'
      have h2 : ((f b) ^ ((p.toNat) ^ k)) ^ p.toNat = f b [ZMOD p] := by
        exact Int.ModEq.trans h1 h22_flt
      have h3 : (f b) ^ ((p.toNat) ^ (k + 1)) = ((f b) ^ ((p.toNat) ^ k)) ^
        → p.toNat := by
        have h31 : (p.toNat) ^ (k + 1) = (p.toNat) * (p.toNat) ^ k := by ring
        rw [h31]
        rw [show (f b) ^ ((p.toNat) * (p.toNat) ^ k) = ((f b) ^ ((p.toNat) ^
          → k)) ^ (p.toNat) by
          rw [← pow_mul]
          <|> ring]
        have h4 : (f b) ^ ((p.toNat) ^ (k + 1)) = f b [ZMOD p] := by
          rw [h3]
          exact h2
        simpa using h4
      have h5 : (f p).toNat = (p.toNat) ^ j := by
        have h324 : ∀ (k : ℕ), (p ^ k : ℤ).toNat = (p.toNat) ^ k := by
          intro k
          have h1 : p ≥ 0 := by linarith
          induction k with
          | zero =>
            simp
            | succ k ih =>
              have h2 : p ^ k ≥ 0 := by positivity
              have h3 : (p ^ (k + 1) : ℤ) = p * (p ^ k) := by ring
              have h4 : (p ^ (k + 1) : ℤ) ≥ 0 := by positivity
              have h5 : ((p ^ (k + 1) : ℤ).toNat) = (p : ℤ).toNat * ((p ^ k : ℤ
                → ).toNat) := by
                rw [h3]
                exact f_is_not_identity_implies_f_p_eq_1_for_p_gt_2_int.toNat_mul p
                → (p ^ k) (by linarith) (by linarith)
                rw [h5]
                rw [ih]
                simp [pow_succ]
                <|> ring
              have h51 : f p = p ^ j := hj_eq
              have h512 : 0 ≤ f p := by linarith
              have h513 : (f p).toNat = ((p ^ j : ℤ).toNat) := by rw [h51]
              rw [h513]
              have h514 := h324 j
              simpa using h514
            have h24 : (f b) ^ ((p.toNat) ^ j) = f b [ZMOD p] := h_induction j (by
              → linarith)
            have h24' : (f b) ^ (f p).toNat = f b [ZMOD p] := by
              have h6 : (f b) ^ ((p.toNat) ^ j) = f b [ZMOD p] := h24
              have h7 : (f p).toNat = (p.toNat) ^ j := h5
              have h8 : (f b) ^ ((p.toNat) ^ j) = (f b) ^ (f p).toNat := by
                rw [h7]
                exact h6
              have h_f_final : b = f b [ZMOD p] := Int.ModEq.trans h23' h24'
              simpa using h_f_final
          theorem f_b_equiv_b_mod_p_of_f_p_ne_1 (n : ℤ) (f : ℤ → ℤ) (hn : n > 0) (hpos :
            → k : ℤ, k > 0 → f k > 0) (hf : ∀ a b : ℤ, a > 0 → b > 0 → f a | b ^
            → a.toNat - (f b) ^ (f a).toNat) (p : ℤ) (hp : Nat.Prime p.toNat)
            → (hfp_ne_1 : f p ≠ 1) :
            ∀ b : ℤ, b > 0 → b = f b [ZMOD p] := by
            have hp_pos : p > 0 := by
              by_contra h
              have h1 : p ≤ 0 := by linarith
              have h2 : p.toNat = 0 := by omega
              rw [h2] at hp
              norm_num at hp
            have h_f1_eq_1 : f 1 = 1 := by
              have h1 := hp_pos 1
              have h2 := hf 1 1
              simp at h2
              have h3 : f 1 | 1 := by
                have h32 := hf 1 1
                have h31 := h32
                have h33 : f 1 | (f 1) ^ (f 1).toNat + (1 ^ (1 : ℤ).toNat - (f 1) ^ (f
                  → 1).toNat) := by
                  apply Int.dvd_add
                  · apply dvd_pow_self
                    omega
                    simp_all
                    have h34 : (f 1) ^ (f 1).toNat + (1 ^ (1 : ℤ).toNat - (f 1) ^ (f
                      → 1).toNat) = 1 := by ring
                    rw [h34] at h33
                    exact h33
                    have h35 : f 1 ≤ 1 := Int.le_of_dvd (by norm_num) h3
                    omega
                    exact f_is_not_identity_implies_f_p_eq_1_for_p_gt_2_main_proof n f hn hp
                    → hf p hp hfp_ne_1 hp_pos h_f1_eq_1
                    → (f_is_not_identity_implies_f_p_eq_1_for_p_gt_2_divides_f_p_stronger
                      → n f hn hp
                      hf p hp hfp_ne_1 hp_pos)
                    theorem f_is_not_identity_implies_f_p_eq_1_for_p_gt_2_case2 (f : ℤ → ℤ) (hpos :
                      → ∀ k : ℤ, k > 0 → f k > 0) (hf : ∀ a b : ℤ, a > 0 → b > 0 → f a | b
                      → a.toNat - (f b) ^ (f a).toNat) (k : ℤ) (hk_pos : k > 0) (hf_not_id :
                      → ∃ i > 0, f i ≠ i) : ∃ p, Nat.Prime p.toNat ∧ p > k ∧ f p = 1 := by
                      rcases hf_not_id with (i₀, hi_pos, hfi_ne_i₀)
                      by_contra! h
                      have h_fi_pos : f i₀ > 0 := hp_pos i₀ hi_pos
                      have h3 : ∃ q : ℕ, Nat.Prime q ∧ q > k.toNat ∧ q > i₀.toNat ∧ q > (f i₀).toNat
                        := by
                          set M : ℕ := max (k.toNat) (max (i₀.toNat) ((f i₀).toNat)) with hM
                          have h1 := Nat.exists_infinite_primes (M + 1)
                          rcases h1 with (q, hq_ge, hq_prime)
                          have hq_gt_M : M < q := by linarith
                          have h11 : (k : ℤ).toNat ≤ M := by simp [hM]
                          have h12 : (i₀ : ℤ).toNat ≤ M := by
                            simp [hM]
                          have h13 : ((f i₀ : ℤ).toNat) ≤ M := by
                            simp [hM]
                          exact q, hq_prime, by linarith, by linarith, by linarith
                          rcases h3 with (q, hq_prime, hq_gt_k, hq_gt_i₀, hq_gt_fi₀)
                          have hq_gt_k2 : (q : ℤ) > k := by
                            have hq_gt_k21 : (q : ℤ) > (k : ℤ).toNat := by exact_mod_cast hq_gt_k
                            have h4 : 0 ≤ k := by linarith
                            have h5 : ((k : ℤ).toNat : ℤ) = k := by
                              simp [Int.toNat_of_nonneg h4]
                              linarith
                            have hq_gt_i2 : (q : ℤ) > i₀ := by
                              have hq_gt_i21 : (q : ℤ) > (i₀ : ℤ).toNat := by exact_mod_cast hq_gt_i₀
                              have h4 : 0 ≤ i₀ := by linarith
                              have h5 : ((f i₀ : ℤ).toNat : ℤ) = f i₀ := by
                                simp [Int.toNat_of_nonneg h4]
                                linarith
                              have hq_gt_fi2 : (q : ℤ) > f i₀ := by
                                have hq_gt_fi21 : (q : ℤ) > ((f i₀ : ℤ).toNat) := by exact_mod_cast
                                  → hq_gt_fi₀
                                have h4 : 0 ≤ f i₀ := by linarith
                                have h5 : (((f i₀ : ℤ).toNat : ℤ)) = f i₀ := by
                                  simp [Int.toNat_of_nonneg h4]
                                  linarith
                              have h5 : f (q : ℤ) ≠ 1 := hq hq_prime hq_gt_k2
                              have h6 : i₀ = f i₀ [ZMOD (q : ℤ)] := by
                                apply f_b_equiv_b_mod_p_of_f_p_ne_1
                                all_goals
                                  assumption
                              simp [Int.ModEq, Int.emod_eq_emod_iff_emod_sub_eq_zero] at h6
                              have h62 : (q : ℤ) | i₀ - f i₀ := by omega
                              by_cases h7 : f i₀ ≤ i₀
                              · have h73 : i₀ - f i₀ > 0 := by omega
                                have h74 : i₀ - f i₀ < (q : ℤ) := by linarith [h_fi_pos]
                                have h75 : (q : ℤ) ≤ i₀ - f i₀ := by exact Int.le_of_dvd (by linarith) h62
                                linarith
                              · have h8 : f i₀ > i₀ := by linarith
                                have h9 : (q : ℤ) | f i₀ - i₀ := by
                                  have h91 : (q : ℤ) | i₀ - f i₀ := h62
                                  have h92 : (q : ℤ) | -(i₀ - f i₀) := by exact dvd_neg.mpr h91
                                  have h93 : -(i₀ - f i₀) = f i₀ - i₀ := by ring
                                  rw [h93] at h92
                                  exact h92
                                have h94 : f i₀ - i₀ > 0 := by linarith
                                have h95 : (q : ℤ) ≤ f i₀ - i₀ := by exact Int.le_of_dvd (by linarith) h9
                                linarith
                            theorem f_is_not_identity_implies_f_p_eq_1_for_p_gt_2_case1 (f : ℤ → ℤ) (hpos :
                              → ∀ k : ℤ, k > 0 → f k > 0) (hf : ∀ a b : ℤ, a > 0 → b > 0 → f a | b
                              → a.toNat - (f b) ^ (f a).toNat) (k : ℤ) (hk_pos : k > 0) (h11 : ∀ k :
                              → ℤ, k > 0 → f k = 1) : ∃ p, Nat.Prime p.toNat ∧ p > k ∧ f p = 1 := by
                              obtain (p, hp_prop) := Nat.exists_infinite_primes k.toNat.succ
                              use p
                              constructor
                              exact hp_prop.2
                              constructor
                              omega
                              apply h11
                              omega
                            theorem f_is_not_identity_implies_f_p_eq_1_for_some_p_gt_k (f : ℤ → ℤ) (hpos :
                              → ∀ k : ℤ, k > 0 → f k > 0) (hf : ∀ a b : ℤ, a > 0 → b > 0 → f a | b ^
                              → a.toNat - (f b) ^ (f a).toNat) (k : ℤ) (hk_pos : k > 0) (hf_not_id :
                              → ∃ i > 0, f i ≠ i) :
                              ∃ p, Nat.Prime p.toNat ∧ p > k ∧ f p = 1 := by
                              apply f_is_not_identity_implies_f_p_eq_1_for_p_gt_2_case2
                              <|> simp_all
                            theorem f_is_not_identity_implies_f_p_eq_1_for_p_gt_2_h_main (n : ℤ)
                              (f : ℤ → ℤ)
                              (hn : n > 0)
                              (hpos : ∀ k : ℤ, k > 0 → f k > 0)
                              (hf : ∀ a b : ℤ, a > 0 → b > 0 → f a | b ^ a.toNat - (f b) ^ (f a).toNat)
                              (h_exists_k : ∃ k : ℤ, k > 1 ∧ f k ≠ k)
                              (p0 : ℤ)
                              (hp0_prime : Nat.Prime p0.toNat)
                              (hfp0_eq_1 : f p0 = 1)
                              (h_f_not_const_1 : ∃ n, n > 0 ∧ f n ≠ 1) :
                              ∀ (p : ℤ), Nat.Prime p.toNat → p ≥ p0 → f p = 1 := by
                              intro p hp_prime hp_ge_p0
                              by_contra h
                              have h_p0_ge_2 : p0 ≥ 2 := by
                                have h1 : Nat.Prime p0.toNat := hp0_prime
                                have h2 : p0.toNat ≥ 2 := Nat.Prime.two_le h1
                                omega
                              have := f_b_equiv_b_mod_p_of_f_p_ne_1 n f hn hpos hf p hp_prime h

```

```

simp_all [Int.ModEq, Int.emod_eq_emod_iff_emod_sub_eq_zero]
obtain k, hk := this p0 (by linarith)
have h5 : k > 0 := by
  by_contra h6
  have h6' : k ≤ 0 := by linarith
  nlinarith
  nlinarith

theorem f_is_1_on_all_primes_ge_p0_if_p0_eq_1_and_f_is_not_const_1 (n : z)
  → (f : z → z) (hn : n > 0) (hpos : ∀ k : z, k > 0 → f k > 0) (hf : ∀ a
  → b : z, a > 0 → b > 0 → f a | b ^ a.toNat - (f b) ^ (f a).toNat)
  → (h_exists_k : ∃ k : z, k > 1 ∧ f k ≠ k) (p0 : z) (hp0_prime :
  → Nat.Prime p0.toNat) (hfp0_eq_1 : f p0 = 1) (h_f_not_const_1 : ∃ n, n
  → > 0 ∧ f n ≠ 1) : ∀ p, Nat.Prime p.toNat → p > p0 → f p = 1 := by
  apply f_is_not_identity_implies_f_p_eq_1_for_p_gt_2_h_main
  all_goals assumption

theorem f_is_not_identity_implies_f_p_eq_1_for_p_gt_2_main (n : z) (f : z → z)
  → (hn : n > 0) (hpos : ∀ k : z, k > 0 → f k > 0) (hf : ∀ a b : z, a > 0
  → b > 0 → f a | b ^ a.toNat - (f b) ^ (f a).toNat) :
  (∃ n : z, n > 0 ∧ f n ≠ n) → ∀ p : z, Nat.Prime p.toNat → p > 2 → f p = 1 :=
  by
  intro h_f_not_id p hp_prime hp_gt_2
  by_contra h_f_neq_1
  cases' imo2025_p3_subproblem_f1_is_1_or_f_is_const_1 f hpos hf with
  → h_f_const_1 h_f1_eq_1
  · have h2 := h_f_const_1 p (by linarith)
    contradiction
  · have h_f1_eq_1 : f 1 = 1 := h_f1_eq_1
  · have h_exists_k : ∃ k : z, k > 1 ∧ f k ≠ k := by
    rcases h_f_not_id with m, hn_pos, hfn_ne_n
    by_cases hn_gt_1 : n > 1
    · refine m, hn_gt_1, hfn_ne_n
    · have hn_le_1 : n ≤ 1 := by linarith
      have h_n_eq_1 : n = 1 := by linarith
      rw [h_n_eq_1] at hfn_ne_n
      contradiction
  have h_exists_p0 := f_is_not_identity_implies_f_p_eq_1_for_some_p_gt_k f
  → hpos hf p (by linarith) h_f_not_id
  rcases h_exists_p0 with p0, hp0_prime, hp0_gt_p, hfp0_eq_1
  have h_f_not_const_1 : ∃ n, n > 0 ∧ f n ≠ 1 := by
    refine p, by linarith, h_f_neq_1
  have h_forall_primes_ge_p0_f_eq_1 :=
  → f_is_1_on_all_primes_ge_p0_if_p0_eq_1_and_f_is_not_const_1 n f hn
  → hpos hf h_exists_k hp0_prime hfp0_eq_1 h_f_not_const_1
  have h_p_toNat_gt_2 : p.toNat > 2 := by
    have h2 := hp_prime
    norm_cast
    omega
  have h_p_toNat_pos : 0 < p.toNat := by linarith
  haveI : Fact (Nat.Prime p.toNat) := (by exact_mod_cast hp_prime)
  have h_exists_q : ∃ q : N, q > p0.toNat ∧ Nat.Prime q ∧ (q : ZMod p.toNat) =
  → (2 : ZMod p.toNat) := by
    have h9 := Nat.forall_exists_prime_gt_and_eq_mod
    (isUnit_iff_ne_zero.mpr (by
      have h2_unit' : (2 : ZMod p.toNat) ≠ 0 := by
        intro h
        have h_dvd : (p.toNat : N) | 2 := by
          exact (ZMod.natCast_zmod_eq_zero_iff_dvd 2 p.toNat).mp h
        have h4 : p.toNat ≤ 2 := Nat.le_of_dvd (by norm_num) h_dvd
        linarith
        exact h2_unit'))
    (p0.toNat)
    rcases h9 with q, hq1, hq2, hq3
    refine q, hq1, hq2, hq3
  rcases h_exists_q with q, hq_gt_p0, hq_prime, hq_mod
  have hq_gt_p0' : (q : z) > p0 := by
    have h10 : q > p0.toNat := hq_gt_p0
    have h11 : (q : z) > (p0.toNat : z) := by exact_mod_cast h10
    have h12 : (p0.toNat : z) = p0 := by
      have h13 : 0 ≤ p0 := by linarith
    simp [Int.toNat_of_nonneg h13]
    rw [h12] at h11
    linarith
  have hq_pos : (q : z) > 0 := by linarith
  have hq_ge_p0 : (q : z) ≥ p0 := by linarith
  have h14 : Nat.Prime q := hq_prime
  have h15 : f (q : z) = 1 := by
    exact h_forall_primes_ge_p0_f_eq_1 (q : z) hq_prime (by linarith)
  have h13 : (q : z) = f (q : z) [ZMOD p] := f_b_equiv_b_mod_p_of_f_p_ne_1 n
  → f hn hpos hf p hp_prime h_f_neq_1 q (by linarith)
  have h14' : (q : z) = 1 [ZMOD p] := by
    rw [h15] at h13
    simp_all
  have h151 : p | (q : z) - 1 := by
    simp_all [Int.ModEq, Int.emod_eq_emod_iff_emod_sub_eq_zero]
  have hq_ge_2 : q ≥ 2 := by linarith
  have h4 : (q : N) % p.toNat = 2 := by
    have h11 : (q : ZMod p.toNat) = (2 : ZMod p.toNat) := hq_mod
    have h12 : (q : N) % p.toNat = (2 : N) % p.toNat := by
      exact (ZMod.nat_cast_eq_nat_cast_iff' q (2 : N) p.toNat).mp hq_mod
    have h13 : (2 : N) % p.toNat = 2 := by
      apply Nat.mod_eq_of_lt
    have h14 : p.toNat > 2 := by exact_mod_cast h_p_toNat_gt_2
    omega
  rw [h13] at h12
  exact h12
  have h2 : ∃ k : N, q = p.toNat * k + 2 := by
    use (q / p.toNat)
    have h8 : q = (q / p.toNat) * p.toNat + q % p.toNat := by
      exact Eq.symm (div_add_mod' q p.toNat)
    rw [h4] at h8
    linarith
  rcases h2 with k, hk
  have h6 : (p.toNat : N) | (q : N) - 2 := by
    use k
    have h8 : q = p.toNat * k + 2 := hk
    omega
  have h7 : (p.toNat : z) | (q : z) - 2 := by
    exact_mod_cast h6
  have h8 : (p : z) = (p.toNat : z) := by
    have h71 : 0 ≤ p := by linarith
    simp [Int.toNat_of_nonneg h71]
  have h9 : (p : z) | (q : z) - 2 := by
    rw [h8]

```

```

    exact h7
    have h10 : p | ((q : z) - 1) - ((q : z) - 2) := by
      exact Int.dvd_sub h151 h9
    have h11 : ((q : z) - 1) - ((q : z) - 2) = 1 := by ring
    rw [h11] at h10
    have h12 : p | 1 := h10
    have h13 : p ≤ 1 := by
      exact Int.le_of_dvd (by norm_num) h12
    linarith

theorem
  → f_is_not_identity_implies_f_p_eq_1_for_p_gt_2_f_is_not_identity_implies_f_p_eq_1_for_p_gt_2
  → (n : z) (f : z → z) (hn : n > 0) (hpos : ∀ k : z, k > 0 → f k > 0)
  → (hf : ∀ a b : z, a > 0 → b > 0 → f a | b ^ a.toNat - (f b) ^ (f a).toNat) :
  (∃ n : z, n > 0 ∧ f n ≠ n) → ∀ p : z, Nat.Prime p.toNat → p > 2 → f p = 1 :=
  by
  apply f_is_not_identity_implies_f_p_eq_1_for_p_gt_2_main
  <> assumption

theorem f_is_not_identity_implies_f_p_eq_1_for_p_gt_2 (n : z) (f : z → z) (hn
  → n > 0) (hpos : ∀ k : z, k > 0 → f k > 0) (hf : ∀ a b : z, a > 0 → b
  → > 0 → f a | b ^ a.toNat - (f b) ^ (f a).toNat) :
  (∃ n : z, n > 0 ∧ f n ≠ n) → ∀ p : z, Nat.Prime p.toNat → p > 2 → f p = 1 :=
  by
  apply
  → f_is_not_identity_implies_f_p_eq_1_for_p_gt_2_f_is_not_identity_implies_f_p_eq_1_for_p_gt_2
  <> assumption

theorem prime_divisor_of_fa_divides_fx_minus_x_h1 (n : z)
  (f : z → z)
  (hn : n > 0)
  (hpos : ∀ k : z, k > 0 → f k > 0)
  (hf : ∀ a b : z, a > 0 → b > 0 → f a | b ^ a.toNat - (f b) ^ (f a).toNat)
  (a x p : z)
  (ha : a > 0)
  (hx : x > 0)
  (hp : Nat.Prime p.toNat)
  (hdiv : p | f a) :
  p < 2 := by
  have := hp.two_le
  omega

theorem prime_divisor_of_fa_divides_fx_minus_x_h2 (n : z)
  (f : z → z)
  (hn : n > 0)
  (hpos : ∀ k : z, k > 0 → f k > 0)
  (hf : ∀ a b : z, a > 0 → b > 0 → f a | b ^ a.toNat - (f b) ^ (f a).toNat)
  (a x p : z)
  (ha : a > 0)
  (hx : x > 0)
  (hp : Nat.Prime p.toNat)
  (hdiv : p | f a)
  (h1 : p ≥ 2) :
  f p ≠ 1 := by
  intro hfp1
  have : p | p ^ a.toNat - (p ^ a.toNat - (f p) ^ (f a).toNat) := by
    apply Int.dvd_sub
    · exact dvd_pow_self p (by omega)
    · exact dvd_trans hdiv (hf a p ha (by linarith))
  simp_all
  rw [-, Int.natAbs_dvd_natAbs] at this
  norm_num at this
  omega

theorem prime_divisor_of_fa_divides_fx_minus_x_h10 (n : z)
  (f : z → z)
  (hn : n > 0)
  (hpos : ∀ k : z, k > 0 → f k > 0)
  (hf : ∀ a b : z, a > 0 → b > 0 → f a | b ^ a.toNat - (f b) ^ (f a).toNat)
  (a x p : z)
  (ha : a > 0)
  (hx : x > 0)
  (hp : Nat.Prime p.toNat)
  (hdiv : p | f a)
  (h2 : f p ≠ 1) :
  ∀ (b : z), b > 0 → b = f b [ZMOD p] := by
  apply f_b_equiv_b_mod_p_of_f_p_ne_1
  <> aesop

theorem prime_divisor_of_fa_divides_fx_minus_x_h11 (n : z)
  (f : z → z)
  (hn : n > 0)
  (hpos : ∀ k : z, k > 0 → f k > 0)
  (hf : ∀ a b : z, a > 0 → b > 0 → f a | b ^ a.toNat - (f b) ^ (f a).toNat)
  (a x p : z)
  (ha : a > 0)
  (hx : x > 0)
  (hp : Nat.Prime p.toNat)
  (hdiv : p | f a)
  (h10 : ∀ (b : z), b > 0 → b = f b [ZMOD p]) :
  x = f x [ZMOD p] := by
  apply h10
  assumption

theorem prime_divisor_of_fa_divides_fx_minus_x_h13 (n : z)
  (f : z → z)
  (hn : n > 0)
  (hpos : ∀ k : z, k > 0 → f k > 0)
  (hf : ∀ a b : z, a > 0 → b > 0 → f a | b ^ a.toNat - (f b) ^ (f a).toNat)
  (a x p : z)
  (ha : a > 0)
  (hx : x > 0)
  (hp : Nat.Prime p.toNat)
  (hdiv : p | f a)
  (h11 : x = f x [ZMOD p]) :
  p | f x - x := by
  exact h11.dvd

theorem prime_divisor_of_fa_divides_fx_minus_x (n : z) (f : z → z) (hn : n >
  → 0) (hpos : ∀ k : z, k > 0 → f k > 0) (hf : ∀ a b : z, a > 0 → b > 0 →
  → f a | b ^ a.toNat - (f b) ^ (f a).toNat) (a x p : z) (ha : a > 0) (hx
  → x > 0) (hp : Nat.Prime p.toNat) (hdiv : p | f a) : p | f x - x := by

```

```

apply prime_divisor_of_fa_divides_fx_minus_x_h13 n f hn hpos hf a x p ha hx
  → hp hdiv
apply prime_divisor_of_fa_divides_fx_minus_x_h11 n f hn hpos hf a x p ha hx
  → hp hdiv
apply prime_divisor_of_fa_divides_fx_minus_x_h10 n f hn hpos hf a x p ha hx
  → hp hdiv
apply prime_divisor_of_fa_divides_fx_minus_x_h2 n f hn hpos hf a x p ha hx
  → hp hdiv
apply prime_divisor_of_fa_divides_fx_minus_x_h1 n f hn hpos hf a x p ha hx
  → hp hdiv

theorem f_n_is_power_of_two_for_even_n_h10 :
  ∀ (m : ℕ), m > 0 → (∀ (p : ℕ, Nat.Prime p → p ∣ m → p = 2) → (∃ (k : ℕ, m = 2 ^
    → k) := by
  intro m hm h_prime
  induction' m using Nat.strong_induction_on with m ih
  by_cases h : m = 1
  · exact 0, h
  · rcases Nat.exists_prime_and_dvd (by omega : m ≠ 1) with (p, hp, hp')
    have := h_prime p hp hp'
    simp_all
    cases' hp' with t ht
    cases' ih t (by omega) (by omega) (fun p hp' hp'' => h_prime p hp' (by rw
      → [ht]; exact dvd_mul_of_dvd_right hp'' 2)) with k hk
    exact (k + 1, by simp_all); ring

theorem f_n_is_power_of_two_for_even_n_h1 (n : ℕ)
  (f : ℕ → ℕ)
  (hn : n > 0)
  (hpos : ∀ k : ℕ, k > 0 → f k > 0)
  (hf : ∀ a b : ℕ, a > 0 → b > 0 → f a ∣ b ^ a.toNat - (f b) ^ (f a).toNat)
  (h_exists_k : ∃ k : ℕ, k > 1 ∧ f k ≠ k) :
  ∀ (q : ℕ), Nat.Prime q.toNat → q ∣ f n → q = 2 := by
  intro q hq_prime hq_divides_fn
  by_contra hq
  obtain k, hk := h_exists_k
  have hq_gt_2 : q > 2 := by
    by_contra hq_le_2
    have hq1 : q ≤ 2 := by linarith
    have hq11 : q.toNat = 0 ∨ q.toNat = 1 := by
      omega
    rcases hq11 with (hq11 | hq11) <|> simp_all [Nat.Prime]
  have := f_is_not_identity_implies_f_eq_1_for_p_gt_2 n f hn hpos hf k, by
    → linarith, hk 2
  have := prime_divisor_of_fa_divides_fx_minus_x n f hn hpos hf n q q hn (by
    → omega) hq_prime hq_divides_fn
  have : q = 1 := by
    have : q ∣ 1 := by simp_all
    exact Int.eq_one_of_dvd_one (by linarith) this
  simp_all

theorem f_n_is_power_of_two_for_even_n_main (n : ℕ)
  (f : ℕ → ℕ)
  (hn : n > 0)
  (hpos : ∀ k : ℕ, k > 0 → f k > 0)
  (hf : ∀ a b : ℕ, a > 0 → b > 0 → f a ∣ b ^ a.toNat - (f b) ^ (f a).toNat)
  (h_exists_k : ∃ k : ℕ, k > 1 ∧ f k ≠ k) :
  ∃ k : ℕ, f n = 2 ^ k := by
  have h6 : := hpos n hn
  have h61 : ∃ (m : ℕ), (m : ℕ) = f n ∧ m > 0 := by
    use (f n).toNat
    constructor
    · simp [Int.toNat_of_nonneg (by linarith : 0 ≤ f n)]
    · omega
  rcases h61 with m, hm1, hm2
  obtain k, hk := f_n_is_power_of_two_for_even_n_h10 m hm2 fun p hp hpdvd =>
    → by
      have hpdvd' : (p : ℕ) ∣ (m : ℕ) := by exact_mod_cast hpdvd
      exact_mod_cast f_n_is_power_of_two_for_even_n_h1 n f hn hpos hf h_exists_k
      → p hp (by simp_all [dvd_gcd_iff])
  exact (k, by linarith)

theorem f_n_is_power_of_two_for_even_n (n : ℕ) (f : ℕ → ℕ) (hn : n > 0) (hpos :
  → ∀ k : ℕ, k > 0 → f k > 0) (hf : ∀ a b : ℕ, a > 0 → b > 0 → f a ∣ b ^ a.toNat - (f b) ^ (f a).toNat)
  (h_exists_k : ∃ k : ℕ, k > 1 ∧ f k ≠ k) :
  ∃ k : ℕ, f n = 2 ^ k := by
  apply f_n_is_power_of_two_for_even_n_main
  <|> assumption

theorem round1_h_main' (n : ℕ) (f : ℕ → ℕ) (hn : n > 0) (hpos : ∀ k : ℕ, k > 0
  → f k > 0) (hf : ∀ a b : ℕ, a > 0 → b > 0 → f a ∣ b ^ a.toNat - (f b)
  → ^ (f a).toNat) : f n ≤ 4 * n := by
  cases' imo2025_p3_subproblem_f1_is_1_or_f_is_const_1 f hpos hf with h19 h20
  · have h21 : f n = 1 := h19 n hn
    linarith
  · by_cases h21 : ∀ k : ℕ, k > 0 → f k = k
    · exact round1_h_subcase1 n f hn hpos hf h21
    · push_neg at h21
      obtain (k, hk_pos, hk_ne) := h21
      have h22 : k > 1 := by
        by_contra h23
        have h24 : k ≤ 1 := by linarith
        have h25 : k = 1 := by omega
        rw [h25] at hk_ne
        contradiction
      have h23 : ∃ k' : ℕ, k' > 1 ∧ f k' ≠ k' := (k, h22, hk_ne)
      have h24 : ∃ n : ℕ, n > 0 ∧ f n ≠ n := by
        obtain (k, hk1, hk2) := h23
        refine' (k, by linarith, hk2)
      have h25 := f_is_not_identity_implies_f_eq_1_for_p_gt_2 n f hn hpos hf
        → h24
      have h26 : f 3 = 1 := h25 3 (by decide) (by norm_num)
      have h27 : f n ∣ 3 ^ n.toNat - 1 := by
        have h28 := hf n 3 hn (by norm_num)
        rw [h26] at h28
      aesop
      have h28 : ∃ k : ℕ, f n = 2 ^ k := f_n_is_power_of_two_for_even_n n f hn
        → hpos hf h23
      obtain (k, hk) := h28
      have h29 : f n = (2 : ℕ) ^ k := hk
      have h30 : (2 : ℕ) ^ k ∣ 3 ^ n.toNat - 1 := by
        rw [h29] at h27
      exact h27
      have h31 := round1_h_k_le_padic n f k hn hpos hf h30
      have h32 := lte_2_3n_minus_1 n hn
      have h33 : k ≤ 2 + padicValNat 2 n.toNat := by
        split_ifs at h32 <|> omega
        exact round1_h6' n f hn hpos hf k (by aesop) (by aesop)

theorem imo2025_p3_left (n : ℕ) (f : ℕ → ℕ) (hn : n > 0) (hpos : ∀ k : ℕ, k > 0
  → f k > 0) (hf : ∀ a b : ℕ, a > 0 → b > 0 → f a ∣ b ^ a.toNat - (f b)
  → ^ (f a).toNat) : f n ≤ 4 * n := by
  apply round1_h_main'
  assumption

theorem imo2025_p3_right : ∃ (n : ℕ) (f : ℕ → ℕ), (n > 0) ∧ (∀ k : ℕ, k > 0 → f
  → k > 0) ∧ (∀ a b : ℕ, a > 0 → b > 0 → f a ∣ b ^ a.toNat - (f b) ^ (f
  → a).toNat) ∧ (f n ≥ 4 * n) := by
  use 4
  use fun k => if k > 0 then if k = 4 then 16 else if k % 2 = 1 then 1 else 2
  → else 0
  constructor
  norm_num
  constructor
  intro k hk
  split_ifs
  <|> omega
  constructor
  intro a b ha hb
  by_cases ha4 : a = 4
  · have h1 : a = 4 := ha4
    by_cases hb4 : b = 4
    · have h2 : b = 4 := hb4
      simp [h1, h2]
      <|> norm_num
    · have h2 : b ≠ 4 := hb4
      by_cases hb10 : b % 2 = 1
      · have h21 : b % 2 = 1 := hb10
        have h22 : (b ^ 4 - 1) % 16 = 0 := by
          have h221 : b % 2 = 1 := h21
          have h222 : b ^ 4 % 16 = 1 := by
            have h223 : b % 16 = 1 ∨ b % 16 = 3 ∨ b % 16 = 5 ∨ b % 16 = 7 ∨ b %
              → 16 = 9 ∨ b % 16 = 11 ∨ b % 16 = 13 ∨ b % 16 = 15 := by omega
            rcases h223 with (h223 | h223 | h223 | h223 | h223 | h223 | h223 |
              → h223) <|> simp [h223, pow_succ, Int.mul_emod]
          omega
          simp [h1, h2, h21] at *
          <|> omega
        have h22 : (b ^ 4 - 1) % 16 = 0 := hb10
        have h23 : b % 2 = 0 := by omega
        have h24 : (b ^ 4 - 2 ^ 16) % 16 = 0 := by
          have h241 : b % 2 = 0 := h23
          have h242 : b ^ 4 % 16 = 0 := by
            have h244 : b % 16 = 0 ∨ b % 16 = 2 ∨ b % 16 = 4 ∨ b % 16 = 6 ∨ b %
              → 16 = 8 ∨ b % 16 = 10 ∨ b % 16 = 12 ∨ b % 16 = 14 := by omega
            rcases h244 with (h244 | h244 | h244 | h244 | h244 | h244 | h244 |
              → h244) <|> simp [h244, pow_succ, Int.mul_emod]
          omega
          simp [h1, h2, h22, h23] at *
          <|> omega
        have ha11 : a = 4 := ha4
        by_cases ha12 : a % 2 = 1
        · have ha121 : a % 2 = 1 := ha12
          have h3 : (if a > 0 then (if a = 4 then 16 else (if a % 2 = 1 then 1
            → else 2)) else 0 : ℕ) = 1 := by
            simp [ha, ha11, ha121]
          rw [h3]
          norm_num
        · have ha122 : a % 2 ≠ 1 := ha12
          have ha13 : a % 2 = 0 := by omega
          have h3 : (if a > 0 then (if a = 4 then 16 else (if a % 2 = 1 then 1
            → else 2)) else 0 : ℕ) = 2 := by
            simp [ha, ha11, ha122, ha13]
          have h4 : (if a > 0 then (if a = 4 then 16 else (if a % 2 = 1 then 1
            → else 2)) else 0 : ℕ).toNat = 2 := by
            simp [h3]
          have h6 : (2 : ℕ) ∣ b ^ a.toNat - (if b > 0 then (if b = 4 then 16 else
            → (if b % 2 = 1 then 1 else 2)) else 0 : ℕ) ^ 2 := by
            have h61 : (b ^ a.toNat) % 2 = b % 2 := by
              by_cases h604 : b % 2 = 0
              · have h605 : (b ^ a.toNat) % 2 = 0 := by
                  have h6061 : a.toNat > 0 := by
                    have h6062 : 0 < a := by linarith
                    have h6063 : a ≥ 1 := by linarith
                    have h6064 : a.toNat ≥ 1 := by omega
                  omega
                have h607 : (b ^ a.toNat) % 2 = 0 := by
                  have h608 : b % 2 = 0 := h604
                  have h609 : ∀ n : ℕ, n > 0 → (b ^ n) % 2 = 0 := by
                    intro n
                    induction n with
                    | zero => contradiction
                    | succ n ih =>
                      by_cases h610 : n = 0
                      · simp [h610, h608]
                      · have h611 : n > 0 := by omega
                        have ih' := ih h611
                        simp [pow_succ, Int.mul_emod, h608, ih']
                        exact h609 a.toNat h6061
                  exact h607
                have h6041 : b % 2 = 0 := h604
                omega
              · have h6041 : b % 2 = 1 := by omega
                have h605 : (b ^ a.toNat) % 2 = 1 := by
                  have h606 : a.toNat > 0 := by
                    have h6061 : 0 < a := by linarith
                    have h6062 : a ≥ 1 := by linarith
                    have h6063 : a.toNat ≥ 1 := by omega
                  omega
                have h607 : (b ^ a.toNat) % 2 = 1 := by
                  have h608 : b % 2 = 1 := h6041
                  have h609 : ∀ n : ℕ, (b ^ n) % 2 = 1 := by
                    intro n
                    induction n with
                    | zero => simp [h608]
                    | succ n ih =>
                      simp [pow_succ, Int.mul_emod, h608, ih]
                  exact h609 a.toNat
                exact h607
                have h610 : b % 2 = 1 := h6041
                omega

```

```

have h61 : ( (if b > 0 then (if b = 4 then 16 else (if b % 2 = 1 then
→ 1 else 2)) else 0 : z) ) % 2 = b % 2 := by
  have h610 : b > 0 := by linarith
  have h611 : (if b > 0 then (if b = 4 then 16 else (if b % 2 = 1 then
→ 1 else 2)) else 0 : z) = (if b = 4 then 16 else (if b % 2 = 1 then 1
→ else 2)) := by
    simp [h610]
  rw [h611]
  by_cases h612 : b = 4
  · rw [if_pos h612]
    <|> omega
  · rw [if_neg h612]
    by_cases h613 : b % 2 = 1
    · rw [if_pos h613]
      <|> omega
    · rw [if_neg h613]
      have h614 : b % 2 = 0 := by omega
      have h615 : (2 : z) % 2 = 0 := by norm_num
      omega
  have h62 : ( (if b > 0 then (if b = 4 then 16 else (if b % 2 = 1 then
→ 1 else 2)) else 0 : z) ^ 2) % 2 = ( (if b > 0 then (if b = 4 then 16
→ else (if b % 2 = 1 then 1 else 2)) else 0 : z) ) % 2 := by
    have h616 : ∀ x : z, (x ^ 2) % 2 = x % 2 := by
      intro x
      have h617 : x % 2 = 0 ∨ x % 2 = 1 := by omega
      rcases h617 with (h617 | h617) <|> simp [h617, pow_two,
→ Int.mul_emod]
    exact h616 ((if b > 0 then (if b = 4 then 16 else (if b % 2 = 1 then
→ 1 else 2)) else 0 : z))
  have h63 : ( (if b > 0 then (if b = 4 then 16 else (if b % 2 = 1 then
→ 1 else 2)) else 0 : z) ^ 2) % 2 = b % 2 := by omega
  have h64 : (b ^ a.toNat - (if b > 0 then (if b = 4 then 16 else (if b
→ % 2 = 1 then 1 else 2)) else 0 : z) ^ 2) % 2 = 0 := by omega
  omega
  simp [h3, h4] using h6
norm_num
#print axioms imo2025_p3_left
#print axioms imo2025_p3_right

```

```

-- P4
import Mathlib
import Aesop
set_option pp.numericTypes true
set_option pp.funBinderTypes true
set_option maxHeartbeats 0
set_option maxRecDepth 1000
set_option tactic.hygienic false

set_option linter.unnecessarySeqFocus false
set_option linter.unusedVariables false
set_option linter.unreachableTactic false

open BigOperators Real Nat Topology Rat Classical Polynomial

theorem a0_is_even1_h_lemma1 (a : ℕ → ℕ)
(hpos : ∀ n : ℕ, a n > 0)
(h1 : ∀ n : ℕ, ∃ b c d : ℕ, b < c < a < d ∧ d < a ∧ b | a ∧ c | a ∧ d | a
→ n ∧ (∀ e : ℕ, e < a → e | a → e ≤ b ∨ e = c ∨ e = d) ∧ a (n + 1) =
→ b + c + d) :
∀ n : ℕ, (a n % 2 = 1) → a (n + 1) < a n := by
intro n h_an_odd
rcases h1 n with ⟨b, c, d, h11, h12, h13, h14, h15, h16, h17, h18⟩
cases' h16 with k hk
have h3 : k ≥ 3 := by
by_contra
interval_cases k <|> simp_all
nlinarith

theorem a0_is_even1_h_lemma2 (a : ℕ → ℕ)
(h1 : ∀ n : ℕ, ∃ b c d : ℕ, b < c < a < d ∧ d < a ∧ b | a ∧ c | a ∧ d | a
→ n ∧ (∀ e : ℕ, e < a → e | a → e ≤ b ∨ e = c ∨ e = d) ∧ a (n + 1) =
→ b + c + d) :
(a 0 % 2 = 1) → ∀ n : ℕ, a n % 2 = 1 := by
intro h_n
induction' n with n ih
simp_all
rcases h1 n with ⟨b, c, d, h11, h12, h13, h14, h15, h16, h17, h18⟩
have : b % 2 = 1 := by
by_contra
have : 2 | b := by omega
have : 2 | a n := dvd_trans this h14
omega
have : c % 2 = 1 := by
by_contra
have : 2 | c := by omega
have : 2 | a n := dvd_trans this h15
omega
have : d % 2 = 1 := by
by_contra
have : 2 | d := by omega
have : 2 | a n := dvd_trans this h16
omega
omega

theorem a0_is_even1_h_main (a : ℕ → ℕ)
(hpos : ∀ n : ℕ, a n > 0)
(h1 : ∀ n : ℕ, ∃ b c d : ℕ, b < c < a < d ∧ d < a ∧ b | a ∧ c | a ∧ d | a
→ n ∧ (∀ e : ℕ, e < a → e | a → e ≤ b ∨ e = c ∨ e = d) ∧ a (n + 1) =
→ b + c + d) :
(h_lemma1 : ∀ n : ℕ, (a n % 2 = 1) → a (n + 1) < a n)
(h_lemma2 : (a 0 % 2 = 1) → ∀ n : ℕ, a n % 2 = 1) :
Even (a 0) := by
by_contra! h_even_a0
have h_even_aux : ∀ n, a n + n ≤ a 0 := by
intro n
induction' n with n hn
simp_all
linarith [h_lemma1 n (h_lemma2 (Nat.not_even_iff.mp h_even_a0) n)]
linarith [h_even_aux (a 0 + 1)]

theorem a0_is_even (a : ℕ → ℕ) (hpos : ∀ n : ℕ, a n > 0) (h1 : ∀ n : ℕ, ∃ b c
→ d : ℕ, b < c < a < d ∧ d < a ∧ b | a ∧ c | a ∧ d | a ∧ a (∀ e : ℕ,
→ e < a → e | a → e ≤ b ∨ e = c ∨ e = d) ∧ a (n + 1) = b + c + d)
→ (h_an_pos : ∀ n : ℕ, a n > 0) (h_an_prop : ∀ n, ∃ b c d : ℕ, b < c < a < d
→ d < a ∧ b | a ∧ c | a ∧ d | a ∧ a (∀ e : ℕ, e < a → e | a →
→ e ≤ b ∨ e = c ∨ e = d) ∧ a (n + 1) = b + c + d) :
Even (a 0) := by
simp_all [a0_is_even1_h_main, a0_is_even1_h_lemma1, a0_is_even1_h_lemma2]

theorem prop_a0_divisible_by_31_h1 (a : ℕ → ℕ) (hpos : ∀ n : ℕ, a n > 0) (h1 :
→ ∀ n : ℕ, ∃ b c d : ℕ, b < c < a < d ∧ d < a ∧ b | a ∧ c | a ∧ d | a
→ a n ∧ (∀ e : ℕ, e < a → e | a → e ≤ b ∨ e = c ∨ e = d) ∧ a (n + 1)
→ b + c + d) : ∀ n : ℕ, a n % 2 = 1 → a (n + 1) % 2 = 1 := by
intro n h
obtain ⟨b, c, d, hb, hc, hd, hb_, hc_, hd_, h_abodcd⟩ := h1 n
have : b % 2 = 1 ∧ c % 2 = 1 ∧ d % 2 = 1 := by
constructor
· by_contra h
have : 2 | b := by omega
have : 2 | a n := dvd_trans this hb_
omega
constructor
· by_contra h
have : 2 | c := by omega
have : 2 | a n := dvd_trans this hc_
omega
· by_contra h
have : 2 | d := by omega
have : 2 | a n := dvd_trans this hd_
omega
omega

theorem prop_a0_divisible_by_31_h2 (a : ℕ → ℕ) (hpos : ∀ n : ℕ, a n > 0) (h1 :
→ ∀ n : ℕ, ∃ b c d : ℕ, b < c < a < d ∧ d < a ∧ b | a ∧ c | a ∧ d | a
→ a n ∧ (∀ e : ℕ, e < a → e | a → e ≤ b ∨ e = c ∨ e = d) ∧ a (n + 1)
→ b + c + d) : ∀ n : ℕ, a n % 2 = 1 → a (n + 1) % 2 = 1 := by
intro n hn
obtain ⟨b, c, d, h12, h13, h14, h15, h16, h17, h18⟩ := h1 n
cases' h17 with k hk
have : k ≥ 3 := by
by_contra
interval_cases k <|> simp_all
nlinarith

theorem prop_a0_divisible_by_31_two_divides_a_n (a : ℕ → ℕ) (hpos : ∀ n : ℕ, a
→ n > 0) (h1 : ∀ n : ℕ, ∃ b c d : ℕ, b < c < a < d ∧ d < a ∧ b | a ∧ c | a

```

```

→ a d | a n ∧ (∀ e : N, e < a → e | a n → e ≤ b v e = c v e = d) ∧ a (n
→ + 1) = b + c + d : ∃ j, 3 | a j ∧ ∀ i < j, ¬ (3 | a i) := by
apply exists_first_term_divisible_by_3_h4 a hpos h1
apply exists_first_term_divisible_by_3_h3 a hpos h1

theorem prop_a0_divisible_by_31_h_lemma1 (a : N → N)
(hpos : ∀ n : N, a n > 0)
(h1 : ∀ n : N, ∃ b c d : N, b < c < a c < d ∧ d < a n ∧ b | a n ∧ c | a n ∧ d | a
→ n ∧ (∀ e : N, e < a n → e | a n → e ≤ b v e = c v e = d) ∧ a (n + 1) =
→ b + c + d) :
∀ n : N, (a n % 2 = 1) → a (n + 1) < a n := by
intro n h_an_odd
rcases h1 n with ⟨b, c, d, _, _, h14, h15, h16, h17⟩
cases' h16 with k hk
have : k ≥ 3 := by
by_contra
interval_cases k <|> simp_all
nlinarith

theorem prop_a0_divisible_by_31_h_lemma2 (a : N → N)
(h1 : ∀ n : N, ∃ b c d : N, b < c < a c < d ∧ d < a n ∧ b | a n ∧ c | a n ∧ d | a
→ n ∧ (∀ e : N, e < a n → e | a n → e ≤ b v e = c v e = d) ∧ a (n + 1) =
→ b + c + d) :
(a 0 % 2 = 1) → ∀ n : N, a n % 2 = 1 := by
intro h_n
induction' n with n ih
simp_all
rcases h1 n with ⟨b, c, d, hbd⟩
have : b % 2 = 1 ∧ c % 2 = 1 ∧ d % 2 = 1 := by
constructor
· by_contra
have : 2 | b := by omega
have : 2 | a n := dvd_trans this (by aesop)
omega
· constructor
· by_contra
have : 2 | c := by omega
have : 2 | a n := dvd_trans this (by aesop)
omega
· by_contra
have : 2 | d := by omega
have : 2 | a n := dvd_trans this (by aesop)
omega
omega

theorem prop_a0_divisible_by_31_h_main (a : N → N)
(hpos : ∀ n : N, a n > 0)
(h1 : ∀ n : N, ∃ b c d : N, b < c < a c < d ∧ d < a n ∧ b | a n ∧ c | a n ∧ d | a
→ n ∧ (∀ e : N, e < a n → e | a n → e ≤ b v e = c v e = d) ∧ a (n + 1) =
→ b + c + d)
(h_lemma1 : ∀ n : N, (a n % 2 = 1) → a (n + 1) < a n)
(h_lemma2 : (a 0 % 2 = 1) → ∀ n : N, a n % 2 = 1) :
Even (a 0) := by
simp_all [Nat.even_iff]
by_contra h_even
have h200 : ∀ n, a n + n ≤ a 0 := by
intro n
induction' n with n inh
simp
linarith [h_lemma1 n (h_lemma2 (by omega) n)]
linarith [h200 (a 0 + 1)]

theorem prop_a0_divisible_by_31_a_n_ge_4 (a : N → N) (hpos : ∀ n : N, a n > 0)
→ (h1 : ∀ n : N, ∃ b c d : N, b < c < a c < d ∧ d < a n ∧ b | a n ∧ c | a n ∧ d | a
→ a d | a n ∧ (∀ e : N, e < a n → e | a n → e ≤ b v e = c v e = d) ∧ a (n
→ + 1) = b + c + d) :
∀ n : N, a n ≥ 4 := by
intro n
obtain ⟨b, c, d, hb⟩ := h1 n
have := hb.2.2.1
have : b > 0 := by
by_contra
simp_all
omega

theorem prop_a0_divisible_by_31_h_main_a_n_ge_4 (a : N → N)
(hpos : ∀ n : N, a n > 0)
(h1 : ∀ n : N, ∃ b c d : N, b < c < a c < d ∧ d < a n ∧ b | a n ∧ c | a n ∧ d | a
→ n ∧ (∀ e : N, e < a n → e | a n → e ≤ b v e = c v e = d) ∧ a (n + 1) =
→ b + c + d)
(n : N) :
a n ≥ 6 := by
by_contra! h
obtain ⟨b, c, d, h_b_lt_c, h_c_lt_d, h_d_lt_an, h_b_div_an, h_c_div_an,
→ h_d_div_an, _, h_an_eq⟩ := h1 n
have : b < 5 := by linarith
have : d < 5 := by linarith
interval_cases b <|> interval_cases d <|> omega

theorem prop_a0_divisible_by_31_a_n_ge_6 (a : N → N) (hpos : ∀ n : N, a n > 0)
→ (h1 : ∀ n : N, ∃ b c d : N, b < c < a c < d ∧ d < a n ∧ b | a n ∧ c | a n
→ a d | a n ∧ (∀ e : N, e < a n → e | a n → e ≤ b v e = c v e = d) ∧ a (n
→ + 1) = b + c + d) (n : N) : a n ≥ 6 := by
apply prop_a0_divisible_by_31_h_main_a_n_ge_4
<|> simp_all

theorem prop_a0_divisible_by_31_mod_3_case_analysis (b c d : N) (h1 : 3 | b + c
→ + d) (h2 : ¬ (3 | b)) (h3 : ¬ (3 | c)) (h4 : ¬ (3 | d)) :
(b % 3 = 1 ∧ c % 3 = 1 ∧ d % 3 = 1) ∨ (b % 3 = 2 ∧ c % 3 = 2 ∧ d % 3 = 2) :=
by
omega

theorem prop_a0_divisible_by_31_main_contradiction
(a : N → N)
(hpos : ∀ n : N, a n > 0)
(h1 : ∀ n : N, ∃ b c d : N, b < c < a c < d ∧ d < a n ∧ b | a n ∧ c | a n ∧ d | a
→ n ∧ (∀ e : N, e < a n → e | a n → e ≤ b v e = c v e = d) ∧ a (n + 1) =
→ b + c + d)
(k : N)
(b : N)
(c : N)
(d : N)
(h9 : b < c)
(h10 : c < d)
(h11 : d < a k)
(h12 : b | a k)
(h13 : c | a k)
(h14 : d | a k)
(h15 : ∀ e : N, e < a k → e | a k → e ≤ b v e = c v e = d)
(h16 : a (k + 1) = b + c + d)
(h3_div_bcd : 3 | b + c + d)
(h_not_div_3_b : ¬ (3 | b))
(h_not_div_3_c : ¬ (3 | c))
(h_not_div_3_d : ¬ (3 | d))
(h4_div_ak : ¬ (4 | a k))
(h_not_div_3_ak : ¬ (3 | a k)) :
False := by
have h2_div_ak : 2 | a k := prop_a0_divisible_by_31_two_divides_a_n a hpos h1
→ k
have hak_ge_6 : a k ≥ 6 := prop_a0_divisible_by_31_a_n_ge_6 a hpos h1 k
have h12' : b | a k := h12
have h13' : c | a k := h13
have h14' : d | a k := h14
have h15' : ∀ e : N, e < a k → e | a k → e ≤ b v e = c v e = d := h15
have h16' : a (k + 1) = b + c + d := h16
have h3_div_bcd' : 3 | b + c + d := h3_div_bcd
have h_not_div_3_b' : ¬ (3 | b) := h_not_div_3_b
have h_not_div_3_c' : ¬ (3 | c) := h_not_div_3_c
have h_not_div_3_d' : ¬ (3 | d) := h_not_div_3_d
rcases h15' 2 (by linarith) (by simp using h2_div_ak) with (h15_2 | h15_2 |
→ h15_2)
ex falso
have h15_a_k_div_2 : a k / 2 < a k := by
omega
have h_a_k_div_2_dvd_a_k : (a k / 2) | a k := by
use 2
<|> omega
have h15_a_k_div_2 : (a k / 2) ≤ b v (a k / 2) = c v (a k / 2) = d := by
have h15_1 : (a k / 2) < a k := h15_a_k_div_2
have h15_2 : (a k / 2) | a k := h_a_k_div_2_dvd_a_k
have h15_3 := h15' (a k / 2) h15_1 h15_2
simp using h15_3
rcases h15_a_k_div_2 with (h15_a_k_div_2 | h15_a_k_div_2 | h15_a_k_div_2)
have h_a_k_le_2_b : a k ≤ 2 * b := by omega
have h_a_k_eq_2_b : a k = 2 * b := by
have h_b_dvd_a_k : b | a k := h12'
have h_b_pos : 0 < b := by linarith
have h_a_k_pos : 0 < a k := by linarith
have h_exists_m : ∃ m : N, a k = b * m := by
exact h12
rcases h_exists_m with ⟨m, hm⟩
have h_m_pos : 0 < m := by
by_contra h
have h_m_eq_0 : m = 0 := by omega
rw [h_m_eq_0] at hm
nlinarith
have h_m_ge_2 : m ≥ 2 := by
by_contra h
have h_m_lt_2 : m < 2 := by linarith
have h_m_ge_1 : m ≥ 1 := by linarith
have h_m_eq_1 : m = 1 := by omega
rw [h_m_eq_1] at hm
nlinarith
have h_a_k_ge_2_b : a k ≥ 2 * b := by
nlinarith
nlinarith
have h_c_dvd_2_b : c | 2 * b := by
have h_c_dvd_a_k : c | a k := h13'
rw [h_a_k_eq_2_b] at h_c_dvd_a_k
simp using h_c_dvd_a_k
have h_b_lt_c : b < c := h9
have h_c_eq_2_b : c = 2 * b := by
have h_c_dvd_2_b' : c | 2 * b := h_c_dvd_2_b
have h_c_pos : 0 < c := by linarith
have h_exists_k : ∃ k : N, 2 * b = c * k := by
exact h_c_dvd_2_b
rcases h_exists_k with ⟨k, hk⟩
have h_k_pos : 0 < k := by
by_contra h
have h_k_eq_0 : k = 0 := by omega
rw [h_k_eq_0] at hk
nlinarith
by_cases h_k_ge_2 : k ≥ 2
·
have h_2_b_ge_2_c : 2 * b ≥ 2 * c := by nlinarith
have h_b_ge_c : b ≥ c := by nlinarith
nlinarith
·
have h_k_lt_2 : k < 2 := by omega
have h_k_eq_1 : k = 1 := by omega
rw [h_k_eq_1] at hk
nlinarith
have h_d_lt_a_k : d < a k := h11
omega
have h_a_k_eq_2_c : a k = 2 * c := by omega
have h_d_dvd_2_c : d | 2 * c := by
have h_d_dvd_a_k : d | a k := h14'
rw [h_a_k_eq_2_c] at h_d_dvd_a_k
simp using h_d_dvd_a_k
have h_d_eq_2_c : d = 2 * c := by
have h_d_dvd_2_c' : d | 2 * c := h_d_dvd_2_c
have h_d_pos : 0 < d := by linarith
have h_c_lt_d' : c < d := h10
have h_exists_k : ∃ k : N, 2 * c = d * k := by
exact h_d_dvd_2_c
rcases h_exists_k with ⟨k, hk⟩
have h_k_pos : 0 < k := by
by_contra h
have h_k_eq_0 : k = 0 := by omega
rw [h_k_eq_0] at hk
nlinarith
by_cases h_k_ge_2 : k ≥ 2
·
have h_2_c_ge_2_d : 2 * c ≥ 2 * d := by nlinarith
have h_c_ge_d : c ≥ d := by nlinarith
nlinarith
·
have h_k_lt_2 : k < 2 := by omega
have h_k_eq_1 : k = 1 := by omega
rw [h_k_eq_1] at hk
nlinarith

```

```

have h_d_lt_a_k : d < a k := h11
rw [h_a_k_eq_2_c, h_d_eq_2_c] at h_d_lt_a_k
linarith

have h_a_k_eq_2_d : a k = 2 * d := by omega
have h_b_dvd_2_d : b | 2 * d := by
  have h_b_dvd_a_k : b | a k := h12'
  rw [h_a_k_eq_2_d] at h_b_dvd_a_k
  simp using h_b_dvd_a_k
have h_b_mode : b % 2 = 0 ∨ b % 2 = 1 := by omega
rcases h_b_mode with (h_b_even | h_b_odd)

have h1 : c % 2 = 0 ∨ c % 2 = 1 := by omega
rcases h1 with (h_c_even | h_c_odd)

have h1 : (b % 3 = 1 ∧ a % 3 = 1 ∧ d % 3 = 1) ∨ (b % 3 = 2 ∧ a % 3 = 2 ∧ d % 3 = 2) := by
  have h1 : b % 3 = 0 ∨ b % 3 = 1 ∨ b % 3 = 2 := by omega
  rcases h1 with (h1 | h1 | h1) <|> omega
  rcases h1 with (h11 | h12)

  have h_b_mod_3 : b % 3 = 1 := h11.1
  have h_c_mod_3 : c % 3 = 1 := h11.2.1
  have h_d_mod_3 : d % 3 = 1 := h11.2.2
  have h_b_mod_6 : b % 6 = 4 := by omega
  have h_c_mod_6 : c % 6 = 4 := by omega
  have h_d_mod_6 : d % 6 = 1 := by omega
  have h_2_div_b_plus_c_plus_d : 2 | b + c + d := by
    have h2_div_a_k_plus_1 : 2 | a (k + 1) :=
      prop_a0_divisible_by_31_two_divides_a_n a hpos h1 (k + 1)
    have h_a_k_plus_1_eq : a (k + 1) = b + c + d := h16
    rw [h_a_k_plus_1_eq] at h2_div_a_k_plus_1
    simp using h2_div_a_k_plus_1
  have h_3_div_b_plus_c_plus_d : 3 | b + c + d := h_3_div_bcd'
  have h_6_div_b_plus_c_plus_d : 6 | b + c + d := by
    omega
  have h_b_plus_c_plus_d_mod_6 : (b + c + d) % 6 = 0 := by omega
  omega

  have h_b_mod_3 : b % 3 = 2 := h12.1
  have h_c_mod_3 : c % 3 = 2 := h12.2.1
  have h_d_mod_3 : d % 3 = 2 := h12.2.2
  have h_b_mod_6 : b % 6 = 2 := by omega
  have h_c_mod_6 : c % 6 = 2 := by omega
  have h_d_even : d % 2 = 0 := by
    have h_b_even : b % 2 = 0 := h_b_even
    have h_c_even : c % 2 = 0 := h_c_even
    have h_b_plus_c_even : (b + c) % 2 = 0 := by omega
    have h2_div_bcd : 2 | b + c + d := by
      have h2_div_a_k_plus_1 : 2 | a (k + 1) :=
        prop_a0_divisible_by_31_two_divides_a_n a hpos h1 (k + 1)
      have h_a_k_plus_1_eq : a (k + 1) = b + c + d := h16
      have h2_div_bcd : 2 | b + c + d := by
        rw [h_a_k_plus_1_eq] at h2_div_a_k_plus_1
        simp using h2_div_a_k_plus_1
      exact h2_div_bcd
    omega
  have h_d_mod_6 : d % 6 = 2 := by omega
  have h_2_div_d : 2 | d := by omega
  have h_exists_m : ∃ m, d = 2 * m := by
    refine' ⟨d / 2, _⟩
  omega
  rcases h_exists_m with m, hm
  have h_a_k_eq_4_m : a k = 4 * m := by
    calc
      a k = 2 * d := by linarith
      _ = 2 * (2 * m) := by rw [hm]
      _ = 4 * m := by ring
  have h_4_div_a_k : 4 | a k := by
    use m
  contradiction

have h_c_odd : c % 2 = 1 := h_c_odd
have h_c_dvd_2_d : c | 2 * d := by simp [h_a_k_eq_2_d] using h13
have h_c_dvd_d : c | d := by
  have h1 : c | 2 * d := h_c_dvd_2_d
  have h2 : c % 2 = 1 := h_c_odd
  have h3 : c | 2 * d := h1
  have h4 : Nat.Coprime c 2 := by
    rw [Nat.coprime_iff_gcd_eq_one]
  have h9 : Nat.gcd c 2 = 1 := by
    have h10 : c % 2 = 1 := h_c_odd
    have h101 : Nat.gcd c 2 | 2 := Nat.gcd_dvd_right c 2
    have h102 : Nat.gcd c 2 ≤ 2 := Nat.le_of_dvd (by norm_num) h101
    interval_cases h : Nat.gcd c 2 <|> norm_num at h101 <|> (try
      {
        have h103 : 2 | c := by
          have h104 : Nat.gcd c 2 = 2 := by omega
          have h105 : 2 | c := by
            have h106 : Nat.gcd c 2 | c := Nat.gcd_dvd_left c 2
            rw [h104] at h106
            exact h106
          exact h105
        omega
      })
    exact h9
  have h10 : c | 2 * d := h3
  have h11 : c | d := by
    exact Nat.Coprime.dvd_of_dvd_mul_left h4 h10
  exact h11
have h_2c_dvd_2d : 2 * c | 2 * d := by
  have h5 : c | d := h_c_dvd_d
  have h6 : ∃ k, d = c * k := by
    exact h_c_dvd_d
  rcases h6 with k, hk
  have h7 : 2 * d = 2 * c * k := by
    calc
      2 * d = 2 * (c * k) := by rw [hk]
      _ = 2 * c * k := by ring
  have h8 : 2 * c | 2 * d := by
    use k
  exact h8
have h_2c_dvd_ak : 2 * c | a k := by
  have h1 : 2 * c | 2 * d := h_2c_dvd_2d
  have h2 : a k = 2 * d := h_a_k_eq_2_d
  rw [h2]
  simp using h1
have h_2c_lt_ak : 2 * c < a k := by
  have h1 : c < d := h10
  have h2 : 2 * c < 2 * d := by linarith
  have h3 : a k = 2 * d := h_a_k_eq_2_d
  linarith
have h15_2b : (2 * b) ≤ b ∨ (2 * b) = c ∨ (2 * b) = d := by
  have h15_1 : (2 * c) < a k := h_2c_lt_ak
  have h15_2 : (2 * c) | a k := h_2c_dvd_ak
  have h15_3 := h15' (2 * c) h15_1 h15_2
  simp using h15_3
have h16 : ¬((2 * c) ≤ b) := by
  have h9 : b < c := h9
  omega
have h17 : ¬((2 * c) = c) := by
  omega
have h18 : (2 * c) = d := by
  rcases h15_2c with (h15_2c | h15_2c | h15_2c) <|> tauto
  have h_d_eq_2c : d = 2 * c := by linarith
  have h3_bcd : 3 | b + c + d := h_3_div_bcd
  have h3_b_plus_3c : 3 | b + 3 * c := by
    have h : b + c + d = b + c + 2 * c := by
      rw [h_d_eq_2c]
    have h1 : b + c + 2 * c = b + 3 * c := by ring
    rw [h, h1] at h3_bcd
    simp using h3_bcd
  have h3_b : 3 | b := by
    have h1 : 3 | b + 3 * c := h3_b_plus_3c
    have h2 : 3 | 3 * c := by
      use c
    omega
  contradiction
have h_b_odd : b % 2 = 1 := h_b_odd
have h_b_dvd_2_d : b | 2 * d := by simp [h_a_k_eq_2_d] using h12
have h_b_dvd_d : b | d := by
  have h1 : b | 2 * d := h_b_dvd_2_d
  have h2 : b % 2 = 1 := h_b_odd
  have h3 : b | 2 * d := h1
  have h4 : Nat.Coprime b 2 := by
    rw [Nat.coprime_iff_gcd_eq_one]
  have h9 : Nat.gcd b 2 = 1 := by
    have h10 : b % 2 = 1 := h_b_odd
    have h101 : Nat.gcd b 2 | 2 := Nat.gcd_dvd_right b 2
    have h102 : Nat.gcd b 2 ≤ 2 := Nat.le_of_dvd (by norm_num) h101
    interval_cases h : Nat.gcd b 2 <|> norm_num at h101 <|> (try {
      have h103 : 2 | b := by
        have h104 : Nat.gcd b 2 = 2 := by omega
        have h105 : 2 | b := by
          have h106 : Nat.gcd b 2 | b := Nat.gcd_dvd_left b 2
          rw [h104] at h106
          exact h106
        exact h105
      omega
    })
    exact h9
  have h10 : b | 2 * d := h3
  have h11 : b | d := by
    exact Nat.Coprime.dvd_of_dvd_mul_left h4 h10
  exact h11
have h_2b_dvd_2d : 2 * b | 2 * d := by
  have h5 : b | d := h_b_dvd_d
  have h6 : ∃ k, d = b * k := by
    exact h_b_dvd_d
  rcases h6 with k, hk
  have h7 : 2 * d = 2 * b * k := by
    calc
      2 * d = 2 * (b * k) := by rw [hk]
      _ = 2 * b * k := by ring
  have h8 : 2 * b | 2 * d := by
    use k
  exact h8
have h_2b_dvd_ak : 2 * b | a k := by
  have h1 : 2 * b | 2 * d := h_2b_dvd_2d
  have h2 : a k = 2 * d := h_a_k_eq_2_d
  rw [h2]
  simp using h1
have h_2b_lt_ak : 2 * b < a k := by
  have h1 : b < d := by linarith
  have h2 : 2 * b < 2 * d := by linarith
  have h3 : a k = 2 * d := h_a_k_eq_2_d
  linarith
have h15_2b : (2 * b) ≤ b ∨ (2 * b) = c ∨ (2 * b) = d := by
  have h15_1 : (2 * b) < a k := h_2b_lt_ak
  have h15_2 : (2 * b) | a k := h_2b_dvd_ak
  have h15_3 := h15' (2 * b) h15_1 h15_2
  simp using h15_3
have h16 : ¬((2 * b) ≤ b) := by
  omega
have h17 : (2 * b) = c ∨ (2 * b) = d := by
  rcases h15_2b with (h15_2b | h15_2b | h15_2b) <|> tauto
rcases h17 with (h17 | h17)

have h_c_eq_2b : c = 2 * b := by linarith
have h3_bcd : 3 | b + c + d := h_3_div_bcd
have h3_3b_plus_d : 3 | 3 * b + d := by
  have h : b + c + d = b + 2 * b + d := by
    rw [h_c_eq_2b]
  have h1 : b + 2 * b + d = 3 * b + d := by ring
  rw [h, h1] at h3_bcd
  simp using h3_bcd
have h3_d : 3 | d := by
  have h1 : 3 | 3 * b + d := h3_3b_plus_d
  have h2 : 3 | 3 * b := by
    use b
  omega
  contradiction
have h_d_eq_2b : d = 2 * b := by linarith
have h3_bcd : 3 | b + c + d := h_3_div_bcd
have h3_3b_plus_c : 3 | 3 * b + c := by
  have h : b + c + d = b + c + 2 * b := by
    rw [h_d_eq_2b]
  have h1 : b + c + 2 * b = 3 * b + c := by ring
  rw [h, h1] at h3_bcd
  simp using h3_bcd
have h3_c : 3 | c := by
  have h1 : 3 | 3 * b + c := h3_3b_plus_c
  have h2 : 3 | 3 * b := by
    use b
  omega
  omega

```



```

contradiction
exfalse
have h9' : b < c := h9
have h2_eq_c : c = 2 := by linarith
rw [h2_eq_c] at h9'
have h9'' : b < 2 := by linarith
have hb_pos : 0 < b := Nat.pos_of_dvd_of_pos h12' (hpos k)
have h12'' : b ≥ 1 := by linarith
have hb_eq_1 : b = 1 := by omega
have h16' : a (k + 1) = b + c + d := h16
have h_3_div_bcd' : 3 | b + c + d := h_3_div_bcd
rw [hb_eq_1, h2_eq_c] at h_3_div_bcd'
have h3_div_d : 3 | d := by
  norm_num at h_3_div_bcd' <|> omega
exact h_not_div_3_d' h_3_div_d

exfalse
have h10' : c < d := h10
have h2_eq_d : d = 2 := by linarith
rw [h2_eq_d] at h10'
have h10'' : c < 2 := by linarith
have h9' : b < c := h9
have hb_pos : 0 < b := Nat.pos_of_dvd_of_pos h12' (hpos k)
have h12'' : b ≥ 1 := by linarith
omega

theorem prop_a0_divisible_by_31_case_j_gt_0_and_not_4_div_ak (a : ℕ → ℕ)
(hpos : ∀ n : ℕ, a n > 0)
(h1 : ∀ n : ℕ, ∃ b c d : ℕ, b < c < a < d < a n ∧ b | a n ∧ c | a n ∧ d | a n
→ n ∧ (∀ e : ℕ, e < a n → e | a n → e ≤ b ∨ e = c ∨ e = d) ∧ a (n + 1) =
→ b + c + d)
(k : ℕ)
(j : ℕ)
(hk : j = k + 1)
(h_not_div_3_ak : ¬ (3 | a k))
(b : ℕ)
(c : ℕ)
(d : ℕ)
(h9 : b < c)
(h10 : c < d)
(h11 : d < a k)
(h12 : b | a k)
(h13 : c | a k)
(h14 : d | a k)
(h15 : ∀ e : ℕ, e < a k → e | a k → e ≤ b ∨ e = c ∨ e = d)
(h16 : a (k + 1) = b + c + d)
(h_3_div_bcd : 3 | b + c + d)
(h_not_div_3_b : ¬ (3 | b))
(h_not_div_3_c : ¬ (3 | c))
(h_not_div_3_d : ¬ (3 | d))
(h_4_div_ak : ¬ (4 | a k)) :
False := by
  apply prop_a0_divisible_by_31_main_contradiction a hpos h1 k b c d
  <|> aesop

theorem prop_a0_divisible_by_31_d_eq_2m (m d : ℕ) (hm_pos : m > 0) (h_dvd : d |
→ 4 * m) (h1 : m * 2 < d) (h2 : d < 4 * m) : d = 2 * m := by
  cases' h_dvd with t ht
  have : t = 1 := by
    nlinarith
  simp_all

theorem prop_a0_divisible_by_31_case_analysis_for_m_times_2
(a : ℕ → ℕ)
(hpos : ∀ n : ℕ, a n > 0)
(h1 : ∀ n : ℕ, ∃ b c d : ℕ, b < c < a < d < a n ∧ b | a n ∧ c | a n ∧ d | a n
→ n ∧ (∀ e : ℕ, e < a n → e | a n → e ≤ b ∨ e = c ∨ e = d) ∧ a (n + 1) =
→ b + c + d)
(k : ℕ)
(b : ℕ)
(c : ℕ)
(d : ℕ)
(h9 : b < c)
(h10 : c < d)
(h11 : d < a k)
(h12 : b | a k)
(h13 : c | a k)
(h14 : d | a k)
(h15 : ∀ e : ℕ, e < a k → e | a k → e ≤ b ∨ e = c ∨ e = d)
(m : ℕ)
(hm : a k = 4 * m)
(h28 : m > 0)
(h29 : m ≥ 2)
(h30 : m + 2 < a k)
(h31 : m + 2 | a k)
(h32 : m + 2 ≤ b ∨ m + 2 = c ∨ m + 2 = d)
(h_3_div_bcd : 3 | b + c + d)
(h_not_div_3_b : ¬ (3 | b))
(h_not_div_3_c : ¬ (3 | c))
(h_not_div_3_d : ¬ (3 | d)) :
False := by
  rcases h32 with (h32 | h32 | h32)

exfalse
have h33 : d | 4 * m := by
  rw [← hm]
  exact h14
have h34 : d = 2 * m := by
  apply prop_a0_divisible_by_31_d_eq_2m
  all_goals omega
linarith
exfalse
have h34 : d | 4 * m := by
  rw [← hm]
  exact h14
have h35 : d = 2 * m := by
  apply prop_a0_divisible_by_31_d_eq_2m
  all_goals omega
linarith
exfalse
have h36 : m * 2 = d := by
  omega
have h37 : d = 2 * m := by

```

```

linarith
have h38 : m < a k := by
  linarith [h28]
have h39 : m | a k := by
  rw [hm]
  use 4
  linarith
have h40 : m ≤ b ∨ m = c ∨ m = d := by
  have h401 := h15 m (by linarith) h39
  tauto
cases h40 with
| inl h40 =>
  have h41 : b < 2 * m := by
    linarith
  have h42 : b | 4 * m := by
    rw [← hm]
    exact h12
  have h43 : ∃ s, 4 * m = b * s := by
    rcases h42 with (s, hs)
    refine' ⟨s, _⟩
    linarith
  rcases h43 with (s, hs)
  have h44 : s > 0 := by
    by_contra h44
    have h441 : s = 0 := by linarith
    rw [h441] at hs
    linarith
  have h45 : s < 5 := by
    by_contra h45
    have h451 : s ≥ 5 := by linarith
    have h46 : 4 * m = b * s := hs
    nlinarith
  have h46 : s = 1 ∨ s = 2 ∨ s = 3 ∨ s = 4 := by omega
  rcases h46 with (h46 | h46 | h46 | h46)

  have h47 : 4 * m = b * 1 := by rw [h46] at hs; linarith
  have h48 : b = 4 * m := by linarith
  linarith

  have h47 : 4 * m = b * 2 := by rw [h46] at hs; linarith
  have h48 : b = 2 * m := by linarith
  linarith

  have h47 : 4 * m = b * 3 := by rw [h46] at hs; linarith
  have h49 : 3 | 4 * m := by
    use b
    linarith
  have h50 : 3 | m := by
    omega
  have h51 : 3 | d := by
    rw [h37]
    exact dvd_mul_of_dvd_right h50 2
  exact h_not_div_3_d h51

  have h47 : 4 * m = b * 4 := by rw [h46] at hs; linarith
  have h48 : b = m := by linarith
  have h49 : m < c := by linarith [h9, h48]
  have h50 : c < d := by linarith
  have h51 : c < 2 * m := by linarith [h37, h50]
  have h52 : 3 | b + c + d := by
    exact h_3_div_bcd
  have h53 : b + c + d = m + c + 2 * m := by
    linarith
  have h54 : 3 | m + c + 2 * m := by
    rw [h53] at h52
    exact h52
  have h55 : 3 | c := by
    omega
  exact h_not_div_3_c h55
| inr h40 =>
  exfalse
  have h401 : m = c := by
    omega
  have h41 : b < m := by
    linarith [h9, h401]
  have h42 : 3 | b + c + d := by
    exact h_3_div_bcd
  have h43 : b + c + d = b + m + 2 * m := by
    linarith
  have h44 : 3 | b + m + 2 * m := by
    rw [h43] at h42
    exact h42
  have h45 : 3 | b + 3 * m := by
    omega
  have h46 : 3 | 3 * m := by
    use m
  have h47 : 3 | b := by
    omega
  exact h_not_div_3_b h47

theorem prop_a0_divisible_by_31_h_main' (a : ℕ → ℕ)
(hpos : ∀ n : ℕ, a n > 0)
(h1 : ∀ n : ℕ, ∃ b c d : ℕ, b < c < a < d < a n ∧ b | a n ∧ c | a n ∧ d | a n
→ n ∧ (∀ e : ℕ, e < a n → e | a n → e ≤ b ∨ e = c ∨ e = d) ∧ a (n + 1) =
→ b + c + d)
(k : ℕ)
(j : ℕ)
(hk : j = k + 1)
(h_not_div_3_ak : ¬ (3 | a k))
(b : ℕ)
(c : ℕ)
(d : ℕ)
(h9 : b < c)
(h10 : c < d)
(h11 : d < a k)
(h12 : b | a k)
(h13 : c | a k)
(h14 : d | a k)
(h15 : ∀ e : ℕ, e < a k → e | a k → e ≤ b ∨ e = c ∨ e = d)
(h16 : a (k + 1) = b + c + d)
(h_3_div_bcd : 3 | b + c + d)
(h_not_div_3_b : ¬ (3 | b))
(h_not_div_3_c : ¬ (3 | c))
(h_not_div_3_d : ¬ (3 | d))
(h_4_div_ak : 4 | a k) :
False := by
  cases' h_4_div_ak with m hm
  have h30 : m + 2 < a k := by omega

```



```

have h31 : m * 2 | a k := by
  use 2
  omega
exact prop_a0_divisible_by_31_case_analysis_for_m_times_2 a hpos h1 k b c d
  → h9 h10 h11 h12 h13 h14 h15 m hm (by omega) (by omega) h30 h31 (by
  → simp_all) h_3_div_bcd h_not_div_3_b h_not_div_3_c h_not_div_3_d

theorem prop_a0_divisible_by_31_case_j_gt_0_and_4_div_ak (a : ℕ → ℕ)
(hpos : ∀ n : ℕ, a n > 0)
(h1 : ∀ n : ℕ, ∃ b c d : ℕ, b < c & c < d & d < a n ∧ b | a n ∧ c | a n ∧ d | a
  → n ∧ (∀ e : ℕ, e < a n → e | a n → e ≤ b ∨ e = c ∨ e = d) ∧ a (n + 1) =
  → b + c + d)
(k : ℕ)
(j : ℕ)
(hk : j = k + 1)
(h_not_div_3_ak : ¬ (3 | a k))
(b : ℕ)
(c : ℕ)
(d : ℕ)
(h9 : b < c)
(h10 : c < d)
(h11 : d < a k)
(h12 : b | a k)
(h13 : c | a k)
(h14 : d | a k)
(h15 : ∀ e : ℕ, e < a k → e | a k → e ≤ b ∨ e = c ∨ e = d)
(h16 : a (k + 1) = b + c + d)
(h_3_div_bcd : 3 | b + c + d)
(h_not_div_3_b : ¬ (3 | b))
(h_not_div_3_c : ¬ (3 | c))
(h_not_div_3_d : ¬ (3 | d))
(h_4_div_ak : 4 | a k)
False := by

exact prop_a0_divisible_by_31_main' a hpos h1 k j hk h_not_div_3_ak b c d
  → h9 h10 h11 h12 h13 h14 h15 h16 h_3_div_bcd h_not_div_3_b
  → h_not_div_3_c h_not_div_3_d h_4_div_ak

theorem prop_a0_divisible_by_31_h3 (a : ℕ → ℕ)
(j : ℕ)
(hj1 : 3 | a j)
(hj2 : ∀ i < j, ¬ (3 | a i))
(h_j_eq_0 : j = 0) :
3 | a 0 := by
simp_all

theorem prop_a0_divisible_by_31_h_j_pos (a : ℕ → ℕ)
(j : ℕ)
(h_j_eq_0 : j ≠ 0) :
j > 0 := by
omega

theorem prop_a0_divisible_by_31_h_contradiction (a : ℕ → ℕ)
(hpos : ∀ n : ℕ, a n > 0)
(h1 : ∀ n : ℕ, ∃ b c d : ℕ, b < c & c < d & d < a n ∧ b | a n ∧ c | a n ∧ d | a
  → n ∧ (∀ e : ℕ, e < a n → e | a n → e ≤ b ∨ e = c ∨ e = d) ∧ a (n + 1) =
  → b + c + d)
(j : ℕ)
(hj1 : 3 | a j)
(hj2 : ∀ i < j, ¬ (3 | a i))
(h_j_pos : j > 0) :
False := by
cases' exists_eq_succ_of_ne_zero (by linarith : j ≠ 0) with k hk
have h_k_lt_j : k < j := by linarith
have h_not_div_3_ak : ¬ (3 | a k) := hj2 k h_k_lt_j
rcases h1 k with ⟨b, c, d, h9, h10, h11, h12, h13, h14, h15, h16⟩
have h_3_div_bcd : 3 | b + c + d := by simp_all
have h_not_div_3_b : ¬ (3 | b) := by
  intro h
  exact h_not_div_3_ak (dvd_trans h h12)
have h_not_div_3_c : ¬ (3 | c) := by
  intro h
  exact h_not_div_3_ak (dvd_trans h h13)
have h_not_div_3_d : ¬ (3 | d) := by
  intro h
  exact h_not_div_3_ak (dvd_trans h h14)
by cases h_4_div_ak : 4 | a k
· exact prop_a0_divisible_by_31_case_j_gt_0_and_4_div_ak a hpos h1 k j hk
  → h_not_div_3_ak b c d h9 h10 h11 h12 h13 h14 h15 h16 h_3_div_bcd
  → h_not_div_3_b h_not_div_3_c h_not_div_3_d h_4_div_ak
· exact prop_a0_divisible_by_31_case_j_gt_0_and_not_4_div_ak a hpos h1 k j hk
  → h_not_div_3_ak b c d h9 h10 h11 h12 h13 h14 h15 h16 h_3_div_bcd
  → h_not_div_3_b h_not_div_3_c h_not_div_3_d h_4_div_ak

theorem prop_a0_divisible_by_3 (a : ℕ → ℕ) (hpos : ∀ n : ℕ, a n > 0) (h1 : ∀ n :
  → ℕ, ∃ b c d : ℕ, b < c & c < d & d < a n ∧ b | a n ∧ c | a n ∧ d | a n
  → (∀ e : ℕ, e < a n → e | a n → e ≤ b ∨ e = c ∨ e = d) ∧ a (n + 1) = b +
  → c + d) (h_exists_first_term_div_3 : ∃ j, 3 | a j) : 3 | a 0 := by
cases' exists_first_term_divisible_by_3 a hpos h1 with j hj
by_cases h_j_eq_0 : j = 0
simp_all
ex falso
apply prop_a0_divisible_by_31_h_contradiction a hpos h1 j hj.1 hj.2
omega

theorem exists_first_term_divisible_by_31_h3 (a : ℕ → ℕ)
(hpos : ∀ n : ℕ, a n > 0)
(h1 : ∀ n : ℕ, ∃ b c d : ℕ, b < c & c < d & d < a n ∧ b | a n ∧ c | a n ∧ d | a
  → n ∧ (∀ e : ℕ, e < a n → e | a n → e ≤ b ∨ e = c ∨ e = d) ∧ a (n + 1) =
  → b + c + d) :
∃ j, 3 | a j := by
by_contra! h
have h' : ∀ n, a (n + 1) < a n := by
  intro n
  obtain ⟨b, c, d, h1b, h2b, h3b, h4b, h5b, h6b, h7b, h8b⟩ := h1 n
  by_contra h16
  have h17 : b + c + d ≥ a n := by linarith [h8b]
  have h18 : d | a n := h6b
  obtain ⟨k, hk⟩ := h18
  have h19 : k ≥ 2 := by linarith
  have h20 : k < 3 := by linarith
  have h21 : k = 2 := by omega
  have h22 : a n = 2 * d := by rw [hk, h21]; linarith
  have h23 : c | 2 * d := by
    have h241 : c | a n := h5b
    rw [h22] at h241
    exact h241
  have h24 : b + c ≥ d := by linarith [h17]
  have h25 : d < 2 * c := by linarith
  have h26 : c > 0 := by omega
  have h27 : d > c := by linarith
  have h28 : ∃ x : ℕ, d = c + x := by
    use d - c
    omega
  rcases h28 with ⟨x, hx⟩
  have h29 : x > 0 := by linarith
  have h30 : x < c := by linarith
  have h31 : c | 2 * x := by
    have h311 : c | 2 * d := h23
    have h312 : d = c + x := hx
    have h313 : 2 * d = 2 * c + 2 * x := by linarith
    have h314 : c | 2 * c + 2 * x := by simp [h313] using h311
    have h315 : c | (2 * c + 2 * x) - 2 * c := Nat.dvd_sub' h314 (by simp)
    have h316 : (2 * c + 2 * x) - 2 * c = 2 * x := by omega
    rw [h316] at h315
    exact h315
  obtain ⟨k, hk⟩ := h31
  have h32 : k < 2 := by linarith
  have h33 : k ≠ 0 := by
    by_contra h331
    have h332 : k = 0 := by linarith
    rw [h332] at hk
    have h333 : 2 * x = 0 := by linarith
    have h334 : x = 0 := by linarith
    linarith
  have h34 : k = 1 := by omega
  have h35 : 2 * x = c := by rw [h34] at hk; linarith
  have h36 : c = 2 * x := by linarith
  have h37 : d = 3 * x := by linarith
  have h38 : a n = 6 * x := by linarith
  have h39 : 3 | a n := by use 2 * x; linarith
  have h49 : ∃ n
  contradiction
have h2 : ∀ n, a n + n ≤ a 0 := by
  intro n
  induction n with
  | zero => simp
  | succ ih =>
    have h326 := h' n
    linarith
  linarith [h2 (a 0 + 1)]

theorem exists_first_term_divisible_by_31_h4 (a : ℕ → ℕ)
(hpos : ∀ n : ℕ, a n > 0)
(h1 : ∀ n : ℕ, ∃ b c d : ℕ, b < c & c < d & d < a n ∧ b | a n ∧ c | a n ∧ d | a
  → n ∧ (∀ e : ℕ, e < a n → e | a n → e ≤ b ∨ e = c ∨ e = d) ∧ a (n + 1) =
  → b + c + d)
(h3 : ∃ j, 3 | a j) :
∃ j, 3 | a j ∧ ∀ i < j, ¬ (3 | a i) := by
have := Nat.find_spec h3
aesop

theorem v2_of_6_not_4_not_51_h11 (a : ℕ → ℕ)
(hpos : ∀ n : ℕ, a n > 0)
(h1 : ∀ n : ℕ, ∃ b c d : ℕ, b < c & c < d & d < a n ∧ b | a n ∧ c | a n ∧ d | a
  → n ∧ (∀ e : ℕ, e < a n → e | a n → e ≤ b ∨ e = c ∨ e = d) ∧ a (n + 1) =
  → b + c + d)
(x : ℕ)
(h_prop : 6 | x ∧ ¬(4 | x) ∧ ¬(5 | x)) :
padicValNat 2 x ≤ 1 := by
  padicValNat
  unfold padicValNat
  aesop

theorem v2_of_6_not_4_not_51_h15 (a : ℕ → ℕ)
(hpos : ∀ n : ℕ, a n > 0)
(h1 : ∀ n : ℕ, ∃ b c d : ℕ, b < c & c < d & d < a n ∧ b | a n ∧ c | a n ∧ d | a
  → n ∧ (∀ e : ℕ, e < a n → e | a n → e ≤ b ∨ e = c ∨ e = d) ∧ a (n + 1) =
  → b + c + d)
(x : ℕ)
(h_prop : 6 | x ∧ ¬(4 | x) ∧ ¬(5 | x)) :
padicValNat 2 x ≠ 0 := by
  simp_all
  omega

theorem v2_of_6_not_4_not_5 (a : ℕ → ℕ) (hpos : ∀ n : ℕ, a n > 0) (h1 : ∀ n : ℕ
  → ∃ b c d : ℕ, b < c & c < d & d < a n ∧ b | a n ∧ c | a n ∧ d | a n
  → (∀ e : ℕ, e < a n → e | a n → e ≤ b ∨ e = c ∨ e = d) ∧ a (n + 1) = b +
  → c + d) (x : ℕ) (h_prop : 6 | x ∧ ¬(4 | x) ∧ ¬(5 | x)) : padicValNat 2 x =
  → 1 := by
  have := v2_of_6_not_4_not_51_h11 a hpos h1 x h_prop
  have := v2_of_6_not_4_not_51_h15 a hpos h1 x h_prop
  omega

theorem v2_decreases_if_div_by_121_main_proof (a : ℕ → ℕ)
(hpos : ∀ n : ℕ, a n > 0)
(h1 : ∀ n : ℕ, ∃ b c d : ℕ, b < c & c < d & d < a n ∧ b | a n ∧ c | a n ∧ d | a
  → n ∧ (∀ e : ℕ, e < a n → e | a n → e ≤ b ∨ e = c ∨ e = d) ∧ a (n + 1) =
  → b + c + d)
(n : ℕ)
(h_div_12 : 12 | a n)
(h_div_4 : 4 | a n)
(h_div_3 : 3 | a n)
(h_bcd_form : ∃ b c d : ℕ, b < c & c < d & d < a n ∧ b | a n ∧ c | a n ∧ d | a
  → n ∧
  (∀ e : ℕ, e < a n → e | a n → e ≤ b ∨ e = c ∨ e = d) ∧ a (n + 1) = b + c +
  → d)
  b = a n / 4 & c = a n / 3 & d = a n / 2) :
padicValNat 2 (a (n + 1)) = padicValNat 2 (a n) - 2 := by
  rcases h_bcd_form with ⟨b, c, d, hb, hc, hd, hb', hc', hd', hbcd'⟩
  obtain ⟨t, ht⟩ := h_div_12
  have h16 : a (n + 1) = 13 * t := by omega
  have h17 : padicValNat 2 (13 * t) = padicValNat 2 13 + padicValNat 2 t := by
    apply padicValNat.mul
    <> norm_num
    <> linarith
  have h171 : padicValNat 2 13 = 0 := by norm_num
  have h1721 : padicValNat 2 (12 * t) = padicValNat 2 12 + padicValNat 2 t :=
    by
      apply padicValNat.mul
      <> norm_num
      <> linarith
  have h_padicValNat_2_4 : padicValNat 2 4 = 2 := by

```

```

have h1 : padicValNat 2 (2 ^ 2) = 2 := by
  rw [padicValNat.pow]
  <|> norm_num
norm_num at h1 <|> simp using h1
have h1722 : padicValNat 2 12 = 2 := by
  have h111 : padicValNat 2 (4 * 3) = padicValNat 2 4 + padicValNat 2 3 := by
    apply padicValNat.mul
    <|> norm_num
  have h112 : padicValNat 2 (4 * 3) = 2 := by
    rw [h111, h_padicValNat_2_4, padicValNat.eq_zero_of_not_dvd (by norm_num
      → : ¬ 2 ∣ 3)]
    norm_num at h112 <|> tauto
simp_all

theorem v2_decreases_if_div_by_12 (a : ℕ → ℕ) (hpos : ∀ n : ℕ, a n > 0) (h1 : ∀
  → n : ℕ, ∃ b c d : ℕ, b < c ∧ c < d ∧ d < a ∧ b ∣ a ∧ c ∣ a ∧ d ∣ a
  → a n ∧ (∀ e : ℕ, e < a n → e ∣ a n → e ≤ b ∨ e = c ∨ e = d) ∧ a (n + 1)
  → b + c + d) (n : ℕ) (h_div_12 : 12 ∣ a n) (h_div_4 : 4 ∣ a n)
  → (h_div_3 : 3 ∣ a n) (h_bcd_form : ∃ b c d : ℕ, b < c ∧ c < d ∧ d < a n
  → a b ∣ a n ∧ c ∣ a n ∧ d ∣ a n)
  (∀ e : ℕ, e < a n → e ∣ a n → e ≤ b ∨ e = c ∨ e = d) ∧ a (n + 1) = b + c +
  → d
  b = a n / 4 ∧ c = a n / 3 ∧ d = a n / 2 :
  padicValNat 2 (a (n + 1)) = padicValNat 2 (a n) - 2 := by
  apply v2_decreases_if_div_by_121_main_proof
  <|> assumption

theorem valuation_of_3_of_sum_of_divisors1_main (a : ℕ → ℕ)
  (hpos : ∀ n : ℕ, a n > 0)
  (h1 : ∀ n : ℕ, ∃ b c d : ℕ, b < c ∧ c < d ∧ d < a ∧ b ∣ a ∧ c ∣ a ∧ d ∣ a
  → a n ∧ (∀ e : ℕ, e < a n → e ∣ a n → e ≤ b ∨ e = c ∨ e = d) ∧ a (n + 1) =
  → b + c + d)
  (x : ℕ)
  (h_div_3 : 3 ∣ x)
  (h_div_4 : 4 ∣ x)
  (h12 : 12 ∣ x) :
  padicValNat 3 (x / 2 + x / 3 + x / 4) = padicValNat 3 x - 1 := by
  cases' h12 with k hk
  by_cases h_k : k = 0
  · simp_all
  have h1' : x / 2 = 6 * k := by omega
  have h2' : x / 3 = 4 * k := by omega
  have h3' : x / 4 = 3 * k := by omega
  have h4' : x / 2 + x / 3 + x / 4 = 13 * k := by linarith
  have h5 : x = 3 * (4 * k) := by linarith
  have h6 : padicValNat 3 (3 * (4 * k)) = 1 + padicValNat 3 (4 * k) := by
    rw [padicValNat.mul]
    <|> norm_num
    <|> omega
  have h7 : padicValNat 3 (4 * k) = padicValNat 3 k := by
    rw [padicValNat.mul]
    <|> norm_num
    <|> omega
  simp_all [padicValNat.mul, h7, h6]
  <|> omega

theorem valuation_of_3_of_sum_of_divisors (a : ℕ → ℕ) (hpos : ∀ n : ℕ, a n >
  → 0) (h1 : ∀ n : ℕ, ∃ b c d : ℕ, b < c ∧ c < d ∧ d < a ∧ b ∣ a ∧ c ∣ a ∧ d
  → a n ∧ (∀ e : ℕ, e < a n → e ∣ a n → e ≤ b ∨ e = c ∨ e = d) ∧ a (n + 1) =
  → b + c + d) (x : ℕ) (h_div_3 : 3 ∣ x) (h_div_4 : 4 ∣ x) :
  padicValNat 3 (x / 2 + x / 3 + x / 4) = padicValNat 3 x - 1 := by
  apply valuation_of_3_of_sum_of_divisors1_main a hpos h1 x
  <|> omega

theorem round1_h_bcd_form (a : ℕ → ℕ) (hpos : ∀ n : ℕ, a n > 0) (h1 : ∀ n : ℕ,
  → b c d : ℕ, b < c ∧ c < d ∧ d < a ∧ b ∣ a ∧ c ∣ a ∧ d ∣ a ∧ (∀ e
  → : ℕ, e < a n → e ∣ a n → e ≤ b ∨ e = c ∨ e = d) ∧ a (n + 1) = b + c +
  → d) (k : ℕ) (h12 : 12 ∣ a k) :
  ∃ b c d : ℕ, b < c ∧ c < d < a k ∧ b ∣ a k ∧ c ∣ a k ∧ d ∣ a k ∧ (∀ e : ℕ, e
  → : a k → e ∣ a k → e ≤ b ∨ e = c ∨ e = d) ∧ a (k + 1) = b + c + d ∧ b =
  → a k / 4 ∧ c = a k / 3 ∧ d = a k / 2 := by
  rcases h1 k with ⟨b, c, d, h11, h121, h122, h123, h124, h125, h126, h127⟩
  use b, c, d
  have h13 : a k > 0 := hpos k
  have h14 : 4 ∣ a k := by omega
  have h15 : 3 ∣ a k := by omega
  have h16 : 2 ∣ a k := by omega
  have h17 : a k / 2 ∣ a k := Nat.div_dvd_of_dvd h16
  have h18 : a k / 3 ∣ a k := Nat.div_dvd_of_dvd h15
  have h19 : a k / 4 ∣ a k := Nat.div_dvd_of_dvd h14
  have h20 : a k / 2 < a k := by omega
  have h21 : a k / 3 < a k := by omega
  have h22 : a k / 4 < a k := by omega
  have h23 : d ≤ a k / 2 := by
    by_contra h
    have h_exists_m : ∃ m, a k = d * m := h125
    rcases h_exists_m with ⟨m, hm⟩
    have h_m_pos : 0 < m := by
      by_contra h_m_nonpos
      have h_m_le_zero : m ≤ 0 := by linarith
      have h_m_eq_zero : m = 0 := by omega
      rw [h_m_eq_zero] at hm
      linarith
    have h_d_mul_m_lt_2_d : d * m < 2 * d := by
      have h1 : a k < 2 * d := by omega
      nlinarith
    have h_m_lt_2 : m < 2 := by nlinarith
    have h_m_ge_1 : m ≥ 1 := by linarith
    have h_m_eq_1 : m = 1 := by omega
    rw [h_m_eq_1] at hm
    have h_ak_eq_d : a k = d := by linarith
    linarith
  have h30 : d = a k / 2 := by
    rcases h126 (a k / 2) (by linarith) h17 with (h301 ∣ h302 ∣ h303)
    · linarith
    · linarith
    · linarith
  have h31 : c = a k / 3 := by
    have h311 : a k / 3 ∣ a k := h18
    have h312 : a k / 3 < a k := by linarith
    have h313 := h126 (a k / 3) (by linarith) h311
    have h314 : a k / 3 = c ∨ a k / 3 ≤ b := by
      have h315 : d = a k / 2 := h30
      have h317 : a k / 3 < a k / 2 := by omega
      omega
  cases h314 with
  | inl h314 =>
    linarith
  | inr h314 =>
    have h3141 : a k / 3 < b := h314
    have h3142 : b < c := h11
    have h3143 : c < d := h121
    have h3144 : d = a k / 2 := h30
    have h3145 : c < a k / 2 := by linarith
    have h_b_pos : 0 < b := by
      have h3146 : b ∣ a k := h123
      exact Nat.pos_of_dvd_of_pos h3146 (by linarith)
    have h_c_pos : 0 < c := by
      have h3146 : c ∣ a k := h124
      exact Nat.pos_of_dvd_of_pos h3146 (by linarith)
    have h3147 : ∃ m, a k = b * m := by
      exact h123
    rcases h3147 with ⟨m, hm⟩
    have h3148 : m ≤ 3 := by
      have h3149 : a k / 3 ≤ b := h3141
      have h3150 : a k ≤ 3 * b := by omega
      nlinarith
    have h3149 : ∃ n, a k = c * n := by
      exact h124
    rcases h3149 with ⟨n, hn⟩
    have h3150 : n ≥ 3 := by
      have h3151 : c < a k / 2 := by linarith
      have h3152 : 2 * c < a k := by omega
      nlinarith
    have h3153 : b * m = c * n := by nlinarith
    have h3154 : b < c := h3142
    nlinarith
  have h32 : b = a k / 4 := by
    have h321 : c = a k / 3 := h31
    have h322 : b < c := h11
    have h323 : b < a k / 3 := by linarith
    have h324 : a k / 4 ∣ a k := h19
    have h325 : a k / 4 < a k := by linarith
    have h326 := h126 (a k / 4) (by linarith) h324
    have h327 : a k / 4 ≤ b := by
      have h328 : d = a k / 2 := h30
      have h329 : a k / 4 < a k / 2 := by omega
      omega
    by_cases h328 : b > a k / 4
    · have h3281 : a k / 4 < b := by linarith
      have h3282 : 0 < b := by
        have h3283 : b ∣ a k := h123
        exact Nat.pos_of_dvd_of_pos h3283 (by linarith)
      have h3284 : ∃ p, a k = b * p := by
        exact h123
      rcases h3284 with ⟨p, hp⟩
      have h3285 : p ≤ 3 := by
        have h3286 : a k / 4 < b := h3281
        have h3287 : a k < 4 * b := by omega
        nlinarith
      have h3286 : p ≥ 4 := by
        have h3289 : b < a k / 3 := h323
        have h3290 : 3 * b < a k := by omega
        nlinarith
      omega
    · have h328 : b ≤ a k / 4 := by linarith
      exact by omega
    simp_all

theorem round1_h1_prime (a : ℕ → ℕ) (hpos : ∀ n : ℕ, a n > 0) (h1 : ∀ n : ℕ,
  → b c d : ℕ, b < c ∧ c < d < a ∧ b ∣ a ∧ c ∣ a ∧ d ∣ a ∧ (∀ e
  → : ℕ, e < a n → e ∣ a n → e ≤ b ∨ e = c ∨ e = d) ∧ a (n + 1) = b + c +
  → d) :
  ∀ k : ℕ, (∀ i < k, 12 ∣ a i) → padicValNat 2 (a k) = padicValNat 2 (a 0) - 2 *
  → k ∧ padicValNat 3 (a k) = padicValNat 3 (a 0) - k := by
  intro k h2
  induction' k with k ih
  simp
  have h21 : ∀ i < k, 12 ∣ a i := by
    intro i hi
    exact h2 i (by linarith)
  have h23 : 12 ∣ a k := h2 k (by linarith)
  rcases round1_h_bcd_form a hpos h1 k h23 with ⟨b, c, d, h28, h29, h30, h31,
  → h32, h33, h34, h35, h36, h37, h38⟩
  rcases h21 with ⟨h51, h52⟩
  have h66 : padicValNat 2 (a (k + 1)) = padicValNat 2 (a k) - 2 := by
    apply v2_decreases_if_div_by_12 a hpos h1 k h23 (by omega) (by omega)
    aesop
  have h67 : padicValNat 3 (a (k + 1)) = padicValNat 3 (a k) - 1 := by
    have h68 : a (k + 1) = b + c + d := h35
    have h69 : b = a k / 4 := h36
    have h70 : c = a k / 3 := h37
    have h71 : d = a k / 2 := h38
    have h72 : a (k + 1) = a k / 4 + a k / 3 + a k / 2 := by linarith
    have h73 : a (k + 1) = a k / 2 + a k / 3 + a k / 4 := by linarith
    have h74 : padicValNat 3 (a k / 2 + a k / 3 + a k / 4) = padicValNat 3 (a
    → k) - 1 := by
      apply valuation_of_3_of_sum_of_divisors a hpos h1 (a k) (by omega) (by
      → omega)
    rw [h73]
    exact h74
  constructor <|> omega

theorem a_k_becomes_6m_form_after_k_steps_of_reduction (a : ℕ → ℕ) (hpos : ∀ n
  → : ℕ, a n > 0) (h1 : ∀ n : ℕ, ∃ b c d : ℕ, b < c ∧ c < d < a ∧ b ∣ a ∧ c
  → a n ∧ (∀ e : ℕ, e < a n → e ∣ a n → e ≤ b ∨ e = c ∨ e = d) ∧ a (n + 1) =
  → b + c + d) (a : ℕ) (h2 : 12 ∣ a) :
  ∃ k : ℕ, (12 ∣ a k) := by
  by_contra! h
  have : a_k_becomes_6m_form_after_k_steps_of_reduction a hpos h1
  → (padicValNat 2 (a 0) + 1)

```

```

    (by aesop)
have := one_le_padicValNat_of_dvd (hpos _) (Nat.dvd_trans (by norm_num : 2 |
  → 12) (h (padicValNat 2 (a 0) + 1)))
omega

theorem round1_h_3_div_a0 (a : ℕ → ℕ)
(hpos : ∀ n : ℕ, a n > 0)
(h1 : ∀ n : ℕ, ∃ b c d : ℕ, b < c ∧ c < d ∧ d < a ∧ b | a n ∧ c | a n ∧ d | a n
  → n ∧ (∀ e : ℕ, e < a → e | a n → e ≤ b ∨ e = c ∨ e = d) ∧ a (n + 1) =
  → b + c + d) :
3 | a 0 := by
  apply prop_a0_divisible_by_3 a hpos h1
have := exists_first_term_divisible_by_3 a hpos h1
aesop

theorem round1_h_main_lemma :
∀ (m : ℕ), m > 0 → ∃ s m, m = 2 ^ s * m' ∧ (2 | m) := by
  intro m hm_pos
  by_cases h : 2 | m
  · obtain s, m, h_t_eq, h_m'_not_div_2 := round1_h_main_lemma (m / 2) (by
    → omega)
    use s + 1, m
    simp_all
    ring_nf at h_t_eq
    omega
  · use 0, m
    simp_all

theorem round1_h_a0_pos (a : ℕ → ℕ)
(hpos : ∀ n : ℕ, a n > 0) :
a 0 > 0 := by
  simp_all

theorem round1_h_main (a : ℕ → ℕ)
(hpos : ∀ n : ℕ, a n > 0)
(h_3_div_a0 : 3 | a 0)
(h_a0_pos : a 0 > 0) :
padicValNat 3 (a 0) ≥ 1 := by
  apply one_le_padicValNat_of_dvd
  assumption'

theorem round1_h_padicValNat_3_a0_ge_1 (a : ℕ → ℕ)
(hpos : ∀ n : ℕ, a n > 0)
(h1 : ∀ n : ℕ, ∃ b c d : ℕ, b < c ∧ c < d ∧ d < a ∧ b | a n ∧ c | a n ∧ d | a n
  → n ∧ (∀ e : ℕ, e < a → e | a n → e ≤ b ∨ e = c ∨ e = d) ∧ a (n + 1) =
  → b + c + d)
(h_3_div_a0 : 3 | a 0) :
padicValNat 3 (a 0) ≥ 1 := by
  unfold padicValNat
  simp_all

theorem round1_coprime_m_10 (m : ℕ) (h2 : ¬(2 | m)) (h5 : ¬(5 | m)) :
→ Nat.Coprime m 10 := by
  rw [Nat.coprime_iff_gcd_eq_one]
  have := Nat.gcd_dvd_left m 10
  have := Nat.gcd_dvd_right m 10
  have h10 := Nat.le_of_dvd (by norm_num) this
  interval_cases m.gcd 10 <|> omega

theorem round1_main_proof (a : ℕ → ℕ) (hpos : ∀ n : ℕ, a n > 0)
(h1 : ∀ n : ℕ, ∃ b c d : ℕ, b < c ∧ c < d ∧ d < a ∧ b | a n ∧ c | a n ∧ d | a n
  → n ∧ (∀ e : ℕ, e < a → e | a n → e ≤ b ∨ e = c ∨ e = d) ∧ a (n + 1) =
  → b + c + d)
(m : ℕ) (hm : a 0 = 6 * m) (h11 : ¬(5 | m)) (h14 : ¬(2 | m)) :
Nat.Coprime m 10 := by
  apply round1_coprime_m_10
  assumption'

theorem round1_h_3_div_a0' (a : ℕ → ℕ)
(hpos : ∀ n : ℕ, a n > 0)
(h1 : ∀ n : ℕ, ∃ b c d : ℕ, b < c ∧ c < d ∧ d < a ∧ b | a n ∧ c | a n ∧ d | a n
  → n ∧ (∀ e : ℕ, e < a → e | a n → e ≤ b ∨ e = c ∨ e = d) ∧ a (n + 1) =
  → b + c + d)
(h_exists_j_div_3 : ∃ j, 3 | a j) :
3 | a 0 := by
  apply prop_a0_divisible_by_3
  all_goals assumption

theorem round1_h_a0_even (a : ℕ → ℕ)
(hpos : ∀ n : ℕ, a n > 0)
(h1 : ∀ n : ℕ, ∃ b c d : ℕ, b < c ∧ c < d ∧ d < a ∧ b | a n ∧ c | a n ∧ d | a n
  → n ∧ (∀ e : ℕ, e < a → e | a n → e ≤ b ∨ e = c ∨ e = d) ∧ a (n + 1) =
  → b + c + d) :
Even (a 0) := by
  apply a0_is_even
  <|> assumption

theorem round1_h_exists_j_div_3 (a : ℕ → ℕ)
(hpos : ∀ n : ℕ, a n > 0)
(h1 : ∀ n : ℕ, ∃ b c d : ℕ, b < c ∧ c < d ∧ d < a ∧ b | a n ∧ c | a n ∧ d | a n
  → n ∧ (∀ e : ℕ, e < a → e | a n → e ≤ b ∨ e = c ∨ e = d) ∧ a (n + 1) =
  → b + c + d) :
∃ j, 3 | a j := by
  have := exists_first_term_divisible_by_3 a hpos h1
  aesop

theorem round2_h2 (a : ℕ → ℕ)
(hpos : ∀ n : ℕ, a n > 0)
(h1 : ∀ n : ℕ, ∃ b c d : ℕ, b < c ∧ c < d ∧ d < a ∧ b | a n ∧ c | a n ∧ d | a n
  → n ∧ (∀ e : ℕ, e < a → e | a n → e ≤ b ∨ e = c ∨ e = d) ∧ a (n + 1) =
  → b + c + d) :
2 | a 0 := by
  apply prop_a0_divisible_by_31_two_divides_a_n
  all_goals simp_all

theorem round2_h3 (a : ℕ → ℕ)
(hpos : ∀ n : ℕ, a n > 0)
(h1 : ∀ n : ℕ, ∃ b c d : ℕ, b < c ∧ c < d ∧ d < a ∧ b | a n ∧ c | a n ∧ d | a n
  → n ∧ (∀ e : ℕ, e < a → e | a n → e ≤ b ∨ e = c ∨ e = d) ∧ a (n + 1) =
  → b + c + d) :
3 | a 0 := by
  simp_all [round1_h_3_div_a0', round1_h_exists_j_div_3]

theorem round1_step1 (a : ℕ → ℕ) (hpos : ∀ n : ℕ, a n > 0) (h1 : ∀ n : ℕ, ∃ b c
  → d : ℕ, b < c ∧ c < d ∧ d < a ∧ b | a n ∧ c | a n ∧ d | a n ∧ (∀ e : ℕ,

```

```

  → e < a → e | a n → e ≤ b ∨ e = c ∨ e = d) ∧ a (n + 1) = b + c + d) :
  → 2 | a 0 ∧ 3 | a 0 := by
  simp_all [round2_h2, round2_h3]

theorem round1_h_exists_m (a : ℕ → ℕ)
(hpos : ∀ n : ℕ, a n > 0)
(h1 : ∀ n : ℕ, ∃ b c d : ℕ, b < c ∧ c < d ∧ d < a ∧ b | a n ∧ c | a n ∧ d | a n
  → n ∧ (∀ e : ℕ, e < a → e | a n → e ≤ b ∨ e = c ∨ e = d) ∧ a (n + 1) =
  → b + c + d)
(h_6_div_a0 : 6 | a 0) :
∃ m, a 0 = 6 * m := by
  aesop

theorem round1_hb (a : ℕ → ℕ) (hpos : ∀ n : ℕ, a n > 0) (h1 : ∀ n : ℕ, ∃ b c d
  → n, b < c ∧ c < d ∧ d < a ∧ b | a n ∧ c | a n ∧ d | a n ∧ (∀ e : ℕ, e
  → < a → e | a n → e ≤ b ∨ e = c ∨ e = d) ∧ a (n + 1) = b + c + d) : ∀
  n : ℕ, 2 | a n := by
  intros
  have := round1_step1 (fun k => a (k + n)) (fun k => hpos (k + n)) (fun k =>
  → by
  simp [Nat.add_assoc, Nat.add_comm, Nat.add_left_comm] using h1 (k + n))
  simp_all

theorem round1_h_2_divides_a_n (a : ℕ → ℕ) (hpos : ∀ n : ℕ, a n > 0) (h1 : ∀ n
  → n, ∃ b c d : ℕ, b < c ∧ c < d ∧ d < a ∧ b | a n ∧ c | a n ∧ d | a n ∧
  → (∀ e : ℕ, e < a → e | a n → e ≤ b ∨ e = c ∨ e = d) ∧ a (n + 1) = b +
  → c + d) : ∀ n : ℕ, 2 | a n := by
  apply round1_hb
  <|> simp_all

theorem round1_h_3_div_a0'' (a : ℕ → ℕ)
(hpos : ∀ n : ℕ, a n > 0)
(h1 : ∀ n : ℕ, ∃ b c d : ℕ, b < c ∧ c < d ∧ d < a ∧ b | a n ∧ c | a n ∧ d | a n
  → n ∧ (∀ e : ℕ, e < a → e | a n → e ≤ b ∨ e = c ∨ e = d) ∧ a (n + 1) =
  → b + c + d)
(h_exists_j_div_3 : ∃ j, 3 | a j) :
3 | a 0 := by
  apply prop_a0_divisible_by_3
  assumption'

theorem round3_h_main (a : ℕ → ℕ) (hpos : ∀ n : ℕ, a n > 0) (h1 : ∀ n : ℕ, ∃ b
  → c d : ℕ, b < c ∧ c < d ∧ d < a ∧ b | a n ∧ c | a n ∧ d | a n ∧ (∀ e : ℕ
  → , e < a → e | a n → e ≤ b ∨ e = c ∨ e = d) ∧ a (n + 1) = b + c + d)
  → : ∀ n : ℕ, 3 | a n := by
  intro n
  apply round1_h_3_div_a0'' _ (fun m => hpos (n + m)) (fun m => h1 (n + m))
  apply round1_h_exists_j_div_3 _ (fun m => hpos (n + m)) (fun m => h1 (n + m))

theorem round1_h_3_divides_a_n (a : ℕ → ℕ) (hpos : ∀ n : ℕ, a n > 0) (h1 : ∀ n
  → n, ∃ b c d : ℕ, b < c ∧ c < d ∧ d < a ∧ b | a n ∧ c | a n ∧ d | a n ∧
  → (∀ e : ℕ, e < a → e | a n → e ≤ b ∨ e = c ∨ e = d) ∧ a (n + 1) = b +
  → c + d) : ∀ n : ℕ, 3 | a n := by
  apply round3_h_main
  <|> assumption

theorem val_5_of_a_succ_if_div_12_h_d_le_an_div_2 (a : ℕ → ℕ) (hpos : ∀ n : ℕ,
  → a n > 0) (n : ℕ) (d : ℕ) (h1_d_dvd_an : d | a n) (h1_d_lt_an : d < a
  → n) : d ≤ a n / 2 := by
  cases' h1_d_dvd_an with k hk
  have := hpos n
  simp_all [Nat.le_div_iff_mul_le]
  nlinarith

theorem val_5_of_a_succ_if_div_12_h_b_lt_an_div_2 (a : ℕ → ℕ) (hpos : ∀ n : ℕ,
  → a n > 0) (n : ℕ) (b c d : ℕ) (h1_b_lt_c : b < c) (h1_c_lt_d : c < d)
  → (h1_d_lt_an : d < a n) (h1_d_dvd_an : d | a n) (h1_d_le_an_div_2 : d ≤
  → a n / 2) : b < a n / 2 := by
  omega

theorem val_5_of_a_succ_if_div_12_h_eq_an_div_2 (a : ℕ → ℕ) (hpos : ∀ n : ℕ,
  → a n > 0) (n : ℕ) (b c d : ℕ) (h1_b_lt_c : b < c) (h1_c_lt_d : c < d)
  → (h1_d_lt_an : d < a n) (h1_b_dvd_an : b | a n) (h1_c_dvd_an : c | a n)
  → (h1_d_dvd_an : d | a n) (h1_forall : ∀ e : ℕ, e < a → e | a n → e ≤
  → b ∨ e = c ∨ e = d) (h3_dvd_an : 3 | a n) (h_d_eq_an_div_2 : d = a n /
  → 2) (h12 : 12 | a n) : c = a n / 3 := by
  rcases h1_forall (a n / 3) (by omega) (Nat.dvd_div_of_dvd h3_dvd_an) with
  → (h2 | h3)
  · ex falso
  · rcases h1_c_dvd_an with k, hk
    have : 2 * c < a n := by omega
    have : a n < 3 * c := by omega
    have : c * k < 3 * c := by nlinarith
    have : k < 3 := by nlinarith
    have : 2 < k := by nlinarith
    omega
  omega

theorem val_5_of_a_succ_if_div_12_h_b_eq_an_div_4 (a : ℕ → ℕ) (hpos : ∀ n : ℕ,
  → a n > 0) (n : ℕ) (b c d : ℕ) (h1_b_lt_c : b < c) (h1_c_lt_d : c < d)
  → (h1_d_lt_an : d < a n) (h1_b_dvd_an : b | a n) (h1_c_dvd_an : c | a n)
  → (h1_d_dvd_an : d | a n) (h1_forall : ∀ e : ℕ, e < a → e | a n → e ≤
  → b ∨ e = c ∨ e = d) (h4_dvd_an : 4 | a n) (h_c_eq_an_div_3 : c = a n /
  → 3) (h_d_eq_an_div_2 : d = a n / 2) (h12 : 12 | a n) : b = a n / 4 :=
  → by
  obtain k, hk := h1_b_dvd_an
  have h80 := h1_forall (a n / 4) (by omega) (Nat.dvd_div_of_dvd h4_dvd_an)
  have h1151 : 3 * b < a n := by omega
  have h1141 : a n ≤ 4 * b := by omega
  have h120 : k = 4 := by nlinarith
  simp_all

theorem val_5_of_a_succ_if_div_12_h_main (a : ℕ → ℕ) (hpos : ∀ n : ℕ, a n > 0)
  → (h1 : ∀ n : ℕ, ∃ b c d : ℕ, b < c ∧ c < d ∧ d < a ∧ b | a n ∧ c | a n
  → d | a n ∧ (∀ e : ℕ, e < a → e | a n → e ≤ b ∨ e = c ∨ e = d) ∧ a (n
  → + 1) = b + c + d) : ∀ n, 12 | a n → padicValNat 5 (a (n + 1)) =
  → padicValNat 5 (a n) := by

```

```

intro n h12
obtain b, c, d, h1_b_lt_c, h1_c_lt_d, h1_d_lt_an, h1_b_dvd_an, h1_c_dvd_an,
  → h1_d_dvd_an, h1_forall, h1_a_succ := h1 n
have h2_dvd_an : 2 ∣ a n := by omega
have h3_dvd_an : 3 ∣ a n := by omega
have h4_dvd_an : 4 ∣ a n := by omega
have h_b_lt_an_div_2 : b < a n / 2 :=
  → val_5_of_a_succ_if_div_12 h_b_lt_an_div_2 a hpos n b c d h1_b_lt_c
  → h1_c_lt_d h1_d_lt_an h1_d_dvd_an
  → (val_5_of_a_succ_if_div_12 h_d_le_an_div_2 a hpos n d h1_d_dvd_an
    → h1_d_lt_an)
have h_d_eq_an_div_2 : d = a n / 2 :=
  → val_5_of_a_succ_if_div_12 h_d_eq_an_div_2 a hpos n b c d h1_b_lt_c
  → h1_c_lt_d h1_d_lt_an h1_b_dvd_an h1_c_dvd_an h1_d_dvd_an h1_forall
  → h2_dvd_an h_b_lt_an_div_2 (val_5_of_a_succ_if_div_12 h_d_le_an_div_2
    → a hpos n d h1_d_dvd_an h1_d_lt_an)
have h_c_eq_an_div_3 : c = a n / 3 :=
  → val_5_of_a_succ_if_div_12 h_c_eq_an_div_3 a hpos n b c d h1_b_lt_c
  → h1_c_lt_d h1_d_lt_an h1_b_dvd_an h1_c_dvd_an h1_d_dvd_an h1_forall
  → h3_dvd_an h_d_eq_an_div_2 h12
have h_b_eq_an_div_4 : b = a n / 4 :=
  → val_5_of_a_succ_if_div_12 h_b_eq_an_div_4 a hpos n b c d h1_b_lt_c
  → h1_c_lt_d h1_d_lt_an h1_b_dvd_an h1_c_dvd_an h1_d_dvd_an h1_forall
  → h4_dvd_an h_c_eq_an_div_3 h_d_eq_an_div_2 h12
have h121 : ∃ k, a n = 12 * k := (a n / 12, by omega)
obtain k, hk_an := h121
have h122 : a (n + 1) = 13 * k := by
  rw [h1_a_succ, h_b_eq_an_div_4, h_c_eq_an_div_3, h_d_eq_an_div_2]
  omega
have h12k_eq : padicValNat 5 (12 * k) = padicValNat 5 k := by
  have h5_prime : Nat.Prime 5 := by norm_num
  have h5 : Fact (Nat.Prime 5) := h5_prime
  rw [padicValNat.mul (by norm_num) (by linarith)]
  norm_num [padicValNat]
have h12k_eq2 : padicValNat 5 (13 * k) = padicValNat 5 k := by
  have h5_prime : Nat.Prime 5 := by norm_num
  have h5 : Fact (Nat.Prime 5) := h5_prime
  rw [padicValNat.mul (by norm_num) (by linarith)]
  norm_num [padicValNat]
simp.all

theorem val_5_of_a_succ_if_div_12 (a : ℕ → ℕ) (hpos : ∀ n : ℕ, a n > 0) (h1 : ∀
  → n : ℕ, ∃ b c d : ℕ, b < c ∧ c < d ∧ d < a n ∧ b ∣ a n ∧ c ∣ a n ∧ d ∣
  → a n ∧ (∀ e : ℕ, e < a n → e ∣ a n → e ≤ b ∨ e = c ∨ e = d) ∧ a (n + 1)
  → b + c + d) : ∀ n, 12 ∣ a n → padicValNat 5 (a (n+1)) = padicValNat 5
  → (a n) := by
  simp.all [val_5_of_a_succ_if_div_12 h_main]

theorem exists_first_k_not_divisible_by_12_and_divisible_by_5_main_proof (a : ℕ
  → ℕ) (hpos : ∀ n : ℕ, a n > 0) (h1 : ∀ n : ℕ, ∃ b c d : ℕ, b < c ∧ c < d
  → d < a n ∧ b ∣ a n ∧ c ∣ a n ∧ d ∣ a n ∧ (∀ e : ℕ, e < a n → e ∣ a n
  → e ≤ b ∨ e = c ∨ e = d) ∧ a (n + 1) = b + c + d) (h5_div : 5 ∣ a
  → 0) :
  ∃ k, ¬ (12 ∣ a k) ∧ (5 ∣ a k) := by
  by_contra h
  push_neg at h
  have h1' : ∀ k, 12 ∣ a k ∨ ¬ (5 ∣ a k) := by
    intro k
    by_cases h12 : 12 ∣ a k
    · left; exact h12
    · right; by_contra h5; exact h k h12 h5
  have h5_div_all : ∀ n : ℕ, 5 ∣ a n := by
    intro n
    induction n with
    | zero => exact h5_div
    | succ n ih =>
      cases' h1' n with h12_div_an h5_div_an
      · have h15 := val_5_of_a_succ_if_div_12 a hpos h1 n h12_div_an
        have h17 : padicValNat 5 (a n) ≥ 1 := by
          by_contra h17
          simp_all [padicValNat]
        have h18 : padicValNat 5 (a (n + 1)) ≥ 1 := by linarith [h15, h17]
        have h5_div_an1 : 5 ∣ a (n + 1) := by
          by_contra h21
          have h22 : ¬ (5 ∣ a (n + 1)) := h21
          have h23 : padicValNat 5 (a (n + 1)) = 0 := by simp [padicValNat]
          <| aesop
          linarith
          exact h5_div_an1
          contradiction
        obtain k, hk := round1_h_exists_k a hpos h1
        exfalse
        have h12_div_an : 12 ∣ a k := by tauto
        contradiction
      · apply exists_first_k_not_divisible_by_12_and_divisible_by_5_main_proof
        <| aesop

theorem if_a_n_is_30k_then_a_n_plus_1_is_odd_main_proof (a : ℕ → ℕ) (hpos : ∀
  → n : ℕ, a n > 0)
(h1 : ∀ n : ℕ, ∃ b c d : ℕ, b < c ∧ c < d ∧ d < a n ∧ b ∣ a n ∧ c ∣ a n ∧ d ∣ a
  → a n ∧ (∀ e : ℕ, e < a n → e ∣ a n → e ≤ b ∨ e = c ∨ e = d) ∧ a (n + 1) =
  → b + c + d)
(n k : ℕ) (hk_coprime_2 : Nat.Coprime k 2) (h : a n = 30 * k) :
Odd (a (n + 1)) := by
rcases h1 n with b, c, d, h_b_lt_c, h_c_lt_d, h_d_lt_an, h_b_dvd_an,
  → h_c_div_an, h_d_div_an, h_all, h_a_plus_1
simp [h] at h_b_dvd_an h_c_div_an h_d_div_an
have h_k_odd : k % 2 = 1 := by
  have h1 : Nat.Coprime k 2 := hk_coprime_2
  have h2 : k % 2 = 0 ∨ k % 2 = 1 := by omega
  rcases h2 with (h2 | h2)
  · have h3 : 2 ∣ k := by omega
    have h4 : Nat.gcd k 2 = 2 := by
      rw [Nat.gcd_eq_right h3]
    have h5 : Nat.gcd k 2 = 1 := by simpa [Nat.coprime_iff_gcd_eq_one] using
      → h1
      omega
    exact h2
  · have h5k_div_an : 15 * k ∣ a n := by

```

```

have h_m_in_4_5 : m = 4 ∨ m = 5 := by omega
rcases h_m_in_4_5 with (h_m_eq_4 | h_m_eq_5)

have h_m_eq_4' : m = 4 := h_m_eq_4
have h_4b_eq_30k : 4 * b = 30 * k := by
  rw [h_m_eq_4'] at hm
  <|> linarith
have h_2b_eq_15k : 2 * b = 15 * k := by linarith
have h1 : (2 * b) % 2 = 0 := by simp [Nat.mul_mod]
have h2 : (15 * k) % 2 = 1 := by
  have h_k_odd' : k % 2 = 1 := h_k_odd
  omega
omega

have h_m_eq_5' : m = 5 := h_m_eq_5
have h_5b_eq_30k : 5 * b = 30 * k := by
  rw [h_m_eq_5'] at hm
  <|> linarith
have h_b_eq_6k : b = 6 * k := by
  nlinarith
exact h_b_eq_6k
have h_a_n_plus_1 : a (n + 1) = 31 * k := by
  have h1 : a (n + 1) = b + c + d := h_a_n_plus_1
  rw [h1, h_b_eq_6k, h_c_eq_10k, h_d_eq_15k]
  <|> ring
use 31 * k / 2
omega

theorem if_a_n_is_30k_then_a_n_plus_1_is_odd (a : ℕ → ℕ) (hpos : ∀ n : ℕ, a n
  → 0)
(h1 : ∀ n : ℕ, ∃ b c d : ℕ, b < c < a < d < a ∧ b | a ∧ c | a ∧ d | a
  → n ∧ (∀ e : ℕ, e < a ∧ n - e | a → e ≤ b ∨ e = c ∨ e = d) ∧ a (n + 1) =
  → b + c + d) (n k : ℕ) (hk_coprime_2 : Nat.Coprime k 2) :
a n = 30 * k → Odd (a (n + 1)) := by
  apply if_a_n_is_30k_then_a_n_plus_1_is_odd_main_proof
  <|> assumption

theorem round1_h_main_5 (a : ℕ → ℕ)
(hpos : ∀ n : ℕ, a n > 0)
(h1 : ∀ n : ℕ, ∃ b c d : ℕ, b < c < a < d < a ∧ b | a ∧ c | a ∧ d | a
  → n ∧ (∀ e : ℕ, e < a ∧ n - e | a → e ≤ b ∨ e = c ∨ e = d) ∧ a (n + 1) =
  → b + c + d) :
  (n : ℕ) → ¬ (5 | a n) := by
intro n h_5_div_a_n
obtain k, h_not_12_div, h_5_div :=
  → exists_first_k_not_divisible_by_12_and_divisible_by_5 (fun i => a (n +
  → i)) (fun i => hpos (n + i)) (fun i => h1 (n + i)) h_5_div_a_n
set m := n + k
have h_5_div_m : 5 | a m := by simp_all
have h_not_12_div_m : ¬ (12 | a m) := by simp_all
have h_2_div_m : 2 | a m := by
  apply round1_h_2_divides_a_n <|> assumption
have h_3_div_m : 3 | a m := by
  apply round1_h_3_divides_a_n <|> assumption
have h_30_div_m : 30 | a m := by
  omega
obtain (t, ht) := h_30_div_m
have h_t_pos : t > 0 := by
  omega
by_cases h2_div_t : 2 | t
  · have h12_div_m : 12 | a m := by
      obtain (s, hs) := h2_div_t
      use 5 * s
      linarith
      contradiction
  · have h_coprime_t_2 : Nat.Coprime t 2 := by
      apply Nat.coprime_iff_gcd_eq_one.mpr
      by_contra h2
      have h3 : t.gcd 2 = 2 := by
        have h4 : t.gcd 2 | 2 := Nat.gcd_dvd_right t 2
        have h5 : t.gcd 2 > 0 := Nat.gcd_pos_of_pos_right t (by norm_num)
        have h6 : t.gcd 2 ≤ 2 := Nat.le_of_dvd (by norm_num) h4
        interval_cases t.gcd 2 <|> tauto
      have h8 : 2 | t := by
        have h9 : t.gcd 2 | t := Nat.gcd_dvd_left t 2
        rw [h3] at h9
        tauto
      have h_odd_a_m_plus_1 : Odd (a (m + 1)) := by
        exact if_a_n_is_30k_then_a_n_plus_1_is_odd a hpos h1 m t h_coprime_t_2
        (by linarith)
      have h_2_div_a_m_plus_1 : 2 | a (m + 1) := by
        apply round1_h_2_divides_a_n <|> assumption
      simp [Nat.odd_iff_not_even, Nat.even_iff] at *
      omega

theorem round1_h_final (a : ℕ → ℕ)
(h_main : ∀ (n : ℕ), ¬ (5 | a n)) :
¬ (5 | a 5) := by
  simp_all

theorem an_cannot_be_divisible_by_5 (a : ℕ → ℕ) (hpos : ∀ n : ℕ, a n > 0) (h1
  → : ∀ n : ℕ, ∃ b c d : ℕ, b < c < a < d < a ∧ b | a ∧ c | a ∧ d | a
  → n ∧ (∀ e : ℕ, e < a ∧ n - e | a → e ≤ b ∨ e = c ∨ e = d) ∧ a (n + 1) =
  → b + c + d) : ¬ (5 | a 0) := by
  simp_all [round1_h_main_5]

theorem round1_h_padicValNat_3_a0_ge_1' (a : ℕ → ℕ) (hpos : ∀ n : ℕ, a n > 0)
(h1 : ∀ n : ℕ, ∃ b c d : ℕ, b < c < a < d < a ∧ b | a ∧ c | a ∧ d | a
  → n ∧ (∀ e : ℕ, e < a ∧ n - e | a → e ≤ b ∨ e = c ∨ e = d) ∧ a (n + 1) =
  → b + c + d) :
  padicValNat 3 (a 0) ≥ 1 := by
  simp_all [round1_h_main, round1_h_3_divides_a_n]

theorem round1_h_6_div_a0 (a : ℕ → ℕ)
(hpos : ∀ n : ℕ, a n > 0)
(h1 : ∀ n : ℕ, ∃ b c d : ℕ, b < c < a < d < a ∧ b | a ∧ c | a ∧ d | a
  → n ∧ (∀ e : ℕ, e < a ∧ n - e | a → e ≤ b ∨ e = c ∨ e = d) ∧ a (n + 1) =
  → b + c + d) :
  6 | a 0 := by
  have := round1_step1 a hpos h1
  omega

theorem round1_exists_m (a : ℕ → ℕ) (hpos : ∀ n : ℕ, a n > 0)
(h1 : ∀ n : ℕ, ∃ b c d : ℕ, b < c < a < d < a ∧ b | a ∧ c | a ∧ d | a
  → n ∧ (∀ e : ℕ, e < a ∧ n - e | a → e ≤ b ∨ e = c ∨ e = d) ∧ a (n + 1) =
  → b + c + d) :
  ∃ m : ℕ, a 0 = 6 * m ∧ ¬ (5 | m) := by
cases' exists_first_term_divisible_by_3 a hpos h1 with j hj
have h6_div_a0 := prop_a0_divisible_by_3 a hpos h1 (j, hj.1)
have h2_div_a0 := even_iff_two_dvd.mp (a0_is_even a hpos h1 hpos h1)
have h6_div_a0 : 6 | a 0 := by
  omega
obtain (m, hm) := h6_div_a0
use m
constructor
exact hm
by_contra h5_div_m
have h5_div_a0 : 5 | a 0 := by
  rw [hm]
  exact dvd_mul_of_dvd_right h5_div_m 6
exact an_cannot_be_divisible_by_5 a hpos h1 (0, h5_div_a0)

theorem round1_h_not_5_div_a0 (a : ℕ → ℕ)
(hpos : ∀ n : ℕ, a n > 0)
(h1 : ∀ n : ℕ, ∃ b c d : ℕ, b < c < a < d < a ∧ b | a ∧ c | a ∧ d | a
  → n ∧ (∀ e : ℕ, e < a ∧ n - e | a → e ≤ b ∨ e = c ∨ e = d) ∧ a (n + 1) =
  → b + c + d) :
  ¬ (5 | a 0) := by
  have := round1_exists_m a hpos h1
  omega

theorem round1_h_padicValNat_2_a0_eq_1 (a : ℕ → ℕ)
(hpos : ∀ n : ℕ, a n > 0)
(h1 : ∀ n : ℕ, ∃ b c d : ℕ, b < c < a < d < a ∧ b | a ∧ c | a ∧ d | a
  → n ∧ (∀ e : ℕ, e < a ∧ n - e | a → e ≤ b ∨ e = c ∨ e = d) ∧ a (n + 1) =
  → b + c + d)
(h_not_4_div_a0 : ¬ (4 | a 0))
(h_6_div_a0 : 6 | a 0)
(h_not_5_div_a0 : ¬ (5 | a 0)) :
  padicValNat 2 (a 0) = 1 := by
  apply v2_of_6_not_4_not_5
  all_goals tauto

theorem round1_h_padicValNat_2_a0_eq_1 (a : ℕ → ℕ) (hpos : ∀ n : ℕ, a n > 0)
(h1 : ∀ n : ℕ, ∃ b c d : ℕ, b < c < a < d < a ∧ b | a ∧ c | a ∧ d | a
  → n ∧ (∀ e : ℕ, e < a ∧ n - e | a → e ≤ b ∨ e = c ∨ e = d) ∧ a (n + 1) =
  → b + c + d)
(h_not_4_div_a0 : ¬ (4 | a 0)) :
  padicValNat 2 (a 0) = 1 := by
  apply round1_h_padicValNat_2_a0_eq_1 a hpos h1 h_not_4_div_a0
  apply round1_h_6_div_a0 a hpos h1
  apply round1_h_not_5_div_a0 a hpos h1

theorem round1_h_main' (a : ℕ → ℕ)
(hpos : ∀ n : ℕ, a n > 0)
(h1 : ∀ n : ℕ, ∃ b c d : ℕ, b < c < a < d < a ∧ b | a ∧ c | a ∧ d | a
  → n ∧ (∀ e : ℕ, e < a ∧ n - e | a → e ≤ b ∨ e = c ∨ e = d) ∧ a (n + 1) =
  → b + c + d)
(h_exists_k : ∃ k, ¬ (12 | a k)) :
  ∃ k, ¬ (12 | a k) ∧ ∀ i < k, 12 | a i := by
  use Nat.find h_exists_k
  simp_all [Nat.find_spec h_exists_k]

theorem round1_h_padicValNat_5_a0_eq_0 (a : ℕ → ℕ) (hpos : ∀ n : ℕ, a n > 0)
(h1 : ∀ n : ℕ, ∃ b c d : ℕ, b < c < a < d < a ∧ b | a ∧ c | a ∧ d | a
  → n ∧ (∀ e : ℕ, e < a ∧ n - e | a → e ≤ b ∨ e = c ∨ e = d) ∧ a (n + 1) =
  → b + c + d) :
  padicValNat 5 (a 0) = 0 := by
  have := an_cannot_be_divisible_by_5 a hpos h1
  simp_all

theorem round1_h_goal (a : ℕ → ℕ)
(hpos : ∀ n : ℕ, a n > 0)
(h1 : ∀ n : ℕ, ∃ b c d : ℕ, b < c < a < d < a ∧ b | a ∧ c | a ∧ d | a
  → n ∧ (∀ e : ℕ, e < a ∧ n - e | a → e ≤ b ∨ e = c ∨ e = d) ∧ a (n + 1) =
  → b + c + d)
(k : ℕ)
(h_k_not_12_div : ¬ (12 | a k))
(h_k_prop : ∀ i < k, 12 | a i) :
  Odd (padicValNat 2 (a 0)) ∧ padicValNat 2 (a 0) < 2 * padicValNat 3 (a 0) ∧
  → padicValNat 5 (a 0) = 0 := by
  have h2_div_ak := round1_h_2_divides_a_n a hpos h1 k
  have h3_div_ak := round1_h_3_divides_a_n a hpos h1 k
  have h6_div_ak : 6 | a k := by omega
  have h_not_4_div_ak : ¬ (4 | a k) := by omega
  have h_not_5_div_ak : ¬ (5 | a k) := by
    have h : ¬ (5 | a n) := an_cannot_be_divisible_by_5 a hpos h1
    intro h1
    exact h k, h1
  have h_v2_ak := padicValNat 2 (a k) = 1 := v2_of_6_not_4_not_5 a hpos h1 (a
    → k) h6_div_ak, h_not_4_div_ak, h_not_5_div_ak
  have h_eq1 := padicValNat 2 (a k) = padicValNat 2 (a 0) - 2 * k := by
    exact (a_k_becomes_6m_form_after_k_steps_of_reduction a hpos h1 k
    → h_k.prop).1
  have h_eq2 := padicValNat 3 (a k) = padicValNat 3 (a 0) - k := by
    exact (a_k_becomes_6m_form_after_k_steps_of_reduction a hpos h1 k
    → h_k.prop).2
  have h_padicValNat_2_a0 := padicValNat 2 (a 0) = 2 * k + 1 := by omega
  have h_odd := Odd (padicValNat 2 (a 0)) := (k, by omega)
  have h_padicValNat_3_a0_ge_k_plus_1 := padicValNat 3 (a 0) ≥ k + 1 := by
    have h10 := padicValNat 3 (a k) = padicValNat 3 (a 0) - k := by omega
    have h11 := padicValNat 3 (a k) ≥ 1 := by
      exact one_le_padicValNat_of_dvd (hpos k) (round1_h_3_divides_a_n a hpos
        → h1 k)
    omega
  have h_ineq := padicValNat 2 (a 0) < 2 * padicValNat 3 (a 0) := by omega
  exact (h_odd, h_ineq, round1_h_padicValNat_5_a0_eq_0 a hpos h1)

theorem imo2025_p4_left (a : ℕ → ℕ) (hpos : ∀ n : ℕ, a n > 0)
(h1 : ∀ n : ℕ, ∃ b c d : ℕ, b < c < a < d < a ∧ b | a ∧ c | a ∧ d | a
  → n ∧ (∀ e : ℕ, e < a ∧ n - e | a → e ≤ b ∨ e = c ∨ e = d) ∧ a (n + 1) =
  → b + c + d) : Odd (padicValNat 2 (a 0)) ∧ padicValNat 2 (a 0) < 2 *
  → padicValNat 3 (a 0) ∧ padicValNat 5 (a 0) = 0 := by
  have h_some_k := round1_h_main' a hpos h1 (round1_h_exists_k a hpos h1)
  exact round1_h_goal a hpos h1 h_some_k.choose h_some_k.choose_spec.1
  → h_some_k.choose_spec.2

theorem imo2025_p4_right8_h1 (a0 k n : ℕ)
(hn : Nat.Coprime n 10)
(ha0 : a0 = 6 * 12 ^ k * n) :
n ≥ 1 := by

```

```

by_contra
simp.all

theorem imo2025_p4_right8_h2 (a0 k n : ℕ)
(hn : Nat.Coprime n 10)
(ha0 : a0 = 6 * 12 ^ k * n)
(h1 : n ≥ 1) :
  ∀ m : ℕ, (if m ≤ k then 6 * 12 ^ (k - m) * 13 ^ m * n else 6 * 13 ^ k * n) >
  → 0 := by
aesop

theorem imo2025_p4_right8_h3 (a0 k n : ℕ)
(hn : Nat.Coprime n 10)
(ha0 : a0 = 6 * 12 ^ k * n)
(h1 : n ≥ 1)
(h2 : ∀ m : ℕ, (if m ≤ k then 6 * 12 ^ (k - m) * 13 ^ m * n else 6 * 13 ^ k * n) > 0) :
  ∀ m : ℕ, (if m ≤ k then 6 * 12 ^ (k - m) * 13 ^ m * n else 6 * 13 ^ k * n) >
  → 3 := by
  intro m
  split_ifs
  all_goals
  calc
  _ ≥ 6 * 1 * 1 * n := by
  gcongr
  <|> apply Nat.one_le_pow
  <|> norm_num
  _ > 3 := by nlinarith

theorem imo2025_p4_right1_main (a0 k n : ℕ)
(hn : Nat.Coprime n 10)
(ha0 : a0 = 6 * 12 ^ k * n)
(h1 : n ≥ 1)
(h2 : ∀ m : ℕ, (if m ≤ k then 6 * 12 ^ (k - m) * 13 ^ m * n else 6 * 13 ^ k * n) > 0)
(h3 : ∀ m : ℕ, (if m ≤ k then 6 * 12 ^ (k - m) * 13 ^ m * n else 6 * 13 ^ k * n) > 3) :
  ∀ m : ℕ, ∃ b c d : ℕ, b < c < d < d < (if m ≤ k then 6 * 12 ^ (k - m) * 13 ^ m * n else 6 * 13 ^ k * n) ∧
  b | (if m ≤ k then 6 * 12 ^ (k - m) * 13 ^ m * n else 6 * 13 ^ k * n) ∧
  c | (if m ≤ k then 6 * 12 ^ (k - m) * 13 ^ m * n else 6 * 13 ^ k * n) ∧
  d | (if m ≤ k then 6 * 12 ^ (k - m) * 13 ^ m * n else 6 * 13 ^ k * n) ∧
  (∀ e : ℕ, e < (if m ≤ k then 6 * 12 ^ (k - m) * 13 ^ m * n else 6 * 13 ^ k * n) →
  → n) →
  e | (if m ≤ k then 6 * 12 ^ (k - m) * 13 ^ m * n else 6 * 13 ^ k * n) →
  e ≤ b ∨ e = c ∨ e = d) ∧
  (if (m + 1) ≤ k then 6 * 12 ^ (k - (m + 1)) * 13 ^ (m + 1) * n else 6 * 13 ^ k * n) =
  → ^ k * n) =
  b + c + d := by
  intro m
  set X := (if m ≤ k then 6 * 12 ^ (k - m) * 13 ^ m * n else 6 * 13 ^ k * n)
  → with hX
  set X' := (if (m + 1) ≤ k then 6 * 12 ^ (k - (m + 1)) * 13 ^ (m + 1) * n
  → else 6 * 13 ^ k * n) with hX'
  have h31 : X > 3 := h3 m
  by_cases h4 : m ≥ k
  ·
  have h41 : X > 0 := by
  have h411 : = h2 m
  simp [hX] using h411
  have h5 : X' = X := by
  by_cases h6 : m = k
  ·
  subst h6
  simp [hX, hX']
  ·
  have h7 : m > k := by omega
  have h8 : -(m + 1 ≤ k) := by omega
  have h9 : -(m ≤ k) := by omega
  simp [hX, hX', h8, h9]
  have h10 : 6 | X := by
  rw [hX]
  by_cases h101 : m ≤ k
  ·
  simp [h101]
  <|> (try { use 12 ^ (k - m) * 13 ^ m * n <|> ring_nf })
  ·
  simp [h101]
  <|> (try { use 13 ^ k * n <|> ring_nf })
  have h102 : ∃ s, X = 6 * s := by
  rcases h10 with (s, hs)
  refine (s, ?_)
  <|> linarith
  rcases h102 with (s, hs)
  have h11 : s ≥ 1 := by
  omega
  have h19 : X = 6 * 13 ^ k * n := by
  by_cases h20 : m ≤ k
  ·
  have h21 : m = k := by omega
  subst h21
  simp [hX]
  ·
  simp [hX, h20]
  have h22 : s = 13 ^ k * n := by
  linarith
  have h231 : Nat.Coprime n 10 := hn
  have h232 : -(2 | n) := by
  by_contra h233
  have h235 : 2 | Nat.gcd n 10 := Nat.dvd_gcd h233 (by norm_num)
  have h236 : Nat.gcd n 10 = 1 := by simp [Nat.coprime_iff_gcd_eq_one]
  → using h231
  rw [h236] at h235
  norm_num at h235
  have h241 : -(5 | n) := by
  by_contra h242
  have h243 : 5 | Nat.gcd n 10 := Nat.dvd_gcd h242 (by norm_num)
  have h244 : Nat.gcd n 10 = 1 := by simp [Nat.coprime_iff_gcd_eq_one]
  → using h231
  rw [h244] at h243
  norm_num at h243
  have h25 : -(2 | s) := by
  by_contra h251
  have h2511 : 2 | s := h251
  have h2512 : s = 13 ^ k * n := h22
  rw [h2512] at h2511
  have h252 : 2 | 13 ^ k * n := h2511
  have h253 : 2 | 13 ^ k * 2 | n := (Nat.Prime.dvd_mul (by norm_num)).mp h252
  have h254 : -(2 | 13 ^ k) := by
  intro h2541
  have h2542 : 2 | 13 ^ k := h2541
  have h2543 : 2 | 13 := by
  exact Nat.Prime.dvd_of_dvd_pow (by norm_num) h2542
  norm_num at h2543
  have h255 : 2 | n := by tauto
  contradiction
  have h26 : -(5 | s) := by
  by_contra h261
  have h2611 : 5 | s := h261
  have h2612 : s = 13 ^ k * n := h22
  rw [h2612] at h2611
  have h262 : 5 | 13 ^ k * n := h2611
  have h263 : 5 | 13 ^ k * 5 | n := (Nat.Prime.dvd_mul (by norm_num)).mp h262
  have h264 : -(5 | 13 ^ k) := by
  intro h2641
  have h2642 : 5 | 13 ^ k := h2641
  have h2643 : 5 | 13 := by
  exact Nat.Prime.dvd_of_dvd_pow (by norm_num) h2642
  norm_num at h2643
  have h265 : 5 | n := by tauto
  contradiction
  have h27 : ∀ e : ℕ, e < X → e | X → e ≤ s ∨ e = 2 * s ∨ e = 3 * s := by
  intro e hei he2
  have h2711 : e | 6 * s := by
  have h2711 : X = 6 * s := by linarith
  rw [h2711] at he2
  simp using he2
  have h272 : e < 6 * s := by
  have h2721 : X = 6 * s := by linarith
  linarith
  by_cases h273 : e ≤ s
  ·
  exact Or.inl h273
  ·
  have h274 : e > s := by linarith
  by_cases h275 : e = 2 * s ∨ e = 3 * s
  ·
  exact Or.inr h275
  ·
  have h2751 : e < 2 * s := by tauto
  have h2752 : e < 3 * s := by tauto
  have h276 : ∃ t, 6 * s = e * t := by
  have h2761 : e | 6 * s := h271
  rcases h2761 with (t, ht)
  refine (t, ?_)
  <|> linarith
  rcases h276 with (t, ht)
  have h277 : 0 < e := by
  by_contra h2771
  have h2772 : e = 0 := by linarith
  rw [h2772] at h272
  linarith
  have h278 : 0 < t := by
  by_contra h2781
  have h2782 : t = 0 := by linarith
  rw [h2782] at ht
  nlinarith
  have h279 : t < 6 := by
  nlinarith
  have h2710 : t = 1 ∨ t = 2 ∨ t = 3 ∨ t = 4 ∨ t = 5 := by omega
  rcases h2710 with (h2710 | h2710 | h2710 | h2710 | h2710)
  ·
  have h2711 : t = 1 := h2710
  rw [h2711] at ht
  nlinarith
  ·
  have h2711 : t = 2 := h2710
  rw [h2711] at ht
  have h2712 : s = 3 * s := by nlinarith
  contradiction
  ·
  have h2711 : t = 3 := h2710
  rw [h2711] at ht
  have h2712 : e = 2 * s := by nlinarith
  contradiction
  ·
  have h2711 : t = 4 := h2710
  rw [h2711] at ht
  have h2713 : 3 * s = 2 * e := by nlinarith
  have h2714 : 2 | 3 * s := by
  omega
  have h2715 : 2 | s := by
  have h27151 : 2 | 3 * s := h2714
  have h27152 : 2 | 3 * 2 | s := (Nat.Prime.dvd_mul (by
  → norm_num)).mp h27151
  tauto
  contradiction
  ·
  have h2711 : t = 5 := h2710
  rw [h2711] at ht
  have h2712 : 6 * s = e * 5 := by nlinarith
  have h2713 : 5 | 6 * s := by
  use e
  <|> linarith
  have h2716 : 5 | s := by
  have h27161 : 5 | 6 * s := h2713
  have h27162 : 5 | 6 * 5 | s := (Nat.Prime.dvd_mul (by
  → norm_num)).mp h27161
  tauto
  contradiction
  refine (s, 2 * s, 3 * s, ?_, ?_, ?_, ?_, ?_, ?_, ?_)
  nlinarith
  nlinarith
  nlinarith
  have h2714 : X = 6 * s := by linarith
  rw [h2714]
  use 6
  <|> ring
  have h2714 : X = 6 * s := by linarith
  rw [h2714]
  use 3
  <|> ring

```



```

have h2714 : X = 6 * s := by linarith
rw [h2714]
use 2
<|> ring

intro e he1 he2
have h2714 : X = 6 * s := by linarith
have h2715 := h27 e he1 he2
simp [h2714] at *
<|> tauto

have h2714 : X = 6 * s := by linarith
have h2716 : X' = X := h5
linarith

have h42 : m < k := by omega
have h12 : m ≤ k := by omega
have h13 : m + 1 ≤ k := by omega
have h14 : 12 * (if (m + 1) ≤ k then 6 * 12 ^ (k - (m + 1)) * 13 ^ (m + 1)
  → * n else 6 * 13 ^ k * n) = 13 * (if m ≤ k then 6 * 12 ^ (k - m) * 13
  → * n else 6 * 13 ^ k * n) := by
  have h141 : m + 1 ≤ k := h13
  have h1411 : m ≤ k := h12
  simp [h141, h1411]
  have h142 : k ≥ m + 1 := by omega
  have h1421 : k - m = (k - (m + 1)) + 1 := by omega
  simp [h1421]
<|> ring_nf
have h15 : 12 | (if m ≤ k then 6 * 12 ^ (k - m) * 13 ^ m * n else 6 * 13 ^
  → k * n) := by
  have h151 : m ≤ k := h12
  have h1511 : k ≥ m + 1 := by omega
  have h152 : 12 | 12 ^ (k - m) := by
    have h1521 : k - m ≥ 1 := by omega
    have h : 3 | t, k - m = t + 1 := by
      use (k - m) - 1
      omega
    rcases h with (t, ht)
    simp [ht, pow_succ]
  <|> ring
  have h153 : 12 | 6 * 12 ^ (k - m) * 13 ^ m * n := by
    rcases h152 with (u, hu)
    use 6 * u * 13 ^ m * n
    rw [hu]
  <|> ring
  simp [if_pos h151]
  <|> tauto
have h155 : 3 | t, (if m ≤ k then 6 * 12 ^ (k - m) * 13 ^ m * n else 6 * 13 ^
  → k * n) = 12 * t := by
  obtain (t, ht) := h15
  refine (t, ?_)
  <|> linarith
rcases h155 with (t, ht)
have h16 : t ≥ 1 := by
  have h161 : (if m ≤ k then 6 * 12 ^ (k - m) * 13 ^ m * n else 6 * 13 ^ k
  → * n) > 3 := h3 m
  linarith
have h17 : (if (m + 1) ≤ k then 6 * 12 ^ (k - (m + 1)) * 13 ^ (m + 1) * n
  → else 6 * 13 ^ k * n) = 13 * t := by
  have h141 : 12 * (if (m + 1) ≤ k then 6 * 12 ^ (k - (m + 1)) * 13 ^ (m +
  → 1) * n else 6 * 13 ^ k * n) = 13 * (if m ≤ k then 6 * 12 ^ (k - m) *
  → 13 ^ m * n else 6 * 13 ^ k * n) := by linarith
  have h172 : (if m ≤ k then 6 * 12 ^ (k - m) * 13 ^ m * n else 6 * 13 ^ k
  → * n) = 12 * t := by linarith
  linarith
have h27 : ∀ e : ℕ, e < 12 * t → e | 12 * t → e ≤ 3 * t ∨ e = 4 * t ∨ e = 6
  → * t := by
  intro e he1 he2
  have h271 : 3 | k : ℕ, 12 * t = e * k := by
    obtain (k, hk) := he2
    refine (k, ?_)
  <|> linarith
rcases h271 with (k, hk)
have h2711 : 0 < e := by
  by_contra h27111
  have h27112 : e = 0 := by linarith
  rw [h27112] at hk
  linarith
have h2712 : 0 < k := by
  by_contra h27121
  have h27122 : k = 0 := by linarith
  rw [h27122] at hk
  nlinarith
have h2713 : k ≥ 2 := by
  by_contra h27131
  have h27132 : k ≤ 1 := by linarith
  by_contra h27133
  have h27134 : k = 1 := by omega
  rw [h27134] at hk
  nlinarith
by_cases h2714 : e ≤ 3 * t
left
exact h2714

have h27141 : e > 3 * t := by linarith
have h2715 : k < 4 := by
  by_contra h27151
  have h27152 : k ≥ 4 := by linarith
  nlinarith
have h2716 : k = 2 ∨ k = 3 := by omega
rcases h2716 with (h27161 | h27162)

have h271611 : k = 2 := h27161
have h271612 : 12 * t = e * 2 := by
  rw [h271611] at hk
  <|> linarith
have h271613 : e = 6 * t := by linarith
right
right
linarith

have h271621 : k = 3 := h27162
have h271622 : 12 * t = e * 3 := by
  rw [h271621] at hk
  <|> linarith
have h271623 : e = 4 * t := by linarith

```

```

right
left
linarith
have hX_eq_simplified : 6 * 12 ^ (k - m) * 13 ^ m * n = 12 * t := by
  have h151 : m ≤ k := h12
  have h1511 : (if m ≤ k then 6 * 12 ^ (k - m) * 13 ^ m * n else 6 * 13 ^
  → k * n) = 6 * 12 ^ (k - m) * 13 ^ m * n := by
    simp [h151]
  have h1512 : (if m ≤ k then 6 * 12 ^ (k - m) * 13 ^ m * n else 6 * 13 ^
  → k * n) = 12 * t := ht
  linarith
have hX_eq_simplified : 6 * 12 ^ (k - (m + 1)) * 13 ^ (m + 1) * n = 13 *
  → t := by
  have h131 : m + 1 ≤ k := h13
  have h132 : (if (m + 1) ≤ k then 6 * 12 ^ (k - (m + 1)) * 13 ^ (m + 1) *
  → n else 6 * 13 ^ k * n) = 6 * 12 ^ (k - (m + 1)) * 13 ^ (m + 1) * n :=
  → by
    simp [h131]
  have h133 : (if (m + 1) ≤ k then 6 * 12 ^ (k - (m + 1)) * 13 ^ (m + 1) *
  → n else 6 * 13 ^ k * n) = 13 * t := h17
  linarith
have h1 : 3 * t | (if m ≤ k then 6 * 12 ^ (k - m) * 13 ^ m * n else 6 * 13
  → * k * n) := by
  have h121 : m ≤ k := h12
  have h122 : (if m ≤ k then 6 * 12 ^ (k - m) * 13 ^ m * n else 6 * 13 ^ k
  → * n) = 6 * 12 ^ (k - m) * 13 ^ m * n := by
    simp [h121]
  have h123 : 6 * 12 ^ (k - m) * 13 ^ m * n = 12 * t := hX_eq_simplified
  have h124 : (if m ≤ k then 6 * 12 ^ (k - m) * 13 ^ m * n else 6 * 13 ^ k
  → * n) = 12 * t := by linarith
  have h125 : 3 * t | 12 * t := by
    use 4
    <|> ring
    rw [h124]
    exact h125
  have h2 : 4 * t | (if m ≤ k then 6 * 12 ^ (k - m) * 13 ^ m * n else 6 * 13
  → * k * n) := by
    have h121 : m ≤ k := h12
    have h122 : (if m ≤ k then 6 * 12 ^ (k - m) * 13 ^ m * n else 6 * 13 ^ k
    → * n) = 6 * 12 ^ (k - m) * 13 ^ m * n := by
      simp [h121]
    have h123 : 6 * 12 ^ (k - m) * 13 ^ m * n = 12 * t := hX_eq_simplified
    have h124 : (if m ≤ k then 6 * 12 ^ (k - m) * 13 ^ m * n else 6 * 13 ^ k
    → * n) = 12 * t := by linarith
    have h125 : 4 * t | 12 * t := by
      use 3
      <|> ring
      rw [h124]
      exact h125
  have h3 : 6 * t | (if m ≤ k then 6 * 12 ^ (k - m) * 13 ^ m * n else 6 * 13
  → * k * n) := by
    have h121 : m ≤ k := h12
    have h122 : (if m ≤ k then 6 * 12 ^ (k - m) * 13 ^ m * n else 6 * 13 ^ k
    → * n) = 6 * 12 ^ (k - m) * 13 ^ m * n := by
      simp [h121]
    have h123 : 6 * 12 ^ (k - m) * 13 ^ m * n = 12 * t := hX_eq_simplified
    have h124 : (if m ≤ k then 6 * 12 ^ (k - m) * 13 ^ m * n else 6 * 13 ^ k
    → * n) = 12 * t := by linarith
    have h125 : 6 * t | 12 * t := by
      use 2
      <|> ring
      rw [h124]
      exact h125
  refine (3 * t, 4 * t, 6 * t, ?_, ?_, ?_, ?_, ?_, ?_, ?_)
  nlinarith
nlinarith
linarith
exact h1
exact h2
exact h3

intro e he1 he2
have h2717 : (if m ≤ k then 6 * 12 ^ (k - m) * 13 ^ m * n else 6 * 13 ^
  → k * n) = 6 * 12 ^ (k - m) * 13 ^ m * n := by simp [h12]
have h2718 : 6 * 12 ^ (k - m) * 13 ^ m * n = 12 * t := hX_eq_simplified
have h2719 : (if m ≤ k then 6 * 12 ^ (k - m) * 13 ^ m * n else 6 * 13 ^
  → k * n) = 12 * t := by linarith
aesop

have h27171 : (if (m + 1) ≤ k then 6 * 12 ^ (k - (m + 1)) * 13 ^ (m + 1)
  → * n else 6 * 13 ^ k * n) = 6 * 12 ^ (k - (m + 1)) * 13 ^ (m + 1) * n
  → := by
  simp [h13]
have h27172 : 6 * 12 ^ (k - (m + 1)) * 13 ^ (m + 1) * n = 13 * t :=
  → hX_eq_simplified
have h27173 : (if (m + 1) ≤ k then 6 * 12 ^ (k - (m + 1)) * 13 ^ (m + 1)
  → * n else 6 * 13 ^ k * n) = 13 * t := by linarith
linarith

theorem imo2025_p4_right (a0 k n : ℕ)
(hn : Nat.Coprime n 10)
(ha0 : a0 = 6 * 12 ^ k * n) :
3 * a : ℕ = N, (∀ n : ℕ, a n > 0) ∧ (∀ n : ℕ, 3 * b * c * d : ℕ, b < c ∧ c < d ∧ d <
  → a * n * b | a * n * c | a * n * d | a * n ∧ (∀ e : ℕ, e < a * n - e | a * n → e ≤ b ∨
  → e = c ∨ e = d) ∧ (a * n + 1) = b + c + d) ∧ (a0 = a0)
/- A \emph{(proper divisor) of a positive integer $$$ is a positive divisor
  → of $$$ other than $$$ itself. The infinite sequence $$$_1, $$$_2,
  → \ldots$ consists of positive integers, each of which has at least
  → three proper divisors. For each $$$ \geqslant 1$, the integer $$$
  → a_{n+1}$ is the sum of the three **largest** proper divisors
  → of $$$_n$.
  When $$$_1$ is $$$ 6 * 12^k * m$, where m is coprime to 10. Please prove that
  → a_n exists. -/

:= by
have h1 := imo2025_p4_right1_main a0 k n hn ha0
have h2 := imo2025_p4_right8_h1 a0 k n hn ha0
have h3 := imo2025_p4_right8_h2 a0 k n hn ha0 h2
have h4 := imo2025_p4_right8_h3 a0 k n hn ha0 h2 h3
use fun m => if m ≤ k then 6 * 12 ^ (k - m) * 13 ^ m * n else 6 * 13 ^ k * n
aesop

```

```

# print axioms prop_a0_divisible_by_3
# print axioms round1_h3_divides_a_n
# print axioms val_5_of_a_succ_if_div_12
# print axioms if_a_n_is_30k_then_a_n_plus_1_is_odd
# print axioms an_cannot_be_divisible_by_5
# print axioms imo2025_p4_left
# print axioms imo2025_p4_right

-- P5
import Mathlib
import Aesop
set_option maxHeartbeats 0
set_option maxRecDepth 1000
set_option tactic.hygienic false
open BigOperators Real Nat Topology Rat

theorem round8_LoseA_iff (l : ℝ) (WinA : ℕ → ℝ → ℝ → Prop)
  (winA_iff : ∀ (n : ℕ) (sum1 sum2 : ℝ), WinA n sum1 sum2 ↔
    (∃ a : ℝ, a ≥ 0 ∧ sum1 + a ≤ (2 * n + 1) * 1 ∧
     ∃ b : ℝ, b ≥ 0 → sum2 + a ^ 2 + b ^ 2 ≤ 2 * n + 2 →
      WinA (n + 1) (sum1 + a + b) (sum2 + a ^ 2 + b ^ 2)))
  (n : ℕ) (sum1 sum2 : ℝ) :
  ~ WinA n sum1 sum2 ↔ (∃ (a : ℝ), a ≥ 0 → sum1 + a > (2 * n + 1) * 1 ∨ (∃ (b
    → : ℝ), b ≥ 0 ∧ sum2 + a ^ 2 + b ^ 2 ≤ 2 * n + 2 ∧ ~ WinA (n + 1) (sum1
    → + a + b) (sum2 + a ^ 2 + b ^ 2))) := by
  rw [winA_iff]
  simp [imp_iff_not_or]

theorem round1_main (l : ℝ)
  (hl : l > Real.sqrt 2 / 2) :
  (N : ℕ), ((2 * (N : ℝ) + 1) * 1 - Real.sqrt 2 * (N : ℝ)) ^ 2 > 2 * (N : ℝ) +
    → 2 := by
  obtain N, hN := exists_nat_gt (4 / ((2 * 1 - Real.sqrt 2) ^ 2) + 2)
  use N
  have h1 : 0 < Real.sqrt 2 := Real.sqrt_pos.mpr (by norm_num)
  have h2 : 0 < 1 := by linarith [Real.sqrt_nonneg 2]
  have h3 : 0 < 2 * 1 - Real.sqrt 2 := by linarith
  have h4 : 0 < (2 * 1 - Real.sqrt 2) ^ 2 := by positivity
  have h5 : 0 < 4 / ((2 * 1 - Real.sqrt 2) ^ 2) := by positivity
  have h6 : (N : ℝ) > 4 / ((2 * 1 - Real.sqrt 2) ^ 2) + 2 := by exact_mod_cast
    → hN
  have h7 : (2 * 1 - Real.sqrt 2) ^ 2 * (N : ℝ) > 4 := by
    calc
    (2 * 1 - Real.sqrt 2) ^ 2 * (N : ℝ) > (2 * 1 - Real.sqrt 2) ^ 2 * (4 /
      → ((2 * 1 - Real.sqrt 2) ^ 2)) := by nlinarith
    _ = 4 := by field_simp [h4.ne']
  have h8 : 4 * (N : ℝ) > 2 * (N : ℝ) + 2 := by linarith
  have h9 : (2 * 1 - Real.sqrt 2) ^ 2 * (N : ℝ) ^ 2 > 2 * (N : ℝ) + 2 := by
    → nlinarith
  ring_nf
  nlinarith

theorem round1_final (l : ℝ)
  (hl : l > Real.sqrt 2 / 2)
  (N : ℕ)
  (h20 : ((2 * (N : ℝ) + 1) * 1 - Real.sqrt 2 * (N : ℝ)) ^ 2 > 2 * (N : ℝ) +
    → 2) :
  (s1 s2 : ℝ), 0 ≤ s1 → s1 ≤ Real.sqrt 2 * (N : ℝ) → 0 ≤ s2 → s2 ≤ 2 * (N : ℝ)
    → s2 + ((2 * (N : ℝ) + 1) * 1 - s1) ^ 2 > 2 * (N : ℝ) + 2 := by
  intros
  nlinarith [show (2 * (N : ℝ) + 1) * 1 - Real.sqrt 2 * (N : ℝ) > 0 by
    nlinarith [Real.sqrt_nonneg 2, Real.sqrt_sqrt (show 0 ≤ 2 by norm_num)]]

theorem round8_quadratic_growth_contradiction (l : ℝ) (hl : l > Real.sqrt 2 /
  → 2) :
  (N : ℕ), (∃ (s1 s2 : ℝ), 0 ≤ s1 → s1 ≤ Real.sqrt 2 * (N : ℝ) → 0 ≤ s2 →
    → s2 ≤ 2 * (N : ℝ) → s2 + ((2 * (N : ℝ) + 1) * 1 - s1) ^ 2 > 2 * (N : ℝ)
    → 2) + 2 := by
  apply (round1_main 1 hl).imp
  exact round1_final 1 hl

theorem round15_lemma1 (l : ℝ) (hl0 : l > 0) (WinA : ℕ → ℝ → ℝ → Prop)
  (winA_iff : ∀ (n : ℕ) (sum1 sum2 : ℝ), WinA n sum1 sum2 ↔
    (∃ a : ℝ, a ≥ 0 ∧ sum1 + a ≤ (2 * n + 1) * 1 ∧
     ∃ b : ℝ, b ≥ 0 → sum2 + a ^ 2 + b ^ 2 ≤ 2 * n + 2 →
      WinA (n + 1) (sum1 + a + b) (sum2 + a ^ 2 + b ^ 2)))
  (hl : l > √2 / 2) :
  (k : ℕ) (s1 s2 : ℝ),
  (~ WinA k s1 s2) →
  (0 ≤ s1) →
  (0 ≤ s2) →
  (s1 ^ 2 ≤ (k : ℝ) * s2) →
  (s2 ≤ 2 * (k : ℝ)) →
  (∃ (b_next : ℝ),
    b_next ≥ 0 ∧
    (~ WinA (k + 1) (s1 + b_next) (s2 + b_next ^ 2)) ∧
    (s2 + b_next ^ 2 ≤ 2 * ((k : ℝ) + 1))) ∧
    ((s1 + b_next) ^ 2 ≤ ((k : ℝ) + 1) * (s2 + b_next ^ 2)) := by
  intro k s1 s2 h1 h2 h3 h4 h5
  simp [round8_LoseA_iff 1 WinA winA_iff k s1 s2] at h1
  have h6 : s1 ≤ Real.sqrt 2 * k := by
    nlinarith [Real.sqrt_nonneg 2, Real.sqrt_sqrt (show 0 ≤ 2 by norm_num),
      → sq_nonneg (k : ℝ), mul_nonneg (Real.sqrt_nonneg 2) (Nat.cast_nonneg
        → k)]
  have h7 : (2 * k + 1) * 1 ≥ Real.sqrt 2 * k := by
    nlinarith [Real.sqrt_nonneg 2, Real.sqrt_sqrt (show 0 ≤ 2 by norm_num),
      → sq_nonneg (k : ℝ)]
  have h8 : ∃ b, b ≥ 0 ∧ s2 + b ^ 2 ≤ 2 * k + 2 ∧ ~ WinA (k + 1) (s1 + b) (s2 +
    → b ^ 2) := by
  have h61 : s1 > (2 * k + 1) * 1 ∨ ∃ b, b ≥ 0 ∧ s2 + 0 ^ 2 + b ^ 2 ≤ 2 * k +
    → 2 ∧ ~ WinA (k + 1) (s1 + 0 + b) (s2 + 0 ^ 2 + b ^ 2) := by
    simp using h1 0 (by linarith)
  have h62 : ~ (s1 > (2 * k + 1) * 1) := by linarith
  have h63 : ∃ b, b ≥ 0 ∧ s2 + 0 ^ 2 + b ^ 2 ≤ 2 * k + 2 ∧ ~ WinA (k + 1) (s1
    → + 0 + b) (s2 + 0 ^ 2 + b ^ 2) := by
    tauto
  rcases h63 with ⟨b, hb1, hb2, hb3⟩
  linarith
  simp using hb3
  rcases h8 with ⟨b, hb1, hb2, hb3⟩
  have h10 : (k : ℝ) * b ^ 2 - 2 * s1 * b + s2 ≥ 0 := by
    by_cases h121 : (k : ℝ) = 0
    · have h1211 : s1 = 0 := by
        have h1212 : s1 ^ 2 ≤ (k : ℝ) * s2 := h4
        rw [h121] at h1212
        nlinarith
      · have h122 : (k : ℝ) > 0 := by positivity
        nlinarith [sq_nonneg (b * (k : ℝ) - s1), Real.sqrt_sqrt (show 0 ≤ 2 by
          → norm_num),
          Real.sqrt_nonneg 2, sq_nonneg s1, sq_nonneg ((k : ℝ))]
    · have h11 : (s1 + b) ^ 2 ≤ ((k : ℝ) + 1) * (s2 + b ^ 2) := by
        nlinarith
    exact ⟨b, hb1, hb3, by linarith, h11⟩

theorem round15_h_main (l : ℝ) (hl0 : l > 0) (WinA : ℕ → ℝ → ℝ → Prop)
  (winA_iff : ∀ (n : ℕ) (sum1 sum2 : ℝ), WinA n sum1 sum2 ↔
    (∃ a : ℝ, a ≥ 0 ∧ sum1 + a ≤ (2 * n + 1) * 1 ∧
     ∃ b : ℝ, b ≥ 0 → sum2 + a ^ 2 + b ^ 2 ≤ 2 * n + 2 →
      WinA (n + 1) (sum1 + a + b) (sum2 + a ^ 2 + b ^ 2)))
  (hl : l > √2 / 2)
  (h : ~ WinA 0 0 0)
  (lemma1 : ∀ (k : ℕ) (s1 s2 : ℝ),
    (~ WinA k s1 s2) →
    (0 ≤ s1) →
    (0 ≤ s2) →
    (s1 ^ 2 ≤ (k : ℝ) * s2) →
    (s2 ≤ 2 * (k : ℝ)) →
    (∃ (b_next : ℝ),
      b_next ≥ 0 ∧
      (~ WinA (k + 1) (s1 + b_next) (s2 + b_next ^ 2)) ∧
      (s2 + b_next ^ 2 ≤ 2 * ((k : ℝ) + 1))) ∧
      ((s1 + b_next) ^ 2 ≤ ((k : ℝ) + 1) * (s2 + b_next ^ 2))) :
  (k : ℕ), ∃ s1 s2 : ℝ, (0 ≤ s1) ∧ (0 ≤ s2) ∧ (s1 ^ 2 ≤ (k : ℝ) * s2) ∧ (s2 ≤ 2 *
    → (k : ℝ)) ∧ (~ WinA k s1 s2) := by
  intro k
  induction' k with k ih
  use 0,
  simp [h]
  rcases ih with ⟨s1, s2, h1, h2, h3, h4, h5⟩
  rcases lemma1 k s1 s2 h5 h1 h2 h3 h4 with ⟨b_next, h_b_next1, h_b_next2,
    → h_b_next3, h_b_next4⟩
  use s1 + b_next, s2 + b_next ^ 2
  norm_num
  repeat' constructor
  nlinarith
  nlinarith
  nlinarith
  nlinarith
  exact h_b_next2

theorem imo2025_p5_algebra_A (l : ℝ) (hl0 : l > 0) (WinA : ℕ → ℝ → ℝ → Prop)
  (winA_iff : ∀ (n : ℕ) (sum1 sum2 : ℝ), WinA n sum1 sum2 ↔
    (∃ a : ℝ, a ≥ 0 ∧ sum1 + a ≤ (2 * n + 1) * 1 ∧
     ∃ b : ℝ, b ≥ 0 → sum2 + a ^ 2 + b ^ 2 ≤ 2 * n + 2 →
      WinA (n + 1) (sum1 + a + b) (sum2 + a ^ 2 + b ^ 2)))
  (hl : l > √2 / 2) : WinA 0 0 0 := by
  by_contra h
  obtain W, h1 := round8_quadratic_growth_contradiction 1 hl
  obtain ⟨s1, s2, h3, h4, h5, h6, h7 := round15_h_main 1 hl0 WinA winA_iff hl h,
    (round15_lemma1 1 hl0 WinA winA_iff hl) N
  have h8 : s1 ≤ Real.sqrt 2 * (N : ℝ) := by
    nlinarith [Real.sqrt_nonneg 2, Real.sqrt_sqrt (show 0 ≤ 2 by norm_num),
      → sq_nonneg s1,
      sq_nonneg (N : ℝ), mul_nonneg (Real.sqrt_nonneg 2) (Nat.cast_nonneg N)]
  have h9 := h s1 s2 h3 h4 h5 h6
  obtain h11 ⟨b, hb1, hb2 := (round8_LoseA_iff 1 WinA winA_iff N s1 s2).mp
    → h7 ((2 * (N : ℝ) + 1) * 1 - s1) (by nlinarith)
  <|> nlinarith

theorem round3_P_holds_for_large_n (l : ℝ) (hl0 : l > 0) (hl : l < √2 / 2)
  (WinB : ℕ → ℝ → ℝ → Prop)
  (winB_iff : ∀ (n : ℕ) (sum1 sum2 : ℝ), WinB n sum1 sum2 ↔
    (∃ a : ℝ, a ≥ 0 → sum1 + a ≤ (2 * n + 1) * 1 →
     ∃ b : ℝ, b ≥ 0 ∧ sum2 + a ^ 2 + b ^ 2 ≤ 2 * n + 2 ∧
      WinB (n + 1) (sum1 + a + b) (sum2 + a ^ 2 + b ^ 2))) :
  (N : ℕ), ∃ n : ℕ, n ≥ N → (s1 : ℝ) (s2 : ℝ), s1 ≥ (n : ℝ) * Real.sqrt 2 → s1
    → 2 * (n : ℝ) → WinB n s1 s1 := by
  rcases exists_nat_gt (1 / (Real.sqrt 2 - 2 * 1)) with ⟨N, hN⟩
  use N + 1
  intro n hn s1 s2 hs hs
  have hn' : (N + 1 : ℝ) > 1 / (Real.sqrt 2 - 2 * 1) := by linarith
  have hn' : (n : ℝ) ≥ (N + 1 : ℝ) := by exact_mod_cast hn
  have h_ineq1 : (n : ℝ) * (Real.sqrt 2 - 2 * 1) > 1 := by
    have h : (n : ℝ) > 1 / (Real.sqrt 2 - 2 * 1) := by linarith
    have h3 : 0 < Real.sqrt 2 - 2 * 1 := by
      nlinarith [Real.sqrt_pos_of_pos (show 0 < 2 by norm_num)]
    have h4 : (n : ℝ) * (Real.sqrt 2 - 2 * 1) > 1 / (Real.sqrt 2 - 2 * 1) *
      → (Real.sqrt 2 - 2 * 1) := by nlinarith
    have h5 : (1 / (Real.sqrt 2 - 2 * 1)) * (Real.sqrt 2 - 2 * 1) = 1 := by
      field_simp [h3.ne']
    linarith
  apply (winB_iff n s1 s1).mpr
  intro a ha, ha,
  nlinarith

theorem round3_P_inductive_step_backward (l : ℝ) (hl0 : l > 0) (hl : l < √2 /
  → 2)
  (WinB : ℕ → ℝ → ℝ → Prop)
  (winB_iff : ∀ (n : ℕ) (sum1 sum2 : ℝ), WinB n sum1 sum2 ↔
    (∃ a : ℝ, a ≥ 0 → sum1 + a ≤ (2 * n + 1) * 1 →
     ∃ b : ℝ, b ≥ 0 ∧ sum2 + a ^ 2 + b ^ 2 ≤ 2 * n + 2 ∧
      WinB (n + 1) (sum1 + a + b) (sum2 + a ^ 2 + b ^ 2)))
  (k : ℕ)
  (P_holds_for_k_plus_1 : ∀ (s1 : ℝ) (s2 : ℝ), s1 ≥ ((k + 1) : ℕ) *
    → Real.sqrt 2 → s1 = 2 * ((k + 1) : ℕ) * (k : ℝ) → WinB (k + 1) s1 s2) :
  (s1 : ℝ) (s2 : ℝ), s1 ≥ (k : ℝ) * Real.sqrt 2 → s1 = 2 * (k : ℝ) → WinB k s1
    → s1 := by
  intro s1 s2 hs hs
  rw [winB_iff]
  intro a ha_nonneg ha_le
  have h_a_lt_sqrt2_div_2 : a < Real.sqrt 2 / 2 := by nlinarith [ha_le, hl]
  have h2_minus_a_sq_pos : 0 < 2 - a ^ 2 := by nlinarith [h_a_lt_sqrt2_div_2,
    → Real.sqrt_sqrt (show 0 ≤ 2 by norm_num), Real.sqrt_nonneg 2]
  set b := Real.sqrt (2 - a ^ 2) with hb_def
  have hb_nonneg : b ≥ 0 := Real.sqrt_nonneg _
  have h_sum2_cond : s1 + a ^ 2 + b ^ 2 ≤ 2 * k + 2 := by

```



```

have h_b_sq : b ^ 2 = 2 - a ^ 2 := by
  rw [hb_def]
  exact Real.sq_sqrt (by nlinarith)
nlinarith [hs, h_b_sq]
have h_a_plus_b_ge_sqrt2 : a + b ≥ Real.sqrt 2 := by
  have h : (a + b) ^ 2 ≥ (Real.sqrt 2) ^ 2 := by
    have h_sqrt2_sq : (Real.sqrt 2) ^ 2 = 2 := by
      rw [Real.sq_sqrt] <|> norm_num
    have h_b_sq : (Real.sqrt (2 - a ^ 2)) ^ 2 = 2 - a ^ 2 := by
      rw [Real.sq_sqrt] <|> nlinarith [ha_nonneg]
    nlinarith
  have h_a_nonneg : 0 ≤ a := by linarith [ha_nonneg]
  have h_sqrt2_nonneg : 0 ≤ Real.sqrt 2 := Real.sqrt_nonneg 2
  nlinarith
have h_S1_next_ge : s, a + a + b ≥ (k + 1 : ℕ) * Real.sqrt 2 := by
  have h_S1_ge_k_sqrt2 : s, ≥ k * Real.sqrt 2 := by nlinarith
  have h : s, a + a + b ≥ k * Real.sqrt 2 + (a + b) := by linarith
  have h' : k * Real.sqrt 2 + (a + b) ≥ k * Real.sqrt 2 + Real.sqrt 2 := by
    → linarith
  have h'' : k * Real.sqrt 2 + Real.sqrt 2 = (k + 1 : ℕ) * Real.sqrt 2 := by
    simp
  <|> ring
  linarith
have h_S2_next : s, a ^ 2 + b ^ 2 = 2 * ((k + 1 : ℕ) : ℝ) := by
  have h_b_sq : b ^ 2 = 2 - a ^ 2 := by
    rw [hb_def]
    exact Real.sq_sqrt (by nlinarith)
  have h1 : s, a ^ 2 + b ^ 2 = 2 * k + 2 := by nlinarith [hs, h_b_sq]
  have h2 : 2 * ((k + 1 : ℕ) : ℝ) = 2 * k + 2 := by
    simp
  <|> ring
  linarith
exact (b, hb_nonneg, h_sum2_cond, P_holds_for_k_plus_1 (s, a + b) (s, a ^ 2 + b ^ 2) h_S1_next_ge h_S2_next)

theorem imo2025_p5_algebra_B (l : ℝ) (h10 : l > 0) (WinB : ℕ → ℝ → ℝ → Prop)
  (winB_iff : ∀ (n : ℕ) (sum1 sum2 : ℝ), WinB n sum1 sum2 ↔
    ∀ a : ℝ, a ≥ 0 → sum1 + a ≤ (2 * n + 1) * l →
    ∃ b : ℝ, b ≥ 0 ∧ sum2 + a ^ 2 + b ^ 2 ≤ 2 * n + 2 * l ∧
    WinB (n + 1) (sum1 + a + b) (sum2 + a ^ 2 + b ^ 2))
  (h1 : l < √2 / 2) (WinB 0 0 0 := by
  choose N hN using round3_P_holds_for_large_n l h10 h1 WinB winB_iff
  have h_P_N : ∀ j : ℕ, j ≤ N → ∃ (s : ℝ) (s1 : ℝ), s1 ≥ (N - j : ℕ) *
    → Real.sqrt 2 + s, s = 2 * (N - j : ℕ) → WinB (N - j) s, s1 := by
    intro j h1
    induction' j with j' ih
    · intro s, s1, hs, hs
      exact hN N (by linarith) s, s1, hs, hs
    · intro s, s1, hs, hs
      have h_k_plus_1_eq_N_minus_j' : ((N - (j' + 1)) + 1) = N - j' := by omega
      have ih' := ih (by linarith)
      have h_P_k_plus_1 : ∃ (s1 : ℝ) (s2 : ℝ), s2 ≥ (((N - (j' + 1)) + 1) : ℕ) *
        → Real.sqrt 2 + s, s = 2 * (((N - (j' + 1)) + 1) : ℕ) → WinB ((N - (j' + 1)) + 1) s, s1 := by
          intro s, s1, hs, hs
          rw [h_k_plus_1_eq_N_minus_j'] at *
          exact ih' s, s1, hs, hs
      exact round3_P_inductive_step_backward l h10 h1 WinB winB_iff (N - (j' + 1)) h_P_k_plus_1 s, s1, hs, hs
  have h_P_0' : WinB (N - N) 0 0 := h_P_N N (by linarith) 0 0 (by norm_num)
  → (by norm_num)
  rw [Nat.sub_self] at h_P_0'
  exact h_P_0'

theorem imo2025_p5_draw1_main (l : ℝ) (h10 : l > 0) (h1 : l = √2 / 2) :
  ∃ sa : (n : ℕ) → (Fin (n + 1) → ℝ), (∀ i x, sa i x ≥ 0) ∧
  ∀ b : ℕ → ℝ, (∀ i : ℕ, b i ≥ 0) →
  ∀ a : ℕ → ℝ, (∀ i : ℕ, a i = sa i (fun j → b (j : ℕ))) →
  ∀ n : ℕ,
    (∀ k, k < n →
      (∃ i ∈ Finset.range k, (a i + b i)) + a k ≤ (2 * k + 1) * l ∧
      (∃ i ∈ Finset.range k, (a i ^ 2 + b i ^ 2)) + a k ^ 2 + b k ^ 2 ≤ 2 *
        → k + 2) →
      (∃ i ∈ Finset.range n, (a i + b i)) + a n ≤ (2 * n + 1) * l := by
    use fun _ => 0
  constructor
  · intro i x
    by_cases h : x (i, by linarith) ≤ Real.sqrt 2
    · simp [h]
  · simp [h]
  · intro a h a b h1 n h2 h3
    have h100 : ∀ m : ℕ, m ≤ n → ∃ i in Finset.range m, (a i ^ 2 + b i ^ 2) ≤ 2 *
      → (m : ℝ) := by
      intro m hm
      induction' m with m hm
      · norm_num
      · have h4 : m ≤ n := by linarith
        have h5 : m < n := by linarith
        have h6 := h2 m h5
        have h61 := h6.2
        have h7 : ∃ i in Finset.range (m + 1), (a i ^ 2 + b i ^ 2) = (∃ i in
          → Finset.range m, (a i ^ 2 + b i ^ 2)) + (a m ^ 2 + b m ^ 2) := by
          rw [Finset.sum_range_succ]
        have h8 : (∃ i in Finset.range m, (a i ^ 2 + b i ^ 2)) + a m ^ 2 + b m
          → ^ 2 ≤ 2 * (m : ℝ) + 2 := by linarith
        have h9 : (∃ i in Finset.range (m + 1), (a i ^ 2 + b i ^ 2)) ≤ 2 * (m :
          → ℝ) + 2 := by linarith [h7, h8]
        have h10 : (2 * (m : ℝ) + 2 : ℝ) = 2 * ((m + 1 : ℕ) : ℝ) := by
          simp [Nat.cast_add, Nat.cast_one]
        <|> ring
        linarith
      have h4 : ∀ i : ℕ, b i = if a i ≤ Real.sqrt 2 then Real.sqrt 2 - a i else 0
        := by
        intro i
        have h11 := h1 i
        simp using h11
        have h5 : ∀ i : ℕ, b i ≥ 0 := by
          intro i
          have h51 := h4 i
          rw [h51]
          by_cases h52 : a i ≤ Real.sqrt 2
          · rw [if_pos h52]
            linarith [Real.sqrt_nonneg 2]
          · rw [if_neg h52]
        have h6 : ∀ i : ℕ, a i + b i ≥ Real.sqrt 2 := by
          intro i
          have h41 := h4 i
          rw [h41]
          by_cases h61 : a i ≤ Real.sqrt 2
          · rw [if_pos h61]
            linarith
          · rw [if_neg h61]
            have h62 : a i > Real.sqrt 2 := by linarith
            linarith

```

```

have h7 : (x i in Finset.range n, (a i + b i)) ≥ (n : ℝ) * Real.sqrt 2 := by
have h71 : ∀ i ∈ Finset.range n, a i + b i ≥ Real.sqrt 2 := fun i _ => h6
  => i
have h72 : (x i in Finset.range n, (a i + b i)) ≥ x i in Finset.range n,
  => Real.sqrt 2 := by
  apply Finset.sum_le_sum
  intro i _
  exact h71 i _
have h73 : (x i in Finset.range n, Real.sqrt 2) = (n : ℝ) * Real.sqrt 2 :=
  by
  simp [mul_comm]
  linarith
have h8 : (x i in Finset.range n, (a i + b i)) + a n ≤ (2 * n + 1) * 1 :=
  by simp using h3
have h9 : (x i in Finset.range n, (a i + b i)) + a n ≤ (2 * (n : ℝ) + 1) *
  (Real.sqrt 2 / 2) := by
have h91 : 1 = Real.sqrt 2 / 2 := by linarith [h1]
rw [h91] at h8
linarith
have h10 : (n : ℝ) * Real.sqrt 2 + a n ≤ (2 * (n : ℝ) + 1) * (Real.sqrt 2
  / 2) := by linarith [h7, h9]
have h11 : a n ≤ Real.sqrt 2 / 2 := by
  nlinarith [Real.sqrt_nonneg 2, Real.sq_sqrt (show (0 : ℝ) ≤ 2 by
    norm_num)]
have h12 : a n ≤ Real.sqrt 2 := by linarith [Real.sqrt_nonneg 2, h11]
have h13 : b n = Real.sqrt 2 - a n := by
  have h131 := h4 n
  rw [h131]
  rw [if_pos h12]
have h14 : a n ^ 2 + b n ^ 2 ≤ 2 := by
  rw [h13]
  have h141 : 0 ≤ a n := ha n
  have h142 : a n ≤ Real.sqrt 2 / 2 := h11
  nlinarith [Real.sqrt_nonneg 2, Real.sq_sqrt (show (0 : ℝ) ≤ 2 by
    norm_num)]
have h15 : x i in Finset.range n, (a i ^ 2 + b i ^ 2) ≤ 2 * (n : ℝ) := by
  specialize h100 n (by linarith)
  simp using h100
have h_final : (x i in Finset.range n, (a i ^ 2 + b i ^ 2)) + a n ^ 2 + b
  n ^ 2 ≤ 2 * (n : ℝ) + 2 := by linarith
norm_cast at h_final

theorem imo2025_p5_draw_a (l : ℝ) (h10 : l > 0) (h1 : l = √2 / 2) :
  sb : (n : ℕ) → (Fin (n + 1) → ℝ) → ℝ, (∀ i x, sb i x ≥ 0) ∧
  ∀ a : ℕ → ℝ, (∀ i : ℕ, a i ≥ 0) →
  ∀ b : ℕ → ℝ, (∀ i : ℕ, b i = sb i (fun j → a (j : ℕ))) →
  ∀ n : ℕ,
    (∀ k, k < n →
      (x i ∈ Finset.range k, (a i + b i)) + a k ≤ (2 * k + 1) * 1 ∧
      (x i ∈ Finset.range k, (a i ^ 2 + b i ^ 2)) + a k ^ 2 + b k ^ 2 ≤ 2 *
        (k + 2) →
      (x i ∈ Finset.range n, (a i + b i)) + a n ≤ (2 * n + 1) * 1 →
      (x i ∈ Finset.range n, (a i ^ 2 + b i ^ 2)) + a n ^ 2 + b n ^ 2 ≤ 2 * n
        + 2 := by
  apply imo2025_p5_draw_a_v22_main
  <|> assumption

#print axioms imo2025_p5_algebra_A
#print axioms imo2025_p5_algebra_B
#print axioms imo2025_p5_draw1_main
#print axioms imo2025_p5_draw_b
#print axioms imo2025_p5_draw_a_v22_main
#print axioms imo2025_p5_draw_a

```
